# Supplementary material for: Fermi Large Area Telescope Third Source Catalog
Source: arXiv:1501.02003 ancillary file (2015-06-09)
Supplement: Supplementary file 1 [file table4_full.pdf]

Table 1. LAT 4-year Catalog

| Name 3FGL    | R.A.  | Decl.   | $l$     | $b$     | $\theta_1$ | $\theta_2$ | $\phi$ | $\sigma$ | $F_{35}$ | $\Delta F_{35}$ | $S_{25}$ | $\Delta S_{25}$ | $\Gamma_{25}$ | $\Delta \Gamma_{25}$ | Mod | Var | Flags | $\gamma$ -ray Assoc.                                                                                                  | TeV | Class | ID or Assoc.             |
|--------------|-------|---------|---------|---------|------------|------------|--------|----------|----------|-----------------|----------|-----------------|---------------|----------------------|-----|-----|-------|-----------------------------------------------------------------------------------------------------------------------|-----|-------|--------------------------|
| J0000.1+6545 | 0.038 | 65.752  | 117.694 | 3.403   | 0.102      | 0.078      | 41     | 6.8      | 1.0      | 0.2             | 13.6     | 2.1             | 2.41          | 0.08                 | PL  | ... | 3     | 2FGL J2359.6+6543c                                                                                                    | ... | ...   | ...                      |
| J0000.2-3738 | 0.061 | -37.648 | 345.411 | -74.947 | 0.073      | 0.068      | -89    | 5.1      | 0.2      | 0.1             | 2.4      | 0.7             | 1.87          | 0.18                 | PL  | ... | ...   | ...                                                                                                                   | ... | ...   | ...                      |
| J0001.0+6314 | 0.254 | 63.244  | 117.293 | 0.926   | 0.248      | 0.160      | -65    | 6.2      | 0.6      | 0.1             | 13.0     | 1.9             | 2.73          | 0.11                 | PL  | ... | 3,4,5 | 2FGL J2358.9+6325                                                                                                     | ... | spp   | ...                      |
| J0001.2-0748 | 0.321 | -7.816  | 89.022  | -67.324 | 0.082      | 0.070      | -19    | 11.3     | 0.7      | 0.1             | 7.8      | 0.9             | 2.15          | 0.09                 | PL  | ... | ...   | 2FGL J0000.9-0748<br>1FGL J0000.9-0745                                                                                | ... | bll   | PMN J0001-0746           |
| J0001.4+2120 | 0.361 | 21.338  | 107.665 | -40.047 | 0.211      | 0.188      | -33    | 11.4     | 0.3      | 0.1             | 8.1      | 0.8             | 2.78          | ...                  | LP  | T   | ...   | 3EG J2359+2041                                                                                                        | ... | fsrq  | TXS 2358+209             |
| J0001.6+3535 | 0.404 | 35.590  | 111.661 | -26.188 | 0.213      | 0.167      | 8      | 4.2      | 0.3      | 0.1             | 3.4      | 0.8             | 2.35          | 0.19                 | PL  | ... | 4     | ...                                                                                                                   | ... | ...   | ...                      |
| J0002.0-6722 | 0.524 | -67.370 | 310.139 | -49.062 | 0.102      | 0.086      | 69     | 5.9      | 0.3      | 0.1             | 3.3      | 0.8             | 1.95          | 0.16                 | PL  | ... | ...   | ...                                                                                                                   | ... | ...   | ...                      |
| J0002.2-4152 | 0.562 | -41.883 | 334.070 | -72.143 | 0.217      | 0.140      | 68     | 5.2      | 0.3      | 0.1             | 3.0      | 0.7             | 2.09          | 0.19                 | PL  | ... | ...   | 2FGL J0001.7-4159                                                                                                     | ... | bcu   | 1RXS<br>J000135.5-415519 |
| J0002.6+6218 | 0.674 | 62.301  | 117.302 | -0.037  | 0.061      | 0.054      | -55    | 18.0     | 2.8      | 0.2             | 18.4     | 1.7             | 2.35          | ...                  | LP  | ... | ...   | 1FGL J0001.9-4158<br>2FGL J0002.7+6220                                                                                | ... | ...   | ...                      |
| J0003.2-5246 | 0.815 | -52.777 | 318.976 | -62.825 | 0.070      | 0.061      | -44    | 5.7      | 0.3      | 0.1             | 3.0      | 0.8             | 1.90          | 0.17                 | PL  | ... | ...   | ...                                                                                                                   | ... | bcu   | RBS 0006                 |
| J0003.4+3100 | 0.858 | 31.008  | 110.964 | -30.745 | 0.181      | 0.163      | 13     | 6.3      | 0.3      | 0.1             | 4.9      | 0.8             | 2.55          | 0.13                 | PL  | ... | ...   | ...                                                                                                                   | ... | ...   | ...                      |
| J0003.5+5721 | 0.890 | 57.360  | 116.486 | -4.912  | 0.089      | 0.072      | 1      | 5.4      | 0.5      | 0.1             | 5.4      | 1.1             | 2.18          | 0.13                 | PL  | ... | ...   | ...                                                                                                                   | ... | ...   | ...                      |
| J0003.8-1151 | 0.959 | -11.863 | 84.432  | -71.084 | 0.130      | 0.100      | -17    | 4.2      | 0.2      | 0.1             | 2.6      | 0.7             | 2.02          | 0.18                 | PL  | ... | ...   | ...                                                                                                                   | ... | bcu   | PMN J0004-1148           |
| J0004.2+6757 | 1.055 | 67.959  | 118.509 | 5.494   | 0.101      | 0.090      | -70    | 6.0      | 0.8      | 0.1             | 12.0     | 2.2             | 2.50          | 0.09                 | PL  | ... | 1,4,5 | ...                                                                                                                   | ... | ...   | ...                      |
| J0004.2+0843 | 1.057 | 8.727   | 103.599 | -52.363 | 0.090      | 0.086      | -67    | 4.7      | 0.3      | 0.1             | 3.0      | 0.8             | 2.05          | 0.19                 | PL  | ... | ...   | ...                                                                                                                   | ... | ...   | ...                      |
| J0004.7-4740 | 1.181 | -47.671 | 323.816 | -67.519 | 0.090      | 0.078      | -41    | 14.5     | 0.7      | 0.1             | 9.2      | 0.8             | 2.40          | 0.08                 | PL  | T   | ...   | 2FGL J0004.7-4736<br>1FGL J0004.7-4737                                                                                | ... | fsrq  | PKS 0002-478             |
| J0006.2+0135 | 1.572 | 1.585   | 100.401 | -59.297 | 0.098      | 0.075      | 58     | 5.5      | 0.3      | 0.1             | 3.4      | 0.8             | 2.19          | 0.17                 | PL  | ... | ...   | ...                                                                                                                   | ... | ...   | ...                      |
| J0006.4+3825 | 1.612 | 38.418  | 113.332 | -23.613 | 0.225      | 0.142      | 32     | 10.5     | 0.6      | 0.1             | 10.4     | 1.0             | 2.62          | 0.08                 | PL  | T   | ...   | 2FGL J0006.1+3821<br>1FGL J0005.7+3815                                                                                | ... | fsrq  | S4 0003+38               |
| J0006.6+4618 | 1.651 | 46.305  | 114.908 | -15.867 | 0.142      | 0.115      | -79    | 4.6      | 0.3      | 0.1             | 4.2      | 1.0             | 2.42          | 0.19                 | PL  | ... | ...   | ...                                                                                                                   | ... | ...   | ...                      |
| J0007.0+7302 | 1.766 | 73.050  | 119.662 | 10.461  | 0.007      | 0.007      | -67    | 288.7    | 64.9     | 0.6             | 425.6    | 3.9             | 1.88          | ...                  | EC  | ... | ...   | 1FHL J0007.3+7303<br>2FGL J0007.0+7303<br>1FGL J0007.0+7303<br>0FGL J0007.4+7303<br>EGR J0008+7308<br>1AGL J0006+7311 | E   | PSR   | LAT PSR J0007+7303       |
| J0007.4+1742 | 1.869 | 17.711  | 108.332 | -43.911 | 0.214      | 0.169      | -19    | 4.6      | 0.3      | 0.1             | 3.4      | 0.8             | 2.31          | 0.17                 | PL  | ... | ...   | ...                                                                                                                   | ... | ...   | ...                      |
| J0007.9+4006 | 1.983 | 40.107  | 113.977 | -22.007 | 0.149      | 0.119      | -80    | 4.5      | 0.3      | 0.1             | 3.6      | 0.8             | 2.28          | 0.16                 | PL  | ... | ...   | ...                                                                                                                   | ... | ...   | ...                      |
| J0008.0+4713 | 2.017 | 47.228  | 115.333 | -15.003 | 0.033      | 0.030      | -13    | 24.7     | 2.0      | 0.1             | 21.9     | 1.5             | 2.02          | 0.05                 | PL  | ... | ...   | 1FHL J0007.7+4709<br>2FGL J0007.8+4713                                                                                | ... | bll   | MG4 J000800+4712         |
| J0008.3+1456 | 2.088 | 14.934  | 107.679 | -46.658 | 0.143      | 0.124      | 60     | 6.5      | 0.4      | 0.1             | 4.9      | 0.8             | 2.27          | 0.13                 | PL  | ... | ...   | 1FGL J0008.3+1452                                                                                                     | ... | ...   | ...                      |
| J0008.5+6853 | 2.141 | 68.887  | 119.067 | 6.338   | 0.493      | 0.454      | -79    | 8.4      | 1.0      | 0.2             | 8.8      | 1.3             | 2.46          | ...                  | LP  | ... | 1,3,9 | 2FGL J0007.7+6825c                                                                                                    | ... | ...   | ...                      |

Table 1—Continued

| Name 3FGL    | R.A.  | Decl.   | $l$     | $b$     | $\theta_1$ | $\theta_2$ | $\phi$ | $\sigma$ | $F_{35}$ | $\Delta F_{35}$ | $S_{25}$ | $\Delta S_{25}$ | $\Gamma_{25}$ | $\Delta \Gamma_{25}$ | Mod | Var | Flags | $\gamma$ -ray Assoc.                                        | TeV | Class | ID or Assoc.                  |
|--------------|-------|---------|---------|---------|------------|------------|--------|----------|----------|-----------------|----------|-----------------|---------------|----------------------|-----|-----|-------|-------------------------------------------------------------|-----|-------|-------------------------------|
| J0008.6–2340 | 2.174 | –23.672 | 50.280  | –79.753 | 0.074      | 0.066      | –61    | 6.7      | 0.2      | 0.1             | 3.5      | 0.9             | 1.60          | 0.18                 | PL  | ... | ...   | 1FGL J0005.1+6829<br>1FHL J0008.7–2340<br>2FGL J0008.7–2344 | ... | bl    | RBS 0016                      |
| J0008.7+6558 | 2.191 | 65.968  | 118.601 | 3.456   | 0.119      | 0.097      | 28     | 8.7      | 0.7      | 0.1             | 13.2     | 1.6             | 2.46          | ...                  | LP  | ... | 4,12  | 2FGL J0010.5+6556c                                          | ... | ...   | ...                           |
| J0009.1+0630 | 2.295 | 6.505   | 104.489 | –54.846 | 0.068      | 0.054      | –46    | 9.0      | 0.5      | 0.1             | 6.2      | 0.9             | 2.18          | 0.11                 | PL  | ... | ...   | 2FGL J0009.0+0632                                           | ... | bl    | CRATES<br>J000903.95+062821.5 |
| J0009.3+5030 | 2.334 | 50.510  | 116.116 | –11.803 | 0.020      | 0.019      | 18     | 36.5     | 3.1      | 0.1             | 35.4     | 1.9             | 1.93          | 0.03                 | PL  | T   | ...   | 1FGL J0008.9+0635<br>1FHL J0009.2+5032                      | ... | bl    | NVSS<br>J000922+503028        |
| J0009.6–3211 | 2.402 | –32.199 | 1.252   | –79.602 | 0.146      | 0.136      | 19     | 5.5      | 0.3      | 0.1             | 3.4      | 0.7             | 2.31          | 0.15                 | PL  | ... | 1     | 2FGL J0009.1+5030<br>2FGL J0009.9–3206                      | ... | bcu   | IC 1531                       |
| J0010.5–1425 | 2.629 | –14.420 | 84.006  | –74.112 | 0.215      | 0.150      | 89     | 4.3      | 0.2      | 0.1             | 3.0      | 0.7             | 2.31          | 0.15                 | PL  | ... | ...   | ...                                                         | ... | ...   | ...                           |
| J0012.4+7040 | 3.110 | 70.672  | 119.687 | 8.046   | 0.119      | 0.092      | –58    | 4.5      | 0.4      | 0.1             | 6.3      | 1.4             | 2.48          | 0.14                 | PL  | ... | 4     | ...                                                         | ... | bcu   | TXS 0008+704                  |
| J0013.2–3954 | 3.304 | –39.908 | 332.324 | –74.962 | 0.058      | 0.051      | 31     | 12.0     | 0.6      | 0.1             | 7.0      | 0.8             | 2.21          | 0.09                 | PL  | ... | ...   | 2FGL J0012.9–3954<br>1FGL J0013.1–3952                      | ... | bl    | PKS 0010–401<br>S             |
| J0013.9–1853 | 3.476 | –18.897 | 74.627  | –78.078 | 0.062      | 0.059      | 56     | 5.6      | 0.2      | 0.1             | 2.7      | 0.7             | 1.94          | 0.17                 | PL  | ... | ...   | ...                                                         | P   | bl    | RBS 0030                      |
| J0014.0–5025 | 3.515 | –50.429 | 317.451 | –65.633 | 0.086      | 0.073      | –38    | 5.7      | 0.2      | 0.1             | 2.8      | 0.7             | 1.92          | 0.16                 | PL  | ... | ...   | 1FGL J0013.7–5022                                           | ... | bl    | RBS 0032                      |
| J0014.3–0455 | 3.586 | –4.920  | 99.590  | –66.096 | 0.127      | 0.108      | –59    | 6.3      | 0.4      | 0.1             | 6.5      | 1.2             | 2.50          | 0.13                 | PL  | ... | 5     | ...                                                         | ... | ...   | ...                           |
| J0014.6+6119 | 3.659 | 61.318  | 118.530 | –1.239  | 0.065      | 0.057      | 20     | 7.4      | 0.7      | 0.1             | 7.8      | 1.4             | 1.89          | 0.11                 | PL  | ... | ...   | ...                                                         | ... | bcu   | 4C +60.01                     |
| J0014.7+5802 | 3.683 | 58.042  | 118.075 | –4.483  | 0.058      | 0.052      | –72    | 5.5      | 0.4      | 0.1             | 4.3      | 1.1             | 1.91          | 0.17                 | PL  | ... | ...   | ...                                                         | ... | bl    | 1RXS<br>J001442.2+580201      |
| J0015.7+5552 | 3.941 | 55.875  | 117.909 | –6.649  | 0.045      | 0.042      | –79    | 6.4      | 0.4      | 0.1             | 5.0      | 1.1             | 2.11          | 0.14                 | PL  | ... | ...   | ...                                                         | ... | bcu   | GB6 J0015+5551                |
| J0016.3–0013 | 4.078 | –0.230  | 104.079 | –61.809 | 0.110      | 0.104      | 42     | 13.6     | 0.6      | 0.1             | 11.0     | 0.9             | 2.62          | 0.07                 | PL  | T   | ...   | 2FGL J0017.4–0018                                           | ... | fsrq  | S3 0013–00                    |
| J0016.5+1713 | 4.135 | 17.221  | 111.141 | –44.850 | 0.216      | 0.178      | 80     | 4.1      | 0.2      | 0.1             | 3.3      | 0.8             | 2.44          | 0.16                 | PL  | ... | ...   | 1FGL J0016.6+1706                                           | ... | ...   | ...                           |
| J0017.1+1445 | 4.294 | 14.761  | 110.672 | –47.293 | 0.085      | 0.080      | 88     | 4.8      | 0.2      | 0.1             | 2.9      | 0.8             | 1.88          | 0.18                 | PL  | ... | ...   | ...                                                         | ... | ...   | ...                           |
| J0017.2–0643 | 4.305 | –6.724  | 99.669  | –68.036 | 0.126      | 0.103      | 68     | 6.2      | 0.4      | 0.1             | 4.3      | 0.8             | 2.12          | 0.14                 | PL  | ... | ...   | ...                                                         | ... | bcu   | PMN J0017–0650                |
| J0017.6–0512 | 4.405 | –5.205  | 101.258 | –66.643 | 0.071      | 0.066      | 8      | 12.0     | 0.8      | 0.1             | 11.8     | 1.3             | 2.51          | 0.08                 | PL  | T   | ...   | 2FGL J0017.6–0510<br>1FGL J0017.4–0510<br>0FGL J0017.4–0503 | ... | FSRQ  | PMN J0017–0512                |
| J0018.4+2947 | 4.603 | 29.794  | 114.432 | –32.532 | 0.083      | 0.074      | 68     | 5.0      | 0.2      | 0.1             | 2.5      | 0.7             | 1.86          | 0.21                 | PL  | ... | ...   | 1FHL J0018.6+2946<br>2FGL J0018.5+2945<br>1FGL J0018.6+2945 | ... | bl    | RBS 0042                      |
| J0018.9–8152 | 4.745 | –81.877 | 304.330 | –35.163 | 0.058      | 0.049      | –11    | 10.7     | 0.7      | 0.1             | 7.3      | 1.0             | 2.08          | 0.10                 | PL  | T   | ...   | 2FGL J0018.8–8154                                           | ... | bl    | PMN J0019–8152                |
| J0019.1–5645 | 4.797 | –56.751 | 311.732 | –59.822 | 0.117      | 0.100      | 19     | 6.8      | 0.3      | 0.1             | 3.7      | 0.7             | 2.39          | 0.17                 | PL  | ... | ...   | 2FGL J0019.4–5645                                           | ... | bcu   | PMN J0019–5641                |
| J0019.4+2021 | 4.862 | 20.366  | 112.844 | –41.878 | 0.166      | 0.105      | 82     | 5.0      | 0.3      | 0.1             | 3.5      | 0.8             | 2.25          | 0.16                 | PL  | ... | ...   | 1FGL J0019.3+2017                                           | ... | bl    | PKS 0017+200                  |
| J0020.9+0323 | 5.231 | 3.395   | 108.198 | –58.601 | 0.058      | 0.055      | –27    | 5.7      | 0.2      | 0.1             | 3.0      | 0.9             | 1.64          | 0.18                 | PL  | ... | ...   | ...                                                         | ... | ...   | ...                           |
| J0021.6–6835 | 5.409 | –68.592 | 307.012 | –48.300 | 0.478      | 0.185      | 47     | 5.4      | 0.2      | 0.1             | 3.8      | 0.7             | 2.65          | 0.16                 | PL  | ... | 9     | ...                                                         | ... | bcu   | PKS 0021–686                  |

Table 1—Continued

| Name 3FGL    | R.A.  | Decl.   | $l$     | $b$     | $\theta_1$ | $\theta_2$ | $\phi$ | $\sigma$ | $F_{35}$ | $\Delta F_{35}$ | $S_{25}$ | $\Delta S_{25}$ | $\Gamma_{25}$ | $\Delta \Gamma_{25}$ | Mod | Var | Flags | $\gamma$ -ray Assoc. | TeV | Class | ID or Assoc.                  |
|--------------|-------|---------|---------|---------|------------|------------|--------|----------|----------|-----------------|----------|-----------------|---------------|----------------------|-----|-----|-------|----------------------|-----|-------|-------------------------------|
| J0021.6–2553 | 5.415 | –25.887 | 41.811  | –83.224 | 0.057      | 0.049      | 15     | 11.6     | 0.6      | 0.1             | 6.6      | 0.8             | 2.10          | 0.10                 | PL  | ... | ...   | 2FGL J0021.6–2551    | ... | bll   | CRATES<br>J002132.55–255049.3 |
|              |       |         |         |         |            |            |        |          |          |                 |          |                 |               |                      |     |     |       | 1FGL J0021.7–2556    |     |       |                               |
| J0022.1–1855 | 5.536 | –18.923 | 82.031  | –79.387 | 0.033      | 0.031      | 62     | 16.7     | 0.9      | 0.1             | 11.1     | 1.4             | 1.80          | 0.07                 | PL  | ... | ...   | 1FHL J0022.2–1853    | ... | bll   | 1RXS<br>J002209.2–185333      |
|              |       |         |         |         |            |            |        |          |          |                 |          |                 |               |                      |     |     |       | 2FGL J0022.2–1853    |     |       |                               |
|              |       |         |         |         |            |            |        |          |          |                 |          |                 |               |                      |     |     |       | 1FGL J0022.2–1850    |     |       |                               |
| J0022.1–5141 | 5.548 | –51.691 | 313.620 | –64.826 | 0.050      | 0.045      | –76    | 13.7     | 0.7      | 0.1             | 7.9      | 1.0             | 1.99          | 0.08                 | PL  | ... | ...   | 2FGL J0022.3–5141    | ... | bll   | 1RXS<br>J002159.2–514028      |
| J0022.5+0608 | 5.643 | 6.138   | 110.024 | –56.009 | 0.038      | 0.034      | –82    | 28.2     | 2.2      | 0.1             | 24.0     | 1.5             | 2.07          | 0.04                 | PL  | T   | ...   | 1FHL J0022.5+0607    | ... | bll   | PKS 0019+058                  |
|              |       |         |         |         |            |            |        |          |          |                 |          |                 |               |                      |     |     |       | 2FGL J0022.5+0607    |     |       |                               |
|              |       |         |         |         |            |            |        |          |          |                 |          |                 |               |                      |     |     |       | 1FGL J0022.5+0607    |     |       |                               |
| J0022.7+4651 | 5.687 | 46.853  | 117.843 | –15.735 | 0.239      | 0.188      | 63     | 4.2      | 0.2      | 0.1             | 4.2      | 0.9             | 2.78          | 0.19                 | PL  | ... | ...   | ...                  | ... | ...   | ...                           |
| J0023.4+0923 | 5.865 | 9.389   | 111.455 | –52.858 | 0.085      | 0.079      | –87    | 13.3     | 1.1      | 0.1             | 7.3      | 0.8             | 2.28          | ...                  | EC  | ... | ...   | 2FGL J0023.5+0924    | ... | PSR   | PSR J0023+0923                |
|              |       |         |         |         |            |            |        |          |          |                 |          |                 |               |                      |     |     |       | 1FGL J0023.5+0930    |     |       |                               |
| J0023.5+4454 | 5.878 | 44.905  | 117.748 | –17.685 | 0.138      | 0.109      | –87    | 9.0      | 0.5      | 0.1             | 7.4      | 0.9             | 2.57          | 0.10                 | PL  | ... | ...   | 2FGL J0023.2+4454    | ... | fsrq  | B3 0020+4460                  |
|              |       |         |         |         |            |            |        |          |          |                 |          |                 |               |                      |     |     |       | 1FGL J0023.0+4453    |     |       |                               |
| J0023.9–7203 | 5.982 | –72.065 | 305.916 | –44.903 | 0.027      | 0.027      | –36    | 46.4     | 4.1      | 0.2             | 26.1     | 1.3             | 2.09          | ...                  | LP  | ... | ...   | 2FGL J0023.9–7204    | ... | glc   | 47 Tuc                        |
|              |       |         |         |         |            |            |        |          |          |                 |          |                 |               |                      |     |     |       | 1FGL J0023.9–7204    |     |       |                               |
|              |       |         |         |         |            |            |        |          |          |                 |          |                 |               |                      |     |     |       | 0FGL J0025.1–7202    |     |       |                               |
| J0024.4+0350 | 6.110 | 3.843   | 110.020 | –58.350 | 0.126      | 0.105      | 33     | 5.7      | 0.4      | 0.1             | 4.7      | 0.9             | 2.28          | 0.12                 | PL  | T   | ...   | 2FGL J0024.5+0346    | ... | fsrq  | GB6 J0024+0349                |
|              |       |         |         |         |            |            |        |          |          |                 |          |                 |               |                      |     |     |       | 1FGL J0024.6+0346    |     |       |                               |
| J0025.7+6404 | 6.433 | 64.069  | 120.126 | 1.338   | 0.141      | 0.097      | –57    | 4.4      | 0.6      | 0.1             | 6.3      | 1.5             | 2.09          | 0.14                 | PL  | ... | ...   | ...                  | P   | snr   | Tycho                         |
| J0026.2–4812 | 6.557 | –48.210 | 314.371 | –68.355 | 0.176      | 0.109      | –68    | 6.0      | 0.3      | 0.1             | 3.6      | 0.7             | 2.19          | 0.15                 | PL  | ... | ...   | ...                  | ... | ...   | ...                           |
| J0026.7–4603 | 6.685 | –46.060 | 315.817 | –70.446 | 0.165      | 0.108      | 7      | 5.1      | 0.2      | 0.1             | 2.9      | 0.6             | 2.45          | 0.18                 | PL  | ... | 1     | ...                  | ... | bll   | 1RXS<br>J002636.3–460101      |
| J0028.6+7507 | 7.161 | 75.119  | 121.437 | 12.313  | 0.091      | 0.074      | 88     | 7.3      | 0.5      | 0.1             | 6.8      | 1.0             | 2.34          | 0.11                 | PL  | ... | ...   | ...                  | ... | bcu   | GB6 J0028+7506                |
| J0028.8+1951 | 7.201 | 19.851  | 115.683 | –42.702 | 0.207      | 0.122      | 2      | 6.3      | 0.4      | 0.1             | 5.2      | 0.8             | 2.43          | 0.12                 | PL  | ... | 9     | ...                  | ... | bcu   | TXS 0025+197                  |
| J0029.1–7045 | 7.296 | –70.756 | 305.581 | –46.258 | 0.064      | 0.057      | 58     | 12.1     | 0.7      | 0.1             | 8.0      | 0.9             | 2.28          | 0.10                 | PL  | T   | ...   | 2FGL J0029.2–7043    | ... | bll   | PKS 0026–710                  |
| J0030.2–1646 | 7.566 | –16.775 | 96.521  | –78.546 | 0.043      | 0.040      | 4      | 9.2      | 0.3      | 0.1             | 4.8      | 1.1             | 1.65          | 0.13                 | PL  | ... | ...   | 1FHL J0030.1–1647    | ... | bcu   | 1RXS<br>J003019.6–164723      |
| J0030.3–4223 | 7.589 | –42.395 | 317.302 | –74.140 | 0.053      | 0.052      | 62     | 28.8     | 1.2      | 0.1             | 19.8     | 0.9             | 2.58          | 0.04                 | PL  | T   | ...   | 2FGL J0030.2–4223    | ... | fsrq  | PKS 0027–426                  |
|              |       |         |         |         |            |            |        |          |          |                 |          |                 |               |                      |     |     |       | 1FGL J0029.9–4221    |     |       |                               |
| J0030.4+0451 | 7.616 | 4.866   | 113.147 | –57.607 | 0.021      | 0.020      | 41     | 80.8     | 9.8      | 0.3             | 60.7     | 1.5             | 2.04          | ...                  | EC  | ... | ...   | 2FGL J0030.4+0450    | ... | PSR   | PSR J0030+0451                |
|              |       |         |         |         |            |            |        |          |          |                 |          |                 |               |                      |     |     |       | 1FGL J0030.4+0451    |     |       |                               |
|              |       |         |         |         |            |            |        |          |          |                 |          |                 |               |                      |     |     |       | 0FGL J0030.3+0450    |     |       |                               |
| J0030.7–0209 | 7.698 | –2.157  | 110.859 | –64.544 | 0.071      | 0.069      | –75    | 15.0     | 0.9      | 0.1             | 11.3     | 1.0             | 2.38          | 0.07                 | PL  | T   | ...   | ...                  | ... | bcu   | PKS B0027–024                 |
| J0031.2–2320 | 7.813 | –23.343 | 71.502  | –84.071 | 0.180      | 0.142      | –65    | 4.2      | 0.2      | 0.1             | 2.7      | 0.7             | 2.14          | 0.17                 | PL  | ... | ...   | ...                  | ... | ...   | ...                           |
| J0031.3+0724 | 7.830 | 7.415   | 114.189 | –55.115 | 0.079      | 0.065      | –52    | 5.1      | 0.2      | 0.1             | 2.7      | 0.8             | 1.82          | 0.19                 | PL  | ... | ...   | 2FGL J0031.0+0724    | ... | bcu   | NVSS<br>J003119+072456        |
| J0031.6+0938 | 7.923 | 9.648   | 114.845 | –52.914 | 0.094      | 0.090      | –61    | 5.1      | 0.2      | 0.1             | 4.3      | 0.9             | 2.66          | 0.16                 | PL  | ... | ...   | ...                  | ... | ...   | ...                           |

Table 1—Continued

| Name 3FGL    | R.A.   | Decl.   | $l$     | $b$     | $\theta_1$ | $\theta_2$ | $\phi$ | $\sigma$ | $F_{35}$ | $\Delta F_{35}$ | $S_{25}$ | $\Delta S_{25}$ | $\Gamma_{25}$ | $\Delta \Gamma_{25}$ | Mod | Var | Flags | $\gamma$ -ray Assoc.                                                             | TeV | Class | ID or Assoc.           |
|--------------|--------|---------|---------|---------|------------|------------|--------|----------|----------|-----------------|----------|-----------------|---------------|----------------------|-----|-----|-------|----------------------------------------------------------------------------------|-----|-------|------------------------|
| J0032.3–2852 | 8.090  | –28.877 | 9.275   | –85.441 | 0.078      | 0.073      | –87    | 4.9      | 0.2      | 0.1             | 2.6      | 0.6             | 2.19          | 0.18                 | PL  | ... | ...   | ...                                                                              | ... | bll   | PMN J0032–2849         |
| J0032.3–5522 | 8.094  | –55.369 | 308.619 | –61.549 | 0.055      | 0.047      | 16     | 18.1     | 0.9      | 0.1             | 11.1     | 0.9             | 2.27          | 0.07                 | PL  | T   | ...   | 2FGL J0032.7–5521<br>1FGL J0032.7–5519                                           | ... | ...   | ...                    |
| J0032.5+3912 | 8.146  | 39.213  | 118.951 | –23.513 | 0.088      | 0.083      | –62    | 5.0      | 0.2      | 0.1             | 3.8      | 0.8             | 2.56          | 0.17                 | PL  | ... | ...   | ...                                                                              | ... | ...   | ...                    |
| J0033.6–1921 | 8.402  | –19.364 | 94.212  | –81.224 | 0.019      | 0.019      | –73    | 39.2     | 2.8      | 0.1             | 37.0     | 2.6             | 1.71          | 0.04                 | PL  | ... | ...   | 1FHL J0033.6–1921<br>2FGL J0033.5–1921<br>1FGL J0033.5–1921<br>0FGL J0033.6–1921 | P   | bll   | KUV 00311–1938         |
| J0034.3–0534 | 8.590  | –5.582  | 111.487 | –68.074 | 0.045      | 0.042      | 70     | 28.9     | 2.4      | 0.2             | 18.0     | 1.0             | 2.21          | ...                  | EC  | ... | ...   | 2FGL J0034.4–0534<br>1FGL J0034.3–0534                                           | ... | PSR   | PSR J0034–0534         |
| J0035.2+1513 | 8.809  | 15.222  | 117.146 | –47.467 | 0.043      | 0.038      | –79    | 14.0     | 0.8      | 0.1             | 10.2     | 1.4             | 1.81          | 0.09                 | PL  | ... | ...   | 1FHL J0035.2+1514<br>2FGL J0035.2+1515<br>1FGL J0035.1+1516                      | ... | bll   | RX J0035.2+1515        |
| J0035.9+5949 | 8.989  | 59.832  | 120.986 | –2.981  | 0.018      | 0.017      | –67    | 27.5     | 2.7      | 0.2             | 30.9     | 2.0             | 1.90          | 0.04                 | PL  | ... | ...   | 1FHL J0035.9+5950<br>2FGL J0035.8+5951<br>1FGL J0035.9+5951<br>0FGL J0036.7+5951 | P   | bll   | 1ES 0033+595<br>4      |
| J0037.9+1239 | 9.477  | 12.652  | 117.785 | –50.085 | 0.045      | 0.042      | –25    | 13.3     | 0.9      | 0.1             | 10.2     | 1.1             | 2.15          | 0.08                 | PL  | ... | ...   | 1FHL J0037.8+1238<br>2FGL J0037.8+1238<br>1FGL J0038.0+1236                      | ... | bll   | NVSS<br>J003750+123818 |
| J0038.0–2501 | 9.509  | –25.032 | 67.046  | –86.333 | 0.106      | 0.101      | –80    | 10.1     | 0.5      | 0.1             | 6.6      | 0.8             | 2.44          | 0.09                 | PL  | T   | ...   | 2FGL J0038.3–2457<br>1FGL J0038.4–2504                                           | ... | fsrq  | PKS 0035–252           |
| J0038.0+0012 | 9.523  | 0.209   | 115.697 | –62.475 | 0.089      | 0.071      | 64     | 7.5      | 0.4      | 0.1             | 4.7      | 0.8             | 2.16          | 0.12                 | PL  | ... | ...   | 2FGL J0038.1+0015                                                                | ... | bll   | NVSS<br>J003808+001336 |
| J0039.0–2218 | 9.750  | –22.307 | 91.911  | –84.413 | 0.105      | 0.094      | –35    | 4.4      | 0.2      | 0.1             | 2.3      | 0.8             | 1.72          | 0.20                 | PL  | ... | ...   | 2FGL J0038.7–2215                                                                | ... | bcu   | PMN J0039–2220         |
| J0039.1–0939 | 9.782  | –9.658  | 112.914 | –72.290 | 0.283      | 0.144      | 87     | 4.8      | 0.2      | 0.1             | 3.9      | 0.8             | 2.59          | 0.15                 | PL  | ... | ...   | 3EG J0038–0949<br>EGR J0039–0945                                                 | ... | fsrq  | TXS 0036–099           |
| J0039.1+4330 | 9.798  | 43.502  | 120.580 | –19.314 | 0.057      | 0.053      | 54     | 7.0      | 0.3      | 0.1             | 3.8      | 0.8             | 1.96          | 0.14                 | PL  | ... | ...   | 2FGL J0039.1+4331<br>1FGL J0039.2+4331                                           | ... | bcu   | NVSS<br>J003907+433015 |
| J0039.3+6256 | 9.834  | 62.942  | 121.557 | 0.102   | 0.056      | 0.054      | –27    | 12.0     | 2.1      | 0.2             | 9.1      | 1.1             | 2.12          | ...                  | LP  | ... | ...   | 2FGL J0038.8+6259<br>1FGL J0038.6+6306                                           | ... | ...   | ...                    |
| J0040.3+4049 | 10.083 | 40.818  | 120.666 | –22.005 | 0.043      | 0.040      | 70     | 6.4      | 0.1      | 0.1             | 2.5      | 0.9             | 1.13          | 0.33                 | PL  | ... | ...   | 1FHL J0040.3+4049                                                                | ... | bcu   | B3 0037+405            |
| J0040.5–2339 | 10.147 | –23.651 | 87.170  | –85.747 | 0.089      | 0.074      | 36     | 4.3      | 0.2      | 0.1             | 2.1      | 0.7             | 1.95          | 0.19                 | PL  | ... | ...   | ...                                                                              | ... | bcu   | PMN J0040–2340         |
| J0041.9+3639 | 10.500 | 36.662  | 120.824 | –26.171 | 0.070      | 0.067      | 46     | 4.6      | 0.2      | 0.1             | 2.5      | 0.7             | 1.98          | 0.21                 | PL  | ... | ...   | ...                                                                              | ... | bll   | RX J0042.0+3641        |
| J0042.0+2318 | 10.518 | 23.305  | 120.145 | –39.516 | 0.200      | 0.118      | –30    | 6.1      | 0.4      | 0.1             | 4.6      | 0.8             | 2.35          | 0.13                 | PL  | ... | ...   | 1FGL J0041.9+2318                                                                | ... | fsrq  | PKS 0039+230           |
| J0042.5+4117 | 10.629 | 41.296  | 121.131 | –21.545 | 0.165      | 0.133      | –42    | 5.8      | 0.4      | 0.1             | 5.9      | 0.9             | 2.56          | 0.11                 | PL  | ... | ...   | 2FGL J0042.5+4114                                                                | ... | gal   | M31                    |

Table 1—Continued

| Name 3FGL    | R.A.   | Decl.   | $l$     | $b$     | $\theta_1$ | $\theta_2$ | $\phi$ | $\sigma$ | $F_{35}$ | $\Delta F_{35}$ | $S_{25}$ | $\Delta S_{25}$ | $\Gamma_{25}$ | $\Delta \Gamma_{25}$ | Mod | Var | Flags | $\gamma$ -ray Assoc.                                                             | TeV | Class | ID or Assoc.             |
|--------------|--------|---------|---------|---------|------------|------------|--------|----------|----------|-----------------|----------|-----------------|---------------|----------------------|-----|-----|-------|----------------------------------------------------------------------------------|-----|-------|--------------------------|
| J0043.5–0444 | 10.892 | –4.740  | 117.796 | –67.533 | 0.062      | 0.053      | 59     | 5.8      | 0.2      | 0.1             | 3.0      | 0.9             | 1.73          | 0.23                 | PL  | ... | ...   | ...                                                                              | ... | bcu   | 1RXS<br>J004333.7–044257 |
| J0043.7–1117 | 10.935 | –11.288 | 116.047 | –74.057 | 0.074      | 0.068      | 1      | 5.9      | 0.2      | 0.1             | 3.7      | 1.1             | 1.59          | 0.16                 | PL  | ... | ...   | 1FHL J0044.0–1111                                                                | ... | bcu   | 1RXS<br>J004349.3–111612 |
| J0043.8+3425 | 10.969 | 34.429  | 121.160 | –28.416 | 0.035      | 0.033      | –85    | 22.6     | 1.6      | 0.1             | 17.9     | 1.3             | 2.04          | 0.05                 | PL  | T   | ...   | 1FHL J0043.7+3425<br>2FGL J0043.7+3426<br>1FGL J0043.6+3424                      | ... | fsrq  | GB6 J0043+3426           |
| J0045.2–3704 | 11.311 | –37.080 | 310.037 | –79.963 | 0.094      | 0.079      | –35    | 13.6     | 0.6      | 0.1             | 8.7      | 0.8             | 2.54          | 0.08                 | PL  | T   | ...   | 2FGL J0044.7–3702                                                                | ... | bcu   | PKS 0042–373             |
| J0045.3+2126 | 11.349 | 21.446  | 121.059 | –41.404 | 0.026      | 0.024      | 29     | 22.3     | 1.4      | 0.1             | 16.1     | 1.4             | 1.90          | 0.06                 | PL  | ... | ...   | 1FHL J0045.2+2126<br>2FGL J0045.3+2127<br>1FGL J0045.3+2127                      | ... | bll   | GB6 J0045+2127           |
| J0045.7+1217 | 11.435 | 12.288  | 120.741 | –50.559 | 0.038      | 0.036      | –87    | 14.5     | 1.0      | 0.1             | 10.8     | 1.2             | 1.96          | 0.08                 | PL  | ... | ...   | 2FGL J0045.5+1218                                                                | ... | bll   | GB6 J0045+1217           |
| J0046.7–8419 | 11.688 | –84.320 | 303.070 | –32.807 | 0.155      | 0.124      | 75     | 6.2      | 0.3      | 0.1             | 6.5      | 1.0             | 2.82          | 0.13                 | PL  | ... | ...   | 2FGL J0046.7–8416<br>1FGL J0048.0–8412                                           | ... | fsrq  | PKS 0044–84              |
| J0047.0+5658 | 11.767 | 56.972  | 122.334 | –5.895  | 0.042      | 0.038      | 73     | 18.1     | 1.6      | 0.1             | 18.3     | 1.3             | 2.22          | 0.05                 | PL  | T   | 3     | 2FGL J0047.2+5657<br>1FGL J0046.8+5658                                           | ... | bll   | GB6 J0047+5657           |
| J0047.5–2516 | 11.887 | –25.275 | 97.502  | –87.952 | 0.097      | 0.068      | –79    | 12.9     | 0.8      | 0.1             | 8.6      | 0.9             | 2.17          | 0.08                 | PL  | ... | ...   | 2FGL J0047.0–2516<br>1FGL J0047.3–2512                                           | P   | sbq   | NGC 253                  |
| J0047.9+5447 | 11.984 | 54.797  | 122.423 | –8.071  | 0.066      | 0.054      | –23    | 5.0      | 0.1      | 0.1             | 2.9      | 1.0             | 1.33          | 0.27                 | PL  | ... | ...   | ...                                                                              | ... | bcu   | 1RXS<br>J004754.5+544758 |
| J0048.0+3950 | 12.007 | 39.843  | 122.221 | –23.024 | 0.077      | 0.054      | –12    | 9.2      | 0.5      | 0.1             | 5.8      | 1.0             | 1.88          | 0.12                 | PL  | ... | ...   | ...                                                                              | ... | bll   | B3 0045+395              |
| J0048.0+2236 | 12.013 | 22.601  | 121.909 | –40.264 | 0.081      | 0.065      | 9      | 14.2     | 0.9      | 0.1             | 11.7     | 1.0             | 2.33          | 0.07                 | PL  | T   | ...   | 2FGL J0047.9+2232<br>1FGL J0048.0+2232                                           | ... | fsrq  | NVSS<br>J004802+223525   |
| J0048.1–6343 | 12.050 | –63.732 | 303.533 | –53.393 | 0.138      | 0.099      | –9     | 6.8      | 0.3      | 0.1             | 3.9      | 0.7             | 2.11          | 0.14                 | PL  | ... | ...   | 2FGL J0048.8–6347                                                                | ... | ...   | ...                      |
| J0049.0+4224 | 12.253 | 42.413  | 122.455 | –20.456 | 0.047      | 0.041      | 70     | 6.9      | 0.3      | 0.1             | 3.3      | 0.8             | 1.77          | 0.17                 | PL  | ... | ...   | ...                                                                              | ... | ...   | ...                      |
| J0049.4–5401 | 12.353 | –54.022 | 303.589 | –63.103 | 0.093      | 0.084      | 38     | 6.0      | 0.3      | 0.1             | 3.1      | 0.7             | 2.14          | 0.16                 | PL  | ... | ...   | ...                                                                              | ... | bcu   | PMN J0049–5402           |
| J0049.4–4149 | 12.360 | –41.825 | 304.397 | –75.298 | 0.085      | 0.068      | –62    | 5.7      | 0.3      | 0.1             | 2.8      | 0.7             | 2.15          | 0.22                 | PL  | ... | ...   | ...                                                                              | ... | bcu   | 1RXS<br>J004939.9–415133 |
| J0049.7+0237 | 12.441 | 2.625   | 122.091 | –60.244 | 0.078      | 0.056      | –42    | 13.1     | 0.8      | 0.1             | 9.3      | 0.9             | 2.24          | 0.08                 | PL  | T   | ...   | 2FGL J0050.2+0234<br>1FGL J0050.2+0235                                           | ... | bll   | PKS 0047+023             |
| J0049.8–5737 | 12.463 | –57.625 | 303.351 | –59.503 | 0.057      | 0.056      | 6      | 10.1     | 0.4      | 0.1             | 6.1      | 0.8             | 2.46          | 0.11                 | PL  | ... | ...   | 2FGL J0049.7–5738<br>1FGL J0049.8–5738                                           | ... | fsrq  | PKS 0047–579             |
| J0050.0–4458 | 12.514 | –44.972 | 303.730 | –72.154 | 0.150      | 0.140      | 26     | 6.1      | 0.2      | 0.1             | 3.8      | 0.7             | 2.53          | 0.15                 | PL  | ... | ...   | ...                                                                              | ... | bcu   | PMN J0049–4457           |
| J0050.4–0449 | 12.621 | –4.832  | 122.307 | –67.703 | 0.113      | 0.100      | 45     | 9.0      | 0.5      | 0.1             | 7.5      | 1.0             | 2.45          | 0.11                 | PL  | ... | ...   | 2FGL J0050.1–0452<br>1FGL J0050.0–0446                                           | ... | fsrq  | PKS 0047–051             |
| J0050.6–0929 | 12.674 | –9.485  | 122.331 | –72.356 | 0.027      | 0.026      | –79    | 42.0     | 3.6      | 0.2             | 40.3     | 1.8             | 2.09          | 0.03                 | PL  | T   | ...   | 1FHL J0050.6–0930<br>2FGL J0050.6–0929<br>1FGL J0050.6–0928<br>0FGL J0050.5–0928 | ... | BLL   | PKS 0048–09              |

Table 1—Continued

| Name 3FGL     | R.A.   | Decl.   | $l$     | $b$     | $\theta_1$ | $\theta_2$ | $\phi$ | $\sigma$ | $F_{35}$ | $\Delta F_{35}$ | $S_{25}$ | $\Delta S_{25}$ | $\Gamma_{25}$ | $\Delta \Gamma_{25}$ | Mod | Var | Flags | $\gamma$ -ray Assoc.                                                             | TeV | Class | ID or Assoc.             |
|---------------|--------|---------|---------|---------|------------|------------|--------|----------|----------|-----------------|----------|-----------------|---------------|----------------------|-----|-----|-------|----------------------------------------------------------------------------------|-----|-------|--------------------------|
| J0051.0–0649  | 12.766 | –6.818  | 122.665 | –69.689 | 0.063      | 0.059      | –74    | 18.4     | 1.4      | 0.1             | 11.9     | 1.1             | 2.29          | ...                  | LP  | T   | ...   | 2FGL J0051.0–0648<br>1FGL J0051.1–0649<br>0FGL J0051.1–0647                      | ... | fsrq  | PKS 0048–071             |
| J0051.2–6241  | 12.820 | –62.688 | 302.963 | –54.440 | 0.029      | 0.026      | 32     | 23.4     | 1.2      | 0.1             | 16.5     | 1.7             | 1.66          | 0.06                 | PL  | ... | ...   | 1FHL J0051.3–6240<br><br>2FGL J0051.4–6241<br>1FGL J0051.4–6242                  | ... | bcu   | 1RXS<br>J005117.7–624154 |
| J0051.6+6445  | 12.904 | 64.759  | 122.951 | 1.888   | 0.072      | 0.059      | 49     | 5.6      | 0.7      | 0.1             | 8.2      | 1.6             | 2.28          | 0.12                 | PL  | ... | 3,4   | ...                                                                              | ... | ...   | ...                      |
| J0054.8–2455  | 13.723 | –24.924 | 142.526 | –87.662 | 0.042      | 0.032      | 17     | 15.8     | 0.8      | 0.1             | 10.5     | 1.4             | 1.78          | 0.08                 | PL  | ... | ...   | 1FHL J0054.8–2456<br>2FGL J0055.0–2454<br>1FGL J0054.9–2455                      | ... | bll   | FRBA J0054–2455          |
| J0055.2–1213  | 13.801 | –12.233 | 126.510 | –75.078 | 0.138      | 0.117      | –64    | 4.7      | 0.2      | 0.1             | 3.2      | 0.7             | 2.40          | 0.17                 | PL  | ... | ...   | ...                                                                              | ... | bcu   | TXS 0052–125             |
| J0056.3–2116  | 14.076 | –21.280 | 133.935 | –84.048 | 0.057      | 0.051      | –88    | 12.0     | 0.6      | 0.1             | 7.7      | 1.2             | 1.81          | 0.09                 | PL  | ... | ...   | 2FGL J0056.8–2111<br>...                                                         | ... | bll   | PMN J0056–2117           |
| J0056.3–0935  | 14.090 | –9.594  | 126.954 | –72.427 | 0.062      | 0.051      | 25     | 9.9      | 0.5      | 0.1             | 6.5      | 1.2             | 1.79          | 0.12                 | PL  | ... | ...   | ...                                                                              | ... | bll   | TXS 0053+098             |
| J0057.9–0542  | 14.483 | –5.708  | 127.349 | –68.524 | 0.169      | 0.127      | –20    | 5.2      | 0.3      | 0.1             | 4.2      | 0.9             | 2.42          | 0.17                 | PL  | ... | 1     | ...                                                                              | ... | fsrq  | PKS 0055+059             |
| J0058.0–3233  | 14.513 | –32.567 | 288.564 | –84.376 | 0.045      | 0.042      | 50     | 20.5     | 1.2      | 0.1             | 13.6     | 1.1             | 2.06          | 0.06                 | PL  | ... | ...   | 1FHL J0058.6–3236<br>2FGL J0057.9–3236<br>1FGL J0058.4–3235                      | ... | bll   | PKS 0055+328             |
| J0058.3+3315  | 14.587 | 33.267  | 124.594 | –29.583 | 0.111      | 0.098      | –68    | 8.3      | 0.5      | 0.1             | 6.2      | 0.8             | 2.41          | 0.11                 | PL  | T   | ...   | 2FGL J0057.9+3311<br>1FGL J0058.0+3314                                           | ... | fsrq  | MG3 J005830+3311         |
| J0059.0–7242e | 14.750 | –72.700 | 302.145 | –44.417 | ...        | ...        | ...    | 27.9     | 3.5      | 0.2             | 40.4     | 2.0             | 2.22          | 0.03                 | PL  | ... | 3     | 2FGL J0059.0–7242e<br>1FGL J0101.3–7257                                          | ... | GAL   | SMC                      |
| J0059.1–5701  | 14.796 | –57.022 | 300.819 | –60.075 | 0.168      | 0.140      | 49     | 11.2     | 0.5      | 0.1             | 8.5      | 0.9             | 2.62          | 0.08                 | PL  | ... | 3     | 2FGL J0059.7–5700                                                                | ... | bcu   | PKS 0056–572             |
| J0059.2–0152  | 14.808 | –1.883  | 127.492 | –64.686 | 0.070      | 0.067      | 32     | 6.0      | 0.3      | 0.1             | 3.4      | 0.9             | 1.74          | 0.20                 | PL  | ... | ...   | 2FGL J0059.2–0151                                                                | ... | bll   | 1RXS<br>J005916.3–015030 |
| J0059.6+0003  | 14.905 | 0.052   | 127.404 | –62.749 | 0.233      | 0.193      | –54    | 4.5      | 0.3      | 0.1             | 3.8      | 0.8             | 2.48          | 0.16                 | PL  | ... | ...   | ...                                                                              | ... | fsrq  | PKS 0056–00              |
| J0100.2+0745  | 15.068 | 7.766   | 126.753 | –55.040 | 0.030      | 0.029      | –69    | 23.1     | 1.6      | 0.1             | 19.3     | 1.8             | 1.80          | 0.05                 | PL  | T   | ...   | 1FHL J0100.2+0747<br>2FGL J0100.2+0746<br>1FGL J0100.2+0747<br>0FGL J0100.2+0750 | ... | bll   | GB6 J0100+0745           |
| J0101.0–6422  | 15.271 | –64.373 | 301.210 | –52.723 | 0.040      | 0.040      | –64    | 26.9     | 1.9      | 0.1             | 12.5     | 0.9             | 2.16          | ...                  | EC  | ... | ...   | 2FGL J0101.2–6425<br>1FGL J0101.0–6423                                           | ... | PSR   | PSR J0101–6422           |
| J0102.1+4458  | 15.537 | 44.972  | 124.922 | –17.859 | 0.175      | 0.121      | 42     | 4.1      | 0.3      | 0.1             | 3.0      | 0.8             | 2.27          | 0.21                 | PL  | ... | ...   | ...                                                                              | ... | ...   | ...                      |
| J0102.1+0943  | 15.540 | 9.728   | 127.331 | –53.052 | 0.082      | 0.067      | –53    | 7.1      | 0.5      | 0.1             | 5.2      | 0.9             | 2.07          | 0.13                 | PL  | ... | 9     | 2FGL J0102.2+0943<br>1FGL J0102.3+0942                                           | ... | ...   | ...                      |
| J0102.3+4217  | 15.595 | 42.289  | 125.093 | –20.537 | 0.124      | 0.108      | 10     | 12.7     | 0.5      | 0.1             | 10.0     | 0.9             | 2.69          | 0.08                 | PL  | T   | ...   | 2FGL J0102.3+4216                                                                | ... | fsrq  | GB6 J0102+4214           |

Table 1—Continued

| Name 3FGL    | R.A.   | Decl.   | $l$     | $b$     | $\theta_1$ | $\theta_2$ | $\phi$ | $\sigma$ | $F_{35}$ | $\Delta F_{35}$ | $S_{25}$ | $\Delta S_{25}$ | $\Gamma_{25}$ | $\Delta \Gamma_{25}$ | Mod | Var | Flags | $\gamma$ -ray Assoc.                                        | TeV | Class | ID or Assoc.             |
|--------------|--------|---------|---------|---------|------------|------------|--------|----------|----------|-----------------|----------|-----------------|---------------|----------------------|-----|-----|-------|-------------------------------------------------------------|-----|-------|--------------------------|
| J0102.8+4840 | 15.701 | 48.673  | 124.867 | -14.156 | 0.038      | 0.036      | 27     | 20.3     | 2.2      | 0.2             | 16.8     | 1.4             | 2.20          | ...                  | EC  | ... | ...   | 1FGL J0102.2+4223<br>2FGL J0102.9+4838                      | ... | PSR   | PSR J0102+4839           |
| J0102.8+5825 | 15.704 | 58.424  | 124.426 | -4.414  | 0.020      | 0.019      | 1      | 51.5     | 6.2      | 0.2             | 59.5     | 1.9             | 2.25          | ...                  | LP  | T   | ...   | 1FGL J0103.1+4840<br>2FGL J0102.7+5827                      | ... | fsrq  | TXS 0059+581             |
| J0103.4+5336 | 15.864 | 53.615  | 124.737 | -9.214  | 0.045      | 0.040      | -50    | 10.4     | 0.7      | 0.1             | 7.6      | 1.0             | 2.04          | 0.10                 | PL  | ... | ...   | 1FGL J0102.8+5827<br>1FHL J0103.4+5336                      | ... | bll   | 1RXS<br>J010325.9+533721 |
| J0103.7+1323 | 15.941 | 13.392  | 127.539 | -49.369 | 0.082      | 0.068      | -48    | 7.1      | 0.4      | 0.1             | 4.3      | 0.8             | 1.98          | 0.14                 | PL  | ... | ...   | 2FGL J0103.5+5336<br>2FGL J0103.8+1324                      | ... | bcu   | NVSS<br>J010345+132346   |
| J0105.1-2415 | 16.291 | -24.259 | 170.832 | -85.783 | 0.119      | 0.102      | 32     | 13.2     | 0.5      | 0.1             | 9.2      | 0.8             | 2.61          | 0.08                 | PL  | T   | ...   | 1FGL J0105.0-2411<br>1FGL J0104.4-2406                      | ... | fsrq  | PKS 0102-245             |
| J0105.3+3928 | 16.330 | 39.472  | 125.850 | -23.321 | 0.092      | 0.083      | -84    | 8.1      | 0.4      | 0.1             | 5.5      | 0.8             | 2.33          | 0.11                 | PL  | ... | ...   | 2FGL J0105.3+3930<br>1FGL J0105.7+3930                      | ... | bll   | GB6 J0105+3928           |
| J0106.5+4855 | 16.627 | 48.924  | 125.481 | -13.873 | 0.034      | 0.032      | -17    | 27.5     | 3.4      | 0.2             | 19.1     | 1.4             | 2.11          | ...                  | EC  | ... | ...   | 2FGL J0106.5+4854<br>1FGL J0106.7+4853                      | ... | PSR   | LAT PSR J0106+4855       |
| J0107.0-1208 | 16.770 | -12.142 | 137.448 | -74.572 | 0.123      | 0.107      | -59    | 5.1      | 0.3      | 0.1             | 3.3      | 0.8             | 2.18          | 0.17                 | PL  | ... | ...   | ...                                                         | ... | bcu   | PMN J0107+1211           |
| J0108.5-0035 | 17.140 | -0.594  | 132.444 | -63.149 | 0.233      | 0.200      | 81     | 4.2      | 0.3      | 0.1             | 3.5      | 0.8             | 2.39          | 0.17                 | PL  | ... | ...   | ...                                                         | ... | fsrq  | PKS 0105-008             |
| J0108.7+0134 | 17.180 | 1.579   | 131.868 | -60.992 | 0.026      | 0.025      | -88    | 71.7     | 5.3      | 0.2             | 63.8     | 1.7             | 2.39          | ...                  | LP  | T   | ...   | 1FHL J0108.4+0134<br>2FGL J0108.6+0135                      | ... | fsrq  | 4C +01.02                |
| J0109.1+1816 | 17.278 | 18.270  | 128.810 | -44.400 | 0.047      | 0.043      | -66    | 10.5     | 0.6      | 0.1             | 6.3      | 0.9             | 2.04          | 0.11                 | PL  | ... | ...   | 1FGL J0108.6+0135<br>2FGL J0109.0+1817                      | ... | bll   | MG1 J010908+1816         |
| J0109.8+6132 | 17.468 | 61.549  | 125.127 | -1.244  | 0.033      | 0.032      | -6     | 36.5     | 3.6      | 0.2             | 50.9     | 1.8             | 2.54          | ...                  | LP  | T   | ...   | 1FGL J0109.0+1816<br>2FGL J0109.9+6132                      | ... | fsrq  | TXS 0106+612             |
| J0109.9-4020 | 17.482 | -40.334 | 287.950 | -76.252 | 0.052      | 0.046      | 84     | 7.7      | 0.3      | 0.1             | 3.5      | 0.9             | 1.73          | 0.16                 | PL  | ... | ...   | 1FHL J0110.0-4023<br>1FGL J0110.0-4023                      | ... | bll   | RBS 0158                 |
| J0110.2+6806 | 17.575 | 68.115  | 124.696 | 5.308   | 0.025      | 0.022      | -14    | 19.9     | 1.9      | 0.2             | 21.5     | 1.7             | 1.99          | 0.06                 | PL  | ... | ...   | 1FHL J0110.3+6805<br>2FGL J0110.3+6805                      | ... | bll   | 4C +67.04                |
| J0110.9-1254 | 17.735 | -12.913 | 141.688 | -75.069 | 0.081      | 0.069      | -57    | 5.8      | 0.3      | 0.1             | 3.3      | 0.8             | 1.93          | 0.19                 | PL  | ... | ...   | 1FGL J0110.0+6806<br>...                                    | ... | bll   | 1RXS<br>J011050.0-125455 |
| J0111.5+0535 | 17.877 | 5.586   | 132.112 | -56.928 | 0.083      | 0.078      | 7      | 5.2      | 0.3      | 0.1             | 2.9      | 0.8             | 1.92          | 0.19                 | PL  | ... | ...   | ...                                                         | ... | bll   | 1RXS<br>J011130.5+053612 |
| J0112.1+2245 | 18.027 | 22.759  | 129.144 | -39.863 | 0.016      | 0.015      | 18     | 81.1     | 8.7      | 0.2             | 77.8     | 2.7             | 2.03          | ...                  | LP  | T   | ...   | 1FHL J0112.0+2244<br>2FGL J0112.1+2245                      | ... | BLL   | S2 0109+22               |
| J0112.8+3207 | 18.210 | 32.127  | 128.193 | -30.526 | 0.028      | 0.026      | -85    | 44.5     | 3.0      | 0.1             | 38.7     | 1.3             | 2.36          | 0.03                 | PL  | T   | ...   | 1FGL J0112.0+2247<br>0FGL J0112.1+2247<br>1FHL J0112.9+3207 | ... | fsrq  | 4C +31.03                |
|              |        |         |         |         |            |            |        |          |          |                 |          |                 |               |                      |     |     |       | 2FGL J0112.8+3208                                           |     |       |                          |

Table 1—Continued

| Name 3FGL    | R.A.   | Decl.   | $l$     | $b$     | $\theta_1$ | $\theta_2$ | $\phi$ | $\sigma$ | $F_{35}$ | $\Delta F_{35}$ | $S_{25}$ | $\Delta S_{25}$ | $\Gamma_{25}$ | $\Delta \Gamma_{25}$ | Mod | Var | Flags | $\gamma$ -ray Assoc. | TeV | Class | ID or Assoc.             |
|--------------|--------|---------|---------|---------|------------|------------|--------|----------|----------|-----------------|----------|-----------------|---------------|----------------------|-----|-----|-------|----------------------|-----|-------|--------------------------|
|              |        |         |         |         |            |            |        |          |          |                 |          |                 |               |                      |     |     |       | 1FGL J0112.9+3207    |     |       |                          |
| J0112.9–7506 | 18.244 | –75.105 | 301.074 | –41.945 | 0.121      | 0.098      | 9      | 5.4      | 0.3      | 0.1             | 3.3      | 0.7             | 2.17          | 0.17                 | PL  | ... | ...   | ...                  | ... | ...   | ...                      |
| J0113.0–3554 | 18.256 | –35.901 | 276.632 | –80.098 | 0.126      | 0.101      | 14     | 7.7      | 0.3      | 0.1             | 4.7      | 0.7             | 2.50          | 0.12                 | PL  | T   | ...   | 2FGL J0113.2–3557    | ... | fsrq  | PMN J0113–3551           |
| J0113.4+4948 | 18.372 | 49.815  | 126.579 | –12.901 | 0.054      | 0.049      | –34    | 12.2     | 0.9      | 0.1             | 10.4     | 1.1             | 2.30          | 0.08                 | PL  | ... | ...   | 2FGL J0113.7+4948    | ... | fsrq  | S4 0110+49               |
|              |        |         |         |         |            |            |        |          |          |                 |          |                 |               |                      |     |     |       | 1FGL J0113.8+4945    |     |       |                          |
| J0114.8+1917 | 18.710 | 19.295  | 130.520 | –43.232 | 0.149      | 0.122      | –86    | 4.1      | 0.2      | 0.1             | 2.9      | 0.8             | 2.31          | 0.23                 | PL  | ... | ...   | ...                  | ... | ...   | ...                      |
| J0114.8+1326 | 18.716 | 13.434  | 131.641 | –49.041 | 0.044      | 0.041      | –88    | 19.0     | 1.3      | 0.1             | 14.5     | 1.2             | 2.08          | 0.06                 | PL  | T   | ...   | 2FGL J0114.7+1326    | ... | bll   | GB6 J0114+1325           |
|              |        |         |         |         |            |            |        |          |          |                 |          |                 |               |                      |     |     |       | 1FGL J0114.4+1327    |     |       |                          |
| J0115.7+0356 | 18.937 | 3.941   | 134.555 | –58.381 | 0.045      | 0.044      | 18     | 17.5     | 1.2      | 0.1             | 13.4     | 1.2             | 2.12          | 0.06                 | PL  | ... | ...   | 2FGL J0115.4+0358    | ... | bll   | PMN J0115+0356           |
|              |        |         |         |         |            |            |        |          |          |                 |          |                 |               |                      |     |     |       | 1FGL J0115.7+0357    |     |       |                          |
|              |        |         |         |         |            |            |        |          |          |                 |          |                 |               |                      |     |     |       | EGR J0117+0254       |     |       |                          |
| J0115.8+2519 | 18.955 | 25.330  | 129.855 | –37.214 | 0.029      | 0.028      | –0     | 17.0     | 1.2      | 0.1             | 12.9     | 1.3             | 1.99          | 0.08                 | PL  | ... | ...   | 1FHL J0115.6+2520    | ... | bll   | RX J0115.7+2519          |
|              |        |         |         |         |            |            |        |          |          |                 |          |                 |               |                      |     |     |       | 2FGL J0115.7+2518    |     |       |                          |
|              |        |         |         |         |            |            |        |          |          |                 |          |                 |               |                      |     |     |       | 1FGL J0115.5+2519    |     |       |                          |
| J0116.0–1134 | 19.013 | –11.578 | 144.514 | –73.410 | 0.062      | 0.059      | –68    | 19.9     | 1.2      | 0.1             | 15.1     | 1.0             | 2.34          | 0.05                 | PL  | T   | ...   | 2FGL J0116.0–1134    | ... | fsrq  | PKS 0113–118             |
|              |        |         |         |         |            |            |        |          |          |                 |          |                 |               |                      |     |     |       | 1FGL J0115.5–1132    |     |       | $\infty$                 |
| J0116.2–2744 | 19.066 | –27.740 | 220.697 | –84.458 | 0.082      | 0.075      | 42     | 5.5      | 0.3      | 0.1             | 3.1      | 0.7             | 2.02          | 0.17                 | PL  | ... | ...   | ...                  | ... | bcu   | 1RXS<br>J011555.6–274428 |
| J0116.3–6153 | 19.099 | –61.891 | 297.811 | –54.989 | 0.044      | 0.040      | 36     | 9.9      | 0.4      | 0.1             | 4.7      | 0.8             | 1.96          | 0.13                 | PL  | ... | ...   | 2FGL J0116.6–6153    | ... | bll   | SUMSS<br>J011619–615343  |
| J0116.8+6913 | 19.220 | 69.228  | 125.198 | 6.468   | 0.434      | 0.228      | –71    | 5.1      | 0.4      | 0.1             | 8.7      | 1.6             | 2.76          | 0.13                 | PL  | ... | 5     | ...                  | ... | ...   | ...                      |
| J0117.8–2113 | 19.452 | –21.218 | 169.830 | –81.571 | 0.087      | 0.069      | –0     | 9.4      | 0.8      | 0.1             | 10.4     | 1.5             | 2.32          | 0.10                 | PL  | ... | 5     | ...                  | ... | fsrq  | PKS 0115–214             |
| J0118.8–2142 | 19.707 | –21.708 | 173.394 | –81.741 | 0.036      | 0.034      | –59    | 28.4     | 3.0      | 0.2             | 28.5     | 1.8             | 2.28          | ...                  | LP  | T   | ...   | 0FGL J0118.7–2139    | ... | fsrq  | PKS 0116–219             |
|              |        |         |         |         |            |            |        |          |          |                 |          |                 |               |                      |     |     |       | 1FGL J0118.7–2137    |     |       |                          |
|              |        |         |         |         |            |            |        |          |          |                 |          |                 |               |                      |     |     |       | 2FGL J0118.8–2142    |     |       |                          |
| J0118.9–1457 | 19.730 | –14.964 | 152.044 | –76.257 | 0.068      | 0.066      | 67     | 7.3      | 0.3      | 0.1             | 3.7      | 0.9             | 1.79          | 0.16                 | PL  | ... | ...   | 1FHL J0118.5–1502    | ... | bll   | 1RXS<br>J011905.4–145906 |
| J0120.4–2700 | 20.124 | –27.015 | 213.585 | –83.531 | 0.021      | 0.020      | –9     | 45.6     | 3.7      | 0.2             | 42.4     | 2.2             | 1.91          | 0.03                 | PL  | T   | ...   | 1FHL J0120.4–2701    | ... | bll   | PKS 0118–272             |
|              |        |         |         |         |            |            |        |          |          |                 |          |                 |               |                      |     |     |       | 2FGL J0120.4–2700    |     |       |                          |
|              |        |         |         |         |            |            |        |          |          |                 |          |                 |               |                      |     |     |       | 1FGL J0120.5–2700    |     |       |                          |
|              |        |         |         |         |            |            |        |          |          |                 |          |                 |               |                      |     |     |       | 0FGL J0120.5–2703    |     |       |                          |
| J0121.7+5154 | 20.449 | 51.905  | 127.689 | –10.686 | 0.051      | 0.050      | –52    | 6.6      | 0.5      | 0.1             | 5.1      | 1.0             | 1.98          | 0.14                 | PL  | ... | ...   | 1FGL J0122.2+5200    | ... | bcu   | NVSS<br>J012133+515557   |
| J0121.8–3917 | 20.457 | –39.286 | 277.343 | –76.294 | 0.071      | 0.063      | 53     | 5.5      | 0.2      | 0.1             | 2.4      | 0.7             | 1.80          | 0.20                 | PL  | ... | ...   | ...                  | ... | ...   | ...                      |
| J0122.8+3423 | 20.723 | 34.391  | 130.281 | –28.031 | 0.049      | 0.039      | –55    | 9.6      | 0.3      | 0.1             | 5.4      | 1.2             | 1.48          | 0.15                 | PL  | ... | ...   | 1FHL J0122.7+3425    | ... | bll   | 1ES 0120+340             |
|              |        |         |         |         |            |            |        |          |          |                 |          |                 |               |                      |     |     |       | 2FGL J0122.6+3425    |     |       |                          |
| J0123.7–2312 | 20.928 | –23.203 | 186.436 | –81.712 | 0.087      | 0.061      | –57    | 11.1     | 0.7      | 0.1             | 7.3      | 1.0             | 1.99          | 0.10                 | PL  | ... | ...   | ...                  | ... | bll   | 1RXS<br>J012338.2–231100 |
| J0125.2–0627 | 21.316 | –6.458  | 145.706 | –67.821 | 0.209      | 0.127      | –82    | 5.5      | 0.4      | 0.1             | 4.1      | 0.8             | 2.21          | 0.13                 | PL  | ... | ...   | 2FGL J0124.5–0621    | ... | bll   | PMN J0124–0624           |
|              |        |         |         |         |            |            |        |          |          |                 |          |                 |               |                      |     |     |       | 1FGL J0124.6–0616    |     |       |                          |



Table 1—Continued

| Name 3FGL    | R.A.   | Decl.   | $l$     | $b$     | $\theta_1$ | $\theta_2$ | $\phi$ | $\sigma$ | $F_{35}$ | $\Delta F_{35}$ | $S_{25}$ | $\Delta S_{25}$ | $\Gamma_{25}$ | $\Delta \Gamma_{25}$ | Mod | Var | Flags | $\gamma$ -ray Assoc. | TeV | Class | ID or Assoc.             |
|--------------|--------|---------|---------|---------|------------|------------|--------|----------|----------|-----------------|----------|-----------------|---------------|----------------------|-----|-----|-------|----------------------|-----|-------|--------------------------|
| J0125.4–2548 | 21.366 | –25.809 | 205.023 | –82.274 | 0.093      | 0.079      | 64     | 8.7      | 0.5      | 0.1             | 5.1      | 0.8             | 2.13          | 0.11                 | PL  | T   | ...   | ...                  | ... | bll   | PKS 0122–260             |
| J0126.1–2227 | 21.530 | –22.464 | 184.161 | –80.855 | 0.099      | 0.088      | 64     | 10.3     | 0.6      | 0.1             | 8.3      | 1.0             | 2.43          | 0.09                 | PL  | T   | ...   | ...                  | ... | fsrq  | PKS 0123–226             |
| J0127.1–0818 | 21.777 | –8.311  | 148.745 | –69.375 | 0.079      | 0.064      | –22    | 10.6     | 0.6      | 0.1             | 7.2      | 0.9             | 2.21          | 0.09                 | PL  | ... | ...   | ...                  | ... | bll   | PMN J0127–0821           |
| J0127.2+0325 | 21.810 | 3.423   | 140.098 | –58.251 | 0.054      | 0.050      | –47    | 14.4     | 0.9      | 0.1             | 10.3     | 1.2             | 1.90          | 0.08                 | PL  | ... | ...   | 2FGL J0127.2+0324    | ... | bcu   | NVSS<br>J012713+032259   |
|              |        |         |         |         |            |            |        |          |          |                 |          |                 |               |                      |     |     |       | 1FGL J0127.0+0322    |     |       |                          |
| J0127.4+5433 | 21.869 | 54.555  | 128.194 | –7.949  | 0.177      | 0.098      | 37     | 4.6      | 0.4      | 0.1             | 5.6      | 1.2             | 2.53          | 0.16                 | PL  | ... | ...   | ...                  | ... | ...   | ...                      |
| J0127.5+5634 | 21.894 | 56.569  | 127.923 | –5.953  | 0.118      | 0.105      | 21     | 5.8      | 0.5      | 0.1             | 8.2      | 1.3             | 2.59          | 0.12                 | PL  | ... | ...   | ...                  | ... | ...   | ...                      |
| J0127.6+4851 | 21.924 | 48.861  | 129.054 | –13.579 | 0.146      | 0.109      | –74    | 5.0      | 0.3      | 0.1             | 4.5      | 1.0             | 2.45          | 0.15                 | PL  | ... | ...   | ...                  | ... | ...   | ...                      |
| J0127.9+2551 | 21.978 | 25.855  | 133.125 | –36.294 | 0.418      | 0.382      | –24    | 7.1      | 0.2      | 0.1             | 7.3      | 1.0             | 3.10          | 0.15                 | PL  | ... | ...   | ...                  | ... | fsrq  | 4C +25.05                |
| J0128.4+6257 | 22.116 | 62.962  | 127.126 | 0.392   | 0.126      | 0.098      | 40     | 8.3      | 1.0      | 0.1             | 14.5     | 1.8             | 2.50          | 0.08                 | PL  | ... | ...   | ...                  | ... | spp   | ...                      |
| J0128.5+4430 | 22.129 | 44.507  | 129.865 | –17.865 | 0.220      | 0.112      | 15     | 7.5      | 0.5      | 0.1             | 6.0      | 0.9             | 2.33          | 0.11                 | PL  | T   | ...   | 2FGL J0128.4+4431    | ... | fsrq  | GB6 J0128+4439           |
|              |        |         |         |         |            |            |        |          |          |                 |          |                 |               |                      |     |     |       | 1FGL J0128.6+4439    |     |       |                          |
| J0130.8+1441 | 22.718 | 14.684  | 137.016 | –47.106 | 0.371      | 0.273      | 86     | 4.3      | 0.2      | 0.1             | 4.1      | 0.9             | 2.65          | 0.17                 | PL  | ... | ...   | ...                  | ... | fsrq  | 4C +14.06                |
| J0131.2+6120 | 22.801 | 61.335  | 127.684 | –1.169  | 0.022      | 0.022      | –1     | 21.3     | 2.0      | 0.2             | 23.7     | 1.9             | 1.86          | 0.06                 | PL  | T   | ...   | 1FHL J0131.3+6121    | ... | bll   | 1RXS<br>J013106.4+612035 |
|              |        |         |         |         |            |            |        |          |          |                 |          |                 |               |                      |     |     |       | 2FGL J0131.1+6121    |     |       |                          |
|              |        |         |         |         |            |            |        |          |          |                 |          |                 |               |                      |     |     |       | 1FGL J0131.2+6121    |     |       |                          |
| J0131.3+5548 | 22.835 | 55.807  | 128.556 | –6.628  | 0.093      | 0.073      | –33    | 4.9      | 0.3      | 0.1             | 4.0      | 1.0             | 1.90          | 0.21                 | PL  | ... | ...   | ...                  | ... | bcu   | TXS 0128+554             |
| J0132.1–5340 | 23.045 | –53.674 | 289.860 | –62.409 | 0.148      | 0.141      | 64     | 4.5      | 0.2      | 0.1             | 3.0      | 0.7             | 2.32          | 0.19                 | PL  | ... | ...   | ...                  | ... | ...   | ...                      |
| J0132.5–0802 | 23.135 | –8.050  | 151.858 | –68.581 | 0.137      | 0.114      | 86     | 4.5      | 0.2      | 0.1             | 3.0      | 0.9             | 1.75          | 0.18                 | PL  | ... | ...   | ...                  | ... | bcu   | PKS 0130–083             |
| J0132.6–1655 | 23.171 | –16.918 | 168.106 | –76.027 | 0.041      | 0.041      | –66    | 34.6     | 1.9      | 0.1             | 26.2     | 1.1             | 2.43          | 0.04                 | PL  | T   | ...   | 1FHL J0132.6–1651    | ... | fsrq  | PKS 0130–17              |
|              |        |         |         |         |            |            |        |          |          |                 |          |                 |               |                      |     |     |       | 2FGL J0132.8–1654    |     |       |                          |
|              |        |         |         |         |            |            |        |          |          |                 |          |                 |               |                      |     |     |       | 1FGL J0132.6–1655    |     |       |                          |
| J0133.0–4413 | 23.252 | –44.232 | 279.585 | –70.964 | 0.095      | 0.084      | –38    | 7.7      | 0.4      | 0.1             | 4.2      | 0.7             | 2.16          | 0.12                 | PL  | ... | ...   | 2FGL J0133.4–4408    | ... | bll   | SUMSS<br>J013306–441422  |
| J0133.2–4737 | 23.307 | –47.620 | 283.941 | –67.938 | 0.285      | 0.213      | –87    | 4.2      | 0.2      | 0.1             | 3.1      | 0.7             | 2.71          | 0.20                 | PL  | ... | ...   | ...                  | ... | ...   | ...                      |
| J0133.2–5159 | 23.320 | –51.987 | 288.193 | –63.928 | 0.134      | 0.123      | 81     | 4.5      | 0.2      | 0.1             | 3.3      | 0.7             | 2.63          | 0.19                 | PL  | ... | ...   | ...                  | ... | bcu   | PKS 0131–522             |
| J0133.3+5930 | 23.336 | 59.514  | 128.232 | –2.926  | 0.108      | 0.085      | 22     | 4.3      | 0.4      | 0.1             | 4.9      | 1.2             | 2.21          | 0.16                 | PL  | ... | ...   | ...                  | ... | ...   | ...                      |
| J0133.3+4324 | 23.338 | 43.403  | 130.957 | –18.815 | 0.156      | 0.127      | 7      | 5.0      | 0.3      | 0.1             | 3.9      | 0.8             | 2.30          | 0.14                 | PL  | ... | ...   | ...                  | ... | bcu   | B3 0129+431              |
| J0134.3–3842 | 23.577 | –38.705 | 267.882 | –75.361 | 0.101      | 0.090      | –49    | 6.9      | 0.3      | 0.1             | 3.9      | 0.7             | 2.33          | 0.14                 | PL  | ... | ...   | ...                  | ... | fsrq  | PMN J0134–3843           |
| J0134.5+2638 | 23.630 | 26.638  | 134.735 | –35.245 | 0.063      | 0.055      | 67     | 12.0     | 0.8      | 0.1             | 9.4      | 1.2             | 1.99          | 0.08                 | PL  | ... | ...   | 1FHL J0134.4+2643    | ... | bcu   | 1RXS<br>J013427.2+263846 |
|              |        |         |         |         |            |            |        |          |          |                 |          |                 |               |                      |     |     |       | 2FGL J0134.4+2636    |     |       |                          |
|              |        |         |         |         |            |            |        |          |          |                 |          |                 |               |                      |     |     |       | 1FGL J0134.4+2632    |     |       |                          |
| J0135.0+6927 | 23.755 | 69.466  | 126.762 | 6.919   | 0.100      | 0.091      | –47    | 4.9      | 0.4      | 0.1             | 6.7      | 1.4             | 2.56          | 0.13                 | PL  | ... | 4     | ...                  | ... | bcu   | TXS 0130+691             |
| J0136.5+3905 | 24.131 | 39.096  | 132.413 | –22.944 | 0.014      | 0.013      | 44     | 56.9     | 4.9      | 0.2             | 66.1     | 3.3             | 1.70          | 0.02                 | PL  | ... | ...   | 1FHL J0136.5+3906    | P   | bll   | B3 0133+388              |
|              |        |         |         |         |            |            |        |          |          |                 |          |                 |               |                      |     |     |       | 2FGL J0136.5+3905    |     |       |                          |
|              |        |         |         |         |            |            |        |          |          |                 |          |                 |               |                      |     |     |       | 1FGL J0136.5+3905    |     |       |                          |

Table 1—Continued

| Name 3FGL    | R.A.   | Decl.   | $l$     | $b$     | $\theta_1$ | $\theta_2$ | $\phi$ | $\sigma$ | $F_{35}$ | $\Delta F_{35}$ | $S_{25}$ | $\Delta S_{25}$ | $\Gamma_{25}$ | $\Delta \Gamma_{25}$ | Mod | Var | Flags | $\gamma$ -ray Assoc.                                                                                  | TeV | Class | ID or Assoc.             |
|--------------|--------|---------|---------|---------|------------|------------|--------|----------|----------|-----------------|----------|-----------------|---------------|----------------------|-----|-----|-------|-------------------------------------------------------------------------------------------------------|-----|-------|--------------------------|
| J0137.0+4752 | 24.257 | 47.876  | 130.794 | -14.298 | 0.023      | 0.022      | 5      | 55.9     | 5.1      | 0.2             | 51.1     | 1.7             | 2.27          | ...                  | LP  | T   | ...   | 0FGL J0136.6+3903<br>1FHL J0136.8+4754<br>2FGL J0136.9+4751<br>1FGL J0137.0+4751<br>0FGL J0137.1+4751 | ... | fsrq  | OC 457                   |
| J0137.6-2430 | 24.415 | -24.510 | 201.377 | -79.278 | 0.058      | 0.054      | 89     | 22.5     | 1.0      | 0.1             | 15.3     | 0.9             | 2.52          | 0.05                 | PL  | T   | ...   | 2FGL J0137.6-2430<br>1FGL J0137.5-2428                                                                | ... | fsrq  | PKS 0135-247             |
| J0137.8+5813 | 24.458 | 58.232  | 129.024 | -4.090  | 0.034      | 0.030      | 68     | 13.5     | 1.2      | 0.1             | 12.9     | 1.4             | 2.06          | 0.08                 | PL  | ... | ...   | 1FHL J0137.7+5812<br>2FGL J0137.7+5811<br>1FGL J0137.8+5814                                           | ... | bcu   | 1RXS<br>J013748.0+581422 |
| J0138.5-4612 | 24.649 | -46.204 | 279.952 | -68.763 | 0.062      | 0.060      | 42     | 6.8      | 0.3      | 0.1             | 3.6      | 0.7             | 2.06          | 0.15                 | PL  | ... | ...   | ...                                                                                                   | ... | ...   | ...                      |
| J0139.9+8735 | 24.983 | 87.600  | 123.487 | 24.781  | 0.064      | 0.052      | 19     | 5.8      | 0.3      | 0.1             | 3.6      | 0.8             | 1.89          | 0.17                 | PL  | ... | ...   | ...                                                                                                   | ... | bcu   | NVSS<br>J013913+873754   |
| J0141.4-0929 | 25.367 | -9.485  | 159.081 | -68.769 | 0.035      | 0.031      | -64    | 29.5     | 2.1      | 0.1             | 23.1     | 1.4             | 2.12          | 0.04                 | PL  | T   | ...   | 1FHL J0141.5-0927<br>2FGL J0141.5-0928<br>1FGL J0141.7-0929                                           | ... | bll   | PKS 0139-09              |
| J0143.7-5845 | 25.929 | -58.766 | 290.472 | -57.079 | 0.035      | 0.031      | -87    | 19.0     | 1.0      | 0.1             | 11.8     | 1.2             | 1.84          | 0.07                 | PL  | ... | ...   | 1FHL J0143.4-5844<br>2FGL J0143.6-5844<br>1FGL J0143.9-5845                                           | ... | bll   | SUMSS<br>J014347-584550  |
| J0144.6+2705 | 26.157 | 27.089  | 137.284 | -34.296 | 0.021      | 0.020      | 77     | 50.6     | 4.5      | 0.2             | 43.9     | 1.9             | 2.16          | ...                  | LP  | T   | ...   | 1FHL J0144.3+2703<br>2FGL J0144.6+2704<br>1FGL J0144.6+2703<br>0FGL J0144.5+2709                      | ... | bll   | TXS 0141+268             |
| J0145.1-2732 | 26.292 | -27.534 | 217.965 | -78.066 | 0.059      | 0.055      | 27     | 29.5     | 1.4      | 0.1             | 21.8     | 1.0             | 2.57          | 0.04                 | PL  | T   | ...   | 2FGL J0145.1-2732<br>1FGL J0144.9-2732<br>0FGL J0145.1-2728                                           | ... | fsrq  | PKS 0142-278             |
| J0145.6+8600 | 26.415 | 86.002  | 123.951 | 23.238  | 0.125      | 0.110      | 7      | 5.0      | 0.3      | 0.1             | 4.0      | 0.8             | 2.52          | 0.18                 | PL  | ... | ...   | ...                                                                                                   | ... | bcu   | NVSS<br>J014929+860114   |
| J0146.4-6746 | 26.619 | -67.768 | 295.124 | -48.518 | 0.071      | 0.066      | 49     | 6.9      | 0.3      | 0.1             | 4.2      | 0.7             | 2.39          | 0.13                 | PL  | ... | ...   | ...                                                                                                   | ... | bcu   | SUMSS<br>J014554-674646  |
| J0147.0-5204 | 26.766 | -52.078 | 283.976 | -62.954 | 0.082      | 0.073      | 53     | 7.2      | 0.4      | 0.1             | 4.0      | 0.7             | 2.20          | 0.13                 | PL  | ... | ...   | 2FGL J0146.6-5206                                                                                     | ... | bcu   | PKS 0144-522             |
| J0148.3+5200 | 27.085 | 52.010  | 131.765 | -9.883  | 0.040      | 0.039      | -86    | 9.9      | 0.5      | 0.1             | 6.7      | 1.1             | 1.77          | 0.11                 | PL  | ... | ...   | ...                                                                                                   | ... | bcu   | GB6 J0148+5202           |
| J0148.6+0128 | 27.161 | 1.474   | 150.924 | -58.254 | 0.054      | 0.050      | 85     | 9.8      | 0.6      | 0.1             | 6.6      | 1.0             | 2.02          | 0.13                 | PL  | ... | ...   | 2FGL J0148.6+0127                                                                                     | ... | bll   | PMN J0148+0129           |
| J0149.6+4846 | 27.421 | 48.769  | 132.724 | -12.992 | 0.110      | 0.100      | 26     | 5.1      | 0.3      | 0.1             | 4.7      | 1.0             | 2.62          | 0.18                 | PL  | ... | 1,4   | ...                                                                                                   | ... | ...   | ...                      |
| J0150.5-5447 | 27.626 | -54.788 | 285.668 | -60.316 | 0.088      | 0.082      | 2      | 4.6      | 0.2      | 0.1             | 2.3      | 0.6             | 2.12          | 0.23                 | PL  | ... | ...   | ...                                                                                                   | ... | bcu   | PMN J0150-5450           |
| J0151.0-3609 | 27.760 | -36.156 | 252.125 | -74.461 | 0.233      | 0.171      | -80    | 5.3      | 0.2      | 0.1             | 3.3      | 0.7             | 2.46          | 0.18                 | PL  | ... | 1     | ...                                                                                                   | ... | bcu   | PMN J0151-3605           |
| J0151.0+0537 | 27.761 | 5.627   | 148.886 | -54.213 | 0.117      | 0.113      | -43    | 4.4      | 0.3      | 0.1             | 3.3      | 0.8             | 2.36          | 0.20                 | PL  | ... | ...   | ...                                                                                                   | ... | bcu   | PMN J0151+0540           |
| J0151.6+2205 | 27.917 | 22.092  | 140.890 | -38.670 | 0.218      | 0.145      | 58     | 7.3      | 0.4      | 0.1             | 6.6      | 0.9             | 2.65          | 0.11                 | PL  | ... | ...   | ...                                                                                                   | ... | fsrq  | PKS 0149+21              |

Table 1—Continued

| Name 3FGL    | R.A.   | Decl.   | $l$     | $b$     | $\theta_1$ | $\theta_2$ | $\phi$ | $\sigma$ | $F_{35}$ | $\Delta F_{35}$ | $S_{25}$ | $\Delta S_{25}$ | $\Gamma_{25}$ | $\Delta \Gamma_{25}$ | Mod | Var | Flags | $\gamma$ -ray Assoc.                                        | TeV | Class | ID or Assoc.               |
|--------------|--------|---------|---------|---------|------------|------------|--------|----------|----------|-----------------|----------|-----------------|---------------|----------------------|-----|-----|-------|-------------------------------------------------------------|-----|-------|----------------------------|
| J0152.2+3707 | 28.072 | 37.132  | 136.188 | -24.168 | 0.133      | 0.104      | 19     | 5.6      | 0.3      | 0.1             | 4.0      | 0.8             | 2.41          | 0.14                 | PL  | ... | ...   | ...                                                         | ... | bcu   | B2 0149+37                 |
| J0152.6+0148 | 28.162 | 1.808   | 152.357 | -57.525 | 0.040      | 0.037      | 22     | 13.1     | 0.8      | 0.1             | 8.9      | 1.2             | 1.89          | 0.10                 | PL  | ... | ...   | 1FHL J0152.6+0148<br>2FGL J0152.6+0148                      | P   | bll   | PMN J0152+0146             |
| J0152.8+7517 | 28.216 | 75.290  | 126.888 | 12.892  | 0.038      | 0.036      | -54    | 8.4      | 0.4      | 0.1             | 4.8      | 0.9             | 1.77          | 0.13                 | PL  | ... | ...   | 1FHL J0153.1+7515                                           | ... | bll   | 1RXS<br>J015308.4+751756   |
| J0153.4+7114 | 28.360 | 71.242  | 127.924 | 8.973   | 0.038      | 0.035      | 71     | 7.1      | 0.2      | 0.1             | 3.9      | 1.0             | 1.57          | 0.20                 | PL  | ... | ...   | ...                                                         | ... | bcu   | TXS 0149+710               |
| J0154.0+0824 | 28.510 | 8.410   | 148.235 | -51.360 | 0.029      | 0.028      | 19     | 24.8     | 1.8      | 0.1             | 21.5     | 1.8             | 1.86          | 0.05                 | PL  | ... | ...   | 1FHL J0154.1+0823<br>2FGL J0153.9+0823<br>1FGL J0154.1+0823 | ... | bll   | GB6 J0154+0823             |
| J0154.1+4642 | 28.535 | 46.702  | 133.983 | -14.820 | 0.197      | 0.153      | -52    | 4.3      | 0.2      | 0.1             | 3.9      | 0.9             | 2.55          | 0.18                 | PL  | ... | ...   | ...                                                         | ... | ...   | ...                        |
| J0154.9+4433 | 28.737 | 44.554  | 134.687 | -16.864 | 0.052      | 0.051      | -72    | 7.8      | 0.4      | 0.1             | 5.0      | 0.8             | 2.18          | 0.12                 | PL  | T   | ...   | 2FGL J0154.9+4434<br>1FGL J0155.0+4433                      | ... | bll   | GB6 J0154+4433             |
| J0156.3+3913 | 29.093 | 39.231  | 136.432 | -21.932 | 0.083      | 0.079      | -88    | 11.7     | 0.6      | 0.1             | 8.3      | 0.9             | 2.50          | 0.09                 | PL  | T   | ...   | 2FGL J0156.4+3909                                           | ... | bcu   | MG4 J015630+3913           |
| J0156.5-2423 | 29.128 | -24.392 | 205.982 | -75.106 | 0.119      | 0.095      | -28    | 4.7      | 0.2      | 0.1             | 2.8      | 0.8             | 1.89          | 0.17                 | PL  | ... | ...   | 1FHL J0156.5-2419<br>2FGL J0156.5-2419                      | ... | ...   | ...                        |
| J0156.9-4742 | 29.240 | -47.711 | 275.399 | -65.763 | 0.085      | 0.069      | -52    | 4.6      | 0.2      | 0.1             | 2.0      | 0.6             | 2.01          | 0.26                 | PL  | ... | ...   | ...                                                         | ... | bcu   | 2MASS<br>J01564603-4744174 |
| J0157.0-5301 | 29.251 | -53.027 | 282.180 | -61.379 | 0.046      | 0.043      | 72     | 12.9     | 0.6      | 0.1             | 7.5      | 1.1             | 1.82          | 0.09                 | PL  | ... | ...   | 2FGL J0157.2-5259<br>1FGL J0157.0-5259                      | ... | bll   | 1RXS<br>J015658.6-530208   |
| J0157.9-4615 | 29.481 | -46.260 | 272.813 | -66.788 | 0.137      | 0.110      | 78     | 9.6      | 0.5      | 0.1             | 6.5      | 0.8             | 2.45          | 0.09                 | PL  | T   | ...   | 2FGL J0158.0-4609<br>1FGL J0157.5-4613                      | ... | fsrq  | PMN J0157-4614             |
| J0158.6-3931 | 29.663 | -39.533 | 258.800 | -71.324 | 0.056      | 0.048      | 72     | 14.7     | 0.9      | 0.1             | 9.8      | 1.1             | 2.02          | 0.07                 | PL  | ... | ...   | 2FGL J0158.3-3931<br>1FGL J0158.0-3931                      | ... | bll   | PMN J0158-3932             |
| J0158.6+0102 | 29.673 | 1.041   | 155.512 | -57.513 | 0.072      | 0.066      | -62    | 5.7      | 0.3      | 0.1             | 4.2      | 0.9             | 2.56          | 0.16                 | PL  | ... | ...   | 2FGL J0158.4+0107                                           | ... | ...   | ...                        |
| J0159.4+1046 | 29.862 | 10.781  | 148.709 | -48.657 | 0.051      | 0.047      | -47    | 12.9     | 0.9      | 0.1             | 10.3     | 1.1             | 2.11          | 0.09                 | PL  | ... | ...   | 1FHL J0159.4+1048<br>2FGL J0159.5+1046<br>1FGL J0159.5+1047 | ... | bll   | RX J0159.5+1047            |
| J0159.8-2741 | 29.959 | -27.696 | 219.018 | -74.822 | 0.062      | 0.060      | -27    | 9.2      | 0.5      | 0.1             | 5.1      | 0.8             | 2.04          | 0.10                 | PL  | ... | ...   | 2FGL J0159.6-2741<br>1FGL J0159.7-2741                      | ... | bll   | PMN J0159-2739             |
| J0200.3-4108 | 30.080 | -41.145 | 262.058 | -70.082 | 0.052      | 0.047      | -52    | 7.2      | 0.3      | 0.1             | 3.3      | 0.7             | 1.88          | 0.17                 | PL  | ... | ...   | 2FGL J0200.4-4105                                           | ... | ...   | ...                        |
| J0200.9-6635 | 30.245 | -66.591 | 292.486 | -49.102 | 0.115      | 0.077      | 7      | 6.9      | 0.3      | 0.1             | 4.2      | 0.7             | 2.33          | 0.13                 | PL  | ... | ...   | 2FGL J0201.5-6626                                           | ... | bcu   | PMN J0201-6638             |
| J0202.3+0851 | 30.592 | 8.858   | 150.924 | -50.119 | 0.128      | 0.113      | -33    | 4.4      | 0.3      | 0.1             | 3.1      | 0.8             | 2.05          | 0.16                 | PL  | ... | ...   | 1FGL J0202.1+0849                                           | ... | fsrq  | TXS 0159+085               |
| J0202.5+4206 | 30.633 | 42.113  | 136.776 | -18.840 | 0.090      | 0.080      | 22     | 7.9      | 0.5      | 0.1             | 5.6      | 0.8             | 2.28          | 0.11                 | PL  | ... | ...   | ...                                                         | ... | bll   | B3 0159+418                |
| J0203.1-0227 | 30.795 | -2.456  | 160.826 | -59.940 | 0.139      | 0.130      | -20    | 5.0      | 0.3      | 0.1             | 3.4      | 0.7             | 2.31          | 0.17                 | PL  | ... | ...   | ...                                                         | ... | bcu   | RX J0202.9-0223            |
| J0203.6+1148 | 30.917 | 11.803  | 149.514 | -47.307 | 0.128      | 0.111      | -20    | 5.6      | 0.3      | 0.1             | 6.2      | 1.2             | 2.71          | 0.16                 | PL  | ... | ...   | ...                                                         | ... | ...   | ...                        |
| J0203.6+3043 | 30.923 | 30.717  | 140.792 | -29.636 | 0.034      | 0.030      | -66    | 36.9     | 3.2      | 0.2             | 28.1     | 1.5             | 2.20          | ...                  | LP  | T   | ...   | 1FHL J0203.6+3042<br>2FGL J0204.0+3045                      | ... | bll   | NVSS<br>J020344+304238     |

Table 1—Continued

| Name 3FGL    | R.A.   | Decl.   | $l$     | $b$     | $\theta_1$ | $\theta_2$ | $\phi$ | $\sigma$ | $F_{35}$ | $\Delta F_{35}$ | $S_{25}$ | $\Delta S_{25}$ | $\Gamma_{25}$ | $\Delta \Gamma_{25}$ | Mod | Var | Flags | $\gamma$ -ray Assoc.                                                                                                 | TeV | Class        | ID or Assoc.             |
|--------------|--------|---------|---------|---------|------------|------------|--------|----------|----------|-----------------|----------|-----------------|---------------|----------------------|-----|-----|-------|----------------------------------------------------------------------------------------------------------------------|-----|--------------|--------------------------|
| J0204.0+7234 | 31.003 | 72.578  | 128.373 | 10.478  | 0.051      | 0.039      | 37     | 11.5     | 1.0      | 0.1             | 11.6     | 1.3             | 2.22          | 0.08                 | PL  | ... | 3     | 1FGL J0203.5+3044<br>1FHL J0203.5+7232<br>2FGL J0203.6+7235<br>1FGL J0203.5+7234                                     | ... | bll          | S5 0159+723              |
| J0204.2+2420 | 31.062 | 24.344  | 143.424 | -35.614 | 0.075      | 0.067      | 77     | 5.1      | 0.2      | 0.1             | 3.1      | 0.9             | 1.79          | 0.20                 | PL  | ... | ...   | ...                                                                                                                  | ... | bcu          | B2 0201+24               |
| J0204.8+3212 | 31.223 | 32.202  | 140.531 | -28.147 | 0.164      | 0.136      | 64     | 9.9      | 0.4      | 0.1             | 10.6     | 1.1             | 2.94          | 0.10                 | PL  | T   | ...   | 2FGL J0205.4+3211<br>1FGL J0205.3+3217                                                                               | ... | fsrq         | B2 0202+31               |
| J0205.0+1510 | 31.260 | 15.180  | 148.023 | -44.077 | 0.078      | 0.073      | -2     | 12.3     | 0.7      | 0.1             | 10.3     | 1.0             | 2.53          | 0.08                 | PL  | T   | ...   | 2FGL J0205.0+1514<br>1FGL J0204.5+1516<br>3EG J0204+1458<br>EGR J0204+1505                                           | ... | bcu          | 4C +15.05                |
| J0205.2-1700 | 31.323 | -17.005 | 186.083 | -70.156 | 0.078      | 0.073      | 31     | 24.0     | 0.9      | 0.1             | 18.2     | 0.9             | 2.76          | 0.05                 | PL  | T   | ...   | 2FGL J0205.3-1657<br>1FGL J0205.0-1702<br>0FGL J0204.8-1704                                                          | ... | fsrq         | PKS 0202-17              |
| J0205.5+6448 | 31.396 | 64.815  | 130.719 | 3.070   | 0.026      | 0.025      | -74    | 43.1     | 5.7      | 0.2             | 54.5     | 1.7             | 2.33          | ...                  | EC  | ... | ...   | 1FHL J0205.7+6448<br>2FGL J0205.8+6448<br>1FGL J0205.6+6449                                                          | P   | PSR          | PSR J0205+6449           |
| J0206.4-1150 | 31.606 | -11.849 | 175.604 | -66.700 | 0.063      | 0.060      | -43    | 14.8     | 0.8      | 0.1             | 9.8      | 0.9             | 2.33          | 0.07                 | PL  | T   | ...   | 2FGL J0206.5-1149                                                                                                    | ... | fsrq         | PMN J0206-1150           |
| J0207.9-3846 | 31.985 | -38.775 | 253.862 | -70.240 | 0.236      | 0.142      | 23     | 6.3      | 0.3      | 0.1             | 4.3      | 0.7             | 2.54          | 0.14                 | PL  | ... | ...   | ...                                                                                                                  | bcu | PKS 0205-391 |                          |
| J0208.0-6838 | 32.025 | -68.648 | 292.847 | -46.951 | 0.094      | 0.077      | -27    | 7.9      | 0.4      | 0.1             | 4.9      | 0.8             | 2.42          | 0.12                 | PL  | ... | ...   | 2FGL J0207.9-6832                                                                                                    | ... | bll          | PKS 0206-688             |
| J0208.6+3522 | 32.170 | 35.383  | 140.222 | -24.882 | 0.046      | 0.045      | 37     | 6.0      | 0.2      | 0.1             | 3.2      | 0.9             | 1.70          | 0.19                 | PL  | ... | ...   | 1FHL J0208.7+3523<br>1FGL J0208.6+3522                                                                               | ... | bll          | MS 0205.7+3509           |
| J0209.4-5229 | 32.371 | -52.498 | 278.346 | -60.744 | 0.026      | 0.022      | 85     | 28.1     | 1.7      | 0.1             | 21.1     | 1.7             | 1.80          | 0.05                 | PL  | T   | ...   | 1FHL J0209.6-5230<br>2FGL J0209.5-5229<br>1FGL J0209.3-5229                                                          | ... | bll          | 1RXS<br>J020922.2-522920 |
| J0209.5+4449 | 32.384 | 44.817  | 137.202 | -15.880 | 0.069      | 0.062      | 69     | 6.7      | 0.4      | 0.1             | 3.9      | 0.8             | 1.97          | 0.17                 | PL  | ... | ...   | ...                                                                                                                  | ... | bll          | 1RXS<br>J020917.6+444951 |
| J0210.7-5101 | 32.697 | -51.028 | 276.112 | -61.768 | 0.024      | 0.023      | 42     | 62.9     | 4.7      | 0.2             | 51.1     | 1.5             | 2.30          | ...                  | LP  | T   | ...   | 1FHL J0210.9-5100<br>2FGL J0210.7-5102<br>1FGL J0210.6-5101<br>0FGL J0210.8-5100<br>3EG J0210-5055<br>EGR J0210-5058 | ... | BCU          | PKS 0208-512             |
| J0211.0+1922 | 32.755 | 19.383  | 147.573 | -39.650 | 0.300      | 0.191      | -61    | 4.8      | 0.3      | 0.1             | 4.4      | 0.9             | 2.38          | 0.14                 | PL  | ... | ...   | ...                                                                                                                  | ... | ...          | ...                      |
| J0211.2+1051 | 32.817 | 10.858  | 152.595 | -47.364 | 0.022      | 0.021      | 76     | 50.8     | 5.3      | 0.2             | 47.2     | 2.0             | 2.13          | ...                  | LP  | T   | ...   | 1FHL J0211.3+1051<br>2FGL J0211.2+1050                                                                               | ... | BLL          | MG1 J021114+1051         |

Table 1—Continued

| Name 3FGL     | R.A.   | Decl.   | $l$     | $b$     | $\theta_1$ | $\theta_2$ | $\phi$ | $\sigma$ | $F_{35}$ | $\Delta F_{35}$ | $S_{25}$ | $\Delta S_{25}$ | $\Gamma_{25}$ | $\Delta \Gamma_{25}$ | Mod | Var | Flags | $\gamma$ -ray Assoc. | TeV | Class | ID or Assoc.            |
|---------------|--------|---------|---------|---------|------------|------------|--------|----------|----------|-----------------|----------|-----------------|---------------|----------------------|-----|-----|-------|----------------------|-----|-------|-------------------------|
| J0211.2–0649  | 32.818 | –6.829  | 169.601 | –62.229 | 0.148      | 0.116      | –16    | 5.2      | 0.3      | 0.1             | 3.2      | 0.7             | 2.10          | 0.17                 | PL  | ... | ...   | 1FGL J0211.2+1049    | ... | bcu   | NVSS<br>J021116–064422  |
| J0211.7+5402  | 32.929 | 54.047  | 134.644 | –6.989  | 0.144      | 0.113      | 75     | 4.5      | 0.4      | 0.1             | 6.8      | 1.4             | 2.69          | 0.14                 | PL  | ... | 5     | ...                  | ... | bcu   | TXS 0207+538            |
| J0212.1+5320  | 33.037 | 53.336  | 134.927 | –7.646  | 0.034      | 0.034      | –77    | 25.1     | 2.7      | 0.2             | 17.1     | 1.6             | 2.19          | ...                  | LP  | ... | ...   | 2FGL J0212.1+5318    | ... | ...   | ...                     |
| J0212.8–3504  | 33.207 | –35.068 | 242.494 | –70.902 | 0.075      | 0.070      | –64    | 8.1      | 0.4      | 0.1             | 4.6      | 0.8             | 2.11          | 0.13                 | PL  | ... | ...   | 1FGL J0212.3+5319    | ... | bll   | RBS 0292                |
| J0213.0+2245  | 33.265 | 22.765  | 146.460 | –36.350 | 0.045      | 0.039      | 55     | 13.3     | 0.9      | 0.1             | 10.3     | 1.1             | 2.10          | 0.08                 | PL  | ... | ...   | 1FHL J0213.1+2246    | ... | bll   | MG3 J021252+2246        |
| J0213.1–2720  | 33.286 | –27.349 | 218.335 | –71.857 | 0.135      | 0.107      | 81     | 4.1      | 0.2      | 0.1             | 2.2      | 0.6             | 2.09          | 0.21                 | PL  | ... | ...   | 2FGL J0213.1+2245    | ... | bcu   | PMN J0212–2719          |
| J0214.4+5143  | 33.611 | 51.723  | 135.774 | –9.067  | 0.045      | 0.042      | –14    | 7.2      | 0.4      | 0.1             | 4.6      | 0.9             | 2.04          | 0.18                 | PL  | ... | 10    | 1FGL J0213.2+2244    | ... | bll   | TXS 0210+515            |
| J0214.7–5823  | 33.692 | –58.388 | 283.707 | –55.520 | 0.116      | 0.097      | –18    | 5.7      | 0.2      | 0.1             | 3.8      | 0.7             | 2.57          | 0.16                 | PL  | ... | ...   | ...                  | ... | bcu   | PMN J0214–5822          |
| J0216.0+0300  | 34.013 | 3.016   | 160.324 | –53.598 | 0.092      | 0.077      | 85     | 4.5      | 0.2      | 0.1             | 2.7      | 0.8             | 2.01          | 0.22                 | PL  | ... | ...   | ...                  | ... | ...   | ...                     |
| J0216.1–7016  | 34.042 | –70.273 | 292.968 | –45.180 | 0.118      | 0.108      | 49     | 6.0      | 0.3      | 0.1             | 4.3      | 0.8             | 2.57          | 0.16                 | PL  | ... | ...   | ...                  | ... | bcu   | PMN J0215–7014          |
| J0216.4+0507  | 34.109 | 5.133   | 158.603 | –51.754 | 0.204      | 0.139      | –50    | 4.3      | 0.3      | 0.1             | 3.2      | 0.8             | 2.24          | 0.18                 | PL  | ... | ...   | ...                  | ... | ...   | ...                     |
| J0216.6–1019  | 34.171 | –10.329 | 177.082 | –63.825 | 0.125      | 0.113      | 66     | 6.1      | 0.3      | 0.1             | 4.3      | 0.8             | 2.33          | 0.13                 | PL  | T   | ...   | ...                  | ... | bcu   | PMN J0216–1017          |
| J0217.0–6635  | 34.259 | –66.592 | 290.324 | –48.387 | 0.061      | 0.057      | –2     | 12.1     | 0.7      | 0.1             | 7.4      | 0.9             | 1.98          | 0.09                 | PL  | ... | ...   | 2FGL J0216.9–6630    | ... | bll   | RBS 0300                |
| J0217.1–0833  | 34.286 | –8.566  | 174.448 | –62.517 | 0.208      | 0.151      | –5     | 4.7      | 0.3      | 0.1             | 3.5      | 0.8             | 2.33          | 0.15                 | PL  | ... | ...   | 1FGL J0217.9–6630    | ... | fsrq  | PKS 0214–085            |
| J0217.2+0837  | 34.325 | 8.618   | 156.131 | –48.640 | 0.047      | 0.042      | –82    | 19.3     | 1.5      | 0.1             | 16.8     | 1.3             | 2.10          | 0.06                 | PL  | T   | ...   | 2FGL J0217.5–0813    | ... | bll   | ZS 0214+083             |
| J0217.3+6209  | 34.347 | 62.154  | 132.785 | 0.938   | 0.113      | 0.092      | –23    | 11.5     | 2.3      | 0.3             | 23.5     | 2.6             | 2.47          | ...                  | LP  | ... | 5     | 1FGL J0217.0–0829    | ... | bcu   | TXS 0213+619            |
| J0217.5+7349  | 34.380 | 73.830  | 128.927 | 11.968  | 0.179      | 0.102      | 24     | 15.8     | 0.8      | 0.1             | 20.6     | 1.3             | 2.91          | 0.06                 | PL  | T   | ...   | 1FHL J0217.4+0836    | ... | fsrq  | S5 0212+73              |
| J0217.8+0143  | 34.468 | 1.733   | 162.175 | –54.417 | 0.025      | 0.024      | 29     | 46.3     | 4.0      | 0.2             | 46.2     | 1.7             | 2.19          | 0.03                 | PL  | T   | ...   | 2FGL J0217.8+7353    | ... | fsrq  | PKS 0215+015            |
| J0218.1+4233  | 34.546 | 42.554  | 139.517 | –17.507 | 0.026      | 0.025      | –77    | 44.0     | 5.4      | 0.2             | 48.1     | 1.8             | 2.29          | ...                  | EC  | ... | ...   | 1FHL J0217.7+0142    | ... | PSR   | PSR J0218+4232          |
| J0218.9+3642  | 34.746 | 36.708  | 141.867 | –22.924 | 0.075      | 0.073      | –13    | 13.9     | 1.0      | 0.1             | 16.0     | 1.4             | 2.58          | 0.07                 | PL  | T   | ...   | 2FGL J0217.9+0143    | ... | bcu   | MG3 J021846+3641        |
| J0219.0+2440  | 34.768 | 24.679  | 147.087 | –34.049 | 0.081      | 0.068      | –42    | 6.0      | 0.3      | 0.1             | 3.7      | 0.9             | 1.86          | 0.16                 | PL  | ... | ...   | 1FGL J0217.9+0144    | ... | bcu   | 87GB<br>021610.9+243205 |
| J0220.1+6202c | 35.048 | 62.044  | 133.131 | 0.942   | 0.119      | 0.088      | 53     | 4.6      | 1.2      | 0.3             | 14.7     | 3.9             | 2.30          | 0.11                 | PL  | ... | 5,6   | 0FGL J0217.8+0146    | ... | spp   | ...                     |

Table 1—Continued

| Name 3FGL     | R.A.   | Decl.   | $l$     | $b$     | $\theta_1$ | $\theta_2$ | $\phi$ | $\sigma$ | $F_{35}$ | $\Delta F_{35}$ | $S_{25}$ | $\Delta S_{25}$ | $\Gamma_{25}$ | $\Delta \Gamma_{25}$ | Mod | Var | Flags | $\gamma$ -ray Assoc.                                                                                                 | TeV | Class | ID or Assoc.          |
|---------------|--------|---------|---------|---------|------------|------------|--------|----------|----------|-----------------|----------|-----------------|---------------|----------------------|-----|-----|-------|----------------------------------------------------------------------------------------------------------------------|-----|-------|-----------------------|
| J0221.1+3556  | 35.280 | 35.941  | 142.607 | -23.481 | 0.021      | 0.021      | 81     | 48.4     | 4.6      | 0.2             | 55.6     | 1.8             | 2.28          | 0.03                 | PL  | T   | ...   | 1FHL J0221.1+3555<br>2FGL J0221.0+3555<br>1FGL J0221.0+3555<br>0FGL J0220.9+3607                                     | P   | FSRQ  | B0218+357             |
| J0221.1+6059  | 35.299 | 60.997  | 133.598 | -0.002  | 0.232      | 0.134      | -49    | 5.5      | 0.9      | 0.2             | 17.3     | 2.9             | 2.68          | 0.10                 | PL  | ... | ...   | ...                                                                                                                  | ... | ...   | ...                   |
| J0221.2+2518  | 35.320 | 25.306  | 147.333 | -33.274 | 0.095      | 0.080      | -40    | 5.5      | 0.3      | 0.1             | 3.8      | 0.9             | 1.94          | 0.17                 | PL  | ... | ...   | 2FGL J0221.2+2516                                                                                                    | ... | ...   | ...                   |
| J0221.8+6138c | 35.473 | 61.641  | 133.456 | 0.632   | 0.109      | 0.073      | -87    | 4.7      | 1.1      | 0.2             | 14.9     | 4.1             | 2.42          | 0.12                 | PL  | ... | 5,6   | ...                                                                                                                  | ... | ...   | ...                   |
| J0222.1-1616  | 35.532 | -16.280 | 190.284 | -66.364 | 0.112      | 0.087      | -30    | 11.6     | 0.5      | 0.1             | 8.5      | 0.9             | 2.60          | 0.09                 | PL  | T   | ...   | 2FGL J0222.0-1615<br>1FGL J0222.1-1618                                                                               | ... | fsrq  | PKS 0219-164          |
| J0222.6+4301  | 35.674 | 43.033  | 140.150 | -16.767 | 0.009      | 0.009      | -5     | 121.3    | 19.3     | 0.4             | 193.5    | 4.9             | 1.94          | ...                  | LP  | T   | ...   | 1FHL J0222.6+4302<br>2FGL J0222.6+4302<br>1FGL J0222.6+4302<br>0FGL J0222.6+4302<br>3EG J0222+4253<br>EGR J0223+4300 | P   | BLL   | 3C 66A                |
| J0222.9-1117  | 35.741 | -11.297 | 181.001 | -63.303 | 0.085      | 0.065      | 80     | 6.2      | 0.3      | 0.1             | 3.4      | 0.8             | 1.82          | 0.16                 | PL  | ... | ...   | 2FGL J0223.0-1118<br>1FGL J0223.0-1118                                                                               | ... | bll   | 1RXS J022314.6-111741 |
| J0223.3+6820  | 35.826 | 68.343  | 131.274 | 6.972   | 0.041      | 0.033      | 7      | 8.5      | 0.6      | 0.1             | 6.8      | 1.2             | 1.91          | 0.13                 | PL  | ... | ...   | 2FGL J0222.7+6820                                                                                                    | ... | bcu   | NVSS J022304+682154   |
| J0223.5+6313  | 35.883 | 63.226  | 133.088 | 2.184   | 0.171      | 0.135      | 21     | 7.9      | 1.3      | 0.2             | 12.2     | 2.1             | 2.48          | ...                  | LP  | ... | 1     | ...                                                                                                                  | ... | bcu   | TXS 0219+628          |
| J0223.6+6204  | 35.906 | 62.081  | 133.496 | 1.115   | 0.039      | 0.036      | -33    | 12.9     | 5.7      | 0.5             | 39.8     | 5.8             | 2.33          | ...                  | LP  | ... | ...   | 2FGL J0224.0+6204                                                                                                    | ... | ...   | ...                   |
| J0223.6+3927  | 35.918 | 39.453  | 141.710 | -20.032 | 0.180      | 0.118      | 7      | 7.8      | 0.5      | 0.1             | 6.3      | 0.9             | 2.40          | 0.11                 | PL  | ... | ...   | ...                                                                                                                  | ... | ...   | ...                   |
| J0224.0+6235  | 36.016 | 62.598  | 133.364 | 1.618   | 0.197      | 0.155      | -22    | 4.6      | 0.9      | 0.2             | 13.4     | 3.3             | 2.48          | 0.12                 | PL  | ... | 5     | EGRc J0225+6240                                                                                                      | ... | spp   | ...                   |
| J0224.1-7941  | 36.048 | -79.692 | 297.903 | -36.514 | 0.078      | 0.073      | 33     | 7.0      | 0.4      | 0.1             | 4.7      | 0.8             | 2.23          | 0.15                 | PL  | ... | ...   | ...                                                                                                                  | ... | bcu   | PMN J0223-7940        |
| J0224.1-1846  | 36.048 | -18.782 | 196.452 | -67.122 | 0.128      | 0.109      | -43    | 7.0      | 0.4      | 0.1             | 4.7      | 0.8             | 2.40          | 0.13                 | PL  | ... | ...   | ...                                                                                                                  | ... | ...   | ...                   |
| J0224.4+1615  | 36.114 | 16.263  | 153.125 | -41.092 | 0.175      | 0.123      | 86     | 4.1      | 0.3      | 0.1             | 3.8      | 1.0             | 2.26          | 0.18                 | PL  | ... | ...   | ...                                                                                                                  | ... | ...   | ...                   |
| J0225.2-2602  | 36.312 | -26.038 | 215.305 | -69.029 | 0.159      | 0.115      | 60     | 15.5     | 0.6      | 0.1             | 10.7     | 0.8             | 2.66          | 0.07                 | PL  | T   | ...   | ...                                                                                                                  | ... | bcu   | PMN J0225-2603        |
| J0225.8+6159  | 36.472 | 61.987  | 133.778 | 1.121   | 0.095      | 0.082      | 55     | 8.3      | 3.3      | 0.4             | 26.3     | 4.7             | 2.37          | ...                  | LP  | ... | 3,5   | 2FGL J0225.9+6154c<br>3EG J0229+6151                                                                                 | ... | ...   | ...                   |
| J0226.3+0941  | 36.580 | 9.684   | 158.176 | -46.592 | 0.079      | 0.072      | -30    | 9.9      | 0.7      | 0.1             | 7.8      | 1.0             | 2.19          | 0.09                 | PL  | T   | ...   | 2FGL J0226.1+0943<br>1FGL J0226.3+0937                                                                               | ... | fsrq  | PMN J0226+0937        |
| J0226.5-4442  | 36.631 | -44.714 | 261.941 | -64.106 | 0.072      | 0.062      | -5     | 9.9      | 0.5      | 0.1             | 5.9      | 0.9             | 1.95          | 0.12                 | PL  | ... | ...   | 2FGL J0226.5-4444                                                                                                    | ... | bcu   | RBS 0318              |
| J0226.7-4747  | 36.695 | -47.784 | 267.303 | -62.216 | 0.221      | 0.160      | -78    | 6.2      | 0.2      | 0.1             | 4.6      | 0.8             | 2.92          | 0.19                 | PL  | ... | ...   | ...                                                                                                                  | ... | ...   | ...                   |
| J0227.2+0201  | 36.806 | 2.031   | 165.091 | -52.817 | 0.064      | 0.063      | 71     | 11.1     | 0.7      | 0.1             | 7.2      | 1.0             | 2.04          | 0.10                 | PL  | ... | ...   | 2FGL J0227.3+0203                                                                                                    | ... | bll   | RX J0227.2+0201       |
| J0228.0+2248  | 37.008 | 22.801  | 150.304 | -34.886 | 0.139      | 0.095      | 67     | 7.9      | 0.6      | 0.1             | 6.9      | 1.0             | 2.12          | 0.11                 | PL  | T   | ...   | 2FGL J0227.7+2249                                                                                                    | ... | bcu   | NVSS J022744+224834   |
| J0228.3-5545  | 37.078 | -55.762 | 278.231 | -56.473 | 0.052      | 0.048      | -70    | 18.5     | 0.9      | 0.1             | 12.2     | 0.8             | 2.43          | 0.06                 | PL  | T   | ...   | ...                                                                                                                  | ... | fsrq  | PKS 0226-559          |

Table 1—Continued

| Name 3FGL    | R.A.   | Decl.   | $l$     | $b$     | $\theta_1$ | $\theta_2$ | $\phi$ | $\sigma$ | $F_{35}$ | $\Delta F_{35}$ | $S_{25}$ | $\Delta S_{25}$ | $\Gamma_{25}$ | $\Delta \Gamma_{25}$ | Mod | Var | Flags | $\gamma$ -ray Assoc.                                                                               | TeV | Class          | ID or Assoc.             |
|--------------|--------|---------|---------|---------|------------|------------|--------|----------|----------|-----------------|----------|-----------------|---------------|----------------------|-----|-----|-------|----------------------------------------------------------------------------------------------------|-----|----------------|--------------------------|
| J0228.5+6703 | 37.132 | 67.056  | 132.204 | 5.948   | 0.183      | 0.150      | 31     | 4.9      | 0.5      | 0.1             | 8.2      | 1.5             | 2.62          | 0.13                 | PL  | ... | 4     | ...                                                                                                | ... | bcu            | GB6 J0229+6706           |
| J0228.5+8213 | 37.133 | 82.222  | 126.326 | 19.998  | 0.202      | 0.118      | 0      | 5.4      | 0.2      | 0.1             | 4.7      | 0.8             | 2.77          | 0.19                 | PL  | ... | 4     | ...                                                                                                | ... | ...            | ...                      |
| J0228.7−3106 | 37.198 | −31.107 | 229.366 | −68.414 | 0.155      | 0.120      | −78    | 4.1      | 0.2      | 0.1             | 2.3      | 0.6             | 2.14          | 0.24                 | PL  | ... | ...   | ...                                                                                                | ... | bcu            | PMN J0228−3102           |
| J0229.3−3643 | 37.345 | −36.731 | 243.945 | −67.197 | 0.062      | 0.055      | −25    | 18.4     | 0.8      | 0.1             | 12.8     | 0.8             | 2.54          | 0.06                 | PL  | T   | ...   | 2FGL J0229.3−3644<br>1FGL J0229.3−3644<br>0FGL J0229.5−3640                                        | ... | fsrq           | PKS 0227−369             |
| J0230.6−5757 | 37.671 | −57.957 | 280.329 | −54.599 | 0.090      | 0.079      | 69     | 5.0      | 0.2      | 0.1             | 2.3      | 0.7             | 1.68          | 0.29                 | PL  | ... | ...   | ...                                                                                                | ... | bll            | PKS 0229−581             |
| J0230.8+4032 | 37.702 | 40.543  | 142.606 | −18.502 | 0.048      | 0.045      | −58    | 17.7     | 1.0      | 0.1             | 15.0     | 1.0             | 2.55          | 0.06                 | PL  | T   | ...   | 2FGL J0230.8+4031<br>1FGL J0230.8+4031                                                             | ... | fsrq           | B3 0227+403              |
| J0231.0+1302 | 37.775 | 13.045  | 157.139 | −43.111 | 0.213      | 0.190      | −22    | 5.1      | 0.3      | 0.1             | 5.2      | 1.0             | 2.55          | 0.15                 | PL  | ... | ...   | ...                                                                                                | ... | ...            | ...                      |
| J0232.6+0646 | 38.163 | 6.772   | 162.464 | −48.178 | 0.363      | 0.267      | −88    | 5.5      | 0.3      | 0.1             | 5.3      | 0.9             | 2.67          | 0.14                 | PL  | ... | 1     | ...                                                                                                | ... | ...            | ...                      |
| J0232.8+2016 | 38.219 | 20.271  | 152.968 | −36.615 | 0.055      | 0.047      | −4     | 7.2      | 0.4      | 0.1             | 4.9      | 1.0             | 2.03          | 0.15                 | PL  | ... | ...   | ...                                                                                                | P   | bll            | 1ES 0229+200             |
| J0232.9+2606 | 38.232 | 26.104  | 149.738 | −31.432 | 0.095      | 0.091      | −71    | 4.3      | 0.3      | 0.1             | 3.0      | 0.8             | 2.09          | 0.20                 | PL  | ... | ...   | ...                                                                                                | ... | bcu            | B2 0230+25               |
| J0233.0+6237 | 38.269 | 62.623  | 134.319 | 2.020   | 0.211      | 0.091      | 27     | 5.7      | 0.7      | 0.1             | 13.6     | 2.5             | 2.67          | 0.12                 | PL  | ... | ...   | 2FGL J0233.9+6238c                                                                                 | ... | ...            | ...                      |
| J0234.2−0629 | 38.564 | −6.498  | 177.423 | −58.034 | 0.067      | 0.061      | 87     | 5.7      | 0.2      | 0.1             | 2.9      | 0.8             | 1.81          | 0.20                 | PL  | ... | ...   | ...                                                                                                | ... | ...            | ...                      |
| J0235.7+5647 | 38.928 | 56.787  | 136.883 | −3.234  | 0.109      | 0.095      | −40    | 8.2      | 0.7      | 0.1             | 11.2     | 1.4             | 2.61          | 0.10                 | PL  | ... | 3,4   | ...                                                                                                | ... | ...            | ...                      |
| J0236.7−6136 | 39.195 | −61.600 | 283.208 | −51.303 | 0.035      | 0.034      | 30     | 31.8     | 1.8      | 0.1             | 22.4     | 1.1             | 2.31          | 0.04                 | PL  | T   | ...   | 2FGL J0237.1−6136<br>1FGL J0238.3−6132                                                             | ... | fsrq           | PKS 0235−618             |
| J0237.5−3603 | 39.399 | −36.059 | 241.181 | −65.792 | 0.040      | 0.039      | 8      | 9.9      | 0.5      | 0.1             | 5.5      | 1.0             | 1.86          | 0.11                 | PL  | ... | ...   | 1FHL J0237.5−3603<br>2FGL J0237.5−3603<br>1FGL J0237.5−3603                                        | ... | bll            | RBS 0334                 |
| J0237.9+2848 | 39.480 | 28.805  | 149.476 | −28.522 | 0.018      | 0.018      | −37    | 105.2    | 9.7      | 0.2             | 111.3    | 1.9             | 2.35          | ...                  | LP  | T   | ...   | 2FGL J0237.8+2846<br>1FGL J0237.9+2848<br>0FGL J0238.4+2855                                        | ... | FSRQ 4C +28.07 | ...                      |
| J0238.0+5237 | 39.505 | 52.626  | 138.848 | −6.921  | 0.059      | 0.052      | 77     | 15.0     | 1.5      | 0.1             | 11.6     | 1.2             | 2.27          | ...                  | LP  | ... | ...   | 2FGL J0237.9+5238                                                                                  | ... | ...            | ...                      |
| J0238.3−3904 | 39.588 | −39.073 | 247.965 | −64.759 | 0.101      | 0.076      | 43     | 6.3      | 0.3      | 0.1             | 3.2      | 0.7             | 1.94          | 0.15                 | PL  | ... | ...   | 2FGL J0238.2−3905                                                                                  | ... | bll            | 1RXS<br>J023800.5−390505 |
| J0238.4−3117 | 39.617 | −31.295 | 229.490 | −66.337 | 0.039      | 0.037      | −34    | 15.5     | 0.8      | 0.1             | 9.8      | 1.2             | 1.84          | 0.08                 | PL  | ... | ...   | 1FHL J0238.6−3117<br>2FGL J0238.6−3117<br>1FGL J0238.6−3117                                        | ... | bll            | 1RXS<br>J023832.6−311658 |
| J0238.6+1636 | 39.667 | 16.615  | 156.777 | −39.108 | 0.016      | 0.016      | 27     | 88.0     | 10.3     | 0.3             | 100.2    | 2.7             | 2.17          | ...                  | LP  | T   | ...   | 1FHL J0238.7+1639<br>2FGL J0238.7+1637<br>1FGL J0238.6+1637<br>0FGL J0238.6+1636<br>3EG J0237+1635 | ... | BLL            | AO 0235+164              |
| J0239.0+2555 | 39.768 | 25.920  | 151.271 | −30.962 | 0.088      | 0.078      | −58    | 4.3      | 0.3      | 0.1             | 2.9      | 0.9             | 2.06          | 0.25                 | PL  | ... | ...   | ...                                                                                                | ... | ...            | ...                      |

Table 1—Continued

| Name 3FGL    | R.A.   | Decl.   | $l$     | $b$     | $\theta_1$ | $\theta_2$ | $\phi$ | $\sigma$ | $F_{35}$ | $\Delta F_{35}$ | $S_{25}$ | $\Delta S_{25}$ | $\Gamma_{25}$ | $\Delta \Gamma_{25}$ | Mod | Var | Flags | $\gamma$ -ray Assoc.                                                                                                  | TeV | Class | ID or Assoc.           |
|--------------|--------|---------|---------|---------|------------|------------|--------|----------|----------|-----------------|----------|-----------------|---------------|----------------------|-----|-----|-------|-----------------------------------------------------------------------------------------------------------------------|-----|-------|------------------------|
| J0239.4+1326 | 39.868 | 13.443  | 159.199 | -41.697 | 0.076      | 0.068      | -89    | 6.6      | 0.4      | 0.1             | 5.0      | 1.0             | 2.00          | 0.16                 | PL  | ... | ...   | 2FGL J0239.5+1324<br>1FGL J0239.5+1324                                                                                | ... | ...   | ...                    |
| J0240.0-0253 | 40.001 | -2.899  | 174.600 | -54.492 | 0.290      | 0.219      | -7     | 4.7      | 0.3      | 0.1             | 3.7      | 0.8             | 2.44          | 0.16                 | PL  | ... | ...   | ...                                                                                                                   | ... | ...   | ...                    |
| J0240.5+6113 | 40.138 | 61.228  | 135.679 | 1.086   | 0.009      | 0.009      | -55    | 196.6    | 46.1     | 0.5             | 472.7    | 4.4             | 2.29          | ...                  | LP  | T   | ...   | 1FHL J0240.2+6113<br>2FGL J0240.5+6113<br>1FGL J0240.5+6113<br>0FGL J0240.3+6113<br>EGR J0240+6112<br>1AGL J0242+6111 | P   | HMB   | LS I+61 303            |
| J0241.3+6542 | 40.344 | 65.702  | 133.925 | 5.205   | 0.046      | 0.040      | 21     | 11.9     | 1.2      | 0.1             | 13.1     | 1.5             | 2.08          | 0.08                 | PL  | ... | ...   | ...                                                                                                                   | ... | bcu   | TXS 0237+655           |
| J0242.1-0534 | 40.532 | -5.570  | 178.612 | -55.968 | 0.207      | 0.135      | -88    | 4.3      | 0.2      | 0.1             | 3.4      | 0.8             | 2.48          | 0.18                 | PL  | ... | 9     | ...                                                                                                                   | ... | ...   | ...                    |
| J0242.3+1059 | 40.584 | 10.995  | 161.834 | -43.344 | 0.203      | 0.166      | 27     | 7.2      | 0.5      | 0.1             | 7.3      | 1.0             | 2.54          | 0.10                 | PL  | T   | ...   | ...                                                                                                                   | ... | fsrq  | OD 166                 |
| J0242.7-0001 | 40.680 | -0.026  | 172.131 | -51.936 | 0.091      | 0.071      | -71    | 9.8      | 0.6      | 0.1             | 7.0      | 0.9             | 2.32          | 0.10                 | PL  | ... | ...   | 2FGL J0242.5+0006<br>1FGL J0242.7+0007                                                                                | ... | sbq   | NGC 1068               |
| J0243.5+7119 | 40.879 | 71.328  | 131.728 | 10.396  | 0.060      | 0.049      | 84     | 9.6      | 0.8      | 0.1             | 9.2      | 1.2             | 2.11          | 0.08                 | PL  | ... | ...   | 2FGL J0242.9+7118<br>1FGL J0243.5+7116                                                                                | ... | bll   | S5 0238+711            |
| J0244.4-8224 | 41.113 | -82.414 | 298.622 | -33.745 | 0.255      | 0.158      | -70    | 5.1      | 0.2      | 0.1             | 4.6      | 0.9             | 2.68          | 0.17                 | PL  | ... | ...   | ...                                                                                                                   | ... | bcu   | PMN J0251-8226         |
| J0244.4+4745 | 41.123 | 47.753  | 141.852 | -10.922 | 0.405      | 0.335      | 53     | 5.7      | 0.3      | 0.1             | 5.9      | 1.0             | 2.62          | 0.12                 | PL  | ... | 1,4   | ...                                                                                                                   | ... | ...   | ...                    |
| J0244.8-5818 | 41.208 | -58.316 | 278.405 | -53.074 | 0.039      | 0.036      | -64    | 10.4     | 0.4      | 0.1             | 5.1      | 1.0             | 1.70          | 0.14                 | PL  | ... | ...   | 1FHL J0244.2-5813                                                                                                     | ... | bll   | RBS 0351               |
| J0245.4+2410 | 41.358 | 24.183  | 153.732 | -31.783 | 0.121      | 0.100      | -3     | 11.7     | 0.7      | 0.1             | 11.8     | 1.1             | 2.58          | 0.08                 | PL  | T   | ...   | 2FGL J0245.1+2406<br>1FGL J0245.4+2413                                                                                | ... | fsrq  | B2 0242+23             |
| J0245.9-4651 | 41.484 | -46.853 | 261.836 | -60.105 | 0.026      | 0.024      | -70    | 73.5     | 4.5      | 0.2             | 56.1     | 1.4             | 2.40          | ...                  | LP  | T   | ...   | 2FGL J0245.9-4652<br>1FGL J0245.9-4652<br>0FGL J0245.6-4656                                                           | ... | fsrq  | PKS 0244-470           |
| J0248.4+5130 | 42.110 | 51.514  | 140.783 | -7.256  | 0.041      | 0.038      | 48     | 11.9     | 1.0      | 0.1             | 11.3     | 1.4             | 2.07          | 0.09                 | PL  | ... | ...   | 2FGL J0248.5+5131<br>1FGL J0248.7+5127                                                                                | ... | ...   | ...                    |
| J0248.5+4232 | 42.126 | 42.536  | 144.861 | -15.296 | 0.125      | 0.097      | 8      | 6.8      | 0.4      | 0.1             | 5.2      | 0.8             | 2.42          | 0.12                 | PL  | ... | 1,3   | ...                                                                                                                   | ... | psr   | PSR J0248+42           |
| J0248.5+6022 | 42.147 | 60.373  | 136.928 | 0.724   | 0.051      | 0.048      | -3     | 23.9     | 4.2      | 0.3             | 45.3     | 3.3             | 2.57          | ...                  | EC  | ... | ...   | 2FGL J0248.1+6021<br>1FGL J0248.3+6021                                                                                | ... | PSR   | PSR J0248+6021         |
| J0249.1+8438 | 42.278 | 84.636  | 125.780 | 22.428  | 0.065      | 0.060      | -43    | 8.4      | 0.4      | 0.1             | 4.9      | 0.8             | 2.15          | 0.13                 | PL  | ... | ...   | 2FGL J0248.6+8440                                                                                                     | ... | bcu   | NVSS<br>J024948+843556 |
| J0250.6+1713 | 42.652 | 17.231  | 159.422 | -37.058 | 0.050      | 0.047      | -90    | 8.2      | 0.5      | 0.1             | 5.5      | 1.0             | 1.98          | 0.19                 | PL  | ... | ...   | 1FHL J0250.6+1712<br>2FGL J0250.6+1713<br>1FGL J0250.4+1715                                                           | ... | fsrq  | NVSS<br>J025037+171209 |
| J0250.6+5630 | 42.661 | 56.515  | 138.864 | -2.624  | 0.056      | 0.049      | 86     | 7.8      | 0.7      | 0.1             | 8.0      | 1.4             | 1.99          | 0.13                 | PL  | ... | ...   | 2FGL J0250.7+5631<br>1FGL J0251.5+5634                                                                                | ... | bcu   | NVSS<br>J025047+562935 |



Table 1—Continued

| Name 3FGL    | R.A.   | Decl.   | $l$     | $b$     | $\theta_1$ | $\theta_2$ | $\phi$ | $\sigma$ | $F_{35}$ | $\Delta F_{35}$ | $S_{25}$ | $\Delta S_{25}$ | $\Gamma_{25}$ | $\Delta \Gamma_{25}$ | Mod | Var | Flags | $\gamma$ -ray Assoc. | TeV | Class | ID or Assoc.     |
|--------------|--------|---------|---------|---------|------------|------------|--------|----------|----------|-----------------|----------|-----------------|---------------|----------------------|-----|-----|-------|----------------------|-----|-------|------------------|
| J0251.1+2603 | 42.776 | 26.064  | 153.917 | -29.512 | 0.108      | 0.098      | -22    | 7.9      | 0.6      | 0.1             | 6.9      | 1.0             | 2.29          | 0.10                 | PL  | ... | ...   | 2FGL J0251.0+2557    | ... | psr   | PSR J0251+26     |
| J0251.1-1829 | 42.797 | -18.486 | 201.866 | -61.166 | 0.094      | 0.082      | -19    | 4.8      | 0.2      | 0.1             | 2.7      | 0.9             | 1.62          | 0.20                 | PL  | ... | ...   | ...                  | ... | ...   | ...              |
| J0251.5-5959 | 42.882 | -59.987 | 279.344 | -51.286 | 0.168      | 0.137      | -4     | 5.3      | 0.3      | 0.1             | 3.3      | 0.7             | 2.29          | 0.15                 | PL  | ... | ...   | ...                  | ... | fsrq  | PKS 0250-602     |
| J0252.3+3830 | 43.084 | 38.508  | 147.481 | -18.533 | 0.218      | 0.180      | 50     | 4.1      | 0.2      | 0.1             | 3.6      | 0.8             | 2.50          | 0.17                 | PL  | ... | ...   | ...                  | ... | fsrq  | B2 0249+38       |
| J0252.8-2218 | 43.201 | -22.310 | 209.723 | -62.091 | 0.024      | 0.023      | 68     | 69.7     | 5.3      | 0.2             | 57.1     | 1.6             | 2.30          | ...                  | LP  | T   | ...   | 1FHL J0252.7-2218    | ... | fsrq  | PKS 0250-225     |
|              |        |         |         |         |            |            |        |          |          |                 |          |                 |               |                      |     |     |       | 2FGL J0252.7-2218    |     |       |                  |
|              |        |         |         |         |            |            |        |          |          |                 |          |                 |               |                      |     |     |       | 1FGL J0252.8-2219    |     |       |                  |
| J0253.0-0125 | 43.257 | -1.420  | 176.666 | -51.142 | 0.131      | 0.105      | -80    | 5.2      | 0.3      | 0.1             | 3.7      | 0.9             | 1.95          | 0.14                 | PL  | ... | ...   | ...                  | ... | bll   | FBQS J0253-0124  |
| J0253.1-5438 | 43.296 | -54.649 | 272.475 | -54.674 | 0.148      | 0.107      | 6      | 7.8      | 0.3      | 0.1             | 4.7      | 0.7             | 2.45          | 0.12                 | PL  | T   | ...   | ...                  | ... | fsrq  | PKS 0252-549     |
| J0253.5+3216 | 43.384 | 32.269  | 150.945 | -23.878 | 0.047      | 0.040      | 15     | 9.9      | 0.6      | 0.1             | 6.9      | 1.0             | 2.05          | 0.11                 | PL  | T   | ...   | 2FGL J0253.4+3218    | ... | bcu   | MG3 J025334+3217 |
| J0253.8+5104 | 43.472 | 51.068  | 141.752 | -7.274  | 0.092      | 0.062      | -21    | 13.2     | 1.2      | 0.1             | 18.7     | 1.5             | 2.54          | 0.06                 | PL  | T   | ...   | 2FGL J0253.5+5107    | ... | fsrq  | NVSS             |
|              |        |         |         |         |            |            |        |          |          |                 |          |                 |               |                      |     |     |       |                      |     |       | J025357+510256   |
|              |        |         |         |         |            |            |        |          |          |                 |          |                 |               |                      |     |     |       | 1FGL J0254.2+5107    |     |       |                  |
| J0254.2+5903 | 43.559 | 59.053  | 138.153 | -0.141  | 0.121      | 0.096      | 10     | 4.7      | 0.6      | 0.1             | 10.1     | 2.2             | 2.66          | 0.16                 | PL  | ... | 4     | 2FGL J0253.9+5908    | ... | ...   | ...              |
| J0255.8+0532 | 43.955 | 5.544   | 170.217 | -45.601 | 0.195      | 0.119      | 38     | 4.3      | 0.3      | 0.1             | 3.8      | 1.0             | 2.07          | 0.19                 | PL  | ... | ...   | ...                  | ... | bcu   | PMN J0255+0533   |
| J0256.3+0335 | 44.083 | 3.596   | 172.234 | -46.968 | 0.084      | 0.066      | -68    | 6.2      | 0.3      | 0.1             | 4.0      | 1.0             | 1.90          | 0.16                 | PL  | ... | ...   | ...                  | ... | bcu   | PKS B0253+033    |
| J0257.8-1216 | 44.456 | -12.277 | 192.545 | -56.895 | 0.161      | 0.149      | -5     | 6.3      | 0.3      | 0.1             | 4.7      | 0.8             | 2.48          | 0.12                 | PL  | T   | ...   | 2FGL J0257.7-1213    | ... | fsrq  | PMN J0257-1211   |
|              |        |         |         |         |            |            |        |          |          |                 |          |                 |               |                      |     |     |       | 1FGL J0257.8-1204    |     |       |                  |
| J0258.0+2030 | 44.518 | 20.513  | 158.981 | -33.348 | 0.079      | 0.073      | 77     | 5.3      | 0.5      | 0.1             | 5.2      | 1.2             | 2.02          | 0.16                 | PL  | ... | 1     | 2FGL J0257.9+2025c   | ... | bll   | MG3 J025805+2029 |
|              |        |         |         |         |            |            |        |          |          |                 |          |                 |               |                      |     |     |       | 1FGL J0258.0+2033    |     |       |                  |
| J0258.2+3555 | 44.558 | 35.929  | 149.895 | -20.218 | 0.257      | 0.214      | -54    | 4.4      | 0.3      | 0.1             | 4.4      | 0.9             | 2.61          | 0.17                 | PL  | ... | 4     | ...                  | ... | ...   | ...              |
| J0258.9+0552 | 44.740 | 5.876   | 170.738 | -44.836 | 0.092      | 0.079      | -78    | 8.0      | 0.6      | 0.1             | 6.8      | 1.1             | 2.12          | 0.11                 | PL  | ... | ...   | ...                  | ... | ...   | ...              |
| J0259.5+0746 | 44.878 | 7.777   | 169.148 | -43.311 | 0.067      | 0.063      | -8     | 11.0     | 0.9      | 0.1             | 10.6     | 1.2             | 2.21          | 0.08                 | PL  | T   | ...   | 2FGL J0259.5+0740    | ... | fsrq  | PKS 0256+075     |
|              |        |         |         |         |            |            |        |          |          |                 |          |                 |               |                      |     |     |       | 1FGL J0259.5+0743    |     |       |                  |
| J0301.4-1652 | 45.371 | -16.869 | 200.890 | -58.270 | 0.135      | 0.118      | -19    | 5.2      | 0.3      | 0.1             | 3.6      | 0.8             | 2.15          | 0.14                 | PL  | ... | ...   | ...                  | ... | bcu   | PMN J0301-1652   |
| J0301.8-7157 | 45.461 | -71.952 | 290.004 | -41.747 | 0.121      | 0.103      | 78     | 10.4     | 0.3      | 0.1             | 7.2      | 0.7             | 2.77          | 0.10                 | PL  | T   | ...   | ...                  | ... | bcu   | PKS 0301-721     |
| J0301.8-2721 | 45.472 | -27.361 | 221.008 | -61.089 | 0.141      | 0.109      | 50     | 4.3      | 0.2      | 0.1             | 2.4      | 0.6             | 2.16          | 0.19                 | PL  | ... | ...   | ...                  | ... | bcu   | NVSS             |
|              |        |         |         |         |            |            |        |          |          |                 |          |                 |               |                      |     |     |       |                      |     |       | J030158-272754   |
| J0302.0+5335 | 45.522 | 53.598  | 141.670 | -4.452  | 0.084      | 0.068      | -58    | 5.5      | 0.5      | 0.1             | 6.9      | 1.4             | 2.38          | 0.12                 | PL  | ... | 4     | ...                  | ... | bcu   | GB6 J0302+5331   |
| J0302.5-7915 | 45.645 | -79.254 | 295.765 | -35.979 | 0.105      | 0.095      | 35     | 8.0      | 0.4      | 0.1             | 6.5      | 0.9             | 2.51          | 0.12                 | PL  | T   | ...   | 2FGL J0302.7-7919    | ... | fsrq  | PMN J0303-7914   |
| J0303.0+3150 | 45.754 | 31.835  | 153.071 | -23.226 | 0.187      | 0.162      | 57     | 4.2      | 0.3      | 0.1             | 4.2      | 1.0             | 2.31          | 0.14                 | PL  | ... | ...   | ...                  | ... | bcu   | B2 0259+31       |
| J0303.4-2407 | 45.871 | -24.123 | 214.631 | -60.168 | 0.015      | 0.014      | 12     | 63.6     | 5.7      | 0.2             | 65.9     | 2.7             | 1.92          | 0.02                 | PL  | T   | ...   | 1FHL J0303.4-2407    | P   | BLL   | PKS 0301-243     |
|              |        |         |         |         |            |            |        |          |          |                 |          |                 |               |                      |     |     |       | 2FGL J0303.4-2407    |     |       |                  |
|              |        |         |         |         |            |            |        |          |          |                 |          |                 |               |                      |     |     |       | 1FGL J0303.5-2406    |     |       |                  |
|              |        |         |         |         |            |            |        |          |          |                 |          |                 |               |                      |     |     |       | 0FGL J0303.7-2410    |     |       |                  |
| J0303.6+4716 | 45.921 | 47.268  | 145.002 | -9.857  | 0.032      | 0.030      | 23     | 27.3     | 2.3      | 0.1             | 27.3     | 1.4             | 2.28          | 0.04                 | PL  | T   | ...   | 1FHL J0303.6+4715    | ... | bll   | 4C +47.08        |
|              |        |         |         |         |            |            |        |          |          |                 |          |                 |               |                      |     |     |       | 2FGL J0303.5+4713    |     |       |                  |

Table 1—Continued

| Name 3FGL    | R.A.   | Decl.   | $l$     | $b$     | $\theta_1$ | $\theta_2$ | $\phi$ | $\sigma$ | $F_{35}$ | $\Delta F_{35}$ | $S_{25}$ | $\Delta S_{25}$ | $\Gamma_{25}$ | $\Delta \Gamma_{25}$ | Mod | Var | Flags | $\gamma$ -ray Assoc.                   | TeV | Class | ID or Assoc.             |
|--------------|--------|---------|---------|---------|------------|------------|--------|----------|----------|-----------------|----------|-----------------|---------------|----------------------|-----|-----|-------|----------------------------------------|-----|-------|--------------------------|
| J0303.7–6211 | 45.931 | –62.184 | 280.236 | –48.704 | 0.061      | 0.056      | 26     | 16.8     | 0.9      | 0.1             | 12.2     | 0.9             | 2.46          | 0.06                 | PL  | T   | ...   | 1FGL J0303.1+4711<br>2FGL J0303.5–6209 | ... | fsrq  | PKS 0302–623             |
| J0304.3–2836 | 46.081 | –28.609 | 223.676 | –60.687 | 0.078      | 0.077      | –0     | 4.1      | 0.1      | 0.0             | 2.0      | 0.8             | 1.61          | 0.23                 | PL  | ... | ...   | 1FGL J0303.4–6209<br>2FGL J0304.5–2836 | ... | bll   | RBS 0385                 |
| J0304.9+6817 | 46.233 | 68.298  | 134.803 | 8.559   | 0.077      | 0.075      | 16     | 14.0     | 0.8      | 0.1             | 18.8     | 1.4             | 2.84          | 0.08                 | PL  | ... | ...   | 2FGL J0303.5+6822                      | ... | bcu   | TXS 0259+681             |
| J0305.2–1607 | 46.304 | –16.120 | 200.326 | –57.143 | 0.082      | 0.067      | –39    | 5.6      | 0.2      | 0.1             | 3.0      | 0.9             | 1.69          | 0.19                 | PL  | ... | ...   | 2FGL J0305.0–1602                      | ... | bcu   | PKS 0302–16              |
| J0307.3+4916 | 46.843 | 49.270  | 144.533 | –7.815  | 0.032      | 0.029      | –44    | 14.8     | 1.3      | 0.1             | 14.4     | 1.4             | 2.10          | 0.07                 | PL  | ... | ...   | 1FGL J0305.2–1601<br>1FHL J0307.4+4915 | ... | ...   | ...                      |
| J0308.0+7442 | 47.018 | 74.707  | 131.720 | 14.217  | 0.039      | 0.036      | –52    | 25.9     | 3.0      | 0.2             | 14.6     | 0.8             | 2.09          | ...                  | EC  | ... | 12    | 2FGL J0307.5+4916<br>2FGL J0307.4+4915 | ... | PSR   | PSR J0307+7443           |
| J0308.4–2852 | 47.103 | –28.873 | 224.367 | –59.818 | 0.212      | 0.151      | –62    | 4.3      | 0.2      | 0.1             | 3.0      | 0.7             | 2.54          | 0.25                 | PL  | ... | ...   | 1FGL J0308.3+7442<br>1FGL J0308.6+7442 | ... | ...   | ...                      |
| J0308.6+0408 | 47.157 | 4.136   | 174.882 | –44.462 | 0.074      | 0.064      | 84     | 8.1      | 0.6      | 0.1             | 6.6      | 1.1             | 2.07          | 0.11                 | PL  | ... | ...   | ...                                    | ... | rdg   | NGC 1218                 |
| J0309.0+1029 | 47.259 | 10.498  | 169.165 | –39.715 | 0.036      | 0.033      | 7      | 25.8     | 2.8      | 0.2             | 24.8     | 1.6             | 2.23          | ...                  | LP  | T   | ...   | 1FGL J0308.3+0403<br>1FHL J0309.1+1027 | ... | fsrq  | PKS 0306+102             |
| J0309.5–0749 | 47.383 | –7.818  | 188.835 | –52.042 | 0.092      | 0.079      | 54     | 6.6      | 0.4      | 0.1             | 4.7      | 1.0             | 1.94          | 0.15                 | PL  | ... | ...   | 2FGL J0309.1+1027<br>2FGL J0309.3–0743 | ... | bll   | NVSS<br>J030943–074427   |
| J0309.9–6057 | 47.478 | –60.963 | 278.103 | –48.953 | 0.047      | 0.042      | –22    | 26.0     | 1.5      | 0.1             | 20.3     | 1.1             | 2.42          | 0.05                 | PL  | T   | ...   | 1FHL J0310.0–6058<br>1FGL J0310.1–6058 | ... | fsrq  | PKS 0308–611             |
| J0310.4–5015 | 47.621 | –50.257 | 263.598 | –54.892 | 0.053      | 0.050      | 22     | 8.4      | 0.3      | 0.1             | 4.2      | 0.9             | 1.75          | 0.14                 | PL  | ... | ...   | 1FHL J0310.5–5014                      | ... | bcu   | 1RXS<br>J031036.0–501615 |
| J0310.8+3814 | 47.709 | 38.237  | 150.915 | –16.945 | 0.107      | 0.079      | –52    | 8.6      | 0.6      | 0.1             | 7.6      | 1.0             | 2.42          | 0.11                 | PL  | T   | ...   | 2FGL J0310.2–5013<br>2FGL J0310.7+3813 | ... | fsrq  | B3 0307+380              |
| J0312.1–0921 | 48.041 | –9.359  | 191.515 | –52.362 | 0.089      | 0.081      | 65     | 10.9     | 0.9      | 0.1             | 5.2      | 0.8             | 2.22          | ...                  | LP  | ... | ...   | 1FGL J0310.6+3812<br>2FGL J0312.5–0914 | ... | ...   | ...                      |
| J0312.7–2222 | 48.176 | –22.371 | 212.360 | –57.682 | 0.056      | 0.052      | –58    | 6.9      | 0.2      | 0.1             | 3.4      | 0.9             | 1.62          | 0.16                 | PL  | ... | ...   | ...                                    | ... | ...   | ...                      |
| J0312.7+2011 | 48.191 | 20.190  | 162.523 | –31.607 | 0.070      | 0.057      | –34    | 6.9      | 0.3      | 0.1             | 4.4      | 1.0             | 1.72          | 0.17                 | PL  | ... | ...   | 1FHL J0312.8+2013<br>2FGL J0312.8+2013 | ... | ...   | ...                      |
| J0312.7+0133 | 48.194 | 1.561   | 178.516 | –45.509 | 0.064      | 0.053      | 62     | 14.4     | 1.0      | 0.1             | 12.1     | 1.1             | 2.28          | 0.07                 | PL  | T   | ...   | 2FGL J0312.6+0132<br>1FGL J0312.6+0131 | ... | fsrq  | PKS 0310+013             |
| J0312.7+3613 | 48.194 | 36.232  | 152.387 | –18.429 | 0.067      | 0.058      | 6      | 6.4      | 0.4      | 0.1             | 5.3      | 1.0             | 2.28          | 0.14                 | PL  | ... | ...   | ...                                    | ... | bll   | V Zw 326                 |
| J0314.3–5103 | 48.579 | –51.061 | 264.329 | –53.979 | 0.066      | 0.065      | 12     | 11.5     | 0.6      | 0.1             | 7.7      | 0.8             | 2.40          | 0.09                 | PL  | ... | ...   | 2FGL J0314.2–5106<br>1FGL J0315.6–5109 | ... | bll   | PMN J0314–5104           |
| J0315.5–1026 | 48.897 | –10.438 | 193.741 | –52.221 | 0.156      | 0.125      | –11    | 5.7      | 0.4      | 0.1             | 5.0      | 0.9             | 2.41          | 0.15                 | PL  | T   | ...   | 2FGL J0315.8–1024<br>1FGL J0315.9–1033 | ... | fsrq  | PKS 0313–107             |
| J0316.1+0904 | 49.042 | 9.077   | 172.096 | –39.599 | 0.029      | 0.026      | 55     | 23.5     | 2.2      | 0.2             | 25.8     | 2.0             | 1.92          | 0.05                 | PL  | T   | ...   | 1FHL J0316.1+0904                      | ... | bll   | GB6 J0316+0904           |

Table 1—Continued

| Name 3FGL    | R.A.   | Decl.   | $l$     | $b$     | $\theta_1$ | $\theta_2$ | $\phi$ | $\sigma$ | $F_{35}$ | $\Delta F_{35}$ | $S_{25}$ | $\Delta S_{25}$ | $\Gamma_{25}$ | $\Delta \Gamma_{25}$ | Mod | Var | Flags | $\gamma$ -ray Assoc. | TeV | Class | ID or Assoc.             |
|--------------|--------|---------|---------|---------|------------|------------|--------|----------|----------|-----------------|----------|-----------------|---------------|----------------------|-----|-----|-------|----------------------|-----|-------|--------------------------|
| J0316.1–2611 | 49.048 | –26.194 | 219.673 | –57.758 | 0.050      | 0.047      | 8      | 12.9     | 0.6      | 0.1             | 7.6      | 1.1             | 1.86          | 0.09                 | PL  | ... | ...   | 2FGL J0316.1+0904    | ... | bll   | RBS 0405                 |
|              |        |         |         |         |            |            |        |          |          |                 |          |                 |               |                      |     |     |       | 1FGL J0316.1+0904    |     |       |                          |
|              |        |         |         |         |            |            |        |          |          |                 |          |                 |               |                      |     |     |       | 1FHL J0316.3–2609    |     |       |                          |
|              |        |         |         |         |            |            |        |          |          |                 |          |                 |               |                      |     |     |       | 2FGL J0315.8–2611    |     |       |                          |
| J0316.2–6436 | 49.050 | –64.607 | 281.534 | –46.050 | 0.058      | 0.051      | 62     | 12.9     | 0.7      | 0.1             | 7.6      | 0.9             | 2.09          | 0.10                 | PL  | ... | ...   | 1FGL J0315.9–2609    | ... | bll   | SUMSS<br>J031614–643732  |
|              |        |         |         |         |            |            |        |          |          |                 |          |                 |               |                      |     |     |       | 2FGL J0316.1–6434    |     |       |                          |
|              |        |         |         |         |            |            |        |          |          |                 |          |                 |               |                      |     |     |       | 1FGL J0316.3–6438    |     |       |                          |
|              |        |         |         |         |            |            |        |          |          |                 |          |                 |               |                      |     |     |       | 1FHL J0316.6+4119    |     |       |                          |
| J0316.6+4119 | 49.165 | 41.329  | 150.172 | –13.736 | 0.039      | 0.035      | 70     | 7.9      | 0.7      | 0.2             | 7.6      | 1.5             | 1.90          | 0.14                 | PL  | ... | ...   | 2FGL J0316.6+4119    | P   | rdg   | IC 310                   |
| J0318.1+0252 | 49.536 | 2.869   | 178.445 | –43.635 | 0.089      | 0.061      | –70    | 12.8     | 1.2      | 0.1             | 5.7      | 0.7             | 2.09          | ...                  | LP  | ... | ...   | 2FGL J0318.0+0255    | ... | ...   | ...                      |
|              |        |         |         |         |            |            |        |          |          |                 |          |                 |               |                      |     |     |       | 1FGL J0318.1+0254    |     |       |                          |
|              |        |         |         |         |            |            |        |          |          |                 |          |                 |               |                      |     |     |       | 1FHL J0318.8+2134    |     |       |                          |
|              |        |         |         |         |            |            |        |          |          |                 |          |                 |               |                      |     |     |       | 2FGL J0319.9+4130    |     |       |                          |
| J0318.7+2134 | 49.689 | 21.583  | 162.828 | –29.649 | 0.049      | 0.042      | –17    | 12.4     | 0.9      | 0.1             | 10.7     | 1.4             | 1.84          | 0.10                 | PL  | T   | ...   | 1FHL J0318.8+2134    | ... | bcu   | MG3 J031849+2135         |
| J0319.8+4130 | 49.959 | 41.514  | 150.580 | –13.256 | 0.010      | 0.010      | –31    | 108.5    | 21.2     | 0.4             | 199.1    | 3.9             | 2.08          | ...                  | LP  | T   | ...   | 1FHL J0319.9+4130    | P   | RDG   | NGC 1275<br>–<br>19<br>– |
|              |        |         |         |         |            |            |        |          |          |                 |          |                 |               |                      |     |     |       | 2FGL J0319.8+4130    |     |       |                          |
|              |        |         |         |         |            |            |        |          |          |                 |          |                 |               |                      |     |     |       | 1FGL J0319.7+4130    |     |       |                          |
|              |        |         |         |         |            |            |        |          |          |                 |          |                 |               |                      |     |     |       | 0FGL J0320.0+4131    |     |       |                          |
| J0319.8+1847 | 49.969 | 18.787  | 165.090 | –31.674 | 0.036      | 0.035      | 57     | 12.2     | 0.6      | 0.1             | 9.5      | 1.6             | 1.57          | 0.10                 | PL  | T   | ...   | 1FHL J0319.8+1847    | P   | bll   | RBS 0413                 |
|              |        |         |         |         |            |            |        |          |          |                 |          |                 |               |                      |     |     |       | 2FGL J0319.6+1849    |     |       |                          |
|              |        |         |         |         |            |            |        |          |          |                 |          |                 |               |                      |     |     |       | 1FGL J0319.7+1847    |     |       |                          |
|              |        |         |         |         |            |            |        |          |          |                 |          |                 |               |                      |     |     |       | 1FHL J0322.1+2337    |     |       |                          |
| J0322.0+2335 | 50.515 | 23.593  | 162.108 | –27.594 | 0.032      | 0.030      | 89     | 15.5     | 1.2      | 0.1             | 13.4     | 1.4             | 1.95          | 0.08                 | PL  | ... | ...   | 2FGL J0322.0+2336    | ... | bll   | MG3 J032201+2336         |
| J0322.5–3721 | 50.643 | –37.358 | 240.440 | –56.697 | 0.123      | 0.091      | –68    | 8.3      | 0.5      | 0.1             | 5.3      | 0.8             | 2.20          | 0.11                 | PL  | ... | ...   | 1FGL J0322.1+2336    | ... | ...   | ...                      |
|              |        |         |         |         |            |            |        |          |          |                 |          |                 |               |                      |     |     |       | 2FGL J0322.4–3717    |     |       |                          |
|              |        |         |         |         |            |            |        |          |          |                 |          |                 |               |                      |     |     |       | 1FHL J0323.5–0107    |     |       |                          |
|              |        |         |         |         |            |            |        |          |          |                 |          |                 |               |                      |     |     |       | 2FGL J0323.6–0108    |     |       |                          |
| J0323.6–0109 | 50.908 | –1.153  | 183.965 | –45.226 | 0.053      | 0.049      | –20    | 12.4     | 0.7      | 0.1             | 8.8      | 1.2             | 1.85          | 0.10                 | PL  | ... | ...   | 1FGL J0323.7–0106    | ... | bll   | 1RXS<br>J032342.6–011131 |
|              |        |         |         |         |            |            |        |          |          |                 |          |                 |               |                      |     |     |       | 2FGL J0323.6–0108    |     |       |                          |
|              |        |         |         |         |            |            |        |          |          |                 |          |                 |               |                      |     |     |       | 1FGL J0323.7–0106    |     |       |                          |
|              |        |         |         |         |            |            |        |          |          |                 |          |                 |               |                      |     |     |       | ...                  |     |       |                          |
| J0323.7–6038 | 50.943 | –60.640 | 276.171 | –47.806 | 0.176      | 0.150      | 48     | 4.4      | 0.2      | 0.1             | 3.1      | 0.8             | 2.44          | 0.18                 | PL  | ... | ...   | ...                  | ... | ...   | ...                      |
| J0324.5–1315 | 51.147 | –13.256 | 199.477 | –51.675 | 0.214      | 0.191      | 26     | 4.2      | 0.2      | 0.1             | 3.7      | 0.8             | 2.65          | 0.18                 | PL  | ... | ...   | ...                  | ... | ...   | ...                      |
| J0325.2+3410 | 51.313 | 34.171  | 155.833 | –18.695 | 0.106      | 0.090      | 2      | 19.0     | 0.7      | 0.1             | 19.4     | 1.2             | 2.81          | ...                  | LP  | T   | ...   | 2FGL J0324.8+3408    | ... | nlsy1 | 1H 0323+342              |
|              |        |         |         |         |            |            |        |          |          |                 |          |                 |               |                      |     |     |       | 1FGL J0325.0+3403    |     |       |                          |
|              |        |         |         |         |            |            |        |          |          |                 |          |                 |               |                      |     |     |       | 2FGL J0325.1–5635    |     |       |                          |
|              |        |         |         |         |            |            |        |          |          |                 |          |                 |               |                      |     |     |       | ...                  |     |       |                          |
| J0325.2–5634 | 51.323 | –56.569 | 270.821 | –49.859 | 0.054      | 0.051      | –35    | 9.7      | 0.5      | 0.1             | 5.3      | 0.7             | 2.22          | 0.11                 | PL  | ... | ...   | 1FGL J0325.6–5626    | ... | bll   | 1RXS<br>J032521.8–563543 |
| J0325.5+2223 | 51.400 | 22.399  | 163.668 | –28.025 | 0.069      | 0.061      | 32     | 22.2     | 1.5      | 0.1             | 25.1     | 1.4             | 2.65          | ...                  | LP  | T   | ...   | 2FGL J0326.1+2226    | ... | fsrq  | TXS 0322+222             |
|              |        |         |         |         |            |            |        |          |          |                 |          |                 |               |                      |     |     |       | 1FGL J0325.9+2219    |     |       |                          |
|              |        |         |         |         |            |            |        |          |          |                 |          |                 |               |                      |     |     |       | ...                  |     |       |                          |
|              |        |         |         |         |            |            |        |          |          |                 |          |                 |               |                      |     |     |       | 1FHL J0325.7–1647    |     |       |                          |
| J0325.6–1648 | 51.410 | –16.802 | 204.906 | –52.950 | 0.036      | 0.034      | 53     | 19.0     | 1.1      | 0.1             | 14.0     | 1.6             | 1.79          | 0.07                 | PL  | ... | ...   | ...                  | ... | bll   | RBS 0421                 |

Table 1—Continued

| Name 3FGL     | R.A.   | Decl.   | $l$     | $b$     | $\theta_1$ | $\theta_2$ | $\phi$ | $\sigma$ | $F_{35}$ | $\Delta F_{35}$ | $S_{25}$ | $\Delta S_{25}$ | $\Gamma_{25}$ | $\Delta \Gamma_{25}$ | Mod | Var | Flags | $\gamma$ -ray Assoc. | TeV | Class | ID or Assoc.     |
|---------------|--------|---------|---------|---------|------------|------------|--------|----------|----------|-----------------|----------|-----------------|---------------|----------------------|-----|-----|-------|----------------------|-----|-------|------------------|
|               |        |         |         |         |            |            |        |          |          |                 |          |                 |               |                      |     |     |       | 2FGL J0325.6–1650    |     |       |                  |
|               |        |         |         |         |            |            |        |          |          |                 |          |                 |               |                      |     |     |       | 1FGL J0325.9–1649    |     |       |                  |
| J0326.0–1842  | 51.508 | –18.704 | 207.918 | –53.570 | 0.100      | 0.082      | –23    | 5.0      | 0.3      | 0.1             | 2.9      | 0.8             | 2.21          | 0.23                 | PL  | ... | ...   | ...                  | ... | bcu   | PMN J0325–1843   |
| J0326.2+0225  | 51.555 | 2.418   | 180.748 | –42.435 | 0.056      | 0.043      | 51     | 12.5     | 0.9      | 0.1             | 9.6      | 1.2             | 2.00          | 0.09                 | PL  | ... | ...   | 1FHL J0326.1+0224    | ... | bll   | 1H 0323+022      |
|               |        |         |         |         |            |            |        |          |          |                 |          |                 |               |                      |     |     |       | 2FGL J0326.1+0224    |     |       |                  |
|               |        |         |         |         |            |            |        |          |          |                 |          |                 |               |                      |     |     |       | 1FGL J0326.2+0222    |     |       |                  |
| J0327.4+5828c | 51.869 | 58.477  | 142.154 | 1.554   | 0.134      | 0.111      | –23    | 6.4      | 0.8      | 0.2             | 12.4     | 1.8             | 2.50          | 0.09                 | PL  | ... | 1,6   | ...                  | ... | ...   | ...              |
| J0330.6+0437  | 52.665 | 4.626   | 179.521 | –40.143 | 0.107      | 0.085      | –61    | 7.4      | 0.6      | 0.1             | 6.7      | 1.1             | 2.24          | 0.11                 | PL  | ... | ...   | ...                  | ... | ...   | ...              |
| J0331.3–6155  | 52.836 | –61.928 | 276.968 | –46.326 | 0.046      | 0.041      | –8     | 12.7     | 0.7      | 0.1             | 7.3      | 0.9             | 2.08          | 0.09                 | PL  | ... | ...   | ...                  | ... | bcu   | PMN J0331–6155   |
| J0332.0+6308  | 53.001 | 63.148  | 139.949 | 5.711   | 0.055      | 0.047      | –38    | 8.5      | 0.9      | 0.1             | 10.8     | 1.4             | 2.33          | 0.08                 | PL  | ... | ...   | 1FHL J0332.1+6307    | ... | bcu   | GB6 J0331+6307   |
|               |        |         |         |         |            |            |        |          |          |                 |          |                 |               |                      |     |     |       | 2FGL J0332.1+6309    |     |       |                  |
|               |        |         |         |         |            |            |        |          |          |                 |          |                 |               |                      |     |     |       | 1FGL J0332.0+6310    |     |       |                  |
| J0332.4+6110  | 53.121 | 61.170  | 141.139 | 4.127   | 0.513      | 0.247      | –58    | 6.5      | 0.5      | 0.2             | 7.3      | 1.3             | 2.50          | ...                  | LP  | ... | 4,9   | ...                  | ... | ...   | ...              |
| J0332.4+4644  | 53.123 | 46.736  | 149.481 | –7.666  | 0.238      | 0.218      | 73     | 5.5      | 0.5      | 0.1             | 7.0      | 1.2             | 2.47          | 0.11                 | PL  | ... | 1     | ...                  | ... | ...   | ...              |
| J0333.4+7853  | 53.360 | 78.890  | 130.515 | 18.483  | 0.058      | 0.057      | 12     | 9.6      | 0.6      | 0.1             | 6.4      | 0.8             | 2.20          | 0.10                 | PL  | ... | ...   | ...                  | ... | bcu   | NVSS             |
|               |        |         |         |         |            |            |        |          |          |                 |          |                 |               |                      |     |     |       | ...                  | ... | ...   | J033344+785027   |
| J0333.4+4003  | 53.368 | 40.052  | 153.613 | –12.976 | 0.098      | 0.084      | 7      | 5.0      | 0.4      | 0.1             | 4.8      | 1.1             | 2.24          | 0.14                 | PL  | ... | ...   | ...                  | ... | bcu   | B3 0330+399      |
| J0333.6+0233  | 53.412 | 2.563   | 182.214 | –40.931 | 0.147      | 0.092      | –78    | 5.4      | 0.4      | 0.1             | 4.0      | 0.9             | 2.07          | 0.17                 | PL  | ... | ...   | ...                  | ... | ...   | ...              |
| J0333.6+2916  | 53.419 | 29.272  | 160.502 | –21.522 | 0.033      | 0.030      | 9      | 17.8     | 1.4      | 0.1             | 17.2     | 1.7             | 1.86          | 0.06                 | PL  | ... | ...   | 1FHL J0333.6+2918    | ... | bll   | TXS 0330+291     |
|               |        |         |         |         |            |            |        |          |          |                 |          |                 |               |                      |     |     |       | 2FGL J0333.7+2918    |     |       |                  |
|               |        |         |         |         |            |            |        |          |          |                 |          |                 |               |                      |     |     |       | 1FGL J0333.7+2919    |     |       |                  |
| J0333.9+6538  | 53.486 | 65.638  | 138.665 | 7.860   | 0.035      | 0.032      | –17    | 11.7     | 0.9      | 0.1             | 10.0     | 1.3             | 1.94          | 0.09                 | PL  | ... | ...   | 1FHL J0334.0+6539    | ... | bll   | TXS 0329+654     |
|               |        |         |         |         |            |            |        |          |          |                 |          |                 |               |                      |     |     |       | 2FGL J0334.3+6538    |     |       |                  |
|               |        |         |         |         |            |            |        |          |          |                 |          |                 |               |                      |     |     |       | 1FGL J0334.3+6536    |     |       |                  |
| J0334.2+3915  | 53.554 | 39.250  | 154.221 | –13.535 | 0.117      | 0.085      | –11    | 5.0      | 0.4      | 0.1             | 4.2      | 1.0             | 2.11          | 0.17                 | PL  | ... | ...   | ...                  | ... | rdg   | 4C +39.12        |
| J0334.3–4008  | 53.577 | –40.148 | 244.773 | –54.058 | 0.023      | 0.022      | 6      | 58.3     | 4.6      | 0.2             | 42.3     | 1.7             | 2.15          | ...                  | LP  | T   | ...   | 1FHL J0334.1–4006    | ... | bll   | PKS 0332–403     |
|               |        |         |         |         |            |            |        |          |          |                 |          |                 |               |                      |     |     |       | 2FGL J0334.2–4008    |     |       |                  |
|               |        |         |         |         |            |            |        |          |          |                 |          |                 |               |                      |     |     |       | 1FGL J0334.2–4010    |     |       |                  |
|               |        |         |         |         |            |            |        |          |          |                 |          |                 |               |                      |     |     |       | 0FGL J0334.1–4006    |     |       |                  |
| J0334.3–3726  | 53.582 | –37.444 | 240.178 | –54.365 | 0.026      | 0.025      | 31     | 36.7     | 2.7      | 0.1             | 30.9     | 1.8             | 1.97          | 0.04                 | PL  | T   | ...   | 1FHL J0334.4–3726    | ... | bll   | PMN J0334–3725   |
|               |        |         |         |         |            |            |        |          |          |                 |          |                 |               |                      |     |     |       | 2FGL J0334.3–3728    |     |       |                  |
|               |        |         |         |         |            |            |        |          |          |                 |          |                 |               |                      |     |     |       | 1FGL J0334.4–3727    |     |       |                  |
| J0335.3–4459  | 53.830 | –44.998 | 252.699 | –52.901 | 0.045      | 0.042      | 73     | 11.5     | 0.5      | 0.1             | 6.3      | 1.0             | 1.84          | 0.10                 | PL  | ... | ...   | 1FHL J0335.3–4501    | ... | bll   | 1RXS             |
|               |        |         |         |         |            |            |        |          |          |                 |          |                 |               |                      |     |     |       | ...                  | ... | ...   | J033514.5–445929 |
|               |        |         |         |         |            |            |        |          |          |                 |          |                 |               |                      |     |     |       | 2FGL J0335.3–4501    |     |       |                  |
|               |        |         |         |         |            |            |        |          |          |                 |          |                 |               |                      |     |     |       | 1FGL J0335.5–4501    |     |       |                  |
| J0336.1+7500  | 54.044 | 75.015  | 133.109 | 15.503  | 0.048      | 0.045      | –47    | 17.8     | 1.5      | 0.1             | 10.0     | 1.0             | 2.18          | ...                  | LP  | ... | ...   | 2FGL J0336.0+7504    | ... | ...   | ...              |

Table 1—Continued

| Name 3FGL     | R.A.   | Decl.   | $l$     | $b$     | $\theta_1$ | $\theta_2$ | $\phi$ | $\sigma$ | $F_{35}$ | $\Delta F_{35}$ | $S_{25}$ | $\Delta S_{25}$ | $\Gamma_{25}$ | $\Delta \Gamma_{25}$ | Mod | Var | Flags | $\gamma$ -ray Assoc.                                        | TeV | Class | ID or Assoc.             |
|---------------|--------|---------|---------|---------|------------|------------|--------|----------|----------|-----------------|----------|-----------------|---------------|----------------------|-----|-----|-------|-------------------------------------------------------------|-----|-------|--------------------------|
| J0336.5+3210  | 54.132 | 32.167  | 159.098 | -18.872 | 0.173      | 0.139      | -16    | 11.7     | 0.8      | 0.1             | 19.8     | 1.7             | 2.89          | 0.07                 | PL  | T   | 3     | 1FGL J0334.2+7501<br>2FGL J0337.0+3200c                     | ... | fsrq  | NRAO 140                 |
| J0336.9-3622  | 54.248 | -36.383 | 238.311 | -53.904 | 0.203      | 0.190      | -12    | 4.8      | 0.3      | 0.1             | 3.6      | 0.8             | 2.44          | 0.14                 | PL  | ... | ...   | ...                                                         | ... | fsrq  | PKS 0335-364             |
| J0336.9-1304  | 54.250 | -13.072 | 201.356 | -48.896 | 0.197      | 0.186      | 19     | 6.2      | 0.3      | 0.1             | 5.3      | 0.8             | 2.67          | 0.13                 | PL  | ... | ...   | ...                                                         | ... | fsrq  | PKS 0334-131             |
| J0338.1-2443  | 54.534 | -24.726 | 218.878 | -52.612 | 0.054      | 0.052      | -40    | 5.7      | 0.1      | 0.0             | 2.3      | 0.9             | 1.29          | 0.26                 | PL  | ... | ...   | 1FHL J0338.1-2443                                           | ... | bl    | 1RXS<br>J033810.1-244337 |
| J0338.5+1303  | 54.631 | 13.066  | 173.562 | -32.921 | 0.034      | 0.031      | 30     | 11.9     | 0.7      | 0.1             | 10.1     | 1.6             | 1.69          | 0.10                 | PL  | ... | ...   | 1FHL J0338.4+1304<br>2FGL J0338.2+1306                      | ... | bcu   | RX J0338.4+1302          |
| J0339.2-1738  | 54.802 | -17.645 | 208.136 | -50.269 | 0.055      | 0.049      | -19    | 9.9      | 0.6      | 0.1             | 6.8      | 1.1             | 1.93          | 0.10                 | PL  | ... | ...   | 2FGL J0339.2-1734                                           | ... | bcu   | PKS 0336-177             |
| J0339.5-0146  | 54.883 | -1.773  | 188.001 | -42.449 | 0.034      | 0.033      | -3     | 45.0     | 3.4      | 0.2             | 41.0     | 1.5             | 2.42          | ...                  | LP  | T   | ...   | 1FGL J0339.1-1734<br>2FGL J0339.4-0144<br>1FGL J0339.2-0143 | ... | fsrq  | PKS 0336-01              |
| J0340.3+4130  | 55.090 | 41.509  | 153.782 | -11.028 | 0.032      | 0.029      | 68     | 31.6     | 3.7      | 0.2             | 22.2     | 1.3             | 2.00          | ...                  | EC  | ... | ...   | 3EG J0340-0201<br>EGR J0338-0203<br>2FGL J0340.4+4131       | ... | PSR   | PSR J0340+4130           |
| J0340.4+5302  | 55.100 | 53.048  | 146.781 | -1.815  | 0.105      | 0.096      | 65     | 22.3     | 0.9      | 0.2             | 36.7     | 1.8             | 2.96          | ...                  | LP  | ... | ...   | 1FGL J0340.4+4130<br>2FGL J0340.5+5307                      | ... | ...   | ...                      |
| J0340.4-2423  | 55.104 | -24.387 | 218.532 | -52.029 | 0.145      | 0.101      | -83    | 4.6      | 0.2      | 0.1             | 2.8      | 0.7             | 2.09          | 0.19                 | PL  | ... | ...   | 1FGL J0341.5+5304<br>2FGL J0340.7-2421                      | ... | ...   | ...                      |
| J0340.5-2119  | 55.141 | -21.322 | 213.785 | -51.186 | 0.067      | 0.062      | 10     | 11.0     | 0.6      | 0.1             | 7.2      | 0.9             | 2.22          | 0.10                 | PL  | T   | ...   | 2FGL J0340.6-2113                                           | ... | bl    | PKS 0338-214             |
| J0342.2+3857  | 55.568 | 38.959  | 155.677 | -12.816 | 0.058      | 0.051      | -82    | 10.2     | 0.7      | 0.1             | 9.4      | 1.2             | 2.37          | 0.10                 | PL  | T   | ...   | 2FGL J0342.4+3859                                           | ... | fsrq  | GB6 J0342+3858           |
| J0342.3+3148c | 55.576 | 31.809  | 160.340 | -18.381 | 0.102      | 0.080      | -10    | 6.8      | 1.0      | 0.2             | 11.4     | 1.8             | 2.28          | 0.10                 | PL  | ... | 5,6   | 1FGL J0342.2+3859<br>2FGL J0341.8+3148c                     | ... | ...   | ...                      |
| J0342.6-3006  | 55.660 | -30.111 | 227.895 | -52.527 | 0.068      | 0.064      | -28    | 4.7      | 0.2      | 0.1             | 2.2      | 0.7             | 1.85          | 0.21                 | PL  | ... | ...   | ...                                                         | ... | bcu   | PKS 0340-302             |
| J0342.8+1321  | 55.711 | 13.362  | 174.190 | -31.966 | 0.073      | 0.068      | -52    | 4.2      | 0.3      | 0.1             | 3.2      | 1.0             | 1.91          | 0.19                 | PL  | ... | ...   | ...                                                         | ... | ...   | ...                      |
| J0343.2-2534  | 55.825 | -25.567 | 220.629 | -51.654 | 0.106      | 0.097      | 67     | 12.5     | 0.6      | 0.1             | 9.4      | 0.9             | 2.56          | 0.08                 | PL  | T   | ...   | 1FGL J0343.4-2536                                           | ... | fsrq  | PKS 0341-256             |
| J0343.3-6443  | 55.827 | -64.724 | 279.211 | -43.661 | 0.058      | 0.052      | -42    | 13.9     | 0.8      | 0.1             | 9.3      | 0.9             | 2.15          | 0.07                 | PL  | T   | ...   | ...                                                         | ... | bcu   | PMN J0343-6442           |
| J0343.3+3622  | 55.850 | 36.373  | 157.516 | -14.700 | 0.111      | 0.090      | -58    | 5.3      | 0.4      | 0.1             | 6.0      | 1.2             | 2.43          | 0.14                 | PL  | ... | ...   | ...                                                         | ... | bcu   | OE 367                   |
| J0345.1-2353  | 56.294 | -23.886 | 218.169 | -50.855 | 0.065      | 0.063      | -12    | 14.2     | 0.8      | 0.1             | 10.7     | 1.0             | 2.41          | 0.07                 | PL  | ... | ...   | 2FGL J0345.2-2356                                           | ... | bl    | NVSS<br>J034518-235218   |
| J0345.3+3236  | 56.350 | 32.602  | 160.337 | -17.353 | 0.130      | 0.101      | -84    | 7.7      | 0.7      | 0.1             | 8.2      | 1.1             | 2.43          | ...                  | LP  | ... | 12    | 1FGL J0345.2-2355                                           | ... | ...   | ...                      |
| J0348.1+4431  | 57.048 | 44.529  | 153.032 | -7.769  | 0.186      | 0.133      | -40    | 4.2      | 0.4      | 0.1             | 5.0      | 1.2             | 2.28          | 0.15                 | PL  | ... | ...   | ...                                                         | ... | ...   | ...                      |
| J0348.4+6039  | 57.105 | 60.663  | 142.998 | 4.885   | 0.112      | 0.083      | -6     | 4.5      | 0.4      | 0.1             | 4.2      | 1.1             | 1.88          | 0.19                 | PL  | ... | ...   | ...                                                         | ... | ...   | ...                      |
| J0348.6-2748  | 57.171 | -27.805 | 224.506 | -50.896 | 0.108      | 0.095      | -29    | 7.0      | 0.4      | 0.1             | 5.0      | 0.8             | 2.38          | 0.12                 | PL  | ... | ...   | 2FGL J0348.6-2750<br>1FGL J0348.5-2751                      | ... | fsrq  | PKS 0346-27              |
| J0348.7-1606  | 57.175 | -16.109 | 207.273 | -47.587 | 0.132      | 0.091      | 33     | 10.6     | 0.6      | 0.1             | 8.0      | 0.9             | 2.47          | 0.09                 | PL  | ... | ...   | ...                                                         | ... | bl    | PKS 0346-163             |

Table 1—Continued

| Name 3FGL    | R.A.   | Decl.   | $l$     | $b$     | $\theta_1$ | $\theta_2$ | $\phi$ | $\sigma$ | $F_{35}$ | $\Delta F_{35}$ | $S_{25}$ | $\Delta S_{25}$ | $\Gamma_{25}$ | $\Delta \Gamma_{25}$ | Mod | Var | Flags | $\gamma$ -ray Assoc.                                        | TeV | Class | ID or Assoc.       |
|--------------|--------|---------|---------|---------|------------|------------|--------|----------|----------|-----------------|----------|-----------------|---------------|----------------------|-----|-----|-------|-------------------------------------------------------------|-----|-------|--------------------|
| J0349.2–1158 | 57.309 | –11.978 | 201.887 | –45.736 | 0.086      | 0.079      | –43    | 7.1      | 0.3      | 0.1             | 4.3      | 1.0             | 1.73          | 0.16                 | PL  | ... | ...   | ...                                                         | P   | bll   | 1ES 0347–121       |
| J0349.9–2102 | 57.478 | –21.049 | 214.395 | –49.025 | 0.068      | 0.066      | –17    | 25.4     | 1.3      | 0.1             | 17.5     | 1.0             | 2.49          | ...                  | LP  | T   | ...   | 2FGL J0350.0–2104<br>1FGL J0349.9–2104<br>0FGL J0349.8–2102 | ... | fsrq  | PKS 0347–211       |
| J0351.0–2816 | 57.769 | –28.277 | 225.377 | –50.453 | 0.083      | 0.082      | –70    | 4.6      | 0.2      | 0.1             | 2.4      | 0.7             | 2.04          | 0.22                 | PL  | ... | 5     | ...                                                         | ... | ...   | ...                |
| J0351.1+0128 | 57.778 | 1.467   | 186.847 | –38.194 | 0.195      | 0.163      | –20    | 4.2      | 0.3      | 0.1             | 4.6      | 1.1             | 2.43          | 0.18                 | PL  | ... | ...   | ...                                                         | ... | ssrq  | TXS 0348+013       |
| J0351.4–3248 | 57.854 | –32.800 | 232.485 | –50.900 | 0.289      | 0.209      | –44    | 4.7      | 0.2      | 0.1             | 3.4      | 0.7             | 2.80          | 0.19                 | PL  | ... | ...   | ...                                                         | ... | ...   | ...                |
| J0352.9+5655 | 58.237 | 56.921  | 145.812 | 2.343   | 0.049      | 0.044      | –53    | 7.6      | 0.5      | 0.1             | 6.6      | 1.2             | 1.83          | 0.12                 | PL  | ... | ...   | 2FGL J0353.2+5653<br>1FGL J0352.8+5658                      | ... | bcu   | GB6 J0353+5654     |
| J0353.0–3622 | 58.265 | –36.375 | 238.155 | –50.672 | 0.076      | 0.064      | –9     | 6.1      | 0.2      | 0.1             | 3.2      | 1.0             | 1.55          | 0.18                 | PL  | ... | ...   | ...                                                         | ... | bll   | XRS J0353–3623     |
| J0353.0–6831 | 58.273 | –68.517 | 282.786 | –40.776 | 0.053      | 0.044      | –42    | 7.8      | 0.3      | 0.1             | 4.0      | 1.0             | 1.61          | 0.18                 | PL  | ... | ...   | ...                                                         | ... | bll   | PKS 0352–686       |
| J0354.1+4643 | 58.531 | 46.718  | 152.446 | –5.418  | 0.130      | 0.107      | –45    | 5.2      | 0.5      | 0.1             | 6.8      | 1.3             | 2.38          | 0.13                 | PL  | ... | 3     | ...                                                         | ... | bcu   | B3 0350+465        |
| J0354.6+8011 | 58.660 | 80.190  | 130.406 | 20.096  | 0.068      | 0.059      | –68    | 12.3     | 0.6      | 0.1             | 8.2      | 0.8             | 2.37          | 0.08                 | PL  | T   | ...   | 2FGL J0354.1+8010<br>1FGL J0354.6+8009                      | ... | bll   | S5 0346+80         |
| J0356.3–6948 | 59.093 | –69.813 | 283.998 | –39.823 | 0.234      | 0.189      | –13    | 4.7      | 0.3      | 0.1             | 3.9      | 0.8             | 2.53          | 0.16                 | PL  | ... | ...   | ...                                                         | ... | bcu   | PMN J0357+6948     |
| J0357.1+2325 | 59.280 | 23.423  | 168.919 | –22.439 | 0.116      | 0.096      | –78    | 5.5      | 0.4      | 0.1             | 5.2      | 1.0             | 2.41          | 0.15                 | PL  | ... | ...   | ...                                                         | ... | bcu   | MG3 J0357.1+2319   |
| J0357.1–4957 | 59.280 | –49.950 | 258.713 | –48.058 | 0.089      | 0.069      | –56    | 8.1      | 0.4      | 0.1             | 4.3      | 0.7             | 2.10          | 0.13                 | PL  | ... | ...   | 2FGL J0357.0–4950<br>1FGL J0357.1–4949                      | ... | bll   | PKS 0355–500       |
| J0357.9+3206 | 59.480 | 32.106  | 162.757 | –15.988 | 0.024      | 0.024      | –77    | 72.5     | 8.7      | 0.3             | 66.0     | 1.5             | 2.23          | ...                  | EC  | ... | ...   | 2FGL J0357.8+3205<br>1FGL J0357.8+3205<br>0FGL J0357.5+3205 | ... | PSR   | LAT PSR J0357+3205 |
| J0358.7+0633 | 59.689 | 6.565   | 183.328 | –33.558 | 0.235      | 0.129      | 64     | 9.6      | 0.6      | 0.1             | 10.6     | 1.2             | 2.63          | 0.10                 | PL  | T   | ...   | ...                                                         | ... | bcu   | PMN J0358+0629     |
| J0358.8+6002 | 59.713 | 60.040  | 144.394 | 5.227   | 0.141      | 0.104      | 79     | 9.9      | 0.9      | 0.1             | 13.4     | 1.4             | 2.52          | 0.08                 | PL  | T   | ...   | 2FGL J0359.1+6003                                           | ... | fsrq  | TXS 0354+599       |
| J0359.3–2612 | 59.837 | –26.203 | 222.778 | –48.259 | 0.099      | 0.090      | –31    | 4.2      | 0.3      | 0.1             | 2.9      | 0.8             | 2.19          | 0.18                 | PL  | ... | ...   | ...                                                         | ... | bll   | PKS 0357–264       |
| J0359.5+5413 | 59.881 | 54.222  | 148.259 | 0.872   | 0.041      | 0.040      | –39    | 19.2     | 3.2      | 0.2             | 24.5     | 1.9             | 2.31          | ...                  | LP  | ... | ...   | 2FGL J0359.5+5410<br>1FGL J0359.5+5410                      | ... | ...   | ...                |
| J0359.7+7649 | 59.935 | 76.831  | 133.024 | 17.813  | 0.072      | 0.060      | 56     | 4.6      | 0.2      | 0.1             | 2.7      | 0.7             | 2.17          | 0.17                 | PL  | ... | ...   | ...                                                         | ... | ...   | ...                |
| J0401.0–5359 | 60.259 | –53.986 | 264.138 | –46.306 | 0.088      | 0.069      | –81    | 4.2      | 0.2      | 0.1             | 2.2      | 0.7             | 2.22          | 0.27                 | PL  | ... | ...   | ...                                                         | ... | ...   | ...                |
| J0401.4+2109 | 60.369 | 21.156  | 171.431 | –23.333 | 0.117      | 0.091      | 83     | 6.2      | 0.5      | 0.1             | 6.3      | 1.1             | 2.35          | 0.11                 | PL  | ... | ...   | ...                                                         | ... | fsrq  | TXS 0358+210       |
| J0401.8–3144 | 60.458 | –31.748 | 231.163 | –48.614 | 0.226      | 0.195      | –82    | 5.2      | 0.2      | 0.1             | 3.6      | 0.7             | 2.54          | 0.20                 | PL  | ... | ...   | 2FGL J0401.6–3153<br>1FGL J0401.3–3152                      | ... | fsrq  | PKS 0400–319       |
| J0402.1–2618 | 60.549 | –26.303 | 223.127 | –47.656 | 0.102      | 0.073      | –1     | 7.5      | 0.5      | 0.1             | 5.3      | 0.9             | 2.13          | 0.12                 | PL  | ... | ...   | 2FGL J0402.0–2616<br>1FGL J0402.1–2618                      | ... | bll   | PKS 0359–264       |
| J0402.7+2616 | 60.676 | 26.270  | 167.760 | –19.518 | 0.188      | 0.154      | –35    | 5.5      | 0.3      | 0.1             | 6.1      | 1.1             | 2.77          | 0.14                 | PL  | ... | 4     | ...                                                         | ... | ...   | ...                |
| J0403.7–2442 | 60.934 | –24.712 | 220.958 | –46.956 | 0.141      | 0.123      | 58     | 4.3      | 0.2      | 0.1             | 2.9      | 0.7             | 2.37          | 0.18                 | PL  | ... | ...   | ...                                                         | ... | fsrq  | TXS 0401–248       |

Table 1—Continued

| Name 3FGL     | R.A.   | Decl.   | $l$     | $b$     | $\theta_1$ | $\theta_2$ | $\phi$ | $\sigma$ | $F_{35}$ | $\Delta F_{35}$ | $S_{25}$ | $\Delta S_{25}$ | $\Gamma_{25}$ | $\Delta \Gamma_{25}$ | Mod | Var | Flags | $\gamma$ -ray Assoc.                                                       | TeV | Class | ID or Assoc.           |
|---------------|--------|---------|---------|---------|------------|------------|--------|----------|----------|-----------------|----------|-----------------|---------------|----------------------|-----|-----|-------|----------------------------------------------------------------------------|-----|-------|------------------------|
| J0403.9–3604  | 60.994 | –36.077 | 237.734 | –48.467 | 0.024      | 0.023      | –26    | 103.6    | 5.8      | 0.2             | 85.4     | 1.5             | 2.49          | ...                  | LP  | T   | ...   | 2FGL J0403.9–3604<br>1FGL J0403.9–3603                                     | ... | FSRQ  | PKS 0402–362           |
| J0405.5–1307  | 61.398 | –13.123 | 205.751 | –42.642 | 0.100      | 0.077      | 89     | 8.7      | 0.5      | 0.1             | 6.4      | 0.9             | 2.35          | 0.11                 | PL  | T   | ...   | 2FGL J0405.8–1309<br>1FGL J0405.6–1309                                     | ... | fsrq  | PKS 0403–13            |
| J0407.1–3825  | 61.796 | –38.420 | 241.255 | –47.851 | 0.048      | 0.045      | –45    | 29.1     | 1.6      | 0.1             | 21.7     | 1.1             | 2.40          | 0.04                 | PL  | T   | ...   | 2FGL J0407.3–3826<br>1FGL J0407.4–3827<br>0FGL J0407.6–3829                | ... | fsrq  | PKS 0405–385           |
| J0407.5+0740  | 61.887 | 7.672   | 183.912 | –31.163 | 0.095      | 0.085      | –58    | 8.7      | 0.6      | 0.1             | 9.7      | 1.2             | 2.57          | 0.10                 | PL  | ... | ...   | 2FGL J0407.7+0740<br>1FGL J0407.5+0749                                     | ... | bl    | TXS 0404+075           |
| J0409.4+3158  | 62.371 | 31.973  | 164.699 | –14.403 | 0.121      | 0.097      | –38    | 5.2      | 0.4      | 0.1             | 5.1      | 1.1             | 2.37          | 0.15                 | PL  | ... | 1     | ...                                                                        | ... | bcu   | NVSS<br>J040928+320245 |
| J0409.8–0358  | 62.457 | –3.968  | 195.864 | –37.374 | 0.081      | 0.069      | 42     | 11.4     | 0.8      | 0.1             | 9.0      | 1.1             | 2.06          | 0.08                 | PL  | ... | ...   | 2FGL J0409.8–0357<br>1FGL J0409.9–0357                                     | ... | bl    | NVSS<br>J040946–040003 |
| J0412.0+0229  | 63.024 | 2.496   | 189.621 | –33.347 | 0.139      | 0.109      | 52     | 4.3      | 0.4      | 0.1             | 4.8      | 1.1             | 2.40          | 0.15                 | PL  | ... | ...   | ...                                                                        | ... | ...   | ...                    |
| J0413.6–5334  | 63.401 | –53.581 | 262.821 | –44.646 | 0.062      | 0.046      | –79    | 16.2     | 0.9      | 0.1             | 11.1     | 0.9             | 2.35          | 0.07                 | PL  | T   | 7     | 2FGL J0413.5–5332<br>1FGL J0413.4–5334<br>0FGL J0412.9–5341                | ... | fsrq  | PMN J0413–5332         |
| J0414.9–0840  | 63.734 | –8.675  | 201.850 | –38.605 | 0.161      | 0.131      | 26     | 5.3      | 0.3      | 0.1             | 4.2      | 0.8             | 2.40          | 0.15                 | PL  | ... | ...   | ...                                                                        | ... | ...   | ...                    |
| J0415.7–4351  | 63.941 | –43.865 | 249.109 | –45.978 | 0.206      | 0.190      | 60     | 7.6      | 0.4      | 0.1             | 5.1      | 0.7             | 2.48          | 0.12                 | PL  | ... | ...   | 2FGL J0416.0–4355                                                          | ... | ...   | ...                    |
| J0416.6–1850  | 64.159 | –18.841 | 214.296 | –42.369 | 0.052      | 0.048      | 72     | 19.8     | 1.1      | 0.1             | 14.0     | 1.0             | 2.34          | 0.06                 | PL  | T   | ...   | 2FGL J0416.7–1849<br>1FGL J0416.5–1851<br>3EG J0412–1853<br>EGR J0413–1851 | ... | fsrq  | PKS 0414–189           |
| J0416.8+0104  | 64.223 | 1.077   | 191.830 | –33.163 | 0.036      | 0.034      | 32     | 11.7     | 0.6      | 0.1             | 8.2      | 1.3             | 1.75          | 0.11                 | PL  | ... | ...   | 2FGL J0416.8+0105<br>1FGL J0416.8+0107                                     | P   | bl    | 1ES 0414+009           |
| J0418.0–0251  | 64.524 | –2.852  | 196.020 | –35.031 | 0.090      | 0.084      | –60    | 13.8     | 0.9      | 0.1             | 12.1     | 1.1             | 2.46          | 0.07                 | PL  | T   | ...   | ...                                                                        | ... | bcu   | PKS B0415–029          |
| J0418.2+3412  | 64.574 | 34.209  | 164.421 | –11.517 | 0.163      | 0.128      | –67    | 4.9      | 0.4      | 0.1             | 5.1      | 1.1             | 2.37          | 0.14                 | PL  | ... | ...   | ...                                                                        | ... | ...   | ...                    |
| J0418.5+3813c | 64.640 | 38.221  | 161.566 | –8.654  | 0.177      | 0.160      | –22    | 10.6     | 0.7      | 0.1             | 16.3     | 1.5             | 2.79          | 0.08                 | PL  | ... | 6     | 1FGL J0419.0+3811                                                          | ... | rdg   | 3C 111                 |
| J0419.1+6636  | 64.778 | 66.605  | 141.536 | 11.568  | 0.054      | 0.049      | –58    | 14.5     | 1.3      | 0.1             | 15.4     | 1.3             | 2.31          | 0.06                 | PL  | ... | 10    | 2FGL J0418.9+6636                                                          | ... | ...   | ...                    |
| J0420.4+1448  | 65.114 | 14.809  | 179.885 | –24.215 | 0.253      | 0.186      | –40    | 4.4      | 0.3      | 0.1             | 6.8      | 1.3             | 2.87          | 0.17                 | PL  | ... | ...   | ...                                                                        | ... | ...   | ...                    |
| J0420.4–6013  | 65.120 | –60.227 | 271.156 | –41.781 | 0.076      | 0.065      | –40    | 6.1      | 0.3      | 0.1             | 3.1      | 0.8             | 1.85          | 0.19                 | PL  | ... | ...   | ...                                                                        | ... | ...   | ...                    |
| J0420.6–3742  | 65.164 | –37.715 | 240.290 | –45.189 | 0.076      | 0.064      | 34     | 10.5     | 0.6      | 0.1             | 7.9      | 1.0             | 2.34          | 0.10                 | PL  | ... | ...   | 2FGL J0420.9–3743                                                          | ... | ...   | ...                    |
| J0421.6+1950  | 65.404 | 19.847  | 175.916 | –20.749 | 0.118      | 0.107      | 59     | 6.1      | 0.6      | 0.1             | 7.5      | 1.3             | 2.33          | 0.11                 | PL  | ... | ...   | ...                                                                        | ... | ...   | ...                    |
| J0422.1–0642  | 65.545 | –6.711  | 200.751 | –36.093 | 0.108      | 0.086      | –24    | 8.9      | 0.5      | 0.1             | 7.0      | 0.9             | 2.41          | 0.10                 | PL  | ... | ...   | 2FGL J0422.1–0645<br>1FGL J0422.0–0647                                     | ... | fsrq  | PMN J0422–0643         |
| J0423.2–0119  | 65.825 | –1.332  | 195.286 | –33.127 | 0.021      | 0.021      | –66    | 56.1     | 5.6      | 0.2             | 59.6     | 2.0             | 2.30          | ...                  | LP  | T   | ...   | 1FHL J0423.3–0121                                                          | ... | FSRQ  | PKS 0420–01            |

Table 1—Continued

| Name 3FGL     | R.A.   | Decl.   | $l$     | $b$     | $\theta_1$ | $\theta_2$ | $\phi$ | $\sigma$ | $F_{35}$ | $\Delta F_{35}$ | $S_{25}$ | $\Delta S_{25}$ | $\Gamma_{25}$ | $\Delta \Gamma_{25}$ | Mod | Var | Flags | $\gamma$ -ray Assoc.                                                             | TeV | Class | ID or Assoc.             |
|---------------|--------|---------|---------|---------|------------|------------|--------|----------|----------|-----------------|----------|-----------------|---------------|----------------------|-----|-----|-------|----------------------------------------------------------------------------------|-----|-------|--------------------------|
|               |        |         |         |         |            |            |        |          |          |                 |          |                 |               |                      |     |     |       | 2FGL J0423.2–0120<br>1FGL J0423.2–0118<br>0FGL J0423.1–0112<br>3EG J0422–0102    |     |       |                          |
| J0423.5+5442  | 65.900 | 54.706  | 150.487 | 3.612   | 0.150      | 0.112      | 80     | 4.4      | 0.7      | 0.2             | 12.9     | 3.1             | 2.63          | 0.15                 | PL  | ... | ...   | ...                                                                              | ... | ...   | ...                      |
| J0423.8+4150  | 65.968 | 41.833  | 159.698 | −5.390  | 0.022      | 0.021      | −85    | 28.0     | 2.9      | 0.2             | 33.9     | 2.2             | 1.89          | 0.04                 | PL  | ... | ...   | 1FHL J0423.8+4151<br>2FGL J0423.8+4149<br>1FGL J0423.8+4148                      | ... | bll   | 4C +41.11                |
| J0424.7+0035  | 66.178 | 0.595   | 193.582 | −31.795 | 0.042      | 0.042      | −69    | 22.0     | 1.9      | 0.1             | 21.3     | 1.4             | 2.20          | 0.05                 | PL  | T   | ...   | 2FGL J0424.7+0034<br>1FGL J0424.8+0036                                           | ... | bll   | PKS 0422+00              |
| J0425.0−5331  | 66.266 | −53.518 | 262.180 | −43.006 | 0.054      | 0.052      | 28     | 15.4     | 0.7      | 0.1             | 9.3      | 0.8             | 2.34          | 0.08                 | PL  | ... | ...   | 2FGL J0424.3−5332                                                                | ... | bll   | PMN J0425−5331           |
| J0425.2+6319  | 66.324 | 63.321  | 144.406 | 9.762   | 0.041      | 0.038      | −59    | 8.5      | 0.6      | 0.1             | 6.5      | 1.2             | 1.96          | 0.15                 | PL  | ... | ...   | 1FHL J0425.3+6320                                                                | ... | bcu   | 1RXS<br>J042523.0+632016 |
| J0425.8+5600  | 66.452 | 56.014  | 149.768 | 4.750   | 0.063      | 0.052      | −60    | 6.3      | 0.7      | 0.1             | 8.3      | 1.8             | 2.35          | 0.17                 | PL  | ... | 3     | 1FHL J0425.4+5601                                                                | ... | ...   | ...                      |
| J0426.3+3510  | 66.588 | 35.170  | 164.885 | −9.657  | 0.259      | 0.168      | −43    | 4.4      | 0.5      | 0.1             | 6.6      | 1.6             | 2.49          | 0.13                 | PL  | ... | ...   | ...                                                                              | ... | ...   | ...                      |
| J0426.3+6827  | 66.590 | 68.458  | 140.645 | 13.345  | 0.070      | 0.069      | −47    | 7.1      | 0.5      | 0.1             | 6.4      | 1.0             | 2.38          | 0.11                 | PL  | ... | ...   | ...                                                                              | ... | bcu   | 4C +68.25                |
| J0426.6+0459  | 66.674 | 4.993   | 189.670 | −28.932 | 0.152      | 0.110      | −54    | 7.9      | 0.6      | 0.1             | 10.1     | 1.4             | 2.56          | 0.10                 | PL  | ... | ...   | 2FGL J0426.6+0509c                                                               | ... | bcu   | 4C +04.15                |
| J0426.7+5437  | 66.681 | 54.617  | 150.867 | 3.874   | 0.071      | 0.068      | 35     | 14.2     | 2.3      | 0.2             | 21.3     | 2.7             | 2.48          | ...                  | LP  | ... | ...   | 2FGL J0426.7+5434<br>1FGL J0426.5+5437                                           | ... | ...   | ...                      |
| J0427.3−3900  | 66.836 | −39.006 | 242.169 | −43.926 | 0.082      | 0.072      | 43     | 14.7     | 1.0      | 0.1             | 18.2     | 1.5             | 2.67          | 0.06                 | PL  | T   | ...   | ...                                                                              | ... | bcu   | PMN J0427−3900           |
| J0427.9−6704  | 66.982 | −67.078 | 279.135 | −38.544 | 0.070      | 0.068      | −27    | 13.9     | 0.7      | 0.1             | 9.4      | 0.8             | 2.46          | 0.07                 | PL  | ... | ...   | 2FGL J0427.2−6705                                                                | ... | ...   | ...                      |
| J0428.6−3756  | 67.168 | −37.936 | 240.704 | −43.618 | 0.010      | 0.010      | −44    | 135.6    | 20.1     | 0.4             | 184.0    | 4.2             | 2.04          | ...                  | LP  | T   | ...   | 1FHL J0428.7−3756<br>2FGL J0428.6−3756<br>1FGL J0428.6−3756<br>0FGL J0428.7−3755 | ... | bll   | PKS 0426−380             |
| J0429.8+2843  | 67.452 | 28.723  | 170.240 | −13.477 | 0.069      | 0.056      | −83    | 6.2      | 0.6      | 0.1             | 6.7      | 1.3             | 1.96          | 0.13                 | PL  | ... | ...   | ...                                                                              | ... | bcu   | MG2 J042948+2843         |
| J0429.8+3611c | 67.469 | 36.195  | 164.622 | −8.435  | 0.314      | 0.227      | 83     | 4.7      | 0.7      | 0.1             | 8.8      | 1.8             | 2.37          | 0.12                 | PL  | ... | 4,5,6 | ...                                                                              | ... | ...   | ...                      |
| J0430.1−3103  | 67.543 | −31.066 | 231.402 | −42.532 | 0.104      | 0.094      | −25    | 4.9      | 0.2      | 0.1             | 2.6      | 0.7             | 1.97          | 0.18                 | PL  | ... | ...   | ...                                                                              | ... | ...   | ...                      |
| J0430.2−2508  | 67.552 | −25.137 | 223.624 | −41.251 | 0.089      | 0.067      | 18     | 7.6      | 0.4      | 0.1             | 5.1      | 0.8             | 2.19          | 0.12                 | PL  | ... | ...   | 2FGL J0430.4−2507<br>1FGL J0430.4−2509                                           | ... | bll   | PMN J0430−2507           |
| J0430.5+1655  | 67.626 | 16.927  | 179.761 | −21.004 | 0.079      | 0.061      | 47     | 9.2      | 0.8      | 0.1             | 10.7     | 1.4             | 2.40          | 0.10                 | PL  | ... | ...   | ...                                                                              | ... | bcu   | MG1 J043022+1655         |
| J0431.6+7403  | 67.903 | 74.058  | 136.574 | 17.361  | 0.046      | 0.039      | 30     | 12.0     | 0.6      | 0.1             | 6.9      | 0.9             | 1.99          | 0.09                 | PL  | ... | ...   | ...                                                                              | ... | bcu   | GB6 J0431+7403           |
| J0431.7+3503  | 67.931 | 35.056  | 165.727 | −8.929  | 0.226      | 0.189      | −55    | 7.9      | 0.9      | 0.2             | 10.7     | 1.6             | 2.51          | ...                  | LP  | ... | 3     | ...                                                                              | ... | ...   | ...                      |
| J0432.5+0539  | 68.136 | 5.661   | 189.987 | −27.354 | 0.166      | 0.137      | −35    | 6.1      | 0.4      | 0.1             | 8.1      | 1.3             | 2.69          | 0.13                 | PL  | ... | ...   | ...                                                                              | ... | ...   | ...                      |
| J0433.1+3228  | 68.292 | 32.478  | 167.871 | −10.435 | 0.060      | 0.051      | −90    | 6.7      | 0.5      | 0.1             | 5.3      | 1.1             | 1.97          | 0.14                 | PL  | ... | ...   | 2FGL J0433.7+3233                                                                | ... | bcu   | NVSS<br>J043307+322840   |
|               |        |         |         |         |            |            |        |          |          |                 |          |                 |               |                      |     |     |       | 1FGL J0433.5+3230                                                                |     |       |                          |



Table 1—Continued

| Name 3FGL     | R.A.   | Decl.   | $l$     | $b$     | $\theta_1$ | $\theta_2$ | $\phi$ | $\sigma$ | $F_{35}$ | $\Delta F_{35}$ | $S_{25}$ | $\Delta S_{25}$ | $\Gamma_{25}$ | $\Delta \Gamma_{25}$ | Mod | Var | Flags | $\gamma$ -ray Assoc.                                                                            | TeV | Class | ID or Assoc.             |
|---------------|--------|---------|---------|---------|------------|------------|--------|----------|----------|-----------------|----------|-----------------|---------------|----------------------|-----|-----|-------|-------------------------------------------------------------------------------------------------|-----|-------|--------------------------|
| J0433.6+2905  | 68.418 | 29.090  | 170.533 | -12.600 | 0.021      | 0.020      | 73     | 29.1     | 3.7      | 0.2             | 41.4     | 2.3             | 2.02          | 0.04                 | PL  | T   | ...   | 1FHL J0433.5+2905<br>2FGL J0433.5+2905<br>1FGL J0433.5+2905<br>3EG J0433+2908<br>EGR J0433+2906 | ... | bll   | MG2 J043337+2905         |
| J0433.7-6028  | 68.429 | -60.482 | 270.817 | -40.145 | 0.068      | 0.064      | -84    | 16.1     | 0.8      | 0.1             | 11.8     | 0.9             | 2.51          | 0.06                 | PL  | T   | ...   | 2FGL J0433.4-6029                                                                               | ... | bcu   | PKS 0432-606             |
| J0434.0-5726  | 68.509 | -57.442 | 266.938 | -40.887 | 0.067      | 0.061      | 26     | 10.0     | 0.5      | 0.1             | 5.4      | 0.8             | 2.00          | 0.11                 | PL  | ... | ...   | 1FHL J0434.1-5725                                                                               | ... | bcu   | SUMSS<br>J043344-572613  |
| J0434.0-2010  | 68.514 | -20.167 | 217.752 | -38.942 | 0.113      | 0.093      | 17     | 8.3      | 0.5      | 0.1             | 6.0      | 0.9             | 2.20          | 0.10                 | PL  | ... | ...   | 2FGL J0433.9-5726<br>2FGL J0434.1-2014<br>1FGL J0434.1-2018                                     | ... | bll   | TXS 0431-203             |
| J0434.3-1411c | 68.577 | -14.197 | 210.736 | -36.714 | 0.140      | 0.123      | 18     | 5.1      | 0.4      | 0.1             | 5.4      | 1.0             | 2.48          | 0.13                 | PL  | ... | 1,6   | ...                                                                                             | ... | ...   | ...                      |
| J0434.4-2341  | 68.623 | -23.694 | 222.142 | -39.922 | 0.115      | 0.103      | -64    | 7.2      | 0.4      | 0.1             | 5.3      | 0.8             | 2.35          | 0.11                 | PL  | ... | ...   | 2FGL J0435.1-2341                                                                               | ... | bcu   | PMN J0434-2342           |
| J0434.6+0921  | 68.666 | 9.360   | 186.959 | -24.793 | 0.162      | 0.107      | -10    | 6.6      | 0.6      | 0.1             | 6.2      | 1.1             | 2.11          | 0.14                 | PL  | ... | ...   | ...                                                                                             | ... | bcu   | TXS 0431+092             |
| J0437.2-4713  | 69.305 | -47.228 | 253.362 | -41.972 | 0.045      | 0.044      | -50    | 34.5     | 2.2      | 0.1             | 17.9     | 0.9             | 2.31          | ...                  | EC  | ... | ...   | 2FGL J0437.3-4712<br>1FGL J0437.2-4715                                                          | ... | PSR   | PSR J0437+4715           |
| J0437.7-7330  | 69.439 | -73.515 | 286.085 | -35.193 | 0.092      | 0.073      | 65     | 6.6      | 0.4      | 0.1             | 4.1      | 0.8             | 2.10          | 0.18                 | PL  | ... | ...   | 2FGL J0438.0-7331                                                                               | ... | ...   | ...                      |
| J0438.3-1258  | 69.583 | -12.982 | 209.850 | -35.329 | 0.115      | 0.091      | 21     | 5.7      | 0.4      | 0.1             | 4.2      | 0.9             | 2.11          | 0.16                 | PL  | ... | ...   | 2FGL J0439.0-1252<br>1FGL J0438.8-1250                                                          | ... | fsrq  | PKS 0436-129             |
| J0438.8-4519  | 69.702 | -45.322 | 250.787 | -41.797 | 0.064      | 0.060      | -23    | 15.8     | 0.8      | 0.1             | 10.8     | 0.9             | 2.39          | 0.07                 | PL  | ... | ...   | 2FGL J0438.8-4521                                                                               | ... | bll   | PKS 0437-454             |
| J0439.6-3159  | 69.903 | -31.989 | 233.079 | -40.707 | 0.067      | 0.057      | 67     | 6.4      | 0.3      | 0.1             | 3.4      | 0.9             | 1.77          | 0.17                 | PL  | ... | ...   | ...                                                                                             | ... | bcu   | 1RXS<br>J043931.4-320045 |
| J0439.9-1859  | 69.977 | -18.999 | 216.942 | -37.251 | 0.043      | 0.036      | 59     | 10.8     | 0.5      | 0.1             | 6.0      | 1.0             | 1.92          | 0.12                 | PL  | ... | ...   | 1FHL J0439.9-1858<br>2FGL J0439.8-1858<br>1FGL J0439.8-1857                                     | ... | bcu   | PMN J0439-1900           |
| J0440.3-2500  | 70.082 | -25.015 | 224.260 | -39.008 | 0.068      | 0.066      | 15     | 4.7      | 0.2      | 0.1             | 2.2      | 0.7             | 1.72          | 0.21                 | PL  | ... | ...   | ...                                                                                             | ... | bll   | RBS 0570                 |
| J0440.3+1444  | 70.093 | 14.734  | 183.171 | -20.479 | 0.159      | 0.114      | -61    | 7.4      | 0.8      | 0.1             | 9.9      | 1.4             | 2.39          | 0.10                 | PL  | ... | 1,3   | 2FGL J0440.4+1433                                                                               | ... | bcu   | TXS 0437+145             |
| J0440.8+2751  | 70.218 | 27.853  | 172.549 | -12.204 | 0.047      | 0.043      | -30    | 7.4      | 0.6      | 0.1             | 6.3      | 1.2             | 1.95          | 0.14                 | PL  | ... | ...   | 2FGL J0440.9+2749<br>1FGL J0440.6+2748                                                          | ... | bll   | B2 0437+27B              |
| J0442.6-0017  | 70.662 | -0.299  | 197.203 | -28.463 | 0.032      | 0.031      | -61    | 50.8     | 3.5      | 0.2             | 51.2     | 1.4             | 2.50          | 0.03                 | PL  | T   | ...   | 1FHL J0442.9-0017<br>2FGL J0442.7-0017<br>1FGL J0442.7-0019<br>3EG J0442-0033<br>EGR J0442+0027 | ... | fsrq  | PKS 0440-00              |
| J0444.5+3425  | 71.135 | 34.424  | 167.962 | -7.368  | 0.077      | 0.071      | -59    | 4.6      | 0.5      | 0.1             | 5.6      | 1.4             | 2.18          | 0.13                 | PL  | ... | ...   | ...                                                                                             | ... | bcu   | B2 0441+34               |
| J0444.6-6012  | 71.171 | -60.215 | 270.034 | -38.901 | 0.090      | 0.079      | -11    | 6.5      | 0.3      | 0.1             | 3.6      | 0.7             | 1.98          | 0.16                 | PL  | ... | ...   | 1FGL J0445.2-6008                                                                               | ... | fsrq  | PMN J0444-6014           |
| J0447.1-2540  | 71.795 | -25.676 | 225.602 | -37.695 | 0.109      | 0.096      | 43     | 7.1      | 0.4      | 0.1             | 5.2      | 0.8             | 2.50          | 0.13                 | PL  | ... | ...   | ...                                                                                             | ... | ...   | ...                      |

Table 1—Continued

| Name 3FGL    | R.A.   | Decl.   | $l$     | $b$     | $\theta_1$ | $\theta_2$ | $\phi$ | $\sigma$ | $F_{35}$ | $\Delta F_{35}$ | $S_{25}$ | $\Delta S_{25}$ | $\Gamma_{25}$ | $\Delta \Gamma_{25}$ | Mod | Var | Flags | $\gamma$ -ray Assoc.                                                                                                 | TeV | Class | ID or Assoc.              |
|--------------|--------|---------|---------|---------|------------|------------|--------|----------|----------|-----------------|----------|-----------------|---------------|----------------------|-----|-----|-------|----------------------------------------------------------------------------------------------------------------------|-----|-------|---------------------------|
| J0447.8–2119 | 71.966 | –21.329 | 220.459 | –36.264 | 0.223      | 0.172      | 35     | 5.2      | 0.3      | 0.1             | 4.5      | 0.9             | 2.55          | 0.15                 | PL  | ... | ...   | 2FGL J0448.6–2118                                                                                                    | ... | fsrq  | PKS 0446–212              |
| J0448.6–1632 | 72.158 | –16.534 | 215.023 | –34.428 | 0.034      | 0.033      | 45     | 15.8     | 0.9      | 0.1             | 10.7     | 1.3             | 1.86          | 0.08                 | PL  | ... | ...   | 1FHL J0448.5–1633<br>2FGL J0448.5–1633<br>1FGL J0448.5–1633                                                          | ... | bll   | RBS 0589                  |
| J0449.0+1121 | 72.251 | 11.359  | 187.409 | –20.760 | 0.052      | 0.050      | 71     | 35.6     | 2.8      | 0.2             | 42.0     | 1.5             | 2.55          | ...                  | LP  | T   | ...   | 2FGL J0448.9+1121<br>1FGL J0448.6+1118<br>3EG J0450+1105                                                             | ... | fsrq  | PKS 0446+11               |
| J0449.4–4350 | 72.362 | –43.836 | 248.806 | –39.912 | 0.012      | 0.011      | –75    | 96.5     | 10.3     | 0.3             | 123.1    | 3.8             | 1.85          | 0.02                 | PL  | T   | ...   | 1FHL J0449.4–4350<br>2FGL J0449.4–4350<br>1FGL J0449.5–4350<br>0FGL J0449.7–4348                                     | P   | bll   | PKS 0447–439              |
| J0451.6+7231 | 72.916 | 72.518  | 138.776 | 17.546  | 0.125      | 0.105      | –31    | 5.0      | 0.2      | 0.1             | 3.9      | 0.8             | 2.65          | 0.21                 | PL  | ... | ...   | ...                                                                                                                  | ... | ...   | ...                       |
| J0451.7+5722 | 72.940 | 57.373  | 151.114 | 8.320   | 0.065      | 0.063      | –13    | 6.0      | 0.5      | 0.1             | 6.7      | 1.2             | 2.49          | 0.14                 | PL  | ... | 4,10  | ...                                                                                                                  | ... | ...   | ...                       |
| J0453.2–2808 | 73.314 | –28.147 | 229.044 | –37.018 | 0.060      | 0.054      | 68     | 32.0     | 1.4      | 0.1             | 25.0     | 1.0             | 2.63          | 0.04                 | PL  | T   | ...   | 2FGL J0453.1–2807<br>1FGL J0453.2–2805                                                                               | ... | fsrq  | PKS 0451–28               |
| J0453.2+6321 | 73.317 | 63.366  | 146.447 | 12.174  | 0.049      | 0.040      | 63     | 10.5     | 0.7      | 0.1             | 8.8      | 1.1             | 2.35          | 0.09                 | PL  | ... | ...   | ...                                                                                                                  | ... | bcu   | NVSS 26<br>J045312+632117 |
| J0454.6–6825 | 73.659 | –68.432 | 279.654 | –35.709 | 0.143      | 0.122      | –55    | 6.3      | 0.5      | 0.1             | 5.4      | 1.0             | 2.20          | 0.11                 | PL  | ... | ...   | ...                                                                                                                  | ... | pwn   | PWN G279.8–35.8           |
| J0455.7–4617 | 73.945 | –46.285 | 251.992 | –38.826 | 0.056      | 0.054      | –40    | 30.0     | 1.5      | 0.1             | 22.8     | 1.0             | 2.55          | 0.04                 | PL  | T   | ...   | 2FGL J0456.1–4613<br>1FGL J0455.6–4618<br>3EG J0458–4635                                                             | ... | fsrq  | PKS 0454–46               |
| J0456.2–6924 | 74.067 | –69.408 | 280.748 | –35.283 | 0.160      | 0.105      | 22     | 9.9      | 0.8      | 0.1             | 9.3      | 1.1             | 2.31          | 0.08                 | PL  | ... | ...   | 2FGL J0455.8–6920                                                                                                    | ... | ...   | LMC field <sup>a</sup>    |
| J0456.3+2702 | 74.087 | 27.047  | 175.380 | –10.031 | 0.091      | 0.078      | –73    | 10.6     | 1.1      | 0.1             | 15.7     | 1.6             | 2.46          | 0.07                 | PL  | T   | ...   | 2FGL J0456.5+2658                                                                                                    | ... | bcu   | MG2 J045613+2702          |
| J0456.3–3131 | 74.090 | –31.521 | 233.354 | –37.123 | 0.163      | 0.126      | 4      | 9.0      | 0.4      | 0.1             | 6.2      | 0.8             | 2.54          | 0.10                 | PL  | T   | ...   | 2FGL J0456.5–3132<br>1FGL J0456.4–3132                                                                               | ... | fsrq  | PMN J0456–3135            |
| J0457.0–2324 | 74.264 | –23.412 | 223.708 | –34.895 | 0.013      | 0.013      | 66     | 161.1    | 18.0     | 0.3             | 176.4    | 2.7             | 2.21          | ...                  | LP  | T   | ...   | 1FHL J0457.1–2326<br>2FGL J0457.0–2325<br>1FGL J0457.0–2325<br>0FGL J0457.1–2325<br>3EG J0456–2338<br>EGR J0456–2334 | ... | FSRQ  | PKS 0454–234              |
| J0457.0+0643 | 74.269 | 6.725   | 192.727 | –21.689 | 0.245      | 0.173      | 57     | 4.9      | 0.4      | 0.1             | 5.7      | 1.2             | 2.55          | 0.17                 | PL  | ... | 9     | 1FGL J0457.9+0649                                                                                                    | ... | fsrq  | 4C +06.21                 |
| J0500.3+5237 | 75.091 | 52.618  | 155.652 | 6.349   | 0.054      | 0.047      | 5      | 8.6      | 0.7      | 0.1             | 9.2      | 1.3             | 2.35          | 0.09                 | PL  | ... | ...   | 1FGL J0500.1+5237                                                                                                    | ... | spp   | ...                       |
| J0501.2–0157 | 75.318 | –1.966  | 201.439 | –25.272 | 0.045      | 0.042      | –60    | 32.5     | 2.3      | 0.1             | 31.1     | 1.3             | 2.41          | 0.04                 | PL  | T   | ...   | 2FGL J0501.2–0155<br>1FGL J0501.0–0200<br>3EG J0500–0159                                                             | ... | fsrq  | S3 0458–02                |

Table 1—Continued

| Name 3FGL    | R.A.   | Decl.   | $l$     | $b$     | $\theta_1$ | $\theta_2$ | $\phi$ | $\sigma$ | $F_{35}$ | $\Delta F_{35}$ | $S_{25}$ | $\Delta S_{25}$ | $\Gamma_{25}$ | $\Delta \Gamma_{25}$ | Mod | Var | Flags | $\gamma$ -ray Assoc.                                                             | TeV | Class | ID or Assoc.             |
|--------------|--------|---------|---------|---------|------------|------------|--------|----------|----------|-----------------|----------|-----------------|---------------|----------------------|-----|-----|-------|----------------------------------------------------------------------------------|-----|-------|--------------------------|
| J0501.8+3046 | 75.469 | 30.777  | 173.130 | −6.802  | 0.064      | 0.055      | 25     | 6.3      | 0.6      | 0.1             | 6.2      | 1.3             | 2.12          | 0.16                 | PL  | ... | 3     | ...                                                                              | ... | bcu   | 1RXS<br>J050140.8+304831 |
| J0502.5+0612 | 75.626 | 6.214   | 193.966 | −20.825 | 0.180      | 0.148      | 61     | 5.9      | 0.4      | 0.1             | 8.3      | 1.6             | 2.71          | 0.14                 | PL  | ... | ...   | 2FGL J0502.5+0607<br>3EG J0459+0544                                              | ... | fsrq  | PKS 0459+060             |
| J0502.6+1759 | 75.655 | 17.995  | 183.708 | −14.246 | 0.202      | 0.174      | 2      | 4.4      | 0.4      | 0.1             | 6.7      | 1.5             | 2.54          | 0.15                 | PL  | ... | ...   | ...                                                                              | ... | ...   | ...                      |
| J0502.7+3438 | 75.686 | 34.650  | 170.148 | −4.307  | 0.086      | 0.072      | 30     | 8.6      | 0.9      | 0.1             | 11.4     | 1.5             | 2.29          | 0.09                 | PL  | T   | 3     | ...                                                                              | ... | bcu   | MG2 J050234+3436         |
| J0503.4+4522 | 75.865 | 45.375  | 161.721 | 2.336   | 0.101      | 0.073      | −33    | 8.1      | 0.9      | 0.1             | 11.1     | 1.5             | 2.36          | 0.10                 | PL  | ... | ...   | 2FGL J0503.3+4517                                                                | ... | bcu   | 1RXS<br>J050339.8+451715 |
| J0503.5+6538 | 75.889 | 65.633  | 145.244 | 14.409  | 0.072      | 0.061      | −72    | 5.4      | 0.3      | 0.1             | 3.6      | 0.9             | 2.21          | 0.17                 | PL  | ... | ...   | 1FGL J0503.2+4526                                                                | ... | bll   | 1E 0458.1+6530           |
| J0505.3+0459 | 76.343 | 4.998   | 195.475 | −20.861 | 0.042      | 0.041      | 34     | 24.7     | 2.7      | 0.2             | 30.5     | 2.0             | 2.43          | ...                  | LP  | T   | ...   | 2FGL J0505.5+0501                                                                | ... | fsrq  | PKS 0502+049             |
| J0505.3−0422 | 76.350 | −4.376  | 204.327 | −25.523 | 0.135      | 0.114      | 86     | 5.2      | 0.5      | 0.1             | 6.1      | 1.2             | 2.26          | 0.11                 | PL  | ... | ...   | 2FGL J0505.8−0411                                                                | ... | fsrq  | S3 0503−04               |
| J0505.5+0416 | 76.382 | 4.274   | 196.158 | −21.205 | 0.078      | 0.070      | −30    | 7.6      | 0.5      | 0.1             | 6.1      | 1.2             | 1.91          | 0.15                 | PL  | ... | ...   | 1FGL J0505.8−0416<br>1FHL J0505.4+0418<br>2FGL J0505.4+0419<br>1FGL J0505.2+0420 | ... | bll   | MG1 J050533+0415         |
| J0505.5−1558 | 76.383 | −15.974 | 216.223 | −30.460 | 0.066      | 0.063      | −20    | 6.3      | 0.4      | 0.1             | 4.1      | 0.8             | 2.10          | 0.14                 | PL  | ... | ...   | ...                                                                              | ... | bcu   | TXS 0503−160             |
| J0505.9+6114 | 76.482 | 61.245  | 149.085 | 12.095  | 0.056      | 0.051      | 83     | 6.5      | 0.4      | 0.1             | 5.0      | 1.0             | 2.01          | 0.15                 | PL  | ... | ...   | 2FGL J0505.9+6116                                                                | ... | bll   | NVSS<br>J050558+611336   |
| J0506.3−0357 | 76.587 | −3.952  | 204.036 | −25.115 | 0.169      | 0.125      | 43     | 4.3      | 0.4      | 0.1             | 4.7      | 1.2             | 2.17          | 0.13                 | PL  | ... | 5     | 1FGL J0505.8−0416                                                                | ... | ...   | ...                      |
| J0506.9+0321 | 76.735 | 3.362   | 197.192 | −21.375 | 0.090      | 0.069      | −56    | 4.6      | 0.2      | 0.1             | 2.9      | 0.9             | 1.80          | 0.22                 | PL  | ... | ...   | ...                                                                              | ... | ...   | ...                      |
| J0506.9−5435 | 76.743 | −54.584 | 262.420 | −36.773 | 0.032      | 0.029      | −86    | 14.9     | 0.6      | 0.1             | 9.0      | 1.4             | 1.60          | 0.09                 | PL  | ... | ...   | 1FHL J0506.9−5434<br>2FGL J0506.7−5435<br>1FGL J0506.9−5435                      | ... | bcu   | 1ES 0505−546             |
| J0507.1−6102 | 76.780 | −61.050 | 270.406 | −36.043 | 0.054      | 0.052      | −78    | 20.0     | 1.0      | 0.1             | 15.5     | 1.0             | 2.52          | 0.06                 | PL  | T   | ...   | 2FGL J0507.5−6102<br>1FGL J0507.3−6103                                           | ... | fsrq  | PKS 0506−61              |
| J0507.5−0906 | 76.888 | −9.102  | 209.298 | −27.191 | 0.183      | 0.095      | 0      | 5.6      | 0.4      | 0.1             | 4.9      | 0.9             | 2.34          | 0.14                 | PL  | ... | 1,9   | 2FGL J0506.5−0901                                                                | ... | ...   | ...                      |
| J0508.0+6736 | 77.004 | 67.614  | 143.807 | 15.891  | 0.014      | 0.014      | 45     | 39.3     | 2.1      | 0.1             | 35.5     | 2.4             | 1.52          | 0.04                 | PL  | T   | ...   | 1FHL J0508.1+6737<br>2FGL J0508.0+6737<br>1FGL J0507.9+6738<br>0FGL J0507.9+6739 | P   | bll   | 1ES 0502+675             |
| J0508.2−1936 | 77.062 | −19.613 | 220.442 | −31.191 | 0.165      | 0.144      | 12     | 4.6      | 0.3      | 0.1             | 3.3      | 0.7             | 2.37          | 0.16                 | PL  | ... | ...   | 2FGL J0508.1−1936                                                                | ... | bcu   | PMN J0508−1936           |
| J0509.3+1012 | 77.346 | 10.200  | 191.375 | −17.249 | 0.063      | 0.057      | −69    | 10.1     | 0.8      | 0.1             | 12.1     | 1.3             | 2.56          | 0.08                 | PL  | ... | ...   | 2FGL J0509.2+1013<br>1FGL J0509.2+1015                                           | ... | fsrq  | PKS 0506+101             |
| J0509.4+0541 | 77.364 | 5.699   | 195.404 | −19.628 | 0.016      | 0.016      | 76     | 54.5     | 6.5      | 0.2             | 72.3     | 2.6             | 2.04          | 0.03                 | PL  | T   | ...   | 1FHL J0509.5+0542<br>2FGL J0509.4+0542<br>1FGL J0509.3+0540<br>EGR J0509+0550    | ... | bll   | TXS 0506+056             |

Table 1—Continued

| Name 3FGL     | R.A.   | Decl.   | $l$     | $b$     | $\theta_1$ | $\theta_2$ | $\phi$ | $\sigma$ | $F_{35}$ | $\Delta F_{35}$ | $S_{25}$ | $\Delta S_{25}$ | $\Gamma_{25}$ | $\Delta \Gamma_{25}$ | Mod | Var | Flags | $\gamma$ -ray Assoc. | TeV | Class | ID or Assoc.   |
|---------------|--------|---------|---------|---------|------------|------------|--------|----------|----------|-----------------|----------|-----------------|---------------|----------------------|-----|-----|-------|----------------------|-----|-------|----------------|
| J0509.7–0400  | 77.427 | –4.010  | 204.528 | –24.403 | 0.111      | 0.094      | 27     | 4.1      | 0.2      | 0.1             | 2.7      | 1.0             | 1.65          | 0.23                 | PL  | ... | ...   | ...                  | ... | bll   | 1H 0506–039    |
| J0509.7–6418  | 77.439 | –64.305 | 274.295 | –35.207 | 0.068      | 0.061      | –41    | 8.5      | 0.4      | 0.1             | 4.5      | 0.8             | 2.00          | 0.14                 | PL  | ... | ...   | 1FHL J0509.9–6419    | ... | bcu   | RBS 0625       |
| J0510.0+1802  | 77.524 | 18.036  | 184.718 | –12.764 | 0.059      | 0.052      | 51     | 14.5     | 1.3      | 0.1             | 17.8     | 1.5             | 2.41          | 0.07                 | PL  | T   | ...   | 2FGL J0509.9+1802    | ... | fsrq  | PKS 0507+17    |
|               |        |         |         |         |            |            |        |          |          |                 |          |                 |               |                      |     |     |       | 1FGL J0510.0+1800    |     |       |                |
| J0512.0–3737  | 78.015 | –37.623 | 241.513 | –35.067 | 0.165      | 0.111      | –72    | 4.1      | 0.2      | 0.1             | 2.7      | 0.8             | 2.07          | 0.21                 | PL  | ... | ...   | ...                  | ... | ...   | ...            |
| J0512.2+2918  | 78.063 | 29.312  | 175.658 | –5.867  | 1.068      | 0.261      | 44     | 4.6      | 0.4      | 0.1             | 7.0      | 1.5             | 2.57          | 0.15                 | PL  | ... | 9     | ...                  | ... | bcu   | B2 0509+29     |
| J0512.9+4038  | 78.249 | 40.647  | 166.555 | 0.906   | 0.084      | 0.064      | –44    | 7.3      | 0.7      | 0.1             | 8.0      | 1.3             | 2.10          | 0.10                 | PL  | ... | ...   | 2FGL J0512.9+4040    | ... | bcu   | B3 0509+406    |
| J0514.4+5603  | 78.606 | 56.056  | 154.064 | 10.029  | 0.222      | 0.158      | 23     | 7.2      | 0.4      | 0.1             | 8.6      | 1.2             | 2.71          | 0.12                 | PL  | ... | 1,4   | 3EG J0510+5545       | ... | fsrq  | TXS 0510+559   |
| J0514.6–4406  | 78.675 | –44.113 | 249.474 | –35.393 | 0.167      | 0.154      | 11     | 9.0      | 0.4      | 0.1             | 4.7      | 0.8             | 2.61          | ...                  | LP  | ... | ...   | 2FGL J0515.0–4411    | ... | ...   | ...            |
|               |        |         |         |         |            |            |        |          |          |                 |          |                 |               |                      |     |     |       | 1FGL J0515.6–4404    |     |       |                |
| J0515.3–4557  | 78.831 | –45.954 | 251.737 | –35.429 | 0.172      | 0.132      | –33    | 5.0      | 0.3      | 0.1             | 4.4      | 1.0             | 2.44          | 0.18                 | PL  | ... | ...   | 2FGL J0516.5–4601    | ... | fsrq  | PKS 0514–459   |
| J0515.5–0123  | 78.893 | –1.397  | 202.787 | –21.871 | 0.056      | 0.053      | 57     | 4.6      | 0.2      | 0.1             | 2.8      | 0.9             | 1.75          | 0.18                 | PL  | ... | ...   | ...                  | ... | bcu   | NVSS           |
|               |        |         |         |         |            |            |        |          |          |                 |          |                 |               |                      |     |     |       |                      |     |       | J051536–012427 |
| J0515.8+1526  | 78.964 | 15.439  | 187.719 | –13.068 | 0.035      | 0.034      | 28     | 15.9     | 1.5      | 0.1             | 16.8     | 1.6             | 2.07          | 0.07                 | PL  | ... | ...   | 1FHL J0515.9+1528    | ... | bll   | GB6 J0515+1527 |
|               |        |         |         |         |            |            |        |          |          |                 |          |                 |               |                      |     |     |       | 2FGL J0515.9+1528    |     |       |                |
|               |        |         |         |         |            |            |        |          |          |                 |          |                 |               |                      |     |     |       | 1FGL J0515.9+1528    |     |       |                |
| J0516.3+7351  | 79.095 | 73.859  | 138.618 | 19.774  | 0.050      | 0.045      | 81     | 9.5      | 0.5      | 0.1             | 5.4      | 0.8             | 1.97          | 0.14                 | PL  | ... | ...   | 1FHL J0516.4+7351    | ... | bll   | GB6 J0516+7350 |
|               |        |         |         |         |            |            |        |          |          |                 |          |                 |               |                      |     |     |       | 2FGL J0515.5+7355    |     |       |                |
|               |        |         |         |         |            |            |        |          |          |                 |          |                 |               |                      |     |     |       | 1FGL J0515.2+7355    |     |       |                |
| J0516.6+1012  | 79.170 | 10.206  | 192.374 | –15.731 | 0.080      | 0.064      | 7      | 4.3      | 0.3      | 0.1             | 3.5      | 1.2             | 2.00          | 0.30                 | PL  | ... | ...   | ...                  | ... | ...   | ...            |
| J0516.7–6207  | 79.189 | –62.121 | 271.513 | –34.760 | 0.027      | 0.025      | 80     | 38.5     | 2.8      | 0.1             | 31.3     | 1.4             | 2.15          | 0.03                 | PL  | T   | ...   | 1FHL J0516.6–6209    | ... | bll   | PKS 0516–621   |
|               |        |         |         |         |            |            |        |          |          |                 |          |                 |               |                      |     |     |       | 2FGL J0516.8–6207    |     |       |                |
|               |        |         |         |         |            |            |        |          |          |                 |          |                 |               |                      |     |     |       | 1FGL J0516.7–6207    |     |       |                |
|               |        |         |         |         |            |            |        |          |          |                 |          |                 |               |                      |     |     |       | 0FGL J0516.2–6200    |     |       |                |
|               |        |         |         |         |            |            |        |          |          |                 |          |                 |               |                      |     |     |       | 3EG J0512–6150       |     |       |                |
| J0517.1+2628c | 79.291 | 26.479  | 178.616 | –6.616  | 0.122      | 0.108      | –32    | 7.0      | 0.8      | 0.1             | 12.7     | 1.8             | 2.53          | 0.10                 | PL  | ... | 1,3,6 | 2FGL J0516.7+2634    | ... | ...   | ...            |
| J0517.4+4540  | 79.373 | 45.668  | 162.941 | 4.492   | 0.227      | 0.104      | 86     | 4.7      | 0.4      | 0.1             | 6.3      | 1.3             | 2.46          | 0.14                 | PL  | T   | 4     | 2FGL J0517.0+4532    | ... | fsrq  | 4C +45.08      |
| J0517.5+0902  | 79.394 | 9.037   | 193.527 | –16.163 | 0.114      | 0.089      | –8     | 4.8      | 0.5      | 0.1             | 6.4      | 1.9             | 2.30          | 0.18                 | PL  | ... | 5     | 2FGL J0517.5+0900    | ... | fsrq  | PMN J0517+0858 |
|               |        |         |         |         |            |            |        |          |          |                 |          |                 |               |                      |     |     |       | 1FGL J0517.6+0857    |     |       |                |
| J0519.2–4542  | 79.809 | –45.707 | 251.500 | –34.731 | 0.154      | 0.117      | –39    | 4.7      | 0.3      | 0.1             | 4.7      | 1.2             | 2.49          | 0.18                 | PL  | ... | ...   | ...                  | ... | rdg   | Pictor A       |
| J0519.3+2746  | 79.850 | 27.773  | 177.831 | –5.470  | 0.114      | 0.107      | –13    | 4.3      | 0.5      | 0.1             | 6.1      | 1.7             | 2.33          | 0.18                 | PL  | ... | ...   | ...                  | ... | bcu   | 4C +27.15      |
| J0519.5+0852  | 79.877 | 8.871   | 193.935 | –15.844 | 0.142      | 0.121      | –64    | 7.9      | 1.1      | 0.2             | 11.1     | 1.9             | 2.42          | ...                  | LP  | ... | 1     | ...                  | ... | bcu   | TXS 0516+087   |
| J0521.4–1740  | 80.353 | –17.676 | 219.666 | –27.584 | 0.103      | 0.095      | –18    | 8.0      | 0.5      | 0.1             | 6.4      | 0.9             | 2.43          | 0.11                 | PL  | ... | ...   | 2FGL J0521.4–1736    | ... | fsrq  | TXS 0519–176   |
| J0521.7+0103  | 80.436 | 1.058   | 201.295 | –19.330 | 0.071      | 0.059      | 84     | 6.7      | 0.3      | 0.1             | 4.2      | 1.0             | 1.70          | 0.17                 | PL  | ... | ...   | 2FGL J0521.9+0108    | ... | bcu   | NVSS           |
|               |        |         |         |         |            |            |        |          |          |                 |          |                 |               |                      |     |     |       |                      |     |       | J052140+010257 |
|               |        |         |         |         |            |            |        |          |          |                 |          |                 |               |                      |     |     |       | 1FGL J0521.6+0103    |     |       |                |
| J0521.7+2113  | 80.443 | 21.222  | 183.599 | –8.702  | 0.014      | 0.014      | –37    | 53.7     | 7.9      | 0.3             | 90.8     | 3.3             | 1.92          | 0.02                 | PL  | T   | ...   | 1FHL J0521.7+2113    | P   | bll   | TXS 0518+211   |

Table 1—Continued

| Name 3FGL     | R.A.   | Decl.   | $l$     | $b$     | $\theta_1$ | $\theta_2$ | $\phi$ | $\sigma$ | $F_{35}$ | $\Delta F_{35}$ | $S_{25}$ | $\Delta S_{25}$ | $\Gamma_{25}$ | $\Delta \Gamma_{25}$ | Mod | Var | Flags | $\gamma$ -ray Assoc.                                                               | TeV | Class | ID or Assoc.           |
|---------------|--------|---------|---------|---------|------------|------------|--------|----------|----------|-----------------|----------|-----------------|---------------|----------------------|-----|-----|-------|------------------------------------------------------------------------------------|-----|-------|------------------------|
|               |        |         |         |         |            |            |        |          |          |                 |          |                 |               |                      |     |     |       | 2FGL J0521.7+2113<br>1FGL J0521.7+2114                                             |     |       |                        |
| J0521.9–3847  | 80.476 | –38.785 | 243.289 | –33.354 | 0.299      | 0.174      | 16     | 4.5      | 0.2      | 0.1             | 4.0      | 0.9             | 2.63          | 0.18                 | PL  | T   | ...   | ...                                                                                | ... | bcu   | PKS 0520–388           |
| J0522.9–3628  | 80.742 | –36.472 | 240.623 | –32.718 | 0.025      | 0.023      | –8     | 70.4     | 4.7      | 0.2             | 61.8     | 1.6             | 2.44          | ...                  | LP  | T   | ...   | 1FHL J0523.3–3620<br>2FGL J0523.0–3628                                             | ... | BCU   | PKS 0521–36            |
|               |        |         |         |         |            |            |        |          |          |                 |          |                 |               |                      |     |     |       | 1FGL J0522.8–3632<br>2FGL J0523.3–2530                                             | ... | ...   | ...                    |
| J0523.3–2528  | 80.839 | –25.476 | 228.202 | –29.826 | 0.042      | 0.041      | 14     | 26.1     | 1.8      | 0.1             | 19.9     | 1.2             | 2.15          | 0.04                 | PL  | ... | 10    | 1FGL J0523.5–2529                                                                  | ... | ...   | ...                    |
| J0523.7+3328  | 80.932 | 33.474  | 173.651 | –1.473  | 0.227      | 0.160      | –70    | 6.4      | 0.6      | 0.1             | 11.0     | 1.6             | 2.63          | 0.11                 | PL  | ... | 1     | ...                                                                                | ... | ...   | ...                    |
| J0524.4+2839  | 81.124 | 28.655  | 177.735 | –4.046  | 0.060      | 0.046      | –78    | 9.2      | 0.9      | 0.1             | 10.0     | 1.5             | 2.12          | 0.11                 | PL  | ... | 3     | 2FGL J0524.1+2843<br>1FGL J0524.1+2842                                             | ... | ...   | ...                    |
| J0524.5–6937  | 81.128 | –69.629 | 280.300 | –32.832 | 0.056      | 0.049      | –11    | 5.7      | 0.2      | 0.1             | 3.6      | 1.0             | 1.63          | 0.19                 | PL  | ... | 1     | ...                                                                                | ... | ...   | LMC field <sup>a</sup> |
| J0525.2–6614  | 81.324 | –66.244 | 276.296 | –33.295 | 0.098      | 0.086      | 77     | 5.7      | 0.4      | 0.1             | 4.9      | 1.0             | 2.11          | 0.16                 | PL  | ... | ...   | ...                                                                                | ... | ...   | LMC field <sup>a</sup> |
| J0525.3–4558  | 81.331 | –45.970 | 251.933 | –33.699 | 0.116      | 0.090      | 59     | 5.5      | 0.3      | 0.1             | 3.6      | 0.8             | 2.20          | 0.16                 | PL  | ... | ...   | ...                                                                                | ... | fsrq  | PKS 0524–460           |
| J0525.6–6013  | 81.415 | –60.232 | 269.113 | –33.873 | 0.039      | 0.038      | –6     | 13.1     | 0.6      | 0.1             | 7.7      | 1.2             | 1.73          | 0.10                 | PL  | ... | ...   | 2FGL J0525.5–6011                                                                  | ... | bcu   | SUMSS J052542+601341   |
| J0525.8–2014  | 81.451 | –20.248 | 222.795 | –27.554 | 0.129      | 0.115      | 88     | 5.3      | 0.3      | 0.1             | 3.6      | 0.8             | 2.06          | 0.16                 | PL  | ... | ...   | ...                                                                                | ... | bcu   | PMN J0525–2010         |
| J0526.0+4253  | 81.523 | 42.889  | 166.112 | 4.191   | 0.160      | 0.141      | 67     | 7.2      | 0.7      | 0.1             | 9.7      | 1.4             | 2.44          | 0.09                 | PL  | ... | ...   | 2FGL J0526.6+4308                                                                  | ... | bcu   | NVSS J052520+425520    |
| J0526.2–4829  | 81.571 | –48.499 | 254.979 | –33.753 | 0.043      | 0.041      | 29     | 18.3     | 1.4      | 0.1             | 17.1     | 1.3             | 2.29          | 0.06                 | PL  | T   | ...   | 2FGL J0526.1–4829<br>1FGL J0526.3–4829                                             | ... | fsrq  | PKS 0524–485           |
| J0526.4+2247  | 81.609 | 22.798  | 182.875 | –6.931  | 0.055      | 0.049      | 42     | 6.0      | 0.7      | 0.1             | 8.9      | 2.3             | 2.40          | 0.17                 | PL  | ... | ...   | 2FGL J0526.6+2248                                                                  | ... | ...   | ...                    |
| J0526.6–6825e | 81.650 | –68.420 | 278.843 | –32.850 | ...        | ...        | ...    | 83.8     | 20.2     | 0.4             | 192.3    | 4.0             | 2.15          | ...                  | LP  | ... | ...   | 0FGL J0538.4–6856<br>1FGL J0538.9–6914<br>1FHL J0526.6–6825e<br>2FGL J0526.6–6825e | ... | GAL   | LMC                    |
| J0526.6+6321  | 81.660 | 63.359  | 148.613 | 15.264  | 0.177      | 0.117      | 26     | 6.2      | 0.3      | 0.1             | 5.2      | 0.8             | 2.54          | 0.12                 | PL  | ... | ...   | 2FGL J0526.8+6326                                                                  | ... | bcu   | GB6 J0526+6317         |
| J0527.3+6647  | 81.836 | 66.785  | 145.568 | 17.050  | 0.086      | 0.065      | –88    | 5.0      | 0.2      | 0.1             | 2.4      | 0.7             | 1.85          | 0.20                 | PL  | ... | ...   | 1FGL J0527.6+6646                                                                  | ... | ...   | ...                    |
| J0528.3+1815  | 82.078 | 18.261  | 186.960 | –9.032  | 0.063      | 0.058      | –52    | 4.9      | 0.2      | 0.1             | 3.3      | 1.0             | 1.65          | 0.21                 | PL  | ... | ...   | ...                                                                                | ... | bcu   | 1RXS J052829.6+181657  |
| J0529.1+0933  | 82.288 | 9.557   | 194.608 | –13.454 | 0.073      | 0.064      | 82     | 8.2      | 0.8      | 0.1             | 9.3      | 1.4             | 2.32          | 0.12                 | PL  | ... | ...   | 1FHL J0529.0+0937<br>2FGL J0529.2+0935                                             | ... | bcu   | GB6 J0529+0934         |
| J0529.2–5917  | 82.300 | –59.299 | 267.964 | –33.480 | 0.099      | 0.082      | –90    | 5.6      | 0.3      | 0.1             | 3.6      | 0.8             | 2.37          | 0.22                 | PL  | ... | ...   | ...                                                                                | ... | bll   | 1RXS J052846.9–592000  |
| J0529.2+3822  | 82.309 | 38.367  | 170.214 | 2.183   | 0.116      | 0.103      | 85     | 9.1      | 1.0      | 0.1             | 15.1     | 1.7             | 2.53          | 0.08                 | PL  | ... | 1,3   | 2FGL J0529.3+3821                                                                  | ... | ...   | ...                    |
| J0529.8–7242  | 82.453 | –72.716 | 283.797 | –31.843 | 0.076      | 0.072      | –17    | 8.7      | 0.5      | 0.1             | 7.1      | 1.0             | 2.48          | 0.10                 | PL  | T   | ...   | ...                                                                                | ... | bcu   | PKS 0530–727           |
| J0530.8+1330  | 82.719 | 13.515  | 191.375 | –11.034 | 0.042      | 0.039      | 14     | 35.9     | 3.7      | 0.2             | 49.6     | 1.8             | 2.51          | ...                  | LP  | T   | ...   | 2FGL J0530.8+1333<br>1FGL J0531.0+1331<br>0FGL J0531.0+1331                        | ... | FSRQ  | PKS 0528+134           |

Table 1—Continued

| Name 3FGL     | R.A.   | Decl.   | $l$     | $b$     | $\theta_1$ | $\theta_2$ | $\phi$ | $\sigma$ | $F_{35}$ | $\Delta F_{35}$ | $S_{25}$ | $\Delta S_{25}$ | $\Gamma_{25}$ | $\Delta \Gamma_{25}$ | Mod | Var | Flags | $\gamma$ -ray Assoc.                                                                             | TeV | Class | ID or Assoc.           |
|---------------|--------|---------|---------|---------|------------|------------|--------|----------|----------|-----------------|----------|-----------------|---------------|----------------------|-----|-----|-------|--------------------------------------------------------------------------------------------------|-----|-------|------------------------|
| J0532.0–4827  | 83.000 | –48.458 | 255.024 | –32.805 | 0.016      | 0.016      | 63     | 73.8     | 8.4      | 0.2             | 77.9     | 2.7             | 2.10          | ...                  | LP  | T   | ...   | 3EG J0530+1323<br>EGR J0530+1331<br>1FHL J0532.1–4826                                            | ... | BCU   | PMN J0531–4827         |
| J0532.7+0732  | 83.177 | 7.545   | 196.850 | –13.726 | 0.026      | 0.024      | 70     | 50.9     | 5.9      | 0.2             | 63.0     | 2.1             | 2.32          | ...                  | LP  | T   | ...   | 2FGL J0532.0–4826<br>1FGL J0532.9+0733                                                           | ... | FSRQ  | OG 050                 |
| J0533.0–3939  | 83.258 | –39.664 | 244.771 | –31.392 | 0.199      | 0.127      | 60     | 6.8      | 0.4      | 0.1             | 5.5      | 0.9             | 2.49          | 0.13                 | PL  | ... | ...   | 2FGL J0532.7+0733<br>...                                                                         | ... | bcu   | PKS 0531–397           |
| J0533.2+4822  | 83.307 | 48.378  | 162.161 | 8.223   | 0.032      | 0.030      | –68    | 32.9     | 2.9      | 0.2             | 37.5     | 1.5             | 2.39          | 0.03                 | PL  | T   | ...   | 1FGL J0533.0+4825<br>3EG J0533+4751                                                              | ... | fsrq  | TXS 0529+483           |
| J0533.2+5944  | 83.311 | 59.742  | 152.249 | 14.111  | 0.170      | 0.152      | 64     | 5.9      | 0.4      | 0.1             | 6.8      | 1.1             | 2.64          | 0.11                 | PL  | ... | ...   | ...                                                                                              | ... | ...   | ...                    |
| J0533.6–8323  | 83.411 | –83.385 | 295.787 | –29.149 | 0.051      | 0.049      | –89    | 11.7     | 0.8      | 0.1             | 9.8      | 1.0             | 2.30          | 0.08                 | PL  | T   | ...   | 2FGL J0533.0–8324<br>1FGL J0533.0–8324                                                           | ... | fsrq  | PKS 0541–834           |
| J0533.8–3754  | 83.464 | –37.905 | 242.793 | –30.887 | 0.095      | 0.052      | 12     | 7.2      | 0.4      | 0.1             | 5.4      | 0.9             | 2.34          | 0.12                 | PL  | ... | 9     | ...                                                                                              | ... | ...   | ...                    |
| J0534.0+6759  | 83.504 | 68.000  | 144.774 | 18.197  | 0.046      | 0.041      | 22     | 18.3     | 1.4      | 0.1             | 9.6      | 0.9             | 2.09          | ...                  | EC  | ... | ...   | 2FGL J0533.9+6759<br>1FGL J0533.9+6758                                                           | ... | PSR   | PSR J0533+6759         |
| J0534.5+2201i | 83.633 | 22.020  | 184.553 | –5.781  | ...        | ...        | ...    | ...      | 27.1     | ...             | 392.6    | ...             | 1.64          | ...                  | PL  | ... | ...   | 1FHL J0534.5+2201<br>2FGL J0534.5+2201<br>0FGL J0534.6+2201<br>EGR J0534+2159<br>1AGL J0535+2205 | P   | PWN   | Crab                   |
| J0534.5+2201s | 83.633 | 22.020  | 184.553 | –5.781  | ...        | ...        | ...    | 16.4     | 0.0      | 0.0             | 51.9     | 6.0             | 5.72          | 0.38                 | PL  | T   | 3,5   | 1FHL J0534.5+2201<br>2FGL J0534.5+2201<br>0FGL J0534.6+2201<br>EGR J0534+2159<br>1AGL J0535+2205 | P   | PWN   | Crab                   |
| J0534.5+2201  | 83.637 | 22.024  | 184.552 | –5.776  | 0.012      | 0.011      | 90     | 30.7     | 157.3    | 1.1             | 1471.9   | 10.6            | 2.23          | ...                  | EC  | T   | 3,5   | 1FHL J0534.5+2201                                                                                | P   | PSR   | PSR J0534+2200         |
| J0535.3–6559  | 83.828 | –65.997 | 275.865 | –32.317 | 0.052      | 0.051      | –31    | 7.8      | 0.5      | 0.1             | 6.0      | 1.0             | 2.20          | 0.12                 | PL  | ... | 3     | ...                                                                                              | ... | ...   | LMC field <sup>a</sup> |
| J0535.6–2749  | 83.921 | –27.817 | 231.709 | –27.921 | 0.235      | 0.168      | –44    | 4.3      | 0.2      | 0.1             | 3.3      | 0.9             | 2.41          | 0.18                 | PL  | ... | ...   | ...                                                                                              | ... | bcu   | PMN J0535–2751         |
| J0535.7–0617c | 83.935 | –6.291  | 209.920 | –19.686 | 0.099      | 0.089      | –88    | 6.2      | 1.0      | 0.2             | 12.6     | 2.1             | 2.40          | 0.10                 | PL  | ... | 1,5,6 | ...                                                                                              | ... | ...   | ...                    |
| J0536.4–3347  | 84.101 | –33.788 | 238.296 | –29.436 | 0.038      | 0.029      | 8      | 26.1     | 1.6      | 0.1             | 19.8     | 1.1             | 2.29          | 0.05                 | PL  | T   | 7     | 1FHL J0536.4–3343<br>2FGL J0536.2–3348<br>1FGL J0536.2–3348                                      | ... | ...   | ...                    |
| J0537.0–7113  | 84.254 | –71.221 | 281.955 | –31.542 | 0.250      | 0.158      | 65     | 5.1      | 0.4      | 0.1             | 5.1      | 1.1             | 2.45          | 0.13                 | PL  | ... | 1     | ...                                                                                              | ... | ...   | LMC field <sup>a</sup> |
| J0537.0+0957  | 84.266 | 9.950   | 195.285 | –11.578 | 0.229      | 0.137      | 61     | 11.5     | 0.7      | 0.1             | 13.6     | 1.5             | 2.68          | ...                  | LP  | T   | ...   | ...                                                                                              | ... | ...   | ...                    |

Table 1—Continued

| Name 3FGL     | R.A.   | Decl.   | $l$     | $b$     | $\theta_1$ | $\theta_2$ | $\phi$ | $\sigma$ | $F_{35}$ | $\Delta F_{35}$ | $S_{25}$ | $\Delta S_{25}$ | $\Gamma_{25}$ | $\Delta \Gamma_{25}$ | Mod | Var | Flags | $\gamma$ -ray Assoc. | TeV | Class | ID or Assoc.             |
|---------------|--------|---------|---------|---------|------------|------------|--------|----------|----------|-----------------|----------|-----------------|---------------|----------------------|-----|-----|-------|----------------------|-----|-------|--------------------------|
| J0537.4+3604c | 84.351 | 36.075  | 173.023 | 2.301   | 0.080      | 0.067      | 21     | 4.5      | 0.7      | 0.2             | 8.3      | 2.1             | 2.27          | 0.13                 | PL  | ... | 6     | ...                  | ... | ...   | ...                      |
| J0537.4–5717  | 84.362 | –57.293 | 265.552 | –32.429 | 0.066      | 0.057      | –81    | 8.4      | 0.4      | 0.1             | 4.9      | 0.8             | 2.05          | 0.14                 | PL  | ... | 10    | 2FGL J0537.7–5716    | ... | bll   | SUMSS<br>J053748–571828  |
|               |        |         |         |         |            |            |        |          |          |                 |          |                 |               |                      |     |     |       | 1FGL J0537.7–5717    |     |       |                          |
| J0538.4–3909  | 84.609 | –39.166 | 244.441 | –30.270 | 0.081      | 0.066      | –38    | 6.5      | 0.3      | 0.1             | 3.7      | 0.8             | 2.04          | 0.17                 | PL  | ... | ...   | 2FGL J0538.5–3909    | ... | bcu   | NVSS<br>J053810–390844   |
|               |        |         |         |         |            |            |        |          |          |                 |          |                 |               |                      |     |     |       | 1FGL J0538.4–3910    |     |       |                          |
| J0538.8–4405  | 84.709 | –44.086 | 250.083 | –31.090 | 0.009      | 0.009      | –19    | 219.2    | 33.0     | 0.4             | 308.4    | 4.9             | 2.04          | ...                  | LP  | T   | ...   | 1FHL J0538.8–4405    | ... | BLL   | PKS 0537–441             |
|               |        |         |         |         |            |            |        |          |          |                 |          |                 |               |                      |     |     |       | 2FGL J0538.8–4405    |     |       |                          |
|               |        |         |         |         |            |            |        |          |          |                 |          |                 |               |                      |     |     |       | 1FGL J0538.8–4404    |     |       |                          |
|               |        |         |         |         |            |            |        |          |          |                 |          |                 |               |                      |     |     |       | 0FGL J0538.8–4403    |     |       |                          |
|               |        |         |         |         |            |            |        |          |          |                 |          |                 |               |                      |     |     |       | 3EG J0540–4402       |     |       |                          |
|               |        |         |         |         |            |            |        |          |          |                 |          |                 |               |                      |     |     |       | EGR J0540–4358       |     |       |                          |
|               |        |         |         |         |            |            |        |          |          |                 |          |                 |               |                      |     |     |       | 1AGL J0538–4424      |     |       |                          |
| J0538.8–0341  | 84.709 | –3.696  | 207.847 | –17.821 | 0.221      | 0.187      | 15     | 4.6      | 0.5      | 0.1             | 7.6      | 1.5             | 2.56          | 0.13                 | PL  | ... | 3     | ...                  | ... | ...   | ...                      |
| J0538.9+1646  | 84.749 | 16.773  | 189.598 | –7.660  | 0.058      | 0.049      | 15     | 5.9      | 0.4      | 0.1             | 5.0      | 1.2             | 1.89          | 0.14                 | PL  | ... | ...   | ...                  | ... | ...   | ...                      |
| J0539.2–0536  | 84.801 | –5.601  | 209.678 | –18.607 | 0.269      | 0.226      | 65     | 7.3      | 0.6      | 0.1             | 10.8     | 1.5             | 2.55          | ...                  | LP  | ... | 12    | 2FGL J0538.5–0534c   | ... | ...   | ...                      |
|               |        |         |         |         |            |            |        |          |          |                 |          |                 |               |                      |     |     |       | 1FGL J0540.9–0547    |     |       | –31–                     |
| J0539.8+1434  | 84.957 | 14.571  | 191.606 | –8.630  | 0.075      | 0.067      | 74     | 7.6      | 0.8      | 0.1             | 9.9      | 1.4             | 2.32          | 0.09                 | PL  | T   | ...   | ...                  | ... | fsrq  | TXS 0536+145             |
| J0539.9–7553  | 84.985 | –75.884 | 287.290 | –30.586 | 0.092      | 0.071      | 6      | 8.1      | 0.5      | 0.1             | 6.1      | 0.9             | 2.33          | 0.11                 | PL  | ... | ...   | 2FGL J0540.1–7554    | ... | ...   | ...                      |
| J0540.0+1208  | 85.002 | 12.148  | 193.735 | –9.837  | 0.072      | 0.064      | 59     | 5.3      | 0.4      | 0.1             | 4.9      | 1.2             | 2.11          | 0.18                 | PL  | ... | ...   | ...                  | ... | ...   | ...                      |
| J0540.0–2837  | 85.012 | –28.627 | 232.909 | –27.251 | 0.076      | 0.073      | 31     | 18.1     | 0.8      | 0.1             | 17.3     | 1.1             | 2.78          | 0.06                 | PL  | T   | ...   | 2FGL J0539.3–2841    | ... | fsrq  | PKS 0537–286             |
|               |        |         |         |         |            |            |        |          |          |                 |          |                 |               |                      |     |     |       | 1FGL J0539.1–2847    |     |       |                          |
| J0540.3+2756e | 85.100 | 27.940  | 180.245 | –1.500  | ...        | ...        | ...    | 20.9     | 7.1      | 0.4             | 80.6     | 4.5             | 2.19          | 0.03                 | PL  | ... | ...   | 1FGL J0538.6+2717    | ... | SNR   | S147                     |
|               |        |         |         |         |            |            |        |          |          |                 |          |                 |               |                      |     |     |       | 2FGL J0538.1+2718    |     |       |                          |
|               |        |         |         |         |            |            |        |          |          |                 |          |                 |               |                      |     |     |       | ...                  |     |       |                          |
| J0540.4+5823  | 85.124 | 58.390  | 153.935 | 14.255  | 0.030      | 0.027      | –79    | 14.1     | 0.9      | 0.1             | 10.2     | 1.1             | 2.00          | 0.09                 | PL  | ... | ...   | 1FHL J0540.5+5822    | ... | bll   | GB6 J0540+5823           |
|               |        |         |         |         |            |            |        |          |          |                 |          |                 |               |                      |     |     |       | 2FGL J0540.4+5822    |     |       |                          |
| J0540.5–5416  | 85.148 | –54.268 | 261.998 | –31.888 | 0.103      | 0.086      | 40     | 14.2     | 0.7      | 0.1             | 12.0     | 0.9             | 2.63          | 0.07                 | PL  | T   | ...   | 2FGL J0540.4–5415    | ... | fsrq  | PKS 0539–543             |
| J0540.8+3503c | 85.215 | 35.064  | 174.254 | 2.359   | 0.569      | 0.095      | –63    | 4.5      | 0.7      | 0.1             | 10.1     | 2.2             | 2.52          | 0.12                 | PL  | ... | 5,6   | ...                  | ... | ...   | ...                      |
| J0541.1+3553  | 85.277 | 35.897  | 173.572 | 2.842   | 0.136      | 0.096      | –56    | 10.9     | 2.1      | 0.2             | 18.3     | 2.3             | 2.40          | ...                  | LP  | ... | 1     | 2FGL J0540.3+3549c   | ... | ...   | ...                      |
|               |        |         |         |         |            |            |        |          |          |                 |          |                 |               |                      |     |     |       | 1FGL J0541.1+3542c   |     |       |                          |
| J0542.2–8737  | 85.560 | –87.618 | 300.361 | –27.813 | 0.078      | 0.061      | –78    | 6.4      | 0.4      | 0.1             | 4.6      | 0.9             | 2.04          | 0.14                 | PL  | ... | 9     | ...                  | ... | bcu   | SUMSS<br>J054923–874001  |
| J0542.5–0907c | 85.638 | –9.121  | 213.406 | –19.418 | 0.195      | 0.156      | 50     | 7.4      | 0.9      | 0.2             | 13.6     | 1.8             | 2.57          | 0.09                 | PL  | ... | 1,4,6 | ...                  | ... | bcu   | PMN J0542–0913           |
| J0543.9–5531  | 85.978 | –55.532 | 263.511 | –31.480 | 0.024      | 0.022      | 31     | 25.3     | 1.6      | 0.1             | 20.4     | 1.8             | 1.77          | 0.05                 | PL  | ... | ...   | 1FHL J0543.9–5532    | ... | bll   | 1RXS<br>J054357.3–553206 |
|               |        |         |         |         |            |            |        |          |          |                 |          |                 |               |                      |     |     |       | 2FGL J0543.9–5532    |     |       |                          |
|               |        |         |         |         |            |            |        |          |          |                 |          |                 |               |                      |     |     |       | 1FGL J0543.8–5531    |     |       |                          |

Table 1—Continued

| Name 3FGL     | R.A.   | Decl.   | $l$     | $b$     | $\theta_1$ | $\theta_2$ | $\phi$ | $\sigma$ | $F_{35}$ | $\Delta F_{35}$ | $S_{25}$ | $\Delta S_{25}$ | $\Gamma_{25}$ | $\Delta \Gamma_{25}$ | Mod | Var | Flags | $\gamma$ -ray Assoc.                                        | TeV | Class | ID or Assoc.            |
|---------------|--------|---------|---------|---------|------------|------------|--------|----------|----------|-----------------|----------|-----------------|---------------|----------------------|-----|-----|-------|-------------------------------------------------------------|-----|-------|-------------------------|
| J0544.7+2239  | 86.176 | 22.657  | 185.256 | -3.447  | 0.154      | 0.119      | 17     | 4.2      | 0.6      | 0.1             | 9.1      | 2.3             | 2.50          | 0.18                 | PL  | ... | 4     | ...                                                         | ... | ...   | ...                     |
| J0545.6+6019  | 86.415 | 60.322  | 152.496 | 15.749  | 0.054      | 0.045      | 56     | 15.4     | 1.3      | 0.1             | 7.9      | 1.0             | 2.01          | ...                  | LP  | ... | ...   | 2FGL J0545.6+6018<br>1FGL J0545.6+6022                      | ... | ...   | ...                     |
| J0546.4+0031c | 86.625 | 0.527   | 204.889 | -14.158 | 0.392      | 0.338      | -73    | 5.0      | 0.6      | 0.1             | 9.3      | 1.7             | 2.57          | 0.12                 | PL  | ... | 6     | 2FGL J0547.1+0020c<br>1FGL J0547.0+0020c                    | ... | ...   | ...                     |
| J0550.3-4521  | 87.587 | -45.351 | 251.920 | -29.284 | 0.300      | 0.221      | 71     | 4.7      | 0.3      | 0.1             | 4.7      | 1.0             | 2.66          | 0.17                 | PL  | ... | ...   | ...                                                         | ... | ...   | ...                     |
| J0550.6-3217  | 87.662 | -32.285 | 237.578 | -26.154 | 0.050      | 0.047      | -1     | 7.2      | 0.3      | 0.1             | 4.0      | 1.0             | 1.61          | 0.16                 | PL  | ... | ...   | 1FHL J0550.6-3215                                           | P   | bll   | PKS 0548-322            |
| J0553.5-2036  | 88.382 | -20.601 | 225.764 | -21.635 | 0.084      | 0.074      | 62     | 9.6      | 0.7      | 0.1             | 7.3      | 1.1             | 1.99          | 0.09                 | PL  | ... | ...   | ...                                                         | ... | bcu   | NVSS<br>J055333-203417  |
| J0554.1+3104  | 88.530 | 31.069  | 179.114 | 2.674   | 0.054      | 0.049      | -10    | 18.6     | 2.8      | 0.2             | 17.3     | 1.4             | 2.24          | ...                  | EC  | ... | ...   | 2FGL J0553.9+3104<br>1FGL J0553.9+3105                      | ... | PSR   | LAT PSR J0554+3107      |
| J0556.0-4353  | 89.011 | -43.888 | 250.504 | -28.010 | 0.098      | 0.081      | 69     | 7.6      | 0.5      | 0.1             | 5.3      | 0.9             | 2.20          | 0.12                 | PL  | ... | ...   | 2FGL J0555.9-4348                                           | ... | bll   | SUMSS<br>J055618-435146 |
| J0556.2+3933  | 89.058 | 39.550  | 171.947 | 7.275   | 0.235      | 0.192      | -73    | 8.0      | 0.3      | 0.1             | 11.6     | 1.3             | 3.09          | 0.13                 | PL  | ... | 3     | ...                                                         | ... | ...   | ...                     |
| J0557.7-0720  | 89.450 | -7.340  | 213.456 | -15.246 | 0.072      | 0.057      | -23    | 4.7      | 0.4      | 0.1             | 4.3      | 1.2             | 2.15          | 0.18                 | PL  | ... | ...   | ...                                                         | ... | ...   | ...                     |
| J0558.1-3838  | 89.539 | -38.645 | 244.869 | -26.417 | 0.050      | 0.042      | -36    | 11.7     | 0.7      | 0.1             | 7.7      | 1.0             | 1.96          | 0.10                 | PL  | ... | ...   | 2FGL J0558.2-3837<br>1FGL J0557.6-3831                      | ... | bll   | EXO 0556-3838<br>5      |
| J0558.6-7459  | 89.669 | -74.996 | 286.092 | -29.539 | 0.057      | 0.050      | 79     | 9.7      | 0.6      | 0.1             | 6.9      | 1.0             | 2.05          | 0.10                 | PL  | ... | ...   | 2FGL J0558.7-7501<br>1FGL J0559.2-7500                      | ... | bll   | PKS 0600-749            |
| J0559.8+3042  | 89.962 | 30.715  | 180.035 | 3.562   | 0.052      | 0.043      | -68    | 5.9      | 0.3      | 0.1             | 4.7      | 1.2             | 1.71          | 0.17                 | PL  | ... | ...   | ...                                                         | ... | ...   | ...                     |
| J0600.4-1934  | 90.118 | -19.573 | 225.412 | -19.737 | 0.208      | 0.192      | -71    | 6.2      | 0.4      | 0.1             | 5.7      | 1.0             | 2.56          | 0.13                 | PL  | ... | 9     | 2FGL J0600.8-1949                                           | ... | ...   | ...                     |
| J0600.9-3943  | 90.239 | -39.717 | 246.179 | -26.164 | 0.194      | 0.152      | -25    | 4.9      | 0.3      | 0.1             | 6.6      | 1.2             | 2.81          | 0.13                 | PL  | ... | ...   | ...                                                         | ... | fsrq  | PKS 0558-396            |
| J0601.0+3837  | 90.267 | 38.625  | 173.223 | 7.646   | 0.056      | 0.051      | -86    | 7.2      | 0.5      | 0.1             | 5.6      | 1.2             | 1.89          | 0.15                 | PL  | ... | ...   | 1FHL J0601.0+3838<br>2FGL J0600.9+3839<br>1FGL J0600.9+3838 | ... | bll   | B2 0557+38              |
| J0601.2-7036  | 90.313 | -70.609 | 281.042 | -29.624 | 0.031      | 0.028      | -39    | 39.6     | 3.0      | 0.2             | 30.9     | 1.3             | 2.32          | ...                  | LP  | T   | ...   | 1FHL J0601.1-7037<br>2FGL J0601.1-7037<br>1FGL J0600.7-7037 | ... | fsrq  | PKS 0601-70             |
| J0601.5+2309  | 90.384 | 23.158  | 186.792 | 0.147   | 0.233      | 0.139      | 7      | 4.8      | 0.7      | 0.2             | 10.2     | 2.0             | 2.48          | 0.12                 | PL  | ... | 9     | ...                                                         | ... | ...   | ...                     |
| J0602.2+5314  | 90.562 | 53.235  | 160.109 | 14.586  | 0.054      | 0.052      | 31     | 8.8      | 0.5      | 0.1             | 6.1      | 1.0             | 2.03          | 0.13                 | PL  | ... | ...   | 2FGL J0602.3+5315                                           | ... | bcu   | GB6 J0601+5315          |
| J0602.8-4016  | 90.715 | -40.272 | 246.879 | -25.952 | 0.041      | 0.036      | 62     | 15.3     | 1.1      | 0.1             | 12.1     | 1.3             | 1.92          | 0.08                 | PL  | ... | ...   | 1FHL J0602.4-4013<br>2FGL J0602.7-4011<br>1FGL J0603.0-4012 | ... | bcu   | SUMSS<br>J060251-401845 |
| J0603.3+2042  | 90.840 | 20.716  | 189.124 | -0.690  | 0.069      | 0.058      | -68    | 4.4      | 0.2      | 0.2             | 3.5      | 1.7             | 1.50          | 0.50                 | PL  | ... | ...   | ...                                                         | ... | ...   | ...                     |
| J0603.8+2155  | 90.963 | 21.927  | 188.126 | 0.005   | 0.065      | 0.052      | -17    | 6.9      | 0.8      | 0.2             | 9.4      | 1.9             | 2.10          | 0.14                 | PL  | T   | ...   | ...                                                         | ... | bcu   | 4C +22.12               |
| J0604.1-4817  | 91.031 | -48.292 | 255.695 | -27.503 | 0.046      | 0.040      | -79    | 7.9      | 0.2      | 0.1             | 3.8      | 1.0             | 1.44          | 0.17                 | PL  | ... | ...   | 1FHL J0604.2-4817<br>2FGL J0604.2-4817                      | ... | bll   | 1ES 0602-482            |



Table 1—Continued

| Name 3FGL     | R.A.   | Decl.   | $l$     | $b$     | $\theta_1$ | $\theta_2$ | $\phi$ | $\sigma$ | $F_{35}$ | $\Delta F_{35}$ | $S_{25}$ | $\Delta S_{25}$ | $\Gamma_{25}$ | $\Delta \Gamma_{25}$ | Mod | Var | Flags | $\gamma$ -ray Assoc.                                        | TeV | Class | ID or Assoc.             |
|---------------|--------|---------|---------|---------|------------|------------|--------|----------|----------|-----------------|----------|-----------------|---------------|----------------------|-----|-----|-------|-------------------------------------------------------------|-----|-------|--------------------------|
| J0604.7–4849  | 91.184 | –48.824 | 256.306 | –27.503 | 0.112      | 0.090      | 80     | 5.1      | 0.3      | 0.1             | 3.7      | 0.9             | 2.40          | 0.19                 | PL  | ... | 1,5   | 1FGL J0604.2–4817<br>...                                    | ... | bcu   | 1RXS<br>J060432.7–485007 |
| J0605.0+3756  | 91.253 | 37.935  | 174.208 | 7.996   | 0.069      | 0.062      | –18    | 11.4     | 1.4      | 0.2             | 6.9      | 1.0             | 2.16          | ...                  | EC  | ... | ...   | 2FGL J0605.3+3758<br>1FGL J0605.3+3800                      | ... | PSR   | PSR J0605+3757           |
| J0605.0–0000  | 91.271 | –0.009  | 207.599 | –10.302 | 0.054      | 0.048      | 38     | 8.1      | 0.7      | 0.1             | 7.8      | 1.3             | 2.01          | 0.12                 | PL  | ... | ...   | 1FHL J0605.0+0001<br>2FGL J0605.0+0001<br>1FGL J0605.1+0005 | ... | ...   | ...                      |
| J0605.9+2039c | 91.477 | 20.653  | 189.472 | –0.202  | 0.106      | 0.085      | 36     | 6.9      | 1.4      | 0.2             | 17.8     | 2.7             | 2.36          | 0.08                 | PL  | ... | 6,9   | ...                                                         | ... | ...   | ...                      |
| J0606.4–4729  | 91.605 | –47.492 | 254.897 | –26.969 | 0.080      | 0.075      | 53     | 6.4      | 0.4      | 0.1             | 4.5      | 0.9             | 2.33          | 0.17                 | PL  | ... | ...   | ...                                                         | ... | bcu   | ESO 254– G 017           |
| J0607.4+4739  | 91.860 | 47.654  | 165.640 | 12.863  | 0.029      | 0.028      | 28     | 30.6     | 2.6      | 0.1             | 28.8     | 1.5             | 2.15          | 0.04                 | PL  | ... | ...   | 2FGL J0607.4+4739<br>1FGL J0607.2+4739                      | ... | bll   | TXS 0603+476             |
| J0608.0–0835  | 92.011 | –8.589  | 215.766 | –13.516 | 0.047      | 0.042      | 7      | 19.7     | 2.1      | 0.2             | 26.9     | 1.7             | 2.37          | 0.05                 | PL  | T   | ...   | 2FGL J0608.0–0836<br>1FGL J0608.2–0837                      | ... | fsrq  | PKS 0605–08              |
| J0608.1–1522  | 92.031 | –15.380 | 222.135 | –16.388 | 0.066      | 0.062      | –74    | 22.3     | 1.6      | 0.1             | 22.7     | 1.3             | 2.55          | ...                  | LP  | T   | 7     | 2FGL J0608.0–1521<br>1FGL J0608.0–1521                      | ... | fsrq  | PMN J0608–1520<br>33     |
| J0608.2–2306  | 92.064 | –23.110 | 229.615 | –19.407 | 0.161      | 0.153      | 62     | 4.5      | 0.3      | 0.1             | 3.3      | 0.8             | 2.20          | 0.16                 | PL  | ... | ...   | ...                                                         | ... | ...   | ...                      |
| J0608.6+5328  | 92.160 | 53.483  | 160.301 | 15.554  | 0.175      | 0.153      | –34    | 4.2      | 0.3      | 0.1             | 4.6      | 1.0             | 2.49          | 0.16                 | PL  | ... | ...   | ...                                                         | ... | ...   | ...                      |
| J0609.2+2051c | 92.319 | 20.863  | 189.671 | 0.588   | 0.067      | 0.064      | –33    | 5.0      | 1.0      | 0.2             | 11.6     | 2.8             | 2.27          | 0.11                 | PL  | ... | 5,6   | ...                                                         | ... | ...   | ...                      |
| J0609.3+2131  | 92.341 | 21.531  | 189.097 | 0.930   | 0.146      | 0.128      | 51     | 9.8      | 2.1      | 0.3             | 16.5     | 2.2             | 2.38          | ...                  | LP  | ... | ...   | ...                                                         | ... | psr   | PSR J0609+2130           |
| J0609.4–0248  | 92.352 | –2.806  | 210.630 | –10.628 | 0.040      | 0.038      | –82    | 12.3     | 1.0      | 0.1             | 11.2     | 1.5             | 1.90          | 0.10                 | PL  | ... | ...   | 1FHL J0609.4–0248<br>2FGL J0609.4–0248<br>1FGL J0609.3–0244 | ... | bll   | NVSS<br>J060915–024754   |
| J0609.6–2851  | 92.418 | –28.863 | 235.460 | –21.184 | 0.243      | 0.187      | –46    | 4.8      | 0.2      | 0.1             | 3.8      | 0.8             | 2.64          | 0.18                 | PL  | ... | ...   | ...                                                         | ... | ...   | ...                      |
| J0609.7–1841  | 92.426 | –18.693 | 225.461 | –17.386 | 0.104      | 0.091      | –48    | 8.6      | 0.6      | 0.1             | 7.4      | 1.0             | 2.30          | 0.10                 | PL  | ... | ...   | 2FGL J0609.6–1847                                           | ... | ...   | ...                      |
| J0610.2–2059  | 92.554 | –20.991 | 227.730 | –18.179 | 0.078      | 0.065      | 5      | 13.4     | 0.9      | 0.1             | 11.5     | 1.1             | 2.34          | 0.07                 | PL  | ... | ...   | 2FGL J0610.3–2059<br>1FGL J0610.7–2059                      | ... | PSR   | PSR J0610–2100           |
| J0610.6+1728  | 92.668 | 17.472  | 192.799 | –0.762  | 0.163      | 0.114      | –30    | 10.0     | 1.5      | 0.3             | 16.5     | 2.0             | 2.46          | ...                  | LP  | ... | ...   | ...                                                         | ... | spp   | ...                      |
| J0611.1–6100  | 92.795 | –61.006 | 270.107 | –28.309 | 0.133      | 0.105      | 0      | 10.5     | 0.4      | 0.1             | 8.1      | 0.8             | 2.70          | 0.10                 | PL  | T   | ...   | 2FGL J0611.8–6059                                           | ... | fsrq  | PKS 0609–609             |
| J0611.2+4323  | 92.816 | 43.387  | 169.854 | 11.563  | 0.062      | 0.057      | –34    | 8.1      | 0.5      | 0.1             | 5.8      | 1.0             | 2.17          | 0.14                 | PL  | ... | ...   | 2FGL J0611.0+4321                                           | ... | bcu   | NVSS<br>J061107+432404   |
| J0611.5+1957  | 92.899 | 19.960  | 190.724 | 0.629   | 0.100      | 0.084      | 13     | 6.9      | 1.2      | 0.2             | 15.9     | 2.4             | 2.38          | 0.08                 | PL  | ... | 1     | ...                                                         | ... | ...   | ...                      |
| J0611.7+2759  | 92.932 | 27.998  | 183.676 | 4.507   | 0.119      | 0.096      | –5     | 5.3      | 0.6      | 0.1             | 7.1      | 1.4             | 2.28          | 0.13                 | PL  | ... | 1     | ...                                                         | ... | bcu   | GB6 J0611+2803           |
| J0612.8+4122  | 93.208 | 41.371  | 171.823 | 10.918  | 0.019      | 0.019      | –40    | 45.8     | 4.6      | 0.2             | 51.2     | 2.1             | 2.03          | 0.03                 | PL  | T   | ...   | 1FHL J0612.8+4121<br>2FGL J0612.8+4122<br>1FGL J0612.7+4120 | ... | bll   | B3 0609+413              |
| J0613.8–0201  | 93.451 | –2.030  | 210.436 | –9.297  | 0.030      | 0.029      | 85     | 35.0     | 5.3      | 0.2             | 33.6     | 1.6             | 2.11          | ...                  | EC  | ... | ...   | 2FGL J0613.8–0200                                           | ... | PSR   | PSR J0613–0200           |

Table 1—Continued

| Name 3FGL     | R.A.   | Decl.   | $l$     | $b$     | $\theta_1$ | $\theta_2$ | $\phi$ | $\sigma$ | $F_{35}$ | $\Delta F_{35}$ | $S_{25}$ | $\Delta S_{25}$ | $\Gamma_{25}$ | $\Delta \Gamma_{25}$ | Mod | Var | Flags | $\gamma$ -ray Assoc. | TeV | Class | ID or Assoc.                  |
|---------------|--------|---------|---------|---------|------------|------------|--------|----------|----------|-----------------|----------|-----------------|---------------|----------------------|-----|-----|-------|----------------------|-----|-------|-------------------------------|
| J0614.1–3329  | 93.537 | –33.495 | 240.496 | –21.831 | 0.013      | 0.013      | 36     | 118.0    | 17.4     | 0.4             | 110.8    | 2.4             | 1.87          | ...                  | EC  | ... | ...   | 1FGL J0613.7–0200    | ... | PSR   | PSR J0614–3329                |
|               |        |         |         |         |            |            |        |          |          |                 |          |                 |               |                      |     |     |       | 0FGL J0613.9–0202    |     |       |                               |
|               |        |         |         |         |            |            |        |          |          |                 |          |                 |               |                      |     |     |       | 1FHL J0614.0–3325    |     |       |                               |
|               |        |         |         |         |            |            |        |          |          |                 |          |                 |               |                      |     |     |       | 2FGL J0614.1–3329    |     |       |                               |
|               |        |         |         |         |            |            |        |          |          |                 |          |                 |               |                      |     |     |       | 1FGL J0614.1–3328    |     |       |                               |
|               |        |         |         |         |            |            |        |          |          |                 |          |                 |               |                      |     |     |       | 0FGL J0614.3–3330    |     |       |                               |
| J0615.4–3116  | 93.861 | –31.271 | 238.342 | –20.834 | 0.078      | 0.063      | –79    | 8.6      | 0.5      | 0.1             | 6.1      | 0.9             | 2.33          | 0.11                 | PL  | ... | ...   | 3EG J0616–3310       | ... | bll   | PKS 0613–312                  |
| J0617.2+5701  | 94.300 | 57.025  | 157.417 | 18.086  | 0.033      | 0.030      | 31     | 19.4     | 1.2      | 0.1             | 13.6     | 1.1             | 2.04          | 0.06                 | PL  | ... | ...   | EGR J0615–3308       | ... | bll   | 87GB                          |
| J0617.2+2234e | 94.310 | 22.580  | 189.048 | 3.034   | ...        | ...        | ...    | 133.3    | 63.3     | 0.7             | 502.1    | 7.0             | 1.98          | ...                  | LP  | ... | ...   | 2FGL J0616.9+5701    | E   | SNR   | IC 443                        |
|               |        |         |         |         |            |            |        |          |          |                 |          |                 |               |                      |     |     |       | 1FGL J0616.9+5701    |     |       |                               |
|               |        |         |         |         |            |            |        |          |          |                 |          |                 |               |                      |     |     |       | 1FHL J0617.2+2234e   |     |       |                               |
|               |        |         |         |         |            |            |        |          |          |                 |          |                 |               |                      |     |     |       | 2FGL J0617.2+2234e   |     |       |                               |
|               |        |         |         |         |            |            |        |          |          |                 |          |                 |               |                      |     |     |       | 1FGL J0617.2+2233    |     |       |                               |
|               |        |         |         |         |            |            |        |          |          |                 |          |                 |               |                      |     |     |       | 0FGL J0617.4+2234    |     |       |                               |
| J0617.6–1717  | 94.408 | –17.298 | 224.927 | –15.097 | 0.041      | 0.038      | 81     | 13.4     | 1.0      | 0.1             | 11.4     | 1.4             | 1.94          | 0.08                 | PL  | ... | ...   | 3EG J0617+2238       | ... | bll   | CRATES<br>J061733.67–171522.8 |
|               |        |         |         |         |            |            |        |          |          |                 |          |                 |               |                      |     |     |       | EGR J0617+2238       |     |       |                               |
|               |        |         |         |         |            |            |        |          |          |                 |          |                 |               |                      |     |     |       | 1AGL J0617+2236      |     |       |                               |
|               |        |         |         |         |            |            |        |          |          |                 |          |                 |               |                      |     |     |       | 1FHL J0617.6–1716    |     |       |                               |
|               |        |         |         |         |            |            |        |          |          |                 |          |                 |               |                      |     |     |       | 2FGL J0617.6–1716    |     |       |                               |
|               |        |         |         |         |            |            |        |          |          |                 |          |                 |               |                      |     |     |       | 1FGL J0617.7–1718    |     |       |                               |
| J0618.0+7819  | 94.519 | 78.323  | 135.682 | 24.861  | 0.073      | 0.071      | –70    | 6.1      | 0.3      | 0.1             | 3.6      | 0.7             | 2.37          | 0.15                 | PL  | ... | 4     | ...                  | ... | fsrq  | 1REX J061757+7816.1           |
| J0618.2–2429  | 94.566 | –24.495 | 231.881 | –17.811 | 0.139      | 0.111      | –50    | 5.8      | 0.4      | 0.1             | 4.8      | 0.9             | 2.42          | 0.12                 | PL  | ... | 1     | ...                  | ... | bcu   | PMN J0618–2426                |
| J0618.9–1138  | 94.739 | –11.642 | 219.784 | –12.423 | 0.168      | 0.104      | 37     | 5.6      | 0.5      | 0.1             | 7.7      | 1.4             | 2.47          | 0.13                 | PL  | ... | 4     | 3EG J0622–1139       | ... | bcu   | TXS 0616–116                  |
| J0619.4+2242  | 94.874 | 22.706  | 189.182 | 3.553   | 0.106      | 0.070      | 89     | 5.5      | 1.4      | 0.3             | 15.4     | 3.5             | 2.01          | 0.13                 | PL  | ... | 5     | ...                  | ... | ...   | ...                           |
| J0620.4+2644  | 95.121 | 26.740  | 185.708 | 5.632   | 0.067      | 0.060      | –83    | 5.0      | 0.3      | 0.1             | 3.9      | 1.1             | 1.65          | 0.19                 | PL  | ... | ...   | ...                  | ... | bcu   | RX J0620.6+2644               |
| J0621.0+2514  | 95.273 | 25.242  | 187.104 | 5.059   | 0.073      | 0.069      | 29     | 8.6      | 1.0      | 0.1             | 11.0     | 1.5             | 2.17          | 0.09                 | PL  | ... | ...   | 2FGL J0621.2+2508    | ... | PSR   | PSR J0621+2514                |
| J0622.2+3747  | 95.555 | 37.797  | 175.903 | 10.956  | 0.058      | 0.053      | 67     | 25.6     | 2.2      | 0.2             | 19.7     | 1.1             | 2.40          | ...                  | EC  | ... | ...   | 1FGL J0621.5+2508    | ... | PSR   | LAT PSR J0622+3749            |
|               |        |         |         |         |            |            |        |          |          |                 |          |                 |               |                      |     |     |       | 2FGL J0621.9+3750    |     |       |                               |
| J0622.4–2606  | 95.609 | –26.115 | 233.829 | –17.552 | 0.040      | 0.034      | –41    | 16.3     | 1.1      | 0.1             | 13.0     | 1.4             | 1.94          | 0.07                 | PL  | T   | ...   | 1FGL J0622.2+3751    | ... | bll   | PMN J0622–2605                |
|               |        |         |         |         |            |            |        |          |          |                 |          |                 |               |                      |     |     |       | 1FHL J0622.4–2604    |     |       |                               |
| J0622.9+3326  | 95.735 | 33.436  | 179.941 | 9.157   | 0.019      | 0.017      | –70    | 56.1     | 7.0      | 0.2             | 70.5     | 2.4             | 2.18          | ...                  | LP  | T   | ...   | 1FGL J0622.3–2604    | ... | BCU   | B2 0619+33                    |
|               |        |         |         |         |            |            |        |          |          |                 |          |                 |               |                      |     |     |       | 1FHL J0622.9+3328    |     |       |                               |
|               |        |         |         |         |            |            |        |          |          |                 |          |                 |               |                      |     |     |       | 2FGL J0622.9+3326    |     |       |                               |

Table 1—Continued

| Name 3FGL     | R.A.   | Decl.   | $l$     | $b$     | $\theta_1$ | $\theta_2$ | $\phi$ | $\sigma$ | $F_{35}$ | $\Delta F_{35}$ | $S_{25}$ | $\Delta S_{25}$ | $\Gamma_{25}$ | $\Delta \Gamma_{25}$ | Mod | Var | Flags | $\gamma$ -ray Assoc.                                                          | TeV | Class | ID or Assoc.             |
|---------------|--------|---------|---------|---------|------------|------------|--------|----------|----------|-----------------|----------|-----------------|---------------|----------------------|-----|-----|-------|-------------------------------------------------------------------------------|-----|-------|--------------------------|
| J0623.1–4143  | 95.780 | –41.726 | 249.549 | –22.666 | 0.118      | 0.111      | 74     | 4.1      | 0.3      | 0.1             | 3.0      | 0.8             | 2.29          | 0.19                 | PL  | ... | ...   | ...                                                                           | ... | ...   | ...                      |
| J0623.3+3043  | 95.827 | 30.725  | 182.425 | 8.008   | 0.072      | 0.058      | –28    | 5.2      | 0.4      | 0.1             | 4.3      | 1.1             | 1.89          | 0.17                 | PL  | ... | ...   | ...                                                                           | ... | bcu   | GB6 J0623+3045           |
| J0625.2+4440  | 96.318 | 44.680  | 169.760 | 14.391  | 0.044      | 0.037      | 52     | 13.2     | 0.9      | 0.1             | 9.5      | 1.1             | 2.05          | 0.09                 | PL  | ... | ...   | 1FHL J0625.3+4440<br>2FGL J0625.2+4441<br>1FGL J0625.4+4440                   | ... | bll   | GB6 J0625+4440           |
| J0626.0–5436  | 96.521 | –54.607 | 263.354 | –25.380 | 0.170      | 0.147      | –28    | 8.4      | 0.3      | 0.1             | 7.2      | 0.9             | 2.92          | 0.15                 | PL  | ... | ...   | 1FGL J0625.9–5430                                                             | ... | fsrq  | PMN J0625–5438           |
| J0626.6–4259  | 96.667 | –42.998 | 251.073 | –22.407 | 0.076      | 0.056      | –42    | 7.4      | 0.3      | 0.1             | 4.5      | 1.0             | 1.74          | 0.15                 | PL  | ... | ...   | 2FGL J0626.8–4258                                                             | ... | bcu   | 1RXS<br>J062635.9–425810 |
| J0626.8+1743  | 96.712 | 17.732  | 194.394 | 2.757   | 0.207      | 0.145      | 27     | 4.4      | 0.7      | 0.2             | 13.7     | 3.1             | 2.70          | 0.13                 | PL  | ... | ...   | 1FGL J0626.6–4254                                                             | ... | ...   | ...                      |
| J0627.0–3529  | 96.773 | –35.489 | 243.454 | –19.972 | 0.035      | 0.031      | 61     | 20.1     | 1.4      | 0.1             | 16.9     | 1.6             | 1.87          | 0.06                 | PL  | ... | ...   | 1FHL J0626.8–3528<br>2FGL J0627.1–3528<br>1FGL J0627.3–3530                   | ... | rdg   | PKS 0625–35              |
| J0627.9–1517  | 96.985 | –15.298 | 224.121 | –12.014 | 0.106      | 0.092      | –17    | 4.5      | 0.3      | 0.1             | 5.4      | 1.2             | 2.72          | 0.18                 | PL  | ... | ...   | ...                                                                           | ... | bcu   | NVSS<br>J062753–152003   |
| J0628.4+2429  | 97.123 | 24.498  | 188.543 | 6.208   | 0.110      | 0.093      | 25     | 4.3      | 0.4      | 0.1             | 5.0      | 1.3             | 2.21          | 0.16                 | PL  | ... | ...   | ...                                                                           | ... | ...   | ...                      |
| J0629.0–6248  | 97.272 | –62.806 | 272.405 | –26.435 | 0.088      | 0.075      | –29    | 9.2      | 0.5      | 0.1             | 6.3      | 0.8             | 2.23          | 0.11                 | PL  | ... | ...   | 2FGL J0628.9–6246                                                             | ... | bll   | PKS 0628–627             |
| J0629.4–1959  | 97.358 | –19.986 | 228.641 | –13.652 | 0.029      | 0.027      | –69    | 33.6     | 3.4      | 0.2             | 38.2     | 1.8             | 2.18          | 0.03                 | PL  | T   | ...   | 2FGL J0629.3–2001<br>1FGL J0629.6–2000                                        | ... | bll   | PKS 0627–199             |
| J0630.2–0929c | 97.571 | –9.496  | 219.057 | –8.982  | 0.377      | 0.235      | 28     | 4.2      | 0.5      | 0.1             | 7.3      | 1.5             | 2.51          | 0.13                 | PL  | ... | 6     | ...                                                                           | ... | ...   | ...                      |
| J0630.3+6906  | 97.589 | 69.112  | 145.688 | 23.383  | 0.226      | 0.167      | –78    | 4.2      | 0.2      | 0.1             | 2.9      | 0.7             | 2.39          | 0.19                 | PL  | ... | ...   | ...                                                                           | ... | bcu   | GB6 J0629+6900           |
| J0630.9–2406  | 97.747 | –24.110 | 232.685 | –14.990 | 0.019      | 0.019      | –56    | 38.4     | 3.5      | 0.2             | 42.9     | 2.6             | 1.81          | 0.04                 | PL  | ... | ...   | 1FHL J0630.9–2406<br>2FGL J0630.9–2406<br>1FGL J0630.9–2406                   | ... | bll   | TXS 0628–240             |
| J0631.2+2019  | 97.803 | 20.328  | 192.560 | 4.868   | 0.123      | 0.091      | 86     | 5.9      | 0.7      | 0.1             | 9.3      | 1.8             | 2.46          | 0.13                 | PL  | ... | ...   | ...                                                                           | ... | bcu   | TXS 0628+203             |
| J0631.5+1036  | 97.886 | 10.613  | 201.233 | 0.467   | 0.031      | 0.029      | 73     | 28.5     | 5.7      | 0.3             | 39.2     | 2.2             | 2.12          | ...                  | EC  | ... | 3     | 2FGL J0631.5+1035<br>1FGL J0631.4+1037<br>0FGL J0631.8+1034                   | ... | PSR   | PSR J0631+1036           |
| J0631.6+0644  | 97.907 | 6.741   | 204.676 | –1.305  | 0.047      | 0.046      | –61    | 14.0     | 3.2      | 0.3             | 21.2     | 2.8             | 2.19          | ...                  | LP  | ... | ...   | 2FGL J0631.6+0640<br>3EG J0631+0642                                           | ... | spp   | ...                      |
| J0633.7+0632  | 98.438 | 6.541   | 205.097 | –0.929  | 0.018      | 0.018      | 71     | 57.9     | 17.1     | 0.5             | 124.4    | 3.6             | 2.16          | ...                  | EC  | ... | ...   | 2FGL J0633.7+0633<br>1FGL J0633.7+0632<br>0FGL J0633.5+0634<br>EGR J0633+0646 | ... | PSR   | LAT PSR J0633+0632       |
| J0633.9+1746  | 98.479 | 17.773  | 195.133 | 4.270   | 0.005      | 0.005      | 78     | 1012.1   | 692.2    | 2.1             | 4153.1   | 10.9            | 1.87          | ...                  | EC  | ... | ...   | 1FHL J0633.9+1746                                                             | E   | PSR   | PSR J0633+1746           |
| J0634.1+0424  | 98.528 | 4.406   | 207.034 | –1.833  | 0.109      | 0.089      | 20     | 21.1     | 4.3      | 0.3             | 46.9     | 2.9             | 2.39          | ...                  | LP  | ... | 3     | ...                                                                           | ... | ...   | ...                      |
| J0634.7–2334  | 98.677 | –23.575 | 232.531 | –13.996 | 0.182      | 0.132      | 87     | 6.6      | 0.5      | 0.1             | 7.3      | 1.1             | 2.54          | 0.11                 | PL  | ... | 1     | 2FGL J0635.0–2334                                                             | ... | fsrq  | PMN J0634–2335           |

Table 1—Continued

| Name 3FGL    | R.A.    | Decl.   | $l$     | $b$     | $\theta_1$ | $\theta_2$ | $\phi$ | $\sigma$ | $F_{35}$ | $\Delta F_{35}$ | $S_{25}$ | $\Delta S_{25}$ | $\Gamma_{25}$ | $\Delta \Gamma_{25}$ | Mod | Var | Flags | $\gamma$ -ray Assoc.                                        | TeV | Class | ID or Assoc.             |
|--------------|---------|---------|---------|---------|------------|------------|--------|----------|----------|-----------------|----------|-----------------|---------------|----------------------|-----|-----|-------|-------------------------------------------------------------|-----|-------|--------------------------|
| J0635.7–7517 | 98.942  | –75.293 | 286.392 | –27.160 | 0.064      | 0.058      | 48     | 22.8     | 1.0      | 0.1             | 20.4     | 1.0             | 2.71          | 0.05                 | PL  | T   | ...   | 2FGL J0635.5–7516<br>1FGL J0636.1–7521                      | ... | fsrq  | PKS 0637–75              |
| J0636.7+7115 | 99.191  | 71.263  | 143.547 | 24.427  | 0.169      | 0.139      | 76     | 6.5      | 0.3      | 0.1             | 4.9      | 0.8             | 2.61          | 0.14                 | PL  | ... | ...   | ...                                                         | ... | ...   | ...                      |
| J0637.5+0418 | 99.383  | 4.315   | 207.507 | –1.117  | 0.089      | 0.078      | 59     | 8.8      | 1.3      | 0.4             | 17.4     | 2.4             | 2.45          | ...                  | LP  | ... | 5     | 2FGL J0637.0+0416c                                          | ... | ...   | ...                      |
| J0638.4+5704 | 99.605  | 57.074  | 158.421 | 20.811  | 0.156      | 0.137      | –32    | 6.3      | 0.2      | 0.1             | 4.8      | 0.7             | 2.93          | 0.18                 | PL  | ... | 1     | ...                                                         | ... | ...   | ...                      |
| J0638.6+7324 | 99.653  | 73.408  | 141.270 | 25.010  | 0.114      | 0.109      | 51     | 11.0     | 0.4      | 0.1             | 7.7      | 0.8             | 2.64          | 0.09                 | PL  | T   | ...   | 1FGL J0639.9+7325                                           | ... | fsrq  | S5 0633+73               |
| J0639.9+3250 | 99.988  | 32.839  | 182.052 | 12.111  | 0.542      | 0.263      | 4      | 4.4      | 0.3      | 0.1             | 5.0      | 1.0             | 2.65          | 0.17                 | PL  | ... | 9     | ...                                                         | ... | ...   | ...                      |
| J0640.0–1252 | 100.021 | –12.876 | 223.196 | –8.312  | 0.041      | 0.039      | –31    | 8.0      | 0.3      | 0.1             | 5.7      | 1.3             | 1.51          | 0.16                 | PL  | ... | 3     | ...                                                         | ... | bcu   | TXS 0637–128             |
| J0640.9+0752 | 100.247 | 7.882   | 204.730 | 1.281   | 0.288      | 0.164      | –35    | 5.7      | 0.8      | 0.1             | 12.4     | 2.3             | 2.56          | 0.11                 | PL  | ... | 1,5   | ...                                                         | ... | spp   | ...                      |
| J0641.1+1004 | 100.286 | 10.083  | 202.788 | 2.321   | 0.181      | 0.148      | 9      | 10.2     | 1.3      | 0.2             | 18.4     | 2.4             | 2.62          | ...                  | LP  | ... | 1     | 2FGL J0641.1+1006c                                          | ... | ...   | ...                      |
| J0641.8–0319 | 100.471 | –3.319  | 214.802 | –3.636  | 0.163      | 0.124      | –78    | 4.1      | 0.6      | 0.1             | 8.2      | 1.8             | 2.45          | 0.14                 | PL  | T   | 3     | ...                                                         | ... | bcu   | TXS 0639–032             |
| J0643.2+0859 | 100.803 | 8.995   | 203.990 | 2.278   | 0.069      | 0.056      | –30    | 15.4     | 2.5      | 0.2             | 25.5     | 2.8             | 2.48          | ...                  | LP  | T   | 3     | 2FGL J0643.2+0858<br>1FGL J0643.2+0859<br>0FGL J0643.2+0858 | ... | fsrq  | PMN J0643+0857           |
| J0643.4–5358 | 100.851 | –53.972 | 263.325 | –22.775 | 0.091      | 0.086      | 46     | 6.6      | 0.4      | 0.1             | 4.9      | 0.9             | 2.44          | 0.14                 | PL  | ... | ...   | ...                                                         | ... | bcu   | PMN J0643–5358           |
| J0644.3–6713 | 101.088 | –67.223 | 277.537 | –25.536 | 0.020      | 0.020      | –6     | 47.8     | 4.0      | 0.2             | 44.0     | 1.7             | 2.10          | 0.03                 | PL  | T   | ...   | 1FHL J0644.2–6713<br>2FGL J0644.2–6713                      | ... | bcu   | PKS 0644–6713            |
| J0644.6+6035 | 101.152 | 60.591  | 155.048 | 22.594  | 0.067      | 0.056      | 10     | 11.1     | 0.6      | 0.1             | 7.1      | 0.8             | 2.28          | 0.09                 | PL  | ... | ...   | 1FHL J0644.2+6036<br>2FGL J0644.6+6034<br>1FGL J0645.5+6033 | ... | ...   | ...                      |
| J0644.6–2853 | 101.159 | –28.896 | 238.476 | –14.091 | 0.081      | 0.078      | 65     | 4.8      | 0.3      | 0.1             | 3.5      | 0.9             | 2.11          | 0.18                 | PL  | ... | ...   | ...                                                         | ... | bcu   | 1RXS<br>J064444.2–285120 |
| J0645.9–3914 | 101.489 | –39.237 | 248.539 | –17.753 | 0.469      | 0.389      | –50    | 5.1      | 0.2      | 0.1             | 5.0      | 0.9             | 2.89          | 0.19                 | PL  | ... | 1     | ...                                                         | ... | fsrq  | PKS 0644–390             |
| J0646.4–5452 | 101.601 | –54.878 | 264.397 | –22.594 | 0.128      | 0.102      | –34    | 7.1      | 0.6      | 0.1             | 2.6      | 0.4             | 2.29          | ...                  | LP  | ... | 3,12  | ...                                                         | ... | bcu   | PMN J0646–5451           |
| J0647.0–5134 | 101.766 | –51.570 | 260.998 | –21.577 | 0.217      | 0.098      | 46     | 5.5      | 0.3      | 0.1             | 3.9      | 0.8             | 2.19          | 0.18                 | PL  | ... | ...   | 1FHL J0647.1–5131<br>2FGL J0647.7–5132                      | ... | bcu   | 1ES 0646–515             |
| J0647.1–4415 | 101.776 | –44.258 | 253.588 | –19.285 | 0.126      | 0.115      | 14     | 4.2      | 0.2      | 0.1             | 3.1      | 0.8             | 2.34          | 0.23                 | PL  | ... | ...   | ...                                                         | ... | bcu   | SUMSS<br>J064648–441929  |
| J0647.6–6058 | 101.908 | –60.967 | 270.863 | –23.945 | 0.050      | 0.045      | –9     | 13.6     | 0.8      | 0.1             | 10.3     | 1.0             | 2.34          | 0.07                 | PL  | T   | ...   | 2FGL J0647.8–6102<br>1FGL J0648.6–6052                      | ... | bcu   | PMN J0647–6058           |
| J0647.6+0032 | 101.913 | 0.535   | 212.025 | –0.598  | 0.086      | 0.071      | –80    | 11.2     | 1.5      | 0.2             | 20.6     | 2.0             | 2.46          | 0.07                 | PL  | ... | ...   | 2FGL J0647.7+0032<br>1FGL J0647.3+0031                      | ... | ...   | ...                      |
| J0647.8+1751 | 101.962 | 17.851  | 196.560 | 7.269   | 0.271      | 0.158      | –79    | 5.3      | 0.4      | 0.1             | 8.0      | 1.5             | 2.70          | 0.13                 | PL  | ... | 1     | ...                                                         | ... | ...   | ...                      |
| J0648.1+1606 | 102.041 | 16.108  | 198.167 | 6.564   | 0.046      | 0.044      | –76    | 5.3      | 0.2      | 0.1             | 3.0      | 0.9             | 1.77          | 0.28                 | PL  | ... | ...   | ...                                                         | ... | bcu   | 1RXS<br>J064814.1+160708 |
| J0648.1–3045 | 102.044 | –30.762 | 240.556 | –14.129 | 0.083      | 0.072      | 33     | 13.5     | 1.0      | 0.1             | 15.7     | 1.2             | 2.56          | 0.07                 | PL  | T   | ...   | ...                                                         | ... | fsrq  | PKS 0646–306             |
| J0648.8+1516 | 102.205 | 15.276  | 198.988 | 6.335   | 0.030      | 0.028      | –77    | 19.2     | 1.5      | 0.1             | 17.5     | 1.7             | 1.83          | 0.07                 | PL  | ... | ...   | 1FHL J0648.9+1516<br>2FGL J0648.9+1516                      | P   | bl    | RX J0648.7+1516          |

Table 1—Continued

| Name 3FGL     | R.A.    | Decl.   | $l$     | $b$     | $\theta_1$ | $\theta_2$ | $\phi$ | $\sigma$ | $F_{35}$ | $\Delta F_{35}$ | $S_{25}$ | $\Delta S_{25}$ | $\Gamma_{25}$ | $\Delta \Gamma_{25}$ | Mod | Var | Flags | $\gamma$ -ray Assoc.                                                             | TeV | Class | ID or Assoc.             |
|---------------|---------|---------|---------|---------|------------|------------|--------|----------|----------|-----------------|----------|-----------------|---------------|----------------------|-----|-----|-------|----------------------------------------------------------------------------------|-----|-------|--------------------------|
| J0648.8–1740  | 102.209 | –17.668 | 228.486 | –8.512  | 0.192      | 0.126      | 47     | 5.8      | 0.6      | 0.1             | 9.5      | 1.7             | 2.52          | 0.12                 | PL  | T   | ...   | 1FGL J0648.8+1516<br>2FGL J0648.7–1739<br>1FGL J0648.7–1740                      | ... | fsrq  | TXS 0646–176             |
| J0649.6–3138  | 102.400 | –31.635 | 241.507 | –14.196 | 0.038      | 0.036      | 19     | 9.7      | 0.5      | 0.1             | 7.1      | 1.3             | 1.73          | 0.13                 | PL  | ... | ...   | 1FHL J0649.5–3138                                                                | ... | bcu   | 1RXS<br>J064933.8–313914 |
| J0650.4–1636  | 102.606 | –16.608 | 227.691 | –7.707  | 0.096      | 0.092      | 21     | 7.2      | 0.8      | 0.1             | 11.6     | 1.7             | 2.43          | 0.10                 | PL  | ... | ...   | 2FGL J0649.7–3138<br>2FGL J0650.4–1632<br>1FGL J0650.6–1635                      | ... | bcu   | PKS 0648–16              |
| J0650.5+2055  | 102.644 | 20.930  | 194.047 | 9.194   | 0.043      | 0.037      | 78     | 10.0     | 0.4      | 0.1             | 6.8      | 1.4             | 1.56          | 0.14                 | PL  | ... | ...   | 1FHL J0650.4+2056                                                                | ... | bcu   | 1RXS<br>J065033.9+205603 |
| J0650.7+2503  | 102.697 | 25.063  | 190.272 | 11.004  | 0.022      | 0.021      | 17     | 29.5     | 2.2      | 0.1             | 28.7     | 2.3             | 1.72          | 0.05                 | PL  | ... | ...   | 1FHL J0650.8+2504<br>2FGL J0650.7+2505<br>1FGL J0650.7+2503                      | P   | bll   | 1ES 0647+250             |
| J0650.9+6524  | 102.748 | 65.415  | 150.128 | 24.452  | 0.184      | 0.114      | 56     | 6.8      | 0.3      | 0.1             | 4.3      | 0.7             | 2.54          | 0.13                 | PL  | ... | 1     | ...                                                                              | ... | ...   | ...                      |
| J0651.3+4014  | 102.829 | 40.246  | 175.932 | 17.112  | 0.077      | 0.061      | –10    | 6.8      | 0.4      | 0.1             | 4.6      | 0.8             | 2.12          | 0.14                 | PL  | ... | ...   | ...                                                                              | ... | bcu   | RX J0651.0+4013          |
| J0652.0–4808  | 103.015 | –48.134 | 257.770 | –19.753 | 0.067      | 0.061      | –42    | 5.6      | 0.3      | 0.1             | 3.4      | 0.8             | 2.04          | 0.25                 | PL  | ... | ...   | ...                                                                              | ... | bcu   | 1RXS<br>J065201.0–480858 |
| J0653.6+2817  | 103.414 | 28.290  | 187.542 | 12.926  | 0.059      | 0.057      | 6      | 10.3     | 0.6      | 0.1             | 7.3      | 0.9             | 2.25          | 0.10                 | PL  | ... | ...   | 2FGL J0653.7+2818                                                                | ... | bcu   | GB6 J0653+2816           |
| J0654.4+4514  | 103.604 | 45.247  | 171.204 | 19.388  | 0.027      | 0.027      | 11     | 39.4     | 2.9      | 0.1             | 34.6     | 1.3             | 2.29          | 0.03                 | PL  | T   | ...   | 1FHL J0654.2+4514<br>2FGL J0654.2+4514<br>1FGL J0654.3+4514<br>0FGL J0654.3+4513 | ... | FSRQ  | B3 0650+453              |
| J0654.4+5042  | 103.609 | 50.702  | 165.688 | 21.115  | 0.033      | 0.031      | 28     | 26.3     | 2.0      | 0.1             | 15.9     | 1.2             | 2.10          | ...                  | LP  | T   | ...   | 1FHL J0654.5+5042<br>2FGL J0654.5+5043<br>1FGL J0654.4+5042<br>0FGL J0654.3+5042 | ... | fsrq  | GB6 J0654+5042           |
| J0654.5+0926  | 103.638 | 9.447   | 204.856 | 4.978   | 0.291      | 0.184      | 34     | 4.9      | 0.4      | 0.1             | 6.5      | 1.3             | 2.67          | 0.16                 | PL  | ... | ...   | ...                                                                              | ... | bcu   | RX J0654.3+0925          |
| J0656.2–0323  | 104.054 | –3.390  | 216.493 | –0.484  | 0.054      | 0.051      | 62     | 17.4     | 2.9      | 0.2             | 27.8     | 2.2             | 2.40          | ...                  | LP  | T   | ...   | 2FGL J0656.2–0320<br>1FGL J0656.2–0321                                           | ... | fsrq  | TXS 0653–033             |
| J0656.4+4232  | 104.101 | 42.542  | 174.028 | 18.815  | 0.099      | 0.068      | –21    | 9.4      | 0.7      | 0.1             | 7.3      | 1.0             | 2.08          | 0.11                 | PL  | ... | ...   | ...                                                                              | ... | bll   | 4C +42.22                |
| J0657.6–4701  | 104.424 | –47.026 | 257.003 | –18.485 | 0.161      | 0.127      | 73     | 4.3      | 0.3      | 0.1             | 3.5      | 0.9             | 2.01          | 0.19                 | PL  | ... | ...   | ...                                                                              | ... | ...   | ...                      |
| J0658.3–5832  | 104.586 | –58.547 | 268.695 | –22.024 | 0.191      | 0.158      | –7     | 4.1      | 0.3      | 0.1             | 3.5      | 0.8             | 2.40          | 0.17                 | PL  | ... | ...   | ...                                                                              | ... | bcu   | PMN J0658–5840           |
| J0658.6+0636  | 104.651 | 6.604   | 207.856 | 4.594   | 0.072      | 0.065      | –29    | 6.1      | 0.5      | 0.1             | 7.3      | 1.3             | 2.48          | 0.13                 | PL  | ... | 1     | 2FGL J0658.4+0633                                                                | ... | bcu   | NVSS<br>J065844+063711   |
| J0658.8+2318  | 104.720 | 23.315  | 192.681 | 11.947  | 0.102      | 0.094      | –51    | 4.4      | 0.3      | 0.1             | 3.5      | 0.9             | 2.29          | 0.18                 | PL  | ... | ...   | 1FGL J0658.5+0641                                                                | ... | ...   | ...                      |
| J0659.2–0439c | 104.802 | –4.653  | 217.958 | –0.396  | 0.100      | 0.084      | –1     | 5.6      | 0.9      | 0.2             | 11.6     | 2.2             | 2.40          | 0.11                 | PL  | ... | 1,6   | ...                                                                              | ... | ...   | ...                      |
| J0659.5+1414  | 104.899 | 14.247  | 201.079 | 8.217   | 0.086      | 0.079      | –45    | 23.4     | 0.6      | 0.1             | 28.4     | 1.3             | 2.84          | ...                  | EC  | ... | ...   | 2FGL J0659.7+1417<br>1FGL J0659.8+1414                                           | ... | PSR   | PSR J0659+1414           |

Table 1—Continued

| Name 3FGL     | R.A.    | Decl.   | $l$     | $b$     | $\theta_1$ | $\theta_2$ | $\phi$ | $\sigma$ | $F_{35}$ | $\Delta F_{35}$ | $S_{25}$ | $\Delta S_{25}$ | $\Gamma_{25}$ | $\Delta \Gamma_{25}$ | Mod | Var | Flags | $\gamma$ -ray Assoc.                                                             | TeV | Class | ID or Assoc.             |     |
|---------------|---------|---------|---------|---------|------------|------------|--------|----------|----------|-----------------|----------|-----------------|---------------|----------------------|-----|-----|-------|----------------------------------------------------------------------------------|-----|-------|--------------------------|-----|
| J0700.0+1709  | 105.023 | 17.156  | 198.480 | 9.591   | 0.135      | 0.100      | 37     | 9.8      | 0.5      | 0.1             | 10.2     | 1.2             | 2.69          | 0.09                 | PL  | ... | 3     | 2FGL J0700.3+1710                                                                | ... | bcu   | TXS 0657+172             |     |
| J0700.2+1304  | 105.073 | 13.078  | 202.214 | 7.855   | 0.073      | 0.058      | −82    | 6.1      | 0.3      | 0.1             | 4.1      | 1.0             | 1.80          | 0.18                 | PL  | ... | ...   | 1FGL J0659.9+1303                                                                | ... | bcu   | GB6 J0700+1304           |     |
| J0700.3−6310  | 105.083 | −63.181 | 273.598 | −23.039 | 0.080      | 0.072      | 79     | 5.7      | 0.3      | 0.1             | 3.3      | 0.8             | 1.99          | 0.18                 | PL  | ... | ...   | 3EG J0702−6212                                                                   | ... | bcu   | SUMSS<br>J065958−631238  |     |
| J0700.6−6610  | 105.158 | −66.173 | 276.765 | −23.747 | 0.023      | 0.022      | −65    | 37.0     | 3.1      | 0.1             | 34.5     | 1.6             | 2.07          | 0.03                 | PL  | T   | ...   | 1FHL J0700.6−6612<br>2FGL J0700.3−6611<br>1FGL J0700.4−6611<br>0FGL J0700.0−6611 | ... | bll   | PKS 0700−661             |     |
| J0700.6+3557  | 105.162 | 35.966  | 180.803 | 17.262  | 0.134      | 0.112      | −87    | 4.7      | 0.3      | 0.1             | 3.8      | 0.8             | 2.40          | 0.15                 | PL  | ... | ...   | ...                                                                              | ... | ...   | ...                      |     |
| J0701.4−4634  | 105.350 | −46.574 | 256.793 | −17.732 | 0.052      | 0.050      | 76     | 21.2     | 1.7      | 0.1             | 19.1     | 1.3             | 2.43          | ...                  | LP  | T   | ...   | 1FGL J0702.0−4628<br>2FGL J0701.7−4630                                           | ... | fsrq  | PKS 0700−465             |     |
| J0702.7−1952  | 105.680 | −19.871 | 231.942 | −6.535  | 0.057      | 0.050      | 50     | 8.6      | 0.9      | 0.1             | 9.5      | 1.4             | 2.06          | 0.10                 | PL  | ... | ...   | 2FGL J0702.7−1951<br>1FGL J0702.2−1954                                           | ... | bll   | TXS 0700−197             |     |
| J0703.4−3914  | 105.861 | −39.238 | 249.866 | −14.615 | 0.075      | 0.067      | −55    | 8.8      | 0.6      | 0.1             | 7.6      | 1.0             | 2.29          | 0.09                 | PL  | ... | ...   | 2FGL J0703.1−3912                                                                | ... | bcu   | 1RXS<br>J070312.7−391417 |     |
| J0704.1−1043  | 106.035 | −10.722 | 223.915 | −2.086  | 0.210      | 0.111      | −10    | 9.0      | 1.5      | 0.2             | 17.4     | 2.4             | 2.47          | ...                  | LP  | ... | 3     | 3EG J0706−3837<br>2FGL J0705.3−1043c                                             | ... | ...   | ...                      | 3   |
| J0704.3−4828  | 106.075 | −48.475 | 258.842 | −17.956 | 0.067      | 0.059      | 29     | 4.6      | 0.3      | 0.1             | 2.9      | 0.9             | 1.97          | 0.24                 | PL  | ... | ...   | ...                                                                              | ... | ...   | ...                      | 1   |
| J0705.7−0006  | 106.438 | −0.113  | 214.666 | 3.133   | 0.116      | 0.099      | −78    | 4.1      | 0.5      | 0.1             | 5.4      | 1.3             | 2.27          | 0.14                 | PL  | ... | ...   | ...                                                                              | ... | ...   | ...                      | ... |
| J0706.1−4849  | 106.537 | −48.826 | 259.302 | −17.797 | 0.114      | 0.086      | 47     | 7.8      | 0.7      | 0.1             | 9.0      | 1.2             | 2.41          | 0.09                 | PL  | ... | ...   | 2FGL J0706.7−4845<br>1FGL J0706.3−4849                                           | ... | bcu   | PMN J0705−4847           |     |
| J0706.5+3744  | 106.629 | 37.749  | 179.487 | 18.991  | 0.027      | 0.025      | −81    | 18.8     | 1.1      | 0.1             | 13.2     | 1.3             | 1.89          | 0.06                 | PL  | ... | ...   | 1FHL J0706.5+3744<br>2FGL J0706.5+3744<br>1FGL J0706.5+3744                      | ... | bll   | GB6 J0706+3744           |     |
| J0707.0+7741  | 106.755 | 77.698  | 136.770 | 27.284  | 0.030      | 0.029      | −86    | 25.3     | 1.4      | 0.1             | 15.3     | 1.0             | 2.05          | 0.05                 | PL  | T   | ...   | 2FGL J0706.5+7741                                                                | ... | bll   | NVSS<br>J070651+774137   |     |
| J0707.2+6101  | 106.812 | 61.029  | 155.265 | 25.382  | 0.389      | 0.245      | 39     | 6.3      | 0.2      | 0.1             | 4.7      | 0.7             | 2.81          | 0.15                 | PL  | ... | ...   | 1FGL J0707.3+7742                                                                | ... | bll   | TXS 0702+612             |     |
| J0707.5−3111  | 106.887 | −31.197 | 242.718 | −10.528 | 0.461      | 0.139      | 66     | 5.5      | 0.3      | 0.1             | 6.2      | 1.1             | 2.71          | 0.15                 | PL  | ... | 1,4,9 | ...                                                                              | ... | ...   | ...                      | ... |
| J0707.7−1035c | 106.927 | −10.592 | 224.203 | −1.246  | 0.167      | 0.113      | 84     | 4.1      | 0.8      | 0.2             | 11.6     | 2.9             | 2.49          | 0.13                 | PL  | ... | 6     | ...                                                                              | ... | ...   | ...                      | ... |
| J0708.7+1747  | 107.196 | 17.794  | 198.795 | 11.738  | 0.066      | 0.054      | 78     | 5.4      | 0.3      | 0.1             | 3.4      | 0.9             | 1.84          | 0.24                 | PL  | ... | ...   | ...                                                                              | ... | ...   | ...                      | ... |
| J0708.9+2239  | 107.237 | 22.666  | 194.264 | 13.792  | 0.086      | 0.083      | 31     | 7.2      | 0.5      | 0.1             | 5.4      | 0.9             | 2.08          | 0.12                 | PL  | ... | ...   | 2FGL J0709.0+2236                                                                | ... | bcu   | GB6 J0708+2241           |     |
| J0709.7−0256  | 107.446 | −2.939  | 217.644 | 2.734   | 0.039      | 0.038      | 17     | 21.1     | 2.3      | 0.2             | 28.2     | 1.7             | 2.32          | 0.05                 | PL  | T   | 3     | 2FGL J0709.3−0256                                                                | ... | bll   | PMN J0709−0255           |     |
| J0710.3+5908  | 107.585 | 59.148  | 157.390 | 25.408  | 0.034      | 0.030      | −29    | 15.3     | 0.6      | 0.1             | 8.9      | 1.2             | 1.66          | 0.09                 | PL  | ... | ...   | 1FHL J0710.5+5908<br>2FGL J0710.5+5908<br>1FGL J0710.6+5911                      | P   | bll   | 1H 0658+595              |     |
| J0710.5+4732  | 107.625 | 47.533  | 169.772 | 22.724  | 0.163      | 0.124      | 75     | 11.2     | 0.5      | 0.1             | 9.1      | 0.9             | 2.65          | 0.08                 | PL  | T   | ...   | 2FGL J0710.8+4733<br>1FGL J0711.4+4731                                           | ... | bll   | S4 0707+47               |     |

Table 1—Continued

| Name 3FGL    | R.A.    | Decl.   | $l$     | $b$     | $\theta_1$ | $\theta_2$ | $\phi$ | $\sigma$ | $F_{35}$ | $\Delta F_{35}$ | $S_{25}$ | $\Delta S_{25}$ | $\Gamma_{25}$ | $\Delta \Gamma_{25}$ | Mod | Var | Flags | $\gamma$ -ray Assoc.                                                                                                                    | TeV | Class | ID or Assoc.             |    |
|--------------|---------|---------|---------|---------|------------|------------|--------|----------|----------|-----------------|----------|-----------------|---------------|----------------------|-----|-----|-------|-----------------------------------------------------------------------------------------------------------------------------------------|-----|-------|--------------------------|----|
| J0711.1–1037 | 107.794 | −10.621 | 224.621 | −0.504  | 0.189      | 0.159      | 61     | 8.0      | 1.3      | 0.2             | 14.5     | 2.3             | 2.51          | ...                  | LP  | ... | 1,3   | ...                                                                                                                                     | ... | ...   | ...                      |    |
| J0712.2–3806 | 108.052 | −38.110 | 249.523 | −12.594 | 0.183      | 0.139      | −35    | 5.0      | 0.4      | 0.1             | 5.9      | 1.2             | 2.40          | 0.13                 | PL  | ... | 1     | ...                                                                                                                                     | ... | ...   | ...                      |    |
| J0712.2–6436 | 108.070 | −64.616 | 275.482 | −22.167 | 0.140      | 0.118      | 21     | 5.4      | 0.3      | 0.1             | 4.5      | 0.9             | 2.38          | 0.14                 | PL  | ... | ...   | ...                                                                                                                                     | ... | bcu   | MRC 0712–643             |    |
| J0712.6+5033 | 108.172 | 50.556  | 166.697 | 23.859  | 0.036      | 0.035      | −39    | 21.2     | 1.4      | 0.1             | 15.2     | 1.1             | 2.14          | 0.05                 | PL  | T   | ...   | 1FHL J0712.8+5034<br>2FGL J0712.9+5032<br>1FGL J0712.7+5033<br>0FGL J0712.9+5034                                                        | ... | bll   | GB6 J0712+5033           |    |
| J0713.9+1933 | 108.496 | 19.559  | 197.677 | 13.593  | 0.042      | 0.036      | −35    | 33.6     | 2.9      | 0.2             | 28.7     | 1.5             | 2.28          | ...                  | LP  | T   | 7     | 2FGL J0714.0+1933<br>1FGL J0714.0+1935<br>0FGL J0714.2+1934                                                                             | ... | fsrq  | MG2 J071354+1934         |    |
| J0714.7–3924 | 108.677 | −39.409 | 250.940 | −12.696 | 0.150      | 0.109      | 41     | 4.6      | 0.4      | 0.1             | 5.6      | 1.3             | 2.38          | 0.14                 | PL  | ... | ...   | ...                                                                                                                                     | ... | ...   | ...                      |    |
| J0716.0–4525 | 109.011 | −45.422 | 256.691 | −14.943 | 0.077      | 0.071      | −27    | 4.2      | 0.3      | 0.1             | 3.1      | 0.9             | 2.26          | 0.18                 | PL  | ... | ...   | ...                                                                                                                                     | ... | ...   | ...                      |    |
| J0718.7–4319 | 109.690 | −43.330 | 254.925 | −13.644 | 0.023      | 0.022      | −30    | 28.7     | 2.4      | 0.1             | 28.0     | 2.0             | 1.87          | 0.04                 | PL  | ... | ...   | 1FHL J0718.7–4321<br>2FGL J0718.7–4320<br>1FGL J0718.7–4320                                                                             | ... | bll   | PMN J0718–4319           |    |
| J0718.9–5004 | 109.738 | −50.079 | 261.333 | −16.338 | 0.221      | 0.196      | 60     | 4.9      | 0.4      | 0.1             | 5.1      | 1.0             | 2.39          | 0.14                 | PL  | ... | ...   | 2FGL J0719.2–5000<br>1FGL J0718.8–4958                                                                                                  | ... | ...   | ...                      | 39 |
| J0719.3+3307 | 109.829 | 33.125  | 185.039 | 19.854  | 0.019      | 0.019      | 6      | 66.6     | 6.3      | 0.2             | 57.3     | 2.0             | 2.14          | ...                  | LP  | T   | ...   | 1FHL J0719.2+3308<br>2FGL J0719.3+3306<br>1FGL J0719.3+3306<br>0FGL J0719.4+3302                                                        | ... | fsrq  | B2 0716+33               |    |
| J0720.0–4010 | 110.017 | −40.181 | 252.104 | −12.092 | 0.076      | 0.074      | 55     | 6.0      | 0.5      | 0.1             | 5.8      | 1.1             | 2.23          | 0.13                 | PL  | ... | ...   | ...                                                                                                                                     | ... | bcu   | 1RXS<br>J071939.2–401153 |    |
| J0721.4+0404 | 110.364 | 4.074   | 212.711 | 8.531   | 0.086      | 0.078      | −52    | 10.6     | 0.7      | 0.1             | 11.2     | 1.2             | 2.53          | 0.08                 | PL  | T   | ...   | 2FGL J0721.5+0404c<br>1FGL J0721.4+0401                                                                                                 | ... | fsrq  | PMN J0721+0406           |    |
| J0721.5–0221 | 110.375 | −2.362  | 218.483 | 5.597   | 0.181      | 0.095      | −85    | 4.1      | 0.3      | 0.1             | 3.7      | 1.0             | 2.00          | 0.20                 | PL  | ... | 9     | 2FGL J0721.2–0223                                                                                                                       | ... | ...   | ...                      |    |
| J0721.9+7120 | 110.490 | 71.345  | 143.980 | 28.023  | 0.009      | 0.009      | −1     | 196.6    | 22.0     | 0.3             | 212.1    | 3.6             | 2.04          | ...                  | LP  | T   | ...   | 1FHL J0721.8+7120<br>2FGL J0721.9+7120<br>1FGL J0721.9+7120<br>0FGL J0722.0+7120<br>3EG J0721+7120<br>EGR J0723+7134<br>1AGL J0722+7125 | P   | BLL   | S5 0716+71               |    |
| J0722.2–2648 | 110.551 | −26.804 | 240.195 | −5.699  | 0.180      | 0.125      | 32     | 5.5      | 0.5      | 0.1             | 7.5      | 1.4             | 2.45          | 0.13                 | PL  | ... | 1,4   | ...                                                                                                                                     | ... | ...   | ...                      |    |
| J0723.2–0728 | 110.805 | −7.470  | 223.218 | 3.595   | 0.109      | 0.074      | 46     | 4.2      | 0.3      | 0.1             | 3.6      | 1.1             | 1.80          | 0.23                 | PL  | ... | ...   | ...                                                                                                                                     | ... | bcu   | 1RXS<br>J072259.5–073131 |    |
| J0723.7+2050 | 110.929 | 20.846  | 197.416 | 16.202  | 0.097      | 0.083      | 66     | 5.7      | 0.4      | 0.1             | 4.6      | 0.9             | 2.40          | 0.16                 | PL  | ... | ...   | ...                                                                                                                                     | ... | bcu   | GB6 J0723+2051           |    |

Table 1—Continued

| Name 3FGL     | R.A.    | Decl.   | $l$     | $b$     | $\theta_1$ | $\theta_2$ | $\phi$ | $\sigma$ | $F_{35}$ | $\Delta F_{35}$ | $S_{25}$ | $\Delta S_{25}$ | $\Gamma_{25}$ | $\Delta \Gamma_{25}$ | Mod | Var | Flags | $\gamma$ -ray Assoc.                                                             | TeV | Class          | ID or Assoc.                        |
|---------------|---------|---------|---------|---------|------------|------------|--------|----------|----------|-----------------|----------|-----------------|---------------|----------------------|-----|-----|-------|----------------------------------------------------------------------------------|-----|----------------|-------------------------------------|
| J0724.1+2857  | 111.032 | 28.959  | 189.565 | 19.358  | 0.149      | 0.124      | −80    | 9.0      | 0.4      | 0.1             | 7.3      | 0.9             | 2.59          | 0.11                 | PL  | T   | ...   | 2FGL J0723.9+2901<br>1FGL J0723.6+2908                                           | ... | fsrq           | GB6 J0723+2859                      |
| J0725.2+1425  | 111.323 | 14.431  | 203.636 | 13.916  | 0.019      | 0.019      | −8     | 69.9     | 7.2      | 0.2             | 72.2     | 2.1             | 2.23          | ...                  | LP  | T   | ...   | 1FGL J0725.3+1431<br>1FHL J0725.2+1423<br>2FGL J0725.3+1426                      | ... | FSRQ 4C +14.23 |                                     |
| J0725.4−5007  | 111.371 | −50.120 | 261.806 | −15.394 | 0.071      | 0.063      | −16    | 4.2      | 0.2      | 0.1             | 2.4      | 0.8             | 1.94          | 0.28                 | PL  | ... | ...   | ...                                                                              | ... | ...            | ...                                 |
| J0725.7−0550  | 111.441 | −5.842  | 222.073 | 4.916   | 0.056      | 0.053      | −18    | 6.0      | 0.4      | 0.1             | 4.4      | 1.1             | 1.85          | 0.17                 | PL  | ... | ...   | 2FGL J0725.8−0549                                                                | ... | ...            | ...                                 |
| J0725.8−3532  | 111.459 | −35.537 | 248.379 | −9.017  | 0.077      | 0.068      | −5     | 4.7      | 0.4      | 0.1             | 5.0      | 1.2             | 2.36          | 0.18                 | PL  | ... | ...   | ...                                                                              | ... | ...            | ...                                 |
| J0725.8+0212  | 111.468 | 2.207   | 214.899 | 8.666   | 0.083      | 0.064      | 14     | 9.2      | 0.8      | 0.1             | 8.5      | 1.2             | 2.18          | 0.10                 | PL  | ... | ...   | ...                                                                              | ... | ...            | ...                                 |
| J0725.8−0054  | 111.468 | −0.909  | 217.695 | 7.237   | 0.046      | 0.041      | −70    | 14.2     | 1.1      | 0.1             | 12.6     | 1.2             | 2.19          | 0.08                 | PL  | ... | ...   | 2FGL J0726.0−0053<br>1FGL J0725.9−0053                                           | ... | bcu            | PKS 0723−008                        |
| J0726.6−4727  | 111.664 | −47.465 | 259.391 | −14.117 | 0.097      | 0.080      | −12    | 14.6     | 1.2      | 0.1             | 17.4     | 1.4             | 2.46          | 0.06                 | PL  | T   | ...   | 2FGL J0727.0−4726<br>3EG J0724−4713<br>EGR J0726−4715                            | ... | fsrq           | PMN J0726−4728                      |
| J0728.0+4828  | 112.019 | 48.472  | 169.570 | 25.804  | 0.137      | 0.101      | −86    | 4.3      | 0.2      | 0.1             | 3.0      | 0.8             | 2.37          | 0.19                 | PL  | ... | ...   | ...                                                                              | ... | bcu            | GB6 J0727+4827                      |
| J0729.5−3127  | 112.394 | −31.458 | 245.090 | −6.443  | 0.162      | 0.152      | 39     | 4.8      | 0.4      | 0.1             | 6.9      | 1.4             | 2.65          | 0.15                 | PL  | ... | ...   | ...                                                                              | ... | bcu            | NVSS J0729.5−3127<br>J072922−313128 |
| J0729.7−1448  | 112.431 | −14.801 | 230.436 | 1.524   | 0.193      | 0.108      | −42    | 4.5      | 0.6      | 0.1             | 8.0      | 1.7             | 2.42          | 0.13                 | PL  | ... | ...   | ...                                                                              | ... | PSR            | PSR J0729−1448                      |
| J0730.2−1141  | 112.574 | −11.684 | 227.763 | 3.137   | 0.014      | 0.013      | −79    | 111.9    | 17.6     | 0.4             | 190.2    | 3.3             | 2.28          | ...                  | LP  | T   | ...   | 1FHL J0730.3−1140<br>2FGL J0730.2−1141<br>1FGL J0730.3−1141<br>0FGL J0730.4−1142 | ... | fsrq           | PKS 0727−11                         |
| J0730.3+6720  | 112.585 | 67.344  | 148.554 | 28.601  | 0.157      | 0.149      | −4     | 5.2      | 0.2      | 0.1             | 3.6      | 0.7             | 2.62          | 0.15                 | PL  | ... | 1     | ...                                                                              | ... | fsrq           | GB6 J0731+6718                      |
| J0730.5+3307  | 112.627 | 33.127  | 185.874 | 22.064  | 0.047      | 0.045      | 8      | 8.5      | 0.5      | 0.1             | 5.2      | 0.8             | 2.12          | 0.12                 | PL  | ... | ...   | 1FHL J0730.2+3307                                                                | ... | bl             | 1RXS J073026.0+330727               |
| J0730.5−0537  | 112.632 | −5.620  | 222.436 | 6.066   | 0.052      | 0.049      | 5      | 8.0      | 0.6      | 0.1             | 6.5      | 1.1             | 2.10          | 0.12                 | PL  | ... | ...   | 2FGL J0729.9+3304                                                                | ... | bcu            | TXS 0728−054                        |
| J0730.5−6606  | 112.646 | −66.106 | 277.651 | −20.832 | 0.071      | 0.052      | 45     | 8.6      | 0.5      | 0.1             | 6.1      | 1.1             | 1.79          | 0.13                 | PL  | ... | ...   | 2FGL J0730.6−6607                                                                | ... | bcu            | PMN J0730−6602                      |
| J0731.7−1914c | 112.944 | −19.237 | 234.563 | −0.177  | 0.492      | 0.353      | 37     | 6.0      | 0.9      | 0.2             | 12.9     | 2.0             | 2.52          | 0.10                 | PL  | ... | 1,6,9 | 1FGL J0731.2−1910c                                                               | ... | ...            | ...                                 |
| J0731.8−3010  | 112.974 | −30.177 | 244.191 | −5.399  | 0.051      | 0.048      | 58     | 4.6      | 0.2      | 0.1             | 3.1      | 1.1             | 1.67          | 0.25                 | PL  | ... | ...   | ...                                                                              | ... | ...            | ...                                 |
| J0732.2−4638  | 113.067 | −46.640 | 259.048 | −12.899 | 0.130      | 0.127      | 19     | 10.8     | 0.8      | 0.1             | 9.3      | 1.2             | 2.56          | ...                  | LP  | T   | ...   | ...                                                                              | ... | bcu            | PKS 0731−465                        |
| J0733.3+5904  | 113.328 | 59.067  | 157.973 | 28.311  | 0.142      | 0.109      | −5     | 7.5      | 0.2      | 0.1             | 5.2      | 0.7             | 2.78          | 0.13                 | PL  | T   | ...   | ...                                                                              | ... | ...            | ...                                 |
| J0733.5+5153  | 113.397 | 51.891  | 166.013 | 27.338  | 0.111      | 0.062      | 62     | 6.3      | 0.3      | 0.1             | 3.3      | 0.8             | 1.74          | 0.17                 | PL  | ... | ...   | ...                                                                              | ... | bcu            | NVSS J073326+515355                 |
| J0733.8+5021  | 113.450 | 50.359  | 167.716 | 27.097  | 0.071      | 0.065      | −77    | 9.0      | 0.4      | 0.1             | 6.4      | 0.8             | 2.50          | 0.11                 | PL  | T   | ...   | 2FGL J0733.9+5023                                                                | ... | fsrq           | TXS 0730+504                        |
| J0733.8+4108  | 113.472 | 41.143  | 177.724 | 25.052  | 0.082      | 0.073      | −1     | 6.8      | 0.4      | 0.1             | 4.3      | 0.8             | 2.22          | 0.15                 | PL  | ... | ...   | ...                                                                              | ... | bl             | GB6 J0733+4111                      |
| J0734.3−7709  | 113.577 | −77.161 | 289.097 | −24.067 | 0.053      | 0.050      | −16    | 17.2     | 1.4      | 0.1             | 16.8     | 1.2             | 2.29          | 0.05                 | PL  | T   | ...   | 1FHL J0735.0−7708<br>2FGL J0734.2−7706                                           | ... | bcu            | PKS 0736−770                        |



Table 1—Continued

| Name 3FGL     | R.A.    | Decl.   | $l$     | $b$     | $\theta_1$ | $\theta_2$ | $\phi$ | $\sigma$ | $F_{35}$ | $\Delta F_{35}$ | $S_{25}$ | $\Delta S_{25}$ | $\Gamma_{25}$ | $\Delta \Gamma_{25}$ | Mod | Var | Flags | $\gamma$ -ray Assoc.                                                                                                 | TeV | Class | ID or Assoc.            |
|---------------|---------|---------|---------|---------|------------|------------|--------|----------|----------|-----------------|----------|-----------------|---------------|----------------------|-----|-----|-------|----------------------------------------------------------------------------------------------------------------------|-----|-------|-------------------------|
| J0734.7–1558  | 113.680 | –15.981 | 232.051 | 2.011   | 0.034      | 0.033      | 34     | 32.0     | 5.4      | 0.3             | 42.3     | 1.9             | 2.27          | ...                  | EC  | ... | ...   | 1FGL J0734.1–7715<br>2FGL J0734.6–1558<br>1FGL J0734.7–1557                                                          | ... | PSR   | LAT PSR J0734–1559      |
| J0737.2–3233  | 114.314 | –32.559 | 246.842 | –5.533  | 0.104      | 0.081      | –40    | 12.9     | 1.6      | 0.2             | 13.8     | 1.5             | 2.42          | ...                  | LP  | ... | ...   | 2FGL J0737.1–3235<br>1FGL J0737.4–3239                                                                               | ... | ...   | ...                     |
| J0737.8–8245  | 114.462 | –82.761 | 295.075 | –25.455 | 0.055      | 0.047      | 86     | 7.5      | 0.4      | 0.1             | 4.8      | 1.0             | 1.92          | 0.15                 | PL  | ... | ...   | 2FGL J0737.5–8246                                                                                                    | ... | ...   | ...                     |
| J0738.1+1741  | 114.536 | 17.698  | 201.856 | 18.073  | 0.017      | 0.017      | 17     | 55.3     | 5.5      | 0.2             | 61.2     | 2.4             | 2.01          | 0.02                 | PL  | T   | ...   | 1FHL J0738.0+1742<br>2FGL J0738.0+1742<br>1FGL J0738.2+1741<br>0FGL J0738.2+1738<br>3EG J0737+1721<br>EGR J0737+1720 | ... | bll   | PKS 0735+17             |
| J0739.4+0137  | 114.851 | 1.627   | 216.994 | 11.408  | 0.043      | 0.040      | –9     | 39.0     | 2.7      | 0.2             | 36.6     | 1.4             | 2.48          | ...                  | LP  | T   | ...   | 2FGL J0739.2+0138<br>1FGL J0739.1+0138                                                                               | ... | fsrq  | PKS 0736+01             |
| J0739.8+1312  | 114.974 | 13.211  | 206.327 | 16.622  | 0.532      | 0.400      | 58     | 4.2      | 0.2      | 0.1             | 4.3      | 0.9             | 2.73          | 0.15                 | PL  | ... | 9     | ...                                                                                                                  | ... | ...   | ...                     |
| J0740.6–5230  | 115.162 | –52.504 | 265.079 | –14.262 | 0.089      | 0.073      | –17    | 6.5      | 0.5      | 0.1             | 6.0      | 1.1             | 2.23          | 0.13                 | PL  | ... | ...   | ...                                                                                                                  | ... | ...   | ...                     |
| J0740.8+6621  | 115.220 | 66.361  | 149.709 | 29.611  | 0.097      | 0.087      | –4     | 8.3      | 0.4      | 0.1             | 4.8      | 0.7             | 2.27          | 0.11                 | PL  | ... | ...   | ...                                                                                                                  | ... | PSR   | PSR J0742+6620          |
| J0742.4–8133c | 115.621 | –81.559 | 293.845 | –24.973 | 0.066      | 0.054      | 89     | 4.5      | 0.1      | 0.1             | 2.4      | 0.9             | 1.46          | 0.34                 | PL  | ... | 6     | ...                                                                                                                  | ... | bcu   | SUMSS<br>J074220–813139 |
| J0742.6+5444  | 115.660 | 54.734  | 163.045 | 29.088  | 0.022      | 0.022      | –53    | 61.6     | 4.7      | 0.2             | 47.4     | 1.5             | 2.25          | ...                  | LP  | T   | ...   | 1FHL J0743.0+5446<br>2FGL J0742.6+5442<br>1FGL J0742.2+5443<br>3EG J0743+5447<br>EGR J0743+5438                      | ... | fsrq  | GB6 J0742+5444          |
| J0742.6–5623  | 115.673 | –56.390 | 268.832 | –15.694 | 0.383      | 0.284      | 7      | 6.1      | 0.3      | 0.1             | 6.3      | 1.0             | 2.68          | 0.13                 | PL  | ... | 9     | ...                                                                                                                  | ... | fsrq  | PMN J0743–5619          |
| J0742.7–2824  | 115.680 | –28.405 | 243.786 | –2.476  | 0.085      | 0.067      | 59     | 12.3     | 1.8      | 0.2             | 15.7     | 1.6             | 2.39          | ...                  | EC  | ... | ...   | 2FGL J0742.4–2821<br>1FGL J0742.8–2822                                                                               | ... | PSR   | PSR J0742–2822          |
| J0742.7–3110  | 115.694 | –31.174 | 246.202 | –3.835  | 0.134      | 0.116      | –45    | 5.5      | 0.7      | 0.1             | 8.6      | 1.7             | 2.34          | 0.13                 | PL  | ... | 4     | 2FGL J0742.7–3113<br>1FGL J0743.0–3110                                                                               | ... | ...   | ...                     |
| J0744.1–3804  | 116.038 | –38.074 | 252.381 | –6.976  | 0.332      | 0.218      | 9      | 4.3      | 0.4      | 0.1             | 7.0      | 1.5             | 2.68          | 0.16                 | PL  | ... | 4     | ...                                                                                                                  | ... | bcu   | PMN J0743–3804          |
| J0744.1–2523  | 116.045 | –25.399 | 241.339 | –0.699  | 0.055      | 0.050      | –30    | 18.1     | 2.7      | 0.2             | 23.9     | 1.8             | 2.34          | ...                  | LP  | ... | ...   | 2FGL J0744.1–2523<br>1FGL J0744.1–2523                                                                               | ... | ...   | ...                     |
| J0744.3+1715  | 116.082 | 17.256  | 202.904 | 19.249  | 0.198      | 0.118      | 22     | 4.9      | 0.4      | 0.1             | 4.2      | 0.9             | 2.26          | 0.14                 | PL  | ... | 9     | ...                                                                                                                  | ... | ...   | ...                     |
| J0744.3+7434  | 116.099 | 74.577  | 140.252 | 29.589  | 0.053      | 0.050      | 40     | 11.9     | 0.6      | 0.1             | 6.3      | 0.8             | 1.97          | 0.11                 | PL  | ... | ...   | 1FHL J0745.2+7439<br>2FGL J0745.0+7436<br>1FGL J0745.2+7438                                                          | ... | bll   | MS 0737.9+7441          |

Table 1—Continued

| Name 3FGL    | R.A.    | Decl.   | $l$     | $b$     | $\theta_1$ | $\theta_2$ | $\phi$ | $\sigma$ | $F_{35}$ | $\Delta F_{35}$ | $S_{25}$ | $\Delta S_{25}$ | $\Gamma_{25}$ | $\Delta \Gamma_{25}$ | Mod | Var | Flags | $\gamma$ -ray Assoc.                                        | TeV | Class | ID or Assoc.           |
|--------------|---------|---------|---------|---------|------------|------------|--------|----------|----------|-----------------|----------|-----------------|---------------|----------------------|-----|-----|-------|-------------------------------------------------------------|-----|-------|------------------------|
| J0744.8–4028 | 116.218 | –40.468 | 254.558 | –8.019  | 0.082      | 0.074      | 0      | 7.5      | 0.8      | 0.1             | 9.4      | 1.4             | 2.34          | 0.11                 | PL  | ... | 3     | ...                                                         | ... | bcu   | PMN J0744–4032         |
| J0746.4+2540 | 116.610 | 25.675  | 194.727 | 22.844  | 0.174      | 0.143      | 9      | 10.7     | 0.3      | 0.1             | 10.3     | 1.0             | 2.96          | 0.10                 | PL  | T   | ...   | 2FGL J0746.6+2549<br>1FGL J0746.6+2548                      | ... | fsrq  | B2 0743+25             |
| J0746.4–0225 | 116.618 | –2.422  | 221.486 | 11.082  | 0.075      | 0.060      | 89     | 9.6      | 0.6      | 0.1             | 7.2      | 1.1             | 2.00          | 0.10                 | PL  | ... | ...   | 1FHL J0746.3–0225<br>2FGL J0746.0–0222                      | ... | ...   | ...                    |
| J0746.6–0706 | 116.660 | –7.115  | 225.689 | 8.870   | 0.104      | 0.093      | –77    | 4.9      | 0.5      | 0.1             | 5.1      | 1.2             | 2.19          | 0.15                 | PL  | ... | 5     | 2FGL J0746.5–0713<br>1FGL J0746.5–0711                      | ... | bcu   | PMN J0746–0709         |
| J0746.6–4756 | 116.663 | –47.937 | 261.365 | –11.318 | 0.040      | 0.038      | –56    | 14.6     | 1.2      | 0.1             | 14.3     | 1.3             | 2.25          | 0.08                 | PL  | ... | ...   | 1FHL J0746.3–4757<br>2FGL J0746.5–4758                      | ... | bcu   | PMN J0746–4755         |
| J0746.9+8511 | 116.725 | 85.198  | 128.223 | 28.180  | 0.054      | 0.043      | 61     | 9.7      | 0.4      | 0.1             | 4.7      | 0.8             | 1.79          | 0.13                 | PL  | ... | ...   | 1FHL J0745.2+8511<br>2FGL J0745.9+8512                      | ... | bcu   | NVSS<br>J074715+851208 |
| J0747.2–3311 | 116.814 | –33.186 | 248.424 | –4.012  | 0.035      | 0.031      | –57    | 19.5     | 2.9      | 0.2             | 35.3     | 2.2             | 2.31          | 0.04                 | PL  | T   | ...   | 1FHL J0747.1–3315<br>2FGL J0747.5–3305                      | ... | bcu   | PKS 0745–330           |
| J0747.4–0734 | 116.863 | –7.580  | 226.199 | 8.820   | 0.089      | 0.069      | 58     | 5.5      | 0.5      | 0.1             | 5.2      | 1.2             | 2.11          | 0.15                 | PL  | ... | ...   | ...                                                         | ... | ...   | ...                    |
| J0747.4+0904 | 116.867 | 9.068   | 211.063 | 16.535  | 0.067      | 0.064      | 51     | 5.9      | 0.3      | 0.1             | 3.5      | 0.8             | 2.07          | 0.15                 | PL  | ... | ...   | ...                                                         | ... | bll   | RX J0747.3+0905        |
| J0747.5–4927 | 116.890 | –49.458 | 262.806 | –11.904 | 0.092      | 0.073      | –58    | 6.2      | 0.5      | 0.1             | 5.9      | 1.2             | 2.27          | 0.17                 | PL  | ... | ...   | ...                                                         | ... | ...   | ...                    |
| J0748.0–1639 | 117.004 | –16.661 | 234.218 | 4.452   | 0.136      | 0.115      | –47    | 8.0      | 0.7      | 0.1             | 11.5     | 1.4             | 2.60          | 0.09                 | PL  | ... | 1     | 2FGL J0747.2–1654                                           | ... | bcu   | TXS 0745–165           |
| J0748.3+2401 | 117.093 | 24.024  | 196.571 | 22.676  | 0.071      | 0.059      | –57    | 9.4      | 0.6      | 0.1             | 6.5      | 0.9             | 2.16          | 0.11                 | PL  | T   | ...   | ...                                                         | ... | fsrq  | S3 0745+24             |
| J0748.5+7910 | 117.136 | 79.177  | 134.975 | 29.281  | 0.178      | 0.147      | –49    | 4.7      | 0.2      | 0.1             | 2.8      | 0.6             | 2.34          | 0.14                 | PL  | ... | ...   | 2FGL J0745.5+7910                                           | ... | bcu   | JVAS J0750+7909        |
| J0748.7–5116 | 117.178 | –51.279 | 264.540 | –12.596 | 0.110      | 0.093      | –58    | 5.1      | 0.4      | 0.1             | 6.3      | 1.3             | 2.62          | 0.14                 | PL  | ... | 1     | ...                                                         | ... | ...   | ...                    |
| J0748.8–2208 | 117.202 | –22.135 | 239.049 | 1.858   | 0.122      | 0.087      | 48     | 5.9      | 0.7      | 0.1             | 8.6      | 1.6             | 2.37          | 0.12                 | PL  | ... | 4     | 2FGL J0748.5–2204                                           | ... | ...   | ...                    |
| J0748.8+4929 | 117.220 | 49.489  | 169.146 | 29.345  | 0.167      | 0.158      | 56     | 5.7      | 0.3      | 0.1             | 4.2      | 0.8             | 2.34          | 0.14                 | PL  | ... | ...   | ...                                                         | ... | bcu   | NVSS<br>J074837+493040 |
| J0749.0+4459 | 117.265 | 44.987  | 174.226 | 28.618  | 0.121      | 0.092      | –58    | 8.5      | 0.4      | 0.1             | 5.8      | 0.8             | 2.37          | 0.11                 | PL  | T   | ...   | 2FGL J0747.7+4501                                           | ... | ...   | ...                    |
| J0749.4+1059 | 117.358 | 10.983  | 209.470 | 17.795  | 0.141      | 0.115      | 38     | 6.0      | 0.4      | 0.1             | 4.7      | 0.9             | 2.20          | 0.14                 | PL  | ... | ...   | ...                                                         | ... | bcu   | TXS 0746+110           |
| J0749.5+1320 | 117.398 | 13.340  | 207.235 | 18.820  | 0.133      | 0.110      | –44    | 6.4      | 0.5      | 0.1             | 5.4      | 1.0             | 2.25          | 0.13                 | PL  | ... | ...   | ...                                                         | ... | ...   | ...                    |
| J0750.6+1232 | 117.674 | 12.539  | 208.123 | 18.731  | 0.077      | 0.060      | 58     | 13.3     | 0.9      | 0.1             | 12.5     | 1.2             | 2.41          | 0.07                 | PL  | T   | ...   | 2FGL J0750.6+1230<br>1FGL J0750.6+1235                      | ... | fsrq  | OI 280                 |
| J0751.2+1806 | 117.805 | 18.107  | 202.757 | 21.093  | 0.048      | 0.043      | 31     | 23.9     | 2.2      | 0.2             | 13.0     | 1.0             | 2.08          | ...                  | EC  | ... | ...   | 2FGL J0751.1+1809<br>1FGL J0751.1+1807                      | ... | PSR   | PSR J0751+1807         |
| J0751.7–2944 | 117.938 | –29.734 | 245.929 | –1.439  | 0.084      | 0.081      | 17     | 5.5      | 0.6      | 0.1             | 8.8      | 1.7             | 2.45          | 0.12                 | PL  | ... | 1,3   | ...                                                         | ... | ...   | ...                    |
| J0752.6–1629 | 118.152 | –16.489 | 234.625 | 5.489   | 0.105      | 0.079      | –39    | 6.5      | 0.5      | 0.1             | 6.2      | 1.1             | 2.20          | 0.13                 | PL  | ... | 1     | 2FGL J0753.2–1634                                           | ... | ...   | ...                    |
| J0753.1+5353 | 118.283 | 53.889  | 164.196 | 30.522  | 0.043      | 0.039      | 51     | 16.7     | 1.0      | 0.1             | 10.8     | 1.0             | 2.11          | 0.07                 | PL  | ... | ...   | 1FHL J0753.0+5351<br>2FGL J0753.0+5352<br>1FGL J0752.8+5353 | ... | bll   | 4C +54.15              |
| J0754.4–1148 | 118.620 | –11.813 | 230.786 | 8.237   | 0.043      | 0.036      | –1     | 18.4     | 1.6      | 0.1             | 18.0     | 1.4             | 2.11          | 0.06                 | PL  | ... | ...   | 1FHL J0754.3–1149                                           | ... | bll   | TXS 0752–116           |

Table 1—Continued

| Name 3FGL    | R.A.    | Decl.   | $l$     | $b$     | $\theta_1$ | $\theta_2$ | $\phi$ | $\sigma$ | $F_{35}$ | $\Delta F_{35}$ | $S_{25}$ | $\Delta S_{25}$ | $\Gamma_{25}$ | $\Delta \Gamma_{25}$ | Mod | Var | Flags | $\gamma$ -ray Assoc.                                        | TeV | Class | ID or Assoc.                |
|--------------|---------|---------|---------|---------|------------|------------|--------|----------|----------|-----------------|----------|-----------------|---------------|----------------------|-----|-----|-------|-------------------------------------------------------------|-----|-------|-----------------------------|
|              |         |         |         |         |            |            |        |          |          |                 |          |                 |               |                      |     |     |       | 2FGL J0754.4–1147<br>1FGL J0754.4–1147                      |     |       |                             |
| J0754.8+4824 | 118.709 | 48.410  | 170.538 | 30.158  | 0.037      | 0.036      | 8      | 18.5     | 1.1      | 0.1             | 12.5     | 1.0             | 2.14          | 0.06                 | PL  | ... | ...   | 2FGL J0754.8+4824                                           | ... | bll   | GB1 0751+485                |
| J0755.2–2633 | 118.802 | –26.562 | 243.599 | 0.846   | 0.410      | 0.233      | 33     | 7.3      | 0.7      | 0.1             | 11.6     | 1.6             | 2.60          | 0.10                 | PL  | ... | 3,9   | ...                                                         | ... | ...   | ...                         |
| J0756.3–6433 | 119.077 | –64.563 | 277.270 | –17.759 | 0.071      | 0.059      | 37     | 7.8      | 0.5      | 0.1             | 5.8      | 0.9             | 2.22          | 0.12                 | PL  | ... | ...   | 2FGL J0756.3–6433                                           | ... | bcu   | SUMSS<br>J075625–643031     |
| J0757.0+0956 | 119.274 | 9.948   | 211.306 | 19.056  | 0.036      | 0.034      | 59     | 24.5     | 1.9      | 0.1             | 21.1     | 1.3             | 2.18          | 0.05                 | PL  | T   | ...   | 1FHL J0757.2+0955<br>2FGL J0757.1+0957<br>1FGL J0757.2+0956 | ... | bll   | PKS 0754+100                |
| J0757.5–0536 | 119.396 | –5.606  | 225.696 | 11.980  | 0.338      | 0.208      | 23     | 6.2      | 0.3      | 0.1             | 6.5      | 1.0             | 2.69          | 0.12                 | PL  | ... | ...   | ...                                                         | ... | ...   | ...                         |
| J0758.1+1130 | 119.545 | 11.504  | 209.932 | 19.958  | 0.135      | 0.117      | –4     | 4.9      | 0.3      | 0.1             | 3.5      | 0.8             | 2.16          | 0.15                 | PL  | ... | ...   | ...                                                         | ... | fsrq  | TXS 0755+117                |
| J0758.6–1451 | 119.656 | –14.866 | 233.960 | 7.562   | 0.078      | 0.071      | 85     | 12.1     | 1.1      | 0.1             | 7.3      | 1.1             | 2.25          | ...                  | LP  | ... | ...   | 2FGL J0758.8–1448<br>1FGL J0758.6–1450                      | ... | ...   | ...                         |
| J0758.7+3747 | 119.679 | 37.789  | 182.687 | 28.877  | 0.099      | 0.093      | –46    | 4.6      | 0.3      | 0.1             | 2.8      | 0.7             | 2.16          | 0.16                 | PL  | ... | ...   | ...                                                         | ... | rdg   | NGC 2484                    |
| J0758.9+2705 | 119.727 | 27.090  | 194.286 | 25.948  | 0.093      | 0.071      | –85    | 8.3      | 0.5      | 0.1             | 5.2      | 0.8             | 2.13          | 0.12                 | PL  | ... | ...   | ...                                                         | ... | bll   | SDSS<br>J075846.99+270515.5 |
| J0800.6–4806 | 120.174 | –48.115 | 262.693 | –9.359  | 0.316      | 0.275      | 77     | 5.6      | 0.4      | 0.1             | 7.3      | 1.3             | 2.69          | 0.15                 | PL  | ... | 1,4   | ...                                                         | ... | ...   | ...                         |
| J0800.9+4401 | 120.244 | 44.017  | 175.757 | 30.536  | 0.137      | 0.097      | –70    | 8.2      | 0.4      | 0.1             | 5.5      | 0.8             | 2.38          | 0.11                 | PL  | ... | ...   | 2FGL J0801.5+4401<br>1FGL J0800.5+4407                      | ... | bll   | B3 0757+441                 |
| J0802.0+1005 | 120.508 | 10.087  | 211.725 | 20.213  | 0.062      | 0.060      | 2      | 5.6      | 0.3      | 0.1             | 3.5      | 0.8             | 2.15          | 0.15                 | PL  | ... | ...   | ...                                                         | ... | bll   | NVSS<br>J080204+100639      |
| J0802.3–5610 | 120.583 | –56.169 | 269.931 | –13.176 | 0.098      | 0.083      | –31    | 12.3     | 0.9      | 0.1             | 13.0     | 1.2             | 2.47          | 0.07                 | PL  | ... | ...   | 2FGL J0802.7–5615<br>1FGL J0802.4–5622                      | ... | ...   | ...                         |
| J0802.3–0941 | 120.590 | –9.696  | 229.917 | 10.974  | 0.065      | 0.058      | 89     | 8.7      | 0.6      | 0.1             | 7.4      | 1.1             | 2.28          | 0.11                 | PL  | ... | ...   | 2FGL J0802.6–0940                                           | ... | ...   | ...                         |
| J0803.3–0339 | 120.832 | –3.663  | 224.672 | 14.178  | 0.066      | 0.049      | –43    | 14.5     | 1.0      | 0.1             | 11.2     | 1.2             | 2.00          | 0.08                 | PL  | ... | ...   | 1FHL J0803.4–0334<br>2FGL J0803.2–0339<br>1FGL J0803.1–0339 | ... | bcu   | TXS 0800–034                |
| J0804.0–3629 | 121.024 | –36.497 | 253.050 | –2.761  | 0.048      | 0.042      | 80     | 9.0      | 0.9      | 0.1             | 10.4     | 1.7             | 1.83          | 0.10                 | PL  | ... | 3     | ...                                                         | ... | bcu   | NVSS<br>J080405–362919      |
| J0804.4+0418 | 121.106 | 4.300   | 217.498 | 18.184  | 0.227      | 0.202      | 14     | 4.7      | 0.3      | 0.1             | 4.1      | 0.8             | 2.57          | 0.17                 | PL  | ... | ...   | ...                                                         | ... | bcu   | MG1 J080357+0420            |
| J0805.0–0622 | 121.253 | –6.375  | 227.314 | 13.207  | 0.066      | 0.055      | 16     | 7.9      | 0.5      | 0.1             | 6.2      | 1.2             | 1.90          | 0.14                 | PL  | ... | ...   | 1FHL J0804.8–0626                                           | ... | bcu   | 1RXS<br>J080458.3–062432    |
| J0805.2–0112 | 121.324 | –1.208  | 222.694 | 15.795  | 0.085      | 0.068      | 15     | 10.4     | 0.6      | 0.1             | 7.8      | 0.9             | 2.34          | 0.09                 | PL  | T   | ...   | 2FGL J0805.2–0121                                           | ... | fsrq  | PKS B0802–010               |
| J0805.4+7534 | 121.352 | 75.581  | 138.888 | 30.791  | 0.024      | 0.023      | 37     | 26.6     | 1.4      | 0.1             | 16.0     | 1.2             | 1.92          | 0.05                 | PL  | T   | ...   | 1FHL J0805.4+7534<br>2FGL J0805.3+7535<br>1FGL J0804.7+7534 | ... | bll   | RX J0805.4+7534             |
| J0805.4+6144 | 121.358 | 61.745  | 155.039 | 32.367  | 0.119      | 0.095      | –72    | 18.3     | 0.6      | 0.1             | 12.5     | 0.8             | 2.75          | 0.06                 | PL  | T   | ...   | 2FGL J0805.5+6145<br>1FGL J0806.2+6148                      | ... | fsrq  | TXS 0800+618                |
| J0806.6+5933 | 121.669 | 59.559  | 157.624 | 32.583  | 0.086      | 0.071      | –9     | 6.6      | 0.3      | 0.1             | 3.5      | 0.7             | 1.88          | 0.15                 | PL  | ... | ...   | ...                                                         | ... | bll   | SBS 0802+596                |
| J0807.1–0541 | 121.782 | –5.695  | 226.977 | 14.002  | 0.039      | 0.035      | –71    | 19.4     | 1.6      | 0.1             | 17.7     | 1.4             | 2.07          | 0.06                 | PL  | T   | ...   | 1FHL J0807.1–0543                                           | ... | bll   | PKS 0804–05                 |

Table 1—Continued

| Name 3FGL    | R.A.    | Decl.   | $l$     | $b$     | $\theta_1$ | $\theta_2$ | $\phi$ | $\sigma$ | $F_{35}$ | $\Delta F_{35}$ | $S_{25}$ | $\Delta S_{25}$ | $\Gamma_{25}$ | $\Delta \Gamma_{25}$ | Mod | Var | Flags | $\gamma$ -ray Assoc.                                        | TeV | Class | ID or Assoc.                |     |
|--------------|---------|---------|---------|---------|------------|------------|--------|----------|----------|-----------------|----------|-----------------|---------------|----------------------|-----|-----|-------|-------------------------------------------------------------|-----|-------|-----------------------------|-----|
| J0807.1+7744 | 121.786 | 77.738  | 136.409 | 30.457  | 0.163      | 0.089      | 79     | 7.7      | 0.3      | 0.1             | 4.3      | 0.6             | 2.44          | 0.12                 | PL  | T   | ...   | 2FGL J0807.1–0543<br>1FGL J0807.0–0544<br>...               | ... | bcu   | NVSS<br>J080637+774607      |     |
| J0807.9+4946 | 121.997 | 49.774  | 169.236 | 32.451  | 0.212      | 0.182      | −64    | 6.1      | 0.3      | 0.1             | 4.4      | 0.7             | 2.57          | 0.14                 | PL  | ... | ...   | ...                                                         | ... | fsrq  | OJ 508                      |     |
| J0808.2−0751 | 122.072 | −7.852  | 229.045 | 13.170  | 0.016      | 0.016      | 63     | 73.8     | 9.7      | 0.3             | 85.2     | 2.6             | 2.09          | ...                  | LP  | T   | ...   | 1FHL J0808.2−0749<br>2FGL J0808.2−0750<br>1FGL J0808.2−0750 | ... | fsrq  | PKS 0805−07                 |     |
| J0809.5+4045 | 122.396 | 40.757  | 179.823 | 31.543  | 0.181      | 0.133      | −74    | 5.4      | 0.2      | 0.1             | 4.3      | 0.8             | 2.65          | 0.16                 | PL  | ... | ...   | ...                                                         | ... | fsrq  | S4 0805+41                  |     |
| J0809.5+5342 | 122.396 | 53.709  | 164.586 | 32.936  | 0.097      | 0.078      | −0     | 8.3      | 0.4      | 0.1             | 5.5      | 0.8             | 2.41          | 0.10                 | PL  | T   | ...   | ...                                                         | ... | fsrq  | 87GB<br>080551.6+535010     |     |
| J0809.6+3456 | 122.409 | 34.942  | 186.461 | 30.350  | 0.048      | 0.043      | 38     | 8.0      | 0.3      | 0.1             | 4.5      | 1.0             | 1.67          | 0.13                 | PL  | ... | ...   | 1FGL J0809.4+3455                                           | ... | bll   | B2 0806+35                  |     |
| J0809.8+5218 | 122.454 | 52.308  | 166.255 | 32.910  | 0.016      | 0.015      | 36     | 56.2     | 4.6      | 0.2             | 53.6     | 2.3             | 1.88          | 0.02                 | PL  | T   | ...   | 1FHL J0809.8+5217<br>2FGL J0809.8+5218<br>1FGL J0809.5+5219 | P   | bll   | 1ES 0806+524                |     |
| J0810.5−5214 | 122.630 | −52.247 | 267.106 | −10.149 | 0.135      | 0.106      | −1     | 7.2      | 0.7      | 0.1             | 10.2     | 1.4             | 2.55          | 0.10                 | PL  | ... | 1     | ...                                                         | ... | ...   | ...                         | ... |
| J0811.2−7529 | 122.811 | −75.492 | 288.279 | −21.430 | 0.024      | 0.023      | −7     | 30.8     | 2.5      | 0.1             | 28.4     | 1.8             | 1.95          | 0.04                 | PL  | ... | ...   | 1FHL J0811.1−7525<br>2FGL J0811.1−7527<br>1FGL J0811.1−7527 | ... | bll   | PMN J0810−7530              |     |
| J0811.3+0146 | 122.848 | 1.781   | 220.700 | 18.557  | 0.030      | 0.028      | 38     | 28.7     | 2.5      | 0.1             | 27.7     | 1.5             | 2.16          | 0.04                 | PL  | T   | ...   | 1FHL J0811.4+0149<br>2FGL J0811.4+0149<br>1FGL J0811.2+0148 | ... | bll   | OJ 014                      |     |
| J0812.0+0237 | 123.003 | 2.626   | 219.989 | 19.091  | 0.051      | 0.047      | 7      | 7.8      | 0.4      | 0.1             | 5.0      | 1.1             | 1.72          | 0.17                 | PL  | ... | ...   | ...                                                         | ... | bll   | PMN J0811+0237              |     |
| J0812.9+5555 | 123.242 | 55.933  | 161.938 | 33.461  | 0.086      | 0.070      | −90    | 5.6      | 0.3      | 0.1             | 2.9      | 0.7             | 2.11          | 0.16                 | PL  | ... | ...   | ...                                                         | ... | bll   | NVSS<br>J081251+555422      |     |
| J0813.3+6509 | 123.349 | 65.166  | 150.909 | 33.001  | 0.113      | 0.110      | −43    | 4.4      | 0.3      | 0.1             | 2.9      | 0.8             | 2.20          | 0.23                 | PL  | ... | ...   | 2FGL J0812.6+6511                                           | ... | bcu   | GB6 J0812+6508              |     |
| J0813.5−0356 | 123.387 | −3.939  | 226.220 | 16.262  | 0.089      | 0.074      | 28     | 5.2      | 0.2      | 0.1             | 3.1      | 0.9             | 1.67          | 0.19                 | PL  | ... | ...   | ...                                                         | ... | ...   | ...                         |     |
| J0814.1−1012 | 123.545 | −10.209 | 231.889 | 13.214  | 0.045      | 0.043      | −5     | 15.3     | 1.3      | 0.1             | 14.2     | 1.4             | 2.07          | 0.07                 | PL  | T   | ...   | 2FGL J0814.0−1006                                           | ... | bll   | NVSS<br>J081411−101208      |     |
| J0814.5+2943 | 123.650 | 29.721  | 192.611 | 30.027  | 0.096      | 0.070      | 53     | 5.8      | 0.3      | 0.1             | 3.2      | 0.7             | 1.94          | 0.16                 | PL  | ... | ...   | 1FGL J0814.5−1011                                           | ... | bll   | EXO 0811.2+2949             |     |
| J0814.7+6428 | 123.677 | 64.480  | 151.705 | 33.214  | 0.031      | 0.030      | −35    | 26.7     | 1.8      | 0.1             | 21.6     | 1.1             | 2.30          | 0.04                 | PL  | T   | ...   | 2FGL J0814.7+6429                                           | ... | bll   | GB6 J0814+6431              |     |
| J0816.1−5044 | 124.028 | −50.748 | 266.294 | −8.613  | 0.187      | 0.133      | 9      | 7.7      | 0.8      | 0.1             | 12.3     | 1.6             | 2.49          | 0.09                 | PL  | ... | ...   | ...                                                         | ... | ...   | ...                         |     |
| J0816.4−1311 | 124.116 | −13.191 | 234.793 | 12.128  | 0.023      | 0.021      | −59    | 26.5     | 2.0      | 0.1             | 25.6     | 2.1             | 1.78          | 0.05                 | PL  | T   | ...   | 1FHL J0816.3−1310<br>2FGL J0816.4−1311<br>1FGL J0816.4−1311 | ... | bll   | PMN J0816−1311              |     |
| J0816.5+2049 | 124.144 | 20.821  | 202.419 | 27.649  | 0.124      | 0.104      | 76     | 4.4      | 0.3      | 0.1             | 2.8      | 0.7             | 2.03          | 0.18                 | PL  | ... | ...   | 2FGL J0816.9+2049                                           | ... | bll   | SDSS<br>J081649.78+205106.4 |     |
| J0816.7−2421 | 124.180 | −24.357 | 244.336 | 6.127   | 0.075      | 0.072      | −14    | 10.6     | 0.8      | 0.1             | 10.5     | 1.1             | 2.43          | 0.08                 | PL  | T   | 3     | 2FGL J0816.7−2420                                           | ... | bcu   | PMN J0816−2421              |     |
| J0816.7+5739 | 124.183 | 57.660  | 159.851 | 33.944  | 0.045      | 0.042      | −4     | 20.0     | 1.2      | 0.1             | 13.1     | 1.0             | 2.11          | 0.06                 | PL  | T   | ...   | 2FGL J0816.5+5739                                           | ... | bll   | SBS 0812+578                |     |

Table 1—Continued

| Name 3FGL     | R.A.    | Decl.   | $l$     | $b$     | $\theta_1$ | $\theta_2$ | $\phi$ | $\sigma$ | $F_{35}$ | $\Delta F_{35}$ | $S_{25}$ | $\Delta S_{25}$ | $\Gamma_{25}$ | $\Delta \Gamma_{25}$ | Mod | Var | Flags | $\gamma$ -ray Assoc.                                                             | TeV | Class | ID or Assoc.     |
|---------------|---------|---------|---------|---------|------------|------------|--------|----------|----------|-----------------|----------|-----------------|---------------|----------------------|-----|-----|-------|----------------------------------------------------------------------------------|-----|-------|------------------|
| J0817.8–0935  | 124.472 | −9.588  | 231.831 | 14.317  | 0.040      | 0.037      | 81     | 17.5     | 1.4      | 0.1             | 15.8     | 1.4             | 2.04          | 0.06                 | PL  | ... | ...   | 1FGL J0816.7+5739<br>1FHL J0818.0−0935<br>2FGL J0818.2−0935<br>1FGL J0818.0−0938 | ... | bll   | TXS 0815−094     |
| J0818.0+3237  | 124.524 | 32.630  | 189.567 | 31.505  | 0.080      | 0.069      | −13    | 6.6      | 0.4      | 0.1             | 4.1      | 0.8             | 2.18          | 0.12                 | PL  | ... | ...   | 2FGL J0817.9+3238                                                                | ... | ...   | ...              |
| J0818.2+4223  | 124.562 | 42.399  | 178.204 | 33.401  | 0.018      | 0.018      | −85    | 67.4     | 6.3      | 0.2             | 58.6     | 2.2             | 2.11          | ...                  | LP  | T   | ...   | 1FHL J0817.9+4224<br>2FGL J0818.2+4223<br>1FGL J0818.2+4222<br>0FGL J0818.3+4222 | ... | bll   | S4 0814+42       |
| J0818.8+2751  | 124.714 | 27.855  | 194.987 | 30.395  | 0.188      | 0.148      | −36    | 5.8      | 0.3      | 0.1             | 4.2      | 0.8             | 2.46          | 0.15                 | PL  | ... | ...   | 2FGL J0819.3+2750                                                                | ... | bll   | 5C 07.119        |
| J0820.4+3640  | 125.124 | 36.682  | 185.024 | 32.876  | 0.115      | 0.082      | −87    | 6.9      | 0.4      | 0.1             | 4.5      | 0.8             | 2.28          | 0.13                 | PL  | ... | ...   | ...                                                                              | ... | bll   | MG2 J082018+3640 |
| J0820.9−1258  | 125.232 | −12.976 | 235.200 | 13.163  | 0.099      | 0.086      | −65    | 4.1      | 0.3      | 0.1             | 3.2      | 0.9             | 2.27          | 0.20                 | PL  | ... | ...   | ...                                                                              | ... | bll   | PKS 0818−128     |
| J0822.6−4250e | 125.660 | −42.840 | 260.318 | −3.276  | ...        | ...        | ...    | 31.7     | 8.3      | 0.3             | 92.3     | 3.8             | 2.05          | 0.03                 | PL  | ... | ...   | 1FGL J0823.3−4248<br>1FHL J0822.6−4250e<br>2FGL J0823.0−4246                     | ... | SNR   | Puppis A         |
| J0822.9+4041  | 125.738 | 40.695  | 180.382 | 34.032  | 0.100      | 0.078      | 63     | 7.9      | 0.4      | 0.1             | 6.3      | 0.9             | 2.49          | 0.13                 | PL  | T   | ...   | 2FGL J0823.0+4041                                                                | ... | fsrq  | B3 0819+408      |
| J0823.3−4205c | 125.848 | −42.093 | 259.783 | −2.736  | 0.066      | 0.058      | 63     | 4.7      | 0.7      | 0.2             | 8.1      | 2.5             | 2.06          | 0.19                 | PL  | ... | 6     | ...                                                                              | ... | ...   | ...              |
| J0823.6−4838  | 125.913 | −48.637 | 265.205 | −6.426  | 0.125      | 0.103      | −49    | 7.4      | 0.8      | 0.1             | 14.4     | 2.0             | 2.61          | 0.09                 | PL  | T   | ...   | ...                                                                              | ... | ...   | ...              |
| J0824.1+2434  | 126.036 | 24.576  | 199.029 | 30.543  | 0.154      | 0.124      | −16    | 7.4      | 0.4      | 0.1             | 6.2      | 1.0             | 2.52          | 0.12                 | PL  | ... | ...   | ...                                                                              | ... | fsrq  | B2 0821+24       |
| J0824.9+5551  | 126.231 | 55.858  | 161.982 | 35.138  | 0.075      | 0.071      | −40    | 15.2     | 0.7      | 0.1             | 11.1     | 0.8             | 2.61          | 0.07                 | PL  | T   | ...   | 2FGL J0824.9+5552<br>1FGL J0825.0+5555<br>0FGL J0824.9+5551                      | ... | fsrq  | OJ 535           |
| J0824.9+3916  | 126.249 | 39.277  | 182.146 | 34.206  | 0.102      | 0.093      | 30     | 9.2      | 0.5      | 0.1             | 6.4      | 0.8             | 2.44          | 0.10                 | PL  | T   | ...   | 2FGL J0824.7+3914                                                                | ... | fsrq  | 4C +39.23        |
| J0825.4−0213  | 126.356 | −2.231  | 226.213 | 19.683  | 0.355      | 0.245      | 28     | 4.2      | 0.3      | 0.1             | 3.7      | 0.8             | 2.40          | 0.18                 | PL  | ... | ...   | ...                                                                              | ... | bcu   | PMN J0825−0204   |
| J0825.8−3217  | 126.454 | −32.286 | 252.035 | 3.302   | 0.071      | 0.062      | −50    | 10.5     | 0.9      | 0.1             | 12.5     | 1.3             | 2.49          | 0.09                 | PL  | T   | 3     | 2FGL J0825.9−3216<br>1FGL J0825.9−3216                                           | ... | bcu   | PKS 0823−321     |
| J0825.9−2230  | 126.498 | −22.505 | 243.984 | 8.926   | 0.018      | 0.018      | −22    | 47.8     | 4.9      | 0.2             | 55.1     | 2.3             | 2.00          | 0.03                 | PL  | T   | ...   | 1FHL J0826.0−2230<br>2FGL J0825.9−2229<br>1FGL J0825.8−2230<br>0FGL J0826.0−2228 | ... | bll   | PKS 0823−223     |
| J0826.0+0307  | 126.519 | 3.125   | 221.280 | 22.426  | 0.086      | 0.075      | −77    | 8.3      | 0.5      | 0.1             | 5.8      | 1.0             | 2.03          | 0.13                 | PL  | ... | ...   | 1FHL J0825.9+0308<br>2FGL J0825.9+0308<br>1FGL J0825.9+0309                      | ... | bll   | PKS 0823+033     |
| J0826.3−5056  | 126.589 | −50.948 | 267.370 | −7.381  | 0.083      | 0.071      | −67    | 7.5      | 0.9      | 0.1             | 10.7     | 1.6             | 2.23          | 0.10                 | PL  | ... | ...   | ...                                                                              | ... | ...   | ...              |
| J0826.3−6400  | 126.593 | −64.011 | 278.437 | −14.649 | 0.127      | 0.106      | −27    | 5.9      | 0.4      | 0.1             | 5.3      | 1.0             | 2.34          | 0.13                 | PL  | ... | ...   | ...                                                                              | ... | ...   | ...              |

Table 1—Continued

| Name 3FGL     | R.A.    | Decl.   | $l$     | $b$     | $\theta_1$ | $\theta_2$ | $\phi$ | $\sigma$ | $F_{35}$ | $\Delta F_{35}$ | $S_{25}$ | $\Delta S_{25}$ | $\Gamma_{25}$ | $\Delta \Gamma_{25}$ | Mod | Var | Flags | $\gamma$ -ray Assoc.                                                       | TeV | Class | ID or Assoc.              |
|---------------|---------|---------|---------|---------|------------|------------|--------|----------|----------|-----------------|----------|-----------------|---------------|----------------------|-----|-----|-------|----------------------------------------------------------------------------|-----|-------|---------------------------|
| J0827.2–0711  | 126.809 | –7.190  | 230.956 | 17.539  | 0.077      | 0.063      | –70    | 8.3      | 0.5      | 0.1             | 5.5      | 0.9             | 2.07          | 0.13                 | PL  | ... | ...   | ...                                                                        | ... | bcu   | PMN J0827–0708            |
| J0828.5+5217  | 127.140 | 52.295  | 166.336 | 35.774  | 0.135      | 0.097      | 81     | 4.2      | 0.2      | 0.1             | 2.3      | 0.6             | 2.13          | 0.19                 | PL  | ... | ...   | ...                                                                        | ... | fsrq  | TXS 0824+524              |
| J0828.8–2420  | 127.208 | –24.340 | 245.886 | 8.417   | 0.114      | 0.085      | –34    | 5.5      | 0.4      | 0.1             | 4.1      | 0.9             | 2.00          | 0.16                 | PL  | ... | 1     | ...                                                                        | ... | bcu   | NVSS<br>J082841–241850    |
| J0829.3+0901  | 127.337 | 9.017   | 215.933 | 25.827  | 0.129      | 0.097      | –12    | 4.2      | 0.2      | 0.1             | 2.6      | 0.8             | 1.95          | 0.22                 | PL  | ... | ...   | 1FHL J0828.9+0902<br>1FGL J0828.9+0901                                     | ... | fsrq  | TXS 0826+091              |
| J0829.6–1137  | 127.404 | –11.621 | 235.199 | 15.680  | 0.091      | 0.080      | 53     | 5.7      | 0.3      | 0.1             | 3.7      | 0.9             | 1.89          | 0.19                 | PL  | ... | ...   | ...                                                                        | ... | bcu   | NVSS<br>J082939–114103    |
| J0829.8–5239  | 127.468 | –52.659 | 269.099 | –7.916  | 0.108      | 0.099      | –18    | 6.0      | 0.6      | 0.1             | 8.9      | 1.5             | 2.56          | 0.11                 | PL  | ... | 1     | ...                                                                        | ... | ...   | ...                       |
| J0830.3–5855  | 127.575 | –58.918 | 274.346 | –11.444 | 0.177      | 0.118      | 85     | 9.2      | 0.6      | 0.1             | 9.7      | 1.1             | 2.61          | 0.09                 | PL  | T   | ...   | ...                                                                        | ... | bcu   | PMN J0829–5856            |
| J0830.5–4452  | 127.635 | –44.869 | 262.800 | –3.288  | 0.094      | 0.070      | –78    | 4.7      | 1.1      | 0.4             | 12.3     | 4.2             | 1.95          | 0.20                 | PL  | ... | ...   | ...                                                                        | ... | ...   | Vela X field <sup>a</sup> |
| J0830.7+2408  | 127.681 | 24.138  | 200.061 | 31.831  | 0.064      | 0.059      | –4     | 21.3     | 1.1      | 0.1             | 19.0     | 1.1             | 2.63          | 0.05                 | PL  | T   | ...   | 2FGL J0830.5+2407<br>1FGL J0830.5+2407<br>3EG J0829+2413<br>EGR J0829+2415 | ... | FSRQ  | OJ 248                    |
| J0830.8+2629  | 127.704 | 26.491  | 197.414 | 32.553  | 0.203      | 0.188      | –55    | 5.2      | 0.3      | 0.1             | 4.3      | 0.9             | 2.56          | 0.16                 | PL  | ... | ...   | ...                                                                        | ... | ...   | ...                       |
| J0831.9+0430  | 127.991 | 4.503   | 220.704 | 24.369  | 0.029      | 0.028      | –24    | 42.3     | 3.4      | 0.2             | 32.5     | 1.5             | 2.24          | ...                  | LP  | T   | ...   | 1FHL J0832.0+0429<br>2FGL J0831.9+0429<br>1FGL J0831.6+0429                | ... | bll   | PKS 0829+046              |
| J0832.6+4914  | 128.167 | 49.249  | 170.105 | 36.426  | 0.124      | 0.113      | 1      | 4.2      | 0.2      | 0.1             | 2.7      | 0.7             | 2.36          | 0.17                 | PL  | ... | ...   | ...                                                                        | ... | bll   | OJ 448                    |
| J0832.8–4321  | 128.215 | –43.357 | 261.825 | –2.060  | 0.061      | 0.053      | 86     | 6.1      | 1.3      | 0.3             | 15.7     | 3.3             | 2.26          | 0.10                 | PL  | ... | 1     | ...                                                                        | ... | ...   | ...                       |
| J0833.1–4511e | 128.287 | –45.190 | 263.333 | –3.106  | ...        | ...        | ...    | ...      | 18.3     | ...             | 244.8    | ...             | 2.41          | ...                  | PL  | ... | 5     | 1FHL J0833.1–4511e<br>2FGL J0833.1–4511e<br>...                            | E   | PWN   | Vela X                    |
| J0834.1+4223  | 128.528 | 42.397  | 178.623 | 36.310  | 0.081      | 0.066      | –85    | 13.6     | 0.7      | 0.1             | 9.3      | 0.9             | 2.44          | 0.08                 | PL  | ... | ...   | 2FGL J0834.3+4221<br>1FGL J0834.4+4221                                     | ... | fsrq  | OJ 451                    |
| J0834.5–4825  | 128.634 | –48.422 | 266.081 | –4.835  | 0.143      | 0.118      | 57     | 4.7      | 0.7      | 0.1             | 9.2      | 2.4             | 2.44          | 0.14                 | PL  | ... | ...   | ...                                                                        | ... | ...   | ...                       |
| J0834.6+6101  | 128.674 | 61.022  | 155.517 | 35.920  | 0.140      | 0.115      | –89    | 4.3      | 0.2      | 0.1             | 2.9      | 0.7             | 2.42          | 0.14                 | PL  | ... | ...   | ...                                                                        | ... | ...   | ...                       |
| J0834.7+4403  | 128.689 | 44.060  | 176.574 | 36.566  | 0.080      | 0.074      | 48     | 6.1      | 0.3      | 0.1             | 3.3      | 0.7             | 2.22          | 0.16                 | PL  | ... | ...   | 2FGL J0834.3+4400                                                          | ... | bll   | B3 0831+442               |
| J0835.3–4510  | 128.838 | –45.178 | 263.555 | –2.787  | 0.005      | 0.005      | 20     | 1049.0   | 1297.7   | 2.9             | 8931.1   | 17.3            | 1.95          | ...                  | EC  | ... | ...   | 1FHL J0835.3–4510                                                          | P   | PSR   | PSR J0835–4510            |
| J0835.4+0930  | 128.865 | 9.510   | 216.170 | 27.400  | 0.145      | 0.095      | –0     | 5.0      | 0.3      | 0.1             | 3.6      | 0.8             | 2.29          | 0.18                 | PL  | ... | ...   | 1FGL J0835.4+0936                                                          | ... | bll   | GB6 J0835+0936            |
| J0836.3+2143  | 129.090 | 21.718  | 203.255 | 32.288  | 0.194      | 0.131      | 28     | 4.7      | 0.2      | 0.1             | 3.8      | 0.8             | 2.57          | 0.17                 | PL  | ... | ...   | ...                                                                        | ... | bcu   | MG2 J083615+2138          |
| J0836.5–2020  | 129.141 | –20.344 | 243.609 | 12.179  | 0.180      | 0.158      | –25    | 7.9      | 0.4      | 0.1             | 7.8      | 1.0             | 2.73          | 0.11                 | PL  | ... | ...   | ...                                                                        | ... | fsrq  | PKS 0834–20               |
| J0838.1–4615  | 129.546 | –46.263 | 264.720 | –3.045  | 0.290      | 0.147      | 70     | 8.7      | 3.5      | 0.4             | 32.7     | 6.7             | 2.58          | ...                  | LP  | T   | 1     | ...                                                                        | ... | spp   | ...                       |
| J0838.8–2829  | 129.704 | –28.489 | 250.605 | 7.801   | 0.056      | 0.053      | 64     | 13.7     | 1.1      | 0.1             | 12.7     | 1.2             | 2.23          | 0.07                 | PL  | ... | ...   | 2FGL J0838.8–2828<br>1FGL J0838.6–2828                                     | ... | ...   | ...                       |
| J0838.9–4056c | 129.745 | –40.938 | 260.573 | 0.301   | 0.198      | 0.144      | 73     | 4.5      | 0.9      | 0.2             | 16.7     | 3.3             | 2.66          | 0.12                 | PL  | ... | 4,6   | ...                                                                        | ... | ...   | ...                       |

Table 1—Continued

| Name 3FGL    | R.A.    | Decl.   | $l$     | $b$     | $\theta_1$ | $\theta_2$ | $\phi$ | $\sigma$ | $F_{35}$ | $\Delta F_{35}$ | $S_{25}$ | $\Delta S_{25}$ | $\Gamma_{25}$ | $\Delta \Gamma_{25}$ | Mod | Var | Flags  | $\gamma$ -ray Assoc.                                        | TeV | Class | ID or Assoc.              |
|--------------|---------|---------|---------|---------|------------|------------|--------|----------|----------|-----------------|----------|-----------------|---------------|----------------------|-----|-----|--------|-------------------------------------------------------------|-----|-------|---------------------------|
| J0839.1–4739 | 129.777 | –47.663 | 265.931 | –3.767  | 0.136      | 0.104      | 3      | 4.4      | 0.8      | 0.2             | 13.0     | 3.6             | 2.59          | 0.14                 | PL  | ... | ...    | ...                                                         | ... | spp   | ...                       |
| J0839.5+0102 | 129.890 | 1.038   | 225.041 | 24.372  | 0.088      | 0.077      | –10    | 8.9      | 0.5      | 0.1             | 6.4      | 0.9             | 2.24          | 0.10                 | PL  | T   | ...    | 2FGL J0839.6+0059<br>1FGL J0839.5+0059                      | ... | fsrq  | PKS 0837+012              |
| J0839.6+3538 | 129.912 | 35.639  | 187.124 | 36.488  | 0.083      | 0.062      | –74    | 8.4      | 0.4      | 0.1             | 5.0      | 0.9             | 1.92          | 0.12                 | PL  | ... | ...    | 2FGL J0839.7+3541                                           | ... | bll   | FIRST<br>J083943.3+354001 |
| J0839.6–4133 | 129.920 | –41.556 | 261.143 | 0.029   | 0.170      | 0.151      | –6     | 8.9      | 1.2      | 0.2             | 22.3     | 2.8             | 2.62          | ...                  | LP  | ... | 1,3,12 | ...                                                         | ... | ...   | ...                       |
| J0839.6+1803 | 129.923 | 18.059  | 207.625 | 31.758  | 0.071      | 0.069      | –15    | 6.3      | 0.3      | 0.1             | 3.4      | 0.8             | 1.90          | 0.17                 | PL  | ... | ...    | 2FGL J0839.4+1802                                           | ... | bll   | TXS 0836+182              |
| J0840.8+1315 | 130.210 | 13.253  | 212.925 | 30.168  | 0.123      | 0.113      | 31     | 9.2      | 0.5      | 0.1             | 7.4      | 0.9             | 2.47          | 0.09                 | PL  | T   | ...    | 2FGL J0840.7+1310<br>1FGL J0840.8+1310                      | ... | ssrq  | 3C 207                    |
| J0841.3–3554 | 130.335 | –35.905 | 256.865 | 3.737   | 0.029      | 0.026      | 41     | 18.8     | 1.6      | 0.2             | 20.2     | 2.0             | 1.76          | 0.06                 | PL  | T   | ...    | 1FHL J0841.2–3556<br>2FGL J0841.3–3556<br>1FGL J0841.4–3558 | ... | bcu   | NVSS<br>J084121–355506    |
| J0841.4+7053 | 130.373 | 70.897  | 143.536 | 34.432  | 0.047      | 0.045      | 65     | 34.5     | 1.3      | 0.1             | 36.4     | 1.1             | 2.84          | ...                  | LP  | T   | ...    | 2FGL J0841.6+7052<br>1FGL J0842.2+7054<br>3EG J0845+7049    | ... | FSRQ  | S5 0836+71<br>–47–6053    |
| J0842.0–6055 | 130.520 | –60.928 | 276.889 | –11.407 | 0.062      | 0.058      | 85     | 14.0     | 1.1      | 0.1             | 13.4     | 1.2             | 2.33          | 0.06                 | PL  | T   | ...    | ...                                                         | ... | bcu   | PMN J0842–6053            |
| J0843.1–4546 | 130.795 | –45.774 | 264.863 | –2.060  | 0.087      | 0.070      | –17    | 6.0      | 1.4      | 0.3             | 18.5     | 5.5             | 2.38          | 0.15                 | PL  | ... | 1      | ...                                                         | ... | spp   | ...                       |
| J0843.4+6713 | 130.859 | 67.218  | 147.799 | 35.606  | 0.061      | 0.049      | 32     | 13.2     | 0.6      | 0.1             | 7.2      | 0.8             | 1.99          | 0.08                 | PL  | ... | ...    | 2FGL J0843.6+6715<br>1FGL J0843.4+6718                      | ... | ...   | ...                       |
| J0843.9+5311 | 130.992 | 53.199  | 165.072 | 38.061  | 0.077      | 0.074      | –71    | 8.7      | 0.4      | 0.1             | 4.6      | 0.7             | 2.24          | 0.12                 | PL  | ... | ...    | 2FGL J0843.9+5312<br>1FGL J0844.0+5314                      | ... | bll   | NVSS<br>J084411+531250    |
| J0844.3–4741 | 131.082 | –47.684 | 266.488 | –3.086  | 0.162      | 0.093      | –45    | 5.3      | 0.9      | 0.2             | 13.2     | 2.8             | 2.46          | 0.12                 | PL  | ... | ...    | ...                                                         | ... | ...   | ...                       |
| J0845.1–5458 | 131.297 | –54.974 | 272.333 | –7.478  | 0.040      | 0.038      | 79     | 19.3     | 1.8      | 0.1             | 21.5     | 1.4             | 2.29          | 0.05                 | PL  | ... | ...    | 2FGL J0844.8–5459<br>1FGL J0845.0–5459                      | ... | bcu   | PMN J0845–5458            |
| J0846.7–0651 | 131.678 | –6.858  | 233.390 | 21.807  | 0.302      | 0.264      | 25     | 6.0      | 0.3      | 0.1             | 5.1      | 0.9             | 2.60          | 0.15                 | PL  | ... | 1      | 2FGL J0848.1–0703<br>...                                    | ... | bll   | TXS 0845–068              |
| J0846.8–2638 | 131.716 | –26.650 | 250.212 | 10.333  | 0.138      | 0.128      | 63     | 4.9      | 0.3      | 0.1             | 5.0      | 1.0             | 2.47          | 0.14                 | PL  | ... | ...    | ...                                                         | ... | ...   | ...                       |
| J0846.9–2336 | 131.750 | –23.604 | 247.762 | 12.206  | 0.042      | 0.040      | 85     | 15.6     | 1.2      | 0.1             | 13.4     | 1.3             | 2.03          | 0.07                 | PL  | ... | ...    | 1FHL J0846.8–2338<br>2FGL J0847.0–2334<br>1FGL J0846.9–2334 | ... | bll   | PMN J0847–2337            |
| J0847.1+1134 | 131.788 | 11.568  | 215.444 | 30.877  | 0.050      | 0.045      | 88     | 10.5     | 0.5      | 0.1             | 6.6      | 1.2             | 1.74          | 0.11                 | PL  | ... | ...    | 1FHL J0847.0+1132<br>2FGL J0847.2+1134<br>1FGL J0847.2+1134 | P   | bll   | RX J0847.1+1133           |
| J0847.2–6936 | 131.808 | –69.613 | 284.434 | –16.103 | 0.149      | 0.105      | –69    | 5.7      | 0.3      | 0.1             | 5.0      | 0.9             | 2.53          | 0.14                 | PL  | ... | 1,4    | ...                                                         | ... | ...   | ...                       |
| J0847.4–4327 | 131.863 | –43.459 | 263.525 | –0.023  | 0.183      | 0.109      | 64     | 12.2     | 2.6      | 0.3             | 28.9     | 3.4             | 2.56          | ...                  | LP  | ... | 3      | ...                                                         | ... | ...   | ...                       |
| J0848.2–4524 | 132.071 | –45.413 | 265.138 | –1.136  | 0.119      | 0.095      | –16    | 7.8      | 1.7      | 0.2             | 26.5     | 4.0             | 2.53          | 0.09                 | PL  | ... | 3      | ...                                                         | ... | ...   | ...                       |

Table 1—Continued

| Name 3FGL     | R.A.    | Decl.   | $l$     | $b$    | $\theta_1$ | $\theta_2$ | $\phi$ | $\sigma$ | $F_{35}$ | $\Delta F_{35}$ | $S_{25}$ | $\Delta S_{25}$ | $\Gamma_{25}$ | $\Delta \Gamma_{25}$ | Mod | Var | Flags | $\gamma$ -ray Assoc.                                                                                                 | TeV | Class | ID or Assoc.                |
|---------------|---------|---------|---------|--------|------------|------------|--------|----------|----------|-----------------|----------|-----------------|---------------|----------------------|-----|-----|-------|----------------------------------------------------------------------------------------------------------------------|-----|-------|-----------------------------|
| J0848.5+7018  | 132.131 | 70.301  | 144.014 | 35.169 | 0.088      | 0.072      | 65     | 6.3      | 0.3      | 0.1             | 3.1      | 0.7             | 2.01          | 0.19                 | PL  | ... | ...   | 3EG J0845+7049                                                                                                       | ... | ...   | ...                         |
| J0849.1+6607  | 132.297 | 66.127  | 148.917 | 36.441 | 0.055      | 0.052      | 59     | 10.8     | 0.5      | 0.1             | 6.1      | 0.8             | 2.02          | 0.10                 | PL  | ... | ...   | 2FGL J0849.2+6606<br>1FGL J0849.3+6607                                                                               | ... | bll   | GB6 J0848+6605              |
| J0849.3+0458  | 132.325 | 4.980   | 222.500 | 28.406 | 0.106      | 0.072      | -49    | 8.4      | 0.5      | 0.1             | 6.0      | 1.0             | 1.97          | 0.12                 | PL  | ... | ...   | 2FGL J0849.0+0455                                                                                                    | ... | bll   | TXS 0846+051                |
| J0849.5-2912  | 132.391 | -29.203 | 252.627 | 9.232  | 0.074      | 0.055      | -33    | 9.5      | 0.7      | 0.1             | 8.2      | 1.1             | 2.12          | 0.10                 | PL  | ... | ...   | 1FGL J0849.4-2912                                                                                                    | ... | bcu   | NVSS<br>J084922-291149      |
| J0849.9-3540  | 132.482 | -35.679 | 257.771 | 5.243  | 0.055      | 0.048      | -37    | 10.9     | 1.1      | 0.1             | 14.0     | 1.5             | 2.37          | 0.07                 | PL  | T   | ...   | 2FGL J0849.9-3540<br>1FGL J0849.6-3540                                                                               | ... | bcu   | PMN J0849-3541              |
| J0849.9+5108  | 132.482 | 51.145  | 167.603 | 39.129 | 0.038      | 0.036      | 67     | 32.4     | 1.9      | 0.1             | 22.4     | 1.1             | 2.28          | 0.04                 | PL  | T   | ...   | ...                                                                                                                  | ... | NLSY1 | SBS 0846+513                |
| J0850.0+4855  | 132.520 | 48.920  | 170.468 | 39.281 | 0.029      | 0.028      | -35    | 34.5     | 2.2      | 0.1             | 25.1     | 1.2             | 2.18          | 0.04                 | PL  | T   | 7     | 1FHL J0850.0+4849<br>2FGL J0849.8+4852<br>1FGL J0849.9+4852                                                          | ... | bll   | GB6 J0850+4855              |
| J0850.2-1214  | 132.557 | -12.234 | 238.676 | 19.529 | 0.030      | 0.027      | 81     | 40.4     | 3.5      | 0.2             | 32.8     | 1.6             | 2.21          | ...                  | LP  | T   | ...   | 1FHL J0850.2-1211<br>2FGL J0850.2-1212<br>1FGL J0850.0-1213<br>3EG J0852-1216<br>EGR J0852-1224                      | ... | fsrq  | PMN J0850-1213<br>48        |
| J0850.2+3500  | 132.566 | 35.001  | 188.356 | 38.523 | 0.090      | 0.082      | -35    | 5.3      | 0.2      | 0.1             | 2.8      | 0.7             | 1.92          | 0.20                 | PL  | ... | ...   | 1FGL J0850.2+3457                                                                                                    | ... | bll   | RX J0850.5+3455             |
| J0851.4-4244  | 132.865 | -42.748 | 263.437 | 0.993  | 0.129      | 0.087      | -47    | 9.9      | 1.6      | 0.3             | 27.0     | 3.4             | 2.61          | ...                  | LP  | ... | 3,5   | ...                                                                                                                  | ... | ...   | ...                         |
| J0851.8+5531  | 132.956 | 55.525  | 161.956 | 38.942 | 0.166      | 0.097      | 44     | 7.1      | 0.3      | 0.1             | 4.2      | 0.7             | 2.34          | 0.13                 | PL  | ... | ...   | ...                                                                                                                  | ... | bll   | SDSS<br>J085135.93+552834.5 |
| J0852.6-5756  | 133.171 | -57.946 | 275.334 | -8.516 | 0.050      | 0.049      | 16     | 15.0     | 1.3      | 0.1             | 16.7     | 1.3             | 2.40          | 0.06                 | PL  | T   | ...   | 2FGL J0852.4-5756                                                                                                    | ... | bcu   | PMN J0852-5755              |
| J0852.7-4631e | 133.200 | -46.520 | 266.491 | -1.233 | ...        | ...        | ...    | 30.3     | 13.0     | 0.5             | 147.1    | 5.9             | 1.94          | 0.03                 | PL  | T   | 10    | 1FGL J0854.0-4632<br>1FHL J0852.7-4631e<br>2FGL J0851.7-4635                                                         | E   | SNR   | Vela Jr                     |
| J0853.0-3654  | 133.273 | -36.913 | 259.135 | 4.955  | 0.052      | 0.043      | -17    | 9.8      | 0.9      | 0.1             | 10.4     | 1.4             | 2.06          | 0.09                 | PL  | ... | ...   | 1FHL J0852.9-3656<br>2FGL J0853.1-3659                                                                               | ... | bcu   | NVSS<br>J085310-365820      |
| J0854.2+4408  | 133.573 | 44.145  | 176.658 | 40.073 | 0.085      | 0.073      | 76     | 4.3      | 0.2      | 0.1             | 2.0      | 0.6             | 1.81          | 0.19                 | PL  | ... | ...   | ...                                                                                                                  | ... | bll   | B3 0850+443                 |
| J0854.4-4404  | 133.620 | -44.076 | 264.808 | 0.563  | 0.146      | 0.108      | -28    | 6.2      | 1.3      | 0.2             | 22.5     | 3.9             | 2.60          | 0.10                 | PL  | ... | 1,5   | ...                                                                                                                  | ... | ...   | ...                         |
| J0854.8+2006  | 133.700 | 20.112  | 206.807 | 35.819 | 0.020      | 0.019      | 51     | 56.5     | 5.9      | 0.2             | 58.0     | 2.2             | 2.18          | ...                  | LP  | T   | ...   | 1FHL J0854.8+2004<br>2FGL J0854.8+2005<br>1FGL J0854.8+2006<br>0FGL J0855.4+2009<br>3EG J0853+1941<br>EGR J0853+2015 | ... | BLL   | OJ 287                      |
| J0854.8-4503  | 133.711 | -45.062 | 265.603 | -0.023 | 0.049      | 0.045      | -53    | 18.2     | 4.5      | 0.3             | 30.7     | 3.0             | 2.28          | ...                  | LP  | ... | ...   | 2FGL J0854.7-4501<br>1FGL J0854.6-4504                                                                               | ... | ...   | ...                         |



Table 1—Continued

| Name 3FGL    | R.A.    | Decl.   | $l$     | $b$     | $\theta_1$ | $\theta_2$ | $\phi$ | $\sigma$ | $F_{35}$ | $\Delta F_{35}$ | $S_{25}$ | $\Delta S_{25}$ | $\Gamma_{25}$ | $\Delta \Gamma_{25}$ | Mod | Var | Flags | $\gamma$ -ray Assoc.                                                             | TeV | Class | ID or Assoc.             |
|--------------|---------|---------|---------|---------|------------|------------|--------|----------|----------|-----------------|----------|-----------------|---------------|----------------------|-----|-----|-------|----------------------------------------------------------------------------------|-----|-------|--------------------------|
| J0855.2–0718 | 133.809 | –7.308  | 235.055 | 23.327  | 0.205      | 0.174      | –34    | 5.6      | 0.3      | 0.1             | 4.7      | 0.9             | 2.57          | 0.15                 | PL  | ... | ...   | 2FGL J0855.1–0712                                                                | ... | bcu   | PKS 0852–07              |
| J0855.4–4818 | 133.855 | –48.316 | 268.153 | –2.049  | 0.099      | 0.087      | 27     | 10.9     | 1.9      | 0.3             | 25.2     | 3.2             | 2.52          | ...                  | LP  | ... | ...   | ...                                                                              | ... | ...   | ...                      |
| J0855.4+7142 | 133.861 | 71.712  | 142.156 | 35.226  | 0.103      | 0.094      | 31     | 9.3      | 0.4      | 0.1             | 6.9      | 0.9             | 2.57          | 0.11                 | PL  | T   | ...   | 2FGL J0856.0+7136                                                                | ... | ...   | ...                      |
| J0856.4+6429 | 134.110 | 64.485  | 150.637 | 37.618  | 0.154      | 0.129      | 78     | 4.7      | 0.2      | 0.1             | 3.2      | 0.7             | 2.55          | 0.17                 | PL  | ... | ...   | ...                                                                              | ... | ...   | ...                      |
| J0856.5+2057 | 134.150 | 20.958  | 205.989 | 36.495  | 0.075      | 0.068      | –44    | 8.3      | 0.6      | 0.1             | 6.9      | 1.1             | 2.19          | 0.13                 | PL  | ... | ...   | 2FGL J0856.3+2058                                                                | ... | bl    | TXS 0853+211             |
| J0856.7–1105 | 134.180 | –11.086 | 238.648 | 21.490  | 0.030      | 0.027      | –26    | 30.8     | 2.5      | 0.1             | 28.1     | 1.7             | 2.05          | 0.04                 | PL  | T   | ...   | 1FGL J0856.6+2103<br>1FHL J0856.7–1106<br>2FGL J0856.6–1105<br>1FGL J0856.6–1105 | ... | bl    | PMN J0856–1105           |
| J0857.6–4258 | 134.409 | –42.982 | 264.345 | 1.707   | 0.189      | 0.139      | 19     | 10.6     | 2.2      | 0.3             | 23.5     | 3.1             | 2.52          | ...                  | LP  | ... | ...   | 3EG J0859–4257                                                                   | ... | ...   | ...                      |
| J0858.0–4834 | 134.519 | –48.569 | 268.631 | –1.878  | 0.104      | 0.081      | 29     | 4.4      | 1.0      | 0.2             | 14.4     | 3.7             | 2.45          | 0.12                 | PL  | ... | ...   | ...                                                                              | ... | ...   | ...                      |
| J0858.1–1951 | 134.541 | –19.855 | 246.320 | 16.545  | 0.089      | 0.071      | 47     | 10.3     | 0.7      | 0.1             | 10.2     | 1.1             | 2.46          | 0.08                 | PL  | T   | ...   | 2FGL J0858.1–1952                                                                | ... | bcu   | PKS 0855–19              |
| J0858.1–3130 | 134.546 | –31.513 | 255.631 | 9.219   | 0.103      | 0.080      | 63     | 4.4      | 0.3      | 0.1             | 3.6      | 1.1             | 1.73          | 0.24                 | PL  | ... | ...   | 2FGL J0858.2–3129                                                                | ... | bcu   | 1RXS<br>J085802.6–313043 |
| J0858.6–4357 | 134.657 | –43.958 | 265.202 | 1.207   | 0.134      | 0.107      | –50    | 14.1     | 3.2      | 0.3             | 30.0     | 3.3             | 2.50          | ...                  | LP  | ... | ...   | ...                                                                              | ... | ...   | ...                      |
| J0859.1+6219 | 134.791 | 62.321  | 153.178 | 38.496  | 0.151      | 0.107      | 88     | 6.0      | 0.3      | 0.1             | 3.7      | 0.7             | 2.43          | 0.13                 | PL  | ... | ...   | ...                                                                              | ... | bl    | 1RXS<br>J085930.5+621737 |
| J0859.3–4732 | 134.847 | –47.549 | 268.003 | –1.045  | 0.124      | 0.089      | 57     | 5.9      | 1.4      | 0.2             | 18.8     | 3.8             | 2.42          | 0.10                 | PL  | ... | 5     | ...                                                                              | ... | ...   | ...                      |
| J0900.0+6754 | 135.022 | 67.914  | 146.393 | 36.917  | 0.331      | 0.240      | –63    | 4.4      | 0.2      | 0.1             | 2.9      | 0.7             | 2.24          | 0.16                 | PL  | ... | 9     | 2FGL J0900.9+6736                                                                | ... | ...   | ...                      |
| J0901.0–6725 | 135.262 | –67.426 | 283.439 | –13.767 | 0.249      | 0.187      | 83     | 4.2      | 0.3      | 0.1             | 3.9      | 0.9             | 2.52          | 0.17                 | PL  | ... | ...   | ...                                                                              | ... | ...   | ...                      |
| J0901.6–4700 | 135.405 | –47.001 | 267.840 | –0.399  | 0.131      | 0.115      | –24    | 9.6      | 2.5      | 0.3             | 20.4     | 3.7             | 2.44          | ...                  | LP  | ... | ...   | 2FGL J0901.7–4655                                                                | ... | ...   | ...                      |
| J0902.4+2050 | 135.622 | 20.847  | 206.678 | 37.761  | 0.038      | 0.037      | –55    | 18.3     | 1.2      | 0.1             | 13.7     | 1.2             | 2.10          | 0.07                 | PL  | T   | ...   | 2FGL J0902.4+2050                                                                | ... | bl    | NVSS<br>J090226+205045   |
| J0903.0–4826 | 135.763 | –48.450 | 269.084 | –1.179  | 0.163      | 0.123      | 30     | 4.5      | 1.2      | 0.2             | 16.5     | 3.6             | 2.47          | 0.10                 | PL  | ... | 5     | 1FGL J0902.4+2050<br>2FGL J0904.0–4823c                                          | ... | ...   | ...                      |
| J0903.1+4649 | 135.799 | 46.820  | 173.082 | 41.580  | 0.153      | 0.118      | –71    | 7.7      | 0.3      | 0.1             | 5.0      | 0.7             | 2.61          | 0.13                 | PL  | ... | ...   | 2FGL J0903.4+4651                                                                | ... | fsrq  | S4 0859+47               |
| J0903.2–4744 | 135.814 | –47.743 | 268.579 | –0.684  | 0.094      | 0.083      | –0     | 6.9      | 1.6      | 0.3             | 19.2     | 3.6             | 2.28          | 0.10                 | PL  | ... | 5     | 2FGL J0902.8–4741c                                                               | ... | ...   | ...                      |
| J0904.3+4240 | 136.088 | 42.682  | 178.620 | 41.886  | 0.106      | 0.094      | 60     | 7.9      | 0.4      | 0.1             | 5.3      | 0.8             | 2.48          | 0.13                 | PL  | ... | ...   | 2FGL J0903.6+4238                                                                | ... | bcu   | S4 0900+42               |
| J0904.8–5734 | 136.218 | –57.570 | 276.105 | –7.033  | 0.030      | 0.030      | –37    | 22.9     | 2.3      | 0.2             | 26.9     | 1.6             | 2.25          | 0.05                 | PL  | T   | ...   | 2FGL J0904.9–5735                                                                | ... | bcu   | PKS 0903–57              |
| J0904.8–3516 | 136.224 | –35.276 | 259.441 | 7.831   | 0.088      | 0.079      | 67     | 15.7     | 1.1      | 0.1             | 19.8     | 1.4             | 2.65          | 0.06                 | PL  | T   | ...   | 1FGL J0905.1–5736<br>2FGL J0904.8–3513                                           | ... | bcu   | NVSS<br>J090442–351423   |
| J0904.9+2739 | 136.227 | 27.661  | 198.452 | 40.184  | 0.194      | 0.154      | –72    | 4.6      | 0.2      | 0.1             | 3.6      | 0.8             | 2.69          | 0.18                 | PL  | ... | ...   | 1FGL J0904.7–3514<br>3EG J0903–3531                                              | ... | fsrq  | GB6 J0905+2748A          |
| J0905.5+1358 | 136.390 | 13.970  | 215.026 | 35.956  | 0.036      | 0.036      | –28    | 16.6     | 1.1      | 0.1             | 12.6     | 1.4             | 1.84          | 0.07                 | PL  | ... | ...   | 1FHL J0905.6+1359<br>2FGL J0905.6+1357<br>1FGL J0905.5+1356                      | ... | bl    | MG1 J090534+1358         |
| J0905.6–4917 | 136.420 | –49.296 | 270.003 | –1.422  | 0.215      | 0.156      | 5      | 10.0     | 2.2      | 0.3             | 22.3     | 2.5             | 2.49          | ...                  | LP  | ... | 1,12  | 2FGL J0908.5–4913                                                                | ... | ...   | ...                      |

Table 1—Continued

| Name 3FGL    | R.A.    | Decl.   | $l$     | $b$     | $\theta_1$ | $\theta_2$ | $\phi$ | $\sigma$ | $F_{35}$ | $\Delta F_{35}$ | $S_{25}$ | $\Delta S_{25}$ | $\Gamma_{25}$ | $\Delta \Gamma_{25}$ | Mod | Var | Flags     | $\gamma$ -ray Assoc.                                        | TeV | Class | ID or Assoc.                |
|--------------|---------|---------|---------|---------|------------|------------|--------|----------|----------|-----------------|----------|-----------------|---------------|----------------------|-----|-----|-----------|-------------------------------------------------------------|-----|-------|-----------------------------|
| J0905.8–2127 | 136.458 | −21.461 | 248.799 | 16.949  | 0.220      | 0.149      | −56    | 6.6      | 0.4      | 0.1             | 7.6      | 1.2             | 2.66          | 0.11                 | PL  | ... | ...       | ...                                                         | ... | ...   | ...                         |
| J0906.0–4705 | 136.506 | −47.098 | 268.412 | 0.096   | 0.085      | 0.080      | −45    | 8.5      | 1.7      | 0.3             | 18.8     | 3.1             | 2.47          | ...                  | LP  | ... | ...       | ...                                                         | ... | ...   | ...                         |
| J0906.3–0906 | 136.579 | −9.101  | 238.375 | 24.565  | 0.047      | 0.046      | −48    | 12.9     | 0.8      | 0.1             | 9.1      | 1.1             | 2.01          | 0.09                 | PL  | ... | ...       | 2FGL J0906.2–0906<br>1FGL J0906.4–0903                      | ... | bll   | PMN J0906–0905              |
| J0907.0–4802 | 136.754 | −48.043 | 269.223 | −0.416  | 0.133      | 0.091      | 26     | 7.9      | 2.2      | 0.3             | 15.9     | 2.8             | 2.42          | ...                  | LP  | ... | 1,3,4,5,9 | ...                                                         | ... | ...   | ...                         |
| J0908.4–4916 | 137.110 | −49.271 | 270.287 | −1.072  | 0.062      | 0.058      | 51     | 7.4      | 1.7      | 0.3             | 24.2     | 3.6             | 2.45          | 0.08                 | PL  | ... | 3,10      | 2FGL J0908.5–4913                                           | ... | PSR   | PSR J0908–4913              |
| J0909.0+2310 | 137.267 | 23.167  | 204.441 | 39.922  | 0.077      | 0.053      | −61    | 10.1     | 0.6      | 0.1             | 7.6      | 1.3             | 1.72          | 0.12                 | PL  | T   | ...       | 1FHL J0909.3+2312<br>2FGL J0909.2+2308<br>1FGL J0909.2+2310 | ... | bll   | RX J0908.9+2311             |
| J0909.1+0121 | 137.298 | 1.358   | 228.950 | 30.929  | 0.033      | 0.032      | −16    | 34.1     | 3.8      | 0.2             | 44.1     | 2.3             | 2.41          | ...                  | LP  | T   | ...       | 2FGL J0909.1+0121<br>1FGL J0909.0+0126                      | ... | fsrq  | PKS 0906+01                 |
| J0909.6+0157 | 137.417 | 1.962   | 228.418 | 31.343  | 0.073      | 0.070      | 68     | 9.6      | 0.9      | 0.1             | 14.1     | 2.0             | 2.54          | 0.10                 | PL  | ... | ...       | 2FGL J0909.6+0158<br>0FGL J0909.7+0145                      | ... | bll   | PKS 0907+022                |
| J0909.8–0229 | 137.458 | −2.500  | 232.819 | 29.011  | 0.051      | 0.047      | 58     | 26.4     | 1.8      | 0.1             | 17.4     | 1.1             | 2.32          | ...                  | LP  | T   | ...       | 2FGL J0909.7–0229<br>1FGL J0909.6–0229                      | ... | fsrq  | PKS 0907–023                |
| J0910.5+3329 | 137.647 | 33.490  | 191.120 | 42.460  | 0.032      | 0.029      | −89    | 17.4     | 1.2      | 0.1             | 13.8     | 1.4             | 1.98          | 0.08                 | PL  | T   | ...       | 1FHL J0910.6+3333<br>2FGL J0910.6+3329<br>1FGL J0910.7+3332 | ... | bll   | Ton 1015 <sup>2</sup><br>   |
| J0910.7+3858 | 137.689 | 38.971  | 183.691 | 42.998  | 0.084      | 0.075      | 40     | 4.6      | 0.2      | 0.1             | 2.1      | 0.6             | 1.88          | 0.21                 | PL  | ... | ...       | ...                                                         | ... | bll   | FBQS<br>J091052.0+390202    |
| J0910.9+2248 | 137.745 | 22.803  | 205.063 | 40.238  | 0.090      | 0.084      | −14    | 8.8      | 0.7      | 0.1             | 8.4      | 1.0             | 2.35          | 0.09                 | PL  | T   | ...       | 2FGL J0910.9+2246<br>1FGL J0911.0+2247                      | ... | fsrq  | TXS 0907+230                |
| J0911.8+3351 | 137.969 | 33.855  | 190.677 | 42.774  | 0.083      | 0.071      | 46     | 5.6      | 0.4      | 0.1             | 4.1      | 1.0             | 2.10          | 0.21                 | PL  | ... | ...       | ...                                                         | ... | bll   | MG2 J091151+3349            |
| J0912.2+4126 | 138.057 | 41.441  | 180.315 | 43.341  | 0.184      | 0.102      | −88    | 6.4      | 0.3      | 0.1             | 4.7      | 0.8             | 2.60          | 0.15                 | PL  | T   | 9         | 2FGL J0912.1+4126<br>1FGL J0912.3+4127                      | ... | fsrq  | B3 0908+416B                |
| J0912.2–6452 | 138.071 | −64.883 | 282.225 | −11.247 | 0.143      | 0.105      | 4      | 5.2      | 0.4      | 0.1             | 4.8      | 1.0             | 2.38          | 0.13                 | PL  | ... | 1         | ...                                                         | ... | glc   | NGC 2808                    |
| J0912.4+2800 | 138.108 | 28.004  | 198.502 | 41.882  | 0.084      | 0.071      | 84     | 5.6      | 0.2      | 0.1             | 3.3      | 1.0             | 1.54          | 0.20                 | PL  | ... | ...       | 1FHL J0912.5+2758<br>2FGL J0912.5+2758<br>1FGL J0912.6+2756 | ... | bll   | 1RXS<br>J091211.9+275955    |
| J0912.6–2757 | 138.167 | −27.958 | 254.976 | 13.921  | 0.190      | 0.130      | −59    | 6.1      | 0.3      | 0.1             | 6.5      | 1.0             | 2.70          | 0.16                 | PL  | ... | ...       | ...                                                         | ... | bcu   | PMN J0912–2752              |
| J0912.7+1556 | 138.196 | 15.934  | 213.609 | 38.327  | 0.087      | 0.071      | 39     | 5.4      | 0.2      | 0.1             | 3.4      | 1.1             | 1.35          | 0.23                 | PL  | ... | ...       | 2FGL J0913.0+1553                                           | ... | bll   | SDSS<br>J091230.61+155528.0 |
| J0912.9–2104 | 138.248 | −21.077 | 249.606 | 18.478  | 0.039      | 0.034      | 79     | 14.4     | 1.0      | 0.1             | 11.6     | 1.3             | 1.94          | 0.09                 | PL  | ... | ...       | 1FHL J0913.1–2104<br>2FGL J0912.9–2102                      | ... | bll   | MRC 0910–208                |
| J0914.5–4736 | 138.641 | −47.615 | 269.776 | 0.801   | 0.123      | 0.101      | 68     | 15.6     | 2.5      | 0.3             | 31.3     | 2.8             | 2.51          | ...                  | LP  | ... | 3         | ...                                                         | ... | ...   | ...                         |
| J0915.0+5844 | 138.770 | 58.740  | 156.979 | 41.351  | 0.250      | 0.156      | 28     | 4.2      | 0.2      | 0.0             | 2.6      | 0.6             | 2.48          | 0.18                 | PL  | ... | ...       | ...                                                         | ... | bcu   | SDSS<br>J091608.57+584434.0 |
| J0915.8–5110 | 138.964 | −51.180 | 272.491 | −1.519  | 0.758      | 0.321      | 23     | 10.1     | 0.5      | 0.1             | 21.7     | 2.3             | 2.69          | ...                  | LP  | ... | 1,3,9,12  | ...                                                         | ... | ...   | ...                         |

Table 1—Continued

| Name 3FGL    | R.A.    | Decl.   | $l$     | $b$    | $\theta_1$ | $\theta_2$ | $\phi$ | $\sigma$ | $F_{35}$ | $\Delta F_{35}$ | $S_{25}$ | $\Delta S_{25}$ | $\Gamma_{25}$ | $\Delta \Gamma_{25}$ | Mod | Var | Flags | $\gamma$ -ray Assoc.                                                             | TeV | Class | ID or Assoc.             |
|--------------|---------|---------|---------|--------|------------|------------|--------|----------|----------|-----------------|----------|-----------------|---------------|----------------------|-----|-----|-------|----------------------------------------------------------------------------------|-----|-------|--------------------------|
| J0915.8+2933 | 138.965 | 29.560  | 196.644 | 42.933 | 0.026      | 0.025      | −62    | 30.0     | 2.0      | 0.1             | 23.5     | 1.7             | 1.88          | 0.04                 | PL  | ... | ...   | 1FHL J0915.8+2932<br>2FGL J0915.8+2932<br>1FGL J0915.7+2931                      | ... | bll   | Ton 0396                 |
| J0916.3+3857 | 139.090 | 38.962  | 183.765 | 44.086 | 0.120      | 0.109      | −84    | 5.0      | 0.3      | 0.1             | 3.3      | 0.7             | 2.36          | 0.16                 | PL  | ... | ...   | 2FGL J0917.0+3900                                                                | ... | fsrq  | S4 0913+39               |
| J0917.3−0344 | 139.347 | −3.737  | 235.204 | 29.894 | 0.105      | 0.080      | −25    | 5.5      | 0.3      | 0.1             | 3.5      | 0.9             | 1.76          | 0.21                 | PL  | ... | ...   | ...                                                                              | ... | bcu   | NVSS<br>J091714−034315   |
| J0918.2−4859 | 139.573 | −48.989 | 271.194 | 0.290  | 0.952      | 0.217      | 36     | 4.1      | 0.8      | 0.2             | 11.6     | 2.7             | 2.44          | 0.13                 | PL  | ... | 3,4,9 | ...                                                                              | ... | ...   | ...                      |
| J0919.4+6604 | 139.871 | 66.075  | 147.690 | 39.351 | 0.131      | 0.106      | −13    | 4.5      | 0.2      | 0.1             | 2.7      | 0.7             | 2.16          | 0.16                 | PL  | ... | ...   | ...                                                                              | ... | ...   | ...                      |
| J0919.5−2200 | 139.883 | −22.005 | 251.396 | 19.027 | 0.207      | 0.102      | 61     | 4.2      | 0.3      | 0.1             | 3.3      | 0.9             | 2.20          | 0.26                 | PL  | ... | ...   | 2FGL J0919.3−2203                                                                | ... | ...   | ...                      |
| J0920.9+4442 | 140.230 | 44.705  | 175.693 | 44.806 | 0.022      | 0.021      | 79     | 82.1     | 5.8      | 0.2             | 61.5     | 1.5             | 2.29          | ...                  | LP  | T   | ...   | 1FHL J0920.9+4443<br>2FGL J0920.9+4441<br>1FGL J0920.9+4441<br>0FGL J0921.2+4437 | ... | fsrq  | S4 0917+44               |
| J0921.0−2258 | 140.252 | −22.967 | 252.396 | 18.645 | 0.095      | 0.085      | 15     | 4.1      | 0.1      | 0.1             | 2.3      | 0.8             | 1.55          | 0.26                 | PL  | ... | ...   | ...                                                                              | ... | bcu   | NVSS<br>J092057−225721   |
| J0921.6+2339 | 140.416 | 23.656  | 204.897 | 42.833 | 0.045      | 0.043      | −71    | 9.7      | 0.5      | 0.1             | 6.0      | 0.9             | 1.98          | 0.11                 | PL  | ... | ...   | 2FGL J0921.9+2335<br>1FGL J0922.0+2337                                           | ... | ...   | ...                      |
| J0921.8+6215 | 140.453 | 62.266  | 152.187 | 41.016 | 0.046      | 0.044      | −55    | 25.8     | 1.1      | 0.1             | 15.9     | 0.8             | 2.45          | 0.05                 | PL  | T   | ...   | 1FGL J0919.6+6216<br>2FGL J0921.9+6216                                           | ... | fsrq  | OK 630                   |
| J0922.4−0529 | 140.602 | −5.497  | 237.695 | 29.907 | 0.079      | 0.069      | 51     | 9.6      | 0.6      | 0.1             | 7.0      | 0.9             | 2.17          | 0.10                 | PL  | ... | ...   | ...                                                                              | ... | fsrq  | TXS 0919−052             |
| J0922.8−3959 | 140.715 | −39.990 | 265.362 | 7.204  | 0.182      | 0.150      | −71    | 6.3      | 0.4      | 0.1             | 8.0      | 1.2             | 2.70          | 0.13                 | PL  | ... | 4     | ...                                                                              | ... | bcu   | PKS 0920−39              |
| J0923.1+3853 | 140.790 | 38.897  | 183.902 | 45.407 | 0.182      | 0.145      | −72    | 7.9      | 0.3      | 0.1             | 6.2      | 0.8             | 2.75          | 0.12                 | PL  | T   | ...   | ...                                                                              | ... | bcu   | B2 0920+39               |
| J0923.3+4127 | 140.846 | 41.463  | 180.245 | 45.432 | 0.085      | 0.065      | −43    | 14.6     | 0.8      | 0.1             | 9.4      | 0.9             | 2.25          | 0.07                 | PL  | T   | ...   | 2FGL J0923.2+4125<br>1FGL J0923.2+4121                                           | ... | fsrq  | B3 0920+416              |
| J0923.8−5154 | 140.965 | −51.904 | 273.882 | −1.145 | 0.133      | 0.116      | 60     | 6.9      | 1.0      | 0.2             | 16.9     | 2.3             | 2.63          | 0.09                 | PL  | ... | 1,4   | ...                                                                              | ... | ...   | ...                      |
| J0924.0+2816 | 141.002 | 28.282  | 198.855 | 44.436 | 0.102      | 0.088      | −24    | 9.3      | 0.4      | 0.1             | 6.4      | 0.8             | 2.63          | 0.11                 | PL  | T   | ...   | 2FGL J0924.0+2819<br>1FGL J0924.2+2812                                           | ... | fsrq  | B2 0920+28               |
| J0924.2+0534 | 141.064 | 5.577   | 226.876 | 36.309 | 0.082      | 0.077      | −26    | 7.5      | 0.4      | 0.1             | 5.8      | 0.9             | 2.43          | 0.12                 | PL  | ... | 3     | ...                                                                              | ... | bll   | RBS 0771                 |
| J0925.6+5959 | 141.404 | 59.994  | 154.823 | 42.238 | 0.084      | 0.073      | 73     | 6.0      | 0.2      | 0.1             | 2.7      | 0.7             | 1.65          | 0.17                 | PL  | ... | ...   | ...                                                                              | ... | bll   | NVSS<br>J092542+595812   |
| J0925.7+3129 | 141.426 | 31.493  | 194.476 | 45.343 | 0.109      | 0.090      | 15     | 4.2      | 0.2      | 0.1             | 2.1      | 0.6             | 2.00          | 0.22                 | PL  | ... | ...   | ...                                                                              | ... | bll   | B2 0922+31B              |
| J0926.3+5409 | 141.580 | 54.156  | 162.423 | 44.077 | 0.108      | 0.097      | −67    | 5.3      | 0.2      | 0.1             | 2.6      | 0.6             | 2.07          | 0.19                 | PL  | ... | ...   | ...                                                                              | ... | bll   | NVSS<br>J092638+541126   |
| J0927.9−2037 | 141.998 | −20.620 | 251.691 | 21.420 | 0.110      | 0.092      | −45    | 9.5      | 0.6      | 0.1             | 7.4      | 0.9             | 2.38          | 0.09                 | PL  | T   | ...   | 2FGL J0927.9−2041                                                                | ... | fsrq  | PKS 0925−203             |
| J0928.3−5255 | 142.085 | −52.923 | 275.081 | −1.404 | 0.076      | 0.075      | −59    | 4.2      | 0.3      | 0.2             | 4.6      | 1.5             | 1.65          | 0.26                 | PL  | ... | ...   | 1FHL J0928.1−5252                                                                | ... | ...   | ...                      |
| J0928.5+4048 | 142.133 | 40.816  | 181.131 | 46.421 | 0.070      | 0.069      | 55     | 5.7      | 0.2      | 0.1             | 2.7      | 0.7             | 1.84          | 0.18                 | PL  | ... | ...   | ...                                                                              | ... | bll   | 1RXS<br>J092837.8+404858 |
| J0928.7+7300 | 142.189 | 73.014  | 139.353 | 36.933 | 0.161      | 0.135      | 4      | 4.8      | 0.1      | 0.0             | 3.2      | 0.7             | 2.92          | 0.27                 | PL  | ... | ...   | ...                                                                              | ... | bcu   | GB6 J0929+7304           |
| J0928.9−3530 | 142.246 | −35.511 | 263.035 | 11.235 | 0.058      | 0.051      | −72    | 10.0     | 0.6      | 0.1             | 9.8      | 1.1             | 2.53          | 0.09                 | PL  | ... | ...   | 2FGL J0928.8−3530                                                                | ... | bcu   | NVSS<br>J092849−352947   |
|              |         |         |         |        |            |            |        |          |          |                 |          |                 |               |                      |     |     |       | 1FGL J0929.0−3531                                                                |     |       |                          |

Table 1—Continued

| Name 3FGL     | R.A.    | Decl.   | $l$     | $b$     | $\theta_1$ | $\theta_2$ | $\phi$ | $\sigma$ | $F_{35}$ | $\Delta F_{35}$ | $S_{25}$ | $\Delta S_{25}$ | $\Gamma_{25}$ | $\Delta \Gamma_{25}$ | Mod | Var | Flags | $\gamma$ -ray Assoc.                   | TeV | Class | ID or Assoc.            |
|---------------|---------|---------|---------|---------|------------|------------|--------|----------|----------|-----------------|----------|-----------------|---------------|----------------------|-----|-----|-------|----------------------------------------|-----|-------|-------------------------|
| J0929.4+5013  | 142.354 | 50.225  | 167.657 | 45.446  | 0.048      | 0.044      | -52    | 14.0     | 1.0      | 0.1             | 11.6     | 1.0             | 2.16          | 0.07                 | PL  | T   | ...   | 1FHL J0929.5+5014<br>2FGL J0929.5+5009 | ... | bl    | GB6 J0929+5013          |
| J0930.0+4951  | 142.522 | 49.853  | 168.145 | 45.627  | 0.148      | 0.098      | -57    | 5.1      | 0.2      | 0.1             | 3.4      | 1.0             | 1.45          | 0.21                 | PL  | ... | ...   | 1FGL J0929.4+5000                      | ... | bl    | 1ES 0927+500            |
| J0930.2+8612  | 142.562 | 86.202  | 126.290 | 29.514  | 0.038      | 0.035      | 80     | 21.1     | 1.3      | 0.1             | 14.5     | 1.0             | 2.18          | 0.05                 | PL  | T   | ...   | 1FHL J0930.4+8611<br>2FGL J0930.4+8611 | ... | bl    | S5 0916+864             |
| J0930.7+5133  | 142.688 | 51.559  | 165.737 | 45.360  | 0.102      | 0.086      | 78     | 4.7      | 0.2      | 0.1             | 2.3      | 0.6             | 2.07          | 0.21                 | PL  | ... | ...   | ...                                    | ... | ...   | ...                     |
| J0930.9-1904  | 142.732 | -19.074 | 250.953 | 22.968  | 0.135      | 0.109      | 83     | 4.4      | 0.3      | 0.1             | 3.0      | 0.9             | 1.85          | 0.16                 | PL  | ... | ...   | ...                                    | ... | PSR   | PSR J0931-1902          |
| J0931.8+6739  | 142.968 | 67.651  | 145.166 | 39.773  | 0.082      | 0.067      | -30    | 6.9      | 0.3      | 0.1             | 3.6      | 0.6             | 2.17          | 0.13                 | PL  | ... | ...   | ...                                    | ... | ...   | ...                     |
| J0933.9-6232  | 143.481 | -62.534 | 282.235 | -7.894  | 0.041      | 0.037      | -9     | 22.1     | 2.7      | 0.2             | 12.3     | 1.1             | 2.02          | ...                  | LP  | ... | ...   | 2FGL J0934.0-6231<br>1FGL J0933.9-6228 | ... | ...   | ...                     |
| J0934.1+3933  | 143.549 | 39.564  | 182.918 | 47.540  | 0.170      | 0.162      | -2     | 6.8      | 0.4      | 0.1             | 4.4      | 0.7             | 2.28          | 0.12                 | PL  | ... | ...   | 2FGL J0934.7+3932<br>1FGL J0934.5+3929 | ... | bl    | GB6 J0934+3926          |
| J0935.1-1736  | 143.787 | -17.606 | 250.499 | 24.696  | 0.056      | 0.054      | 79     | 6.8      | 0.3      | 0.1             | 4.4      | 1.1             | 1.75          | 0.16                 | PL  | ... | ...   | ...                                    | ... | ...   | ...                     |
| J0935.2+0903  | 143.801 | 9.052   | 224.675 | 40.367  | 0.148      | 0.117      | 3      | 7.3      | 0.4      | 0.1             | 5.8      | 0.9             | 2.40          | 0.11                 | PL  | ... | ...   | ...                                    | ... | ...   | ...                     |
| J0936.3-2114  | 144.100 | -21.245 | 253.625 | 22.433  | 0.077      | 0.065      | -78    | 5.7      | 0.3      | 0.1             | 3.5      | 0.9             | 1.84          | 0.18                 | PL  | ... | ...   | ...                                    | ... | ...   | ...                     |
| J0937.1-4544c | 144.292 | -45.744 | 271.258 | 4.842   | 0.181      | 0.128      | -44    | 4.6      | 0.5      | 0.1             | 6.9      | 1.5             | 2.49          | 0.16                 | PL  | ... | 4,6   | ...                                    | ... | ...   | ...                     |
| J0937.7+5008  | 144.446 | 50.145  | 167.344 | 46.770  | 0.116      | 0.094      | -60    | 7.3      | 0.3      | 0.1             | 4.4      | 0.7             | 2.38          | 0.14                 | PL  | T   | ...   | 2FGL J0937.6+5009<br>1FGL J0937.7+5005 | ... | fsrq  | GB6 J0937+5008          |
| J0937.8-6407  | 144.475 | -64.122 | 283.654 | -8.759  | 0.142      | 0.121      | 45     | 5.5      | 0.4      | 0.1             | 6.1      | 1.1             | 2.55          | 0.12                 | PL  | ... | 1     | ...                                    | ... | ...   | ...                     |
| J0937.9-1435  | 144.483 | -14.598 | 248.507 | 27.204  | 0.068      | 0.063      | -24    | 6.0      | 0.3      | 0.1             | 3.8      | 0.9             | 1.89          | 0.15                 | PL  | ... | ...   | 2FGL J0937.9-1434                      | ... | ...   | ...                     |
| J0939.2-1732  | 144.814 | -17.537 | 251.174 | 25.464  | 0.097      | 0.080      | 48     | 8.9      | 0.6      | 0.1             | 7.5      | 1.0             | 2.27          | 0.09                 | PL  | T   | ...   | 2FGL J0939.1-1734                      | ... | bcu   | TXS 0936-173            |
| J0939.9-2831  | 144.979 | -28.520 | 259.716 | 17.864  | 0.115      | 0.081      | 70     | 10.0     | 0.6      | 0.1             | 8.8      | 1.0             | 2.47          | 0.09                 | PL  | T   | ...   | 2FGL J0940.3-2827                      | ... | bcu   | TXS 0937-282            |
| J0940.6-7609  | 145.164 | -76.161 | 292.247 | -17.425 | 0.097      | 0.084      | 14     | 10.1     | 0.8      | 0.1             | 10.8     | 1.2             | 2.39          | 0.08                 | PL  | ... | ...   | 2FGL J0942.8-7558<br>1FGL J0940.2-7605 | ... | ...   | ...                     |
| J0940.7-6102  | 145.188 | -61.047 | 281.830 | -6.250  | 0.207      | 0.121      | 52     | 6.4      | 0.6      | 0.1             | 8.3      | 1.3             | 2.42          | 0.10                 | PL  | ... | 3     | 2FGL J0940.8-6105                      | ... | bcu   | MRC 0939-608            |
| J0940.9-1337  | 145.243 | -13.618 | 248.232 | 28.405  | 0.104      | 0.079      | -16    | 10.1     | 0.6      | 0.1             | 8.4      | 0.9             | 2.41          | 0.09                 | PL  | T   | ...   | ...                                    | ... | fsrq  | TXS 0938-133            |
| J0941.0+6151  | 145.275 | 61.866  | 151.483 | 43.249  | 0.078      | 0.076      | -87    | 9.0      | 0.4      | 0.1             | 4.8      | 0.7             | 2.30          | 0.13                 | PL  | ... | ...   | 2FGL J0941.4+6148<br>1FGL J0941.2+6149 | ... | ...   | ...                     |
| J0941.6+2727  | 145.423 | 27.451  | 201.130 | 48.109  | 0.138      | 0.111      | 65     | 6.8      | 0.3      | 0.1             | 4.5      | 0.7             | 2.50          | 0.13                 | PL  | ... | ...   | 2FGL J0941.4+2724<br>1FGL J0941.2+2722 | ... | fsrq  | MG2 J094148+2728        |
| J0942.1-0756  | 145.541 | -7.943  | 243.448 | 32.313  | 0.109      | 0.081      | -75    | 6.1      | 0.4      | 0.1             | 3.9      | 0.8             | 2.07          | 0.13                 | PL  | T   | ...   | 2FGL J0941.9-0755                      | ... | bl    | PMN J0942-0800          |
| J0945.9+5756  | 146.483 | 57.943  | 156.125 | 45.427  | 0.082      | 0.067      | 65     | 13.2     | 0.6      | 0.1             | 7.2      | 0.7             | 2.33          | 0.08                 | PL  | ... | ...   | 2FGL J0945.9+5751<br>1FGL J0945.6+5754 | ... | bl    | GB6 J0945+5757          |
| J0946.2+0103  | 146.573 | 1.065   | 235.376 | 38.565  | 0.073      | 0.063      | 37     | 4.9      | 0.2      | 0.1             | 2.9      | 0.9             | 1.70          | 0.23                 | PL  | ... | ...   | 1FHL J0946.2+0106<br>2FGL J0946.2+0104 | ... | bl    | RXS<br>J094620.5+010459 |

Table 1—Continued

| Name 3FGL     | R.A.    | Decl.   | $l$     | $b$     | $\theta_1$ | $\theta_2$ | $\phi$ | $\sigma$ | $F_{35}$ | $\Delta F_{35}$ | $S_{25}$ | $\Delta S_{25}$ | $\Gamma_{25}$ | $\Delta \Gamma_{25}$ | Mod | Var | Flags | $\gamma$ -ray Assoc.                                                                               | TeV | Class | ID or Assoc.                  |
|---------------|---------|---------|---------|---------|------------|------------|--------|----------|----------|-----------------|----------|-----------------|---------------|----------------------|-----|-----|-------|----------------------------------------------------------------------------------------------------|-----|-------|-------------------------------|
| J0946.2+5209  | 146.574 | 52.151  | 163.976 | 47.514  | 0.238      | 0.206      | 50     | 6.7      | 0.2      | 0.1             | 4.2      | 0.6             | 2.74          | 0.14                 | PL  | ... | ...   | ...                                                                                                | ... | ...   | ...                           |
| J0946.5+1017  | 146.636 | 10.288  | 224.967 | 43.415  | 0.054      | 0.051      | -19    | 23.3     | 1.4      | 0.1             | 19.2     | 1.1             | 2.46          | 0.05                 | PL  | T   | ...   | 2FGL J0946.5+1015<br>1FGL J0946.6+1012                                                             | ... | fsrq  | TXS 0943+105                  |
| J0947.1-2542  | 146.789 | -25.709 | 258.896 | 21.010  | 0.069      | 0.064      | -6     | 10.4     | 0.7      | 0.1             | 7.9      | 1.1             | 1.95          | 0.10                 | PL  | ... | ...   | 2FGL J0946.9-2541                                                                                  | ... | bcu   | 1RXS<br>J094709.2-254056      |
| J0948.1-3641  | 147.036 | -36.693 | 266.762 | 12.994  | 0.255      | 0.135      | 16     | 9.4      | 0.5      | 0.1             | 10.2     | 1.1             | 2.72          | 0.09                 | PL  | ... | ...   | ...                                                                                                | ... | ...   | ...                           |
| J0948.6+4041  | 147.170 | 40.696  | 180.947 | 50.236  | 0.195      | 0.126      | -73    | 8.6      | 0.3      | 0.1             | 5.6      | 0.7             | 2.67          | 0.11                 | PL  | ... | ...   | 2FGL J0948.8+4040                                                                                  | ... | fsrq  | 4C +40.24                     |
| J0948.8-4243  | 147.204 | -42.721 | 270.845 | 8.492   | 0.103      | 0.089      | 53     | 6.2      | 0.5      | 0.1             | 7.1      | 1.2             | 2.49          | 0.12                 | PL  | ... | 1     | ...                                                                                                | ... | ...   | ...                           |
| J0948.8+0021  | 147.223 | 0.363   | 236.590 | 38.694  | 0.042      | 0.041      | 16     | 39.4     | 2.7      | 0.2             | 49.4     | 1.3             | 2.63          | ...                  | LP  | T   | ...   | 2FGL J0948.8+0020<br>1FGL J0949.0+0021<br>0FGL J0948.3+0019                                        | ... | NLSY1 | PMN J0948+0022                |
| J0950.1+4554  | 147.535 | 45.903  | 172.874 | 49.721  | 0.053      | 0.045      | -32    | 10.4     | 0.5      | 0.1             | 5.2      | 0.8             | 1.95          | 0.13                 | PL  | ... | ...   | 2FGL J0950.1+4554                                                                                  | ... | bll   | RX J0950.2+4553               |
| J0950.4+7550  | 147.610 | 75.850  | 135.411 | 36.536  | 0.162      | 0.141      | 90     | 4.3      | 0.2      | 0.0             | 2.2      | 0.5             | 2.20          | 0.19                 | PL  | ... | ...   | ...                                                                                                | ... | ...   | ...                           |
| J0952.8+0711  | 148.217 | 7.199   | 229.723 | 43.266  | 0.076      | 0.057      | 47     | 5.8      | 0.2      | 0.1             | 3.3      | 0.9             | 1.70          | 0.17                 | PL  | ... | ...   | ...                                                                                                | ... | ...   | ...                           |
| J0953.0-0839  | 148.255 | -8.663  | 246.175 | 33.899  | 0.026      | 0.025      | -42    | 29.8     | 2.3      | 0.1             | 28.5     | 2.2             | 1.81          | 0.04                 | PL  | T   | ...   | 1FHL J0952.9-0839<br>2FGL J0953.1-0839<br>1FGL J0953.0-0838                                        | ... | bll   | PMN J0953-0840<br>53          |
| J0953.1-7657c | 148.293 | -76.963 | 293.377 | -17.530 | 0.058      | 0.056      | -24    | 6.9      | 0.5      | 0.1             | 5.4      | 1.1             | 1.91          | 0.15                 | PL  | ... | 6     | 2FGL J0953.9-7659                                                                                  | ... | bcu   | 1RXS<br>J095306.1-765755<br>1 |
| J0953.7-1510  | 148.429 | -15.175 | 251.938 | 29.605  | 0.070      | 0.064      | -56    | 14.0     | 1.2      | 0.1             | 5.9      | 0.7             | 2.10          | ...                  | LP  | ... | ...   | 2FGL J0953.6-1504<br>1FGL J0953.6-1505                                                             | ... | ...   | ...                           |
| J0954.2+4913  | 148.555 | 49.220  | 167.646 | 49.578  | 0.054      | 0.046      | 32     | 6.5      | 0.1      | 0.0             | 2.6      | 0.8             | 1.33          | 0.23                 | PL  | ... | ...   | ...                                                                                                | ... | bll   | 1ES 0950+495                  |
| J0954.8-3948  | 148.712 | -39.809 | 269.844 | 11.458  | 0.088      | 0.067      | -1     | 18.9     | 1.3      | 0.1             | 18.3     | 1.2             | 2.54          | ...                  | LP  | ... | ...   | 2FGL J0955.0-3949<br>1FGL J0955.2-3949                                                             | ... | ...   | ...                           |
| J0955.4+6940  | 148.870 | 69.673  | 141.443 | 40.543  | 0.043      | 0.038      | -78    | 17.8     | 0.9      | 0.1             | 10.7     | 0.8             | 2.21          | 0.06                 | PL  | ... | ...   | 2FGL J0955.9+6936<br>1FGL J0956.5+6938                                                             | P   | sbq   | M 82                          |
| J0955.6-6148  | 148.913 | -61.814 | 283.699 | -5.696  | 0.106      | 0.067      | 3      | 7.0      | 0.7      | 0.1             | 8.2      | 1.3             | 2.33          | 0.10                 | PL  | ... | ...   | ...                                                                                                | ... | psr   | PSR J0955-61                  |
| J0956.6+2515  | 149.154 | 25.266  | 205.477 | 50.937  | 0.078      | 0.074      | 3      | 15.9     | 0.9      | 0.1             | 12.2     | 0.9             | 2.44          | 0.06                 | PL  | T   | 7     | 2FGL J0956.9+2516<br>1FGL J0956.9+2513                                                             | ... | fsrq  | OK 290                        |
| J0956.7-6441  | 149.185 | -64.693 | 285.595 | -7.877  | 0.093      | 0.082      | 30     | 6.3      | 0.4      | 0.1             | 6.9      | 1.2             | 2.54          | 0.13                 | PL  | ... | 1     | ...                                                                                                | ... | bcu   | AT20G<br>J095612-643928       |
| J0957.4+4728  | 149.369 | 47.472  | 170.034 | 50.578  | 0.193      | 0.158      | 49     | 7.7      | 0.3      | 0.1             | 4.8      | 0.7             | 2.67          | 0.12                 | PL  | ... | ...   | 2FGL J0957.7+4735                                                                                  | ... | fsrq  | OK 492                        |
| J0957.5-1351  | 149.383 | -13.863 | 251.596 | 31.182  | 0.096      | 0.087      | -84    | 13.2     | 0.8      | 0.1             | 9.6      | 1.0             | 2.52          | ...                  | LP  | T   | ...   | 2FGL J0957.6-1350                                                                                  | ... | fsrq  | PMN J0957-1350                |
| J0957.6+5523  | 149.413 | 55.387  | 158.592 | 47.929  | 0.012      | 0.012      | -24    | 112.9    | 10.4     | 0.2             | 95.9     | 2.7             | 2.00          | ...                  | LP  | ... | ...   | 1FHL J0957.6+5522<br>2FGL J0957.7+5522<br>1FGL J0957.7+5523<br>0FGL J0957.6+5522<br>EGR J0957+5513 | ... | fsrq  | 4C +55.17                     |

Table 1—Continued

| Name 3FGL     | R.A.    | Decl.   | $l$     | $b$     | $\theta_1$ | $\theta_2$ | $\phi$ | $\sigma$ | $F_{35}$ | $\Delta F_{35}$ | $S_{25}$ | $\Delta S_{25}$ | $\Gamma_{25}$ | $\Delta \Gamma_{25}$ | Mod | Var | Flags | $\gamma$ -ray Assoc.                                                                            | TeV | Class | ID or Assoc.             |
|---------------|---------|---------|---------|---------|------------|------------|--------|----------|----------|-----------------|----------|-----------------|---------------|----------------------|-----|-----|-------|-------------------------------------------------------------------------------------------------|-----|-------|--------------------------|
| J0958.3–0318  | 149.585 | −3.303  | 242.148 | 38.362  | 0.151      | 0.095      | 64     | 4.9      | 0.2      | 0.1             | 3.2      | 1.0             | 1.52          | 0.21                 | PL  | ... | ...   | ...                                                                                             | ... | bll   | 1RXS<br>J095806.4−031729 |
| J0958.4−6752  | 149.600 | −67.874 | 287.725 | −10.270 | 0.045      | 0.041      | 66     | 6.9      | 0.5      | 0.1             | 5.2      | 1.0             | 2.21          | 0.15                 | PL  | ... | ...   | ...                                                                                             | ... | bcu   | 1RXS<br>J095812.8−675241 |
| J0958.6+6534  | 149.660 | 65.567  | 145.756 | 43.118  | 0.036      | 0.035      | 21     | 27.2     | 1.4      | 0.1             | 17.9     | 0.9             | 2.38          | 0.04                 | PL  | T   | ...   | 1FHL J0959.5+6535<br>2FGL J0958.6+6533<br>1FGL J1000.1+6539<br>3EG J0958+6533<br>EGR J0956+6524 | ... | bll   | S4 0954+65               |
| J0958.6−2447  | 149.669 | −24.798 | 260.307 | 23.441  | 0.173      | 0.137      | −68    | 6.2      | 0.4      | 0.1             | 4.8      | 0.9             | 2.24          | 0.13                 | PL  | ... | ...   | 2FGL J0958.6−2446                                                                               | ... | bcu   | TXS 0956−244             |
| J0959.7+2124  | 149.927 | 21.414  | 211.656 | 50.634  | 0.091      | 0.085      | 83     | 5.8      | 0.3      | 0.1             | 3.6      | 0.8             | 2.15          | 0.16                 | PL  | ... | ...   | ...                                                                                             | ... | bll   | RX J0959.4+2123          |
| J1001.0+2913  | 150.251 | 29.226  | 199.449 | 52.588  | 0.083      | 0.061      | −57    | 13.2     | 0.7      | 0.1             | 8.3      | 0.9             | 2.16          | 0.08                 | PL  | T   | ...   | 2FGL J1001.0+2913<br>1FGL J1000.9+2915                                                          | ... | bll   | GB6 J1001+2911           |
| J1002.0−2837  | 150.503 | −28.628 | 263.619 | 21.026  | 0.496      | 0.325      | 15     | 4.2      | 0.3      | 0.1             | 4.3      | 0.9             | 2.58          | 0.15                 | PL  | ... | ...   | ...                                                                                             | ... | ...   | ...                      |
| J1002.3+2220  | 150.599 | 22.338  | 210.528 | 51.495  | 0.237      | 0.173      | −79    | 4.7      | 0.3      | 0.1             | 3.5      | 0.8             | 2.31          | 0.17                 | PL  | ... | ...   | 2FGL J1003.0+2219                                                                               | ... | bll   | 1RXS<br>J100235.8+221609 |
| J1002.5−5709  | 150.646 | −57.163 | 281.558 | −1.472  | 0.144      | 0.101      | 63     | 9.4      | 2.7      | 0.3             | 24.8     | 3.8             | 2.49          | ...                  | LP  | ... | 3,5   | ...                                                                                             | ... | ...   | ...                      |
| J1003.6+2608  | 150.920 | 26.137  | 204.630 | 52.674  | 0.140      | 0.125      | −21    | 4.9      | 0.3      | 0.1             | 3.3      | 0.8             | 2.29          | 0.18                 | PL  | ... | ...   | ...                                                                                             | ... | bcu   | PKS 1000+26              |
| J1003.7−5215  | 150.947 | −52.252 | 278.768 | 2.574   | 0.147      | 0.104      | −74    | 4.1      | 0.5      | 0.1             | 6.4      | 1.5             | 2.31          | 0.13                 | PL  | ... | ...   | ...                                                                                             | ... | ...   | ...                      |
| J1005.0−4959  | 151.261 | −49.986 | 277.579 | 4.514   | 0.208      | 0.186      | −59    | 5.1      | 0.3      | 0.1             | 7.4      | 1.3             | 2.78          | 0.16                 | PL  | ... | 1,4   | ...                                                                                             | ... | bcu   | PMN J1006−5018           |
| J1006.7+3453  | 151.695 | 34.893  | 190.078 | 54.134  | 0.097      | 0.071      | 34     | 5.5      | 0.2      | 0.1             | 2.4      | 0.8             | 1.66          | 0.22                 | PL  | ... | ...   | 1FGL J1007.0+3454                                                                               | ... | bll   | EXO 1004.0+3509          |
| J1006.7−2159  | 151.700 | −21.985 | 259.804 | 26.784  | 0.053      | 0.043      | −70    | 21.7     | 1.3      | 0.1             | 18.3     | 1.1             | 2.43          | 0.05                 | PL  | T   | ...   | 1FGL J1007.1−2157<br>2FGL J1007.1−2157                                                          | ... | fsrq  | PKS 1004−217             |
| J1007.4−3334  | 151.875 | −33.576 | 267.884 | 17.913  | 0.336      | 0.331      | −17    | 4.1      | 0.3      | 0.1             | 4.6      | 1.0             | 2.54          | 0.14                 | PL  | ... | ...   | ...                                                                                             | ... | fsrq  | PKS 1005−333             |
| J1007.8+0026  | 151.964 | 0.442   | 240.226 | 42.550  | 0.118      | 0.103      | −68    | 5.6      | 0.4      | 0.1             | 3.9      | 0.8             | 2.09          | 0.15                 | PL  | ... | ...   | 2FGL J1008.6+0028                                                                               | ... | bcu   | PKS 1005+007             |
| J1007.9+0621  | 151.986 | 6.358   | 233.506 | 45.999  | 0.053      | 0.050      | −85    | 16.8     | 1.2      | 0.1             | 14.5     | 1.2             | 2.28          | 0.06                 | PL  | T   | ...   | 2FGL J1007.7+0621<br>1FGL J1007.9+0619                                                          | ... | bll   | MG1 J100800+0621         |
| J1008.6−5706  | 152.172 | −57.113 | 282.198 | −0.944  | 0.102      | 0.060      | −84    | 8.3      | 2.2      | 0.3             | 32.5     | 4.4             | 2.51          | 0.08                 | PL  | ... | 3     | ...                                                                                             | ... | ...   | ...                      |
| J1008.9−2910  | 152.229 | −29.174 | 265.246 | 21.560  | 0.114      | 0.100      | −16    | 5.4      | 0.3      | 0.1             | 4.3      | 0.9             | 2.39          | 0.15                 | PL  | ... | 1     | ...                                                                                             | ... | bcu   | PMN J1008−2912           |
| J1009.0−3137  | 152.251 | −31.624 | 266.882 | 19.648  | 0.100      | 0.095      | 4      | 5.5      | 0.5      | 0.1             | 6.6      | 1.2             | 2.35          | 0.12                 | PL  | ... | 5     | ...                                                                                             | ... | bcu   | PKS 1006−313             |
| J1010.2−3120  | 152.572 | −31.340 | 266.926 | 20.040  | 0.034      | 0.030      | 71     | 14.1     | 0.8      | 0.1             | 12.5     | 1.8             | 1.58          | 0.10                 | PL  | T   | ...   | 1FHL J1009.6−3118<br>2FGL J1009.7−3123                                                          | P   | bll   | 1RXS<br>J101015.9−311909 |
| J1010.8−7645c | 152.710 | −76.756 | 294.058 | −16.738 | 0.182      | 0.127      | −73    | 4.2      | 0.4      | 0.1             | 4.9      | 1.2             | 2.31          | 0.16                 | PL  | ... | 6     | ...                                                                                             | ... | ...   | ...                      |
| J1010.8−0158  | 152.713 | −1.976  | 243.398 | 41.620  | 0.132      | 0.111      | 89     | 5.7      | 0.3      | 0.1             | 4.3      | 0.8             | 2.38          | 0.14                 | PL  | ... | ...   | 2FGL J1010.8−0158<br>1FGL J1011.0−0156                                                          | ... | fsrq  | PKS 1008−01              |
| J1012.0−4235  | 153.022 | −42.598 | 274.198 | 11.211  | 0.066      | 0.064      | 29     | 8.9      | 0.7      | 0.1             | 7.5      | 1.1             | 2.03          | 0.10                 | PL  | ... | 10    | 2FGL J1012.1−4236                                                                               | ... | psr   | PSR J1012−42             |
| J1012.2+0631  | 153.072 | 6.523   | 234.163 | 46.992  | 0.054      | 0.049      | −10    | 10.2     | 0.7      | 0.1             | 7.3      | 1.1             | 2.08          | 0.11                 | PL  | ... | ...   | 2FGL J1012.1+0631<br>1FGL J1012.2+0634                                                          | ... | bll   | NRAO 350                 |

Table 1—Continued

| Name 3FGL    | R.A.    | Decl.   | $l$     | $b$    | $\theta_1$ | $\theta_2$ | $\phi$ | $\sigma$ | $F_{35}$ | $\Delta F_{35}$ | $S_{25}$ | $\Delta S_{25}$ | $\Gamma_{25}$ | $\Delta \Gamma_{25}$ | Mod | Var | Flags                                                              | $\gamma$ -ray Assoc.                                                             | TeV  | Class | ID or Assoc. |                          |
|--------------|---------|---------|---------|--------|------------|------------|--------|----------|----------|-----------------|----------|-----------------|---------------|----------------------|-----|-----|--------------------------------------------------------------------|----------------------------------------------------------------------------------|------|-------|--------------|--------------------------|
| J1012.6+2439 | 153.152 | 24.660  | 207.763 | 54.340 | 0.035      | 0.033      | 38     | 40.8     | 3.0      | 0.2             | 29.7     | 1.4             | 2.27          | ...                  | LP  | T   | ...<br>2FGL J1012.6+2440<br>1FGL J1012.7+2440<br>0FGL J1012.9+2435 | ...                                                                              | fsrq | MG2   | J101241+2439 |                          |
| J1012.7+4229 | 153.184 | 42.494  | 176.901 | 54.401 | 0.058      | 0.051      | 17     | 9.8      | 0.4      | 0.1             | 4.9      | 1.0             | 1.66          | 0.13                 | PL  | ... | ...                                                                | 2FGL J1012.5+4227                                                                | ...  | bll   | B3           | 1009+427                 |
| J1013.4-4008 | 153.367 | -40.150 | 272.958 | 13.354 | 0.234      | 0.101      | 32     | 4.4      | 0.3      | 0.1             | 4.0      | 1.0             | 2.25          | 0.18                 | PL  | ... | 9                                                                  | ...                                                                              | ...  | ...   | ...          |                          |
| J1013.5+3440 | 153.383 | 34.678  | 190.398 | 55.526 | 0.140      | 0.110      | -29    | 8.7      | 0.4      | 0.1             | 6.5      | 0.8             | 2.62          | 0.11                 | PL  | ... | ...                                                                | 2FGL J1013.6+3434                                                                | ...  | fsrq  | OL           | 318                      |
| J1013.6-5734 | 153.412 | -57.569 | 283.008 | -0.935 | 0.088      | 0.064      | 4      | 9.5      | 2.5      | 0.4             | 22.9     | 3.0             | 2.36          | ...                  | LP  | ... | 5                                                                  | 3EG J1014-5705                                                                   | ...  | ...   | ...          | ...                      |
| J1014.2+4115 | 153.560 | 41.254  | 178.900 | 54.930 | 0.124      | 0.106      | -50    | 5.6      | 0.3      | 0.1             | 3.5      | 0.7             | 2.42          | 0.15                 | PL  | ... | ...                                                                | ...                                                                              | ...  | bcu   | GB6          | J1014+4112               |
| J1015.0+4925 | 153.771 | 49.433  | 165.534 | 52.715 | 0.013      | 0.012      | -12    | 84.6     | 7.4      | 0.2             | 88.7     | 3.1             | 1.83          | 0.02                 | PL  | T   | ...                                                                | 1FHL J1015.0+4925<br>2FGL J1015.1+4925<br>1FGL J1015.1+4927<br>0FGL J1015.2+4927 | P    | bll   | 1H           | 1013+498                 |
| J1015.2-4512 | 153.807 | -45.213 | 276.196 | 9.396  | 0.123      | 0.082      | -44    | 5.8      | 0.5      | 0.1             | 5.5      | 1.0             | 2.24          | 0.13                 | PL  | ... | 1                                                                  | ...                                                                              | ...  | bcu   | PMN          | J1014-4508               |
| J1016.0+0513 | 154.003 | 5.217   | 236.512 | 47.024 | 0.028      | 0.027      | 85     | 27.2     | 2.5      | 0.2             | 28.2     | 1.7             | 2.12          | 0.04                 | PL  | T   | ...                                                                | 1FHL J1016.0+0512<br>2FGL J1016.0+0513<br>1FGL J1016.1+0514<br>0FGL J1015.9+0515 | ...  | fsrq  | TXS          | 1013+054<br> <br>55<br>- |
| J1016.0-0635 | 154.022 | -6.590  | 249.075 | 39.519 | 0.220      | 0.169      | 82     | 4.5      | 0.3      | 0.1             | 4.0      | 0.8             | 2.54          | 0.16                 | PL  | ... | ...                                                                | 2FGL J1016.2-0638                                                                | ...  | bcu   | NVSS         | J101626-063624           |
| J1016.1+5555 | 154.034 | 55.922  | 156.069 | 50.012 | 0.096      | 0.089      | 3      | 9.5      | 0.3      | 0.1             | 5.1      | 0.6             | 2.53          | 0.11                 | PL  | ... | ...                                                                | 2FGL J1016.1+5600                                                                | ...  | bcu   | TXS          | 1012+560                 |
| J1016.3-5858 | 154.079 | -58.967 | 284.083 | -1.894 | 0.031      | 0.029      | -86    | 18.9     | 7.8      | 0.5             | 65.5     | 7.4             | 2.35          | ...                  | EC  | ... | 5                                                                  | 2FGL J1016.5-5858<br>3EG J1013-5915                                              | E    | PSR   | PSR          | J1016-5857               |
| J1016.5-6034 | 154.135 | -60.576 | 285.005 | -3.214 | 0.219      | 0.171      | 55     | 11.3     | 0.7      | 0.2             | 20.0     | 2.0             | 2.69          | ...                  | LP  | ... | ...                                                                | ...                                                                              | ...  | ...   | ...          | ...                      |
| J1016.6-4244 | 154.164 | -42.746 | 274.986 | 11.573 | 0.093      | 0.083      | 57     | 5.7      | 0.4      | 0.1             | 4.4      | 1.1             | 1.78          | 0.16                 | PL  | ... | ...                                                                | 2FGL J1016.4-4244                                                                | ...  | ...   | ...          | ...                      |
| J1016.9-2653 | 154.246 | -26.898 | 265.244 | 24.450 | 0.219      | 0.157      | -77    | 4.8      | 0.3      | 0.1             | 4.5      | 0.9             | 2.61          | 0.15                 | PL  | ... | ...                                                                | ...                                                                              | ...  | ...   | ...          | ...                      |
| J1018.1+1904 | 154.526 | 19.076  | 217.534 | 53.980 | 0.041      | 0.039      | 74     | 11.3     | 0.6      | 0.1             | 6.9      | 1.0             | 1.98          | 0.11                 | PL  | ... | ...                                                                | ...                                                                              | ...  | bll   | NVSS         | J101808+190614           |
| J1018.2-6254 | 154.559 | -62.905 | 286.470 | -5.038 | 0.174      | 0.130      | -66    | 5.3      | 0.5      | 0.1             | 7.7      | 1.5             | 2.57          | 0.12                 | PL  | ... | 1                                                                  | ...                                                                              | ...  | ...   | ...          | ...                      |
| J1018.3+3542 | 154.582 | 35.713  | 188.467 | 56.455 | 0.165      | 0.114      | 40     | 6.1      | 0.3      | 0.1             | 4.3      | 0.8             | 2.55          | 0.14                 | PL  | T   | ...                                                                | 2FGL J1017.0+3531                                                                | ...  | fsrq  | B2           | 1015+35B                 |
| J1018.4-3119 | 154.612 | -31.323 | 268.402 | 21.102 | 0.184      | 0.120      | -51    | 8.7      | 0.5      | 0.1             | 8.4      | 1.1             | 2.53          | 0.09                 | PL  | ... | ...                                                                | 2FGL J1018.3-3119                                                                | ...  | fsrq  | PKS          | 1016-311                 |
| J1018.5+0530 | 154.628 | 5.503   | 236.693 | 47.698 | 0.080      | 0.070      | -68    | 9.3      | 0.8      | 0.1             | 9.9      | 1.4             | 2.35          | 0.09                 | PL  | ... | 5                                                                  | 2FGL J1018.6+0531                                                                | ...  | fsrq  | TXS          | 1015+057                 |
| J1018.8+5913 | 154.719 | 59.231  | 151.460 | 48.581 | 0.079      | 0.073      | -77    | 7.4      | 0.3      | 0.1             | 3.4      | 0.6             | 2.09          | 0.15                 | PL  | ... | ...                                                                | 2FGL J1019.0+5915                                                                | ...  | bll   | TXS          | 1015+594                 |
| J1018.9-5856 | 154.730 | -58.946 | 284.351 | -1.690 | 0.014      | 0.014      | 28     | 52.2     | 27.1     | 0.6             | 250.3    | 8.3             | 2.30          | ...                  | LP  | ... | ...                                                                | 1FHL J1018.9-5855<br>2FGL J1019.0-5856<br>1FGL J1018.6-5856<br>0FGL J1018.2-5858 | E    | HMB   | 1FGL         | J1018.6-5856             |
| J1020.0-5749 | 155.000 | -57.817 | 283.851 | -0.669 | 0.049      | 0.046      | 26     | 11.1     | 4.0      | 0.4             | 49.2     | 6.1             | 2.33          | 0.06                 | PL  | ... | 3,5                                                                | ...                                                                              | ...  | PSR   | PSR          | J1019-5749               |

Table 1—Continued

| Name 3FGL     | R.A.    | Decl.   | $l$     | $b$     | $\theta_1$ | $\theta_2$ | $\phi$ | $\sigma$ | $F_{35}$ | $\Delta F_{35}$ | $S_{25}$ | $\Delta S_{25}$ | $\Gamma_{25}$ | $\Delta \Gamma_{25}$ | Mod | Var | Flags | $\gamma$ -ray Assoc.                                        | TeV | Class | ID or Assoc.             |
|---------------|---------|---------|---------|---------|------------|------------|--------|----------|----------|-----------------|----------|-----------------|---------------|----------------------|-----|-----|-------|-------------------------------------------------------------|-----|-------|--------------------------|
| J1020.0+6323  | 155.023 | 63.384  | 146.355 | 46.266  | 0.089      | 0.084      | −30    | 7.9      | 0.4      | 0.1             | 4.3      | 0.6             | 2.29          | 0.11                 | PL  | ... | ...   | 2FGL J1019.8+6322                                           | ... | bll   | GB6 J1019+6319           |
| J1021.8+8023  | 155.470 | 80.385  | 130.009 | 34.589  | 0.077      | 0.074      | −60    | 9.9      | 0.5      | 0.1             | 5.6      | 0.7             | 2.33          | 0.10                 | PL  | ... | ...   | 2FGL J1021.6+8021                                           | ... | bcu   | NVSS<br>J102201+802350   |
| J1021.9−5815c | 155.484 | −58.265 | 284.309 | −0.905  | 0.156      | 0.094      | −89    | 5.7      | 1.8      | 0.4             | 22.3     | 5.3             | 2.30          | 0.10                 | PL  | ... | 1,5,6 | 1AGL J1022−5822                                             | ... | ...   | ...                      |
| J1022.3−4234  | 155.598 | −42.578 | 275.783 | 12.302  | 0.129      | 0.105      | 23     | 4.3      | 0.3      | 0.1             | 4.0      | 1.0             | 2.34          | 0.18                 | PL  | ... | ...   | ...                                                         | ... | bcu   | PMN J1022−4232           |
| J1022.8−0113  | 155.704 | −1.224  | 245.274 | 44.380  | 0.047      | 0.041      | 78     | 11.2     | 0.7      | 0.1             | 8.0      | 1.2             | 1.87          | 0.09                 | PL  | ... | ...   | 2FGL J1023.1−0115<br>1FGL J1022.8−0115                      | ... | bll   | RX J1022.7−0112          |
| J1023.1+3952  | 155.779 | 39.873  | 180.734 | 56.850  | 0.181      | 0.155      | −8     | 8.5      | 0.3      | 0.1             | 5.8      | 0.8             | 2.73          | 0.12                 | PL  | T   | ...   | 2FGL J1023.6+3947<br>1FGL J1023.6+3937                      | ... | fsrq  | 4C +40.25                |
| J1023.1−5745  | 155.790 | −57.759 | 284.174 | −0.392  | 0.018      | 0.018      | −32    | 31.2     | 19.9     | 0.8             | 148.1    | 8.2             | 2.25          | ...                  | EC  | ... | ...   | 1FGL J1023.0−5746<br>1FHL J1022.6−5745<br>2FGL J1022.7−5741 | E   | PSR   | LAT PSR J1023−5746       |
| J1023.7+3000  | 155.947 | 30.014  | 198.950 | 57.593  | 0.068      | 0.061      | 81     | 6.2      | 0.2      | 0.1             | 3.0      | 0.8             | 1.75          | 0.21                 | PL  | ... | ...   | 1FHL J1023.6+2959<br>2FGL J1023.6+2959                      | ... | bll   | RX J1023.6+3001          |
| J1023.9−4335  | 155.985 | −43.585 | 276.590 | 11.615  | 0.024      | 0.024      | 34     | 19.7     | 1.4      | 0.1             | 17.2     | 1.7             | 1.79          | 0.06                 | PL  | ... | ...   | 1FHL J1023.9−4337<br>2FGL J1023.8−4335<br>1FGL J1024.0−4332 | ... | bll   | RX J1023.9−4336          |
| J1024.1−3232  | 156.041 | −32.539 | 270.216 | 20.816  | 0.053      | 0.050      | −57    | 21.1     | 1.4      | 0.1             | 20.1     | 1.2             | 2.46          | 0.05                 | PL  | T   | ...   | 2FGL J1023.8−3248<br>...                                    | ... | fsrq  | PKS 1021−323             |
| J1024.3−5757  | 156.085 | −57.951 | 284.409 | −0.470  | 0.064      | 0.047      | 70     | 5.4      | 1.2      | 0.5             | 13.8     | 4.3             | 1.90          | 0.19                 | PL  | ... | 5     | 0FGL J1024.0−5754                                           | E   | ...   | ...                      |
| J1024.4−4545  | 156.104 | −45.752 | 277.859 | 9.841   | 0.061      | 0.049      | −86    | 5.2      | 0.3      | 0.1             | 3.4      | 1.0             | 1.96          | 0.20                 | PL  | ... | ...   | ...                                                         | ... | ...   | ...                      |
| J1024.6−0718  | 156.152 | −7.311  | 251.683 | 40.517  | 0.110      | 0.101      | 69     | 9.0      | 0.8      | 0.1             | 3.6      | 0.5             | 2.13          | ...                  | EC  | ... | 12    | 2FGL J1024.6−0719<br>1FGL J1024.6−0718                      | ... | PSR   | PSR J1024−0719           |
| J1024.8+0105  | 156.224 | 1.096   | 243.246 | 46.283  | 0.301      | 0.220      | 21     | 6.5      | 0.4      | 0.1             | 5.8      | 0.9             | 2.55          | 0.12                 | PL  | ... | ...   | ...                                                         | ... | bcu   | PMN J1024+0056           |
| J1025.1+2333  | 156.284 | 23.562  | 210.825 | 56.868  | 0.135      | 0.109      | −28    | 7.1      | 0.3      | 0.1             | 5.0      | 0.8             | 2.57          | 0.14                 | PL  | ... | ...   | ...                                                         | ... | bll   | MG2 J102456+2332         |
| J1025.1−6507  | 156.292 | −65.121 | 288.321 | −6.485  | 0.092      | 0.077      | 83     | 7.3      | 0.7      | 0.1             | 9.3      | 1.4             | 2.42          | 0.09                 | PL  | ... | 3     | ...                                                         | ... | ...   | ...                      |
| J1025.7−5659c | 156.443 | −57.000 | 284.067 | 0.438   | 0.077      | 0.056      | 82     | 4.5      | 1.1      | 0.3             | 13.4     | 3.7             | 2.35          | 0.13                 | PL  | ... | 5,6   | ...                                                         | ... | ...   | ...                      |
| J1025.9−5930  | 156.475 | −59.513 | 285.410 | −1.686  | 0.152      | 0.090      | −49    | 5.7      | 1.2      | 0.2             | 13.7     | 3.2             | 2.22          | 0.14                 | PL  | ... | ...   | ...                                                         | ... | ...   | ...                      |
| J1026.2−5730  | 156.560 | −57.517 | 284.394 | 0.033   | 0.054      | 0.049      | 84     | 13.1     | 5.9      | 0.5             | 46.9     | 5.1             | 2.28          | ...                  | LP  | ... | 5     | ...                                                         | ... | ...   | ...                      |
| J1026.4−8542  | 156.605 | −85.715 | 300.168 | −23.646 | 0.046      | 0.040      | −70    | 13.4     | 0.9      | 0.1             | 10.1     | 1.2             | 2.01          | 0.08                 | PL  | ... | ...   | 1FHL J1029.0−8543<br>2FGL J1026.3−8546<br>1FGL J1028.7−8543 | ... | bll   | PKS 1029−85              |
| J1026.5+7423  | 156.637 | 74.392  | 134.776 | 39.224  | 0.160      | 0.120      | −28    | 4.7      | 0.3      | 0.1             | 5.1      | 1.1             | 2.57          | 0.12                 | PL  | ... | 5     | ...                                                         | ... | bcu   | GB6 J1027+7428           |
| J1026.9−1750  | 156.729 | −17.840 | 260.927 | 32.995  | 0.033      | 0.030      | 50     | 23.1     | 1.8      | 0.1             | 20.2     | 1.7             | 1.92          | 0.05                 | PL  | T   | ...   | 2FGL J1026.7−1749<br>1FGL J1027.1−1747                      | ... | bll   | 1RXS<br>J102658.5−174905 |
| J1027.0+0609  | 156.758 | 6.161   | 237.740 | 49.806  | 0.067      | 0.054      | 54     | 6.1      | 0.3      | 0.1             | 3.6      | 0.8             | 2.09          | 0.20                 | PL  | ... | ...   | ...                                                         | ... | bll   | NVSS<br>J102703+060934   |



Table 1—Continued

| Name 3FGL     | R.A.    | Decl.   | $l$     | $b$     | $\theta_1$ | $\theta_2$ | $\phi$ | $\sigma$ | $F_{35}$ | $\Delta F_{35}$ | $S_{25}$ | $\Delta S_{25}$ | $\Gamma_{25}$ | $\Delta \Gamma_{25}$ | Mod | Var | Flags | $\gamma$ -ray Assoc.                                                                               | TeV | Class | ID or Assoc.                |
|---------------|---------|---------|---------|---------|------------|------------|--------|----------|----------|-----------------|----------|-----------------|---------------|----------------------|-----|-----|-------|----------------------------------------------------------------------------------------------------|-----|-------|-----------------------------|
| J1027.7+6316  | 156.932 | 63.275  | 145.695 | 47.002  | 0.072      | 0.064      | -31    | 7.1      | 0.3      | 0.1             | 3.3      | 0.6             | 2.00          | 0.15                 | PL  | ... | ...   | ...                                                                                                | ... | bll   | RX J1027.4+6317             |
| J1027.8+8253  | 156.963 | 82.898  | 127.879 | 32.794  | 0.103      | 0.092      | 76     | 6.2      | 0.3      | 0.1             | 3.2      | 0.6             | 2.07          | 0.14                 | PL  | ... | ...   | ...                                                                                                | ... | ...   | ...                         |
| J1028.0+1829  | 157.017 | 18.496  | 219.935 | 55.980  | 0.089      | 0.084      | 23     | 5.8      | 0.3      | 0.1             | 3.5      | 0.7             | 2.24          | 0.16                 | PL  | ... | ...   | ...                                                                                                | ... | bcu   | GB6 J1027+1831              |
| J1028.3-7419  | 157.089 | -74.327 | 293.561 | -14.120 | 0.387      | 0.257      | -86    | 4.8      | 0.3      | 0.1             | 5.6      | 1.1             | 2.69          | 0.16                 | PL  | ... | ...   | ...                                                                                                | ... | ...   | ...                         |
| J1028.4-5819  | 157.123 | -58.320 | 285.069 | -0.495  | 0.012      | 0.012      | -74    | 57.5     | 33.3     | 0.7             | 251.2    | 6.2             | 2.18          | ...                  | EC  | ... | ...   | 1FHL J1028.4-5819<br>2FGL J1028.5-5819<br>1FGL J1028.4-5819<br>0FGL J1028.6-5817<br>3EG J1027-5817 | ... | PSR   | PSR J1028-5819              |
| J1028.5-0235  | 157.144 | -2.585  | 248.041 | 44.532  | 0.124      | 0.112      | -55    | 4.7      | 0.3      | 0.1             | 3.5      | 0.8             | 2.40          | 0.16                 | PL  | T   | ...   | ...                                                                                                | ... | fsrq  | PMN J1028-0237              |
| J1030.0-5809  | 157.509 | -58.153 | 285.157 | -0.248  | 0.064      | 0.054      | 78     | 5.7      | 1.0      | 0.5             | 12.7     | 3.9             | 1.79          | 0.23                 | PL  | ... | 5     | 3EG J1027-5817                                                                                     | ... | ...   | ...                         |
| J1030.4-2030  | 157.608 | -20.507 | 263.636 | 31.398  | 0.065      | 0.061      | -41    | 10.1     | 0.6      | 0.1             | 7.3      | 1.1             | 1.89          | 0.11                 | PL  | ... | ...   | ...                                                                                                | ... | bcu   | NVSS<br>J103040-203032      |
| J1031.0+7440  | 157.762 | 74.682  | 134.237 | 39.209  | 0.071      | 0.061      | 30     | 6.8      | 0.4      | 0.1             | 4.4      | 0.9             | 2.15          | 0.16                 | PL  | ... | ...   | 2FGL J1029.9+7437                                                                                  | ... | bcu   | S5 1027+74                  |
| J1031.2+5053  | 157.817 | 50.887  | 161.453 | 54.437  | 0.029      | 0.026      | 74     | 18.9     | 0.8      | 0.1             | 11.3     | 1.3             | 1.71          | 0.07                 | PL  | ... | ...   | 1FHL J1031.0+5052<br>2FGL J1031.0+5053<br>1FGL J1031.0+5051                                        | ... | bll   | 1ES 1028+511                |
| J1031.4-5855  | 157.864 | -58.920 | 285.709 | -0.811  | 0.112      | 0.079      | 65     | 5.0      | 1.0      | 0.3             | 11.5     | 2.9             | 2.09          | 0.14                 | PL  | ... | ...   | ...                                                                                                | ... | ...   | ...                         |
| J1031.6+6021  | 157.917 | 60.359  | 148.628 | 49.211  | 0.077      | 0.065      | -26    | 9.0      | 0.6      | 0.1             | 11.3     | 1.7             | 2.63          | 0.12                 | PL  | T   | ...   | ...                                                                                                | ... | fsrq  | TXS 1028+605                |
| J1032.5+6623  | 158.145 | 66.394  | 141.850 | 45.299  | 0.094      | 0.085      | 39     | 4.6      | 0.2      | 0.0             | 2.0      | 0.5             | 2.15          | 0.18                 | PL  | ... | ...   | ...                                                                                                | ... | bll   | SDSS<br>J103239.06+662323.2 |
| J1032.7+3735  | 158.183 | 37.590  | 184.336 | 59.106  | 0.076      | 0.063      | -45    | 16.7     | 0.9      | 0.1             | 10.7     | 0.9             | 2.33          | 0.07                 | PL  | ... | ...   | 2FGL J1032.6+3733<br>1FGL J1032.7+3737                                                             | ... | bll   | B3 1029+378                 |
| J1033.0-5945  | 158.266 | -59.751 | 286.308 | -1.423  | 0.052      | 0.044      | -75    | 11.3     | 2.4      | 0.2             | 30.6     | 3.4             | 2.38          | 0.06                 | PL  | ... | ...   | ...                                                                                                | ... | ...   | ...                         |
| J1033.2+4116  | 158.303 | 41.276  | 177.359 | 58.393  | 0.044      | 0.043      | -20    | 24.7     | 1.3      | 0.1             | 15.6     | 0.9             | 2.32          | 0.05                 | PL  | T   | ...   | 2FGL J1033.2+4117<br>1FGL J1033.2+4116                                                             | ... | fsrq  | S4 1030+41                  |
| J1033.4-5035  | 158.374 | -50.595 | 281.724 | 6.509   | 0.056      | 0.053      | 69     | 10.4     | 0.9      | 0.1             | 10.0     | 1.3             | 2.02          | 0.10                 | PL  | ... | ...   | 2FGL J1033.5-5032<br>1FGL J1033.5-5033                                                             | ... | ...   | ...                         |
| J1033.8+6051  | 158.461 | 60.859  | 147.778 | 49.101  | 0.020      | 0.019      | -1     | 51.4     | 5.2      | 0.2             | 47.1     | 2.3             | 2.20          | ...                  | LP  | T   | ...   | 1FHL J1033.7+6051<br>2FGL J1033.9+6050<br>1FGL J1033.8+6048<br>0FGL J1034.0+6051                   | ... | FSRQ  | S4 1030+61                  |
| J1034.0-5731c | 158.516 | -57.517 | 285.295 | 0.572   | 0.263      | 0.129      | 36     | 7.5      | 1.8      | 0.3             | 22.1     | 3.3             | 2.28          | 0.08                 | PL  | ... | 5,6,9 | ...                                                                                                | ... | ...   | ...                         |
| J1035.2+5545  | 158.822 | 55.751  | 153.993 | 52.371  | 0.235      | 0.175      | -52    | 5.7      | 0.1      | 0.0             | 4.3      | 0.7             | 2.94          | 0.17                 | PL  | ... | ...   | ...                                                                                                | ... | bcu   | GB6 J1035+5542              |
| J1035.7-6720  | 158.926 | -67.334 | 290.391 | -7.828  | 0.037      | 0.034      | -58    | 30.5     | 3.6      | 0.2             | 25.9     | 1.5             | 2.21          | ...                  | LP  | ... | ...   | 2FGL J1036.1-6722<br>1FGL J1036.2-6719                                                             | ... | ...   | ...                         |
| J1036.0-8317  | 159.022 | -83.288 | 298.921 | -21.497 | 0.117      | 0.109      | 26     | 6.7      | 0.5      | 0.1             | 5.8      | 1.0             | 2.33          | 0.11                 | PL  | ... | ...   | ...                                                                                                | ... | psr   | PSR J1036-83                |

Table 1—Continued

| Name 3FGL     | R.A.    | Decl.   | $l$     | $b$    | $\theta_1$ | $\theta_2$ | $\phi$ | $\sigma$ | $F_{35}$ | $\Delta F_{35}$ | $S_{25}$ | $\Delta S_{25}$ | $\Gamma_{25}$ | $\Delta \Gamma_{25}$ | Mod | Var | Flags      | $\gamma$ -ray Assoc. | TeV | Class | ID or Assoc.       |
|---------------|---------|---------|---------|--------|------------|------------|--------|----------|----------|-----------------|----------|-----------------|---------------|----------------------|-----|-----|------------|----------------------|-----|-------|--------------------|
| J1036.4−4348  | 159.113 | −43.812 | 278.678 | 12.612 | 0.197      | 0.166      | 73     | 4.6      | 0.4      | 0.1             | 4.4      | 0.9             | 2.28          | 0.15                 | PL  | ... | ...        | ...                  | ... | ...   | ...                |
| J1037.0−2934  | 159.266 | −29.583 | 270.921 | 24.809 | 0.195      | 0.154      | 66     | 7.2      | 0.5      | 0.1             | 7.4      | 1.1             | 2.49          | 0.11                 | PL  | T   | 5          | ...                  | ... | fsrq  | PKS 1034−293       |
| J1037.2−6052  | 159.319 | −60.875 | 287.321 | −2.136 | 0.670      | 0.520      | 16     | 7.3      | 1.3      | 0.2             | 12.5     | 2.0             | 2.34          | ...                  | LP  | ... | 1,4,5,9    | ...                  | ... | ...   | ...                |
| J1037.4−3742  | 159.358 | −37.715 | 275.612 | 17.947 | 0.223      | 0.191      | −51    | 4.6      | 0.2      | 0.1             | 4.3      | 0.9             | 2.76          | 0.16                 | PL  | ... | ...        | ...                  | ... | fsrq  | PKS 1034−374       |
| J1037.5−2821  | 159.377 | −28.364 | 270.277 | 25.885 | 0.065      | 0.056      | 47     | 12.1     | 0.8      | 0.1             | 11.3     | 1.1             | 2.49          | 0.08                 | PL  | T   | ...        | 2FGL J1037.5−2820    | ... | fsrq  | PKS B1035−281      |
|               |         |         |         |        |            |            |        |          |          |                 |          |                 |               |                      |     |     |            | 1FGL J1037.7−2820    |     |       |                    |
| J1037.5+5711  | 159.389 | 57.195  | 151.801 | 51.766 | 0.020      | 0.019      | 10     | 51.2     | 3.8      | 0.2             | 34.3     | 2.1             | 1.87          | ...                  | LP  | T   | ...        | 1FHL J1037.4+5712    | ... | bll   | GB6 J1037+5711     |
|               |         |         |         |        |            |            |        |          |          |                 |          |                 |               |                      |     |     |            | 2FGL J1037.6+5712    |     |       |                    |
|               |         |         |         |        |            |            |        |          |          |                 |          |                 |               |                      |     |     |            | 1FGL J1037.7+5711    |     |       |                    |
| J1037.9−5843  | 159.488 | −58.730 | 286.342 | −0.226 | 0.094      | 0.060      | −17    | 11.1     | 3.6      | 0.4             | 27.2     | 3.5             | 2.19          | ...                  | LP  | ... | 3          | ...                  | ... | ...   | ...                |
| J1038.0−2425  | 159.519 | −24.431 | 267.943 | 29.232 | 0.139      | 0.108      | −3     | 5.1      | 0.3      | 0.1             | 4.2      | 0.9             | 2.40          | 0.15                 | PL  | ... | ...        | 2FGL J1038.2−2423    | ... | ...   | ...                |
| J1038.9−5311  | 159.735 | −53.186 | 283.752 | 4.679  | 0.059      | 0.055      | −64    | 24.4     | 1.9      | 0.2             | 31.6     | 1.6             | 2.62          | ...                  | LP  | T   | ...        | ...                  | ... | bcu   | MRC 1036−529       |
| J1039.1−5809  | 159.789 | −58.157 | 286.200 | 0.351  | 0.349      | 0.306      | 1      | 7.4      | 2.5      | 0.4             | 16.3     | 3.2             | 2.20          | ...                  | LP  | ... | 1,5,9      | 1AGL J1043−5749      | ... | ...   | ...                |
| J1039.5+7324  | 159.885 | 73.409  | 134.735 | 40.556 | 0.109      | 0.080      | −78    | 5.6      | 0.3      | 0.1             | 3.4      | 0.8             | 2.09          | 0.16                 | PL  | ... | ...        | ...                  | ... | ...   | ...                |
| J1040.4+0615  | 160.116 | 6.260   | 240.792 | 52.545 | 0.046      | 0.041      | 45     | 20.5     | 1.4      | 0.1             | 16.7     | 1.2             | 2.23          | 0.05                 | PL  | T   | ...        | 2FGL J1040.7+0614    | ... | bcu   | GB6 J1040+0617     |
|               |         |         |         |        |            |            |        |          |          |                 |          |                 |               |                      |     |     |            | 1FGL J1040.5+0616    |     |       |                    |
| J1040.5−5926c | 160.137 | −59.433 | 286.975 | −0.679 | 0.095      | 0.083      | 3      | 6.0      | 1.6      | 0.3             | 17.8     | 3.8             | 2.17          | 0.10                 | PL  | ... | 1,3,5,6,10 | 1AGL J1043−5936      | ... | ...   | ...                |
| J1040.8+1342  | 160.220 | 13.703  | 230.134 | 56.733 | 0.101      | 0.076      | 46     | 4.9      | 0.2      | 0.1             | 2.7      | 0.8             | 1.76          | 0.21                 | PL  | ... | ...        | ...                  | ... | bcu   | 1RXS               |
|               |         |         |         |        |            |            |        |          |          |                 |          |                 |               |                      |     |     |            |                      |     |       | J104057.7+134216   |
| J1040.9−1205  | 160.241 | −12.089 | 259.765 | 39.606 | 0.135      | 0.081      | 30     | 5.5      | 0.3      | 0.1             | 3.5      | 0.8             | 2.11          | 0.20                 | PL  | ... | ...        | 1FGL J1040.9−1205    | ... | bcu   | NVSS               |
|               |         |         |         |        |            |            |        |          |          |                 |          |                 |               |                      |     |     |            |                      |     |       | J104108−120332     |
| J1041.8+3901  | 160.451 | 39.018  | 180.832 | 60.557 | 0.071      | 0.068      | −44    | 4.7      | 0.2      | 0.1             | 2.2      | 0.6             | 1.97          | 0.16                 | PL  | ... | ...        | ...                  | ... | bll   | B3 1038+392        |
| J1042.0−0557  | 160.501 | −5.957  | 254.704 | 44.460 | 0.074      | 0.059      | −46    | 6.2      | 0.3      | 0.1             | 3.4      | 0.8             | 1.94          | 0.32                 | PL  | ... | ...        | ...                  | ... | bcu   | PMN J1042−0558     |
| J1042.1−4126  | 160.535 | −41.434 | 278.387 | 15.194 | 0.085      | 0.069      | 31     | 4.7      | 0.3      | 0.1             | 2.8      | 0.8             | 1.98          | 0.23                 | PL  | ... | ...        | ...                  | ... | bcu   | 1RXS               |
|               |         |         |         |        |            |            |        |          |          |                 |          |                 |               |                      |     |     |            |                      |     |       | J104204.1−412936   |
| J1043.1+2407  | 160.797 | 24.131  | 211.610 | 61.015 | 0.056      | 0.051      | 20     | 13.0     | 0.8      | 0.1             | 9.1      | 0.9             | 2.24          | 0.08                 | PL  | ... | ...        | 1FHL J1043.2+2407    | ... | fsrq  | B2 1040+24A        |
|               |         |         |         |        |            |            |        |          |          |                 |          |                 |               |                      |     |     |            | 2FGL J1043.1+2404    |     |       |                    |
|               |         |         |         |        |            |            |        |          |          |                 |          |                 |               |                      |     |     |            | 1FGL J1043.1+2404    |     |       |                    |
| J1043.6−5930  | 160.905 | −59.505 | 287.352 | −0.556 | 0.076      | 0.050      | 29     | 6.2      | 1.9      | 0.5             | 21.4     | 5.0             | 2.07          | 0.11                 | PL  | ... | 5          | 1AGL J1043−5936      | ... | ...   | ...                |
| J1043.8−5851  | 160.974 | −58.859 | 287.079 | 0.030  | 0.091      | 0.079      | −42    | 4.3      | 0.7      | 0.2             | 8.0      | 2.5             | 1.93          | 0.18                 | PL  | ... | 4,5        | ...                  | ... | ...   | ...                |
| J1044.4+8058  | 161.119 | 80.968  | 128.696 | 34.691 | 0.123      | 0.103      | 87     | 5.9      | 0.3      | 0.1             | 6.5      | 1.3             | 2.76          | 0.12                 | PL  | T   | 5          | 2FGL J1042.6+8053    | ... | fsrq  | S5 1039+81         |
|               |         |         |         |        |            |            |        |          |          |                 |          |                 |               |                      |     |     |            | 1FGL J1048.7+8054    |     |       |                    |
| J1044.5−5737  | 161.129 | −57.630 | 286.575 | 1.154  | 0.018      | 0.018      | 47     | 57.6     | 16.4     | 0.4             | 136.0    | 3.9             | 2.30          | ...                  | EC  | ... | ...        | 2FGL J1044.5−5737    | ... | PSR   | LAT PSR J1044−5737 |
|               |         |         |         |        |            |            |        |          |          |                 |          |                 |               |                      |     |     |            | 1FGL J1044.5−5737    |     |       |                    |
|               |         |         |         |        |            |            |        |          |          |                 |          |                 |               |                      |     |     |            | 1AGL J1043−5749      |     |       |                    |
| J1045.1−5941  | 161.277 | −59.692 | 287.606 | −0.633 | 0.015      | 0.014      | −51    | 33.1     | 17.2     | 0.7             | 137.6    | 7.0             | 2.13          | ...                  | LP  | ... | ...        | 1FHL J1045.0−5943    | ... | BIN   | Eta Carinae        |
|               |         |         |         |        |            |            |        |          |          |                 |          |                 |               |                      |     |     |            | 2FGL J1045.0−5941    |     |       |                    |
|               |         |         |         |        |            |            |        |          |          |                 |          |                 |               |                      |     |     |            | 1FGL J1045.2−5942    |     |       |                    |

Table 1—Continued

| Name 3FGL    | R.A.    | Decl.   | $l$     | $b$    | $\theta_1$ | $\theta_2$ | $\phi$ | $\sigma$ | $F_{35}$ | $\Delta F_{35}$ | $S_{25}$ | $\Delta S_{25}$ | $\Gamma_{25}$ | $\Delta\Gamma_{25}$ | Mod | Var | Flags  | $\gamma$ -ray Assoc. | TeV | Class | ID or Assoc.           |
|--------------|---------|---------|---------|--------|------------|------------|--------|----------|----------|-----------------|----------|-----------------|---------------|---------------------|-----|-----|--------|----------------------|-----|-------|------------------------|
|              |         |         |         |        |            |            |        |          |          |                 |          |                 |               |                     |     |     |        | 0FGL J1045.6–5937    |     |       |                        |
|              |         |         |         |        |            |            |        |          |          |                 |          |                 |               |                     |     |     |        | 1AGL J1043–5936      |     |       |                        |
| J1045.3–6414 | 161.330 | –64.243 | 289.753 | –4.647 | 0.227      | 0.173      | –66    | 6.4      | 0.8      | 0.1             | 11.1     | 1.8             | 2.49          | 0.10                | PL  | ... | 1,5    | ...                  | ... | ...   | ...                    |
| J1045.5–2335 | 161.397 | –23.591 | 269.063 | 30.878 | 0.125      | 0.114      | 86     | 4.1      | 0.3      | 0.1             | 3.4      | 0.9             | 2.37          | 0.18                | PL  | ... | ...    | ...                  | ... | ...   | ...                    |
| J1045.7–2926 | 161.443 | –29.440 | 272.616 | 25.933 | 0.072      | 0.063      | 83     | 12.9     | 0.8      | 0.1             | 11.1     | 1.1             | 2.46          | 0.08                | PL  | T   | ...    | 2FGL J1045.5–2931    | ... | fsrq  | PKS B1043–291          |
| J1046.9–2531 | 161.728 | –25.526 | 270.553 | 29.404 | 0.072      | 0.064      | –71    | 5.1      | 0.3      | 0.1             | 3.1      | 0.9             | 1.85          | 0.18                | PL  | ... | ...    | ...                  | ... | bll   | NVSS<br>J104651–253547 |
| J1047.3–6005 | 161.844 | –60.098 | 288.046 | –0.862 | 0.085      | 0.071      | 87     | 9.0      | 3.5      | 0.4             | 26.6     | 4.0             | 2.23          | ...                 | LP  | ... | 3,5,7  | 2FGL J1046.8–6005c   | ... | ...   | ...                    |
|              |         |         |         |        |            |            |        |          |          |                 |          |                 |               |                     |     |     |        | 1AGL J1043–5936      |     |       |                        |
| J1047.6+7240 | 161.918 | 72.667  | 134.735 | 41.506 | 0.047      | 0.039      | 46     | 12.0     | 0.7      | 0.1             | 7.5      | 0.9             | 2.06          | 0.10                | PL  | T   | ...    | 1FGL J1048.5+7239    | ... | bll   | GB6 J1047+7238         |
|              |         |         |         |        |            |            |        |          |          |                 |          |                 |               |                     |     |     |        | 1FHL J1048.3+7241    |     |       |                        |
|              |         |         |         |        |            |            |        |          |          |                 |          |                 |               |                     |     |     |        | 2FGL J1049.7+7240    |     |       |                        |
| J1047.8–6216 | 161.963 | –62.283 | 289.099 | –2.778 | 0.048      | 0.041      | 58     | 18.7     | 2.8      | 0.2             | 36.1     | 2.4             | 2.52          | ...                 | LP  | T   | 3      | 2FGL J1047.7–6216    | ... | bcu   | PMN J1047–6217         |
| J1047.8–3737 | 161.968 | –37.625 | 277.451 | 19.058 | 0.096      | 0.079      | 34     | 6.3      | 0.4      | 0.1             | 4.5      | 1.0             | 1.90          | 0.18                | PL  | ... | ...    | ...                  | ... | ...   | ...                    |
| J1048.2–5928 | 162.055 | –59.477 | 287.856 | –0.261 | 0.061      | 0.058      | 7      | 9.4      | 3.9      | 0.4             | 28.8     | 4.1             | 3.18          | ...                 | LP  | ... | 3,5    | 1AGL J1043–5936      | ... | ...   | ...                    |
| J1048.2–5832 | 162.067 | –58.535 | 287.433 | 0.580  | 0.013      | 0.013      | –33    | 79.4     | 26.6     | 0.5             | 201.0    | 4.5             | 2.20          | ...                 | EC  | ... | ...    | 1FHL J1048.4–5832    | ... | PSR   | PSR J1048.2–5832       |
|              |         |         |         |        |            |            |        |          |          |                 |          |                 |               |                     |     |     |        | 2FGL J1048.2–5831    |     |       |                        |
|              |         |         |         |        |            |            |        |          |          |                 |          |                 |               |                     |     |     |        | 1FGL J1048.2–5832    |     |       |                        |
|              |         |         |         |        |            |            |        |          |          |                 |          |                 |               |                     |     |     |        | 0FGL J1047.6–5834    |     |       |                        |
|              |         |         |         |        |            |            |        |          |          |                 |          |                 |               |                     |     |     |        | 3EG J1048–5840       |     |       |                        |
|              |         |         |         |        |            |            |        |          |          |                 |          |                 |               |                     |     |     |        | EGR J1048–5839       |     |       |                        |
| J1048.4+7144 | 162.122 | 71.742  | 135.430 | 42.275 | 0.029      | 0.028      | 23     | 40.7     | 2.8      | 0.1             | 36.6     | 1.2             | 2.39          | 0.03                | PL  | T   | ...    | 2FGL J1048.3+7144    | ... | FSRQ  | S5 1044+71             |
|              |         |         |         |        |            |            |        |          |          |                 |          |                 |               |                     |     |     |        | 1FGL J1048.8+7145    |     |       |                        |
| J1048.6+2338 | 162.172 | 23.641  | 213.217 | 62.126 | 0.116      | 0.097      | –33    | 9.0      | 0.6      | 0.1             | 6.7      | 0.9             | 2.29          | 0.10                | PL  | ... | ...    | 2FGL J1048.6+2336    | ... | bll   | NVSS<br>J104900+233821 |
|              |         |         |         |        |            |            |        |          |          |                 |          |                 |               |                     |     |     |        | 1FGL J1048.7+2335    |     |       |                        |
| J1048.8–5006 | 162.206 | –50.106 | 283.645 | 8.117  | 0.159      | 0.122      | 51     | 4.3      | 0.4      | 0.1             | 5.1      | 1.2             | 2.30          | 0.17                | PL  | ... | ...    | ...                  | ... | ...   | ...                    |
| J1049.7+1548 | 162.433 | 15.807  | 228.514 | 59.610 | 0.089      | 0.080      | 42     | 7.6      | 0.4      | 0.1             | 4.8      | 0.8             | 2.15          | 0.13                | PL  | ... | ...    | 2FGL J1049.4+1551    | ... | ...   | ...                    |
| J1049.8+1425 | 162.473 | 14.431  | 230.930 | 58.998 | 0.125      | 0.099      | –80    | 7.3      | 0.4      | 0.1             | 5.3      | 0.8             | 2.33          | 0.12                | PL  | T   | ...    | ...                  | ... | bcu   | MG1 J104945+1429       |
| J1050.4+0435 | 162.617 | 4.599   | 245.550 | 53.413 | 0.088      | 0.070      | 4      | 17.1     | 1.1      | 0.1             | 15.1     | 1.1             | 2.47          | 0.06                | PL  | T   | ...    | ...                  | ... | ...   | ...                    |
| J1050.6–6112 | 162.675 | –61.212 | 288.914 | –1.670 | 0.123      | 0.099      | 71     | 5.1      | 1.1      | 0.2             | 13.4     | 2.9             | 2.35          | 0.10                | PL  | ... | 1,5,10 | ...                  | ... | ...   | ...                    |
| J1051.0+5332 | 162.763 | 53.549  | 154.680 | 55.514 | 0.390      | 0.282      | –44    | 4.6      | 0.1      | 0.0             | 3.2      | 0.7             | 2.87          | 0.20                | PL  | ... | ...    | ...                  | ... | ...   | ...                    |
| J1051.4+3941 | 162.861 | 39.692  | 178.420 | 62.167 | 0.082      | 0.063      | –22    | 6.3      | 0.2      | 0.1             | 3.3      | 0.9             | 1.66          | 0.17                | PL  | ... | ...    | 2FGL J1051.3+3938    | ... | bll   | RBS 0909               |
| J1051.5–6517 | 162.876 | –65.290 | 290.822 | –5.278 | 0.072      | 0.056      | 42     | 9.6      | 1.0      | 0.1             | 16.6     | 2.0             | 2.60          | 0.08                | PL  | ... | ...    | ...                  | ... | bcu   | PKS 1049–650           |
| J1051.8+0105 | 162.969 | 1.088   | 250.145 | 51.271 | 0.051      | 0.050      | 62     | 7.1      | 0.4      | 0.1             | 4.4      | 0.9             | 2.07          | 0.15                | PL  | ... | ...    | 2FGL J1051.8+0107    | ... | bll   | NVSS<br>J105151+010312 |
|              |         |         |         |        |            |            |        |          |          |                 |          |                 |               |                     |     |     |        | 1FGL J1051.9+0106    |     |       |                        |
| J1052.0+0816 | 163.018 | 8.281   | 241.059 | 56.058 | 0.134      | 0.111      | 88     | 4.5      | 0.3      | 0.1             | 3.2      | 0.8             | 2.22          | 0.16                | PL  | ... | ...    | ...                  | ... | ...   | ...                    |

Table 1—Continued

| Name 3FGL     | R.A.    | Decl.   | $l$     | $b$     | $\theta_1$ | $\theta_2$ | $\phi$ | $\sigma$ | $F_{35}$ | $\Delta F_{35}$ | $S_{25}$ | $\Delta S_{25}$ | $\Gamma_{25}$ | $\Delta \Gamma_{25}$ | Mod | Var | Flags | $\gamma$ -ray Assoc.                                                                                               | TeV | Class | ID or Assoc.            |
|---------------|---------|---------|---------|---------|------------|------------|--------|----------|----------|-----------------|----------|-----------------|---------------|----------------------|-----|-----|-------|--------------------------------------------------------------------------------------------------------------------|-----|-------|-------------------------|
| J1052.8–3741  | 163.202 | –37.695 | 278.397 | 19.460  | 0.154      | 0.092      | –7     | 5.4      | 0.4      | 0.1             | 4.0      | 0.9             | 2.00          | 0.20                 | PL  | ... | ...   | ...                                                                                                                | ... | bcu   | PMN J1053–3743          |
| J1053.7+4929  | 163.430 | 49.488  | 160.255 | 58.235  | 0.037      | 0.036      | 25     | 12.5     | 0.6      | 0.1             | 7.0      | 1.1             | 1.80          | 0.10                 | PL  | ... | ...   | 1FHL J1053.6+4931<br>2FGL J1053.6+4928<br>1FGL J1053.6+4927<br>0FGL J1053.7+4926                                   | ... | bll   | GB6 J1053+4930          |
| J1054.2–3123  | 163.569 | –31.392 | 275.456 | 25.155  | 0.263      | 0.237      | –30    | 5.8      | 0.3      | 0.1             | 5.5      | 0.9             | 2.72          | 0.13                 | PL  | ... | 1     | ...                                                                                                                | ... | ...   | ...                     |
| J1054.5+2210  | 163.646 | 22.180  | 217.052 | 63.057  | 0.033      | 0.031      | –6     | 22.7     | 1.4      | 0.1             | 16.4     | 1.1             | 2.20          | 0.06                 | PL  | T   | ...   | 1FHL J1054.6+2214<br><br>2FGL J1054.5+2212<br>1FGL J1054.5+2212<br>0FGL J1054.5+2212                               | ... | bll   | 87GB<br>105148.6+222705 |
| J1054.7–6006  | 163.697 | –60.111 | 288.878 | –0.461  | 0.100      | 0.077      | –14    | 7.3      | 2.0      | 0.3             | 22.4     | 4.1             | 2.18          | 0.09                 | PL  | ... | 5     | ...                                                                                                                | ... | ...   | ...                     |
| J1055.8–6025  | 163.967 | –60.426 | 289.135 | –0.688  | 0.061      | 0.049      | 72     | 12.7     | 4.7      | 0.4             | 29.5     | 4.2             | 2.25          | ...                  | EC  | ... | ...   | 2FGL J1056.2–6021                                                                                                  | ... | PSR   | PSR J1055–6028          |
| J1056.7–5853  | 164.179 | –58.896 | 288.576 | 0.741   | 0.086      | 0.077      | 35     | 16.1     | 3.5      | 0.3             | 31.0     | 2.6             | 2.40          | ...                  | LP  | ... | ...   | 2FGL J1056.0–5853                                                                                                  | ... | ...   | ...                     |
| J1057.3–2341  | 164.343 | –23.693 | 271.826 | 32.199  | 0.147      | 0.121      | 16     | 7.0      | 0.5      | 0.1             | 5.9      | 0.9             | 2.32          | 0.11                 | PL  | ... | 10    | ...                                                                                                                | ... | fsrq  | PKS B1054–234           |
| J1057.6–4051  | 164.409 | –40.862 | 280.791 | 17.067  | 0.067      | 0.056      | –81    | 5.6      | 0.2      | 0.1             | 3.2      | 0.9             | 1.76          | 0.22                 | PL  | ... | ...   | ...                                                                                                                | ... | ...   | ...                     |
| J1057.6–2754  | 164.411 | –27.908 | 274.293 | 28.560  | 0.064      | 0.054      | –25    | 5.5      | 0.3      | 0.1             | 3.2      | 0.8             | 1.89          | 0.18                 | PL  | ... | ...   | ...                                                                                                                | ... | bll   | RX J1057.8–2753         |
| J1057.7–6624  | 164.436 | –66.403 | 291.887 | –6.001  | 0.064      | 0.050      | 27     | 9.1      | 0.9      | 0.1             | 12.5     | 1.7             | 2.46          | 0.10                 | PL  | ... | 3     | 2FGL J1058.7–6621                                                                                                  | ... | ...   | ...                     |
| J1057.9–5227  | 164.499 | –52.455 | 285.989 | 6.644   | 0.010      | 0.010      | 17     | 200.1    | 49.4     | 0.6             | 289.7    | 2.8             | 2.02          | ...                  | EC  | ... | ...   | 2FGL J1057.9–5226<br>1FGL J1057.9–5226<br>0FGL J1058.1–5225<br>3EG J1058–5234<br>EGR J1058–5221<br>1AGL J1058–5239 | ... | PSR   | PSR J1057–5226          |
| J1058.1+7010  | 164.536 | 70.175  | 135.858 | 44.000  | 0.129      | 0.115      | 67     | 12.4     | 0.4      | 0.1             | 8.7      | 0.8             | 2.70          | 0.08                 | PL  | T   | ...   | 2FGL J1057.1+7001                                                                                                  | ... | fsrq  | S5 1053+70              |
| J1058.4+8112  | 164.621 | 81.203  | 127.987 | 34.787  | 0.095      | 0.081      | –5     | 8.6      | 0.4      | 0.1             | 8.3      | 1.2             | 2.67          | 0.10                 | PL  | T   | ...   | 2FGL J1059.4+8113                                                                                                  | ... | fsrq  | S5 1053+81              |
| J1058.5+0133  | 164.626 | 1.564   | 251.517 | 52.775  | 0.020      | 0.019      | 39     | 55.0     | 6.5      | 0.2             | 65.4     | 2.5             | 2.21          | ...                  | LP  | T   | ...   | 1FHL J1058.5+0133<br>2FGL J1058.4+0133<br>1FGL J1058.4+0134<br>0FGL J1057.8+0138                                   | ... | BLL   | 4C +01.28               |
| J1058.5–8003  | 164.631 | –80.051 | 297.995 | –18.280 | 0.030      | 0.029      | –48    | 39.0     | 3.6      | 0.2             | 35.4     | 1.6             | 2.27          | ...                  | LP  | T   | ...   | 2FGL J1057.0–8004<br>1FGL J1058.1–8006<br>0FGL J1100.2–8000                                                        | ... | bll   | PKS 1057–79             |
| J1058.5–6106c | 164.644 | –61.110 | 289.726 | –1.166  | 0.135      | 0.121      | 25     | 4.9      | 1.2      | 0.3             | 13.5     | 3.9             | 2.16          | 0.16                 | PL  | ... | 5,6   | 2FGL J1059.3–6118c<br>3EG J1102–6103<br>EGR J1058–6101                                                             | ... | ...   | ...                     |

Table 1—Continued

| Name 3FGL     | R.A.    | Decl.   | $l$     | $b$     | $\theta_1$ | $\theta_2$ | $\phi$ | $\sigma$ | $F_{35}$ | $\Delta F_{35}$ | $S_{25}$ | $\Delta S_{25}$ | $\Gamma_{25}$ | $\Delta \Gamma_{25}$ | Mod | Var | Flags | $\gamma$ -ray Assoc.                                                                                                                    | TeV | Class | ID or Assoc.     |
|---------------|---------|---------|---------|---------|------------|------------|--------|----------|----------|-----------------|----------|-----------------|---------------|----------------------|-----|-----|-------|-----------------------------------------------------------------------------------------------------------------------------------------|-----|-------|------------------|
| J1058.6+5627  | 164.665 | 56.455  | 149.606 | 54.438  | 0.017      | 0.016      | −30    | 54.6     | 3.6      | 0.1             | 41.2     | 1.8             | 1.95          | 0.03                 | PL  | T   | ...   | 1FHL J1058.6+5627<br>2FGL J1058.6+5628<br>1FGL J1058.6+5628<br>0FGL J1058.9+5629                                                        | ... | BLL   | TXS 1055+567     |
| J1059.2−1133  | 164.803 | −11.551 | 264.100 | 42.702  | 0.032      | 0.029      | −4     | 32.9     | 2.6      | 0.1             | 29.3     | 1.5             | 2.14          | 0.04                 | PL  | T   | ...   | 1FHL J1058.8−1134<br>2FGL J1059.3−1132<br>1FGL J1059.3−1132                                                                             | ... | bll   | PKS B1056−113    |
| J1059.3+0224  | 164.845 | 2.417   | 250.783 | 53.537  | 0.102      | 0.095      | −26    | 6.8      | 0.6      | 0.1             | 7.6      | 1.4             | 2.35          | 0.12                 | PL  | ... | ...   | 2FGL J1059.0+0222                                                                                                                       | ... | ...   | ...              |
| J1059.9+2056  | 164.982 | 20.946  | 220.534 | 63.861  | 0.110      | 0.104      | 61     | 4.4      | 0.2      | 0.1             | 3.4      | 0.9             | 2.57          | 0.23                 | PL  | ... | ...   | ...                                                                                                                                     | ... | fsrq  | MG2 J105938+2057 |
| J1100.2−2044  | 165.055 | −20.747 | 270.724 | 35.076  | 0.218      | 0.160      | 51     | 4.7      | 0.3      | 0.1             | 3.8      | 0.8             | 2.41          | 0.18                 | PL  | ... | ...   | 2FGL J1059.9−2051                                                                                                                       | ... | ...   | ...              |
| J1100.5+4020  | 165.145 | 40.338  | 175.802 | 63.600  | 0.067      | 0.053      | −69    | 9.1      | 0.4      | 0.1             | 4.9      | 0.9             | 1.84          | 0.15                 | PL  | ... | ...   | 1FHL J1100.6+4018<br>2FGL J1100.9+4014                                                                                                  | ... | bll   | RX J1100.3+4019  |
| J1101.3−6032  | 165.330 | −60.542 | 289.793 | −0.510  | 0.080      | 0.058      | −6     | 5.1      | 1.0      | 0.3             | 11.3     | 3.3             | 1.97          | 0.16                 | PL  | ... | 5     | 3EG J1102−6103                                                                                                                          | ... | ...   | ...              |
| J1101.5+4106  | 165.385 | 41.108  | 174.048 | 63.477  | 0.095      | 0.064      | −48    | 7.1      | 0.3      | 0.1             | 3.7      | 0.8             | 1.77          | 0.17                 | PL  | ... | ...   | ...                                                                                                                                     | ... | bll   | RX J1101.3+4108  |
| J1101.9−6053  | 165.481 | −60.896 | 290.006 | −0.803  | 0.083      | 0.054      | 82     | 10.6     | 4.8      | 0.5             | 44.6     | 6.1             | 2.28          | ...                  | LP  | ... | 3,5   | 3EG J1102−6103                                                                                                                          | ... | spp   | ...              |
| J1103.1+1155  | 165.778 | 11.930  | 238.515 | 60.407  | 0.082      | 0.066      | 2      | 11.4     | 0.6      | 0.1             | 8.4      | 0.9             | 2.52          | 0.09                 | PL  | T   | ...   | ...                                                                                                                                     | ... | fsrq  | TXS 1103+122     |
| J1103.3+5239  | 165.837 | 52.662  | 153.788 | 57.501  | 0.213      | 0.155      | −19    | 6.7      | 0.2      | 0.1             | 4.0      | 0.6             | 2.62          | 0.14                 | PL  | ... | ...   | ...                                                                                                                                     | ... | ...   | ...              |
| J1103.5−2329  | 165.895 | −23.490 | 273.178 | 33.076  | 0.049      | 0.043      | 62     | 9.0      | 0.4      | 0.1             | 5.8      | 1.2             | 1.64          | 0.14                 | PL  | ... | ...   | 1FHL J1103.3−2329<br>2FGL J1103.4−2330<br>1FGL J1103.7−2329                                                                             | P   | bll   | 1ES 1101−232     |
| J1103.9−5357  | 165.977 | −53.954 | 287.425 | 5.648   | 0.029      | 0.027      | −72    | 32.3     | 4.2      | 0.2             | 38.9     | 2.2             | 2.20          | ...                  | LP  | T   | ...   | 1FHL J1104.2−5356<br>2FGL J1103.9−5356<br>1FGL J1103.9−5355                                                                             | ... | bll   | PKS 1101−536     |
| J1104.3+0730  | 166.077 | 7.511   | 245.673 | 57.920  | 0.064      | 0.060      | −78    | 10.9     | 0.7      | 0.1             | 7.9      | 1.0             | 2.19          | 0.09                 | PL  | ... | ...   | 2FGL J1104.3+0729<br>1FGL J1104.4+0734                                                                                                  | ... | bll   | MG1 J110424+0730 |
| J1104.3−7736c | 166.079 | −77.611 | 297.162 | −15.956 | 0.181      | 0.162      | 15     | 6.3      | 0.6      | 0.1             | 8.8      | 1.4             | 2.51          | 0.10                 | PL  | ... | 1,6   | ...                                                                                                                                     | ... | ...   | ...              |
| J1104.4+3812  | 166.118 | 38.210  | 179.827 | 65.035  | 0.007      | 0.007      | −12    | 190.3    | 30.3     | 0.4             | 383.0    | 6.9             | 1.77          | 0.01                 | PL  | T   | ...   | 1FHL J1104.4+3812<br>2FGL J1104.4+3812<br>1FGL J1104.4+3812<br>0FGL J1104.5+3811<br>3EG J1104+3809<br>EGR J1104+3813<br>1AGL J1104+3754 | P   | BLL   | Mkn 421          |
| J1104.9−6036  | 166.248 | −60.609 | 290.233 | −0.389  | 0.045      | 0.043      | −55    | 15.4     | 5.7      | 0.4             | 37.2     | 4.6             | 2.28          | ...                  | LP  | ... | ...   | 2FGL J1104.7−6036<br>3EG J1102−6103                                                                                                     | ... | ...   | ...              |

Table 1—Continued

| Name 3FGL    | R.A.    | Decl.   | $l$     | $b$    | $\theta_1$ | $\theta_2$ | $\phi$ | $\sigma$ | $F_{35}$ | $\Delta F_{35}$ | $S_{25}$ | $\Delta S_{25}$ | $\Gamma_{25}$ | $\Delta \Gamma_{25}$ | Mod | Var | Flags | $\gamma$ -ray Assoc.                                                      | TeV | Class | ID or Assoc.             |
|--------------|---------|---------|---------|--------|------------|------------|--------|----------|----------|-----------------|----------|-----------------|---------------|----------------------|-----|-----|-------|---------------------------------------------------------------------------|-----|-------|--------------------------|
| J1105.2–6113 | 166.305 | –61.223 | 290.503 | –0.941 | 0.087      | 0.067      | 10     | 10.9     | 3.1      | 0.3             | 41.9     | 4.5             | 2.43          | 0.06                 | PL  | ... | 5,10  | 1AGL J1108–6103<br>2FGL J1105.6–6114<br>3EG J1102–6103<br>1AGL J1108–6103 | ... | PSR   | PSR J1105–6107           |
| J1105.7+4427 | 166.427 | 44.456  | 166.686 | 62.649 | 0.076      | 0.075      | –62    | 5.3      | 0.2      | 0.1             | 2.9      | 0.6             | 2.41          | 0.17                 | PL  | ... | ...   | ...                                                                       | ... | ...   | ...                      |
| J1105.9+2814 | 166.495 | 28.237  | 204.051 | 66.673 | 0.069      | 0.060      | 68     | 19.0     | 0.9      | 0.1             | 13.3     | 0.9             | 2.47          | 0.06                 | PL  | T   | ...   | 2FGL J1106.1+2814<br>1FGL J1106.5+2809                                    | ... | fsrq  | MG2 J110606+2812         |
| J1106.4–3643 | 166.604 | –36.733 | 280.529 | 21.528 | 0.063      | 0.054      | –40    | 11.7     | 0.8      | 0.1             | 9.3      | 1.0             | 2.29          | 0.08                 | PL  | ... | ...   | 2FGL J1106.3–3643                                                         | ... | bcu   | PMN J1106–3647           |
| J1106.6–1744 | 166.661 | –17.740 | 270.465 | 38.437 | 0.122      | 0.111      | 2      | 5.2      | 0.4      | 0.1             | 3.9      | 0.9             | 2.03          | 0.13                 | PL  | ... | 1     | 1FGL J1106.2–1752                                                         | ... | ...   | ...                      |
| J1107.4–4447 | 166.857 | –44.789 | 284.207 | 14.268 | 0.111      | 0.095      | 49     | 13.8     | 0.9      | 0.1             | 17.2     | 1.3             | 2.71          | 0.06                 | PL  | T   | ...   | 2FGL J1107.2–4448                                                         | ... | fsrq  | PKS 1104–445             |
| J1107.5+0223 | 166.886 | 2.384   | 253.344 | 54.922 | 0.076      | 0.064      | 42     | 6.9      | 0.4      | 0.1             | 4.9      | 0.9             | 2.12          | 0.13                 | PL  | ... | ...   | 1FHL J1107.5+0223                                                         | ... | bll   | NVSS<br>J110735+022225   |
| J1107.8+1502 | 166.960 | 15.046  | 234.306 | 63.065 | 0.062      | 0.057      | –69    | 11.7     | 0.6      | 0.1             | 7.0      | 1.0             | 1.99          | 0.10                 | PL  | ... | ...   | 2FGL J1107.5+0223<br>2FGL J1107.8+1505<br>1FGL J1107.8+1502               | ... | bll   | RX J1107.7+1502          |
| J1109.4+2411 | 167.365 | 24.198  | 214.483 | 66.875 | 0.096      | 0.076      | 50     | 6.2      | 0.3      | 0.1             | 3.6      | 0.8             | 1.89          | 0.18                 | PL  | ... | ...   | 2FGL J1109.3+2414                                                         | ... | bll   | 1ES 1106+2411            |
| J1109.4–4815 | 167.368 | –48.256 | 285.947 | 11.224 | 0.144      | 0.127      | 87     | 6.6      | 0.5      | 0.1             | 7.3      | 1.2             | 2.49          | 0.11                 | PL  | ... | ...   | ...                                                                       | ... | bcu   | PMN J1109–4815           |
| J1109.6+3734 | 167.417 | 37.578  | 180.491 | 66.207 | 0.064      | 0.055      | 10     | 5.0      | 0.2      | 0.1             | 2.2      | 0.7             | 1.66          | 0.22                 | PL  | ... | ...   | ...                                                                       | ... | bll   | NVSS<br>J110938+373609   |
| J1110.0+7134 | 167.504 | 71.573  | 133.665 | 43.379 | 0.067      | 0.048      | 63     | 8.8      | 0.3      | 0.1             | 3.7      | 0.6             | 2.03          | 0.15                 | PL  | ... | ...   | 2FGL J1110.2+7134<br>1FGL J1109.9+7134                                    | ... | bll   | RX J1110.5+7133          |
| J1110.4–1835 | 167.620 | –18.597 | 272.013 | 38.139 | 0.059      | 0.056      | 7      | 13.0     | 0.9      | 0.1             | 10.1     | 1.2             | 2.02          | 0.08                 | PL  | ... | ...   | 2FGL J1110.1–1835<br>1FGL J1110.2–1839                                    | ... | bll   | CRATES J1110–1835        |
| J1111.9–6058 | 167.978 | –60.969 | 291.151 | –0.394 | 0.048      | 0.044      | 19     | 14.1     | 5.8      | 0.6             | 41.8     | 5.3             | 2.21          | ...                  | EC  | T   | 5     | 1AGL J1108–6103<br>1FHL J1112.5–6105<br>2FGL J1112.5–6105                 | ... | PSR   | PSR J1112–6103           |
| J1111.9–6038 | 167.993 | –60.641 | 291.035 | –0.088 | 0.022      | 0.021      | –34    | 29.2     | 11.1     | 0.5             | 83.7     | 5.0             | 2.16          | ...                  | LP  | ... | ...   | 1FHL J1111.5–6038<br>2FGL J1112.1–6040<br>1AGL J1108–6103                 | ... | spp   | ...                      |
| J1112.0–6135 | 168.017 | –61.584 | 291.398 | –0.958 | 0.099      | 0.068      | –2     | 15.7     | 5.0      | 0.4             | 43.8     | 3.9             | 2.38          | ...                  | LP  | ... | 7     | 1AGL J1108–6103                                                           | ... | ...   | ...                      |
| J1112.1+0500 | 168.034 | 5.010   | 251.588 | 57.616 | 0.066      | 0.060      | 64     | 5.3      | 0.3      | 0.1             | 3.7      | 0.9             | 2.09          | 0.17                 | PL  | ... | ...   | 1FGL J1112.3+0458                                                         | ... | ...   | ...                      |
| J1112.1+1034 | 168.039 | 10.574  | 243.480 | 61.370 | 0.126      | 0.118      | 31     | 4.7      | 0.3      | 0.1             | 3.7      | 0.9             | 2.48          | 0.18                 | PL  | ... | ...   | ...                                                                       | ... | ...   | ...                      |
| J1112.4+3449 | 168.116 | 34.823  | 186.840 | 67.506 | 0.060      | 0.046      | –60    | 24.5     | 1.3      | 0.1             | 14.7     | 1.0             | 2.39          | ...                  | LP  | T   | ...   | 2FGL J1112.4+3450<br>1FGL J1112.8+3444                                    | ... | fsrq  | TXS 1109+350             |
| J1112.6+1749 | 168.154 | 17.820  | 229.979 | 65.407 | 0.093      | 0.068      | –25    | 4.6      | 0.1      | 0.1             | 2.2      | 0.8             | 1.47          | 0.36                 | PL  | ... | ...   | ...                                                                       | ... | bll   | 1RXS<br>J111224.2+175131 |
| J1113.1–4515 | 168.286 | –45.251 | 285.352 | 14.239 | 0.119      | 0.118      | 26     | 4.2      | 0.4      | 0.1             | 4.3      | 1.1             | 2.32          | 0.16                 | PL  | ... | ...   | ...                                                                       | ... | ...   | ...                      |
| J1115.0–0701 | 168.761 | –7.028  | 265.110 | 48.636 | 0.054      | 0.051      | –1     | 10.0     | 0.6      | 0.1             | 6.9      | 1.0             | 2.11          | 0.11                 | PL  | T   | ...   | 1FHL J1115.0–0701                                                         | ... | ...   | ...                      |

Table 1—Continued

| Name 3FGL    | R.A.    | Decl.   | $l$     | $b$    | $\theta_1$ | $\theta_2$ | $\phi$ | $\sigma$ | $F_{35}$ | $\Delta F_{35}$ | $S_{25}$ | $\Delta S_{25}$ | $\Gamma_{25}$ | $\Delta \Gamma_{25}$ | Mod | Var | Flags | $\gamma$ -ray Assoc. | TeV | Class            | ID or Assoc.     |
|--------------|---------|---------|---------|--------|------------|------------|--------|----------|----------|-----------------|----------|-----------------|---------------|----------------------|-----|-----|-------|----------------------|-----|------------------|------------------|
|              |         |         |         |        |            |            |        |          |          |                 |          |                 |               |                      |     |     |       | 2FGL J1115.0–0701    |     |                  |                  |
| J1116.7–4854 | 169.182 | −48.901 | 287.328 | 11.080 | 0.263      | 0.197      | 85     | 5.1      | 0.4      | 0.1             | 6.1      | 1.2             | 2.46          | 0.13                 | PL  | ... | 1     | 2FGL J1117.2–4844    | ... | ...              | ...              |
| J1117.0+2014 | 169.274 | 20.233  | 225.589 | 67.370 | 0.027      | 0.024      | −71    | 26.4     | 1.7      | 0.1             | 20.5     | 1.7             | 1.87          | 0.05                 | PL  | T   | ...   | 1FHL J1117.2+2013    | ... | bll              | RBS 0958         |
|              |         |         |         |        |            |            |        |          |          |                 |          |                 |               |                      |     |     |       | 2FGL J1117.2+2013    |     |                  |                  |
|              |         |         |         |        |            |            |        |          |          |                 |          |                 |               |                      |     |     |       | 1FGL J1117.1+2013    |     |                  |                  |
| J1117.2–5338 | 169.307 | −53.648 | 289.136 | 6.681  | 0.050      | 0.049      | 21     | 10.4     | 0.9      | 0.1             | 9.6      | 1.3             | 2.00          | 0.10                 | PL  | ... | 3     | 2FGL J1117.2–5341    | ... | ...              | ...              |
|              |         |         |         |        |            |            |        |          |          |                 |          |                 |               |                      |     |     |       | 1FGL J1117.0–5339    |     |                  |                  |
| J1117.3+2546 | 169.330 | 25.781  | 211.238 | 68.922 | 0.161      | 0.131      | 20     | 5.0      | 0.3      | 0.1             | 2.9      | 0.7             | 2.15          | 0.18                 | PL  | ... | ...   | ...                  | ... | bll              | RX J1117.6+2548  |
| J1117.7+0217 | 169.439 | 2.284   | 256.864 | 56.531 | 0.087      | 0.079      | −37    | 6.1      | 0.4      | 0.1             | 4.2      | 0.9             | 2.15          | 0.14                 | PL  | ... | ...   | ...                  | ... | ...              | ...              |
| J1117.7–4632 | 169.449 | −46.542 | 286.621 | 13.343 | 0.132      | 0.090      | −56    | 7.5      | 0.6      | 0.1             | 8.2      | 1.2             | 2.43          | 0.09                 | PL  | ... | ...   | 2FGL J1118.1–4629    | ... | fsrq             | PKS 1116–46      |
| J1117.9+5355 | 169.497 | 53.929  | 149.209 | 58.170 | 0.035      | 0.032      | 38     | 16.2     | 0.7      | 0.1             | 8.1      | 0.9             | 1.93          | 0.08                 | PL  | ... | ...   | 1FHL J1117.7+5355    | ... | bll              | NVSS             |
|              |         |         |         |        |            |            |        |          |          |                 |          |                 |               |                      |     |     |       |                      |     | J111757+535553   |                  |
|              |         |         |         |        |            |            |        |          |          |                 |          |                 |               |                      |     |     |       | 2FGL J1118.0+5354    |     |                  |                  |
|              |         |         |         |        |            |            |        |          |          |                 |          |                 |               |                      |     |     |       | 1FGL J1118.0+5354    |     |                  |                  |
| J1118.2–0411 | 169.572 | −4.199  | 263.699 | 51.435 | 0.132      | 0.119      | 20     | 11.7     | 0.7      | 0.1             | 11.4     | 1.1             | 2.57          | 0.08                 | PL  | T   | ...   | ...                  | ... | agn              | PMN J1118–0413   |
| J1119.1–6127 | 169.794 | −61.466 | 292.146 | −0.542 | 0.029      | 0.027      | −86    | 27.0     | 6.7      | 0.3             | 84.9     | 3.8             | 2.36          | 0.03                 | PL  | ... | ...   | 2FGL J1118.8–6128    | E   | PSR              | PSR J1119.1–6127 |
|              |         |         |         |        |            |            |        |          |          |                 |          |                 |               |                      |     |     |       | 1FGL J1119.4–6127c   |     |                  |                  |
| J1119.7–3046 | 169.937 | −30.778 | 280.641 | 28.095 | 0.090      | 0.078      | −85    | 4.5      | 0.1      | 0.1             | 2.5      | 0.9             | 1.54          | 0.23                 | PL  | ... | ...   | 1FGL J1119.5–3044    | ... | bll              | 1RXS             |
|              |         |         |         |        |            |            |        |          |          |                 |          |                 |               |                      |     |     |       |                      |     | J111941.0–304652 |                  |
| J1119.8–2647 | 169.971 | −26.790 | 278.832 | 31.761 | 0.080      | 0.073      | −33    | 5.6      | 0.3      | 0.1             | 3.4      | 0.9             | 1.83          | 0.20                 | PL  | ... | ...   | ...                  | ... | ...              | ...              |
| J1119.9–2204 | 169.984 | −22.067 | 276.470 | 36.059 | 0.042      | 0.039      | 89     | 30.2     | 2.7      | 0.2             | 16.8     | 1.0             | 2.18          | ...                  | LP  | ... | ...   | 2FGL J1120.0–2204    | ... | ...              | ...              |
|              |         |         |         |        |            |            |        |          |          |                 |          |                 |               |                      |     |     |       | 1FGL J1119.9–2205    |     |                  |                  |
| J1120.6+0713 | 170.172 | 7.223   | 251.532 | 60.685 | 0.073      | 0.068      | 82     | 13.2     | 1.1      | 0.1             | 6.1      | 0.8             | 2.12          | ...                  | LP  | ... | ...   | 2FGL J1120.4+0710    | ... | ...              | ...              |
|              |         |         |         |        |            |            |        |          |          |                 |          |                 |               |                      |     |     |       | 1FGL J1120.4+0710    |     |                  |                  |
| J1120.8+4212 | 170.210 | 42.205  | 167.841 | 66.168 | 0.026      | 0.024      | 7      | 23.5     | 1.2      | 0.1             | 17.3     | 1.8             | 1.62          | 0.06                 | PL  | ... | ...   | 1FHL J1120.9+4211    | ... | bll              | RBS 0970         |
|              |         |         |         |        |            |            |        |          |          |                 |          |                 |               |                      |     |     |       | 2FGL J1121.0+4211    |     |                  |                  |
|              |         |         |         |        |            |            |        |          |          |                 |          |                 |               |                      |     |     |       | 1FGL J1121.0+4209    |     |                  |                  |
| J1121.4–0554 | 170.367 | −5.902  | 266.235 | 50.448 | 0.038      | 0.036      | 65     | 29.3     | 2.2      | 0.1             | 28.5     | 1.4             | 2.37          | 0.04                 | PL  | T   | ...   | 2FGL J1121.5–0554    | ... | fsrq             | PKS 1118–05      |
|              |         |         |         |        |            |            |        |          |          |                 |          |                 |               |                      |     |     |       | 1FGL J1121.5–0554    |     |                  |                  |
| J1123.2–6415 | 170.808 | −64.261 | 293.536 | −3.010 | 0.084      | 0.073      | 54     | 14.0     | 1.3      | 0.4             | 26.3     | 2.1             | 2.61          | ...                  | LP  | T   | ...   | 1FGL J1122.9–6415    | ... | bcu              | AT20G            |
|              |         |         |         |        |            |            |        |          |          |                 |          |                 |               |                      |     |     |       |                      |     | J112319–641735   |                  |
|              |         |         |         |        |            |            |        |          |          |                 |          |                 |               |                      |     |     |       | 0FGL J1123.0–6416    |     |                  |                  |
| J1123.3–2529 | 170.841 | −25.494 | 279.060 | 33.262 | 0.147      | 0.113      | 61     | 5.9      | 0.4      | 0.1             | 4.6      | 0.9             | 2.29          | 0.14                 | PL  | ... | ...   | 2FGL J1123.3–2527    | ... | ...              | ...              |
|              |         |         |         |        |            |            |        |          |          |                 |          |                 |               |                      |     |     |       | 1FGL J1123.6–2528    |     |                  |                  |
| J1123.6+7231 | 170.900 | 72.525  | 131.773 | 43.063 | 0.070      | 0.068      | −87    | 4.7      | 0.1      | 0.1             | 1.7      | 0.6             | 1.59          | 0.35                 | PL  | ... | ...   | ...                  | ... | bll              | RX J1123.8+7230  |
| J1123.6–4558 | 170.915 | −45.968 | 287.388 | 14.237 | 0.227      | 0.113      | 6      | 4.1      | 0.4      | 0.1             | 4.2      | 1.0             | 2.19          | 0.14                 | PL  | ... | 9     | 1FGL J1123.6–4555    | ... | ...              | ...              |
| J1123.9–3653 | 170.990 | −36.891 | 284.084 | 22.759 | 0.040      | 0.037      | 83     | 21.7     | 2.2      | 0.2             | 13.2     | 1.1             | 2.07          | ...                  | EC  | ... | ...   | 2FGL J1124.2–3654    | ... | PSR              | PSR J1124–3653   |
|              |         |         |         |        |            |            |        |          |          |                 |          |                 |               |                      |     |     |       | 1FGL J1124.4–3654    |     |                  |                  |

Table 1—Continued

| Name 3FGL    | R.A.    | Decl.   | $l$     | $b$     | $\theta_1$ | $\theta_2$ | $\phi$ | $\sigma$ | $F_{35}$ | $\Delta F_{35}$ | $S_{25}$ | $\Delta S_{25}$ | $\Gamma_{25}$ | $\Delta \Gamma_{25}$ | Mod | Var | Flags | $\gamma$ -ray Assoc.                                        | TeV | Class | ID or Assoc.             |
|--------------|---------|---------|---------|---------|------------|------------|--------|----------|----------|-----------------|----------|-----------------|---------------|----------------------|-----|-----|-------|-------------------------------------------------------------|-----|-------|--------------------------|
| J1124.1+2337 | 171.037 | 23.628  | 218.152 | 70.002  | 0.087      | 0.084      | 29     | 9.7      | 0.5      | 0.1             | 6.7      | 0.8             | 2.46          | 0.10                 | PL  | ... | ...   | 2FGL J1124.2+2338<br>1FGL J1123.9+2339                      | ... | fsrq  | OM 235                   |
| J1124.5−5915 | 171.128 | −59.254 | 292.016 | 1.763   | 0.029      | 0.027      | 53     | 35.1     | 6.8      | 0.3             | 61.3     | 3.1             | 2.36          | ...                  | EC  | ... | ...   | 2FGL J1124.6−5913<br>1FGL J1124.6−5916                      | ... | PSR   | PSR J1124−5916           |
| J1124.9+4932 | 171.248 | 49.544  | 153.656 | 62.110  | 0.053      | 0.049      | −19    | 7.8      | 0.3      | 0.1             | 3.5      | 0.7             | 1.80          | 0.15                 | PL  | ... | ...   | 2FGL J1125.2+4933                                           | ... | bll   | GB6 J1124+4933           |
| J1125.0−2101 | 171.255 | −21.022 | 277.259 | 37.504  | 0.067      | 0.051      | 15     | 8.4      | 0.4      | 0.1             | 5.3      | 1.1             | 1.78          | 0.14                 | PL  | ... | ...   | ...                                                         | ... | bcb   | PMN J1125−2100           |
| J1125.1−5803 | 171.295 | −58.064 | 291.707 | 2.916   | 0.080      | 0.059      | −35    | 4.6      | 0.4      | 0.2             | 4.9      | 1.5             | 1.88          | 0.24                 | PL  | ... | ...   | ...                                                         | ... | ...   | ...                      |
| J1125.3−5824 | 171.342 | −58.406 | 291.842 | 2.601   | 0.070      | 0.060      | −20    | 6.6      | 1.1      | 0.2             | 14.5     | 2.7             | 2.39          | 0.11                 | PL  | ... | ...   | 2FGL J1125.0−5821                                           | ... | PSR   | PSR J1125−5825           |
| J1125.5−3558 | 171.382 | −35.970 | 284.046 | 23.731  | 0.052      | 0.043      | 76     | 12.8     | 0.9      | 0.1             | 10.3     | 1.3             | 1.88          | 0.09                 | PL  | T   | ...   | 1FHL J1125.9−3557<br>2FGL J1125.6−3559<br>1FGL J1125.5−3559 | ... | bll   | PMN J1125−3556           |
| J1125.6−6012 | 171.403 | −60.209 | 292.460 | 0.906   | 0.064      | 0.055      | −90    | 5.6      | 0.9      | 0.2             | 11.8     | 2.5             | 2.37          | 0.11                 | PL  | ... | ...   | ...                                                         | ... | psr   | PSR J1125−6014           |
| J1125.8−0745 | 171.472 | −7.752  | 269.181 | 49.431  | 0.107      | 0.100      | −81    | 5.1      | 0.3      | 0.1             | 3.3      | 0.8             | 1.95          | 0.18                 | PL  | ... | 1     | 2FGL J1126.0−0743                                           | ... | bll   | 1RXS<br>J112551.6−074219 |
| J1125.9+2007 | 171.478 | 20.131  | 228.031 | 69.235  | 0.139      | 0.115      | −75    | 5.1      | 0.3      | 0.1             | 3.4      | 0.7             | 2.31          | 0.15                 | PL  | ... | ...   | 1FGL J1126.0−0741                                           | ... | fsrq  | 4C +20.25                |
| J1126.7−3834 | 171.689 | −38.572 | 285.281 | 21.380  | 0.093      | 0.088      | 8      | 6.4      | 0.4      | 0.1             | 5.2      | 0.9             | 2.26          | 0.12                 | PL  | ... | ...   | ...                                                         | ... | bcb   | PKS 1124−382             |
| J1126.8−5001 | 171.725 | −50.024 | 289.301 | 10.597  | 0.163      | 0.149      | 73     | 7.1      | 0.5      | 0.1             | 7.4      | 1.1             | 2.43          | 0.11                 | PL  | ... | ...   | ...                                                         | ... | ...   | ...                      |
| J1127.0−1857 | 171.763 | −18.956 | 276.720 | 39.582  | 0.020      | 0.019      | 77     | 76.3     | 7.3      | 0.2             | 74.4     | 2.1             | 2.24          | ...                  | LP  | T   | ...   | 1FGL J1126.8−1854<br>1FHL J1127.1−1855<br>2FGL J1126.6−1856 | ... | fsrq  | PKS 1124−186             |
| J1127.8+3618 | 171.962 | 36.308  | 180.349 | 70.054  | 0.060      | 0.056      | −44    | 14.5     | 0.9      | 0.1             | 11.2     | 1.0             | 2.35          | 0.07                 | PL  | T   | ...   | 2FGL J1127.6+3622                                           | ... | fsrq  | MG2 J112758+3620         |
| J1128.0+5921 | 172.003 | 59.351  | 141.243 | 54.712  | 0.193      | 0.162      | 33     | 4.8      | 0.2      | 0.0             | 3.4      | 0.7             | 2.72          | 0.17                 | PL  | ... | ...   | ...                                                         | ... | fsrq  | TXS 1125+596             |
| J1128.6−5434 | 172.161 | −54.579 | 291.037 | 6.369   | 0.358      | 0.258      | −4     | 8.5      | 0.1      | 0.1             | 9.4      | 1.3             | 2.85          | ...                  | LP  | ... | 1,3   | ...                                                         | ... | ...   | ...                      |
| J1128.7−6232 | 172.194 | −62.535 | 293.563 | −1.177  | 0.229      | 0.170      | 40     | 8.6      | 2.4      | 0.4             | 18.2     | 2.5             | 2.32          | ...                  | LP  | ... | 3,4   | 1FGL J1127.7−6244c                                          | ... | ...   | ...                      |
| J1129.0+3758 | 172.253 | 37.972  | 175.663 | 69.596  | 0.062      | 0.057      | 69     | 10.3     | 0.7      | 0.1             | 8.4      | 1.2             | 2.29          | 0.10                 | PL  | ... | ...   | 2FGL J1129.5+3758<br>1FGL J1129.3+3757                      | ... | ...   | ...                      |
| J1129.0+3705 | 172.271 | 37.095  | 177.945 | 69.980  | 0.060      | 0.053      | −43    | 8.7      | 0.5      | 0.1             | 5.1      | 0.9             | 2.08          | 0.13                 | PL  | T   | ...   | ...                                                         | ... | bll   | MG2 J112910+3702         |
| J1129.4−4215 | 172.358 | −42.262 | 287.110 | 18.076  | 0.135      | 0.122      | 74     | 5.6      | 0.3      | 0.1             | 5.0      | 0.9             | 2.48          | 0.13                 | PL  | ... | 1     | ...                                                         | ... | bcb   | SUMSS<br>J113006−421441  |
| J1129.9−1446 | 172.499 | −14.774 | 275.215 | 43.671  | 0.082      | 0.079      | −75    | 22.1     | 0.9      | 0.1             | 19.8     | 1.0             | 2.79          | 0.05                 | PL  | T   | ...   | 2FGL J1130.3−1448<br>1FGL J1130.2−1447<br>0FGL J1129.8−1443 | ... | fsrq  | PKS 1127−14              |
| J1130.7−7800 | 172.682 | −78.010 | 298.661 | −15.813 | 0.074      | 0.064      | 86     | 7.4      | 0.4      | 0.1             | 5.6      | 1.1             | 1.74          | 0.14                 | PL  | ... | ...   | 1FHL J1129.2−7759                                           | ... | ...   | ...                      |
| J1131.1+5810 | 172.780 | 58.168  | 141.787 | 55.922  | 0.063      | 0.063      | −19    | 10.6     | 0.4      | 0.1             | 5.2      | 0.7             | 2.28          | 0.12                 | PL  | ... | ...   | 1FHL J1130.4+5814                                           | ... | bll   | 1RXS<br>J113117.8+580911 |
| J1131.4+3819 | 172.850 | 38.330  | 174.126 | 69.852  | 0.247      | 0.162      | 35     | 5.5      | 0.4      | 0.1             | 6.0      | 1.1             | 2.57          | 0.12                 | PL  | ... | 5     | 2FGL J1130.9+5809<br>...                                    | ... | fsrq  | B2 1128+38               |



Table 1—Continued

| Name 3FGL    | R.A.    | Decl.   | $l$     | $b$     | $\theta_1$ | $\theta_2$ | $\phi$ | $\sigma$ | $F_{35}$ | $\Delta F_{35}$ | $S_{25}$ | $\Delta S_{25}$ | $\Gamma_{25}$ | $\Delta \Gamma_{25}$ | Mod | Var | Flags | $\gamma$ -ray Assoc.                                                          | TeV | Class | ID or Assoc.             |
|--------------|---------|---------|---------|---------|------------|------------|--------|----------|----------|-----------------|----------|-----------------|---------------|----------------------|-----|-----|-------|-------------------------------------------------------------------------------|-----|-------|--------------------------|
| J1131.9–0503 | 172.999 | –5.056  | 269.139 | 52.525  | 0.113      | 0.091      | 84     | 8.8      | 0.5      | 0.1             | 8.2      | 1.0             | 2.66          | 0.11                 | PL  | ... | 3     | ...                                                                           | ... | bcu   | PKS 1128–047             |
| J1132.0–4736 | 173.012 | –47.602 | 289.335 | 13.163  | 0.081      | 0.067      | 66     | 5.7      | 0.4      | 0.1             | 4.5      | 0.9             | 2.11          | 0.14                 | PL  | ... | 1     | ...                                                                           | ... | ...   | ...                      |
| J1132.7+0034 | 173.186 | 0.575   | 264.247 | 57.413  | 0.036      | 0.034      | –2     | 27.5     | 2.1      | 0.1             | 23.6     | 1.5             | 2.07          | 0.04                 | PL  | ... | ...   | 1FHL J1132.6+0036<br>2FGL J1132.9+0033<br>1FGL J1133.1+0033<br>3EG J1133+0033 | ... | bll   | PKS B1130+008            |
| J1132.8+1015 | 173.211 | 10.258  | 251.527 | 64.955  | 0.533      | 0.492      | 18     | 5.2      | 0.2      | 0.1             | 4.7      | 0.9             | 2.72          | 0.17                 | PL  | ... | 1,9   | ...                                                                           | ... | fsrq  | 4C +10.33                |
| J1135.2–6054 | 173.818 | –60.913 | 293.806 | 0.602   | 0.031      | 0.029      | –34    | 27.8     | 6.0      | 0.3             | 47.4     | 2.6             | 2.30          | ...                  | EC  | ... | ...   | 2FGL J1135.3–6054<br>1FGL J1134.8–6055                                        | ... | PSR   | LAT PSR J1135–6055       |
| J1136.1–7411 | 174.034 | –74.199 | 297.777 | –12.086 | 0.111      | 0.091      | 60     | 10.0     | 0.8      | 0.1             | 11.2     | 1.2             | 2.48          | 0.08                 | PL  | ... | 3     | 2FGL J1134.4–7415                                                             | ... | bcu   | PKS 1133–739             |
| J1136.1+7523 | 174.044 | 75.388  | 129.104 | 40.825  | 0.135      | 0.109      | 54     | 4.3      | 0.2      | 0.0             | 2.3      | 0.6             | 2.30          | 0.23                 | PL  | ... | ...   | ...                                                                           | ... | PSR   | PSR J1137+7528           |
| J1136.4+3405 | 174.110 | 34.098  | 184.954 | 72.459  | 0.129      | 0.109      | –4     | 8.1      | 0.2      | 0.1             | 5.8      | 0.8             | 2.83          | 0.12                 | PL  | ... | ...   | ...                                                                           | ... | fsrq  | MG2 J113627+3408         |
| J1136.6+7009 | 174.153 | 70.152  | 131.894 | 45.652  | 0.024      | 0.020      | –10    | 27.2     | 1.3      | 0.1             | 16.0     | 1.3             | 1.82          | 0.05                 | PL  | ... | ...   | 1FHL J1136.4+7009<br>2FGL J1136.7+7009<br>1FGL J1136.6+7009                   | P   | bll   | Mkn 180                  |
| J1136.6+6736 | 174.157 | 67.608  | 133.443 | 47.964  | 0.035      | 0.034      | 64     | 15.3     | 0.6      | 0.1             | 7.9      | 1.1             | 1.72          | 0.08                 | PL  | ... | ...   | 1FHL J1136.2+6739<br>1FHL J1135.7+6736<br>2FGL J1136.3+6736                   | P   | bll   | RX J1136.2+6737          |
| J1136.6–6826 | 174.173 | –68.438 | 296.126 | –6.560  | 0.112      | 0.099      | –76    | 7.8      | 0.6      | 0.1             | 12.1     | 1.6             | 2.71          | 0.11                 | PL  | ... | ...   | 2FGL J1135.2–6829                                                             | ... | bcu   | PKS 1133–681             |
| J1136.9+2551 | 174.235 | 25.861  | 213.056 | 73.299  | 0.056      | 0.043      | 70     | 7.1      | 0.2      | 0.1             | 3.4      | 0.9             | 1.68          | 0.22                 | PL  | ... | ...   | 1FHL J1137.0+2553<br>2FGL J1137.0+2553<br>1FGL J1136.9+2551                   | ... | bll   | RX J1136.8+2551          |
| J1138.2+4905 | 174.553 | 49.099  | 150.783 | 63.881  | 0.232      | 0.182      | 73     | 5.4      | 0.1      | 0.0             | 3.7      | 0.7             | 2.85          | 0.18                 | PL  | ... | ...   | ...                                                                           | ... | bcu   | GB6 J1138+4858           |
| J1139.0–6244 | 174.751 | –62.737 | 294.746 | –1.022  | 0.053      | 0.041      | –55    | 12.2     | 2.7      | 0.3             | 32.6     | 3.0             | 2.27          | 0.06                 | PL  | ... | 3     | 2FGL J1138.8–6233c                                                            | ... | ...   | ...                      |
| J1140.4+1529 | 175.100 | 15.498  | 244.510 | 69.818  | 0.058      | 0.053      | 23     | 5.2      | 0.1      | 0.1             | 2.7      | 1.0             | 1.26          | 0.28                 | PL  | ... | ...   | ...                                                                           | ... | bll   | NVSS<br>J114023+152808   |
| J1141.2+6805 | 175.324 | 68.099  | 132.545 | 47.699  | 0.067      | 0.050      | 60     | 7.1      | 0.2      | 0.0             | 2.9      | 0.7             | 1.61          | 0.16                 | PL  | ... | ...   | 2FGL J1141.0+6803                                                             | ... | bcu   | 1RXS<br>J114118.3+680433 |
| J1141.6–1406 | 175.423 | –14.116 | 278.477 | 45.418  | 0.108      | 0.070      | 57     | 7.6      | 0.5      | 0.1             | 5.3      | 0.9             | 2.18          | 0.13                 | PL  | ... | ...   | 2FGL J1141.7–1404                                                             | ... | bcu   | 1RXS<br>J114142.2–140757 |
| J1142.0+1546 | 175.501 | 15.782  | 244.552 | 70.297  | 0.054      | 0.051      | 37     | 10.2     | 0.7      | 0.1             | 8.4      | 0.9             | 2.30          | 0.09                 | PL  | ... | ...   | 1FGL J1141.8–1403<br>2FGL J1141.9+1550<br>1FGL J1141.8+1549                   | ... | bll   | MG1 J114208+1547         |
| J1142.1–6941 | 175.532 | –69.685 | 296.944 | –7.623  | 0.153      | 0.132      | –43    | 4.3      | 0.4      | 0.1             | 6.6      | 1.5             | 2.66          | 0.16                 | PL  | ... | ...   | ...                                                                           | ... | ...   | ...                      |
| J1142.9+0120 | 175.742 | 1.349   | 267.576 | 59.437  | 0.058      | 0.052      | 13     | 13.7     | 1.0      | 0.1             | 6.2      | 0.8             | 1.95          | ...                  | EC  | ... | ...   | 2FGL J1142.9+0121<br>1FGL J1142.7+0127                                        | ... | PSR   | PSR J1142+0119           |
| J1143.0+6123 | 175.774 | 61.384  | 136.740 | 53.874  | 0.045      | 0.040      | 62     | 17.1     | 0.9      | 0.1             | 9.5      | 0.9             | 2.02          | 0.07                 | PL  | ... | ...   | 2FGL J1143.1+6119                                                             | ... | bll   | 87GB<br>114026.7+613850  |
| J1145.1+1935 | 176.287 | 19.594  | 235.789 | 73.046  | 0.087      | 0.077      | 69     | 5.7      | 0.3      | 0.1             | 3.0      | 0.7             | 1.98          | 0.20                 | PL  | ... | ...   | ...                                                                           | ... | rdg   | 3C 264                   |

Table 1—Continued

| Name 3FGL    | R.A.    | Decl.   | $l$     | $b$    | $\theta_1$ | $\theta_2$ | $\phi$ | $\sigma$ | $F_{35}$ | $\Delta F_{35}$ | $S_{25}$ | $\Delta S_{25}$ | $\Gamma_{25}$ | $\Delta \Gamma_{25}$ | Mod | Var | Flags  | $\gamma$ -ray Assoc.                                        | TeV | Class | ID or Assoc.             |
|--------------|---------|---------|---------|--------|------------|------------|--------|----------|----------|-----------------|----------|-----------------|---------------|----------------------|-----|-----|--------|-------------------------------------------------------------|-----|-------|--------------------------|
| J1145.8+4425 | 176.462 | 44.421  | 155.931 | 68.271 | 0.149      | 0.106      | −48    | 4.1      | 0.2      | 0.1             | 2.1      | 0.7             | 1.85          | 0.20                 | PL  | ... | ...    | ...                                                         | ... | fsrq  | B3 1143+446A             |
| J1146.1−0640 | 176.547 | −6.683  | 275.534 | 52.683 | 0.096      | 0.076      | −24    | 6.0      | 0.3      | 0.1             | 3.9      | 0.9             | 1.92          | 0.17                 | PL  | ... | ...    | ...                                                         | ... | ...   | ...                      |
| J1146.8+3958 | 176.724 | 39.970  | 164.995 | 71.464 | 0.027      | 0.026      | −17    | 48.7     | 3.3      | 0.1             | 41.1     | 1.3             | 2.32          | 0.03                 | PL  | T   | ...    | 1FHL J1146.9+3958<br>2FGL J1146.9+4000<br>1FGL J1146.8+4004 | ... | fsrq  | S4 1144+40               |
| J1147.0−3811 | 176.764 | −38.185 | 289.242 | 22.970 | 0.042      | 0.040      | −48    | 22.4     | 1.7      | 0.1             | 19.7     | 1.2             | 2.25          | 0.05                 | PL  | T   | ...    | 2FGL J1146.8−3812<br>1FGL J1146.9−3812<br>0FGL J1146.7−3808 | ... | fsrq  | PKS 1144−379             |
| J1147.8−0725 | 176.961 | −7.425  | 276.643 | 52.170 | 0.050      | 0.041      | −61    | 18.0     | 1.4      | 0.1             | 17.1     | 1.3             | 2.32          | 0.06                 | PL  | T   | ...    | 2FGL J1147.7−0724<br>1FGL J1147.7−0722                      | ... | fsrq  | PKS 1145−071             |
| J1149.1+2815 | 177.295 | 28.251  | 204.670 | 76.182 | 0.145      | 0.120      | −16    | 5.0      | 0.2      | 0.1             | 3.8      | 0.8             | 2.58          | 0.20                 | PL  | ... | ...    | ...                                                         | ... | ...   | ...                      |
| J1149.5+2443 | 177.376 | 24.722  | 219.275 | 75.878 | 0.156      | 0.106      | 24     | 4.2      | 0.3      | 0.1             | 3.7      | 1.1             | 2.11          | 0.22                 | PL  | ... | 5      | ...                                                         | ... | bll   | RX J1149.5+2439          |
| J1150.3+2417 | 177.599 | 24.295  | 221.181 | 75.971 | 0.043      | 0.042      | 32     | 16.4     | 1.4      | 0.1             | 16.0     | 1.4             | 2.21          | 0.06                 | PL  | ... | ...    | 1FHL J1150.8+2419<br>2FGL J1150.1+2419<br>1FGL J1150.2+2419 | ... | bll   | OM 280                   |
| J1150.5+4155 | 177.635 | 41.920  | 159.109 | 70.669 | 0.022      | 0.021      | −15    | 34.0     | 2.2      | 0.1             | 27.6     | 2.0             | 1.76          | 0.04                 | PL  | ... | ...    | 1FHL J1150.5+4155<br>2FGL J1150.5+4154<br>1FGL J1150.5+4152 | ... | bll   | RBS 1040                 |
| J1150.7−4816 | 177.692 | −48.283 | 292.623 | 13.371 | 0.085      | 0.080      | −26    | 4.3      | 0.3      | 0.1             | 3.6      | 0.9             | 2.33          | 0.15                 | PL  | ... | ...    | ...                                                         | ... | ...   | ...                      |
| J1151.4−1346 | 177.855 | −13.783 | 281.477 | 46.573 | 0.062      | 0.054      | 45     | 7.2      | 0.4      | 0.1             | 4.4      | 0.9             | 1.98          | 0.17                 | PL  | ... | ...    | 2FGL J1151.5−1347<br>1FGL J1151.4−1345                      | ... | bll   | PMN J1151−1347           |
| J1151.4+5858 | 177.861 | 58.981  | 136.911 | 56.490 | 0.028      | 0.027      | −9     | 17.5     | 0.8      | 0.1             | 9.2      | 1.0             | 1.92          | 0.08                 | PL  | ... | ...    | 1FHL J1151.5+5857<br>2FGL J1151.5+5857<br>1FGL J1151.6+5857 | ... | bll   | TXS 1148+592             |
| J1151.5+0957 | 177.884 | 9.965   | 260.648 | 67.774 | 0.218      | 0.152      | −84    | 4.2      | 0.3      | 0.1             | 3.1      | 0.8             | 2.22          | 0.21                 | PL  | ... | ...    | ...                                                         | ... | ...   | ...                      |
| J1151.8−6108 | 177.955 | −61.144 | 295.801 | 0.900  | 0.105      | 0.094      | 60     | 6.1      | 1.0      | 0.2             | 13.4     | 2.2             | 2.43          | 0.11                 | PL  | ... | 1,3,10 | ...                                                         | ... | ...   | ...                      |
| J1152.3−0841 | 178.084 | −8.692  | 279.086 | 51.422 | 0.069      | 0.067      | 22     | 13.0     | 0.9      | 0.1             | 11.9     | 1.1             | 2.44          | 0.08                 | PL  | T   | ...    | 2FGL J1152.4−0840<br>1FGL J1152.2−0836                      | ... | fsrq  | PKS B1149−084            |
| J1153.4+4932 | 178.350 | 49.536  | 145.530 | 64.969 | 0.033      | 0.033      | 55     | 42.5     | 2.3      | 0.1             | 29.2     | 1.0             | 2.38          | 0.03                 | PL  | T   | ...    | 2FGL J1153.2+4935                                           | ... | FSRQ  | OM 484                   |
| J1153.4+4033 | 178.361 | 40.557  | 160.953 | 72.013 | 0.136      | 0.082      | 62     | 5.8      | 0.3      | 0.1             | 3.2      | 0.8             | 1.77          | 0.16                 | PL  | ... | ...    | ...                                                         | ... | fsrq  | B3 1151+408              |
| J1153.7−2555 | 178.430 | −25.930 | 287.025 | 35.153 | 0.082      | 0.072      | −8     | 4.2      | 0.2      | 0.1             | 2.7      | 0.8             | 2.01          | 0.19                 | PL  | ... | ...    | ...                                                         | ... | bcu   | PMN J1153−2553           |
| J1154.0−3243 | 178.512 | −32.723 | 289.195 | 28.613 | 0.041      | 0.037      | 3      | 16.2     | 1.2      | 0.1             | 13.1     | 1.2             | 2.05          | 0.06                 | PL  | ... | ...    | 2FGL J1154.1−3242<br>1FGL J1154.2−3242                      | ... | bcu   | PKS 1151−324             |
| J1154.2−0010 | 178.553 | −0.178  | 273.869 | 59.426 | 0.052      | 0.050      | 72     | 9.4      | 0.4      | 0.1             | 5.9      | 1.2             | 1.68          | 0.15                 | PL  | ... | ...    | 1FHL J1154.0−0010<br>2FGL J1154.0−0010                      | ... | bll   | 1RXS<br>J115404.9−001008 |

Table 1—Continued

| Name 3FGL    | R.A.    | Decl.   | $l$     | $b$    | $\theta_1$ | $\theta_2$ | $\phi$ | $\sigma$ | $F_{35}$ | $\Delta F_{35}$ | $S_{25}$ | $\Delta S_{25}$ | $\Gamma_{25}$ | $\Delta \Gamma_{25}$ | Mod | Var | Flags | $\gamma$ -ray Assoc.                                                                               | TeV | Class | ID or Assoc.                |
|--------------|---------|---------|---------|--------|------------|------------|--------|----------|----------|-----------------|----------|-----------------|---------------|----------------------|-----|-----|-------|----------------------------------------------------------------------------------------------------|-----|-------|-----------------------------|
| J1154.3+6023 | 178.590 | 60.387  | 135.302 | 55.349 | 0.116      | 0.093      | 43     | 10.4     | 0.4      | 0.1             | 8.0      | 0.9             | 2.66          | 0.09                 | PL  | T   | ...   | 1FGL J1154.0–0008<br>2FGL J1154.4+6019<br>1FGL J1152.1+6027                                        | ... | fsrq  | RX J1154.0+6022             |
| J1155.3–1112 | 178.827 | –11.203 | 281.530 | 49.322 | 0.051      | 0.048      | 39     | 5.4      | 0.2      | 0.1             | 2.9      | 1.0             | 1.53          | 0.20                 | PL  | ... | ...   | ...                                                                                                | ... | ...   | ...                         |
| J1155.4–3417 | 178.862 | –34.299 | 289.955 | 27.158 | 0.044      | 0.041      | –34    | 6.2      | 0.1      | 0.1             | 3.0      | 1.0             | 1.34          | 0.22                 | PL  | ... | ...   | ...                                                                                                | ... | bcu   | NVSS<br>J115520–341718      |
| J1155.9+6136 | 178.975 | 61.603  | 134.208 | 54.293 | 0.139      | 0.100      | –74    | 4.5      | 0.2      | 0.0             | 2.3      | 0.7             | 1.65          | 0.19                 | PL  | ... | ...   | ...                                                                                                | ... | bll   | SDSS<br>J115548.40+613553.8 |
| J1156.7–2250 | 179.181 | –22.847 | 286.809 | 38.306 | 0.066      | 0.060      | 69     | 6.0      | 0.3      | 0.1             | 4.0      | 1.0             | 1.89          | 0.17                 | PL  | ... | ...   | ...                                                                                                | ... | bcu   | NVSS<br>J115633–225004      |
| J1158.8+0941 | 179.719 | 9.687   | 265.042 | 68.600 | 0.111      | 0.072      | –2     | 10.5     | 0.7      | 0.1             | 7.8      | 1.0             | 2.04          | 0.10                 | PL  | ... | ...   | 2FGL J1158.8+0939                                                                                  | ... | bll   | GB6 J1158+0937              |
| J1158.9+0818 | 179.733 | 8.313   | 267.059 | 67.451 | 0.064      | 0.061      | –48    | 5.4      | 0.2      | 0.1             | 2.7      | 0.7             | 1.87          | 0.20                 | PL  | ... | ...   | ...                                                                                                | ... | bcu   | RX J1158.8+0819             |
| J1159.2–2141 | 179.825 | –21.684 | 287.153 | 39.584 | 0.056      | 0.051      | 20     | 14.7     | 1.3      | 0.1             | 16.0     | 1.5             | 2.36          | 0.07                 | PL  | T   | ...   | 2FGL J1159.3–2142                                                                                  | ... | fsrq  | PMN J1159–2142              |
| J1159.3–2226 | 179.826 | –22.440 | 287.407 | 38.855 | 0.049      | 0.046      | –65    | 17.9     | 1.7      | 0.1             | 22.4     | 1.7             | 2.37          | 0.05                 | PL  | T   | ...   | 2FGL J1159.0–2226                                                                                  | ... | bcu   | PKS 1156–221                |
| J1159.5+2914 | 179.882 | 29.238  | 199.453 | 78.375 | 0.017      | 0.016      | –60    | 93.4     | 8.4      | 0.2             | 83.4     | 2.2             | 2.21          | ...                  | LP  | T   | ...   | 1FHL J1159.6+2913<br>2FGL J1159.5+2914<br>1FGL J1159.4+2914<br>0FGL J1159.2+2912<br>3EG J1200+2847 | ... | fsrq  | Ton 599 –<br>67 –           |
| J1159.6–0723 | 179.906 | –7.392  | 281.112 | 53.270 | 0.071      | 0.068      | –63    | 8.4      | 0.5      | 0.1             | 6.1      | 1.0             | 2.10          | 0.13                 | PL  | ... | ...   | ...                                                                                                | ... | bcu   | PMN J1159–0723              |
| J1200.4+0202 | 180.111 | 2.042   | 274.817 | 62.097 | 0.068      | 0.064      | –7     | 8.8      | 0.5      | 0.1             | 5.7      | 0.9             | 2.04          | 0.12                 | PL  | ... | ...   | 2FGL J1200.0+0159<br>1FGL J1159.8+0200                                                             | ... | ...   | ...                         |
| J1200.8+1228 | 180.221 | 12.476  | 261.514 | 71.160 | 0.082      | 0.072      | 8      | 7.3      | 0.4      | 0.1             | 4.8      | 0.8             | 2.25          | 0.13                 | PL  | ... | ...   | ...                                                                                                | ... | bcu   | GB6 J1200+1230              |
| J1200.9–1432 | 180.243 | –14.539 | 285.021 | 46.570 | 0.108      | 0.089      | 54     | 4.7      | 0.3      | 0.1             | 3.8      | 0.9             | 2.25          | 0.22                 | PL  | ... | ...   | ...                                                                                                | ... | ...   | ...                         |
| J1200.9+2010 | 180.244 | 20.180  | 241.289 | 76.530 | 0.127      | 0.104      | –37    | 6.8      | 0.3      | 0.1             | 5.1      | 0.8             | 2.52          | 0.13                 | PL  | ... | ...   | ...                                                                                                | ... | bcu   | TXS 1158+204                |
| J1203.1+6029 | 180.799 | 60.498  | 133.436 | 55.636 | 0.054      | 0.047      | 89     | 15.6     | 0.8      | 0.1             | 8.9      | 0.8             | 2.21          | 0.08                 | PL  | ... | ...   | 1FHL J1203.2+6028<br>2FGL J1203.2+6030<br>1FGL J1202.9+6032                                        | ... | bll   | SBS 1200+608                |
| J1203.2+3847 | 180.805 | 38.790  | 160.715 | 74.593 | 0.122      | 0.107      | 57     | 4.8      | 0.2      | 0.1             | 2.9      | 0.7             | 2.43          | 0.18                 | PL  | ... | ...   | ...                                                                                                | ... | bll   | NVSS<br>J120257+385147      |
| J1203.5–3925 | 180.882 | –39.425 | 292.939 | 22.515 | 0.046      | 0.045      | –65    | 7.3      | 0.3      | 0.1             | 4.2      | 1.0             | 1.64          | 0.15                 | PL  | ... | ...   | ...                                                                                                | ... | bcu   | PMN J1203–3926              |
| J1203.9–1745 | 180.979 | –17.762 | 287.210 | 43.655 | 0.114      | 0.097      | 79     | 5.1      | 0.3      | 0.1             | 3.7      | 0.8             | 2.17          | 0.15                 | PL  | ... | ...   | ...                                                                                                | ... | ...   | ...                         |
| J1203.9–6243 | 180.996 | –62.727 | 297.527 | –0.354 | 0.050      | 0.045      | –74    | 14.8     | 4.8      | 0.4             | 43.6     | 4.3             | 2.41          | ...                  | LP  | ... | 5     | 2FGL J1203.6–6243c                                                                                 | ... | psr   | PSR J1203–63                |
| J1204.0+1144 | 181.012 | 11.739  | 264.780 | 71.011 | 0.072      | 0.067      | –12    | 8.3      | 0.5      | 0.1             | 5.5      | 1.0             | 1.88          | 0.13                 | PL  | ... | ...   | 2FGL J1204.2+1144                                                                                  | ... | bll   | 1RXS<br>J120413.0+114549    |
| J1204.3–0708 | 181.094 | –7.141  | 282.857 | 53.886 | 0.040      | 0.039      | 10     | 15.8     | 1.0      | 0.1             | 12.4     | 1.4             | 1.86          | 0.08                 | PL  | ... | ...   | 1FGL J1204.4+1139<br>1FHL J1204.4–0708                                                             | ... | bll   | 1RXS<br>J120417.0–070959    |
| J1205.4+0412 | 181.374 | 4.213   | 275.358 | 64.597 | 0.249      | 0.201      | 84     | 5.0      | 0.2      | 0.1             | 4.3      | 0.8             | 2.64          | 0.16                 | PL  | ... | ...   | 2FGL J1204.3–0711<br>1FGL J1204.3–0714                                                             | ... | fsrq  | MG1 J120448+0408            |

Table 1—Continued

| Name 3FGL     | R.A.    | Decl.   | $l$     | $b$     | $\theta_1$ | $\theta_2$ | $\phi$ | $\sigma$ | $F_{35}$ | $\Delta F_{35}$ | $S_{25}$ | $\Delta S_{25}$ | $\Gamma_{25}$ | $\Delta \Gamma_{25}$ | Mod | Var | Flags | $\gamma$ -ray Assoc.                    | TeV | Class | ID or Assoc.                |
|---------------|---------|---------|---------|---------|------------|------------|--------|----------|----------|-----------------|----------|-----------------|---------------|----------------------|-----|-----|-------|-----------------------------------------|-----|-------|-----------------------------|
| J1205.8–2636  | 181.464 | –26.602 | 290.453 | 35.162  | 0.076      | 0.070      | –32    | 11.6     | 0.8      | 0.1             | 11.7     | 1.2             | 2.54          | 0.08                 | PL  | T   | …     | 2FGL J1206.0–2638<br>1FGL J1205.9–2637  | …   | fsrq  | PKS 1203–26                 |
| J1205.9+3315  | 181.483 | 33.255  | 178.232 | 78.426  | 0.134      | 0.109      | –59    | 4.9      | 0.2      | 0.1             | 3.6      | 0.8             | 2.71          | 0.19                 | PL  | …   | …     | …                                       | …   | …     | …                           |
| J1206.4–7123  | 181.624 | –71.397 | 299.326 | –8.841  | 0.250      | 0.188      | –83    | 6.7      | 0.4      | 0.1             | 8.3      | 1.2             | 2.68          | 0.11                 | PL  | …   | 1,4   | …                                       | …   | …     | …                           |
| J1207.2–5052  | 181.824 | –50.870 | 295.854 | 11.394  | 0.099      | 0.090      | 29     | 7.7      | 0.7      | 0.1             | 7.9      | 1.2             | 2.14          | 0.10                 | PL  | …   | …     | 2FGL J1207.3–5055<br>1FGL J1207.0–5055  | …   | psr   | PSR J1207–5050              |
| J1207.6–4537  | 181.913 | –45.628 | 294.969 | 16.566  | 0.157      | 0.130      | 9      | 4.6      | 0.4      | 0.1             | 4.2      | 0.9             | 2.11          | 0.13                 | PL  | …   | …     | …                                       | …   | bcu   | PMN J1207–4531              |
| J1207.6–2232  | 181.920 | –22.540 | 289.858 | 39.218  | 0.141      | 0.124      | –77    | 6.7      | 0.4      | 0.1             | 6.8      | 1.1             | 2.57          | 0.12                 | PL  | …   | …     | …                                       | …   | bcu   | NVSS<br>J120738–223250      |
| J1208.0–6901  | 182.010 | –69.026 | 299.044 | –6.482  | 0.146      | 0.113      | –76    | 6.0      | 0.5      | 0.1             | 7.5      | 1.3             | 2.48          | 0.11                 | PL  | …   | 1     | …                                       | …   | …     | …                           |
| J1208.2–7810c | 182.074 | –78.168 | 300.651 | –15.488 | 0.077      | 0.076      | –1     | 4.9      | 0.4      | 0.1             | 4.1      | 1.0             | 2.15          | 0.18                 | PL  | …   | 6     | …                                       | …   | bcu   | PKS 1205–778                |
| J1208.4–6239  | 182.120 | –62.661 | 298.023 | –0.200  | 0.039      | 0.037      | –31    | 16.2     | 5.9      | 0.5             | 37.0     | 4.9             | 2.36          | …                    | LP  | …   | …     | 2FGL J1208.5–6240                       | …   | …     | …                           |
| J1208.7+5442  | 182.188 | 54.707  | 135.822 | 61.340  | 0.042      | 0.040      | 48     | 37.2     | 1.6      | 0.1             | 24.2     | 0.9             | 2.54          | 0.04                 | PL  | T   | …     | 2FGL J1208.8+5441<br>1FGL J1209.3+5444  | …   | fsrq  | TXS 1206+549                |
| J1209.1–5224  | 182.279 | –52.404 | 296.402 | 9.931   | 0.161      | 0.126      | –15    | 4.8      | 0.4      | 0.1             | 5.2      | 1.1             | 2.35          | 0.14                 | PL  | …   | …     | …                                       | …   | spp   | …                           |
| J1209.4+4119  | 182.354 | 41.332  | 151.533 | 73.381  | 0.054      | 0.051      | –46    | 9.9      | 0.4      | 0.1             | 5.1      | 0.8             | 1.94          | 0.12                 | PL  | …   | …     | 2FGL J1209.6+4121<br>1FGL J1209.4+4119  | …   | bll   | B3 1206+516<br>J120940+4119 |
| J1209.8+1810  | 182.469 | 18.178  | 253.841 | 76.896  | 0.053      | 0.048      | –46    | 12.8     | 0.8      | 0.1             | 9.3      | 1.0             | 2.30          | 0.08                 | PL  | T   | …     | 2FGL J1209.7+1807<br>1FGL J1209.7+1806  | …   | fsrq  | MG1 J120953+1809            |
| J1209.9+7607  | 182.477 | 76.124  | 126.202 | 40.739  | 0.082      | 0.079      | –49    | 7.4      | 0.3      | 0.1             | 3.8      | 0.6             | 2.40          | 0.14                 | PL  | …   | …     | …                                       | …   | …     | …                           |
| J1210.1–2742  | 182.546 | –27.714 | 291.876 | 34.270  | 0.121      | 0.114      | 66     | 6.8      | 0.4      | 0.1             | 7.2      | 1.1             | 2.59          | 0.13                 | PL  | T   | 9     | …                                       | …   | …     | …                           |
| J1211.8+6413  | 182.973 | 64.224  | 129.955 | 52.362  | 0.099      | 0.086      | 4      | 4.5      | 0.2      | 0.0             | 2.3      | 0.6             | 2.43          | 0.20                 | PL  | …   | …     | …                                       | …   | …     | …                           |
| J1212.2–6251  | 183.068 | –62.852 | 298.482 | –0.319  | 0.080      | 0.057      | –57    | 8.5      | 3.2      | 0.4             | 46.5     | 6.4             | 2.49          | 0.07                 | PL  | …   | 5     | …                                       | …   | spp   | …                           |
| J1212.6+5135  | 183.150 | 51.597  | 136.994 | 64.458  | 0.137      | 0.093      | 2      | 5.5      | 0.3      | 0.1             | 3.1      | 0.6             | 2.19          | 0.15                 | PL  | …   | …     | …                                       | …   | bll   | 1RXS<br>J121301.8+512942    |
| J1213.1–2619  | 183.300 | –26.325 | 292.362 | 35.761  | 0.083      | 0.074      | –55    | 5.9      | 0.4      | 0.1             | 4.2      | 1.0             | 1.89          | 0.20                 | PL  | …   | …     | 2FGL J1213.2–2616                       | …   | bll   | RBS 1080                    |
| J1213.7+1306  | 183.433 | 13.102  | 268.918 | 73.432  | 0.160      | 0.130      | 16     | 9.1      | 0.5      | 0.1             | 7.2      | 0.9             | 2.52          | 0.10                 | PL  | …   | …     | 2FGL J1214.6+1309                       | …   | fsrq  | 4C +13.46                   |
| J1213.9–4412  | 183.486 | –44.215 | 295.877 | 18.142  | 0.102      | 0.091      | –10    | 8.1      | 0.6      | 0.1             | 7.6      | 1.1             | 2.27          | 0.10                 | PL  | …   | …     | 2FGL J1214.1–4410<br>1FGL J1213.6–4424  | …   | …     | …                           |
| J1214.0–6236  | 183.502 | –62.612 | 298.643 | –0.052  | 0.045      | 0.038      | 76     | 13.9     | 5.3      | 0.4             | 44.3     | 6.0             | 2.33          | …                    | LP  | …   | …     | 2FGL J1214.0–6237<br>1FGL J1213.7–6240c | …   | spp   | …                           |
| J1214.4–2315  | 183.602 | –23.263 | 291.998 | 38.822  | 0.136      | 0.103      | –7     | 5.8      | 0.4      | 0.1             | 5.3      | 1.0             | 2.38          | 0.15                 | PL  | …   | …     | 1FGL J1214.4–2305                       | …   | …     | …                           |
| J1215.0+5002  | 183.774 | 50.036  | 137.405 | 66.058  | 0.049      | 0.045      | 56     | 10.3     | 0.4      | 0.1             | 5.1      | 0.8             | 1.92          | 0.11                 | PL  | …   | …     | 2FGL J1214.9+5004<br>1FGL J1214.9+5004  | …   | bll   | NVSS<br>J121500+500216      |
| J1215.1+1658  | 183.778 | 16.971  | 261.473 | 76.820  | 0.086      | 0.073      | 1      | 9.5      | 0.6      | 0.1             | 6.9      | 0.9             | 2.32          | 0.09                 | PL  | …   | …     | 2FGL J1214.8+1653                       | …   | fsrq  | TXS 1212+171                |
| J1215.9–1926  | 183.992 | –19.435 | 291.534 | 42.650  | 0.275      | 0.211      | 84     | 4.7      | 0.3      | 0.1             | 4.3      | 0.9             | 2.41          | 0.17                 | PL  | …   | …     | …                                       | …   | …     | …                           |
| J1216.6–0557  | 184.161 | –5.965  | 287.389 | 55.854  | 0.313      | 0.274      | 43     | 4.1      | 0.3      | 0.1             | 4.6      | 1.0             | 2.48          | 0.17                 | PL  | …   | …     | …                                       | …   | …     | …                           |

Table 1—Continued

| Name 3FGL    | R.A.    | Decl.   | $l$     | $b$    | $\theta_1$ | $\theta_2$ | $\phi$ | $\sigma$ | $F_{35}$ | $\Delta F_{35}$ | $S_{25}$ | $\Delta S_{25}$ | $\Gamma_{25}$ | $\Delta \Gamma_{25}$ | Mod | Var | Flags | $\gamma$ -ray Assoc.                                                                                | TeV | Class | ID or Assoc.             |
|--------------|---------|---------|---------|--------|------------|------------|--------|----------|----------|-----------------|----------|-----------------|---------------|----------------------|-----|-----|-------|-----------------------------------------------------------------------------------------------------|-----|-------|--------------------------|
| J1217.8+3007 | 184.465 | 30.118  | 188.873 | 82.051 | 0.016      | 0.015      | -76    | 54.7     | 6.1      | 0.2             | 68.0     | 2.6             | 1.97          | 0.02                 | PL  | T   | ...   | 1FHL J1217.8+3006<br>2FGL J1217.8+3006<br>1FGL J1217.7+3007<br>0FGL J1218.0+3006                    | P   | bl    | 1ES 1215+303             |
| J1218.0-0029 | 184.513 | -0.497  | 285.379 | 61.232 | 0.096      | 0.076      | -41    | 8.7      | 0.7      | 0.1             | 8.5      | 1.2             | 2.39          | 0.10                 | PL  | T   | ...   | ...                                                                                                 | ... | bl    | PKS 1215-002             |
| J1218.4-0121 | 184.606 | -1.363  | 286.030 | 60.421 | 0.070      | 0.056      | -23    | 13.8     | 1.1      | 0.1             | 12.8     | 1.3             | 2.20          | 0.08                 | PL  | ... | ...   | 2FGL J1218.5-0122<br>1FGL J1218.4-0128                                                              | ... | bl    | PKS 1216-010             |
| J1218.5+6912 | 184.639 | 69.216  | 127.250 | 47.635 | 0.376      | 0.306      | -60    | 5.4      | 0.1      | 0.0             | 3.8      | 0.6             | 3.02          | 0.17                 | PL  | ... | 5     | ...                                                                                                 | ... | bcu   | NVSS<br>J122044+690522   |
| J1218.8-4827 | 184.713 | -48.458 | 297.373 | 14.062 | 0.080      | 0.069      | 64     | 8.1      | 0.6      | 0.1             | 7.7      | 1.1             | 2.34          | 0.11                 | PL  | ... | ...   | 2FGL J1218.8-4827                                                                                   | ... | bcu   | PMN J1219-4826           |
| J1219.7-0314 | 184.932 | -3.235  | 287.569 | 58.687 | 0.074      | 0.071      | 51     | 8.7      | 0.6      | 0.1             | 6.4      | 1.0             | 2.00          | 0.12                 | PL  | ... | ...   | 2FGL J1219.8-0310                                                                                   | ... | bl    | 1RXS<br>J121946.0-031419 |
| J1220.0-2502 | 185.011 | -25.044 | 293.988 | 37.282 | 0.092      | 0.085      | 32     | 4.5      | 0.3      | 0.1             | 3.6      | 1.0             | 2.25          | 0.20                 | PL  | ... | ...   | 1FGL J1219.8-0309                                                                                   | ... | ...   | ...                      |
| J1220.1-3715 | 185.048 | -37.254 | 296.066 | 25.200 | 0.073      | 0.067      | -51    | 6.8      | 0.4      | 0.1             | 4.7      | 0.9             | 2.05          | 0.14                 | PL  | ... | ...   | ...                                                                                                 | ... | ...   | ...                      |
| J1220.2+3434 | 185.063 | 34.569  | 162.964 | 79.999 | 0.075      | 0.070      | 26     | 10.0     | 0.5      | 0.1             | 5.8      | 0.8             | 2.19          | 0.11                 | PL  | ... | ...   | 1FGL J1220.2+3432                                                                                   | ... | bl    | GB2 1217+343             |
| J1220.2+7105 | 185.068 | 71.093  | 126.546 | 45.816 | 0.084      | 0.077      | 19     | 14.6     | 0.6      | 0.1             | 8.0      | 0.7             | 2.46          | 0.07                 | PL  | T   | ...   | 2FGL J1219.2+7107<br>1FGL J1221.5+7106                                                              | ... | fsrq  | S5 1217+71               |
| J1220.3+6055 | 185.091 | 60.929  | 129.641 | 55.793 | 0.121      | 0.099      | 39     | 4.2      | 0.2      | 0.0             | 2.4      | 0.6             | 2.52          | 0.21                 | PL  | ... | ...   | ...                                                                                                 | ... | ...   | ...                      |
| J1221.3+3010 | 185.341 | 30.177  | 186.363 | 82.734 | 0.015      | 0.014      | 71     | 38.9     | 3.3      | 0.2             | 46.7     | 3.0             | 1.66          | 0.04                 | PL  | T   | ...   | 1FHL J1221.3+3011<br>2FGL J1221.3+3010<br>1FGL J1221.3+3008                                         | P   | bl    | PG 1218+304              |
| J1221.4+2814 | 185.374 | 28.240  | 201.683 | 83.280 | 0.022      | 0.020      | 39     | 49.9     | 4.1      | 0.2             | 45.9     | 1.8             | 2.10          | 0.03                 | PL  | T   | ...   | 1FHL J1221.6+2814<br>2FGL J1221.4+2814<br>1FGL J1221.5+2814<br>0FGL J1221.7+2814<br>1AGL J1222+2851 | P   | bl    | W Comae                  |
| J1221.5-0632 | 185.378 | -6.550  | 289.713 | 55.552 | 0.096      | 0.073      | -61    | 11.5     | 0.8      | 0.1             | 9.5      | 1.1             | 2.25          | 0.09                 | PL  | ... | ...   | 2FGL J1221.4-0633<br>1FGL J1221.4-0635                                                              | ... | ...   | ...                      |
| J1222.4+0414 | 185.611 | 4.234   | 284.851 | 66.083 | 0.077      | 0.071      | -72    | 30.0     | 1.2      | 0.1             | 28.7     | 1.4             | 2.77          | ...                  | LP  | T   | ...   | 2FGL J1222.4+0413<br>1FGL J1222.5+0415                                                              | ... | fsrq  | 4C +04.42                |
| J1222.7+7952 | 185.683 | 79.867  | 124.513 | 37.173 | 0.055      | 0.052      | -7     | 5.5      | 0.2      | 0.1             | 2.4      | 0.7             | 1.74          | 0.21                 | PL  | ... | ...   | 1FHL J1223.3+7953<br>2FGL J1223.3+7954                                                              | ... | ...   | ...                      |
| J1222.7+8041 | 185.695 | 80.698  | 124.366 | 36.350 | 0.053      | 0.044      | 78     | 16.9     | 1.0      | 0.1             | 11.7     | 0.9             | 2.29          | 0.05                 | PL  | T   | ...   | 2FGL J1223.9+8043<br>1FGL J1224.8+8044                                                              | ... | bl    | S5 1221+80               |
| J1223.0-5622 | 185.752 | -56.376 | 298.980 | 6.277  | 0.185      | 0.164      | -21    | 6.1      | 0.4      | 0.1             | 9.6      | 1.5             | 2.78          | 0.12                 | PL  | ... | 1,4   | ...                                                                                                 | ... | ...   | ...                      |
| J1223.2+1215 | 185.804 | 12.262  | 277.570 | 73.728 | 0.144      | 0.135      | -33    | 4.8      | 0.3      | 0.1             | 3.7      | 0.8             | 2.21          | 0.16                 | PL  | ... | ...   | ...                                                                                                 | ... | ...   | ...                      |

Table 1—Continued

| Name 3FGL    | R.A.    | Decl.   | $l$     | $b$     | $\theta_1$ | $\theta_2$ | $\phi$ | $\sigma$ | $F_{35}$ | $\Delta F_{35}$ | $S_{25}$ | $\Delta S_{25}$ | $\Gamma_{25}$ | $\Delta \Gamma_{25}$ | Mod | Var | Flags | $\gamma$ -ray Assoc.                                                                                               | TeV | Class | ID or Assoc.             |
|--------------|---------|---------|---------|---------|------------|------------|--------|----------|----------|-----------------|----------|-----------------|---------------|----------------------|-----|-----|-------|--------------------------------------------------------------------------------------------------------------------|-----|-------|--------------------------|
| J1223.3+0818 | 185.840 | 8.313   | 282.182 | 70.046  | 0.098      | 0.081      | −30    | 6.4      | 0.4      | 0.1             | 4.1      | 0.9             | 1.98          | 0.16                 | PL  | ... | ...   | ...                                                                                                                | ... | ...   | ...                      |
| J1223.3−3028 | 185.843 | −30.471 | 295.800 | 32.012  | 0.164      | 0.098      | −44    | 4.4      | 0.3      | 0.1             | 3.2      | 0.9             | 1.89          | 0.22                 | PL  | ... | ...   | 1FGL J1223.4−3034                                                                                                  | ... | bcu   | NVSS<br>J122337−303246   |
| J1224.5+4957 | 186.127 | 49.960  | 133.875 | 66.592  | 0.182      | 0.128      | −14    | 6.4      | 0.3      | 0.1             | 4.5      | 0.8             | 2.46          | 0.13                 | PL  | ... | ...   | ...                                                                                                                | ... | fsrq  | SBS 1221+503             |
| J1224.5+2436 | 186.136 | 24.611  | 234.030 | 83.449  | 0.045      | 0.042      | −20    | 13.4     | 0.7      | 0.1             | 8.2      | 1.1             | 1.89          | 0.09                 | PL  | ... | ...   | 1FHL J1224.5+2437                                                                                                  | P   | bll   | MS 1221.8+2452           |
| J1224.6+4332 | 186.158 | 43.546  | 139.468 | 72.712  | 0.115      | 0.094      | 16     | 11.2     | 0.4      | 0.1             | 6.9      | 0.7             | 2.64          | 0.09                 | PL  | ... | ...   | 2FGL J1224.4+2436<br>2FGL J1225.0+4335<br>1FGL J1225.8+4336<br>3EG J1227+4302                                      | ... | bll   | B3 1222+438              |
| J1224.6−8312 | 186.165 | −83.209 | 302.090 | −20.381 | 0.127      | 0.110      | 10     | 7.5      | 0.4      | 0.1             | 8.6      | 1.2             | 2.69          | 0.11                 | PL  | ... | ...   | 2FGL J1228.7−8310                                                                                                  | ... | bcu   | PKS 1221−82              |
| J1224.9+2122 | 186.226 | 21.382  | 255.059 | 81.662  | 0.010      | 0.010      | 90     | 219.7    | 25.5     | 0.4             | 283.9    | 3.4             | 2.29          | ...                  | LP  | T   | ...   | 1FHL J1224.8+2122<br>2FGL J1224.9+2122<br>1FGL J1224.7+2121<br>3EG J1224+2118                                      | P   | FSRQ  | 4C +21.35                |
| J1225.4−3448 | 186.356 | −34.807 | 296.900 | 27.760  | 0.055      | 0.053      | −6     | 4.8      | 0.2      | 0.1             | 2.5      | 0.8             | 1.76          | 0.24                 | PL  | ... | ...   | ...                                                                                                                | ... | ...   | ...                      |
| J1225.7−7314 | 186.440 | −73.241 | 301.053 | −10.463 | 0.079      | 0.071      | −55    | 5.4      | 0.5      | 0.1             | 5.8      | 1.2             | 2.31          | 0.14                 | PL  | ... | 1     | ...                                                                                                                | ... | bcu   | PMN J1225−7313           |
| J1225.9+2953 | 186.496 | 29.890  | 185.152 | 83.765  | 0.054      | 0.049      | −45    | 17.4     | 1.4      | 0.1             | 8.7      | 1.0             | 2.02          | ...                  | LP  | ... | ...   | 2FGL J1226.0+2953<br>1FGL J1226.0+2954                                                                             | ... | ...   | ...                      |
| J1226.8+0638 | 186.700 | 6.649   | 285.872 | 68.701  | 0.068      | 0.060      | −29    | 5.5      | 0.2      | 0.1             | 2.8      | 0.9             | 1.56          | 0.24                 | PL  | ... | ...   | 1FGL J1226.8+0638                                                                                                  | ... | bll   | 1RXS<br>J122645.2+063906 |
| J1226.9−1329 | 186.742 | −13.499 | 293.855 | 48.941  | 0.048      | 0.046      | −37    | 13.4     | 1.0      | 0.1             | 11.6     | 1.4             | 1.98          | 0.09                 | PL  | ... | 10    | 2FGL J1226.7−1331<br>1FGL J1226.7−1332                                                                             | ... | bll   | PMN J1226−1328           |
| J1227.9−4854 | 186.976 | −48.901 | 298.954 | 13.789  | 0.037      | 0.034      | 12     | 38.6     | 3.7      | 0.2             | 41.4     | 1.7             | 2.38          | ...                  | LP  | T   | ...   | 2FGL J1227.7−4853<br>1FGL J1227.9−4852                                                                             | ... | psr   | PSR J1227−4853           |
| J1228.4−0317 | 187.111 | −3.295  | 291.714 | 59.075  | 0.152      | 0.097      | 70     | 5.7      | 0.4      | 0.1             | 4.7      | 0.9             | 2.27          | 0.17                 | PL  | ... | ...   | 3EG J1230−0247                                                                                                     | ... | ...   | ...                      |
| J1228.7+4857 | 187.181 | 48.964  | 132.801 | 67.727  | 0.064      | 0.056      | −14    | 7.9      | 0.4      | 0.1             | 5.6      | 1.0             | 2.36          | 0.12                 | PL  | ... | ...   | 1FHL J1228.5+4857<br>2FGL J1228.6+4857<br>1FGL J1228.2+4855                                                        | ... | fsrq  | TXS 1226+492             |
| J1229.1+0202 | 187.287 | 2.041   | 289.979 | 64.351  | 0.019      | 0.018      | −85    | 149.0    | 9.4      | 0.3             | 181.0    | 2.2             | 2.66          | ...                  | LP  | T   | ...   | 2FGL J1229.1+0202<br>1FGL J1229.1+0203<br>0FGL J1229.1+0202<br>3EG J1229+0210<br>EGR J1229+0203<br>1AGL J1228+0142 | ... | FSRQ  | 3C 273                   |
| J1229.8−5305 | 187.469 | −53.093 | 299.652 | 9.641   | 0.119      | 0.113      | 74     | 4.2      | 0.4      | 0.1             | 4.1      | 1.1             | 2.15          | 0.22                 | PL  | ... | ...   | 2FGL J1230.2−5258                                                                                                  | ... | bcu   | AT20G<br>J122939−530332  |
| J1230.3+2519 | 187.575 | 25.326  | 232.571 | 84.929  | 0.061      | 0.049      | −90    | 18.0     | 1.1      | 0.1             | 13.0     | 1.0             | 2.24          | 0.06                 | PL  | T   | ...   | 1FHL J1230.3+2522<br>2FGL J1230.2+2517                                                                             | ... | bll   | ON 246                   |

Table 1—Continued

| Name 3FGL    | R.A.    | Decl.   | $l$     | $b$    | $\theta_1$ | $\theta_2$ | $\phi$ | $\sigma$ | $F_{35}$ | $\Delta F_{35}$ | $S_{25}$ | $\Delta S_{25}$ | $\Gamma_{25}$ | $\Delta \Gamma_{25}$ | Mod | Var | Flags | $\gamma$ -ray Assoc.                                                                               | TeV | Class | ID or Assoc.            |
|--------------|---------|---------|---------|--------|------------|------------|--------|----------|----------|-----------------|----------|-----------------|---------------|----------------------|-----|-----|-------|----------------------------------------------------------------------------------------------------|-----|-------|-------------------------|
| J1230.9+1224 | 187.728 | 12.406  | 283.839 | 74.512 | 0.043      | 0.041      | 87     | 18.9     | 1.3      | 0.1             | 14.5     | 1.3             | 2.04          | 0.07                 | PL  | ... | ...   | 1FGL J1230.4+2520<br>1FHL J1230.8+1224<br>2FGL J1230.8+1224<br>1FGL J1230.8+1223                   | P   | rdg   | M 87                    |
| J1231.2−1411 | 187.801 | −14.198 | 295.539 | 48.383 | 0.015      | 0.014      | 43     | 105.7    | 17.8     | 0.4             | 102.9    | 2.1             | 1.93          | ...                  | EC  | ... | ...   | 1FHL J1231.2−1414<br>2FGL J1231.2−1411<br>1FGL J1231.1−1410<br>0FGL J1231.5−1410<br>EGR J1231−1412 | ... | PSR   | PSR J1231−1411          |
| J1231.5+6414 | 187.879 | 64.234  | 126.507 | 52.756 | 0.068      | 0.052      | 6      | 6.3      | 0.2      | 0.1             | 2.7      | 0.6             | 1.94          | 0.20                 | PL  | ... | ...   | ...                                                                                                | ... | bll   | MS 1229.2+6430          |
| J1231.6−5113 | 187.902 | −51.221 | 299.766 | 11.529 | 0.105      | 0.092      | 16     | 13.5     | 0.8      | 0.1             | 12.4     | 1.2             | 2.59          | ...                  | LP  | ... | ...   | 2FGL J1231.3−5112<br>1FGL J1232.2−5118                                                             | ... | ...   | ...                     |
| J1231.6+4825 | 187.908 | 48.418  | 131.870 | 68.365 | 0.099      | 0.089      | −74    | 5.9      | 0.3      | 0.1             | 4.7      | 0.9             | 2.52          | 0.13                 | PL  | ... | 5     | ...                                                                                                | ... | ...   | ...                     |
| J1231.7−6513 | 187.926 | −65.223 | 300.865 | −2.430 | 0.086      | 0.075      | −40    | 9.5      | 1.3      | 0.2             | 17.7     | 2.0             | 2.42          | 0.07                 | PL  | ... | 3     | 2FGL J1231.1−6512                                                                                  | ... | ...   | ...                     |
| J1231.7+2847 | 187.946 | 28.792  | 190.812 | 85.353 | 0.023      | 0.023      | −65    | 37.0     | 2.7      | 0.1             | 31.0     | 1.8             | 1.95          | 0.04                 | PL  | T   | ...   | 1FGL J1231.6+2850<br>1FHL J1231.8+2849<br>2FGL J1231.7+2848                                        | ... | bll   | B2 1229+29              |
| J1231.8+1421 | 187.966 | 14.364  | 282.287 | 76.445 | 0.136      | 0.100      | 77     | 5.9      | 0.4      | 0.1             | 4.3      | 0.9             | 2.07          | 0.17                 | PL  | ... | ...   | 2FGL J1231.6+1417                                                                                  | ... | bll   | GB6 J1231+1421          |
| J1232.3+1701 | 188.085 | 17.023  | 278.347 | 78.972 | 0.141      | 0.106      | 40     | 5.7      | 0.3      | 0.1             | 3.8      | 0.9             | 1.84          | 0.17                 | PL  | ... | ...   | ...                                                                                                | ... | ...   | ...                     |
| J1232.5−3720 | 188.137 | −37.342 | 298.778 | 25.377 | 0.069      | 0.056      | −4     | 6.4      | 0.3      | 0.1             | 3.9      | 0.9             | 1.92          | 0.20                 | PL  | ... | ...   | ...                                                                                                | ... | ...   | ...                     |
| J1232.8+1332 | 188.219 | 13.535  | 284.323 | 75.731 | 0.162      | 0.146      | −10    | 4.3      | 0.3      | 0.1             | 5.1      | 1.1             | 2.67          | 0.15                 | PL  | ... | ...   | ...                                                                                                | ... | ...   | ...                     |
| J1233.7−0145 | 188.434 | −1.757  | 293.837 | 60.802 | 0.046      | 0.041      | 73     | 15.7     | 1.1      | 0.1             | 12.9     | 1.2             | 2.22          | 0.08                 | PL  | ... | ...   | 2FGL J1233.7−0145                                                                                  | ... | bll   | NVSS<br>J123341−014426  |
| J1233.9−5736 | 188.497 | −57.607 | 300.587 | 5.185  | 0.037      | 0.034      | −39    | 13.6     | 1.5      | 0.1             | 17.1     | 1.7             | 2.16          | 0.07                 | PL  | ... | ...   | 1FGL J1233.6−0146<br>1FHL J1234.1−5735<br>2FGL J1234.0−5733<br>1FGL J1234.0−5736                   | ... | bcu   | AT20G<br>J123407−573552 |
| J1234.7−0437 | 188.697 | −4.622  | 295.087 | 57.996 | 0.122      | 0.080      | 29     | 4.9      | 0.2      | 0.1             | 3.0      | 0.9             | 1.65          | 0.28                 | PL  | ... | 10    | ...                                                                                                | ... | ...   | ...                     |
| J1236.5−6154 | 189.128 | −61.904 | 301.176 | 0.916  | 0.112      | 0.103      | −62    | 4.1      | 0.9      | 0.2             | 11.3     | 2.7             | 2.37          | 0.14                 | PL  | ... | 4     | 2FGL J1236.1−6155                                                                                  | ... | ...   | ...                     |
| J1236.6−7050 | 189.157 | −70.846 | 301.706 | −8.010 | 0.105      | 0.091      | 61     | 5.4      | 0.5      | 0.1             | 6.0      | 1.3             | 2.21          | 0.14                 | PL  | ... | 1     | ...                                                                                                | ... | ...   | ...                     |
| J1236.6+3901 | 189.165 | 39.024  | 136.536 | 77.711 | 0.111      | 0.104      | −29    | 5.3      | 0.2      | 0.1             | 3.1      | 0.7             | 2.49          | 0.20                 | PL  | ... | ...   | ...                                                                                                | ... | bll   | RX J1236.4+3859         |
| J1237.9+6258 | 189.495 | 62.979  | 125.537 | 54.082 | 0.068      | 0.058      | −11    | 6.3      | 0.2      | 0.1             | 2.4      | 0.6             | 1.84          | 0.22                 | PL  | ... | ...   | ...                                                                                                | ... | bll   | 1H 1241+626             |
| J1238.2−1958 | 189.565 | −19.983 | 298.712 | 42.781 | 0.061      | 0.060      | 87     | 8.5      | 0.5      | 0.1             | 6.6      | 0.9             | 2.35          | 0.13                 | PL  | ... | ...   | 2FGL J1238.1−1953                                                                                  | ... | bcu   | PMN J1238−1959          |
| J1238.3−4543 | 189.595 | −45.724 | 300.549 | 17.087 | 0.076      | 0.060      | −52    | 8.0      | 0.5      | 0.1             | 6.2      | 1.0             | 2.15          | 0.13                 | PL  | ... | ...   | ...                                                                                                | ... | bcu   | PMN J1238−4541          |
| J1239.1−1158 | 189.799 | −11.978 | 298.194 | 50.781 | 0.256      | 0.220      | 33     | 6.7      | 0.2      | 0.1             | 7.0      | 1.0             | 3.07          | 0.16                 | PL  | ... | ...   | ...                                                                                                | ... | ...   | ...                     |
| J1239.4+0727 | 189.873 | 7.463   | 294.191 | 70.131 | 0.085      | 0.068      | −5     | 8.0      | 0.5      | 0.1             | 6.6      | 1.0             | 2.40          | 0.12                 | PL  | ... | ...   | 2FGL J1239.5+0728                                                                                  | ... | bcu   | PKS 1236+077            |

Table 1—Continued

| Name 3FGL    | R.A.    | Decl.   | $l$     | $b$    | $\theta_1$ | $\theta_2$ | $\phi$ | $\sigma$ | $F_{35}$ | $\Delta F_{35}$ | $S_{25}$ | $\Delta S_{25}$ | $\Gamma_{25}$ | $\Delta \Gamma_{25}$ | Mod | Var | Flags | $\gamma$ -ray Assoc.                                                                             | TeV | Class | ID or Assoc.             |
|--------------|---------|---------|---------|--------|------------|------------|--------|----------|----------|-----------------|----------|-----------------|---------------|----------------------|-----|-----|-------|--------------------------------------------------------------------------------------------------|-----|-------|--------------------------|
| J1239.5+0443 | 189.895 | 4.719   | 295.221 | 67.413 | 0.025      | 0.024      | −3     | 65.0     | 5.6      | 0.2             | 61.6     | 1.8             | 2.35          | ...                  | LP  | T   | ...   | 1FHL J1239.6+0443<br>2FGL J1239.5+0443<br>1FGL J1239.5+0443<br>EGR J1237+0434<br>1AGL J1238+0406 | ... | fsrq  | MG1 J123931+0443         |
| J1240.3−7149 | 190.077 | −71.826 | 302.054 | −8.973 | 0.052      | 0.042      | −6     | 11.0     | 0.9      | 0.1             | 10.2     | 1.4             | 1.96          | 0.10                 | PL  | ... | ...   | 1FHL J1240.4−7150<br>2FGL J1240.6−7151<br>1FGL J1240.3−7154                                      | ... | ...   | ...                      |
| J1241.6−1456 | 190.406 | −14.945 | 299.399 | 47.859 | 0.089      | 0.072      | 29     | 6.2      | 0.3      | 0.1             | 3.9      | 0.9             | 1.96          | 0.17                 | PL  | ... | ...   | 2FGL J1241.6−1457                                                                                | ... | bll   | RX J1241.8−1455          |
| J1241.9+0639 | 190.475 | 6.661   | 296.186 | 69.408 | 0.109      | 0.080      | −25    | 5.2      | 0.3      | 0.1             | 3.1      | 0.9             | 1.78          | 0.24                 | PL  | ... | ...   | ...                                                                                              | ... | bll   | 1ES 1239+069             |
| J1243.1+3627 | 190.797 | 36.454  | 133.043 | 80.512 | 0.023      | 0.023      | 4      | 31.2     | 2.0      | 0.1             | 25.0     | 1.9             | 1.77          | 0.04                 | PL  | ... | ...   | 1FHL J1243.2+3628<br>2FGL J1243.1+3627<br>1FGL J1243.1+3627                                      | ... | bll   | Ton 116                  |
| J1243.9−0217 | 190.977 | −2.284  | 299.107 | 60.531 | 0.142      | 0.137      | −57    | 5.1      | 0.3      | 0.1             | 3.8      | 0.8             | 2.19          | 0.17                 | PL  | ... | 1     | ...                                                                                              | ... | bcu   | PMN J1243−0218           |
| J1244.1+1615 | 191.045 | 16.263  | 293.764 | 79.005 | 0.192      | 0.162      | 63     | 5.5      | 0.3      | 0.1             | 4.1      | 0.8             | 2.43          | 0.16                 | PL  | ... | 1     | ...                                                                                              | ... | bll   | SDSS J124444.35+161621.7 |
| J1244.2−6227 | 191.059 | −62.453 | 302.100 | 0.407  | 0.113      | 0.086      | 1      | 6.0      | 1.5      | 0.2             | 18.3     | 3.1             | 2.32          | 0.09                 | PL  | ... | 4     | 2FGL J1243.9−6232                                                                                | ... | ...   | ...                      |
| J1244.3−5515 | 191.085 | −55.257 | 301.912 | 7.601  | 0.192      | 0.157      | −61    | 6.9      | 0.6      | 0.1             | 9.5      | 1.4             | 2.62          | 0.11                 | PL  | ... | 1     | ...                                                                                              | ... | ...   | ...                      |
| J1244.3−4955 | 191.090 | −49.926 | 301.764 | 12.929 | 0.132      | 0.092      | −19    | 4.8      | 0.4      | 0.1             | 4.7      | 1.1             | 2.19          | 0.18                 | PL  | ... | 4     | ...                                                                                              | ... | bcu   | SUMSS J124422−495422     |
| J1244.8+5707 | 191.212 | 57.121  | 124.720 | 59.984 | 0.101      | 0.087      | 15     | 7.1      | 0.3      | 0.1             | 3.7      | 0.7             | 2.07          | 0.15                 | PL  | ... | ...   | 1FHL J1244.9+5708<br>2FGL J1245.1+5708                                                           | ... | bll   | 1RXS J124510.5+571020    |
| J1246.7−2547 | 191.689 | −25.791 | 301.612 | 37.068 | 0.018      | 0.017      | −60    | 92.6     | 9.8      | 0.3             | 103.3    | 2.3             | 2.28          | ...                  | LP  | T   | ...   | 1FHL J1246.6−2548<br>2FGL J1246.7−2546<br>1FGL J1246.7−2545<br>0FGL J1246.6−2544                 | ... | fsrq  | PKS 1244−255             |
| J1247.0+4421 | 191.753 | 44.355  | 125.601 | 72.750 | 0.105      | 0.087      | −60    | 5.7      | 0.3      | 0.1             | 2.8      | 0.6             | 2.06          | 0.25                 | PL  | ... | ...   | ...                                                                                              | ... | bll   | RX J1246.9+4423          |
| J1248.0+5130 | 192.021 | 51.506  | 124.196 | 65.614 | 0.133      | 0.117      | 68     | 5.2      | 0.3      | 0.1             | 2.9      | 0.6             | 2.16          | 0.17                 | PL  | ... | ...   | ...                                                                                              | ... | bll   | RX J1248.4+5128          |
| J1248.2+5820 | 192.070 | 58.348  | 123.731 | 58.776 | 0.018      | 0.018      | −85    | 55.5     | 4.0      | 0.1             | 45.0     | 1.9             | 1.95          | 0.03                 | PL  | ... | ...   | 0FGL J1248.7+5811<br>1FGL J1248.2+5820<br>1FHL J1248.1+5821<br>2FGL J1248.2+5820                 | ... | bll   | PG 1246+586              |
| J1249.1−2808 | 192.293 | −28.144 | 302.325 | 34.725 | 0.075      | 0.062      | −82    | 8.2      | 0.5      | 0.1             | 5.9      | 1.0             | 2.07          | 0.13                 | PL  | ... | ...   | 2FGL J1249.5−2811<br>1FGL J1249.3−2812                                                           | ... | ...   | ...                      |
| J1249.5−0546 | 192.382 | −5.779  | 302.057 | 57.089 | 0.145      | 0.129      | 66     | 5.4      | 0.4      | 0.1             | 5.4      | 1.2             | 2.41          | 0.16                 | PL  | ... | ...   | ...                                                                                              | ... | ...   | ...                      |
| J1249.7+3705 | 192.442 | 37.091  | 124.856 | 80.031 | 0.052      | 0.044      | 41     | 11.3     | 0.5      | 0.1             | 6.9      | 1.2             | 1.65          | 0.10                 | PL  | ... | ...   | 1FHL J1249.7+3706<br>2FGL J1249.9+3705                                                           | ... | bll   | RX J1249.8+3708          |



Table 1—Continued

| Name 3FGL    | R.A.    | Decl.   | $l$     | $b$    | $\theta_1$ | $\theta_2$ | $\phi$ | $\sigma$ | $F_{35}$ | $\Delta F_{35}$ | $S_{25}$ | $\Delta S_{25}$ | $\Gamma_{25}$ | $\Delta \Gamma_{25}$ | Mod | Var | Flags | $\gamma$ -ray Assoc. | TeV | Class | ID or Assoc.               |
|--------------|---------|---------|---------|--------|------------|------------|--------|----------|----------|-----------------|----------|-----------------|---------------|----------------------|-----|-----|-------|----------------------|-----|-------|----------------------------|
|              |         |         |         |        |            |            |        |          |          |                 |          |                 |               |                      |     |     |       | 1FGL J1249.8+3706    |     |       |                            |
| J1250.2–0233 | 192.568 | –2.564  | 302.344 | 60.307 | 0.076      | 0.064      | 64     | 5.1      | 0.1      | 0.1             | 2.8      | 1.1             | 1.10          | 0.30                 | PL  | ... | ...   | ...                  | ... | ...   | ...                        |
| J1250.5+0217 | 192.626 | 2.297   | 302.378 | 65.168 | 0.112      | 0.089      | 67     | 6.4      | 0.4      | 0.1             | 5.0      | 0.9             | 2.33          | 0.16                 | PL  | ... | ...   | ...                  | ... | bll   | PKS 1247+025               |
| J1251.0–0203 | 192.763 | –2.057  | 302.734 | 60.815 | 0.098      | 0.090      | –63    | 6.9      | 0.5      | 0.1             | 5.9      | 0.9             | 2.39          | 0.12                 | PL  | T   | ...   | ...                  | ... | bcu   | TXS 1248–017               |
| J1251.0–4943 | 192.773 | –49.731 | 302.875 | 13.140 | 0.096      | 0.070      | 28     | 6.8      | 0.5      | 0.1             | 6.0      | 1.1             | 2.03          | 0.14                 | PL  | ... | ...   | 1FGL J1250.9–4940    | ... | ...   | ...                        |
| J1251.3+1041 | 192.846 | 10.688  | 302.886 | 73.560 | 0.175      | 0.138      | –75    | 6.4      | 0.4      | 0.1             | 5.1      | 0.9             | 2.44          | 0.16                 | PL  | ... | ...   | 2FGL J1251.2+1045    | ... | bll   | 1RXS<br>J125117.4+103914   |
|              |         |         |         |        |            |            |        |          |          |                 |          |                 |               |                      |     |     |       | 1FGL J1251.3+1044    |     |       |                            |
| J1253.2+5300 | 193.301 | 53.013  | 122.323 | 64.113 | 0.019      | 0.018      | –14    | 47.5     | 4.2      | 0.2             | 36.9     | 2.2             | 2.00          | ...                  | LP  | ... | ...   | 1FHL J1253.1+5301    | ... | bll   | S4 1250+53                 |
|              |         |         |         |        |            |            |        |          |          |                 |          |                 |               |                      |     |     |       | 2FGL J1253.1+5302    |     |       |                            |
|              |         |         |         |        |            |            |        |          |          |                 |          |                 |               |                      |     |     |       | 1FGL J1253.0+5301    |     |       |                            |
|              |         |         |         |        |            |            |        |          |          |                 |          |                 |               |                      |     |     |       | 0FGL J1253.4+5300    |     |       |                            |
| J1253.7+0327 | 193.435 | 3.464   | 304.363 | 66.329 | 0.047      | 0.041      | 64     | 12.1     | 0.7      | 0.1             | 9.0      | 1.3             | 1.84          | 0.10                 | PL  | ... | ...   | 1FHL J1253.6+0329    | ... | bll   | MG1 J125348+0326           |
|              |         |         |         |        |            |            |        |          |          |                 |          |                 |               |                      |     |     |       | 1FGL J1253.7+0326    |     |       |                            |
| J1254.1–2203 | 193.532 | –22.060 | 303.757 | 40.808 | 0.094      | 0.088      | –68    | 7.2      | 0.6      | 0.1             | 6.8      | 1.1             | 2.30          | 0.12                 | PL  | ... | ...   | 2FGL J1254.2–2203    | ... | bcu   | NVSS  <br>J125422–220413   |
| J1254.1+6240 | 193.543 | 62.678  | 122.393 | 54.448 | 0.075      | 0.068      | 36     | 7.1      | 0.3      | 0.1             | 3.0      | 0.6             | 1.90          | 0.15                 | PL  | ... | ...   | 2FGL J1254.1+6237    | ... | bll   | 1RXS  <br>J125400.1+624303 |
|              |         |         |         |        |            |            |        |          |          |                 |          |                 |               |                      |     |     |       | 1FGL J1254.0+6236    |     |       |                            |
| J1254.5+2210 | 193.630 | 22.175  | 311.140 | 84.997 | 0.056      | 0.051      | 83     | 10.8     | 0.6      | 0.1             | 6.7      | 1.0             | 2.00          | 0.12                 | PL  | ... | ...   | 2FGL J1254.4+2209    | ... | bll   | TXS 1252+224               |
|              |         |         |         |        |            |            |        |          |          |                 |          |                 |               |                      |     |     |       | 1FGL J1254.4+2209    |     |       |                            |
| J1254.9–4423 | 193.742 | –44.393 | 303.597 | 18.474 | 0.088      | 0.076      | 59     | 4.4      | 0.3      | 0.1             | 3.6      | 1.0             | 2.19          | 0.27                 | PL  | ... | ...   | ...                  | ... | bll   | PKS 1252–441               |
| J1256.1–0547 | 194.041 | –5.791  | 305.095 | 57.061 | 0.012      | 0.012      | 55     | 160.6    | 20.6     | 0.4             | 239.2    | 3.1             | 2.34          | ...                  | LP  | T   | ...   | 1FHL J1256.1–0547    | P   | FSRQ  | 3C 279                     |
|              |         |         |         |        |            |            |        |          |          |                 |          |                 |               |                      |     |     |       | 2FGL J1256.1–0547    |     |       |                            |
|              |         |         |         |        |            |            |        |          |          |                 |          |                 |               |                      |     |     |       | 1FGL J1256.2–0547    |     |       |                            |
|              |         |         |         |        |            |            |        |          |          |                 |          |                 |               |                      |     |     |       | 0FGL J1256.1–0547    |     |       |                            |
|              |         |         |         |        |            |            |        |          |          |                 |          |                 |               |                      |     |     |       | 3EG J1255–0549       |     |       |                            |
|              |         |         |         |        |            |            |        |          |          |                 |          |                 |               |                      |     |     |       | EGR J1256–0552       |     |       |                            |
|              |         |         |         |        |            |            |        |          |          |                 |          |                 |               |                      |     |     |       | 1AGL J1256–0549      |     |       |                            |
| J1256.1–5703 | 194.045 | –57.050 | 303.580 | 5.815  | 0.176      | 0.151      | –3     | 6.4      | 0.6      | 0.1             | 11.2     | 1.7             | 2.69          | 0.10                 | PL  | ... | ...   | ...                  | ... | ...   | ...                        |
| J1256.1–5919 | 194.045 | –59.324 | 303.538 | 3.542  | 0.056      | 0.052      | –50    | 7.9      | 0.9      | 0.1             | 11.4     | 1.7             | 2.29          | 0.10                 | PL  | ... | 4     | 1FGL J1256.1–5922    | ... | bcu   | PMN J1256–5919             |
| J1256.3–1146 | 194.087 | –11.781 | 304.845 | 51.073 | 0.043      | 0.036      | –31    | 11.1     | 0.7      | 0.1             | 7.7      | 1.2             | 1.91          | 0.11                 | PL  | ... | ...   | 1FHL J1256.4–1146    | ... | bcu   | PMN J1256–1146             |
|              |         |         |         |        |            |            |        |          |          |                 |          |                 |               |                      |     |     |       | 2FGL J1256.5–1145    |     |       |                            |
|              |         |         |         |        |            |            |        |          |          |                 |          |                 |               |                      |     |     |       | 1FGL J1256.5–1148    |     |       |                            |
| J1256.7+5328 | 194.189 | 53.469  | 121.150 | 63.641 | 0.152      | 0.136      | 23     | 5.8      | 0.3      | 0.1             | 6.1      | 1.1             | 2.64          | 0.12                 | PL  | ... | 5     | ...                  | ... | bcu   | TXS 1254+538               |
| J1256.9+3649 | 194.232 | 36.819  | 116.435 | 80.240 | 0.067      | 0.057      | –74    | 12.5     | 0.7      | 0.1             | 7.4      | 0.9             | 2.08          | 0.09                 | PL  | ... | ...   | 2FGL J1257.0+3650    | ... | bll   | 1RXS<br>J125716.0+364713   |
|              |         |         |         |        |            |            |        |          |          |                 |          |                 |               |                      |     |     |       | 1FGL J1256.9+3650    |     |       |                            |
| J1257.0–6338 | 194.253 | –63.636 | 303.551 | –0.771 | 0.051      | 0.043      | 28     | 8.5      | 1.9      | 0.2             | 21.7     | 3.0             | 2.24          | 0.09                 | PL  | T   | 3     | 1FGL J1256.9–6337c   | ... | ...   | ...                        |

Table 1—Continued

| Name 3FGL     | R.A.    | Decl.   | $l$     | $b$     | $\theta_1$ | $\theta_2$ | $\phi$ | $\sigma$ | $F_{35}$ | $\Delta F_{35}$ | $S_{25}$ | $\Delta S_{25}$ | $\Gamma_{25}$ | $\Delta \Gamma_{25}$ | Mod | Var | Flags | $\gamma$ -ray Assoc.                                        | TeV | Class | ID or Assoc.             |
|---------------|---------|---------|---------|---------|------------|------------|--------|----------|----------|-----------------|----------|-----------------|---------------|----------------------|-----|-----|-------|-------------------------------------------------------------|-----|-------|--------------------------|
| J1258.0+6120  | 194.523 | 61.340  | 121.513 | 55.770  | 0.092      | 0.087      | −48    | 5.1      | 0.2      | 0.0             | 2.2      | 0.5             | 2.10          | 0.21                 | PL  | ... | ...   | ...                                                         | ... | bll   | NVSS<br>J125820+612049   |
| J1258.1+3233  | 194.535 | 32.557  | 108.355 | 84.381  | 0.070      | 0.063      | 67     | 11.9     | 0.6      | 0.1             | 8.2      | 0.9             | 2.47          | 0.09                 | PL  | T   | ...   | 2FGL J1258.2+3231<br>1FGL J1258.3+3227                      | ... | fsrq  | ON 393                   |
| J1258.4+2123  | 194.618 | 21.386  | 318.906 | 84.038  | 0.130      | 0.106      | −86    | 5.0      | 0.2      | 0.1             | 4.2      | 1.1             | 2.64          | 0.24                 | PL  | ... | ...   | 1FGL J1258.3+2125                                           | ... | ...   | ...                      |
| J1258.6−1800  | 194.650 | −18.004 | 305.334 | 44.834  | 0.054      | 0.052      | −68    | 22.4     | 1.5      | 0.1             | 21.0     | 1.2             | 2.45          | 0.05                 | PL  | T   | ...   | 2FGL J1258.4−1801<br>1FGL J1258.4−1802                      | ... | fsrq  | PKS B1256−177            |
| J1258.7−2219  | 194.694 | −22.330 | 305.165 | 40.510  | 0.045      | 0.042      | 55     | 16.5     | 1.5      | 0.1             | 19.1     | 1.5             | 2.34          | 0.06                 | PL  | T   | ...   | 2FGL J1258.8−2223<br>1FGL J1258.7−2221<br>EGR J1259−2209    | ... | fsrq  | PKS 1256−220             |
| J1258.7+5137  | 194.699 | 51.628  | 120.182 | 65.461  | 0.103      | 0.094      | −41    | 4.9      | 0.2      | 0.1             | 2.6      | 0.6             | 2.16          | 0.19                 | PL  | ... | ...   | ...                                                         | ... | bcu   | NVSS<br>J125825+514225   |
| J1259.0−2310  | 194.772 | −23.183 | 305.217 | 39.655  | 0.068      | 0.056      | 6      | 8.2      | 0.6      | 0.1             | 6.8      | 1.1             | 2.03          | 0.12                 | PL  | ... | ...   | ...                                                         | ... | bcu   | PKS B1256−229            |
| J1259.3−8151  | 194.835 | −81.861 | 303.228 | −18.993 | 0.108      | 0.095      | −2     | 6.0      | 0.5      | 0.1             | 6.3      | 1.1             | 2.44          | 0.13                 | PL  | ... | ...   | ...                                                         | ... | ...   | ...                      |
| J1259.5−3231  | 194.886 | −32.519 | 304.912 | 30.322  | 0.259      | 0.154      | 81     | 6.0      | 0.4      | 0.1             | 8.0      | 1.2             | 2.71          | 0.13                 | PL  | ... | ...   | ...                                                         | ... | ...   | ...                      |
| J1259.8−3749  | 194.958 | −37.826 | 304.761 | 25.016  | 0.055      | 0.049      | 15     | 9.3      | 0.6      | 0.1             | 7.4      | 1.0             | 2.24          | 0.12                 | PL  | ... | ...   | 2FGL J1259.8−3749                                           | ... | bcu   | NVSS<br>J125949−374856   |
| J1300.2+1416  | 195.066 | 14.278  | 312.472 | 76.986  | 0.191      | 0.157      | 62     | 11.9     | 0.4      | 0.1             | 10.3     | 1.0             | 2.86          | 0.09                 | PL  | T   | ...   | 1FGL J1300.9−3745                                           | ... | fsrq  | OW 197                   |
| J1301.5+3333  | 195.394 | 33.562  | 104.781 | 83.206  | 0.116      | 0.101      | 5      | 7.9      | 0.4      | 0.1             | 5.1      | 0.8             | 2.40          | 0.12                 | PL  | ... | ...   | 2FGL J1301.6+3331                                           | ... | ...   | ...                      |
| J1301.6+0832  | 195.418 | 8.540   | 310.829 | 71.254  | 0.069      | 0.068      | 73     | 13.6     | 0.8      | 0.1             | 10.6     | 1.0             | 2.38          | 0.07                 | PL  | ... | ...   | 2FGL J1301.5+0835<br>1FGL J1301.8+0837                      | ... | PSR   | PSR J1301+0833           |
| J1302.3−3259  | 195.595 | −32.988 | 305.577 | 29.828  | 0.048      | 0.046      | −23    | 18.8     | 2.0      | 0.2             | 11.3     | 1.1             | 2.12          | ...                  | EC  | ... | ...   | 2FGL J1302.4−3257<br>1FGL J1302.3−3255                      | ... | PSR   | PSR J1302−3258           |
| J1302.6+5748  | 195.674 | 57.811  | 119.999 | 59.253  | 0.088      | 0.078      | −67    | 6.3      | 0.3      | 0.1             | 3.0      | 0.6             | 2.27          | 0.18                 | PL  | ... | ...   | ...                                                         | ... | bcu   | TXS 1300+580             |
| J1303.0−6312e | 195.750 | −63.200 | 304.235 | −0.358  | ...        | ...        | ...    | 7.6      | 1.6      | 0.4             | 22.7     | 3.8             | 1.64          | 0.12                 | PL  | ... | 1,3   | 2FGL J1303.7−6316c<br>...                                   | E   | PWN   | HESS J1303−631           |
| J1303.0+2435  | 195.752 | 24.595  | 349.347 | 86.368  | 0.037      | 0.036      | −42    | 28.5     | 1.9      | 0.1             | 21.7     | 1.2             | 2.18          | 0.04                 | PL  | T   | ...   | 1FHL J1302.9+2433<br>2FGL J1303.1+2435<br>1FGL J1303.0+2433 | ... | bll   | MG2 J130304+2434         |
| J1303.7−4619  | 195.947 | −46.319 | 305.156 | 16.500  | 0.100      | 0.072      | 0      | 9.4      | 0.7      | 0.1             | 8.8      | 1.1             | 2.39          | 0.10                 | PL  | T   | ...   | 2FGL J1303.5−4622<br>1FGL J1304.0−4622                      | ... | fsrq  | PMN J1303−4621           |
| J1304.2−2411  | 196.061 | −24.194 | 306.669 | 38.585  | 0.048      | 0.047      | −7     | 9.4      | 0.6      | 0.1             | 7.3      | 1.2             | 1.96          | 0.10                 | PL  | ... | ...   | 1FHL J1304.1−2413<br>2FGL J1304.1−2415                      | ... | bcu   | PMN J1304−2412           |
| J1304.3−5535  | 196.092 | −55.585 | 304.773 | 7.241   | 0.137      | 0.128      | 85     | 8.0      | 0.6      | 0.1             | 12.3     | 1.6             | 2.70          | 0.09                 | PL  | ... | ...   | 2FGL J1303.8−5537                                           | ... | bcu   | PMN J1303−5540           |
| J1304.3−4353  | 196.096 | −43.900 | 305.397 | 18.910  | 0.022      | 0.020      | −21    | 33.5     | 3.2      | 0.2             | 36.8     | 2.2             | 1.91          | 0.04                 | PL  | T   | ...   | 1FHL J1304.3−4354                                           | ... | bll   | 1RXS<br>J130421.2−435308 |
|               |         |         |         |         |            |            |        |          |          |                 |          |                 |               |                      |     |     |       | 2FGL J1304.3−4353<br>1FGL J1304.3−4352                      |     |       |                          |

Table 1—Continued

| Name 3FGL    | R.A.    | Decl.   | $l$     | $b$    | $\theta_1$ | $\theta_2$ | $\phi$ | $\sigma$ | $F_{35}$ | $\Delta F_{35}$ | $S_{25}$ | $\Delta S_{25}$ | $\Gamma_{25}$ | $\Delta \Gamma_{25}$ | Mod | Var | Flags | $\gamma$ -ray Assoc. | TeV | Class | ID or Assoc.          |
|--------------|---------|---------|---------|--------|------------|------------|--------|----------|----------|-----------------|----------|-----------------|---------------|----------------------|-----|-----|-------|----------------------|-----|-------|-----------------------|
|              |         |         |         |        |            |            |        |          |          |                 |          |                 |               |                      |     |     |       | 3EG J1300–4406       |     |       |                       |
| J1304.6+1200 | 196.171 | 12.006  | 315.189 | 74.562 | 0.209      | 0.147      | 26     | 5.4      | 0.4      | 0.1             | 4.6      | 0.9             | 2.37          | 0.14                 | PL  | ... | ...   | 2FGL J1305.0+1152    | ... | ...   | ...                   |
| J1304.8–0338 | 196.206 | –3.648  | 309.438 | 59.055 | 0.158      | 0.130      | –6     | 4.4      | 0.3      | 0.1             | 3.5      | 0.9             | 2.28          | 0.19                 | PL  | T   | ...   | ...                  | ... | fsrq  | PKS 1302–035          |
| J1304.9–2109 | 196.246 | –21.157 | 307.157 | 41.603 | 0.095      | 0.080      | –45    | 4.9      | 0.4      | 0.1             | 4.1      | 1.0             | 2.15          | 0.16                 | PL  | ... | ...   | 2FGL J1305.1–2110    | ... | bcu   | PKS B1302–208         |
| J1305.4–4926 | 196.370 | –49.434 | 305.278 | 13.374 | 0.068      | 0.050      | –25    | 12.9     | 1.0      | 0.1             | 13.8     | 1.2             | 2.43          | 0.07                 | PL  | ... | ...   | 2FGL J1305.8–4925    | ... | sbq   | NGC 4945              |
|              |         |         |         |        |            |            |        |          |          |                 |          |                 |               |                      |     |     |       | 1FGL J1305.4–4928    |     |       |                       |
| J1305.5+7854 | 196.381 | 78.910  | 122.071 | 38.195 | 0.082      | 0.072      | –2     | 9.4      | 0.4      | 0.1             | 4.9      | 0.6             | 2.38          | 0.10                 | PL  | ... | ...   | 2FGL J1305.7+7854    | ... | bll   | S5 1304+79            |
|              |         |         |         |        |            |            |        |          |          |                 |          |                 |               |                      |     |     |       | 1FGL J1306.0+7852    |     |       |                       |
| J1305.7–6241 | 196.434 | –62.686 | 304.572 | 0.140  | 0.037      | 0.034      | 67     | 11.1     | 2.8      | 0.3             | 31.2     | 3.9             | 2.10          | 0.08                 | PL  | ... | ...   | ...                  | ... | snr   | Kes 17                |
| J1306.4–6043 | 196.615 | –60.732 | 304.768 | 2.086  | 0.027      | 0.026      | 34     | 25.4     | 5.5      | 0.3             | 35.1     | 2.5             | 2.13          | ...                  | LP  | ... | ...   | 2FGL J1306.2–6044    | ... | ...   | ...                   |
|              |         |         |         |        |            |            |        |          |          |                 |          |                 |               |                      |     |     |       | 1FGL J1306.4–6038    |     |       |                       |
|              |         |         |         |        |            |            |        |          |          |                 |          |                 |               |                      |     |     |       | 3EG J1308–6112       |     |       |                       |
| J1306.8–2146 | 196.714 | –21.778 | 307.674 | 40.952 | 0.097      | 0.082      | –64    | 4.3      | 0.3      | 0.1             | 3.8      | 1.0             | 2.15          | 0.16                 | PL  | ... | ...   | ...                  | ... | bcu   | PKS 1304–215          |
| J1306.8–4031 | 196.725 | –40.533 | 306.105 | 22.244 | 0.071      | 0.066      | –4     | 15.0     | 0.9      | 0.1             | 14.7     | 1.1             | 2.54          | 0.07                 | PL  | ... | ...   | 2FGL J1306.9–4028    | ... | ...   | ...                   |
|              |         |         |         |        |            |            |        |          |          |                 |          |                 |               |                      |     |     |       | 1FGL J1307.0–4030    |     |       |                       |
| J1307.6–4300 | 196.918 | –43.001 | 306.085 | 19.772 | 0.022      | 0.022      | –55    | 23.7     | 2.0      | 0.1             | 23.5     | 1.9             | 1.84          | 0.06                 | PL  | ... | ...   | 1FHL J1307.7–4259    | ... | bcu   | 1RXS J130737.8–425940 |
|              |         |         |         |        |            |            |        |          |          |                 |          |                 |               |                      |     |     |       | 2FGL J1307.5–4300    |     |       |                       |
|              |         |         |         |        |            |            |        |          |          |                 |          |                 |               |                      |     |     |       | 1FGL J1307.6–4259    |     |       |                       |
| J1308.1–6707 | 197.043 | –67.120 | 304.562 | –4.301 | 0.058      | 0.047      | –26    | 16.3     | 1.8      | 0.2             | 24.8     | 1.8             | 2.45          | 0.06                 | PL  | T   | ...   | 2FGL J1307.6–6704    | ... | bcu   | PKS 1304–668          |
|              |         |         |         |        |            |            |        |          |          |                 |          |                 |               |                      |     |     |       | 1FGL J1307.3–6701    |     |       |                       |
| J1308.7+3545 | 197.185 | 35.761  | 100.886 | 80.615 | 0.159      | 0.094      | –58    | 10.9     | 0.6      | 0.1             | 7.0      | 0.8             | 2.36          | 0.09                 | PL  | T   | ...   | 2FGL J1308.5+3547    | ... | fsrq  | 5C 12.291             |
|              |         |         |         |        |            |            |        |          |          |                 |          |                 |               |                      |     |     |       | 1FGL J1308.5+3550    |     |       |                       |
| J1308.7–5738 | 197.199 | –57.639 | 305.263 | 5.154  | 0.226      | 0.182      | –14    | 5.4      | 0.5      | 0.1             | 9.5      | 1.7             | 2.68          | 0.14                 | PL  | ... | 1,4   | ...                  | ... | ...   | ...                   |
| J1309.0+0347 | 197.258 | 3.791   | 313.902 | 66.287 | 0.150      | 0.126      | 29     | 4.1      | 0.3      | 0.1             | 2.8      | 0.7             | 2.09          | 0.19                 | PL  | ... | ...   | ...                  | ... | ...   | ...                   |
| J1309.3+4304 | 197.345 | 43.075  | 111.227 | 73.643 | 0.027      | 0.023      | 83     | 29.0     | 1.7      | 0.1             | 19.9     | 1.4             | 1.94          | 0.05                 | PL  | ... | ...   | 1FHL J1309.3+4304    | ... | bll   | B3 1307+433           |
|              |         |         |         |        |            |            |        |          |          |                 |          |                 |               |                      |     |     |       | 2FGL J1309.4+4304    |     |       |                       |
|              |         |         |         |        |            |            |        |          |          |                 |          |                 |               |                      |     |     |       | 1FGL J1309.5+4304    |     |       |                       |
| J1309.5+1154 | 197.393 | 11.901  | 319.425 | 74.189 | 0.093      | 0.078      | –46    | 9.1      | 0.6      | 0.1             | 6.6      | 0.9             | 2.14          | 0.11                 | PL  | ... | ...   | 2FGL J1309.3+1154    | ... | bll   | 4C +12.46             |
|              |         |         |         |        |            |            |        |          |          |                 |          |                 |               |                      |     |     |       | 1FGL J1309.2+1156    |     |       |                       |
| J1310.2–1159 | 197.568 | –11.985 | 310.203 | 50.620 | 0.058      | 0.052      | –76    | 6.9      | 0.3      | 0.1             | 4.2      | 1.0             | 1.80          | 0.19                 | PL  | ... | ...   | ...                  | ... | bll   | TXS 1307–117          |
| J1310.6+2446 | 197.650 | 24.782  | 5.420   | 85.095 | 0.159      | 0.115      | 31     | 4.1      | 0.2      | 0.1             | 2.6      | 0.7             | 2.20          | 0.22                 | PL  | ... | ...   | ...                  | ... | bcu   | MG2 J131037+2447      |
| J1310.6+3222 | 197.657 | 32.370  | 85.623  | 83.307 | 0.026      | 0.024      | 37     | 52.0     | 3.7      | 0.2             | 37.5     | 1.5             | 2.25          | ...                  | LP  | T   | ...   | 1FHL J1310.6+3222    | ... | fsrq  | OP 313                |
|              |         |         |         |        |            |            |        |          |          |                 |          |                 |               |                      |     |     |       | 2FGL J1310.6+3222    |     |       |                       |
|              |         |         |         |        |            |            |        |          |          |                 |          |                 |               |                      |     |     |       | 1FGL J1310.6+3222    |     |       |                       |
|              |         |         |         |        |            |            |        |          |          |                 |          |                 |               |                      |     |     |       | 0FGL J1310.6+3220    |     |       |                       |

Table 1—Continued

| Name 3FGL    | R.A.    | Decl.   | $l$     | $b$    | $\theta_1$ | $\theta_2$ | $\phi$ | $\sigma$ | $F_{35}$ | $\Delta F_{35}$ | $S_{25}$ | $\Delta S_{25}$ | $\Gamma_{25}$ | $\Delta \Gamma_{25}$ | Mod | Var | Flags | $\gamma$ -ray Assoc.                                                          | TeV | Class | ID or Assoc.             |
|--------------|---------|---------|---------|--------|------------|------------|--------|----------|----------|-----------------|----------|-----------------|---------------|----------------------|-----|-----|-------|-------------------------------------------------------------------------------|-----|-------|--------------------------|
| J1310.7+5515 | 197.678 | 55.262  | 117.146 | 61.650 | 0.117      | 0.113      | 44     | 6.1      | 0.2      | 0.1             | 3.6      | 0.6             | 2.53          | 0.14                 | PL  | T   | ...   | ...                                                                           | ... | fsrq  | TXS 1308+554             |
| J1311.0+0036 | 197.771 | 0.614   | 313.829 | 63.069 | 0.076      | 0.060      | -69    | 4.7      | 0.2      | 0.1             | 2.7      | 1.0             | 1.55          | 0.28                 | PL  | ... | ...   | 1FHL J1310.9+0036<br>2FGL J1310.9+0036                                        | ... | bll   | RX J1311.1+0035          |
| J1311.8-3430 | 197.959 | -34.502 | 307.699 | 28.181 | 0.022      | 0.022      | -20    | 62.3     | 7.5      | 0.2             | 64.7     | 1.9             | 2.23          | ...                  | EC  | ... | ...   | 2FGL J1311.7-3429<br>1FGL J1311.7-3429<br>0FGL J1311.9-3419<br>3EG J1314-3431 | ... | PSR   | LAT PSR J1311-3430       |
| J1311.8-6230 | 197.968 | -62.507 | 305.288 | 0.271  | 0.075      | 0.061      | 21     | 9.3      | 2.6      | 0.3             | 36.9     | 4.3             | 2.46          | 0.07                 | PL  | ... | ...   | ...                                                                           | ... | ...   | ...                      |
| J1312.3+8513 | 198.091 | 85.225  | 122.420 | 31.882 | 0.100      | 0.084      | -2     | 5.9      | 0.3      | 0.1             | 4.2      | 0.8             | 2.57          | 0.16                 | PL  | ... | 1     | ...                                                                           | ... | ...   | ...                      |
| J1312.5-2155 | 198.126 | -21.932 | 309.378 | 40.676 | 0.038      | 0.035      | -69    | 20.8     | 1.8      | 0.1             | 20.0     | 1.5             | 2.07          | 0.05                 | PL  | ... | ...   | 1FHL J1312.2-2158<br>2FGL J1312.4-2157<br>1FGL J1312.4-2156                   | ... | bll   | PKS 1309-216             |
| J1312.7+4828 | 198.188 | 48.474  | 113.366 | 68.256 | 0.019      | 0.018      | 55     | 66.0     | 4.9      | 0.2             | 47.7     | 1.8             | 2.13          | ...                  | LP  | T   | ...   | 1FHL J1312.8+4827<br>2FGL J1312.8+4828<br>1FGL J1312.4+4827                   | ... | agn   | GB 1310+487              |
| J1312.7+0051 | 198.195 | 0.861   | 314.850 | 63.238 | 0.046      | 0.044      | 35     | 20.7     | 2.4      | 0.2             | 16.5     | 1.1             | 2.17          | ...                  | EC  | ... | ...   | 2FGL J1312.7+0051<br>1FGL J1312.6+0048                                        | ... | PSR   | PSR J1312.7+0051         |
| J1312.7-2349 | 198.197 | -23.823 | 309.201 | 38.789 | 0.050      | 0.041      | -89    | 9.8      | 0.6      | 0.1             | 7.3      | 1.3             | 1.80          | 0.12                 | PL  | ... | ...   | 2FGL J1312.9-2351                                                             | ... | bcu   | NVSS<br>J131248-235046   |
| J1312.8-0424 | 198.221 | -4.403  | 313.071 | 58.046 | 0.087      | 0.070      | 49     | 16.5     | 1.0      | 0.1             | 14.1     | 1.1             | 2.49          | 0.06                 | PL  | T   | ...   | 2FGL J1313.0-0425                                                             | ... | fsrq  | PKS B1310-041            |
| J1314.7-4237 | 198.694 | -42.627 | 307.499 | 20.038 | 0.129      | 0.097      | -27    | 4.5      | 0.4      | 0.1             | 3.9      | 1.1             | 2.08          | 0.21                 | PL  | ... | ...   | 1FHL J1314.9-4241                                                             | P   | bcu   | MS 13121-4221            |
| J1314.8+2349 | 198.714 | 23.826  | 2.218   | 83.769 | 0.040      | 0.038      | -72    | 21.9     | 1.4      | 0.1             | 15.8     | 1.2             | 2.05          | 0.06                 | PL  | ... | ...   | 1FHL J1315.0+2346<br>2FGL J1314.6+2348<br>1FGL J1314.7+2346                   | ... | bll   | TXS 1312+240             |
| J1315.1-5329 | 198.786 | -53.488 | 306.501 | 9.219  | 0.071      | 0.067      | 8      | 14.6     | 1.5      | 0.2             | 16.8     | 1.5             | 2.50          | ...                  | LP  | T   | ...   | 2FGL J1314.5-5330<br>1FGL J1314.9-5338                                        | ... | bcu   | PMN J1315-5334           |
| J1315.4+1130 | 198.869 | 11.515  | 323.973 | 73.397 | 0.153      | 0.112      | 1      | 4.3      | 0.3      | 0.1             | 2.9      | 0.8             | 1.96          | 0.26                 | PL  | ... | ...   | ...                                                                           | ... | bcu   | 1RXS<br>J131531.9+113327 |
| J1315.7-0732 | 198.947 | -7.549  | 313.448 | 54.825 | 0.051      | 0.042      | -17    | 12.9     | 0.8      | 0.1             | 9.3      | 1.1             | 2.02          | 0.09                 | PL  | T   | ...   | 1FHL J1315.7-0730<br>2FGL J1315.6-0730<br>1FGL J1315.6-0729                   | ... | ...   | ...                      |
| J1316.0-3338 | 199.000 | -33.649 | 308.773 | 28.944 | 0.044      | 0.038      | -20    | 25.3     | 2.3      | 0.1             | 28.3     | 1.5             | 2.32          | 0.04                 | PL  | T   | ...   | 1FHL J1315.9-3333<br>2FGL J1315.9-3339<br>1FGL J1316.1-3341                   | ... | fsrq  | PKS 1313-333             |
| J1316.2-6446 | 199.063 | -64.770 | 305.574 | -2.025 | 0.150      | 0.089      | 84     | 10.1     | 1.0      | 0.2             | 23.3     | 2.4             | 2.79          | 0.09                 | PL  | T   | ...   | 2FGL J1312.0-6458                                                             | ... | ...   | ...                      |
| J1317.6-6315 | 199.403 | -63.260 | 305.872 | -0.538 | 0.056      | 0.049      | -3     | 13.5     | 4.0      | 0.4             | 29.5     | 3.4             | 2.34          | ...                  | LP  | ... | ...   | 1FGL J1317.5-6318c                                                            | ... | ...   | ...                      |
| J1317.8+3429 | 199.463 | 34.500  | 87.003  | 80.704 | 0.180      | 0.172      | -23    | 6.1      | 0.3      | 0.1             | 4.1      | 0.7             | 2.58          | 0.14                 | PL  | ... | ...   | 2FGL J1317.9+3426                                                             | ... | fsrq  | S4 1315+34               |

Table 1—Continued

| Name 3FGL     | R.A.    | Decl.   | $l$     | $b$    | $\theta_1$ | $\theta_2$ | $\phi$ | $\sigma$ | $F_{35}$ | $\Delta F_{35}$ | $S_{25}$ | $\Delta S_{25}$ | $\Gamma_{25}$ | $\Delta \Gamma_{25}$ | Mod | Var | Flags | $\gamma$ -ray Assoc. | TeV | Class | ID or Assoc.           |
|---------------|---------|---------|---------|--------|------------|------------|--------|----------|----------|-----------------|----------|-----------------|---------------|----------------------|-----|-----|-------|----------------------|-----|-------|------------------------|
|               |         |         |         |        |            |            |        |          |          |                 |          |                 |               |                      |     |     |       | 1FGL J1317.8+3425    |     |       |                        |
| J1318.7–1232  | 199.694 | –12.541 | 313.297 | 49.780 | 0.095      | 0.068      | 43     | 8.4      | 0.5      | 0.1             | 6.9      | 1.0             | 2.35          | 0.11                 | PL  | ... | ...   | 2FGL J1318.9–1228    | ... | bcu   | PMN J1318–1235         |
| J1319.3+1402  | 199.837 | 14.050  | 330.787 | 75.390 | 0.086      | 0.076      | –6     | 4.3      | 0.2      | 0.1             | 2.2      | 0.7             | 1.87          | 0.24                 | PL  | ... | ...   | ...                  | ... | bll   | RX J1319.4+1405        |
| J1319.6+7759  | 199.903 | 77.998  | 121.051 | 39.027 | 0.060      | 0.051      | –68    | 9.1      | 0.3      | 0.1             | 4.2      | 0.8             | 1.79          | 0.13                 | PL  | ... | ...   | ...                  | ... | bcu   | NVSS<br>J131921+775823 |
| J1321.0+2215  | 200.269 | 22.263  | 358.672 | 81.697 | 0.058      | 0.054      | –85    | 20.6     | 1.3      | 0.1             | 17.4     | 1.2             | 2.42          | 0.06                 | PL  | T   | ...   | 2FGL J1321.1+2215    | ... | fsrq  | TXS 1318+225           |
|               |         |         |         |        |            |            |        |          |          |                 |          |                 |               |                      |     |     |       | 1FGL J1321.1+2214    |     |       |                        |
| J1321.7+8312  | 200.431 | 83.207  | 121.857 | 33.858 | 0.077      | 0.071      | –25    | 12.7     | 0.5      | 0.1             | 8.1      | 0.8             | 2.57          | 0.08                 | PL  | T   | ...   | 2FGL J1322.6+8313    | ... | fsrq  | S5 1322+83             |
|               |         |         |         |        |            |            |        |          |          |                 |          |                 |               |                      |     |     |       | 1FGL J1321.3+8310    |     |       |                        |
| J1322.3+0839  | 200.582 | 8.657   | 325.949 | 70.136 | 0.123      | 0.097      | –2     | 7.8      | 0.5      | 0.1             | 5.6      | 0.9             | 2.25          | 0.14                 | PL  | T   | ...   | 1FGL J1322.1+0838    | ... | bcu   | NVSS<br>J132210+084231 |
| J1322.6–1619  | 200.666 | –16.319 | 313.728 | 45.897 | 0.116      | 0.107      | –2     | 5.3      | 0.4      | 0.1             | 4.6      | 0.9             | 2.36          | 0.15                 | PL  | ... | ...   | ...                  | ... | bcu   | PMN J1322–1617         |
| J1322.8–0938  | 200.706 | –9.645  | 315.690 | 52.448 | 0.094      | 0.086      | 82     | 14.4     | 0.7      | 0.1             | 12.8     | 1.0             | 2.63          | 0.07                 | PL  | T   | ...   | 2FGL J1322.7–0938    | ... | fsrq  | PKS B1319–093          |
|               |         |         |         |        |            |            |        |          |          |                 |          |                 |               |                      |     |     |       | 1FGL J1322.7–0943    |     |       |                        |
| J1322.9+0435  | 200.733 | 4.597   | 322.751 | 66.249 | 0.075      | 0.067      | 42     | 6.1      | 0.3      | 0.1             | 3.5      | 0.9             | 1.74          | 0.20                 | PL  | ... | ...   | ...                  | ... | bll   | RBS 1257               |
| J1323.0+2942  | 200.751 | 29.712  | 55.203  | 82.596 | 0.042      | 0.036      | –88    | 17.7     | 1.1      | 0.1             | 12.9     | 1.1             | 2.15          | 0.07                 | PL  | ... | ...   | 1FHL J1322.9+2942    | ... | bcu   | 4C +29.48 ↗            |
|               |         |         |         |        |            |            |        |          |          |                 |          |                 |               |                      |     |     |       | 2FGL J1323.0+2941    |     |       |                        |
|               |         |         |         |        |            |            |        |          |          |                 |          |                 |               |                      |     |     |       | 1FGL J1323.1+2942    |     |       |                        |
| J1323.2–3901  | 200.810 | –39.025 | 309.658 | 23.431 | 0.130      | 0.125      | –21    | 5.6      | 0.4      | 0.1             | 6.3      | 1.2             | 2.52          | 0.14                 | PL  | ... | 1     | ...                  | ... | ...   | ...                    |
| J1323.9+1405  | 200.992 | 14.094  | 334.755 | 74.918 | 0.111      | 0.082      | –61    | 6.3      | 0.4      | 0.1             | 4.2      | 0.8             | 2.08          | 0.14                 | PL  | ... | ...   | ...                  | ... | bll   | RX J1323.9+1406        |
| J1324.0–4330e | 201.000 | –43.500 | 309.168 | 18.977 | ...        | ...        | ...    | 12.1     | 3.4      | 0.3             | 51.7     | 4.2             | 2.53          | 0.05                 | PL  | T   | 3,5   | 1FGL J1322.0–4515    | ... | RDG   | Cen A Lobes            |
|               |         |         |         |        |            |            |        |          |          |                 |          |                 |               |                      |     |     |       | 2FGL J1324.0–4330e   |     |       |                        |
|               |         |         |         |        |            |            |        |          |          |                 |          |                 |               |                      |     |     |       | 3EG J1324–4314       |     |       |                        |
| J1325.2–5411  | 201.314 | –54.186 | 307.921 | 8.358  | 0.104      | 0.091      | 56     | 7.0      | 0.8      | 0.1             | 10.8     | 1.7             | 2.47          | 0.10                 | PL  | ... | ...   | 2FGL J1324.4–5411    | ... | ...   | ...                    |
| J1325.4–4301  | 201.367 | –43.030 | 309.516 | 19.406 | 0.030      | 0.027      | 38     | 43.9     | 3.4      | 0.2             | 66.5     | 2.1             | 2.70          | 0.03                 | PL  | ... | ...   | 1FHL J1326.1–4303    | P   | RDG   | Cen A Core             |
|               |         |         |         |        |            |            |        |          |          |                 |          |                 |               |                      |     |     |       | 2FGL J1325.6–4300    |     |       |                        |
|               |         |         |         |        |            |            |        |          |          |                 |          |                 |               |                      |     |     |       | 1FGL J1325.6–4300    |     |       |                        |
|               |         |         |         |        |            |            |        |          |          |                 |          |                 |               |                      |     |     |       | 0FGL J1325.4–4303    |     |       |                        |
|               |         |         |         |        |            |            |        |          |          |                 |          |                 |               |                      |     |     |       | 3EG J1324–4314       |     |       |                        |
| J1326.1+2931  | 201.533 | 29.533  | 52.445  | 81.998 | 0.061      | 0.057      | 37     | 4.8      | 0.2      | 0.1             | 2.5      | 0.8             | 2.07          | 0.25                 | PL  | ... | ...   | ...                  | ... | bll   | TXS 1323+298           |
| J1326.2–4651  | 201.559 | –46.852 | 309.098 | 15.603 | 0.098      | 0.096      | 16     | 4.7      | 0.4      | 0.1             | 8.0      | 1.6             | 2.69          | 0.13                 | PL  | ... | ...   | ...                  | ... | ...   | ...                    |
| J1326.6–5256  | 201.663 | –52.939 | 308.299 | 9.565  | 0.045      | 0.040      | –45    | 21.0     | 2.3      | 0.2             | 29.5     | 1.7             | 2.37          | 0.05                 | PL  | T   | ...   | 1FHL J1327.1–5258    | ... | bll   | PMN J1326–5256         |
|               |         |         |         |        |            |            |        |          |          |                 |          |                 |               |                      |     |     |       | 2FGL J1326.7–5254    |     |       |                        |
|               |         |         |         |        |            |            |        |          |          |                 |          |                 |               |                      |     |     |       | 1FGL J1327.0–5257    |     |       |                        |
|               |         |         |         |        |            |            |        |          |          |                 |          |                 |               |                      |     |     |       | 0FGL J1326.6–5302    |     |       |                        |
| J1326.7–4727  | 201.695 | –47.465 | 309.103 | 14.983 | 0.054      | 0.052      | 40     | 11.3     | 2.0      | 0.2             | 9.7      | 1.3             | 2.24          | ...                  | LP  | ... | ...   | 2FGL J1326.4–4729    | ... | glc   | Omega Cen              |
| J1326.8+2211  | 201.722 | 22.184  | 3.304   | 80.553 | 0.048      | 0.046      | 84     | 26.2     | 1.7      | 0.1             | 19.8     | 1.3             | 2.45          | ...                  | LP  | T   | ...   | 2FGL J1326.8+2210    | ... | fsrq  | B2 1324+22             |

Table 1—Continued

| Name 3FGL    | R.A.    | Decl.   | $l$     | $b$    | $\theta_1$ | $\theta_2$ | $\phi$ | $\sigma$ | $F_{35}$ | $\Delta F_{35}$ | $S_{25}$ | $\Delta S_{25}$ | $\Gamma_{25}$ | $\Delta \Gamma_{25}$ | Mod | Var | Flags | $\gamma$ -ray Assoc. | TeV | Class | ID or Assoc.             |
|--------------|---------|---------|---------|--------|------------|------------|--------|----------|----------|-----------------|----------|-----------------|---------------|----------------------|-----|-----|-------|----------------------|-----|-------|--------------------------|
| J1327.9+2524 | 201.990 | 25.401  | 23.069  | 81.634 | 0.069      | 0.062      | −27    | 4.3      | 0.1      | 0.1             | 1.9      | 0.7             | 1.68          | 0.31                 | PL  | ... | ...   | 1FGL J1326.6+2213    | ... | bll   | NVSS<br>J132758+252750   |
| J1328.5−4728 | 202.147 | −47.481 | 309.414 | 14.922 | 0.030      | 0.027      | 22     | 12.1     | 0.8      | 0.2             | 10.9     | 1.7             | 1.70          | 0.13                 | PL  | ... | 10    | 1FHL J1328.5−4728    | ... | bcu   | 1WGA J1328.6−4727        |
|              |         |         |         |        |            |            |        |          |          |                 |          |                 |               |                      |     |     |       | 2FGL J1328.5−4728    |     |       |                          |
| J1328.9−5607 | 202.240 | −56.131 | 308.177 | 6.358  | 0.022      | 0.022      | −46    | 46.1     | 6.8      | 0.2             | 70.5     | 2.4             | 2.34          | ...                  | LP  | T   | ...   | 1FGL J1328.2−4729    |     |       |                          |
|              |         |         |         |        |            |            |        |          |          |                 |          |                 |               |                      |     |     |       | 1FHL J1328.7−5604    | ... | bcu   | PMN J1329−5608           |
|              |         |         |         |        |            |            |        |          |          |                 |          |                 |               |                      |     |     |       | 2FGL J1329.2−5608    |     |       |                          |
|              |         |         |         |        |            |            |        |          |          |                 |          |                 |               |                      |     |     |       | 1FGL J1329.2−5605    |     |       |                          |
|              |         |         |         |        |            |            |        |          |          |                 |          |                 |               |                      |     |     |       | 0FGL J1328.8−5604    |     |       |                          |
| J1329.1−0536 | 202.299 | −5.608  | 319.910 | 56.014 | 0.178      | 0.114      | 0      | 5.6      | 0.5      | 0.1             | 6.4      | 1.5             | 2.35          | 0.17                 | PL  | ... | 9     | 2FGL J1329.3−0528    | ... | ...   | ...                      |
| J1329.8−6109 | 202.468 | −61.162 | 307.551 | 1.365  | 0.052      | 0.050      | −39    | 11.9     | 2.5      | 0.3             | 16.5     | 2.4             | 2.24          | ...                  | LP  | ... | ...   | 2FGL J1329.7−6108    | ... | ...   | ...                      |
| J1330.0−3818 | 202.506 | −38.313 | 311.203 | 23.938 | 0.330      | 0.215      | −59    | 5.4      | 0.3      | 0.1             | 6.9      | 1.2             | 2.78          | 0.14                 | PL  | ... | ...   | ...                  | ... | fsrq  | Tol 1326−379             |
| J1330.0+4437 | 202.510 | 44.631  | 101.591 | 70.863 | 0.100      | 0.089      | 37     | 7.3      | 0.3      | 0.1             | 3.6      | 0.7             | 2.03          | 0.14                 | PL  | ... | ...   | ...                  | ... | bll   | 1RXS<br>J133021.4+444117 |
| J1330.1−7002 | 202.538 | −70.046 | 306.249 | −7.424 | 0.032      | 0.031      | −61    | 32.5     | 3.7      | 0.2             | 37.5     | 2.0             | 2.35          | ...                  | LP  | T   | ...   | 1FHL J1330.4−7005    | ... | bcu   | PKS 1326−697             |
|              |         |         |         |        |            |            |        |          |          |                 |          |                 |               |                      |     |     |       | 2FGL J1330.1−7002    |     |       |                          |
|              |         |         |         |        |            |            |        |          |          |                 |          |                 |               |                      |     |     |       | 1FGL J1330.7−7006    |     |       |                          |
| J1330.4+5641 | 202.612 | 56.688  | 112.329 | 59.630 | 0.556      | 0.446      | 43     | 5.1      | 0.1      | 0.0             | 3.4      | 0.7             | 3.00          | 0.22                 | PL  | ... | 1,9   | ...                  | ... | ...   | ...                      |
| J1330.5+3023 | 202.636 | 30.389  | 56.068  | 80.835 | 0.308      | 0.185      | 47     | 5.2      | 0.2      | 0.1             | 4.1      | 0.8             | 2.60          | 0.16                 | PL  | ... | ...   | ...                  | ... | css   | 3C 286                   |
| J1330.6+7002 | 202.669 | 70.036  | 118.065 | 46.720 | 0.044      | 0.044      | 47     | 10.9     | 0.4      | 0.1             | 4.6      | 0.8             | 1.84          | 0.12                 | PL  | ... | ...   | 2FGL J1330.9+7001    | ... | bll   | NVSS<br>J133025+700141   |
|              |         |         |         |        |            |            |        |          |          |                 |          |                 |               |                      |     |     |       | 1FGL J1331.0+6957    |     |       |                          |
| J1330.9+5201 | 202.745 | 52.029  | 108.982 | 64.015 | 0.074      | 0.063      | −85    | 6.1      | 0.3      | 0.1             | 3.1      | 0.7             | 2.25          | 0.20                 | PL  | ... | ...   | 1FGL J1331.0+5202    | ... | bcu   | 87GB<br>132842.6+521750  |
| J1331.1−1328 | 202.787 | −13.482 | 317.519 | 48.262 | 0.122      | 0.104      | −67    | 5.5      | 0.5      | 0.1             | 6.5      | 1.4             | 2.37          | 0.13                 | PL  | T   | 5     | ...                  | ... | bcu   | PMN J1331−1326           |
| J1331.5+1711 | 202.884 | 17.198  | 348.019 | 76.419 | 0.164      | 0.132      | −89    | 9.1      | 0.4      | 0.1             | 7.5      | 0.9             | 2.76          | 0.13                 | PL  | ... | ...   | 3EG J1329+1708       | ... | bll   | TXS 1329+174             |
| J1331.8+4718 | 202.972 | 47.303  | 104.129 | 68.321 | 0.161      | 0.132      | 46     | 8.6      | 0.4      | 0.1             | 5.6      | 0.7             | 2.53          | 0.10                 | PL  | T   | ...   | 2FGL J1332.7+4725    | ... | fsrq  | B3 1330+476              |
|              |         |         |         |        |            |            |        |          |          |                 |          |                 |               |                      |     |     |       | 1FGL J1332.9+4728    |     |       |                          |
| J1332.0−0508 | 203.015 | −5.148  | 321.366 | 56.263 | 0.029      | 0.028      | −56    | 49.7     | 4.7      | 0.2             | 65.5     | 2.0             | 2.50          | ...                  | LP  | T   | ...   | 1FHL J1332.0−0508    | ... | fsrq  | PKS 1329−049             |
|              |         |         |         |        |            |            |        |          |          |                 |          |                 |               |                      |     |     |       | 2FGL J1332.0−0508    |     |       |                          |
|              |         |         |         |        |            |            |        |          |          |                 |          |                 |               |                      |     |     |       | 1FGL J1331.9−0506    |     |       |                          |
|              |         |         |         |        |            |            |        |          |          |                 |          |                 |               |                      |     |     |       | 0FGL J1331.7−0506    |     |       |                          |
| J1332.6−1256 | 203.158 | −12.939 | 318.241 | 48.705 | 0.044      | 0.041      | −26    | 19.3     | 1.9      | 0.1             | 25.7     | 1.8             | 2.42          | 0.05                 | PL  | T   | ...   | 2FGL J1332.5−1255    | ... | fsrq  | PMN J1332−1256           |
|              |         |         |         |        |            |            |        |          |          |                 |          |                 |               |                      |     |     |       | 1FGL J1332.6−1255    |     |       |                          |
| J1332.8+2723 | 203.209 | 27.395  | 36.961  | 80.799 | 0.106      | 0.090      | −84    | 9.4      | 0.5      | 0.1             | 5.9      | 0.8             | 2.38          | 0.11                 | PL  | T   | ...   | 2FGL J1332.7+2726    | ... | fsrq  | MG2 J133305+2725         |
| J1333.7+5057 | 203.426 | 50.954  | 107.154 | 64.860 | 0.062      | 0.059      | 54     | 14.9     | 0.7      | 0.1             | 10.1     | 0.9             | 2.50          | 0.07                 | PL  | T   | ...   | 2FGL J1333.5+5058    | ... | fsrq  | CLASS J1333+5057         |
|              |         |         |         |        |            |            |        |          |          |                 |          |                 |               |                      |     |     |       | 1FGL J1333.2+5056    |     |       |                          |
|              |         |         |         |        |            |            |        |          |          |                 |          |                 |               |                      |     |     |       | 0FGL J1333.3+5058    |     |       |                          |

Table 1—Continued

| Name 3FGL    | R.A.    | Decl.   | $l$     | $b$    | $\theta_1$ | $\theta_2$ | $\phi$ | $\sigma$ | $F_{35}$ | $\Delta F_{35}$ | $S_{25}$ | $\Delta S_{25}$ | $\Gamma_{25}$ | $\Delta \Gamma_{25}$ | Mod | Var | Flags  | $\gamma$ -ray Assoc.                                        | TeV | Class | ID or Assoc.                |
|--------------|---------|---------|---------|--------|------------|------------|--------|----------|----------|-----------------|----------|-----------------|---------------|----------------------|-----|-----|--------|-------------------------------------------------------------|-----|-------|-----------------------------|
| J1333.8–4417 | 203.454 | –44.289 | 310.884 | 17.928 | 0.296      | 0.275      | –64    | 5.6      | 0.4      | 0.1             | 7.5      | 1.4             | 2.69          | 0.15                 | PL  | ... | ...    | ...                                                         | ... | ...   | ...                         |
| J1334.3–4152 | 203.587 | –41.868 | 311.431 | 20.294 | 0.062      | 0.061      | –61    | 4.2      | 0.3      | 0.1             | 2.8      | 1.1             | 2.01          | 0.33                 | PL  | ... | ...    | ...                                                         | ... | ...   | ...                         |
| J1335.1–5655 | 203.783 | –56.924 | 308.895 | 5.441  | 0.094      | 0.060      | –70    | 8.2      | 1.0      | 0.1             | 12.9     | 1.9             | 2.34          | 0.10                 | PL  | ... | ...    | 2FGL J1335.4–5658                                           | ... | ...   | ...                         |
| J1335.2–4056 | 203.808 | –40.935 | 311.784 | 21.182 | 0.116      | 0.088      | –61    | 7.2      | 0.5      | 0.1             | 10.1     | 1.4             | 2.68          | 0.11                 | PL  | ... | ...    | 2FGL J1335.3–4058                                           | ... | ...   | ...                         |
| J1335.4–2949 | 203.853 | –29.829 | 314.191 | 32.079 | 0.059      | 0.057      | 49     | 6.9      | 0.4      | 0.1             | 4.6      | 0.9             | 2.05          | 0.14                 | PL  | ... | ...    | ...                                                         | ... | bll   | 1ES 1332–295                |
| J1337.6–1257 | 204.415 | –12.957 | 320.023 | 48.375 | 0.052      | 0.051      | –56    | 19.1     | 1.6      | 0.1             | 17.3     | 1.4             | 2.44          | ...                  | LP  | T   | ...    | 2FGL J1337.7–1257<br>1FGL J1337.7–1255<br>EGR J1337–1310    | ... | fsrq  | PKS 1335–127                |
| J1338.6–2403 | 204.666 | –24.054 | 316.566 | 37.564 | 0.136      | 0.112      | 25     | 7.9      | 0.5      | 0.1             | 7.3      | 1.0             | 2.58          | 0.11                 | PL  | ... | ...    | ...                                                         | ... | bcu   | PKS 1336–237                |
| J1338.9+6532 | 204.743 | 65.542  | 115.169 | 50.864 | 0.463      | 0.364      | 24     | 7.3      | 0.1      | 0.0             | 4.5      | 0.6             | 3.02          | 0.14                 | PL  | ... | ...    | ...                                                         | ... | fsrq  | 87GB<br>133543.8+654752     |
| J1339.0+1153 | 204.755 | 11.892  | 341.471 | 71.111 | 0.047      | 0.045      | 74     | 11.5     | 0.7      | 0.1             | 7.5      | 1.0             | 1.97          | 0.10                 | PL  | ... | ...    | 2FGL J1338.9+1152                                           | ... | bll   | SDSS<br>J133859.05+115316.7 |
| J1339.8–0133 | 204.971 | –1.556  | 326.990 | 59.034 | 0.352      | 0.221      | 64     | 5.0      | 0.3      | 0.1             | 4.4      | 0.9             | 2.47          | 0.14                 | PL  | ... | ...    | ...                                                         | ... | fsrq  | PKS 1337–013                |
| J1340.6+4412 | 205.164 | 44.212  | 96.047  | 70.257 | 0.076      | 0.062      | 9      | 5.8      | 0.3      | 0.1             | 2.9      | 0.8             | 1.93          | 0.25                 | PL  | ... | ...    | 2FGL J1340.5+4407<br>1FGL J1340.6+4406                      | ... | bll   | RX J1340.4+4410             |
| J1340.6–0408 | 205.166 | –4.137  | 325.619 | 56.551 | 0.096      | 0.083      | 14     | 6.7      | 0.4      | 0.1             | 4.8      | 0.9             | 1.98          | 0.13                 | PL  | ... | ...    | 2FGL J1340.5–0412                                           | ... | bcu   | NVSS<br>J134042–041006      |
| J1341.0+3955 | 205.263 | 39.918  | 87.266  | 73.588 | 0.125      | 0.111      | –33    | 5.5      | 0.2      | 0.1             | 3.3      | 0.7             | 2.54          | 0.18                 | PL  | ... | ...    | 1FGL J1340.5–0413<br>1FGL J1341.3+3951                      | ... | bll   | SDSS<br>J134105.10+395945.4 |
| J1341.5+5517 | 205.385 | 55.293  | 108.453 | 60.404 | 0.126      | 0.102      | –28    | 6.0      | 0.2      | 0.1             | 3.5      | 0.7             | 2.56          | 0.17                 | PL  | ... | ...    | ...                                                         | ... | bll   | SBS 1339+554                |
| J1341.9–2053 | 205.490 | –20.895 | 318.504 | 40.444 | 0.167      | 0.128      | –37    | 12.4     | 0.7      | 0.1             | 12.3     | 1.1             | 2.65          | 0.08                 | PL  | T   | ...    | 2FGL J1341.3–2048<br>1FGL J1341.1–2045                      | ... | fsrq  | PKS B1339–206               |
| J1342.4–6904 | 205.611 | –69.071 | 307.485 | –6.652 | 0.193      | 0.141      | 61     | 4.5      | 0.4      | 0.1             | 7.2      | 1.7             | 2.64          | 0.17                 | PL  | ... | 4      | ...                                                         | ... | ...   | ...                         |
| J1342.7+0945 | 205.678 | 9.766   | 340.215 | 68.840 | 0.121      | 0.087      | –22    | 5.2      | 0.3      | 0.1             | 3.5      | 0.9             | 1.87          | 0.16                 | PL  | ... | ...    | ...                                                         | ... | bcu   | NVSS<br>J134240+094752      |
| J1343.6+5753 | 205.912 | 57.899  | 109.884 | 57.887 | 0.124      | 0.100      | –89    | 4.5      | 0.2      | 0.0             | 2.4      | 0.6             | 2.41          | 0.23                 | PL  | ... | ...    | 1FGL J1342.7+5753                                           | ... | fsrq  | 1RXS<br>J134357.9+575426    |
| J1344.2–1724 | 206.051 | –17.401 | 320.453 | 43.668 | 0.030      | 0.027      | 8      | 33.1     | 3.2      | 0.2             | 28.4     | 1.6             | 2.18          | ...                  | LP  | T   | ...    | 1FHL J1344.0–1722<br>2FGL J1344.2–1723<br>1FGL J1344.2–1723 | ... | fsrq  | PMN J1344–1723              |
| J1344.5–3655 | 206.126 | –36.930 | 314.585 | 24.739 | 0.069      | 0.058      | 10     | 5.7      | 0.4      | 0.1             | 4.4      | 1.0             | 2.18          | 0.17                 | PL  | ... | ...    | ...                                                         | ... | bcu   | PKS 1341–366                |
| J1345.1–6224 | 206.298 | –62.412 | 309.111 | –0.187 | 0.080      | 0.068      | –13    | 10.5     | 3.4      | 0.4             | 48.4     | 4.2             | 2.47          | 0.05                 | PL  | ... | 3,5,10 | ...                                                         | ... | spp   | ...                         |
| J1345.1+1949 | 206.300 | 19.827  | 5.123   | 75.688 | 0.247      | 0.184      | 63     | 4.8      | 0.2      | 0.1             | 4.0      | 0.8             | 2.60          | 0.18                 | PL  | ... | ...    | ...                                                         | ... | ...   | ...                         |
| J1345.6+4453 | 206.401 | 44.894  | 95.095  | 69.193 | 0.019      | 0.019      | 44     | 75.8     | 6.5      | 0.2             | 71.6     | 1.9             | 2.29          | ...                  | LP  | T   | ...    | 2FGL J1345.4+4453<br>1FGL J1345.4+4453                      | ... | fsrq  | B3 1343+451                 |
| J1345.8+0704 | 206.462 | 7.080   | 338.192 | 66.153 | 0.066      | 0.058      | –53    | 15.9     | 1.0      | 0.1             | 12.5     | 1.0             | 2.31          | 0.06                 | PL  | T   | ...    | 2FGL J1345.9+0706<br>1FGL J1346.0+0703                      | ... | fsrq  | TXS 1343+073                |
| J1345.9–3357 | 206.497 | –33.964 | 315.675 | 27.554 | 0.161      | 0.134      | –65    | 6.5      | 0.4      | 0.1             | 5.9      | 0.9             | 2.47          | 0.14                 | PL  | ... | ...    | 2FGL J1345.8–3356                                           | ... | bcu   | NVSS<br>J134543–335643      |

Table 1—Continued

| Name 3FGL    | R.A.    | Decl.   | $l$     | $b$    | $\theta_1$ | $\theta_2$ | $\phi$ | $\sigma$ | $F_{35}$ | $\Delta F_{35}$ | $S_{25}$ | $\Delta S_{25}$ | $\Gamma_{25}$ | $\Delta \Gamma_{25}$ | Mod | Var | Flags | $\gamma$ -ray Assoc. | TeV | Class | ID or Assoc.     |
|--------------|---------|---------|---------|--------|------------|------------|--------|----------|----------|-----------------|----------|-----------------|---------------|----------------------|-----|-----|-------|----------------------|-----|-------|------------------|
| J1346.2–2608 | 206.570 | –26.140 | 318.010 | 35.121 | 0.128      | 0.099      | 86     | 6.5      | 0.4      | 0.1             | 5.6      | 0.9             | 2.33          | 0.12                 | PL  | ... | ...   | 2FGL J1346.0–2605    | ... | ...   | ...              |
| J1346.6–6027 | 206.652 | –60.454 | 309.687 | 1.692  | 0.055      | 0.047      | 66     | 10.4     | 2.0      | 0.2             | 24.9     | 3.0             | 2.32          | 0.09                 | PL  | ... | ...   | 2FGL J1346.6–6027    | ... | rdg   | Cen B            |
| J1346.9–2958 | 206.745 | –29.972 | 317.025 | 31.375 | 0.074      | 0.056      | –20    | 8.2      | 0.5      | 0.1             | 6.7      | 1.3             | 1.74          | 0.13                 | PL  | ... | ...   | 2FGL J1347.0–2956    | ... | bcu   | NVSS             |
|              |         |         |         |        |            |            |        |          |          |                 |          |                 |               |                      |     |     |       |                      |     |       | J134706–295840   |
| J1347.6–3754 | 206.924 | –37.903 | 315.015 | 23.645 | 0.064      | 0.060      | –27    | 13.1     | 0.9      | 0.1             | 13.6     | 1.2             | 2.49          | 0.07                 | PL  | T   | ...   | 2FGL J1347.7–3752    | ... | fsrq  | PMN J1347–3750   |
|              |         |         |         |        |            |            |        |          |          |                 |          |                 |               |                      |     |     |       | 1FGL J1347.8–3751    |     |       |                  |
| J1348.5–7150 | 207.142 | –71.839 | 307.404 | –9.465 | 0.239      | 0.130      | –46    | 5.2      | 0.4      | 0.1             | 6.6      | 1.3             | 2.64          | 0.18                 | PL  | ... | ...   | ...                  | ... | ...   | ...              |
| J1348.5–5833 | 207.149 | –58.563 | 310.342 | 3.484  | 0.128      | 0.105      | –11    | 7.1      | 0.6      | 0.1             | 14.5     | 2.1             | 2.79          | 0.13                 | PL  | ... | 1,4   | ...                  | ... | ...   | ...              |
| J1349.6–1133 | 207.407 | –11.560 | 324.878 | 48.817 | 0.054      | 0.051      | 12     | 18.4     | 1.3      | 0.1             | 17.6     | 1.2             | 2.39          | 0.06                 | PL  | T   | ...   | ...                  | ... | fsrq  | PKS 1346–112     |
| J1350.4–6224 | 207.622 | –62.412 | 309.710 | –0.320 | 0.040      | 0.036      | –79    | 12.3     | 4.7      | 0.5             | 25.0     | 3.2             | 2.18          | ...                  | LP  | ... | 3     | 2FGL J1349.9–6222    | ... | ...   | ...              |
| J1350.8+3035 | 207.704 | 30.598  | 51.395  | 76.556 | 0.062      | 0.051      | –44    | 20.2     | 1.0      | 0.1             | 13.4     | 0.9             | 2.37          | 0.05                 | PL  | T   | ...   | 2FGL J1350.8+3035    | ... | fsrq  | B2 1348+30B      |
|              |         |         |         |        |            |            |        |          |          |                 |          |                 |               |                      |     |     |       | 1FGL J1351.0+3035    |     |       |                  |
| J1351.1–2743 | 207.793 | –27.720 | 318.773 | 33.307 | 0.098      | 0.082      | –2     | 5.4      | 0.4      | 0.1             | 4.6      | 1.0             | 2.38          | 0.15                 | PL  | ... | 1     | 2FGL J1351.1–2749    | ... | ...   | ...              |
| J1351.1+0030 | 207.794 | 0.514   | 333.717 | 59.766 | 0.128      | 0.091      | –35    | 7.3      | 0.5      | 0.1             | 5.7      | 0.9             | 2.31          | 0.13                 | PL  | T   | ...   | 2FGL J1351.1+0032    | ... | fsrq  | PKS 1348+007     |
| J1351.4+1115 | 207.851 | 11.267  | 347.440 | 68.783 | 0.037      | 0.034      | 88     | 12.9     | 0.7      | 0.1             | 8.9      | 1.4             | 1.71          | 0.10                 | PL  | ... | ...   | 1FHL J1351.4+1115    | ... | bll   | RX J1351.3+1115  |
|              |         |         |         |        |            |            |        |          |          |                 |          |                 |               |                      |     |     |       | 2FGL J1351.4+1115    |     |       |                  |
|              |         |         |         |        |            |            |        |          |          |                 |          |                 |               |                      |     |     |       | 1FGL J1351.5+1115    |     |       |                  |
| J1351.7–2913 | 207.927 | –29.226 | 318.419 | 31.826 | 0.079      | 0.072      | –44    | 9.0      | 0.6      | 0.1             | 8.5      | 1.1             | 2.40          | 0.09                 | PL  | T   | ...   | 2FGL J1351.3–2909    | ... | bcu   | PKS 1348–289     |
| J1351.8–1524 | 207.960 | –15.407 | 323.742 | 45.011 | 0.089      | 0.084      | 9      | 4.4      | 0.3      | 0.1             | 3.9      | 1.1             | 2.40          | 0.20                 | PL  | ... | ...   | 1FGL J1351.8–1523    | ... | ...   | ...              |
| J1353.1–4414 | 208.283 | –44.245 | 314.440 | 17.244 | 0.078      | 0.075      | 27     | 9.8      | 0.6      | 0.1             | 9.8      | 1.1             | 2.59          | 0.10                 | PL  | ... | ...   | 2FGL J1352.6–4413    | ... | bll   | PKS 1349–439     |
| J1353.2+1435 | 208.317 | 14.600  | 355.008 | 70.915 | 0.067      | 0.054      | 16     | 10.7     | 0.6      | 0.1             | 7.5      | 0.9             | 2.34          | 0.10                 | PL  | ... | ...   | 2FGL J1353.3+1435    | ... | bll   | OP 186           |
|              |         |         |         |        |            |            |        |          |          |                 |          |                 |               |                      |     |     |       | 1FGL J1353.3+1434    |     |       |                  |
| J1353.5–6640 | 208.390 | –66.667 | 309.039 | –4.534 | 0.039      | 0.035      | 55     | 10.0     | 0.8      | 0.1             | 9.6      | 1.4             | 1.91          | 0.10                 | PL  | ... | ...   | 1FHL J1353.0–6642    | ... | bll   | 1RXS             |
|              |         |         |         |        |            |            |        |          |          |                 |          |                 |               |                      |     |     |       |                      |     |       | J135341.1–664002 |
|              |         |         |         |        |            |            |        |          |          |                 |          |                 |               |                      |     |     |       | 2FGL J1353.5–6640    |     |       |                  |
|              |         |         |         |        |            |            |        |          |          |                 |          |                 |               |                      |     |     |       | 1FGL J1353.6–6640    |     |       |                  |
| J1354.5+3705 | 208.632 | 37.087  | 73.650  | 73.376 | 0.106      | 0.087      | 79     | 7.8      | 0.4      | 0.1             | 4.5      | 0.7             | 2.26          | 0.12                 | PL  | ... | ...   | 2FGL J1354.5+3703    | ... | bll   | FIRST            |
|              |         |         |         |        |            |            |        |          |          |                 |          |                 |               |                      |     |     |       |                      |     |       | J135426.6+370654 |
| J1355.0–1044 | 208.752 | –10.738 | 327.202 | 49.114 | 0.092      | 0.080      | –18    | 11.6     | 0.8      | 0.1             | 10.8     | 1.1             | 2.39          | 0.08                 | PL  | T   | ...   | 2FGL J1354.7–1047    | ... | fsrq  | PKS 1352–104     |
|              |         |         |         |        |            |            |        |          |          |                 |          |                 |               |                      |     |     |       | 1FGL J1354.9–1041    |     |       |                  |
|              |         |         |         |        |            |            |        |          |          |                 |          |                 |               |                      |     |     |       | 0FGL J1355.0–1044    |     |       |                  |
| J1356.3–4029 | 209.081 | –40.488 | 316.062 | 20.723 | 0.103      | 0.067      | 56     | 5.7      | 0.4      | 0.1             | 4.3      | 1.0             | 2.06          | 0.18                 | PL  | ... | ...   | ...                  | ... | bcu   | SUMSS            |
|              |         |         |         |        |            |            |        |          |          |                 |          |                 |               |                      |     |     |       |                      |     |       | J135625–402820   |
| J1356.6–6428 | 209.164 | –64.480 | 309.886 | –2.492 | 0.067      | 0.055      | –75    | 17.9     | 2.6      | 0.2             | 41.8     | 2.5             | 2.56          | 0.05                 | PL  | ... | ...   | 2FGL J1356.0–6436    | E   | PSR   | PSR J1357–6429   |
|              |         |         |         |        |            |            |        |          |          |                 |          |                 |               |                      |     |     |       | ...                  |     |       |                  |
| J1357.5+0125 | 209.399 | 1.433   | 337.391 | 59.803 | 0.148      | 0.095      | 40     | 5.8      | 0.4      | 0.1             | 4.6      | 1.0             | 2.14          | 0.17                 | PL  | ... | ...   | 2FGL J1358.0+0137    | ... | bll   | RX J1357.6+0128  |
| J1357.6+7643 | 209.407 | 76.722  | 118.050 | 39.772 | 0.107      | 0.081      | –15    | 12.8     | 0.5      | 0.1             | 7.5      | 0.7             | 2.48          | 0.09                 | PL  | T   | ...   | 2FGL J1358.1+7644    | ... | fsrq  | S5 1357+76       |
|              |         |         |         |        |            |            |        |          |          |                 |          |                 |               |                      |     |     |       | 1FGL J1358.1+7646    |     |       |                  |
| J1358.5–6025 | 209.643 | –60.430 | 311.127 | 1.369  | 0.056      | 0.052      | 7      | 15.4     | 4.1      | 0.3             | 42.0     | 3.7             | 2.48          | ...                  | LP  | ... | ...   | 2FGL J1358.8–6027c   | ... | ...   | ...              |



Table 1—Continued

| Name 3FGL    | R.A.    | Decl.   | $l$     | $b$    | $\theta_1$ | $\theta_2$ | $\phi$ | $\sigma$ | $F_{35}$ | $\Delta F_{35}$ | $S_{25}$ | $\Delta S_{25}$ | $\Gamma_{25}$ | $\Delta \Gamma_{25}$ | Mod | Var | Flags | $\gamma$ -ray Assoc. | TeV | Class | ID or Assoc.            |
|--------------|---------|---------|---------|--------|------------|------------|--------|----------|----------|-----------------|----------|-----------------|---------------|----------------------|-----|-----|-------|----------------------|-----|-------|-------------------------|
| J1359.0+5544 | 209.765 | 55.746  | 104.463 | 58.891 | 0.081      | 0.067      | 42     | 17.4     | 0.6      | 0.1             | 10.2     | 0.7             | 2.59          | 0.07                 | PL  | T   | ...   | 2FGL J1359.4+5541    | ... | fsrq  | 87GB<br>135720.6+555936 |
|              |         |         |         |        |            |            |        |          |          |                 |          |                 |               |                      |     |     |       | 1FGL J1359.1+5539    |     |       |                         |
| J1359.2+0204 | 209.808 | 2.070   | 338.744 | 60.140 | 0.195      | 0.147      | -15    | 4.8      | 0.4      | 0.1             | 4.6      | 1.1             | 2.33          | 0.16                 | PL  | ... | ...   | ...                  | ... | fsrq  | PKS 1356+022            |
| J1359.9-3746 | 209.982 | -37.776 | 317.591 | 23.138 | 0.036      | 0.032      | 8      | 11.7     | 0.8      | 0.1             | 9.2      | 1.2             | 2.02          | 0.11                 | PL  | ... | ...   | 1FHL J1359.9-3746    | ... | bll   | PMN J1359-3746          |
|              |         |         |         |        |            |            |        |          |          |                 |          |                 |               |                      |     |     |       | 2FGL J1359.9-3746    |     |       |                         |
|              |         |         |         |        |            |            |        |          |          |                 |          |                 |               |                      |     |     |       | 1FGL J1400.1-3743    |     |       |                         |
| J1400.2-2413 | 210.067 | -24.232 | 322.416 | 36.022 | 0.157      | 0.093      | -7     | 6.7      | 0.5      | 0.1             | 5.8      | 1.0             | 2.16          | 0.12                 | PL  | ... | 3     | 2FGL J1400.2-2412    | ... | ...   | ...                     |
| J1400.5-1437 | 210.145 | -14.617 | 326.929 | 45.009 | 0.116      | 0.079      | 73     | 10.2     | 0.8      | 0.1             | 9.4      | 1.1             | 2.30          | 0.08                 | PL  | ... | 10    | 2FGL J1400.7-1438    | ... | psr   | PSR J1400-1438          |
| J1400.7-5605 | 210.175 | -56.091 | 312.535 | 5.484  | 0.124      | 0.119      | 51     | 9.1      | 0.9      | 0.1             | 13.7     | 1.6             | 2.50          | 0.09                 | PL  | T   | ...   | 2FGL J1400.6-5601    | ... | bcu   | PMN J1400-5605          |
|              |         |         |         |        |            |            |        |          |          |                 |          |                 |               |                      |     |     |       | 1FGL J1400.9-5559    |     |       |                         |
| J1402.7-3240 | 210.690 | -32.667 | 319.882 | 27.847 | 0.189      | 0.162      | -12    | 4.4      | 0.3      | 0.1             | 4.3      | 0.9             | 2.44          | 0.16                 | PL  | ... | ...   | ...                  | ... | ...   | ...                     |
| J1403.1+1304 | 210.796 | 13.080  | 356.532 | 68.119 | 0.217      | 0.140      | -35    | 4.3      | 0.3      | 0.1             | 3.1      | 0.7             | 2.27          | 0.18                 | PL  | ... | ...   | ...                  | ... | ...   | ...                     |
| J1404.3-5241 | 211.077 | -52.698 | 313.979 | 8.603  | 0.213      | 0.152      | 32     | 4.7      | 0.5      | 0.1             | 6.9      | 1.4             | 2.35          | 0.13                 | PL  | ... | ...   | 2FGL J1404.0-5244    | ... | ...   | ...                     |
| J1404.7-5844 | 211.191 | -58.739 | 312.337 | 2.787  | 0.063      | 0.053      | 50     | 5.0      | 0.6      | 0.2             | 7.1      | 2.3             | 2.04          | 0.27                 | PL  | ... | 4     | 1FGL J1405.5-5846    | ... | ...   | ...                     |
| J1404.8+6554 | 211.215 | 65.912  | 111.504 | 49.556 | 0.076      | 0.068      | -9     | 7.2      | 0.3      | 0.1             | 3.1      | 0.6             | 2.09          | 0.14                 | PL  | ... | ...   | ...                  | ... | bll   | NVSS<br>J140450+655428  |
| J1404.8+0401 | 211.221 | 4.026   | 343.333 | 60.999 | 0.052      | 0.050      | -19    | 10.4     | 0.6      | 0.1             | 6.9      | 1.0             | 1.98          | 0.11                 | PL  | ... | ...   | 2FGL J1405.1+0405    | ... | bll   | MS 1402.3+0416          |
| J1405.4-6119 | 211.356 | -61.317 | 311.691 | 0.290  | 0.031      | 0.025      | -83    | 24.8     | 12.3     | 0.6             | 101.4    | 6.3             | 2.25          | ...                  | LP  | ... | ...   | 2FGL J1405.5-6121    | ... | ...   | ...                     |
| J1406.0-2508 | 211.522 | -25.148 | 323.566 | 34.715 | 0.050      | 0.039      | 65     | 9.5      | 0.6      | 0.1             | 6.7      | 1.1             | 1.89          | 0.11                 | PL  | ... | ...   | 1FHL J1406.3-2509    | ... | bcu   | NVSS<br>J140609-250808  |
|              |         |         |         |        |            |            |        |          |          |                 |          |                 |               |                      |     |     |       | 2FGL J1406.2-2510    |     |       |                         |
|              |         |         |         |        |            |            |        |          |          |                 |          |                 |               |                      |     |     |       | 1FGL J1406.2-2510    |     |       |                         |
| J1406.6+1644 | 211.651 | 16.737  | 5.946   | 69.746 | 0.081      | 0.072      | -78    | 5.1      | 0.2      | 0.1             | 2.7      | 0.9             | 1.65          | 0.21                 | PL  | ... | ...   | 1FHL J1406.4+1646    | ... | bll   | RBS 1350                |
| J1407.7-4256 | 211.949 | -42.942 | 317.492 | 17.760 | 0.092      | 0.065      | 12     | 8.2      | 0.6      | 0.1             | 6.6      | 1.0             | 2.14          | 0.13                 | PL  | ... | ...   | 2FGL J1407.5-4257    | ... | bcu   | SUMSS<br>J140739-430231 |
|              |         |         |         |        |            |            |        |          |          |                 |          |                 |               |                      |     |     |       | 1FGL J1407.5-4256    |     |       |                         |
| J1408.0-2924 | 212.008 | -29.405 | 322.316 | 30.568 | 0.360      | 0.190      | 43     | 7.4      | 0.4      | 0.1             | 7.0      | 0.9             | 2.69          | 0.11                 | PL  | ... | ...   | 2FGL J1407.4-2948    | ... | ...   | ...                     |
|              |         |         |         |        |            |            |        |          |          |                 |          |                 |               |                      |     |     |       | 1FGL J1407.9-2928    |     |       |                         |
| J1408.8-0751 | 212.204 | -7.857  | 333.852 | 50.312 | 0.048      | 0.042      | -53    | 20.8     | 1.8      | 0.1             | 23.2     | 1.4             | 2.38          | 0.04                 | PL  | T   | ...   | 2FGL J1408.8-0751    | ... | fsrq  | PKS B1406-076           |
|              |         |         |         |        |            |            |        |          |          |                 |          |                 |               |                      |     |     |       | 1FGL J1408.9-0751    |     |       |                         |
|              |         |         |         |        |            |            |        |          |          |                 |          |                 |               |                      |     |     |       | 3EG J1409-0745       |     |       |                         |
| J1409.2-3743 | 212.303 | -37.722 | 319.508 | 22.634 | 0.214      | 0.147      | -86    | 5.8      | 0.3      | 0.1             | 6.5      | 1.0             | 2.70          | 0.15                 | PL  | ... | ...   | ...                  | ... | ...   | ...                     |
| J1409.7-6132 | 212.425 | -61.535 | 312.117 | -0.067 | 0.083      | 0.055      | 87     | 11.4     | 5.3      | 0.5             | 63.1     | 6.9             | 2.26          | 0.06                 | PL  | ... | 3,5   | 2FGL J1409.9-6129    | ... | PSR   | PSR J1410-6132          |
|              |         |         |         |        |            |            |        |          |          |                 |          |                 |               |                      |     |     |       | 1FGL J1410.3-6128c   |     |       |                         |
|              |         |         |         |        |            |            |        |          |          |                 |          |                 |               |                      |     |     |       | 3EG J1410-6147       |     |       |                         |
|              |         |         |         |        |            |            |        |          |          |                 |          |                 |               |                      |     |     |       | 1AGL J1412-6149      |     |       |                         |
| J1410.4+2821 | 212.620 | 28.356  | 41.542  | 72.488 | 0.101      | 0.073      | 47     | 7.0      | 0.3      | 0.1             | 3.8      | 0.8             | 1.97          | 0.16                 | PL  | ... | ...   | 2FGL J1410.3+2811    | ... | bll   | RX J1410.4+2821         |
| J1410.9+7406 | 212.742 | 74.107  | 115.745 | 41.893 | 0.042      | 0.038      | 79     | 15.8     | 0.7      | 0.1             | 7.6      | 0.7             | 2.16          | 0.09                 | PL  | ... | 10    | 1FHL J1410.4+7408    | ... | ...   | ...                     |

Table 1—Continued

| Name 3FGL    | R.A.    | Decl.   | $l$     | $b$    | $\theta_1$ | $\theta_2$ | $\phi$ | $\sigma$ | $F_{35}$ | $\Delta F_{35}$ | $S_{25}$ | $\Delta S_{25}$ | $\Gamma_{25}$ | $\Delta \Gamma_{25}$ | Mod | Var | Flags | $\gamma$ -ray Assoc. | TeV | Class | ID or Assoc.          |
|--------------|---------|---------|---------|--------|------------|------------|--------|----------|----------|-----------------|----------|-----------------|---------------|----------------------|-----|-----|-------|----------------------|-----|-------|-----------------------|
|              |         |         |         |        |            |            |        |          |          |                 |          |                 |               |                      |     |     |       | 1FGL J1412.6+7406    |     |       |                       |
| J1411.1+3717 | 212.796 | 37.299  | 69.106  | 70.366 | 0.188      | 0.110      | 39     | 5.1      | 0.2      | 0.1             | 3.3      | 0.7             | 2.48          | 0.18                 | PL  | ... | 1     | ...                  | ... | ...   | ...                   |
| J1411.4-0724 | 212.855 | -7.414  | 335.071 | 50.399 | 0.072      | 0.063      | -5     | 4.7      | 0.3      | 0.1             | 3.1      | 0.9             | 1.90          | 0.21                 | PL  | ... | ...   | ...                  | ... | ...   | ...                   |
| J1411.8-5743 | 212.974 | -57.717 | 313.536 | 3.488  | 0.101      | 0.087      | -10    | 9.7      | 0.8      | 0.2             | 14.5     | 1.7             | 2.49          | ...                  | LP  | ... | 12    | 2FGL J1411.9-5744    | ... | ...   | ...                   |
| J1412.0+5249 | 213.020 | 52.817  | 98.112  | 60.251 | 0.089      | 0.080      | 39     | 4.6      | 0.2      | 0.0             | 2.7      | 0.7             | 2.56          | 0.23                 | PL  | ... | ...   | ...                  | ... | bcu   | SBS 1410+530          |
| J1412.3-6635 | 213.093 | -66.597 | 310.858 | -4.979 | 0.149      | 0.117      | -60    | 7.5      | 1.1      | 0.2             | 8.2      | 1.5             | 2.36          | ...                  | LP  | ... | ...   | ...                  | ... | ...   | ...                   |
| J1413.2-6518 | 213.317 | -65.304 | 311.348 | -3.778 | 0.148      | 0.096      | -53    | 7.1      | 1.0      | 0.1             | 13.0     | 2.0             | 2.43          | 0.10                 | PL  | ... | 3,4   | ...                  | ... | sey   | Circinus galaxy       |
| J1413.4-6205 | 213.372 | -62.087 | 312.375 | -0.729 | 0.014      | 0.013      | -39    | 62.4     | 28.2     | 0.6             | 198.4    | 5.5             | 2.17          | ...                  | EC  | ... | ...   | 1FHL J1413.4-6205    | ... | PSR   | LAT PSR J1413-6205    |
|              |         |         |         |        |            |            |        |          |          |                 |          |                 |               |                      |     |     |       | 2FGL J1413.4-6204    |     |       |                       |
|              |         |         |         |        |            |            |        |          |          |                 |          |                 |               |                      |     |     |       | 1FGL J1413.4-6205    |     |       |                       |
|              |         |         |         |        |            |            |        |          |          |                 |          |                 |               |                      |     |     |       | 0FGL J1413.1-6203    |     |       |                       |
|              |         |         |         |        |            |            |        |          |          |                 |          |                 |               |                      |     |     |       | EGRc J1414-6224      |     |       |                       |
|              |         |         |         |        |            |            |        |          |          |                 |          |                 |               |                      |     |     |       | 1AGL J1412-6149      |     |       |                       |
| J1415.0-1001 | 213.756 | -10.018 | 334.382 | 47.684 | 0.220      | 0.170      | -54    | 4.1      | 0.3      | 0.1             | 4.2      | 1.0             | 2.49          | 0.15                 | PL  | ... | ...   | 1FGL J1416.2-1001    | ... | fsrq  | PKS B1412-096         |
| J1415.2+4832 | 213.811 | 48.540  | 91.344  | 63.128 | 0.104      | 0.096      | 41     | 6.7      | 0.2      | 0.1             | 4.1      | 0.7             | 2.67          | 0.16                 | PL  | ... | ...   | ...                  | ... | bll   | RX J1415.5+4830       |
| J1416.0+1325 | 214.006 | 13.426  | 2.395   | 65.958 | 0.084      | 0.070      | -84    | 9.3      | 0.5      | 0.1             | 6.8      | 0.9             | 2.36          | 0.11                 | PL  | T   | ...   | 2FGL J1416.0+1323    | ... | bcu   | PKS B1413.9+1335      |
| J1416.1-2417 | 214.039 | -24.299 | 326.531 | 34.661 | 0.064      | 0.058      | 3      | 7.6      | 0.5      | 0.1             | 5.6      | 1.1             | 1.85          | 0.13                 | PL  | ... | ...   | 2FGL J1416.3-2415    | ... | bll   | NVSS J141612-241812   |
| J1417.5-4402 | 214.377 | -44.043 | 318.864 | 16.150 | 0.062      | 0.058      | 17     | 12.6     | 1.0      | 0.1             | 12.4     | 1.2             | 2.37          | 0.08                 | PL  | ... | ...   | 2FGL J1417.5-4404    | ... | ...   | ...                   |
|              |         |         |         |        |            |            |        |          |          |                 |          |                 |               |                      |     |     |       | 1FGL J1417.7-4407    |     |       |                       |
| J1417.7-5026 | 214.430 | -50.440 | 316.692 | 10.113 | 0.106      | 0.096      | -0     | 6.2      | 0.6      | 0.1             | 8.8      | 1.5             | 2.49          | 0.13                 | PL  | ... | ...   | 2FGL J1417.7-5028    | ... | ...   | ...                   |
|              |         |         |         |        |            |            |        |          |          |                 |          |                 |               |                      |     |     |       | 1FGL J1417.7-5030    |     |       |                       |
| J1417.8+2540 | 214.462 | 25.670  | 33.523  | 70.619 | 0.063      | 0.060      | -6     | 6.5      | 0.4      | 0.1             | 4.0      | 0.8             | 2.16          | 0.19                 | PL  | ... | ...   | 1FHL J1418.6+2539    | ... | bll   | 1E 1415.6+2557        |
|              |         |         |         |        |            |            |        |          |          |                 |          |                 |               |                      |     |     |       | 2FGL J1418.1+2539    |     |       |                       |
|              |         |         |         |        |            |            |        |          |          |                 |          |                 |               |                      |     |     |       | 1FGL J1417.8+2541    |     |       |                       |
| J1418.4-0233 | 214.609 | -2.564  | 341.582 | 53.649 | 0.022      | 0.022      | -20    | 33.0     | 2.8      | 0.2             | 29.0     | 2.7             | 1.71          | ...                  | LP  | T   | ...   | 1FHL J1418.4-0234    | ... | bll   | NVSS J141826-023336   |
|              |         |         |         |        |            |            |        |          |          |                 |          |                 |               |                      |     |     |       | 2FGL J1418.4-0234    |     |       |                       |
|              |         |         |         |        |            |            |        |          |          |                 |          |                 |               |                      |     |     |       | 1FGL J1418.3-0235    |     |       |                       |
| J1418.5+3543 | 214.650 | 35.719  | 63.190  | 69.578 | 0.027      | 0.025      | -23    | 36.3     | 2.5      | 0.1             | 27.9     | 1.5             | 2.06          | 0.04                 | PL  | T   | ...   | ...                  | ... | BCU   | NVSS J141828+354250   |
| J1418.6-6058 | 214.665 | -60.971 | 313.317 | 0.130  | 0.014      | 0.013      | 39     | 40.0     | 40.7     | 1.2             | 310.4    | 12.4            | 2.27          | ...                  | EC  | ... | 5     | 1FHL J1418.6-6059    | E   | PSR   | LAT PSR J1418-6058    |
|              |         |         |         |        |            |            |        |          |          |                 |          |                 |               |                      |     |     |       | 2FGL J1418.7-6058    |     |       |                       |
|              |         |         |         |        |            |            |        |          |          |                 |          |                 |               |                      |     |     |       | 1FGL J1418.7-6057    |     |       |                       |
|              |         |         |         |        |            |            |        |          |          |                 |          |                 |               |                      |     |     |       | 0FGL J1418.8-6058    |     |       |                       |
|              |         |         |         |        |            |            |        |          |          |                 |          |                 |               |                      |     |     |       | 1AGL J1419-6055      |     |       |                       |
| J1418.9+7731 | 214.747 | 77.517  | 117.015 | 38.587 | 0.048      | 0.041      | -6     | 11.2     | 0.5      | 0.1             | 5.4      | 0.8             | 1.91          | 0.11                 | PL  | ... | ...   | 1FHL J1419.0+7730    | ... | bcu   | 1RXS J141901.8+773229 |
|              |         |         |         |        |            |            |        |          |          |                 |          |                 |               |                      |     |     |       | 2FGL J1419.4+7730    |     |       |                       |

Table 1—Continued

| Name 3FGL    | R.A.    | Decl.   | $l$     | $b$     | $\theta_1$ | $\theta_2$ | $\phi$ | $\sigma$ | $F_{35}$ | $\Delta F_{35}$ | $S_{25}$ | $\Delta S_{25}$ | $\Gamma_{25}$ | $\Delta \Gamma_{25}$ | Mod | Var | Flags | $\gamma$ -ray Assoc.                                                                                               | TeV | Class | ID or Assoc.                |
|--------------|---------|---------|---------|---------|------------|------------|--------|----------|----------|-----------------|----------|-----------------|---------------|----------------------|-----|-----|-------|--------------------------------------------------------------------------------------------------------------------|-----|-------|-----------------------------|
|              |         |         |         |         |            |            |        |          |          |                 |          |                 |               |                      |     |     |       | 1FGL J1419.7+7731                                                                                                  |     |       |                             |
| J1419.1–5156 | 214.776 | –51.942 | 316.390 | 8.624   | 0.211      | 0.097      | 45     | 6.5      | 0.6      | 0.1             | 11.1     | 1.7             | 2.66          | 0.11                 | PL  | ... | 1,9   | ...                                                                                                                | ... | bcu   | PMN J1419–5155              |
| J1419.1–5534 | 214.784 | –55.577 | 315.169 | 5.197   | 0.231      | 0.100      | 19     | 9.2      | 0.7      | 0.1             | 16.1     | 1.8             | 2.82          | 0.10                 | PL  | ... | 1,4,9 | ...                                                                                                                | ... | ...   | ...                         |
| J1419.5–0836 | 214.875 | –8.611  | 336.849 | 48.376  | 0.075      | 0.065      | –47    | 14.9     | 1.1      | 0.1             | 13.1     | 1.1             | 2.27          | 0.06                 | PL  | T   | ...   | 2FGL J1419.4–0835                                                                                                  | ... | bcu   | NVSS<br>J141922–083830      |
| J1419.5+0449 | 214.897 | 4.826   | 350.126 | 59.362  | 0.167      | 0.101      | 13     | 4.4      | 0.2      | 0.1             | 2.8      | 0.9             | 1.75          | 0.21                 | PL  | ... | ...   | ...                                                                                                                | ... | bll   | SDSS<br>J141927.49+044513.7 |
| J1419.8+3819 | 214.956 | 38.325  | 69.693  | 68.386  | 0.087      | 0.076      | 54     | 12.5     | 0.6      | 0.1             | 7.7      | 0.8             | 2.36          | 0.08                 | PL  | ... | ...   | 2FGL J1419.4+3820                                                                                                  | ... | fsrq  | B3 1417+385                 |
| J1419.9+5425 | 214.984 | 54.419  | 98.306  | 58.272  | 0.050      | 0.045      | –38    | 20.1     | 1.0      | 0.1             | 11.8     | 0.8             | 2.31          | 0.06                 | PL  | T   | ...   | 2FGL J1420.2+5422                                                                                                  | ... | bll   | OQ 530                      |
| J1420.0–6048 | 215.008 | –60.815 | 313.526 | 0.222   | 0.024      | 0.023      | 48     | 23.0     | 17.5     | 1.0             | 161.2    | 11.6            | 2.27          | ...                  | EC  | ... | ...   | 1FHL J1420.1–6047<br>2FGL J1420.1–6047<br>1FGL J1420.1–6048<br>3EG J1420–6038<br>EGR J1418–6040<br>1AGL J1419–6055 | E   | PSR   | PSR J1420–6048              |
| J1420.9–4615 | 215.243 | –46.255 | 318.668 | 13.863  | 0.165      | 0.120      | 22     | 6.7      | 0.4      | 0.1             | 7.8      | 1.2             | 2.70          | 0.15                 | PL  | ... | 1     | ...                                                                                                                | ... | ...   | ...                         |
| J1421.0–2431 | 215.260 | –24.528 | 327.655 | 34.006  | 0.122      | 0.115      | 67     | 5.4      | 0.4      | 0.1             | 4.7      | 0.9             | 2.20          | 0.13                 | PL  | ... | ...   | ...                                                                                                                | ... | ...   | ...                         |
| J1421.0–1122 | 215.262 | –11.375 | 335.330 | 45.785  | 0.091      | 0.082      | –69    | 6.5      | 0.4      | 0.1             | 5.0      | 1.0             | 2.06          | 0.13                 | PL  | ... | ...   | 2FGL J1421.1–1117                                                                                                  | ... | bcu   | PMN J1420–1118              |
| J1421.8–7920 | 215.466 | –79.348 | 307.199 | –17.233 | 0.170      | 0.139      | 72     | 4.4      | 0.4      | 0.1             | 4.2      | 1.0             | 2.14          | 0.14                 | PL  | ... | ...   | ...                                                                                                                | ... | ...   | ...                         |
| J1422.4+3227 | 215.614 | 32.452  | 53.540  | 69.592  | 0.245      | 0.214      | 38     | 4.6      | 0.2      | 0.1             | 3.3      | 0.7             | 2.56          | 0.21                 | PL  | ... | ...   | ...                                                                                                                | ... | fsrq  | OQ 334                      |
| J1422.4–6137 | 215.615 | –61.633 | 313.523 | –0.647  | 0.023      | 0.021      | –13    | 25.4     | 8.1      | 0.5             | 48.6     | 3.5             | 2.04          | ...                  | EC  | ... | ...   | 2FGL J1422.5–6137c                                                                                                 | ... | PSR   | LAT PSR J1422–6138          |
| J1422.8–7828 | 215.719 | –78.479 | 307.572 | –16.440 | 0.111      | 0.089      | –67    | 4.4      | 0.3      | 0.1             | 3.6      | 0.9             | 2.05          | 0.15                 | PL  | ... | ...   | 1FGL J1424.5–7847                                                                                                  | ... | fsrq  | PKS 1418–782                |
| J1422.8+5801 | 215.722 | 58.027  | 101.808 | 55.190  | 0.079      | 0.058      | –89    | 7.0      | 0.3      | 0.1             | 3.0      | 0.6             | 2.02          | 0.22                 | PL  | ... | 10    | 1FGL J1422.2+5757                                                                                                  | ... | bll   | 1ES 1421+582                |
| J1424.3+0434 | 216.092 | 4.581   | 351.538 | 58.389  | 0.106      | 0.095      | –3     | 6.2      | 0.4      | 0.1             | 4.6      | 0.9             | 2.36          | 0.14                 | PL  | ... | ...   | ...                                                                                                                | ... | bll   | TXS 1421+048                |
| J1424.3–1753 | 216.094 | –17.886 | 332.120 | 39.661  | 0.068      | 0.055      | 89     | 7.3      | 0.5      | 0.1             | 5.7      | 1.0             | 2.17          | 0.13                 | PL  | ... | ...   | 2FGL J1424.2–1752                                                                                                  | ... | ...   | ...                         |
| J1424.6–6807 | 216.159 | –68.132 | 311.465 | –6.818  | 0.062      | 0.057      | –26    | 17.5     | 1.6      | 0.1             | 24.8     | 1.6             | 2.54          | 0.05                 | PL  | T   | ...   | ...                                                                                                                | ... | bcu   | PKS 1420–679                |
| J1424.9+3615 | 216.244 | 36.254  | 63.470  | 68.186  | 0.040      | 0.037      | –18    | 15.4     | 0.9      | 0.1             | 9.6      | 1.0             | 2.10          | 0.08                 | PL  | ... | ...   | 1FHL J1425.1+3613                                                                                                  | ... | bll   | FBQS<br>J142455.5+361536    |
|              |         |         |         |         |            |            |        |          |          |                 |          |                 |               |                      |     |     |       | 2FGL J1425.1+3615<br>1FGL J1425.0+3614                                                                             |     |       |                             |
| J1426.2+3402 | 216.564 | 34.044  | 57.500  | 68.514  | 0.075      | 0.066      | 82     | 6.9      | 0.3      | 0.1             | 3.7      | 0.8             | 1.93          | 0.14                 | PL  | ... | ...   | 2FGL J1426.1+3406<br>1FGL J1426.0+3403                                                                             | ... | bll   | RGB J1426+340               |
| J1427.0+2347 | 216.757 | 23.800  | 29.490  | 68.203  | 0.010      | 0.010      | 48     | 107.4    | 13.6     | 0.3             | 148.6    | 5.0             | 1.82          | ...                  | LP  | T   | ...   | 1FHL J1427.0+2347<br>2FGL J1427.0+2347<br>1FGL J1426.9+2347<br>0FGL J1427.1+2347                                   | P   | BLL   | PKS 1424+240                |
| J1427.2+1610 | 216.808 | 16.174  | 11.591  | 65.256  | 0.436      | 0.332      | –16    | 5.0      | 0.1      | 0.1             | 4.8      | 0.9             | 3.01          | 0.20                 | PL  | ... | ...   | ...                                                                                                                | ... | ...   | ...                         |
| J1427.6–3305 | 216.909 | –33.092 | 325.177 | 25.591  | 0.043      | 0.041      | –46    | 19.6     | 1.6      | 0.1             | 21.4     | 1.3             | 2.42          | 0.05                 | PL  | T   | ...   | 2FGL J1427.4–3306                                                                                                  | ... | bll   | PKS B1424–328               |

Table 1—Continued

| Name 3FGL    | R.A.    | Decl.   | $l$     | $b$    | $\theta_1$ | $\theta_2$ | $\phi$ | $\sigma$ | $F_{35}$ | $\Delta F_{35}$ | $S_{25}$ | $\Delta S_{25}$ | $\Gamma_{25}$ | $\Delta \Gamma_{25}$ | Mod | Var | Flags | $\gamma$ -ray Assoc.                                                                            | TeV | Class | ID or Assoc.             |
|--------------|---------|---------|---------|--------|------------|------------|--------|----------|----------|-----------------|----------|-----------------|---------------|----------------------|-----|-----|-------|-------------------------------------------------------------------------------------------------|-----|-------|--------------------------|
| J1427.8–3215 | 216.960 | –32.252 | 325.598 | 26.342 | 0.099      | 0.087      | 10     | 4.5      | 0.3      | 0.1             | 3.5      | 0.9             | 2.04          | 0.19                 | PL  | ... | ...   | ...                                                                                             | ... | bcu   | NVSS<br>J142750–321515   |
| J1427.9–4206 | 216.991 | –42.111 | 321.451 | 17.264 | 0.013      | 0.012      | 21     | 129.8    | 18.2     | 0.3             | 179.9    | 3.1             | 2.21          | ...                  | LP  | T   | ...   | 1FHL J1428.0–4206<br>2FGL J1428.0–4206<br>1FGL J1428.2–4204<br>3EG J1429–4217<br>EGR J1428–4240 | ... | FSRQ  | PKS B1424–418            |
| J1428.5+4240 | 217.149 | 42.671  | 77.472  | 64.891 | 0.028      | 0.026      | –58    | 16.7     | 0.7      | 0.1             | 10.3     | 1.5             | 1.57          | 0.09                 | PL  | ... | ...   | 1FHL J1428.6+4239<br>2FGL J1428.6+4240<br>1FGL J1428.7+4239                                     | P   | bll   | H 1426+428               |
| J1429.8–5910 | 217.468 | –59.176 | 315.256 | 1.320  | 0.025      | 0.024      | 77     | 40.4     | 11.7     | 0.4             | 87.6     | 3.2             | 2.30          | ...                  | EC  | ... | ...   | 2FGL J1430.0–5909<br>1FGL J1429.9–5911                                                          | ... | PSR   | LAT PSR J1429–5911       |
| J1430.8–4434 | 217.713 | –44.569 | 320.973 | 14.793 | 0.069      | 0.068      | –17    | 7.7      | 0.6      | 0.1             | 7.8      | 1.2             | 2.35          | 0.12                 | PL  | ... | ...   | ...                                                                                             | ... | ...   | ...                      |
| J1431.1–6425 | 217.796 | –64.423 | 313.441 | –3.606 | 0.391      | 0.228      | 63     | 5.0      | 0.6      | 0.1             | 10.3     | 1.9             | 2.59          | 0.12                 | PL  | ... | 4     | ...                                                                                             | ... | ...   | ...                      |
| J1434.1+4203 | 218.539 | 42.057  | 75.064  | 64.287 | 0.096      | 0.076      | 86     | 8.4      | 0.4      | 0.1             | 4.8      | 0.7             | 2.39          | 0.12                 | PL  | T   | ...   | 2FGL J1433.8+4205<br>1FGL J1433.9+4204                                                          | ... | fsrq  | B3 1432+422              |
| J1434.6+6640 | 218.655 | 66.682  | 108.193 | 47.385 | 0.047      | 0.043      | –86    | 6.9      | 0.1      | 0.0             | 2.5      | 0.7             | 1.52          | 0.18                 | PL  | ... | ...   | ...                                                                                             | ... | bcu   | 1RXS<br>J143442.0+664031 |
| J1434.6+1951 | 218.656 | 19.865  | 21.375  | 65.307 | 0.152      | 0.132      | –87    | 4.5      | 0.4      | 0.1             | 4.2      | 1.2             | 2.25          | 0.23                 | PL  | ... | 5     | ...                                                                                             | ... | fsrq  | OQ 253                   |
| J1435.2+2023 | 218.820 | 20.387  | 22.674  | 65.355 | 0.125      | 0.103      | 4      | 5.8      | 0.4      | 0.1             | 6.8      | 1.4             | 2.55          | 0.15                 | PL  | ... | ...   | 2FGL J1435.1+2022                                                                               | ... | bll   | TXS 1433+205             |
| J1436.8+5639 | 219.213 | 56.661  | 97.753  | 55.009 | 0.043      | 0.035      | 50     | 11.7     | 0.5      | 0.1             | 5.3      | 0.7             | 1.98          | 0.13                 | PL  | ... | ...   | 1FHL J1436.9+5642<br>2FGL J1437.1+5640<br>1FGL J1437.0+5640                                     | ... | bll   | RBS 1409                 |
| J1436.8+2322 | 219.215 | 23.367  | 29.829  | 65.912 | 0.087      | 0.078      | 3      | 8.1      | 0.4      | 0.1             | 6.0      | 0.9             | 2.41          | 0.14                 | PL  | ... | ...   | 2FGL J1436.9+2319<br>1FGL J1436.9+2314                                                          | ... | fsrq  | PKS B1434+235            |
| J1438.6–4209 | 219.669 | –42.161 | 323.331 | 16.424 | 0.102      | 0.088      | –37    | 5.1      | 0.4      | 0.1             | 4.9      | 1.3             | 2.32          | 0.22                 | PL  | ... | ...   | ...                                                                                             | ... | ...   | ...                      |
| J1438.7+3710 | 219.688 | 37.168  | 63.620  | 65.278 | 0.047      | 0.046      | –38    | 28.1     | 1.5      | 0.1             | 19.3     | 1.0             | 2.36          | 0.04                 | PL  | T   | ...   | 2FGL J1438.7+3712<br>1FGL J1438.7+3711                                                          | ... | fsrq  | B2 1436+37B              |
| J1439.2+3931 | 219.822 | 39.520  | 68.795  | 64.433 | 0.054      | 0.047      | 68     | 10.1     | 0.4      | 0.1             | 5.6      | 1.0             | 1.77          | 0.11                 | PL  | ... | ...   | 1FHL J1439.3+3933<br>2FGL J1439.2+3932<br>1FGL J1439.2+3930                                     | ... | bll   | PG 1437+398              |
| J1440.0–3955 | 220.005 | –39.923 | 324.564 | 18.344 | 0.064      | 0.059      | 3      | 5.5      | 0.3      | 0.1             | 3.8      | 1.0             | 1.86          | 0.21                 | PL  | ... | ...   | ...                                                                                             | ... | bcu   | 1RXS<br>J143949.8–395524 |
| J1440.1+4955 | 220.027 | 49.925  | 87.935  | 59.168 | 0.158      | 0.101      | –74    | 10.5     | 0.4      | 0.1             | 6.7      | 0.7             | 2.60          | 0.10                 | PL  | ... | ...   | 2FGL J1440.3+4948                                                                               | ... | bll   | GB6 J1439+4958           |
| J1440.2–1538 | 220.062 | –15.634 | 337.860 | 39.745 | 0.111      | 0.104      | –48    | 6.9      | 0.6      | 0.1             | 7.2      | 1.1             | 2.35          | 0.11                 | PL  | ... | ...   | 2FGL J1440.3–1540<br>1FGL J1441.7–1538                                                          | ... | bll   | PKS 1437–153             |
| J1440.4–3845 | 220.119 | –38.763 | 325.175 | 19.354 | 0.052      | 0.045      | –83    | 8.1      | 0.5      | 0.1             | 6.1      | 1.3             | 1.73          | 0.15                 | PL  | ... | ...   | 1FHL J1440.6–3847                                                                               | ... | bll   | 1RXS<br>J144037.4–384658 |
| J1440.9+0610 | 220.246 | 6.181   | 359.085 | 56.589 | 0.040      | 0.036      | 88     | 14.5     | 0.9      | 0.1             | 11.0     | 1.0             | 2.25          | 0.08                 | PL  | T   | ...   | 1FHL J1441.0+0609                                                                               | ... | bll   | PMN J1440+0610           |

Table 1—Continued

| Name 3FGL     | R.A.    | Decl.   | $l$     | $b$    | $\theta_1$ | $\theta_2$ | $\phi$ | $\sigma$ | $F_{35}$ | $\Delta F_{35}$ | $S_{25}$ | $\Delta S_{25}$ | $\Gamma_{25}$ | $\Delta \Gamma_{25}$ | Mod | Var | Flags | $\gamma$ -ray Assoc. | TeV | Class | ID or Assoc.                |
|---------------|---------|---------|---------|--------|------------|------------|--------|----------|----------|-----------------|----------|-----------------|---------------|----------------------|-----|-----|-------|----------------------|-----|-------|-----------------------------|
| J1441.5−5955c | 220.397 | −59.928 | 316.328 | 0.048  | 0.095      | 0.056      | −48    | 6.7      | 2.2      | 0.3             | 24.9     | 4.1             | 2.18          | 0.09                 | PL  | ... | 3,6   | 2FGL J1440.9+0611    | ... | spp   | ...                         |
|               |         |         |         |        |            |            |        |          |          |                 |          |                 |               |                      |     |     |       | 1FGL J1440.9+0613    |     |       |                             |
|               |         |         |         |        |            |            |        |          |          |                 |          |                 |               |                      |     |     |       | 2FGL J1441.6−5956    |     |       |                             |
| J1442.0+4348  | 220.510 | 43.815  | 77.050  | 62.195 | 0.072      | 0.057      | −23    | 7.8      | 0.3      | 0.1             | 3.7      | 0.8             | 1.78          | 0.15                 | PL  | ... | ...   | 1FGL J1442.0−6000c   | ... | bll   | SDSS<br>J144207.15+434836.6 |
|               |         |         |         |        |            |            |        |          |          |                 |          |                 |               |                      |     |     |       | 2FGL J1442.0+4352    |     |       |                             |
|               |         |         |         |        |            |            |        |          |          |                 |          |                 |               |                      |     |     |       | 1FGL J1442.1+4348    |     |       |                             |
| J1442.6+5156  | 220.669 | 51.937  | 90.464  | 57.601 | 0.125      | 0.110      | 75     | 4.3      | 0.2      | 0.1             | 2.2      | 0.6             | 1.91          | 0.18                 | PL  | ... | ...   | ...                  | ... | rdg   | 3C 303                      |
| J1442.8+1200  | 220.722 | 12.015  | 8.360   | 59.825 | 0.042      | 0.040      | 2      | 11.1     | 0.6      | 0.1             | 6.9      | 1.2             | 1.80          | 0.12                 | PL  | ... | ...   | 1FHL J1442.9+1158    | P   | bll   | 1ES 1440+122                |
| J1443.9+2502  | 220.996 | 25.039  | 34.590  | 64.695 | 0.052      | 0.048      | −38    | 15.2     | 0.9      | 0.1             | 10.6     | 1.0             | 2.13          | 0.07                 | PL  | ... | ...   | 2FGL J1442.7+1159    | ... | fsrq  | PKS 1441+25                 |
|               |         |         |         |        |            |            |        |          |          |                 |          |                 |               |                      |     |     |       | 1FGL J1442.8+1158    |     |       |                             |
|               |         |         |         |        |            |            |        |          |          |                 |          |                 |               |                      |     |     |       | 2FGL J1444.1+2500    |     |       |                             |
| J1444.0−3907  | 221.009 | −39.130 | 325.664 | 18.721 | 0.018      | 0.017      | −71    | 34.0     | 3.2      | 0.2             | 39.6     | 2.5             | 1.81          | 0.04                 | PL  | ... | ...   | 1FHL J1443.8+2457    | ... | bll   | PKS 1440−389                |
|               |         |         |         |        |            |            |        |          |          |                 |          |                 |               |                      |     |     |       | 1FHL J1444.0−3908    |     |       |                             |
|               |         |         |         |        |            |            |        |          |          |                 |          |                 |               |                      |     |     |       | 2FGL J1443.9−3908    |     |       |                             |
| J1444.0−7033  | 221.013 | −70.564 | 312.098 | −9.723 | 0.143      | 0.127      | −71    | 4.9      | 0.4      | 0.1             | 5.6      | 1.1             | 2.45          | 0.16                 | PL  | ... | ...   | 1FGL J1444.0−3906    | ... | ...   | ...                         |
|               |         |         |         |        |            |            |        |          |          |                 |          |                 |               |                      |     |     |       | ...                  |     |       |                             |
|               |         |         |         |        |            |            |        |          |          |                 |          |                 |               |                      |     |     |       | ...                  |     |       |                             |
| J1445.0−0328  | 221.263 | −3.472  | 349.200 | 48.920 | 0.091      | 0.068      | −47    | 8.1      | 0.6      | 0.1             | 7.2      | 1.2             | 1.96          | 0.12                 | PL  | ... | ...   | ...                  | ... | bll   | RBS 1424                    |
| J1445.7−5925  | 221.447 | −59.428 | 317.019 | 0.280  | 0.155      | 0.125      | 11     | 4.2      | 1.4      | 0.3             | 18.1     | 4.5             | 2.34          | 0.13                 | PL  | ... | 3,4   | ...                  | ... | ...   | ...                         |
| J1446.1−1628  | 221.527 | −16.472 | 338.811 | 38.283 | 0.115      | 0.093      | 29     | 5.6      | 0.5      | 0.1             | 5.8      | 1.1             | 2.36          | 0.14                 | PL  | ... | ...   | ...                  | ... | bll   | PKS B1443−162               |
| J1446.6−4701  | 221.662 | −47.033 | 322.505 | 11.414 | 0.076      | 0.072      | −58    | 11.0     | 1.0      | 0.1             | 12.6     | 1.3             | 2.30          | 0.08                 | PL  | ... | 7,10  | 2FGL J1446.8−4701    | ... | PSR   | PSR J1446−4701              |
| J1446.8−1831  | 221.710 | −18.531 | 337.599 | 36.454 | 0.109      | 0.091      | 37     | 4.2      | 0.2      | 0.1             | 3.3      | 1.0             | 1.72          | 0.21                 | PL  | ... | ...   | 1FGL J1446.8−4702    | ... | bcu   | NVSS<br>J144644−182922      |
|               |         |         |         |        |            |            |        |          |          |                 |          |                 |               |                      |     |     |       | ...                  |     |       |                             |
|               |         |         |         |        |            |            |        |          |          |                 |          |                 |               |                      |     |     |       | ...                  |     |       |                             |
| J1447.3−5800  | 221.831 | −58.005 | 317.808 | 1.480  | 0.119      | 0.086      | −53    | 14.2     | 2.0      | 0.3             | 37.8     | 3.0             | 2.72          | ...                  | LP  | ... | ...   | 2FGL J1446.6−5753    | ... | ...   | ...                         |
| J1448.0+3608  | 222.010 | 36.145  | 60.270  | 63.717 | 0.032      | 0.030      | 76     | 23.1     | 1.3      | 0.1             | 15.8     | 1.5             | 1.82          | 0.06                 | PL  | T   | ...   | 1FHL J1448.2+3607    | ... | bll   | RBS 1432                    |
|               |         |         |         |        |            |            |        |          |          |                 |          |                 |               |                      |     |     |       | 2FGL J1448.0+3608    |     |       |                             |
|               |         |         |         |        |            |            |        |          |          |                 |          |                 |               |                      |     |     |       | 1FGL J1447.9+3608    |     |       |                             |
| J1450.4+0911  | 222.620 | 9.191   | 6.032   | 56.670 | 0.098      | 0.082      | 70     | 7.2      | 0.4      | 0.1             | 5.5      | 0.9             | 2.35          | 0.13                 | PL  | ... | ...   | ...                  | ... | fsrq  | TXS 1448+093                |
| J1450.9+5200  | 222.745 | 52.003  | 89.118  | 56.551 | 0.069      | 0.062      | −65    | 9.7      | 0.6      | 0.1             | 6.5      | 0.9             | 2.18          | 0.09                 | PL  | ... | ...   | 2FGL J1451.0+5159    | ... | bll   | SDSS<br>J145059.99+520111.7 |
|               |         |         |         |        |            |            |        |          |          |                 |          |                 |               |                      |     |     |       | ...                  |     |       |                             |
|               |         |         |         |        |            |            |        |          |          |                 |          |                 |               |                      |     |     |       | 1FGL J1451.0+5204    |     |       |                             |
| J1451.2+6355  | 222.805 | 63.919  | 103.603 | 48.468 | 0.084      | 0.068      | 9      | 5.6      | 0.2      | 0.1             | 2.3      | 0.6             | 1.88          | 0.20                 | PL  | ... | ...   | ...                  | ... | bll   | RX J1451.4+6354             |
| J1454.0+1622  | 223.503 | 16.380  | 18.549  | 59.680 | 0.174      | 0.148      | −71    | 6.4      | 0.3      | 0.1             | 5.3      | 0.9             | 2.59          | 0.13                 | PL  | ... | ...   | ...                  | ... | fsrq  | CLASS J1454+1623            |
| J1454.2−3751  | 223.566 | −37.856 | 328.160 | 18.926 | 0.132      | 0.109      | 75     | 9.1      | 0.5      | 0.1             | 10.1     | 1.2             | 2.76          | 0.11                 | PL  | ... | ...   | ...                  | ... | fsrq  | PKS 1451−375                |
| J1454.5+5124  | 223.630 | 51.408  | 87.664  | 56.449 | 0.026      | 0.025      | −21    | 33.6     | 2.4      | 0.1             | 26.9     | 1.4             | 2.08          | 0.04                 | PL  | T   | ...   | 1FHL J1454.4+5120    | ... | bll   | TXS 1452+516                |
|               |         |         |         |        |            |            |        |          |          |                 |          |                 |               |                      |     |     |       | 2FGL J1454.4+5123    |     |       |                             |
|               |         |         |         |        |            |            |        |          |          |                 |          |                 |               |                      |     |     |       | 1FGL J1454.6+5125    |     |       |                             |

Table 1—Continued

| Name 3FGL    | R.A.    | Decl.   | $l$     | $b$     | $\theta_1$ | $\theta_2$ | $\phi$ | $\sigma$ | $F_{35}$ | $\Delta F_{35}$ | $S_{25}$ | $\Delta S_{25}$ | $\Gamma_{25}$ | $\Delta \Gamma_{25}$ | Mod | Var | Flags  | $\gamma$ -ray Assoc.                                                                               | TeV | Class | ID or Assoc.                |
|--------------|---------|---------|---------|---------|------------|------------|--------|----------|----------|-----------------|----------|-----------------|---------------|----------------------|-----|-----|--------|----------------------------------------------------------------------------------------------------|-----|-------|-----------------------------|
| J1456.7–6046 | 224.195 | –60.777 | 317.646 | –1.537  | 0.150      | 0.102      | 71     | 6.3      | 1.2      | 0.3             | 28.4     | 4.6             | 2.37          | ...                  | LP  | ... | 1,5,12 | ...                                                                                                | E   | ...   | ...                         |
| J1457.4–3539 | 224.355 | –35.657 | 329.888 | 20.536  | 0.021      | 0.020      | 60     | 62.2     | 6.6      | 0.2             | 68.3     | 2.1             | 2.29          | ...                  | LP  | T   | ...    | 1FHL J1457.3–3544<br>2FGL J1457.4–3540<br>1FGL J1457.5–3540<br>0FGL J1457.6–3538<br>3EG J1500–3509 | ... | FSRQ  | PKS 1454–354                |
| J1457.6–6249 | 224.400 | –62.830 | 316.777 | –3.400  | 0.242      | 0.229      | –79    | 5.0      | 0.8      | 0.2             | 11.0     | 2.2             | 2.45          | 0.12                 | PL  | ... | ...    | 2FGL J1456.7–6247c                                                                                 | ... | ...   | ...                         |
| J1457.6–5355 | 224.412 | –53.926 | 320.935 | 4.475   | 0.091      | 0.083      | 75     | 4.5      | 0.6      | 0.1             | 7.6      | 1.8             | 2.42          | 0.16                 | PL  | ... | 4      | ...                                                                                                | ... | ...   | ...                         |
| J1458.7+3719 | 224.685 | 37.325  | 61.838  | 61.378  | 0.181      | 0.122      | 90     | 4.5      | 0.2      | 0.1             | 2.7      | 0.7             | 2.24          | 0.18                 | PL  | ... | ...    | ...                                                                                                | ... | bll   | B3 1456+375                 |
| J1458.7–2120 | 224.688 | –21.335 | 338.591 | 32.578  | 0.102      | 0.084      | 69     | 7.4      | 0.6      | 0.1             | 7.1      | 1.0             | 2.34          | 0.11                 | PL  | ... | ...    | 2FGL J1458.5–2121                                                                                  | ... | ...   | ...                         |
| J1459.4–6053 | 224.866 | –60.900 | 317.878 | –1.798  | 0.020      | 0.020      | 52     | 37.4     | 12.4     | 0.5             | 110.4    | 5.2             | 2.37          | ...                  | EC  | ... | ...    | 2FGL J1459.4–6054<br>1FGL J1459.4–6053<br>0FGL J1459.4–6056                                        | E   | PSR   | LAT PSR J1459–6053          |
| J1500.6+4750 | 225.173 | 47.841  | 81.118  | 57.443  | 0.108      | 0.098      | –21    | 4.7      | 0.3      | 0.1             | 5.1      | 1.2             | 2.64          | 0.15                 | PL  | ... | 5      | ...                                                                                                | ... | bll   | TXS 1459+480                |
| J1500.9+2238 | 225.241 | 22.636  | 31.439  | 60.365  | 0.032      | 0.027      | 43     | 20.4     | 1.3      | 0.1             | 14.8     | 1.4             | 1.92          | 0.06                 | PL  | T   | ...    | 1FHL J1501.0+2238<br>2FGL J1501.0+2238<br>1FGL J1501.1+2237                                        | ... | bll   | MS 1458.8+2249              |
| J1502.2+5553 | 225.555 | 55.886  | 92.785  | 52.899  | 0.070      | 0.064      | 47     | 12.6     | 0.5      | 0.1             | 8.5      | 0.7             | 2.58          | 0.08                 | PL  | T   | ...    | 2FGL J1502.1+5548                                                                                  | ... | ...   | ...                         |
| J1503.5–5801 | 225.893 | –58.029 | 319.709 | 0.472   | 0.071      | 0.053      | 44     | 12.8     | 4.3      | 0.4             | 35.5     | 4.1             | 2.42          | ...                  | LP  | ... | ...    | 2FGL J1503.9–5800c<br>1FGL J1503.4–5805c                                                           | E   | ...   | ...                         |
| J1503.7+4759 | 225.925 | 47.987  | 80.927  | 56.928  | 0.089      | 0.069      | –68    | 8.7      | 0.6      | 0.1             | 6.4      | 1.0             | 2.22          | 0.13                 | PL  | ... | ...    | 1FGL J1503.3+4759                                                                                  | ... | bll   | SDSS<br>J150347.99+475930.9 |
| J1503.7–6426 | 225.929 | –64.449 | 316.600 | –5.147  | 0.049      | 0.043      | 50     | 10.7     | 1.2      | 0.1             | 15.4     | 1.7             | 2.33          | 0.07                 | PL  | T   | ...    | ...                                                                                                | ... | bcu   | AT20G<br>J150350–642539     |
| J1503.7–1540 | 225.947 | –15.676 | 343.762 | 36.493  | 0.043      | 0.038      | –46    | 13.5     | 0.9      | 0.1             | 12.0     | 1.6             | 1.77          | 0.09                 | PL  | ... | ...    | 1FHL J1503.9–1540<br>2FGL J1503.7–1541<br>1FGL J1503.5–1544<br>3EG J1504–1537<br>EGR J1504–1539    | ... | bll   | RBS 1457                    |
| J1504.4+1029 | 226.105 | 10.494  | 11.382  | 54.580  | 0.012      | 0.011      | –67    | 189.5    | 24.0     | 0.4             | 243.9    | 3.1             | 2.24          | ...                  | LP  | T   | ...    | 1FHL J1504.3+1029<br>2FGL J1504.3+1029<br>1FGL J1504.4+1029<br>0FGL J1504.4+1030                   | ... | FSRQ  | PKS 1502+106                |
| J1504.5–8242 | 226.142 | –82.710 | 307.209 | –20.970 | 0.151      | 0.124      | 36     | 4.1      | 0.3      | 0.1             | 3.6      | 0.9             | 2.30          | 0.17                 | PL  | ... | 4      | ...                                                                                                | ... | bcu   | 1RXS<br>J150537.1–824233    |
| J1505.0–3432 | 226.250 | –34.547 | 331.917 | 20.699  | 0.091      | 0.072      | –20    | 7.5      | 0.6      | 0.1             | 7.1      | 1.1             | 2.23          | 0.11                 | PL  | ... | ...    | 2FGL J1504.9–3433<br>1FGL J1505.1–3435<br>3EG J1500–3509                                           | ... | bll   | PMN J1505–3432              |

Table 1—Continued

| Name 3FGL    | R.A.    | Decl.   | $l$     | $b$    | $\theta_1$ | $\theta_2$ | $\phi$ | $\sigma$ | $F_{35}$ | $\Delta F_{35}$ | $S_{25}$ | $\Delta S_{25}$ | $\Gamma_{25}$ | $\Delta \Gamma_{25}$ | Mod | Var | Flags | $\gamma$ -ray Assoc.                                                             | TeV | Class | ID or Assoc.             |
|--------------|---------|---------|---------|--------|------------|------------|--------|----------|----------|-----------------|----------|-----------------|---------------|----------------------|-----|-----|-------|----------------------------------------------------------------------------------|-----|-------|--------------------------|
| J1505.1+0326 | 226.278 | 3.449   | 2.237   | 50.258 | 0.060      | 0.057      | −67    | 22.0     | 1.3      | 0.1             | 21.6     | 1.2             | 2.61          | 0.05                 | PL  | ... | ...   | 2FGL J1505.1+0324<br>1FGL J1505.0+0328                                           | ... | nlsy1 | PKS 1502+036             |
| J1506.1+3728 | 226.549 | 37.479  | 61.577  | 59.895 | 0.080      | 0.070      | 32     | 15.3     | 0.8      | 0.1             | 10.7     | 0.9             | 2.45          | 0.07                 | PL  | T   | ...   | 2FGL J1506.0+3729<br>1FGL J1505.8+3725                                           | ... | fsrq  | B2 1504+37               |
| J1506.3+4332 | 226.594 | 43.544  | 72.973  | 58.278 | 0.086      | 0.080      | −67    | 5.8      | 0.3      | 0.1             | 2.9      | 0.7             | 1.95          | 0.15                 | PL  | ... | ...   | ...                                                                              | ... | bll   | NVSS<br>J150617+433413   |
| J1506.4−0340 | 226.622 | −3.668  | 354.808 | 45.170 | 0.122      | 0.103      | 35     | 4.2      | 0.4      | 0.1             | 4.4      | 1.2             | 2.33          | 0.17                 | PL  | ... | ...   | ...                                                                              | ... | ...   | ...                      |
| J1506.6−6219 | 226.668 | −62.331 | 317.934 | −3.466 | 0.072      | 0.053      | −1     | 7.2      | 0.8      | 0.2             | 9.3      | 1.7             | 1.86          | 0.15                 | PL  | ... | ...   | 1FHL J1507.0−6223<br>2FGL J1507.0−6223                                           | E   | ...   | ...                      |
| J1506.6+0811 | 226.675 | 8.185   | 8.670   | 52.827 | 0.070      | 0.057      | −1     | 9.5      | 0.6      | 0.1             | 6.8      | 1.1             | 1.87          | 0.11                 | PL  | ... | ...   | 2FGL J1506.6+0806                                                                | ... | bll   | PMN J1506+0814           |
| J1507.4+1725 | 226.869 | 17.420  | 22.922  | 57.185 | 0.120      | 0.109      | −24    | 4.7      | 0.2      | 0.1             | 2.8      | 0.8             | 1.78          | 0.20                 | PL  | ... | ...   | ...                                                                              | ... | bll   | NVSS<br>J150716+172103   |
| J1507.6−3710 | 226.909 | −37.178 | 330.937 | 18.179 | 0.145      | 0.092      | −73    | 5.5      | 0.4      | 0.1             | 4.9      | 1.0             | 2.13          | 0.15                 | PL  | ... | ...   | ...                                                                              | ... | bcu   | NVSS<br>J150720−370903   |
| J1508.6+2709 | 227.165 | 27.157  | 41.000  | 59.570 | 0.051      | 0.044      | −37    | 6.9      | 0.3      | 0.1             | 3.6      | 0.9             | 1.71          | 0.21                 | PL  | ... | ...   | 2FGL J1508.5+2709                                                                | ... | bll   | RBS 1467                 |
| J1508.7−4956 | 227.184 | −49.933 | 324.388 | 7.131  | 0.102      | 0.075      | 77     | 10.1     | 1.0      | 0.1             | 19.7     | 2.0             | 2.73          | 0.07                 | PL  | T   | 5     | 2FGL J1508.5−4957                                                                | ... | bcu   | PMN J1508−4953           |
| J1509.4−5850 | 227.365 | −58.845 | 319.976 | −0.618 | 0.020      | 0.020      | −75    | 36.4     | 15.4     | 0.6             | 102.9    | 5.5             | 2.33          | ...                  | EC  | ... | ...   | 2FGL J1509.6−5850<br>1FGL J1509.4−5850<br>0FGL J1509.5−5848<br>1AGL J1506−5859   | ... | PSR   | PSR J1509−5850           |
| J1509.7+5556 | 227.438 | 55.935  | 91.832  | 52.016 | 0.048      | 0.044      | 89     | 10.7     | 0.5      | 0.1             | 5.4      | 0.9             | 1.87          | 0.11                 | PL  | ... | ...   | 2FGL J1509.7+5556<br>1FGL J1509.4+5602                                           | ... | bll   | SBS 1508+561             |
| J1509.9−2951 | 227.484 | −29.864 | 335.597 | 24.083 | 0.367      | 0.269      | −26    | 6.2      | 0.3      | 0.1             | 7.6      | 1.2             | 2.78          | 0.13                 | PL  | ... | 1     | ...                                                                              | ... | bcu   | TXS 1507−296             |
| J1510.2−5754 | 227.570 | −57.916 | 320.538 | 0.130  | 0.156      | 0.076      | −6     | 9.1      | 2.9      | 0.3             | 43.5     | 5.3             | 2.52          | 0.08                 | PL  | ... | 4     | 1FGL J1510.8−5804c                                                               | ... | ...   | ...                      |
| J1510.9−0542 | 227.747 | −5.706  | 353.945 | 42.928 | 0.047      | 0.043      | −30    | 16.7     | 2.0      | 0.2             | 27.0     | 2.0             | 2.43          | 0.05                 | PL  | ... | ...   | 2FGL J1510.9−0545<br>1FGL J1511.1−0545<br>0FGL J1511.2−0536                      | ... | fsrq  | PKS 1508−05              |
| J1511.8−0513 | 227.960 | −5.219  | 354.618 | 43.128 | 0.050      | 0.041      | −82    | 10.6     | 0.9      | 0.1             | 10.6     | 1.6             | 2.03          | 0.11                 | PL  | ... | ...   | 2FGL J1511.8−0513                                                                | ... | bcu   | NVSS<br>J151148−051345   |
| J1512.2+0202 | 228.065 | 2.033   | 2.330   | 47.980 | 0.038      | 0.035      | 18     | 23.7     | 2.0      | 0.1             | 23.4     | 1.5             | 2.20          | 0.05                 | PL  | ... | ...   | 1FGL J1511.8−0513<br>1FHL J1512.2+0204<br>2FGL J1512.2+0201<br>1FGL J1512.3+0201 | ... | fsrq  | PKS 1509+022             |
| J1512.2−2255 | 228.075 | −22.931 | 340.523 | 29.471 | 0.060      | 0.051      | −48    | 8.3      | 0.6      | 0.1             | 7.5      | 1.3             | 1.91          | 0.12                 | PL  | ... | ...   | 1FHL J1512.1−2255                                                                | ... | bcu   | 1RXS<br>J151213.1−225515 |
| J1512.3+6622 | 228.087 | 66.373  | 103.792 | 45.164 | 0.139      | 0.119      | 78     | 4.1      | 0.2      | 0.1             | 2.3      | 0.6             | 2.23          | 0.20                 | PL  | ... | ...   | 1FGL J1511.9−2253                                                                | ... | ...   | ...                      |
| J1512.3+8005 | 228.089 | 80.088  | 115.965 | 35.052 | 0.134      | 0.111      | 52     | 5.0      | 0.2      | 0.0             | 2.8      | 0.6             | 2.51          | 0.19                 | PL  | ... | ...   | ...                                                                              | ... | bcu   | 1RXS<br>J151026.3+795946 |
| J1512.8−5639 | 228.203 | −56.666 | 321.471 | 1.029  | 0.053      | 0.047      | 71     | 7.1      | 1.5      | 0.2             | 21.5     | 3.2             | 2.46          | 0.09                 | PL  | T   | 1,4,5 | ...                                                                              | ... | ...   | ...                      |
| J1512.8−0906 | 228.213 | −9.103  | 351.289 | 40.135 | 0.010      | 0.009      | −26    | 207.3    | 41.1     | 0.5             | 492.8    | 4.9             | 2.36          | ...                  | LP  | T   | ...   | 1FHL J1512.8−0906                                                                | P   | FSRQ  | PKS 1510−08              |

Table 1—Continued

| Name 3FGL     | R.A.    | Decl.   | $l$     | $b$    | $\theta_1$ | $\theta_2$ | $\phi$ | $\sigma$ | $F_{35}$ | $\Delta F_{35}$ | $S_{25}$ | $\Delta S_{25}$ | $\Gamma_{25}$ | $\Delta \Gamma_{25}$ | Mod | Var | Flags   | $\gamma$ -ray Assoc. | TeV | Class | ID or Assoc.     |
|---------------|---------|---------|---------|--------|------------|------------|--------|----------|----------|-----------------|----------|-----------------|---------------|----------------------|-----|-----|---------|----------------------|-----|-------|------------------|
|               |         |         |         |        |            |            |        |          |          |                 |          |                 |               |                      |     |     |         | 2FGL J1512.8–0906    |     |       |                  |
|               |         |         |         |        |            |            |        |          |          |                 |          |                 |               |                      |     |     |         | 1FGL J1512.8–0906    |     |       |                  |
|               |         |         |         |        |            |            |        |          |          |                 |          |                 |               |                      |     |     |         | 0FGL J1512.7–0905    |     |       |                  |
|               |         |         |         |        |            |            |        |          |          |                 |          |                 |               |                      |     |     |         | 3EG J1512–0849       |     |       |                  |
|               |         |         |         |        |            |            |        |          |          |                 |          |                 |               |                      |     |     |         | EGR J1512–0857       |     |       |                  |
|               |         |         |         |        |            |            |        |          |          |                 |          |                 |               |                      |     |     |         | 1AGL J1511–0908      |     |       |                  |
| J1513.1–1014  | 228.290 | −10.241 | 350.372 | 39.239 | 0.230      | 0.161      | 43     | 4.6      | 0.5      | 0.1             | 11.5     | 2.6             | 2.77          | 0.17                 | PL  | ... | 5       | ...                  | ... | fsrq  | PKS 1511–100     |
| J1513.3–3719  | 228.329 | −37.319 | 331.863 | 17.458 | 0.091      | 0.076      | −26    | 4.3      | 0.2      | 0.1             | 2.9      | 0.9             | 1.68          | 0.22                 | PL  | ... | ...     | ...                  | ... | ...   | ...              |
| J1513.4–2549  | 228.368 | −25.827 | 338.848 | 26.965 | 0.079      | 0.069      | 68     | 11.0     | 1.2      | 0.1             | 7.0      | 1.0             | 2.23          | ...                  | LP  | ... | ...     | 2FGL J1513.5–2546    | ... | psr   | PSR J1513–25     |
|               |         |         |         |        |            |            |        |          |          |                 |          |                 |               |                      |     |     |         | 3EG J1517–2538       |     |       |                  |
| J1513.5–3233  | 228.377 | −32.553 | 334.669 | 21.422 | 0.092      | 0.068      | −19    | 12.6     | 1.1      | 0.1             | 14.2     | 1.3             | 2.34          | 0.07                 | PL  | T   | ...     | 2FGL J1513.6–3233    | ... | fsrq  | PKS 1510–324     |
| J1513.8–6250c | 228.454 | −62.845 | 318.382 | −4.326 | 0.139      | 0.063      | 0      | 9.8      | 1.3      | 0.2             | 21.6     | 2.2             | 2.58          | 0.07                 | PL  | ... | 1,3,6,9 | 2FGL J1512.5–6247c   | ... | ...   | ...              |
| J1513.9–5908  | 228.482 | −59.136 | 320.321 | −1.162 | ...        | ...        | ...    | 7.4      | 1.1      | 0.3             | 45.0     | 5.3             | 3.12          | 0.13                 | PL  | ... | 1,3     | 1FGL J1513.2–5904    | ... | PSR   | PSR J1513–5908   |
|               |         |         |         |        |            |            |        |          |          |                 |          |                 |               |                      |     |     |         | ...                  |     |       |                  |
| J1514.0–5915e | 228.507 | −59.256 | 320.270 | −1.271 | ...        | ...        | ...    | ...      | 2.9      | ...             | 45.6     | ...             | 1.57          | ...                  | PL  | ... | ...     | 1FHL J1514.0–5915e   | E   | PWN   | MSH 15–52        |
|               |         |         |         |        |            |            |        |          |          |                 |          |                 |               |                      |     |     |         | 2FGL J1514.0–5915e   |     |       | $\infty$         |
|               |         |         |         |        |            |            |        |          |          |                 |          |                 |               |                      |     |     |         | 1FGL J1514.7–5917    |     |       |                  |
| J1514.1+2940  | 228.536 | 29.682  | 46.139  | 58.637 | 0.248      | 0.237      | −42    | 4.4      | 0.2      | 0.1             | 4.2      | 1.0             | 2.88          | 0.21                 | PL  | ... | ...     | ...                  | ... | fsrq  | MG2 J151421+2930 |
| J1514.2–4947  | 228.558 | −49.784 | 325.231 | 6.803  | 0.021      | 0.021      | −32    | 39.4     | 6.6      | 0.3             | 42.8     | 2.1             | 2.07          | ...                  | EC  | ... | ...     | 1FHL J1514.3–4945    | ... | PSR   | PSR J1514–4946   |
|               |         |         |         |        |            |            |        |          |          |                 |          |                 |               |                      |     |     |         | 2FGL J1514.1–4946    |     |       |                  |
|               |         |         |         |        |            |            |        |          |          |                 |          |                 |               |                      |     |     |         | 1FGL J1514.1–4945    |     |       |                  |
|               |         |         |         |        |            |            |        |          |          |                 |          |                 |               |                      |     |     |         | 0FGL J1514.3–4946    |     |       |                  |
| J1514.5–4750  | 228.641 | −47.835 | 326.309 | 8.434  | 0.071      | 0.055      | 59     | 13.1     | 1.4      | 0.1             | 17.4     | 1.6             | 2.33          | 0.07                 | PL  | T   | ...     | 2FGL J1514.6–4751    | ... | fsrq  | PMN J1514–4748   |
|               |         |         |         |        |            |            |        |          |          |                 |          |                 |               |                      |     |     |         | 1FGL J1514.1–4745    |     |       |                  |
| J1514.8+4446  | 228.711 | 44.778  | 74.177  | 56.432 | 0.078      | 0.066      | −69    | 15.7     | 0.8      | 0.1             | 10.4     | 0.9             | 2.34          | 0.07                 | PL  | ... | ...     | 2FGL J1514.6+4449    | ... | fsrq  | NVSS             |
|               |         |         |         |        |            |            |        |          |          |                 |          |                 |               |                      |     |     |         |                      |     |       | J151436+445003   |
|               |         |         |         |        |            |            |        |          |          |                 |          |                 |               |                      |     |     |         | 1FGL J1514.7+4447    |     |       |                  |
| J1514.8–3623  | 228.719 | −36.385 | 332.673 | 18.070 | 0.171      | 0.145      | 87     | 5.0      | 0.4      | 0.1             | 5.5      | 1.1             | 2.41          | 0.13                 | PL  | ... | ...     | ...                  | ... | bcu   | PMN J1514–3617   |
| J1516.7+3648  | 229.192 | 36.809  | 59.685  | 57.912 | 0.109      | 0.097      | 45     | 5.6      | 0.3      | 0.1             | 3.3      | 0.7             | 2.23          | 0.14                 | PL  | ... | ...     | 2FGL J1517.2+3645    | ... | bll   | MG2 J151646+3650 |
| J1516.9+1926  | 229.236 | 19.446  | 27.834  | 55.842 | 0.256      | 0.199      | 16     | 6.4      | 0.3      | 0.1             | 6.0      | 0.9             | 2.77          | 0.14                 | PL  | ... | ...     | 2FGL J1516.9+1925    | ... | bll   | PKS 1514+197     |
|               |         |         |         |        |            |            |        |          |          |                 |          |                 |               |                      |     |     |         | 1FGL J1516.9+1928    |     |       |                  |
| J1517.0+2637  | 229.253 | 26.631  | 40.537  | 57.649 | 0.109      | 0.085      | −55    | 4.1      | 0.2      | 0.1             | 2.2      | 0.7             | 2.00          | 0.23                 | PL  | ... | ...     | ...                  | ... | ...   | ...              |
| J1517.6–4442  | 229.405 | −44.702 | 328.456 | 10.805 | 0.252      | 0.141      | −77    | 6.7      | 0.6      | 0.1             | 9.6      | 1.5             | 2.57          | 0.11                 | PL  | ... | 1,3     | ...                  | ... | ...   | ...              |
| J1517.6+6524  | 229.419 | 65.415  | 102.263 | 45.403 | 0.032      | 0.029      | −29    | 18.5     | 0.8      | 0.1             | 10.2     | 1.1             | 1.78          | 0.07                 | PL  | ... | ...     | 1FHL J1517.9+6526    | ... | bll   | 1H 1515+660      |
|               |         |         |         |        |            |            |        |          |          |                 |          |                 |               |                      |     |     |         | 2FGL J1518.0+6526    |     |       |                  |
|               |         |         |         |        |            |            |        |          |          |                 |          |                 |               |                      |     |     |         | 1FGL J1517.8+6530    |     |       |                  |



Table 1—Continued

| Name 3FGL    | R.A.    | Decl.   | $l$     | $b$    | $\theta_1$ | $\theta_2$ | $\phi$ | $\sigma$ | $F_{35}$ | $\Delta F_{35}$ | $S_{25}$ | $\Delta S_{25}$ | $\Gamma_{25}$ | $\Delta \Gamma_{25}$ | Mod | Var | Flags | $\gamma$ -ray Assoc.                                                             | TeV | Class | ID or Assoc.             |
|--------------|---------|---------|---------|--------|------------|------------|--------|----------|----------|-----------------|----------|-----------------|---------------|----------------------|-----|-----|-------|----------------------------------------------------------------------------------|-----|-------|--------------------------|
| J1517.6–2422 | 229.421 | –24.376 | 340.676 | 27.577 | 0.020      | 0.020      | –54    | 45.4     | 5.2      | 0.2             | 58.4     | 2.2             | 2.11          | 0.03                 | PL  | ... | ...   | 1FHL J1517.8–2421<br>2FGL J1517.7–2421<br>1FGL J1517.8–2423<br>0FGL J1517.9–2423 | P   | bll   | AP Librae                |
| J1518.0–2732 | 229.520 | –27.539 | 338.667 | 24.974 | 0.036      | 0.034      | 49     | 18.4     | 1.8      | 0.1             | 20.7     | 1.6             | 2.13          | 0.06                 | PL  | T   | ...   | 1FHL J1518.4–2733<br>2FGL J1518.2–2733                                           | ... | bcu   | TXS 1515–273             |
| J1518.2–5232 | 229.571 | –52.535 | 324.313 | 4.132  | 0.068      | 0.058      | –25    | 10.4     | 1.4      | 0.2             | 16.4     | 1.8             | 2.24          | 0.07                 | PL  | ... | ...   | 2FGL J1518.4–5233<br>1FGL J1518.0–5233                                           | ... | ...   | ...                      |
| J1520.3+4209 | 230.093 | 42.154  | 69.121  | 56.235 | 0.111      | 0.107      | 66     | 10.0     | 0.5      | 0.1             | 6.9      | 0.8             | 2.50          | 0.09                 | PL  | T   | ...   | 2FGL J1520.9+4209<br>1FGL J1519.7+4216                                           | ... | fsrq  | B3 1518+423              |
| J1520.8–0348 | 230.203 | –3.812  | 358.118 | 42.506 | 0.039      | 0.034      | –64    | 15.8     | 1.2      | 0.1             | 14.7     | 1.7             | 1.83          | 0.07                 | PL  | ... | ...   | 1FHL J1520.8–0348<br>2FGL J1520.8–0349<br>1FGL J1521.0–0350                      | ... | bll   | NVSS<br>J152048–034850   |
| J1521.1+5543 | 230.296 | 55.722  | 90.145  | 50.786 | 0.105      | 0.073      | 90     | 6.5      | 0.3      | 0.1             | 3.2      | 0.6             | 2.17          | 0.18                 | PL  | ... | ...   | ...                                                                              | ... | bll   | SDSS J152034.98+554256.9 |
| J1521.8+4340 | 230.466 | 43.674  | 71.608  | 55.573 | 0.156      | 0.143      | 59     | 5.8      | 0.3      | 0.1             | 4.4      | 0.8             | 2.61          | 0.14                 | PL  | T   | ...   | 2FGL J1522.0+4348                                                                | ... | fsrq  | B3 1520+437              |
| J1521.9–5736 | 230.486 | –57.611 | 322.021 | –0.428 | 0.032      | 0.031      | 31     | 27.0     | 9.4      | 0.5             | 69.3     | 3.9             | 2.35          | ...                  | EC  | ... | ...   | 2FGL J1521.8–5735<br>1FGL J1521.8–5734c                                          | ... | PSR   | LAT PSR J1522–5734       |
| J1522.1+3144 | 230.543 | 31.736  | 50.163  | 57.022 | 0.012      | 0.012      | 21     | 192.7    | 17.9     | 0.3             | 211.9    | 2.7             | 2.35          | ...                  | LP  | T   | ...   | 1FHL J1522.2+3145<br>2FGL J1522.1+3144<br>1FGL J1522.1+3143<br>0FGL J1522.2+3143 | ... | fsrq  | B2 1520+31               |
| J1522.6–2730 | 230.662 | –27.508 | 339.585 | 24.399 | 0.035      | 0.031      | –74    | 26.0     | 2.9      | 0.2             | 32.7     | 1.9             | 2.13          | 0.04                 | PL  | T   | ...   | 2FGL J1522.7–2731<br>1FGL J1522.6–2732                                           | ... | bll   | PKS 1519–273             |
| J1525.2–5905 | 231.317 | –59.087 | 321.576 | –1.902 | 0.243      | 0.175      | 23     | 4.1      | 0.7      | 0.2             | 15.4     | 3.7             | 2.79          | 0.22                 | PL  | ... | 4,5   | ...                                                                              | ... | bcu   | PMN J1524–5903           |
| J1525.8–0834 | 231.470 | –8.579  | 354.760 | 38.289 | 0.079      | 0.065      | 73     | 4.2      | 0.2      | 0.1             | 2.6      | 0.9             | 1.64          | 0.26                 | PL  | ... | ...   | ...                                                                              | ... | ...   | ...                      |
| J1526.3–4505 | 231.586 | –45.086 | 329.549 | 9.631  | 0.090      | 0.080      | 48     | 5.4      | 0.5      | 0.1             | 7.7      | 1.7             | 2.52          | 0.17                 | PL  | ... | 1     | ...                                                                              | ... | ...   | ...                      |
| J1527.0–3804 | 231.754 | –38.080 | 333.757 | 15.308 | 0.087      | 0.080      | 30     | 4.5      | 0.4      | 0.1             | 4.7      | 1.1             | 2.33          | 0.18                 | PL  | ... | ...   | ...                                                                              | ... | ...   | ...                      |
| J1528.1–2904 | 232.036 | –29.068 | 339.610 | 22.426 | 0.082      | 0.059      | 24     | 4.3      | 0.2      | 0.1             | 3.0      | 1.0             | 1.70          | 0.24                 | PL  | ... | ...   | ...                                                                              | ... | ...   | ...                      |
| J1528.3–5836 | 232.078 | –58.608 | 322.171 | –1.724 | 0.055      | 0.049      | –64    | 11.5     | 3.1      | 0.3             | 12.5     | 1.3             | 2.44          | ...                  | LP  | ... | 12    | 2FGL J1528.0–5841                                                                | ... | ...   | ...                      |
| J1528.7–2247 | 232.175 | –22.787 | 344.018 | 27.271 | 0.185      | 0.134      | –36    | 4.4      | 0.4      | 0.1             | 4.6      | 1.0             | 2.24          | 0.15                 | PL  | ... | ...   | 3EG J1527–2358                                                                   | ... | ...   | ...                      |
| J1529.5+6733 | 232.399 | 67.559  | 103.487 | 43.114 | 0.137      | 0.111      | –16    | 4.6      | 0.2      | 0.0             | 2.4      | 0.6             | 2.24          | 0.17                 | PL  | ... | ...   | ...                                                                              | ... | ...   | ...                      |
| J1531.0+5737 | 232.767 | 57.621  | 91.599  | 48.649 | 0.066      | 0.054      | 19     | 9.3      | 0.4      | 0.1             | 4.7      | 0.7             | 2.27          | 0.13                 | PL  | ... | ...   | 2FGL J1531.0+5725                                                                | ... | bll   | 87GB<br>152947.5+574636  |
| J1531.8+4704 | 232.954 | 47.081  | 76.297  | 52.896 | 0.143      | 0.111      | 65     | 4.9      | 0.2      | 0.1             | 2.7      | 0.6             | 2.32          | 0.20                 | PL  | ... | ...   | ...                                                                              | ... | bll   | 1RXS<br>J153148.8+465912 |
| J1532.0–2618 | 233.014 | –26.303 | 342.211 | 24.063 | 0.095      | 0.080      | –34    | 4.4      | 0.4      | 0.1             | 4.5      | 1.1             | 2.18          | 0.17                 | PL  | ... | ...   | ...                                                                              | ... | ...   | ...                      |

Table 1—Continued

| Name 3FGL    | R.A.    | Decl.   | $l$     | $b$     | $\theta_1$ | $\theta_2$ | $\phi$ | $\sigma$ | $F_{35}$ | $\Delta F_{35}$ | $S_{25}$ | $\Delta S_{25}$ | $\Gamma_{25}$ | $\Delta \Gamma_{25}$ | Mod | Var | Flags | $\gamma$ -ray Assoc.                                                             | TeV | Class | ID or Assoc.           |
|--------------|---------|---------|---------|---------|------------|------------|--------|----------|----------|-----------------|----------|-----------------|---------------|----------------------|-----|-----|-------|----------------------------------------------------------------------------------|-----|-------|------------------------|
| J1532.0+3018 | 233.022 | 30.308  | 47.846  | 54.815  | 0.054      | 0.048      | 8      | 8.2      | 0.4      | 0.1             | 4.5      | 0.9             | 1.77          | 0.13                 | PL  | ... | ...   | 1FGL J1531.8+3018                                                                | ... | bll   | RX J1531.9+3016        |
| J1532.7−1319 | 233.188 | −13.325 | 352.143 | 33.719  | 0.024      | 0.023      | −64    | 35.6     | 3.9      | 0.2             | 43.2     | 2.0             | 2.09          | 0.03                 | PL  | T   | ...   | 1FHL J1532.6−1317                                                                | ... | bcu   | TXS 1530−131           |
| J1533.2+1852 | 233.312 | 18.871  | 29.161  | 52.028  | 0.083      | 0.078      | 42     | 6.7      | 0.4      | 0.1             | 4.2      | 0.9             | 1.89          | 0.18                 | PL  | ... | ...   | ...                                                                              | ... | bll   | RX J1533.1+1854        |
| J1533.5+3416 | 233.387 | 34.281  | 54.746  | 54.666  | 0.094      | 0.087      | −45    | 5.9      | 0.3      | 0.1             | 3.3      | 0.8             | 1.85          | 0.16                 | PL  | ... | ...   | ...                                                                              | ... | bll   | RX J1533.3+3416        |
| J1533.8−5231 | 233.473 | −52.533 | 326.289 | 2.812   | 0.055      | 0.048      | −21    | 6.4      | 0.8      | 0.2             | 9.1      | 1.8             | 1.97          | 0.12                 | PL  | ... | ...   | ...                                                                              | ... | ...   | ...                    |
| J1534.4+5323 | 233.607 | 53.398  | 85.503  | 50.182  | 0.156      | 0.136      | 54     | 4.1      | 0.2      | 0.1             | 2.2      | 0.6             | 1.96          | 0.20                 | PL  | ... | ...   | ...                                                                              | ... | bll   | 1ES 1533+535           |
| J1534.5+0128 | 233.645 | 1.483   | 6.676   | 43.270  | 0.150      | 0.141      | −52    | 8.5      | 0.4      | 0.1             | 8.9      | 1.1             | 2.78          | 0.11                 | PL  | T   | ...   | ...                                                                              | ... | fsrq  | PKS 1532+01            |
| J1535.0+3721 | 233.754 | 37.365  | 60.025  | 54.236  | 0.107      | 0.071      | −10    | 7.7      | 0.4      | 0.1             | 4.6      | 0.8             | 2.11          | 0.12                 | PL  | ... | ...   | 2FGL J1535.4+3720                                                                | ... | bll   | RGB J1534+372          |
| J1535.7+3920 | 233.931 | 39.335  | 63.340  | 53.899  | 0.101      | 0.096      | 86     | 4.8      | 0.2      | 0.1             | 2.7      | 0.6             | 2.10          | 0.15                 | PL  | ... | ...   | ...                                                                              | ... | bll   | RX J1535.4+3922        |
| J1536.3−4949 | 234.099 | −49.822 | 328.196 | 4.782   | 0.016      | 0.016      | −87    | 60.1     | 11.8     | 0.3             | 87.4     | 3.0             | 2.04          | ...                  | LP  | ... | ...   | 1FHL J1536.4−4951<br>2FGL J1536.4−4949<br>1FGL J1536.5−4949<br>0FGL J1536.7−4947 | ... | psr   | PSR J1536−4948         |
| J1536.6+8331 | 234.162 | 83.532  | 117.908 | 31.898  | 0.259      | 0.132      | −16    | 4.3      | 0.2      | 0.1             | 3.1      | 0.7             | 2.48          | 0.17                 | PL  | ... | ...   | ...                                                                              | ... | bcu   | NVSS<br>J153556+832614 |
| J1537.8−8000 | 234.470 | −80.009 | 309.952 | −19.489 | 0.052      | 0.046      | 13     | 12.2     | 0.9      | 0.1             | 10.7     | 1.1             | 2.19          | 0.08                 | PL  | T   | ...   | 2FGL J1537.4−7957                                                                | ... | bcu   | PMN J1537.8−7958       |
| J1538.4−4656 | 234.603 | −46.935 | 330.187 | 6.909   | 0.477      | 0.291      | 39     | 12.5     | 0.9      | 0.1             | 21.1     | 1.8             | 2.85          | 0.08                 | PL  | ... | 3,9   | 2FGL J1539.3−4636                                                                | ... | ...   | ...                    |
| J1539.2−3324 | 234.823 | −33.414 | 338.759 | 17.534  | 0.037      | 0.035      | 67     | 19.2     | 2.4      | 0.2             | 11.6     | 1.0             | 1.81          | ...                  | LP  | ... | ...   | 2FGL J1539.2−3325<br>1FGL J1539.0−3328                                           | ... | ...   | ...                    |
| J1539.5+2746 | 234.887 | 27.767  | 43.910  | 52.883  | 0.053      | 0.048      | 47     | 14.8     | 0.9      | 0.1             | 10.2     | 1.0             | 2.08          | 0.07                 | PL  | T   | ...   | 2FGL J1539.5+2747<br>1FGL J1539.7+2747                                           | ... | fsrq  | MG2 J153938+2744       |
| J1539.8−1128 | 234.958 | −11.479 | 355.183 | 33.808  | 0.101      | 0.081      | 55     | 5.8      | 0.5      | 0.1             | 5.4      | 1.2             | 2.08          | 0.16                 | PL  | ... | ...   | ...                                                                              | ... | bcu   | PMN J1539−1128         |
| J1540.1+8155 | 235.025 | 81.924  | 116.478 | 32.966  | 0.040      | 0.030      | −39    | 14.6     | 0.5      | 0.1             | 8.1      | 1.2             | 1.60          | 0.08                 | PL  | ... | ...   | 1FHL J1537.5+8159<br>2FGL J1538.1+8159<br>...                                    | ... | bll   | 1ES 1544+820           |
| J1540.8+1449 | 235.201 | 14.833  | 24.375  | 48.819  | 0.098      | 0.076      | −87    | 4.8      | 0.4      | 0.1             | 4.7      | 1.2             | 2.34          | 0.17                 | PL  | ... | ...   | 2FGL J1540.4+1438                                                                | ... | bll   | 4C +14.60              |
| J1541.6+1414 | 235.403 | 14.234  | 23.676  | 48.392  | 0.083      | 0.074      | 43     | 4.9      | 0.3      | 0.1             | 3.4      | 0.9             | 1.98          | 0.23                 | PL  | ... | ...   | ...                                                                              | ... | ...   | ...                    |
| J1541.8+1105 | 235.462 | 11.092  | 19.541  | 46.935  | 0.170      | 0.155      | −1     | 6.5      | 0.3      | 0.1             | 6.3      | 1.0             | 2.73          | 0.14                 | PL  | ... | ...   | ...                                                                              | ... | fsrq  | MG1 J154207+1110       |
| J1542.4−5911 | 235.622 | −59.198 | 323.312 | −3.272  | 0.194      | 0.142      | −19    | 5.5      | 0.7      | 0.1             | 11.3     | 2.1             | 2.60          | 0.13                 | PL  | ... | 1     | ...                                                                              | ... | ...   | ...                    |
| J1542.9+6129 | 235.738 | 61.495  | 95.388  | 45.394  | 0.019      | 0.018      | −32    | 62.7     | 4.9      | 0.2             | 44.8     | 2.0             | 1.99          | ...                  | LP  | T   | ...   | 1FHL J1542.9+6128<br>2FGL J1542.9+6129<br>1FGL J1542.9+6129<br>0FGL J1543.1+6130 | ... | bll   | GB6 J1542+6129         |
| J1542.9−5141 | 235.746 | −51.692 | 327.913 | 2.660   | 0.183      | 0.141      | 39     | 8.6      | 1.5      | 0.2             | 21.8     | 2.6             | 2.49          | 0.08                 | PL  | ... | ...   | ...                                                                              | ... | PSR   | PSR J1543−5149         |
| J1543.5+0451 | 235.879 | 4.864   | 12.244  | 43.393  | 0.102      | 0.080      | 74     | 5.3      | 0.4      | 0.1             | 4.3      | 1.0             | 1.98          | 0.19                 | PL  | ... | ...   | ...                                                                              | ... | bcu   | CGCG 050−083           |
| J1543.5−0244 | 235.889 | −2.748  | 4.074   | 38.900  | 0.179      | 0.112      | −85    | 8.1      | 0.7      | 0.1             | 6.5      | 1.1             | 2.41          | ...                  | LP  | ... | ...   | 2FGL J1543.7−0241                                                                | ... | ...   | ...                    |

Table 1—Continued

| Name 3FGL     | R.A.    | Decl.   | $l$     | $b$    | $\theta_1$ | $\theta_2$ | $\phi$ | $\sigma$ | $F_{35}$ | $\Delta F_{35}$ | $S_{25}$ | $\Delta S_{25}$ | $\Gamma_{25}$ | $\Delta \Gamma_{25}$ | Mod | Var | Flags    | $\gamma$ -ray Assoc. | TeV | Class | ID or Assoc.        |
|---------------|---------|---------|---------|--------|------------|------------|--------|----------|----------|-----------------|----------|-----------------|---------------|----------------------|-----|-----|----------|----------------------|-----|-------|---------------------|
|               |         |         |         |        |            |            |        |          |          |                 |          |                 |               |                      |     |     |          | 1FGL J1544.0–0252    |     |       |                     |
| J1544.0+4938  | 236.018 | 49.650  | 79.199  | 50.161 | 0.141      | 0.106      | 82     | 6.2      | 0.3      | 0.1             | 3.6      | 0.6             | 2.30          | 0.14                 | PL  | ... | ...      | ...                  | ... | PSR   | PSR J1544+4937      |
| J1544.1–2555  | 236.028 | –25.920 | 344.735 | 22.612 | 0.128      | 0.087      | 39     | 9.5      | 0.9      | 0.1             | 11.5     | 1.3             | 2.36          | 0.08                 | PL  | ... | ...      | 2FGL J1544.1–2554    | ... | ...   | ...                 |
| J1544.6–1125  | 236.170 | –11.427 | 356.211 | 32.984 | 0.077      | 0.067      | 52     | 10.8     | 1.0      | 0.1             | 13.5     | 1.4             | 2.41          | 0.07                 | PL  | ... | ...      | 2FGL J1544.5–1126    | ... | ...   | ...                 |
|               |         |         |         |        |            |            |        |          |          |                 |          |                 |               |                      |     |     |          | 1FGL J1544.5–1127    |     |       |                     |
| J1545.0–6641  | 236.269 | –66.692 | 318.930 | –9.378 | 0.038      | 0.036      | 64     | 7.5      | 0.3      | 0.1             | 4.4      | 1.0             | 1.67          | 0.18                 | PL  | ... | ...      | 1FHL J1545.2–6640    | ... | ...   | ...                 |
| J1546.0+0818  | 236.502 | 8.307   | 16.769  | 44.682 | 0.040      | 0.038      | 66     | 10.3     | 0.5      | 0.1             | 7.0      | 1.3             | 1.69          | 0.11                 | PL  | ... | ...      | 2FGL J1546.1+0820    | ... | bll   | 1RXS                |
|               |         |         |         |        |            |            |        |          |          |                 |          |                 |               |                      |     |     |          |                      |     |       | J154604.6+081912    |
| J1546.6+1812  | 236.672 | 18.204  | 29.927  | 48.810 | 0.105      | 0.097      | –85    | 5.0      | 0.3      | 0.1             | 3.9      | 0.9             | 2.30          | 0.18                 | PL  | ... | ...      | ...                  | ... | bll   | MG1 J154628+1817    |
| J1547.1–2801  | 236.782 | –28.030 | 343.781 | 20.583 | 0.107      | 0.082      | 83     | 4.3      | 0.3      | 0.1             | 3.8      | 1.1             | 1.71          | 0.17                 | PL  | ... | ...      | ...                  | ... | bcu   | 1RXS                |
|               |         |         |         |        |            |            |        |          |          |                 |          |                 |               |                      |     |     |          |                      |     |       | J154711.8–280222    |
| J1548.4+1455  | 237.110 | 14.926  | 25.633  | 47.175 | 0.039      | 0.039      | 57     | 17.3     | 1.3      | 0.1             | 14.5     | 1.3             | 2.11          | 0.07                 | PL  | ... | ...      | 1FHL J1548.3+1455    | ... | ...   | ...                 |
|               |         |         |         |        |            |            |        |          |          |                 |          |                 |               |                      |     |     |          | 2FGL J1548.3+1453    |     |       |                     |
|               |         |         |         |        |            |            |        |          |          |                 |          |                 |               |                      |     |     |          | 1FGL J1548.6+1451    |     |       |                     |
| J1548.8–2250  | 237.215 | –22.849 | 347.853 | 24.165 | 0.047      | 0.042      | 12     | 12.1     | 1.1      | 0.1             | 12.7     | 1.5             | 2.05          | 0.08                 | PL  | ... | ...      | 1FHL J1548.8–2251    | ... | bll   | PMN J1548–2251      |
|               |         |         |         |        |            |            |        |          |          |                 |          |                 |               |                      |     |     |          | 2FGL J1548.8–2251    |     |       |                     |
|               |         |         |         |        |            |            |        |          |          |                 |          |                 |               |                      |     |     |          | 1FGL J1548.7–2250    |     |       |                     |
| J1549.0+6309  | 237.260 | 63.153  | 96.900  | 43.948 | 0.125      | 0.119      | 32     | 5.2      | 0.2      | 0.0             | 3.4      | 0.7             | 2.73          | 0.16                 | PL  | ... | 1        | 1FGL J1548.7+6311    | ... | bcu   | SDSS                |
|               |         |         |         |        |            |            |        |          |          |                 |          |                 |               |                      |     |     |          |                      |     |       | J154958.45+631021.2 |
| J1549.1–5347c | 237.300 | –53.784 | 327.369 | 0.432  | 0.104      | 0.088      | –50    | 11.6     | 4.2      | 0.4             | 66.2     | 5.2             | 2.56          | 0.05                 | PL  | ... | 1,6,7,10 | ...                  | ... | spp   | ...                 |
| J1549.4+0237  | 237.372 | 2.631   | 10.861  | 40.912 | 0.050      | 0.047      | 25     | 23.4     | 1.8      | 0.1             | 24.9     | 1.3             | 2.46          | 0.05                 | PL  | T   | ...      | 2FGL J1549.5+0237    | ... | fsrq  | PKS 1546+027        |
|               |         |         |         |        |            |            |        |          |          |                 |          |                 |               |                      |     |     |          | 1FGL J1549.3+0235    |     |       |                     |
| J1549.4–4832  | 237.375 | –48.538 | 330.684 | 4.501  | 0.131      | 0.103      | –18    | 8.7      | 0.9      | 0.2             | 18.8     | 2.3             | 2.74          | 0.10                 | PL  | ... | 1        | ...                  | ... | ...   | ...                 |
| J1549.5+1709  | 237.377 | 17.156  | 28.822  | 47.805 | 0.110      | 0.087      | –42    | 4.4      | 0.2      | 0.1             | 2.8      | 0.8             | 1.92          | 0.25                 | PL  | ... | ...      | ...                  | ... | bcu   | MG1 J154930+1708    |
| J1549.7–0658  | 237.444 | –6.977  | 1.225   | 35.014 | 0.049      | 0.040      | –86    | 11.6     | 1.0      | 0.1             | 11.0     | 1.4             | 1.92          | 0.09                 | PL  | ... | ...      | 1FHL J1549.9–0658    | ... | bcu   | NVSS                |
|               |         |         |         |        |            |            |        |          |          |                 |          |                 |               |                      |     |     |          |                      |     |       | J154952–065907      |
|               |         |         |         |        |            |            |        |          |          |                 |          |                 |               |                      |     |     |          | 2FGL J1549.7–0657    |     |       |                     |
|               |         |         |         |        |            |            |        |          |          |                 |          |                 |               |                      |     |     |          | 1FGL J1549.7–0659    |     |       |                     |
| J1549.9–3044  | 237.475 | –30.746 | 342.368 | 18.142 | 0.066      | 0.062      | –21    | 5.0      | 0.2      | 0.1             | 3.4      | 1.1             | 1.44          | 0.18                 | PL  | ... | ...      | ...                  | ... | ...   | ...                 |
| J1550.3+7409  | 237.598 | 74.157  | 108.881 | 37.680 | 0.166      | 0.116      | 81     | 5.4      | 0.2      | 0.0             | 3.3      | 0.6             | 2.69          | 0.19                 | PL  | ... | 1        | ...                  | ... | bcu   | 87GB                |
|               |         |         |         |        |            |            |        |          |          |                 |          |                 |               |                      |     |     |          |                      |     |       | 155014.9+741816     |
| J1550.4+6027  | 237.623 | 60.462  | 93.476  | 45.093 | 0.056      | 0.053      | 87     | 7.7      | 0.3      | 0.1             | 3.7      | 0.7             | 1.84          | 0.14                 | PL  | ... | ...      | ...                  | ... | ...   | ...                 |
| J1550.5+0526  | 237.639 | 5.445   | 14.202  | 42.233 | 0.073      | 0.061      | 40     | 16.2     | 1.3      | 0.1             | 15.7     | 1.2             | 2.34          | 0.06                 | PL  | ... | ...      | 2FGL J1550.7+0526    | ... | fsrq  | 4C +05.64           |
|               |         |         |         |        |            |            |        |          |          |                 |          |                 |               |                      |     |     |          | 1FGL J1550.7+0527    |     |       |                     |
| J1551.1–5610  | 237.779 | –56.175 | 326.087 | –1.605 | 0.067      | 0.059      | 2      | 6.0      | 1.0      | 0.3             | 12.9     | 2.9             | 1.79          | 0.15                 | PL  | ... | 5        | ...                  | ... | spp   | ...                 |
| J1552.1+0852  | 238.033 | 8.877   | 18.506  | 43.650 | 0.141      | 0.113      | 3      | 6.4      | 0.5      | 0.1             | 5.3      | 0.9             | 2.21          | 0.12                 | PL  | ... | ...      | 2FGL J1551.9+0855    | ... | bll   | TXS 1549+089        |
|               |         |         |         |        |            |            |        |          |          |                 |          |                 |               |                      |     |     |          | 1FGL J1551.7+0851    |     |       |                     |
| J1552.8–5330  | 238.212 | –53.513 | 327.960 | 0.303  | 0.078      | 0.071      | 73     | 11.2     | 7.2      | 0.7             | 41.9     | 5.2             | 2.26          | ...                  | LP  | ... | 7        | ...                  | ... | ...   | ...                 |
| J1552.9–5610  | 238.231 | –56.169 | 326.286 | –1.759 | 0.036      | 0.027      | 37     | 18.4     | 5.2      | 0.3             | 57.9     | 3.8             | 2.08          | 0.04                 | PL  | ... | 7        | 1FHL J1552.6–5610    | ... | spp   | ...                 |
|               |         |         |         |        |            |            |        |          |          |                 |          |                 |               |                      |     |     |          | 2FGL J1552.8–5609    |     |       |                     |

Table 1—Continued

| Name 3FGL     | R.A.    | Decl.   | $l$     | $b$     | $\theta_1$ | $\theta_2$ | $\phi$ | $\sigma$ | $F_{35}$ | $\Delta F_{35}$ | $S_{25}$ | $\Delta S_{25}$ | $\Gamma_{25}$ | $\Delta \Gamma_{25}$ | Mod | Var | Flags  | $\gamma$ -ray Assoc. | TeV | Class | ID or Assoc.             |
|---------------|---------|---------|---------|---------|------------|------------|--------|----------|----------|-----------------|----------|-----------------|---------------|----------------------|-----|-----|--------|----------------------|-----|-------|--------------------------|
|               |         |         |         |         |            |            |        |          |          |                 |          |                 |               |                      |     |     |        | 1FGL J1552.4–5609    |     |       |                          |
| J1553.1+5437  | 238.292 | 54.624  | 85.581  | 47.170  | 0.087      | 0.085      | 34     | 8.5      | 0.4      | 0.1             | 4.5      | 0.6             | 2.26          | 0.12                 | PL  | ... | ...    | ...                  | ... | ...   | ...                      |
| J1553.3–0322c | 238.347 | –3.381  | 5.366   | 36.581  | 0.224      | 0.181      | –20    | 6.5      | 0.6      | 0.1             | 9.1      | 1.4             | 2.56          | 0.12                 | PL  | ... | 1,6    | 2FGL J1553.5–0324    | ... | ...   | ...                      |
| J1553.3–2421  | 238.349 | –24.359 | 347.553 | 22.352  | 0.122      | 0.102      | –66    | 8.1      | 0.8      | 0.1             | 9.8      | 1.3             | 2.28          | 0.09                 | PL  | ... | ...    | 2FGL J1553.2–2424    | ... | fsrq  | PKS 1550–242             |
|               |         |         |         |         |            |            |        |          |          |                 |          |                 |               |                      |     |     |        | 1FGL J1553.4–2425    |     |       |                          |
| J1553.5–3118  | 238.377 | –31.306 | 342.587 | 17.210  | 0.034      | 0.032      | –58    | 13.0     | 0.8      | 0.1             | 8.2      | 1.4             | 1.60          | ...                  | LP  | ... | ...    | 1FHL J1553.4–3117    | ... | bll   | 1RXS<br>J155333.4–311841 |
|               |         |         |         |         |            |            |        |          |          |                 |          |                 |               |                      |     |     |        | 2FGL J1553.5–3116    |     |       |                          |
|               |         |         |         |         |            |            |        |          |          |                 |          |                 |               |                      |     |     |        | 1FGL J1553.5–3116    |     |       |                          |
| J1553.5+1256  | 238.386 | 12.946  | 23.787  | 45.220  | 0.035      | 0.033      | 81     | 32.5     | 2.8      | 0.2             | 29.9     | 1.5             | 2.36          | ...                  | LP  | T   | ...    | 2FGL J1553.5+1255    | ... | fsrq  | PKS 1551+130             |
|               |         |         |         |         |            |            |        |          |          |                 |          |                 |               |                      |     |     |        | 1FGL J1553.4+1255    |     |       |                          |
|               |         |         |         |         |            |            |        |          |          |                 |          |                 |               |                      |     |     |        | 0FGL J1553.4+1255    |     |       |                          |
| J1554.4–5315c | 238.610 | –53.262 | 328.303 | 0.347   | 0.049      | 0.044      | –47    | 8.8      | 3.9      | 0.5             | 43.3     | 6.0             | 2.13          | 0.07                 | PL  | ... | 5,6,10 | 2FGL J1554.4–5317c   | ... | ...   | ...                      |
|               |         |         |         |         |            |            |        |          |          |                 |          |                 |               |                      |     |     |        | 1FGL J1554.8–5312c   |     |       |                          |
| J1554.4+2010  | 238.611 | 20.170  | 33.632  | 47.744  | 0.085      | 0.082      | 16     | 5.7      | 0.3      | 0.1             | 3.9      | 0.9             | 2.25          | 0.18                 | PL  | ... | ...    | ...                  | ... | bll   | 1ES 1552+203             |
| J1555.7+1111  | 238.936 | 11.194  | 21.918  | 43.960  | 0.009      | 0.009      | –62    | 97.5     | 13.2     | 0.3             | 164.1    | 6.0             | 1.68          | ...                  | LP  | T   | ...    | 1FHL J1555.7+1111    | P   | BLL   | PG 1553+1113             |
|               |         |         |         |         |            |            |        |          |          |                 |          |                 |               |                      |     |     |        | 2FGL J1555.7+1111    |     |       |                          |
|               |         |         |         |         |            |            |        |          |          |                 |          |                 |               |                      |     |     |        | 1FGL J1555.7+1111    |     |       |                          |
|               |         |         |         |         |            |            |        |          |          |                 |          |                 |               |                      |     |     |        | 0FGL J1555.8+1110    |     |       |                          |
| J1557.0–4225  | 239.264 | –42.422 | 335.641 | 8.362   | 0.264      | 0.164      | –81    | 11.5     | 0.7      | 0.2             | 16.5     | 1.8             | 2.68          | ...                  | LP  | ... | 3      | ...                  | ... | ...   | ...                      |
| J1557.4–7040  | 239.374 | –70.678 | 317.206 | –13.159 | 0.073      | 0.064      | –66    | 8.2      | 0.6      | 0.1             | 6.9      | 1.0             | 2.30          | 0.11                 | PL  | ... | ...    | 2FGL J1558.6–7039    | ... | bcu   | PKS 1552–705             |
| J1558.9–6432  | 239.738 | –64.541 | 321.436 | –8.639  | 0.031      | 0.029      | –32    | 17.9     | 1.5      | 0.1             | 17.2     | 1.5             | 2.02          | 0.06                 | PL  | ... | ...    | 1FHL J1558.5–6428    | ... | bll   | PMN J1558–6432           |
|               |         |         |         |         |            |            |        |          |          |                 |          |                 |               |                      |     |     |        | 2FGL J1558.9–6428    |     |       |                          |
| J1558.9+5625  | 239.742 | 56.418  | 87.575  | 45.754  | 0.060      | 0.050      | –39    | 16.1     | 0.9      | 0.1             | 10.6     | 0.9             | 2.21          | 0.08                 | PL  | T   | ...    | 2FGL J1559.0+5627    | ... | bll   | TXS 1557+565             |
|               |         |         |         |         |            |            |        |          |          |                 |          |                 |               |                      |     |     |        | 1FGL J1558.9+5627    |     |       |                          |
| J1559.7+8512  | 239.944 | 85.213  | 118.872 | 30.329  | 0.075      | 0.058      | –74    | 12.8     | 0.6      | 0.1             | 8.0      | 0.8             | 2.35          | 0.08                 | PL  | ... | ...    | 2FGL J1558.3+8513    | ... | bcu   | WN B1609.6+8517          |
| J1559.8–2525  | 239.966 | –25.422 | 347.903 | 20.570  | 0.078      | 0.062      | 1      | 4.4      | 0.3      | 0.1             | 3.3      | 1.0             | 1.94          | 0.24                 | PL  | ... | ...    | ...                  | ... | bcu   | NVSS<br>J160005–252439   |
| J1559.9+2319  | 239.987 | 23.326  | 38.662  | 47.441  | 0.078      | 0.075      | –21    | 7.1      | 0.5      | 0.1             | 5.6      | 1.0             | 2.10          | 0.12                 | PL  | ... | ...    | ...                  | ... | bll   | 87GB<br>155744.0+232525  |
| J1600.3–5810  | 240.076 | –58.169 | 325.763 | –3.932  | 0.086      | 0.072      | –14    | 4.6      | 0.5      | 0.1             | 5.5      | 1.4             | 2.01          | 0.16                 | PL  | ... | ...    | ...                  | ... | bcu   | MRC 1556–580             |
| J1600.8–3053  | 240.212 | –30.891 | 344.093 | 16.458  | 0.059      | 0.052      | 6      | 10.7     | 1.1      | 0.1             | 6.2      | 1.1             | 1.97          | ...                  | EC  | ... | ...    | 2FGL J1600.7–3053    | ... | PSR   | PSR J1600–3053           |
|               |         |         |         |         |            |            |        |          |          |                 |          |                 |               |                      |     |     |        | 1FGL J1600.7–3055    |     |       |                          |
| J1601.9+2306  | 240.489 | 23.111  | 38.538  | 46.939  | 0.111      | 0.090      | 83     | 7.8      | 0.9      | 0.1             | 3.5      | 0.5             | 2.17          | ...                  | LP  | ... | 12     | 2FGL J1602.4+2308    | ... | ...   | ...                      |
| J1602.8–1924  | 240.720 | –19.407 | 353.056 | 24.310  | 0.137      | 0.116      | –70    | 4.8      | 0.5      | 0.1             | 5.8      | 1.3             | 2.31          | 0.14                 | PL  | ... | ...    | ...                  | ... | ...   | ...                      |
| J1603.7–6011  | 240.931 | –60.195 | 324.750 | –5.744  | 0.087      | 0.067      | –12    | 5.1      | 0.5      | 0.1             | 5.6      | 1.2             | 1.96          | 0.13                 | PL  | ... | 1      | ...                  | ... | ...   | ...                      |
| J1603.7+1106  | 240.949 | 11.108  | 23.035  | 42.159  | 0.124      | 0.103      | –18    | 6.2      | 0.5      | 0.1             | 6.1      | 1.2             | 2.32          | 0.13                 | PL  | T   | ...    | ...                  | ... | bll   | MG1 J160340+1106         |
| J1603.9–4903  | 240.979 | –49.064 | 332.162 | 2.569   | 0.014      | 0.014      | 71     | 41.8     | 9.3      | 0.3             | 104.1    | 3.6             | 2.14          | 0.03                 | PL  | T   | ...    | 1FHL J1603.7–4903    | ... | bll   | PMN J1603–4904           |

Table 1—Continued

| Name 3FGL     | R.A.    | Decl.   | $l$     | $b$     | $\theta_1$ | $\theta_2$ | $\phi$ | $\sigma$ | $F_{35}$ | $\Delta F_{35}$ | $S_{25}$ | $\Delta S_{25}$ | $\Gamma_{25}$ | $\Delta \Gamma_{25}$ | Mod | Var | Flags | $\gamma$ -ray Assoc.                                                       | TeV | Class | ID or Assoc.           |
|---------------|---------|---------|---------|---------|------------|------------|--------|----------|----------|-----------------|----------|-----------------|---------------|----------------------|-----|-----|-------|----------------------------------------------------------------------------|-----|-------|------------------------|
|               |         |         |         |         |            |            |        |          |          |                 |          |                 |               |                      |     |     |       | 2FGL J1603.8–4904<br>1FGL J1603.8–4903<br>0FGL J1604.0–4904                |     |       |                        |
| J1604.4–4442  | 241.109 | –44.715 | 335.130 | 5.757   | 0.040      | 0.037      | –2     | 25.5     | 3.6      | 0.2             | 50.5     | 2.4             | 2.45          | 0.04                 | PL  | T   | ...   | 2FGL J1604.5–4442<br>1FGL J1604.7–4443                                     | ... | bcu   | PMN J1604–4441         |
| J1604.6+5714  | 241.170 | 57.241  | 88.268  | 44.729  | 0.043      | 0.042      | –19    | 26.2     | 1.6      | 0.1             | 19.7     | 1.1             | 2.43          | ...                  | LP  | T   | ...   | 2FGL J1604.6+5710<br>1FGL J1604.3+5710                                     | ... | fsrq  | GB6 J1604+5714         |
| J1606.1+5630  | 241.548 | 56.507  | 87.197  | 44.788  | 0.046      | 0.045      | –35    | 6.5      | 0.3      | 0.1             | 3.1      | 0.7             | 1.97          | 0.19                 | PL  | ... | ...   | ...                                                                        | ... | bll   | RBS 1558               |
| J1607.0+1551  | 241.764 | 15.862  | 29.376  | 43.421  | 0.036      | 0.033      | –71    | 27.6     | 2.1      | 0.1             | 24.8     | 1.3             | 2.28          | 0.04                 | PL  | ... | ...   | 2FGL J1607.0+1552<br>1FGL J1607.1+1552<br>3EG J1605+1553<br>EGR J1607+1533 | ... | fsrq  | 4C +15.54              |
| J1607.9–2040  | 241.987 | –20.669 | 352.948 | 22.578  | 0.063      | 0.058      | –52    | 6.7      | 0.6      | 0.1             | 6.6      | 1.3             | 2.01          | 0.13                 | PL  | ... | ...   | ...                                                                        | ... | bcu   | NVSS<br>J160756–203942 |
| J1608.6+1029  | 242.171 | 10.499  | 23.032  | 40.813  | 0.068      | 0.062      | 34     | 19.6     | 1.3      | 0.1             | 22.2     | 1.3             | 2.62          | 0.05                 | PL  | T   | ...   | 2FGL J1608.5+1029<br>1FGL J1609.0+1031<br>3EG J1608+1055<br>EGR J1608+1051 | ... | fsrq  | 4C +10.45<br>OS<br>–   |
| J1610.6–3956  | 242.650 | –39.942 | 339.233 | 8.497   | 0.221      | 0.151      | –35    | 7.4      | 0.8      | 0.1             | 13.3     | 1.8             | 2.61          | 0.10                 | PL  | ... | ...   | 2FGL J1610.6–4002<br>1FGL J1610.8–3955                                     | ... | fsrq  | PMN J1610–3958         |
| J1610.8–6649  | 242.706 | –66.822 | 320.787 | –11.146 | 0.023      | 0.022      | –24    | 26.3     | 2.1      | 0.1             | 26.4     | 2.0             | 1.77          | 0.05                 | PL  | ... | ...   | 1FHL J1610.9–6650<br>2FGL J1610.8–6650<br>1FGL J1610.6–6649                | ... | bll   | PMN J1610–6649         |
| J1611.9+1404  | 242.981 | 14.079  | 27.783  | 41.637  | 0.152      | 0.107      | 13     | 6.8      | 0.5      | 0.1             | 5.8      | 1.0             | 2.21          | 0.12                 | PL  | ... | ...   | 2FGL J1612.0+1403                                                          | ... | ...   | ...                    |
| J1612.4–3100  | 243.102 | –31.015 | 345.853 | 14.646  | 0.082      | 0.065      | 7      | 9.0      | 1.0      | 0.2             | 6.2      | 1.0             | 1.96          | ...                  | LP  | ... | ...   | ...                                                                        | ... | bcu   | NVSS<br>J161219–305937 |
| J1613.4–4222  | 243.366 | –42.374 | 337.936 | 6.364   | 0.115      | 0.103      | 90     | 4.8      | 0.7      | 0.1             | 8.9      | 2.0             | 2.43          | 0.15                 | PL  | ... | 4     | ...                                                                        | ... | ...   | ...                    |
| J1613.8+3410  | 243.455 | 34.182  | 55.110  | 46.348  | 0.071      | 0.054      | –83    | 13.2     | 0.7      | 0.1             | 8.2      | 0.8             | 2.35          | 0.08                 | PL  | ... | ...   | 2FGL J1613.4+3409<br>1FGL J1613.5+3411<br>3EG J1614+3424                   | ... | fsrq  | OS 319                 |
| J1614.5–2231  | 243.630 | –22.522 | 352.610 | 20.198  | 0.032      | 0.032      | 35     | 28.7     | 4.5      | 0.2             | 23.4     | 1.5             | 2.05          | ...                  | EC  | ... | ...   | 1FGL J1614.0–2230<br>2FGL J1614.5–2230<br>3EG J1616–2221                   | ... | PSR   | PSR J1614–2230         |
| J1615.3–5146e | 243.830 | –51.780 | 331.659 | –0.659  | ...        | ...        | ...    | 19.8     | 9.3      | 0.6             | 109.4    | 6.7             | 1.86          | 0.04                 | PL  | ... | 3,10  | 1FGL J1614.7–5138c<br>1FHL J1615.3–5146e<br>2FGL J1615.2–5138              | E   | spp   | ...                    |
| J1615.6–4450  | 243.914 | –44.837 | 336.510 | 4.312   | 0.160      | 0.095      | 8      | 6.9      | 1.0      | 0.2             | 16.5     | 2.5             | 2.56          | 0.11                 | PL  | ... | 1,4,5 | ...                                                                        | ... | ...   | ...                    |

Table 1—Continued

| Name 3FGL     | R.A.    | Decl.   | $l$     | $b$     | $\theta_1$ | $\theta_2$ | $\phi$ | $\sigma$ | $F_{35}$ | $\Delta F_{35}$ | $S_{25}$ | $\Delta S_{25}$ | $\Gamma_{25}$ | $\Delta \Gamma_{25}$ | Mod | Var | Flags   | $\gamma$ -ray Assoc.                                                               | TeV | Class | ID or Assoc.     |
|---------------|---------|---------|---------|---------|------------|------------|--------|----------|----------|-----------------|----------|-----------------|---------------|----------------------|-----|-----|---------|------------------------------------------------------------------------------------|-----|-------|------------------|
| J1615.8+4712  | 243.954 | 47.210  | 73.874  | 45.587  | 0.090      | 0.073      | 6      | 6.3      | 0.3      | 0.1             | 3.6      | 0.7             | 2.02          | 0.17                 | PL  | ... | ...     | 2FGL J1614.8+4703                                                                  | ... | fsrq  | TXS 1614+473     |
| J1616.2–5054e | 244.060 | –50.910 | 332.366 | –0.131  | ...        | ...        | ...    | 21.0     | 13.9     | 0.7             | 156.1    | 8.4             | 2.14          | 0.03                 | PL  | T   | ...     | 0FGL J1615.6–5049<br>1FGL J1617.5–5105c<br>1FHL J1616.2–5054e<br>2FGL J1615.0–5051 | E   | PWN   | HESS J1616–508   |
| J1616.4+4631  | 244.119 | 46.518  | 72.871  | 45.570  | 0.217      | 0.155      | –12    | 4.7      | 0.2      | 0.1             | 4.0      | 0.8             | 2.59          | 0.17                 | PL  | ... | ...     | 1FGL J1616.1+4637                                                                  | ... | fsrq  | MG4 J161600+4632 |
| J1616.8–5343  | 244.205 | –53.724 | 330.475 | –2.218  | 0.089      | 0.065      | –79    | 10.6     | 1.7      | 0.2             | 26.5     | 2.6             | 2.53          | 0.07                 | PL  | ... | 3,10    | 2FGL J1617.3–5336                                                                  | ... | ...   | ...              |
| J1616.8+4111  | 244.213 | 41.192  | 65.254  | 45.935  | 0.128      | 0.105      | –86    | 4.9      | 0.2      | 0.1             | 2.9      | 0.6             | 2.33          | 0.17                 | PL  | ... | ...     | ...                                                                                | ... | bll   | B3 1615+412      |
| J1616.8+5846  | 244.216 | 58.783  | 89.516  | 42.688  | 0.328      | 0.234      | –62    | 5.9      | 0.1      | 0.0             | 4.2      | 0.7             | 3.12          | 0.21                 | PL  | ... | 1       | ...                                                                                | ... | ...   | ...              |
| J1616.8–2300  | 244.219 | –23.011 | 352.620 | 19.467  | 0.107      | 0.093      | –25    | 5.1      | 0.6      | 0.1             | 6.7      | 1.5             | 2.14          | 0.14                 | PL  | ... | ...     | 2FGL J1616.8–2302                                                                  | ... | glc   | M80              |
| J1617.3–2519  | 244.348 | –25.331 | 350.905 | 17.806  | 0.373      | 0.215      | –14    | 6.5      | 0.7      | 0.1             | 11.9     | 1.8             | 2.59          | 0.10                 | PL  | ... | ...     | 2FGL J1617.6–2526c<br>EGR J1617–2610                                               | ... | bcu   | PMN J1617–2537   |
| J1617.4–5846  | 244.368 | –58.767 | 327.011 | –5.894  | 0.083      | 0.065      | –25    | 15.8     | 1.4      | 0.1             | 24.3     | 1.7             | 2.61          | 0.06                 | PL  | T   | ...     | 1FGL J1617.7–5843                                                                  | ... | fsrq  | MRC 1613–586     |
| J1617.7–7717  | 244.447 | –77.299 | 313.422 | –18.859 | 0.066      | 0.055      | 49     | 18.3     | 1.4      | 0.1             | 19.4     | 1.3             | 2.53          | ...                  | LP  | T   | ...     | 2FGL J1618.2–7718<br>1FGL J1617.9–7716                                             | ... | fsrq  | PKS 1610–77      |
| J1617.8+5137  | 244.452 | 51.620  | 79.935  | 44.486  | 0.165      | 0.121      | –52    | 9.7      | 0.3      | 0.1             | 6.3      | 0.7             | 2.70          | 0.10                 | PL  | T   | ...     | ...                                                                                | ... | fsrq  | TXS 1617+517     |
| J1618.8+5520  | 244.704 | 55.346  | 84.913  | 43.451  | 0.193      | 0.145      | –0     | 4.2      | 0.2      | 0.1             | 2.5      | 0.6             | 2.33          | 0.17                 | PL  | ... | ...     | ...                                                                                | ... | ...   | ...              |
| J1619.0–5014c | 244.773 | –50.244 | 333.155 | 0.031   | 0.098      | 0.085      | –65    | 6.1      | 3.1      | 0.5             | 42.5     | 7.2             | 2.43          | 0.08                 | PL  | ... | 1,4,5,6 | ...                                                                                | ... | ...   | ...              |
| J1619.1+7538  | 244.799 | 75.641  | 109.091 | 35.296  | 0.044      | 0.040      | –75    | 6.7      | 0.2      | 0.0             | 2.2      | 0.6             | 1.71          | 0.21                 | PL  | ... | ...     | 1FHL J1619.8+7540                                                                  | ... | ...   | ...              |
| J1620.0–5101  | 245.009 | –51.028 | 332.711 | –0.633  | 0.045      | 0.044      | –62    | 8.2      | 3.5      | 0.5             | 41.5     | 6.3             | 2.26          | 0.07                 | PL  | ... | 3,4,5   | ...                                                                                | ... | ...   | ...              |
| J1620.8–5149  | 245.203 | –51.830 | 332.232 | –1.287  | 0.075      | 0.060      | –59    | 5.0      | 1.2      | 0.3             | 13.2     | 3.3             | 2.09          | 0.14                 | PL  | ... | ...     | ...                                                                                | ... | ...   | ...              |
| J1620.8–4928  | 245.204 | –49.471 | 333.896 | 0.386   | 0.014      | 0.014      | –46    | 47.1     | 25.0     | 0.7             | 180.4    | 6.8             | 2.18          | ...                  | EC  | ... | ...     | 1FHL J1620.7–4928<br>2FGL J1620.8–4928<br>1FGL J1620.8–4928c<br>1AGL J1624–4946    | ... | PSR   | PSR J1620–4927   |
| J1621.1–2331  | 245.279 | –23.523 | 352.911 | 18.402  | 0.212      | 0.183      | 71     | 7.6      | 0.5      | 0.1             | 11.8     | 1.6             | 2.45          | ...                  | LP  | ... | 12      | 2FGL J1620.5–2320c                                                                 | ... | agn   | PKS 1617–235     |
| J1622.9–5004  | 245.726 | –50.075 | 333.707 | –0.280  | 0.024      | 0.023      | 43     | 20.7     | 10.6     | 0.7             | 66.6     | 5.4             | 2.14          | ...                  | LP  | ... | ...     | 2FGL J1622.8–5006<br>1AGL J1624–4946                                               | ... | ...   | ...              |
| J1622.9–0312  | 245.741 | –3.204  | 10.758  | 30.714  | 0.090      | 0.072      | –9     | 9.5      | 0.9      | 0.1             | 10.2     | 1.3             | 2.23          | 0.09                 | PL  | ... | ...     | 2FGL J1622.8–0314                                                                  | ... | psr   | PSR J1622–03     |
| J1624.1–4700  | 246.042 | –47.006 | 336.037 | 1.729   | 0.090      | 0.081      | 20     | 13.9     | 1.1      | 0.2             | 39.1     | 3.1             | 2.67          | ...                  | LP  | ... | 12      | ...                                                                                | ... | ...   | ...              |
| J1624.2–4041  | 246.059 | –40.687 | 340.572 | 6.142   | 0.045      | 0.042      | 31     | 19.3     | 4.2      | 0.3             | 25.3     | 2.4             | 2.27          | ...                  | LP  | ... | ...     | 2FGL J1624.1–4040<br>1FGL J1624.0–4041                                             | ... | ...   | ...              |
| J1624.2–3957  | 246.066 | –39.957 | 341.102 | 6.647   | 0.133      | 0.118      | –72    | 5.1      | 0.9      | 0.2             | 13.1     | 2.5             | 2.52          | 0.13                 | PL  | ... | 5       | ...                                                                                | ... | ...   | ...              |
| J1624.8–4233  | 246.200 | –42.566 | 339.293 | 4.755   | 0.153      | 0.100      | 13     | 6.8      | 0.9      | 0.2             | 17.1     | 2.7             | 2.65          | 0.11                 | PL  | ... | 1,4     | ...                                                                                | ... | ...   | ...              |
| J1625.0+5651  | 246.252 | 56.864  | 86.598  | 42.217  | 0.132      | 0.114      | –24    | 4.9      | 0.2      | 0.1             | 2.8      | 0.6             | 2.39          | 0.16                 | PL  | ... | ...     | ...                                                                                | ... | bll   | SBS 1623+569     |

Table 1—Continued

| Name 3FGL     | R.A.    | Decl.   | $l$     | $b$     | $\theta_1$ | $\theta_2$ | $\phi$ | $\sigma$ | $F_{35}$ | $\Delta F_{35}$ | $S_{25}$ | $\Delta S_{25}$ | $\Gamma_{25}$ | $\Delta \Gamma_{25}$ | Mod | Var | Flags | $\gamma$ -ray Assoc.                                                                               | TeV | Class | ID or Assoc.        |
|---------------|---------|---------|---------|---------|------------|------------|--------|----------|----------|-----------------|----------|-----------------|---------------|----------------------|-----|-----|-------|----------------------------------------------------------------------------------------------------|-----|-------|---------------------|
| J1625.1–0021  | 246.279 | −0.359  | 13.881  | 31.838  | 0.038      | 0.037      | 61     | 28.5     | 3.6      | 0.2             | 18.4     | 1.3             | 2.05          | ...                  | LP  | ... | ...   | 2FGL J1625.2–0020<br>1FGL J1625.3–0019                                                             | ... | ...   | ...                 |
| J1625.2–2845  | 246.308 | −28.754 | 349.523 | 14.201  | 0.122      | 0.086      | 61     | 4.7      | 0.6      | 0.1             | 8.4      | 2.0             | 2.52          | 0.17                 | PL  | ... | ...   | ...                                                                                                | ... | ...   | ...                 |
| J1625.6–2058  | 246.422 | −20.979 | 355.668 | 19.288  | 0.103      | 0.094      | −6     | 6.5      | 0.7      | 0.1             | 10.6     | 1.6             | 2.54          | 0.11                 | PL  | ... | ...   | 1FGL J1626.2–2038                                                                                  | ... | ...   | ...                 |
| J1625.7–2527  | 246.445 | −25.456 | 352.145 | 16.322  | 0.020      | 0.019      | 71     | 56.3     | 11.2     | 0.3             | 108.7    | 3.2             | 2.31          | ...                  | LP  | T   | ...   | 1FHL J1625.7–2531<br>2FGL J1625.7–2526<br>1FGL J1625.7–2524<br>0FGL J1625.8–2527<br>3EG J1626–2519 | ... | fsrq  | PKS 1622–253        |
| J1625.9+4125  | 246.500 | 41.423  | 65.527  | 44.213  | 0.175      | 0.124      | 12     | 8.1      | 0.3      | 0.1             | 6.0      | 0.8             | 2.70          | 0.12                 | PL  | ... | ...   | ...                                                                                                | ... | fsrq  | B3 1624+414         |
| J1626.0–2951  | 246.518 | −29.862 | 348.809 | 13.317  | 0.053      | 0.051      | 75     | 20.9     | 2.5      | 0.2             | 29.5     | 2.2             | 2.45          | ...                  | LP  | T   | ...   | 2FGL J1626.1–2948<br>1FGL J1626.2–2956<br>3EG J1625–2955<br>EGR J1625–2958                         | ... | FSRQ  | PKS 1622–29         |
| J1626.1+3512  | 246.546 | 35.215  | 56.895  | 43.911  | 0.078      | 0.073      | 36     | 4.8      | 0.2      | 0.1             | 2.2      | 0.7             | 1.70          | 0.23                 | PL  | ... | ...   | ...                                                                                                | ... | bll   | RGB J1626+352       |
| J1626.2–4911  | 246.569 | −49.197 | 334.715 | −0.054  | 0.081      | 0.065      | 87     | 5.4      | 2.1      | 0.5             | 23.2     | 6.0             | 2.11          | 0.14                 | PL  | ... | ...   | 1FGL J1626.0–4917c<br>1AGL J1624–4946                                                              | E   | ...   | ...                 |
| J1626.2–2428c | 246.572 | −24.467 | 352.996 | 16.892  | 0.057      | 0.051      | −90    | 9.4      | 2.2      | 0.3             | 26.7     | 3.6             | 2.28          | 0.07                 | PL  | ... | 6     | 1FGL J1625.8–2429c<br>0FGL J1625.9–2423<br>3EG J1627–2419                                          | ... | ...   | ...                 |
| J1626.3–4406  | 246.579 | −44.112 | 338.373 | 3.481   | 0.133      | 0.129      | 90     | 7.7      | 0.6      | 0.1             | 19.1     | 3.3             | 2.60          | ...                  | LP  | ... | 10,12 | 2FGL J1626.4–4408                                                                                  | ... | ...   | ...                 |
| J1626.4–7640  | 246.611 | −76.670 | 314.260 | −18.806 | 0.046      | 0.043      | −32    | 8.5      | 0.5      | 0.1             | 5.9      | 1.1             | 1.99          | 0.14                 | PL  | ... | ...   | 2FGL J1626.0–7636                                                                                  | ... | bcu   | PKS 1619–765        |
| J1627.8+3217  | 246.968 | 32.299  | 52.958  | 43.210  | 0.072      | 0.070      | 71     | 10.2     | 0.6      | 0.1             | 6.4      | 0.8             | 2.14          | 0.09                 | PL  | ... | 3     | 2FGL J1627.8+3219<br>1FGL J1627.6+3218                                                             | ... | ...   | ...                 |
| J1628.0–3203  | 247.016 | −32.061 | 347.447 | 11.515  | 0.090      | 0.083      | 20     | 11.9     | 1.6      | 0.2             | 12.1     | 1.5             | 2.34          | ...                  | LP  | ... | ...   | 2FGL J1628.3–3206<br>1FGL J1627.8–3204                                                             | ... | psr   | PSR J1628–3205      |
| J1628.1–3344  | 247.027 | −33.742 | 346.196 | 10.368  | 0.063      | 0.052      | 69     | 5.6      | 0.6      | 0.1             | 6.3      | 1.5             | 2.12          | 0.17                 | PL  | ... | 1     | ...                                                                                                | ... | ...   | ...                 |
| J1628.1–5740  | 247.034 | −57.675 | 328.784 | −6.129  | 0.145      | 0.099      | 47     | 4.5      | 0.5      | 0.1             | 6.9      | 1.6             | 2.46          | 0.15                 | PL  | ... | 4     | ...                                                                                                | ... | ...   | ...                 |
| J1628.1+0254  | 247.042 | 2.909   | 17.647  | 32.908  | 0.125      | 0.109      | 42     | 4.2      | 0.3      | 0.1             | 3.8      | 0.9             | 2.12          | 0.16                 | PL  | ... | ...   | 1FGL J1627.9+0254                                                                                  | ... | ...   | ...                 |
| J1628.2–2431c | 247.069 | −24.528 | 353.260 | 16.512  | 0.100      | 0.091      | −22    | 7.9      | 1.8      | 0.3             | 23.6     | 3.5             | 2.37          | 0.08                 | PL  | ... | 5,6   | 3EG J1627–2419                                                                                     | ... | ...   | ...                 |
| J1628.2+7703  | 247.070 | 77.051  | 110.248 | 34.126  | 0.164      | 0.134      | 42     | 4.9      | 0.2      | 0.1             | 3.0      | 0.6             | 2.45          | 0.17                 | PL  | ... | ...   | ...                                                                                                | ... | bcu   | 6C B163030.4+771303 |
| J1628.4–4546  | 247.116 | −45.778 | 337.435 | 2.052   | 0.263      | 0.193      | −65    | 7.3      | 1.5      | 0.2             | 25.9     | 3.5             | 2.63          | 0.08                 | PL  | ... | 4     | ...                                                                                                | ... | ...   | ...                 |
| J1628.7–8056  | 247.176 | −80.934 | 310.846 | −21.622 | 0.431      | 0.268      | −67    | 5.1      | 0.3      | 0.1             | 5.8      | 1.1             | 2.75          | 0.15                 | PL  | ... | ...   | ...                                                                                                | ... | ...   | ...                 |
| J1628.9–4852  | 247.238 | −48.874 | 335.252 | −0.146  | 0.097      | 0.075      | 23     | 8.5      | 4.8      | 0.6             | 32.8     | 5.4             | 2.23          | ...                  | LP  | ... | 4     | 2FGL J1628.1–4857c                                                                                 | ... | spp   | ...                 |
| J1630.2+3733  | 247.553 | 37.562  | 60.216  | 43.291  | 0.066      | 0.058      | 69     | 15.2     | 1.3      | 0.1             | 6.9      | 1.0             | 2.26          | ...                  | EC  | ... | ...   | 2FGL J1630.3+3732                                                                                  | ... | PSR   | PSR J1630+3734      |

Table 1—Continued

| Name 3FGL     | R.A.    | Decl.   | $l$     | $b$    | $\theta_1$ | $\theta_2$ | $\phi$ | $\sigma$ | $F_{35}$ | $\Delta F_{35}$ | $S_{25}$ | $\Delta S_{25}$ | $\Gamma_{25}$ | $\Delta \Gamma_{25}$ | Mod | Var | Flags        | $\gamma$ -ray Assoc.                                                                               | TeV | Class | ID or Assoc.             |
|---------------|---------|---------|---------|--------|------------|------------|--------|----------|----------|-----------------|----------|-----------------|---------------|----------------------|-----|-----|--------------|----------------------------------------------------------------------------------------------------|-----|-------|--------------------------|
| J1630.2−1052  | 247.554 | −10.867 | 4.907   | 24.782 | 0.236      | 0.178      | −22    | 4.9      | 0.6      | 0.1             | 6.7      | 1.3             | 2.30          | 0.12                 | PL  | ... | ...          | 1FGL J1630.5+3735<br>2FGL J1631.0−1050<br>1FGL J1630.3−1042<br>3EG J1631−1018                      | ... | ...   | ...                      |
| J1630.3−6126  | 247.584 | −61.436 | 326.205 | −8.901 | 0.189      | 0.144      | 39     | 10.8     | 0.6      | 0.1             | 13.9     | 1.3             | 2.79          | 0.09                 | PL  | T   | ...          | ...                                                                                                | ... | ...   | ...                      |
| J1630.3−4346  | 247.594 | −43.767 | 339.128 | 3.191  | 0.125      | 0.086      | 45     | 4.5      | 0.7      | 0.4             | 8.1      | 4.9             | 2.13          | 0.48                 | PL  | ... | 4            | ...                                                                                                | ... | ...   | ...                      |
| J1630.6+8232  | 247.652 | 82.535  | 115.799 | 31.251 | 0.058      | 0.047      | 58     | 21.0     | 1.3      | 0.1             | 11.0     | 0.9             | 2.22          | ...                  | LP  | ... | ...          | 1FGL J1635.4+8228<br>2FGL J1629.4+8236<br>3EG J1621+8203                                           | ... | rdg   | NGC 6251                 |
| J1630.7+5222  | 247.681 | 52.367  | 80.419  | 42.391 | 0.038      | 0.035      | 57     | 17.9     | 1.0      | 0.1             | 10.8     | 1.1             | 1.97          | 0.06                 | PL  | T   | ...          | 1FHL J1631.0+5224<br>2FGL J1630.4+5218<br>1FGL J1630.2+5220                                        | ... | bll   | TXS 1629+524             |
| J1630.8+1047  | 247.712 | 10.797  | 26.459  | 36.064 | 0.244      | 0.221      | 36     | 6.8      | 0.3      | 0.1             | 7.6      | 1.1             | 2.80          | 0.13                 | PL  | ... | ...          | ...                                                                                                | ... | bcu   | MG1 J163119+1051         |
| J1632.4−4820  | 248.111 | −48.337 | 336.039 | −0.197 | 0.073      | 0.062      | 79     | 9.1      | 5.5      | 0.6             | 36.0     | 5.6             | 2.20          | ...                  | LP  | ... | 3            | 2FGL J1632.4−4820c                                                                                 | ... | psr   | PSR J1632−4818           |
| J1632.8+3838  | 248.202 | 38.648  | 61.741  | 42.847 | 0.092      | 0.079      | −20    | 4.8      | 0.4      | 0.1             | 5.8      | 1.8             | 2.45          | 0.20                 | PL  | ... | ...          | ...                                                                                                | ... | ...   | ...                      |
| J1633.0−4746e | 248.250 | −47.770 | 336.517 | 0.121  | ...        | ...        | ...    | 32.0     | 22.6     | 0.8             | 252.3    | 9.5             | 2.11          | 0.02                 | PL  | T   | 10           | 1FGL J1632.7−4733c<br>1FHL J1633.0−4746e<br>2FGL J1632.4−4753c                                     | E   | PWN   | HESS J1632−478           |
| J1635.2+3809  | 248.812 | 38.153  | 61.110  | 42.340 | 0.016      | 0.015      | 29     | 87.0     | 11.4     | 0.3             | 140.0    | 2.8             | 2.40          | ...                  | LP  | T   | ...          | 1FHL J1635.0+3808<br>2FGL J1635.2+3810<br>1FGL J1635.0+3808<br>0FGL J1635.2+3809<br>3EG J1635+3813 | ... | FSRQ  | 4C +38.41                |
| J1635.3+4257  | 248.850 | 42.965  | 67.626  | 42.458 | 0.235      | 0.138      | −4     | 5.8      | 0.3      | 0.1             | 3.8      | 0.7             | 2.42          | 0.16                 | PL  | ... | ...          | ...                                                                                                | ... | ...   | ...                      |
| J1636.2−4709c | 249.058 | −47.160 | 337.337 | 0.132  | 0.173      | 0.105      | −47    | 10.4     | 6.0      | 0.6             | 68.7     | 8.2             | 2.21          | 0.06                 | PL  | ... | 3,5,6,7,9,10 | 2FGL J1635.4−4717c<br>1FGL J1635.7−4715c<br>3EG J1639−4702<br>1AGL J1639−4702                      | ... | spp   | ...                      |
| J1636.2−4734  | 249.069 | −47.580 | 337.030 | −0.156 | 0.051      | 0.033      | 36     | 22.2     | 15.8     | 0.8             | 114.2    | 7.9             | 2.21          | ...                  | LP  | ... | 7            | 1FGL J1636.4−4737c                                                                                 | ... | snr   | SNR G337.0−00.1          |
| J1636.7+2624  | 249.187 | 26.416  | 45.746  | 40.149 | 0.081      | 0.072      | −31    | 6.3      | 0.3      | 0.1             | 3.9      | 0.8             | 2.04          | 0.16                 | PL  | ... | ...          | ...                                                                                                | ... | bcu   | NVSS<br>J163651+262657   |
| J1637.1+1314  | 249.284 | 13.245  | 29.999  | 35.702 | 0.115      | 0.090      | 8      | 4.9      | 0.3      | 0.1             | 3.9      | 1.0             | 2.22          | 0.24                 | PL  | ... | ...          | ...                                                                                                | ... | bll   | 1RXS<br>J163717.1+131418 |
| J1637.6−3449  | 249.415 | −34.822 | 346.724 | 8.180  | 0.044      | 0.040      | −79    | 9.5      | 0.8      | 0.1             | 10.1     | 1.6             | 1.73          | 0.11                 | PL  | ... | ...          | 1FHL J1637.9−3450                                                                                  | ... | bcu   | NVSS<br>J163750−344915   |
| J1637.7+4715  | 249.431 | 47.264  | 73.403  | 41.885 | 0.042      | 0.041      | −64    | 32.0     | 1.8      | 0.1             | 22.6     | 1.0             | 2.37          | 0.04                 | PL  | T   | ...          | 2FGL J1637.9−3451<br>2FGL J1637.7+4714<br>1FGL J1637.9+4707                                        | ... | fsrq  | 4C +47.44                |



Table 1—Continued

| Name 3FGL     | R.A.    | Decl.   | $l$     | $b$    | $\theta_1$ | $\theta_2$ | $\phi$ | $\sigma$ | $F_{35}$ | $\Delta F_{35}$ | $S_{25}$ | $\Delta S_{25}$ | $\Gamma_{25}$ | $\Delta \Gamma_{25}$ | Mod | Var | Flags | $\gamma$ -ray Assoc.                                                                              | TeV | Class | ID or Assoc.            |
|---------------|---------|---------|---------|--------|------------|------------|--------|----------|----------|-----------------|----------|-----------------|---------------|----------------------|-----|-----|-------|---------------------------------------------------------------------------------------------------|-----|-------|-------------------------|
| J1637.8+7325  | 249.468 | 73.419  | 105.974 | 35.226 | 0.072      | 0.063      | −3     | 5.3      | 0.2      | 0.1             | 2.1      | 0.5             | 1.91          | 0.23                 | PL  | ... | ...   | ...                                                                                               | ... | bl    | RX J1637.9+7326         |
| J1637.9+5719  | 249.493 | 57.327  | 86.632  | 40.397 | 0.136      | 0.115      | 11     | 9.5      | 0.3      | 0.1             | 6.5      | 0.7             | 2.81          | 0.11                 | PL  | T   | ...   | ...                                                                                               | ... | fsrq  | OS 562                  |
| J1638.6−4654  | 249.650 | −46.902 | 337.798 | 0.005  | 0.070      | 0.061      | −40    | 13.4     | 9.5      | 0.7             | 73.0     | 7.3             | 2.30          | ...                  | LP  | T   | ...   | 3EG J1639−4702<br>1AGL J1639−4702                                                                 | ... | spp   | ...                     |
| J1639.4−5146  | 249.870 | −51.779 | 334.253 | −3.349 | 0.031      | 0.030      | −73    | 20.1     | 3.2      | 0.2             | 40.8     | 2.6             | 2.35          | 0.05                 | PL  | ... | ...   | 2FGL J1639.8−5145<br>3EG J1638−5155<br>EGR J1638−5157                                             | ... | ...   | ...                     |
| J1639.8+4125  | 249.970 | 41.428  | 65.570  | 41.611 | 0.153      | 0.137      | −54    | 5.8      | 0.3      | 0.1             | 4.5      | 0.9             | 2.54          | 0.15                 | PL  | ... | ...   | ...                                                                                               | ... | fsrq  | MG4 J163918+4127        |
| J1640.4−4634c | 250.118 | −46.580 | 338.252 | −0.020 | 0.030      | 0.027      | 78     | 10.4     | 3.2      | 0.7             | 37.6     | 6.1             | 1.86          | 0.11                 | PL  | ... | 6     | 1FHL J1640.5−4634<br>2FGL J1640.5−4633<br>1FGL J1640.8−4634c<br>3EG J1639−4702<br>1AGL J1639−4702 | E   | spp   | ...                     |
| J1640.6−4917  | 250.156 | −49.289 | 336.240 | −1.834 | 0.099      | 0.075      | −51    | 8.8      | 2.2      | 0.3             | 26.6     | 3.5             | 2.31          | 0.08                 | PL  | T   | ...   | 2FGL J1639.8−4921c                                                                                | ... | ...   | ...                     |
| J1640.6+3945  | 250.159 | 39.755  | 63.346  | 41.395 | 0.032      | 0.030      | −66    | 28.3     | 3.9      | 0.2             | 35.6     | 2.9             | 2.33          | ...                  | LP  | T   | ...   | 1FHL J1640.7+3943<br>2FGL J1640.7+3945<br>EGR J1642+3940                                          | ... | FSRQ  | NRAO 512                |
| J1640.9+1142  | 250.247 | 11.707  | 28.768  | 34.208 | 0.081      | 0.074      | −0     | 5.7      | 0.4      | 0.1             | 4.7      | 1.0             | 2.30          | 0.17                 | PL  | ... | ...   | 2FGL J1641.0+1141<br>1FGL J1641.0+1143                                                            | ... | bcu   | TXS 1638+118            |
| J1641.1−4619c | 250.283 | −46.330 | 338.515 | 0.060  | 0.049      | 0.039      | −3     | 7.9      | 4.5      | 0.5             | 57.9     | 7.6             | 2.38          | 0.06                 | PL  | ... | 3,6   | ...                                                                                               | P   | spp   | ...                     |
| J1641.5−5319  | 250.378 | −53.324 | 333.296 | −4.602 | 0.084      | 0.074      | 37     | 13.2     | 1.9      | 0.2             | 18.4     | 2.2             | 2.52          | ...                  | LP  | ... | ...   | 2FGL J1641.8−5319                                                                                 | ... | ...   | ...                     |
| J1641.5−2856  | 250.392 | −28.948 | 351.792 | 11.383 | 0.168      | 0.110      | −68    | 5.0      | 0.6      | 0.1             | 7.5      | 1.5             | 2.33          | 0.12                 | PL  | ... | 1     | ...                                                                                               | ... | ...   | ...                     |
| J1641.8−0619  | 250.452 | −6.324  | 10.821  | 25.077 | 0.061      | 0.054      | −50    | 10.7     | 1.4      | 0.2             | 16.9     | 2.1             | 2.32          | 0.08                 | PL  | ... | ...   | 2FGL J1641.6−0614                                                                                 | ... | bl    | TXS 1639−062            |
| J1642.4+8045  | 250.612 | 80.764  | 113.746 | 31.755 | 0.188      | 0.135      | 28     | 6.1      | 0.3      | 0.1             | 4.0      | 0.7             | 2.49          | 0.13                 | PL  | ... | ...   | ...                                                                                               | ... | ...   | ...                     |
| J1642.9+3950  | 250.748 | 39.849  | 63.506  | 40.949 | 0.041      | 0.039      | −29    | 20.5     | 2.5      | 0.2             | 34.8     | 2.4             | 2.45          | 0.05                 | PL  | T   | ...   | 2FGL J1642.9+3949<br>EGR J1642+3940                                                               | ... | FSRQ  | 3C 345                  |
| J1643.6−5002  | 250.914 | −50.039 | 335.998 | −2.698 | 0.133      | 0.095      | −45    | 8.0      | 1.4      | 0.3             | 17.0     | 2.6             | 2.43          | ...                  | LP  | ... | 1     | ...                                                                                               | ... | ...   | ...                     |
| J1643.6−0642  | 250.921 | −6.706  | 10.759  | 24.478 | 0.060      | 0.047      | 31     | 7.2      | 0.7      | 0.2             | 8.2      | 1.8             | 2.07          | 0.17                 | PL  | ... | ...   | 2FGL J1643.5−0641<br>1FGL J1643.5−0646                                                            | ... | bcu   | NVSS<br>J164328−064619  |
| J1644.4+2632  | 251.123 | 26.542  | 46.465  | 38.503 | 0.201      | 0.163      | −28    | 4.5      | 0.2      | 0.1             | 4.3      | 0.9             | 2.75          | 0.22                 | PL  | ... | ...   | ...                                                                                               | ... | ...   | ...                     |
| J1644.6−0911  | 251.174 | −9.186  | 8.676   | 22.873 | 0.079      | 0.073      | 21     | 4.9      | 0.5      | 0.1             | 7.4      | 1.5             | 2.57          | 0.14                 | PL  | ... | ...   | ...                                                                                               | ... | ...   | ...                     |
| J1645.2−5747  | 251.323 | −57.790 | 330.234 | −7.914 | 0.115      | 0.103      | −19    | 4.5      | 0.4      | 0.1             | 7.7      | 1.7             | 2.67          | 0.16                 | PL  | ... | 4,5   | ...                                                                                               | ... | bcu   | AT20G<br>J164513−575122 |
| J1645.7−2149  | 251.448 | −21.824 | 358.092 | 15.134 | 0.123      | 0.083      | 60     | 8.8      | 1.5      | 0.2             | 8.3      | 1.2             | 2.20          | ...                  | LP  | ... | 1,3   | 2FGL J1645.7−2148c<br>1FGL J1645.0−2155c                                                          | ... | ...   | ...                     |
| J1645.9−5420  | 251.484 | −54.349 | 332.942 | −5.765 | 0.345      | 0.230      | −80    | 5.0      | 0.5      | 0.1             | 10.8     | 2.1             | 2.71          | 0.13                 | PL  | ... | 5     | ...                                                                                               | ... | spp   | ...                     |

Table 1—Continued

| Name 3FGL     | R.A.    | Decl.   | $l$     | $b$     | $\theta_1$ | $\theta_2$ | $\phi$ | $\sigma$ | $F_{35}$ | $\Delta F_{35}$ | $S_{25}$ | $\Delta S_{25}$ | $\Gamma_{25}$ | $\Delta \Gamma_{25}$ | Mod | Var | Flags | $\gamma$ -ray Assoc.                                                          | TeV | Class | ID or Assoc.            |
|---------------|---------|---------|---------|---------|------------|------------|--------|----------|----------|-----------------|----------|-----------------|---------------|----------------------|-----|-----|-------|-------------------------------------------------------------------------------|-----|-------|-------------------------|
| J1645.9+6336  | 251.498 | 63.611  | 94.182  | 37.904  | 0.137      | 0.107      | −3     | 9.9      | 0.3      | 0.1             | 6.1      | 0.7             | 2.69          | 0.11                 | PL  | T   | ...   | ...                                                                           | ... | fsrq  | TXS 1645+635            |
| J1646.9−1332  | 251.748 | −13.548 | 5.202   | 19.892  | 0.101      | 0.077      | −22    | 4.9      | 0.4      | 0.1             | 5.2      | 1.4             | 1.85          | 0.19                 | PL  | ... | ...   | 2FGL J1646.7−1333                                                             | ... | ...   | ...                     |
| J1647.1−6438  | 251.781 | −64.645 | 324.992 | −12.434 | 0.063      | 0.054      | 40     | 7.9      | 0.6      | 0.1             | 6.7      | 1.0             | 2.19          | 0.11                 | PL  | ... | ...   | ...                                                                           | ... | bcu   | PMN J1647−6437          |
| J1647.4+4950  | 251.873 | 49.837  | 76.651  | 40.090  | 0.042      | 0.041      | −8     | 29.3     | 1.5      | 0.1             | 20.0     | 0.9             | 2.43          | 0.04                 | PL  | T   | ...   | 2FGL J1647.5+4950<br>1FGL J1647.4+4948                                        | ... | bcu   | SBS 1646+499            |
| J1648.0+4230  | 252.018 | 42.510  | 67.066  | 40.125  | 0.293      | 0.207      | −34    | 4.7      | 0.2      | 0.1             | 3.4      | 0.7             | 2.48          | 0.17                 | PL  | ... | ...   | ...                                                                           | ... | ...   | ...                     |
| J1648.3−4611  | 252.096 | −46.196 | 339.434 | −0.802  | 0.038      | 0.033      | −60    | 13.9     | 6.5      | 0.7             | 38.2     | 5.5             | 2.18          | ...                  | EC  | ... | 3     | 2FGL J1648.4−4612<br>1FGL J1648.4−4609c<br>0FGL J1648.1−4606                  | E   | PSR   | PSR J1648−4611          |
| J1648.5−4829  | 252.150 | −48.494 | 337.699 | −2.309  | 0.167      | 0.115      | 43     | 6.0      | 1.3      | 0.2             | 18.2     | 3.3             | 2.44          | 0.11                 | PL  | ... | 4,10  | ...                                                                           | ... | bcu   | PMN J1648−4826          |
| J1648.6−5635  | 252.166 | −56.584 | 331.464 | −7.494  | 0.190      | 0.148      | −7     | 5.5      | 0.5      | 0.1             | 10.7     | 1.9             | 2.80          | 0.13                 | PL  | ... | 1     | ...                                                                           | ... | ...   | ...                     |
| J1649.4+5238  | 252.367 | 52.634  | 80.242  | 39.530  | 0.058      | 0.055      | −78    | 13.0     | 0.7      | 0.1             | 7.8      | 0.8             | 2.22          | 0.07                 | PL  | T   | ...   | 2FGL J1649.6+5238                                                             | ... | bll   | 87GB<br>164812.2+524023 |
| J1649.6−3007  | 252.420 | −30.129 | 352.006 | 9.270   | 0.121      | 0.096      | 45     | 8.7      | 1.1      | 0.2             | 13.3     | 1.6             | 2.31          | 0.09                 | PL  | ... | ...   | 1FGL J1649.6+5241<br>2FGL J1649.2−3004                                        | ... | ...   | ...                     |
| J1650.0−4438c | 252.507 | −44.639 | 340.813 | −0.022  | 0.135      | 0.080      | 71     | 11.5     | 3.8      | 0.5             | 75.0     | 4.9             | 2.71          | 0.06                 | PL  | ... | 3,6   | ...                                                                           | ... | ...   | ...                     |
| J1650.0+0356  | 252.514 | 3.949   | 21.856  | 28.683  | 0.283      | 0.199      | −32    | 4.7      | 0.4      | 0.1             | 4.3      | 1.0             | 2.17          | 0.19                 | PL  | T   | ...   | ...                                                                           | ... | ...   | ...                     |
| J1650.2−5044  | 252.564 | −50.749 | 336.136 | −3.959  | 0.023      | 0.023      | −65    | 26.3     | 4.4      | 0.2             | 53.0     | 2.6             | 2.30          | 0.04                 | PL  | T   | ...   | 1FHL J1650.1−5045<br>2FGL J1650.1−5044<br>1FGL J1650.4−5042                   | ... | bcu   | PMN J1650−5044          |
| J1650.3−4600  | 252.599 | −46.014 | 339.798 | −0.952  | 0.035      | 0.032      | 19     | 16.2     | 9.2      | 0.7             | 61.2     | 6.4             | 2.23          | ...                  | LP  | ... | 5     | 2FGL J1650.6−4603c<br>1FGL J1651.5−4602c<br>EGR J1652−4552                    | E   | ...   | ...                     |
| J1650.8+0830  | 252.714 | 8.514   | 26.613  | 30.633  | 0.165      | 0.136      | 14     | 8.0      | 0.5      | 0.1             | 9.1      | 1.1             | 2.66          | 0.10                 | PL  | ... | ...   | 2FGL J1650.8+0830                                                             | ... | fsrq  | MG1 J165034+0824        |
| J1651.5−4626  | 252.898 | −46.434 | 339.606 | −1.379  | 0.060      | 0.047      | −90    | 4.9      | 1.2      | 0.5             | 13.9     | 4.8             | 1.92          | 0.26                 | PL  | ... | 5     | ...                                                                           | E   | ...   | ...                     |
| J1651.6+7219  | 252.911 | 72.318  | 104.261 | 34.708  | 0.071      | 0.056      | 44     | 5.8      | 0.2      | 0.1             | 2.3      | 0.6             | 1.80          | 0.19                 | PL  | ... | ...   | ...                                                                           | ... | bll   | RX J1651.6+7218         |
| J1652.2−4649  | 253.063 | −46.830 | 339.373 | −1.719  | 0.111      | 0.090      | −16    | 5.9      | 1.6      | 0.4             | 18.3     | 4.0             | 2.09          | 0.13                 | PL  | ... | ...   | ...                                                                           | ... | ...   | ...                     |
| J1652.8−4351  | 253.203 | −43.857 | 341.734 | 0.092   | 0.077      | 0.047      | 53     | 10.2     | 5.5      | 0.6             | 26.2     | 3.5             | 2.28          | ...                  | LP  | ... | ...   | 2FGL J1652.5−4351c<br>1FGL J1652.8−4350c                                      | ... | ...   | ...                     |
| J1653.6−0158  | 253.419 | −1.980  | 16.618  | 24.925  | 0.036      | 0.034      | −41    | 31.9     | 4.2      | 0.2             | 33.7     | 1.8             | 2.24          | ...                  | LP  | ... | ...   | 2FGL J1653.6−0159<br>1FGL J1653.6−0158<br>0FGL J1653.4−0200<br>3EG J1652−0223 | ... | ...   | ...                     |
| J1653.9+3945  | 253.478 | 39.754  | 63.593  | 38.850  | 0.010      | 0.010      | −71    | 93.3     | 9.7      | 0.2             | 129.8    | 4.4             | 1.72          | 0.02                 | PL  | T   | ...   | 1FHL J1653.9+3945<br>2FGL J1653.9+3945<br>1FGL J1653.9+3945                   | P   | BLL   | Mkn 501                 |

Table 1—Continued

| Name 3FGL         | R.A.    | Decl.   | $l$     | $b$    | $\theta_1$ | $\theta_2$ | $\phi$ | $\sigma$ | $F_{35}$ | $\Delta F_{35}$ | $S_{25}$ | $\Delta S_{25}$ | $\Gamma_{25}$ | $\Delta \Gamma_{25}$ | Mod | Var | Flags      | $\gamma$ -ray Assoc. | TeV | Class | ID or Assoc.       |
|-------------------|---------|---------|---------|--------|------------|------------|--------|----------|----------|-----------------|----------|-----------------|---------------|----------------------|-----|-----|------------|----------------------|-----|-------|--------------------|
| 0FGL J1653.9+3946 |         |         |         |        |            |            |        |          |          |                 |          |                 |               |                      |     |     |            |                      |     |       |                    |
| J1654.0–4617      | 253.501 | −46.297 | 339.976 | −1.614 | 0.049      | 0.041      | −17    | 6.2      | 1.5      | 0.3             | 16.4     | 3.5             | 2.01          | 0.13                 | PL  | ... | 1          | 3EG J1655−4554       | ... | ...   | ...                |
| J1654.3–4907      | 253.598 | −49.122 | 337.821 | −3.444 | 0.401      | 0.213      | 25     | 6.9      | 0.8      | 0.2             | 13.7     | 2.2             | 2.46          | ...                  | LP  | ... | 1,4,5,9,12 | ...                  | ... | ...   | ...                |
| J1655.1–4644      | 253.780 | −46.735 | 339.756 | −2.039 | 0.072      | 0.053      | −48    | 5.2      | 0.9      | 0.3             | 10.5     | 3.4             | 1.93          | 0.20                 | PL  | ... | 1          | ...                  | ... | ...   | ...                |
| J1655.1–3954      | 253.784 | −39.905 | 345.073 | 2.250  | 0.053      | 0.049      | −37    | 4.1      | 0.4      | 0.2             | 5.1      | 1.9             | 1.68          | 0.29                 | PL  | ... | ...        | ...                  | ... | ...   | ...                |
| J1655.5–4748      | 253.896 | −47.809 | 338.969 | −2.774 | 0.143      | 0.104      | 88     | 4.8      | 1.1      | 0.2             | 13.4     | 3.2             | 2.25          | 0.15                 | PL  | ... | 4          | ...                  | ... | ...   | ...                |
| J1655.7–4712      | 253.947 | −47.210 | 339.457 | −2.426 | 0.132      | 0.115      | −44    | 4.7      | 1.3      | 0.3             | 15.0     | 3.7             | 2.23          | 0.13                 | PL  | ... | ...        | ...                  | ... | ...   | ...                |
| J1656.0+2044      | 254.008 | 20.739  | 40.538  | 34.270 | 0.131      | 0.113      | −13    | 7.4      | 0.4      | 0.1             | 6.6      | 0.9             | 2.49          | 0.13                 | PL  | T   | ...        | ...                  | ... | bcu   | MG2 J165546+2043   |
| J1656.2–3303      | 254.075 | −33.052 | 350.590 | 6.344  | 0.153      | 0.092      | 34     | 13.3     | 1.3      | 0.2             | 27.4     | 2.1             | 2.78          | 0.07                 | PL  | T   | ...        | 2FGL J1656.1–3256    | ... | fsrq  | Swift J1656.3–3302 |
| 1FGL J1656.2–3257 |         |         |         |        |            |            |        |          |          |                 |          |                 |               |                      |     |     |            |                      |     |       |                    |
| J1656.8–2010      | 254.218 | −20.175 | 1.066   | 14.073 | 0.064      | 0.057      | −76    | 9.4      | 1.0      | 0.1             | 11.2     | 1.6             | 1.96          | 0.08                 | PL  | ... | ...        | 2FGL J1656.9–2008    | ... | bcu   | 1RXS               |
| 2FGL J1656.9–2008 |         |         |         |        |            |            |        |          |          |                 |          |                 |               |                      |     |     |            |                      |     |       |                    |
| J165655.0–201049  |         |         |         |        |            |            |        |          |          |                 |          |                 |               |                      |     |     |            |                      |     |       |                    |
| J1656.9–3919c     | 254.245 | −39.327 | 345.746 | 2.334  | 0.072      | 0.066      | 50     | 5.5      | 1.2      | 0.3             | 16.2     | 9.0             | 2.45          | 0.38                 | PL  | ... | 1,4,6      | ...                  | ... | ...   | ...                |
| J1656.9+6008      | 254.246 | 60.143  | 89.546  | 37.420 | 0.106      | 0.097      | 64     | 9.3      | 0.3      | 0.1             | 5.9      | 0.7             | 2.62          | 0.11                 | PL  | ... | ...        | 2FGL J1656.5+6012    | ... | fsrq  | 87GB               |
| 165604.4+601702   |         |         |         |        |            |            |        |          |          |                 |          |                 |               |                      |     |     |            |                      |     |       |                    |
| 1FGL J1656.9+6017 |         |         |         |        |            |            |        |          |          |                 |          |                 |               |                      |     |     |            |                      |     |       |                    |
| J1657.6–4653      | 254.419 | −46.896 | 339.903 | −2.481 | 0.050      | 0.044      | 28     | 5.8      | 1.1      | 0.3             | 12.4     | 3.2             | 2.05          | 0.14                 | PL  | ... | ...        | 2FGL J1657.5–4652    | ... | ...   | ...                |
| J1657.7+4807      | 254.428 | 48.132  | 74.355  | 38.489 | 0.042      | 0.041      | −19    | 28.1     | 1.4      | 0.1             | 19.8     | 0.9             | 2.48          | 0.04                 | PL  | T   | ...        | 2FGL J1657.9+4809    | ... | fsrq  | 4C +48.41          |
| J1658.3+6149      | 254.595 | 61.828  | 91.583  | 36.937 | 0.087      | 0.071      | 10     | 6.2      | 0.3      | 0.1             | 2.8      | 0.6             | 2.03          | 0.17                 | PL  | ... | ...        | ...                  | ... | bll   | NVSS               |
| J165808+615001    |         |         |         |        |            |            |        |          |          |                 |          |                 |               |                      |     |     |            |                      |     |       |                    |
| J1658.4–5323      | 254.621 | −53.389 | 334.863 | −6.598 | 0.061      | 0.054      | −8     | 16.9     | 2.6      | 0.2             | 20.3     | 2.0             | 2.39          | ...                  | EC  | ... | ...        | 2FGL J1658.4–5322    | ... | PSR   | PSR J1658–5324     |
| 1FGL J1658.8–5317 |         |         |         |        |            |            |        |          |          |                 |          |                 |               |                      |     |     |            |                      |     |       |                    |
| J1659.0–0142      | 254.774 | −1.702  | 17.647  | 23.908 | 0.098      | 0.083      | −84    | 8.5      | 0.9      | 0.1             | 10.6     | 1.5             | 2.19          | 0.11                 | PL  | ... | 3          | 2FGL J1659.2–0142    | ... | ...   | ...                |
| J1659.4+2631      | 254.862 | 26.526  | 47.544  | 35.271 | 0.389      | 0.280      | 89     | 4.1      | 0.2      | 0.1             | 3.8      | 0.9             | 2.71          | 0.22                 | PL  | ... | ...        | ...                  | ... | fsrq  | 4C +26.51          |
| J1659.7–3132      | 254.950 | −31.549 | 352.240 | 6.686  | 0.102      | 0.080      | 5      | 6.4      | 0.8      | 0.1             | 11.0     | 1.9             | 2.40          | 0.11                 | PL  | ... | ...        | ...                  | ... | bcu   | NVSS               |
| J165949–313047    |         |         |         |        |            |            |        |          |          |                 |          |                 |               |                      |     |     |            |                      |     |       |                    |
| J1700.1+6829      | 255.050 | 68.485  | 99.542  | 35.204 | 0.026      | 0.025      | 34     | 49.4     | 3.0      | 0.1             | 39.4     | 1.1             | 2.40          | 0.02                 | PL  | T   | ...        | 2FGL J1700.2+6831    | ... | fsrq  | TXS 1700+685       |
| 1FGL J1700.1+6830 |         |         |         |        |            |            |        |          |          |                 |          |                 |               |                      |     |     |            |                      |     |       |                    |
| J1700.4–4019c     | 255.109 | −40.331 | 345.370 | 1.191  | 0.085      | 0.070      | 2      | 5.6      | 1.6      | 0.5             | 31.1     | 20.9            | 2.69          | 0.63                 | PL  | ... | 3,6,10     | ...                  | ... | ...   | ...                |
| J1701.1–4930      | 255.286 | −49.514 | 338.195 | −4.551 | 0.132      | 0.105      | 3      | 5.3      | 0.9      | 0.2             | 12.4     | 2.6             | 2.44          | 0.12                 | PL  | ... | 1          | ...                  | ... | ...   | ...                |
| J1701.2–3006      | 255.323 | −30.104 | 353.593 | 7.310  | 0.042      | 0.041      | −35    | 18.9     | 3.1      | 0.2             | 20.8     | 1.9             | 2.20          | ...                  | LP  | ... | ...        | 2FGL J1701.2–3007    | ... | glc   | M62                |
| 1FGL J1701.1–3005 |         |         |         |        |            |            |        |          |          |                 |          |                 |               |                      |     |     |            |                      |     |       |                    |
| J1701.3–5216      | 255.343 | −52.269 | 336.024 | −6.259 | 0.138      | 0.096      | −14    | 4.5      | 0.6      | 0.1             | 8.1      | 1.9             | 2.48          | 0.14                 | PL  | ... | 5          | ...                  | ... | ...   | ...                |
| J1701.4–4654      | 255.364 | −46.907 | 340.294 | −2.996 | 0.126      | 0.087      | 84     | 5.9      | 1.6      | 0.3             | 27.9     | 5.4             | 2.64          | 0.09                 | PL  | ... | 4          | ...                  | ... | ...   | ...                |
| J1702.0–5414      | 255.504 | −54.247 | 334.497 | −7.534 | 0.389      | 0.272      | 51     | 4.1      | 0.5      | 0.1             | 8.0      | 1.8             | 2.58          | 0.14                 | PL  | ... | 5          | ...                  | ... | ...   | ...                |
| J1702.1–2524      | 255.530 | −25.413 | 357.496 | 9.984  | 0.088      | 0.065      | 84     | 4.1      | 0.3      | 0.1             | 4.0      | 1.3             | 1.76          | 0.28                 | PL  | ... | 3          | ...                  | ... | ...   | ...                |
| J1702.1–4623      | 255.537 | −46.387 | 340.779 | −2.772 | 0.140      | 0.116      | −17    | 4.9      | 1.4      | 0.3             | 20.7     | 5.1             | 2.51          | 0.13                 | PL  | ... | 4          | ...                  | ... | ...   | ...                |
| J1702.6+3116      | 255.661 | 31.268  | 53.403  | 35.759 | 0.101      | 0.077      | −66    | 5.8      | 0.2      | 0.1             | 3.7      | 1.1             | 1.40          | 0.15                 | PL  | ... | ...        | ...                  | ... | bll   | RX J1702.6+3115    |
| J1702.8–5656      | 255.720 | −56.936 | 332.398 | −9.245 | 0.044      | 0.037      | 68     | 28.8     | 3.2      | 0.2             | 32.0     | 1.7             | 2.39          | ...                  | LP  | ... | ...        | 2FGL J1702.5–5654    | ... | ...   | ...                |

Table 1—Continued

| Name 3FGL     | R.A.    | Decl.   | $l$     | $b$     | $\theta_1$ | $\theta_2$ | $\phi$ | $\sigma$ | $F_{35}$ | $\Delta F_{35}$ | $S_{25}$ | $\Delta S_{25}$ | $\Gamma_{25}$ | $\Delta \Gamma_{25}$ | Mod | Var | Flags | $\gamma$ -ray Assoc. | TeV | Class            | ID or Assoc.    |
|---------------|---------|---------|---------|---------|------------|------------|--------|----------|----------|-----------------|----------|-----------------|---------------|----------------------|-----|-----|-------|----------------------|-----|------------------|-----------------|
|               |         |         |         |         |            |            |        |          |          |                 |          |                 |               |                      |     |     |       | 1FGL J1702.4–5653    |     |                  |                 |
| J1703.6–6211  | 255.917 | –62.196 | 328.134 | –12.430 | 0.040      | 0.038      | 87     | 34.6     | 2.8      | 0.2             | 40.1     | 1.5             | 2.47          | 0.03                 | PL  | T   | ...   | 1FGL J1702.7–6217    | ... | fsrq             | MRC 1659–621    |
| J1703.6–2850  | 255.924 | –28.848 | 354.922 | 7.650   | 0.085      | 0.077      | –18    | 4.1      | 0.5      | 0.1             | 5.9      | 1.5             | 2.23          | 0.17                 | PL  | ... | 3     | ...                  | ... | ...              | ...             |
| J1703.9–4843  | 255.990 | –48.724 | 339.106 | –4.436  | 0.128      | 0.096      | –53    | 7.2      | 1.2      | 0.2             | 17.8     | 2.7             | 2.48          | 0.09                 | PL  | ... | ...   | ...                  | ... | ...              | ...             |
| J1704.0+7646  | 256.023 | 76.769  | 108.934 | 32.401  | 0.234      | 0.131      | –44    | 7.2      | 0.3      | 0.1             | 4.5      | 0.7             | 2.57          | 0.13                 | PL  | T   | ...   | ...                  | ... | bcu              | NVSS            |
|               |         |         |         |         |            |            |        |          |          |                 |          |                 |               |                      |     |     |       |                      |     | J170357+764611   |                 |
| J1704.1+1234  | 256.033 | 12.574  | 32.465  | 29.424  | 0.069      | 0.069      | 72     | 9.4      | 0.6      | 0.1             | 9.4      | 1.2             | 2.58          | 0.10                 | PL  | ... | ...   | 2FGL J1704.3+1235    | ... | ...              | ...             |
| J1704.4–0528  | 256.121 | –5.478  | 14.913  | 20.797  | 0.089      | 0.062      | 88     | 7.9      | 0.9      | 0.1             | 10.1     | 1.5             | 2.18          | 0.11                 | PL  | ... | ...   | 2FGL J1704.6–0529    | ... | ...              | ...             |
| J1705.5+0948  | 256.376 | 9.803   | 29.763  | 27.951  | 0.231      | 0.203      | –52    | 6.0      | 0.3      | 0.1             | 7.3      | 1.2             | 2.81          | 0.14                 | PL  | ... | ...   | ...                  | ... | ...              | ...             |
| J1705.5+7134  | 256.389 | 71.567  | 102.988 | 33.919  | 0.187      | 0.142      | 13     | 4.1      | 0.2      | 0.0             | 2.5      | 0.6             | 2.45          | 0.21                 | PL  | ... | ...   | ...                  | ... | bll              | GB6 J1704+7138  |
| J1705.5–4128c | 256.396 | –41.481 | 345.052 | –0.281  | 0.141      | 0.084      | –64    | 5.1      | 1.4      | 1.7             | 29.2     | 13.6            | 2.77          | 1.06                 | PL  | ... | 1,4,6 | ...                  | ... | ...              | ...             |
| J1707.8+5626  | 256.956 | 56.443  | 84.719  | 36.505  | 0.231      | 0.175      | –74    | 5.4      | 0.2      | 0.1             | 3.7      | 0.7             | 2.76          | 0.19                 | PL  | ... | 1     | ...                  | ... | ...              | ...             |
| J1709.4–0917  | 257.368 | –9.284  | 12.197  | 17.725  | 0.172      | 0.146      | 21     | 5.7      | 0.7      | 0.1             | 9.8      | 1.6             | 2.46          | 0.11                 | PL  | ... | 3     | 3EG J1709–0828       | ... | ...              | ...             |
| J1709.5–0335  | 257.386 | –3.595  | 17.334  | 20.697  | 0.221      | 0.157      | 30     | 6.1      | 0.6      | 0.1             | 9.7      | 1.6             | 2.59          | 0.13                 | PL  | ... | 1     | 2FGL J1710.0–0323    | ... | ...              | ...             |
|               |         |         |         |         |            |            |        |          |          |                 |          |                 |               |                      |     |     |       | 1FGL J1709.1–0343    |     |                  |                 |
| J1709.6+4318  | 257.424 | 43.312  | 68.392  | 36.223  | 0.023      | 0.023      | 58     | 62.2     | 4.4      | 0.2             | 47.0     | 1.5             | 2.28          | ...                  | LP  | T   | ...   | 1FHL J1709.5+4320    | ... | fsrq             | B3 1708+433     |
|               |         |         |         |         |            |            |        |          |          |                 |          |                 |               |                      |     |     |       | 2FGL J1709.7+4319    |     |                  | 0               |
|               |         |         |         |         |            |            |        |          |          |                 |          |                 |               |                      |     |     |       | 1FGL J1709.6+4320    |     |                  |                 |
| J1709.7–4429  | 257.432 | –44.487 | 343.098 | –2.689  | 0.006      | 0.006      | 9      | 360.8    | 187.3    | 1.2             | 1314.8   | 8.0             | 2.02          | ...                  | EC  | ... | ...   | 1FHL J1709.7–4429    | E   | PSR              | PSR J1709–4429  |
|               |         |         |         |         |            |            |        |          |          |                 |          |                 |               |                      |     |     |       | 2FGL J1709.7–4429    |     |                  |                 |
|               |         |         |         |         |            |            |        |          |          |                 |          |                 |               |                      |     |     |       | 1FGL J1709.7–4429    |     |                  |                 |
|               |         |         |         |         |            |            |        |          |          |                 |          |                 |               |                      |     |     |       | 0FGL J1709.7–4428    |     |                  |                 |
|               |         |         |         |         |            |            |        |          |          |                 |          |                 |               |                      |     |     |       | 1AGL J1709–4428      |     |                  |                 |
| J1709.9+4624  | 257.487 | 46.412  | 72.234  | 36.385  | 0.275      | 0.183      | 1      | 4.8      | 0.2      | 0.1             | 3.6      | 0.7             | 2.51          | 0.17                 | PL  | ... | ...   | ...                  | ... | ...              | ...             |
| J1710.6–4317  | 257.660 | –43.289 | 344.162 | –2.111  | 0.154      | 0.113      | –28    | 5.0      | 1.3      | 0.3             | 19.9     | 4.2             | 2.53          | 0.13                 | PL  | ... | 4,5   | ...                  | ... | ...              | ...             |
| J1711.5–5029  | 257.890 | –50.484 | 338.420 | –6.472  | 0.081      | 0.078      | –69    | 5.4      | 0.6      | 0.1             | 9.9      | 1.9             | 2.56          | 0.12                 | PL  | ... | 1     | ...                  | ... | bcu              | PMN J1711–5028  |
| J1711.6+8846  | 257.908 | 88.774  | 121.677 | 27.640  | 0.057      | 0.048      | –32    | 6.7      | 0.2      | 0.1             | 3.3      | 0.8             | 1.57          | 0.18                 | PL  | ... | ...   | ...                  | ... | bcu              | 1RXS            |
|               |         |         |         |         |            |            |        |          |          |                 |          |                 |               |                      |     |     |       |                      |     | J171643.8+884414 |                 |
| J1712.6+2932  | 258.160 | 29.537  | 51.984  | 33.254  | 0.086      | 0.062      | –20    | 6.5      | 0.3      | 0.1             | 3.9      | 1.0             | 1.58          | 0.15                 | PL  | ... | ...   | ...                  | ... | bll              | RX J1712.8+2931 |
| J1713.5–3945e | 258.390 | –39.760 | 347.336 | –0.473  | ...        | ...        | ...    | 14.4     | 4.5      | 0.6             | 66.9     | 5.9             | 1.62          | 0.07                 | PL  | ... | 3     | 1FGL J1711.7–3944c   | E   | SNR              | RX J1713.7–3946 |
|               |         |         |         |         |            |            |        |          |          |                 |          |                 |               |                      |     |     |       | 1FHL J1713.5–3951e   |     |                  |                 |
|               |         |         |         |         |            |            |        |          |          |                 |          |                 |               |                      |     |     |       | 2FGL J1712.4–3941    |     |                  |                 |
|               |         |         |         |         |            |            |        |          |          |                 |          |                 |               |                      |     |     |       | ...                  |     |                  |                 |
| J1714.0+0748  | 258.504 | 7.802   | 28.782  | 25.184  | 0.062      | 0.059      | 90     | 13.6     | 1.5      | 0.2             | 9.4      | 1.2             | 2.19          | ...                  | EC  | ... | ...   | 2FGL J1714.0+0751    | ... | PSR              | PSR J1713+0747  |
|               |         |         |         |         |            |            |        |          |          |                 |          |                 |               |                      |     |     |       | 1FGL J1713.9+0750    |     |                  |                 |
| J1714.1–2029  | 258.533 | –20.496 | 3.196   | 10.588  | 0.058      | 0.055      | –64    | 6.8      | 0.3      | 0.1             | 5.7      | 1.5             | 1.34          | 0.18                 | PL  | ... | ...   | ...                  | ... | bcu              | 1RXS            |
|               |         |         |         |         |            |            |        |          |          |                 |          |                 |               |                      |     |     |       |                      |     | J171405.2–202747 |                 |
| J1714.5–3832  | 258.643 | –38.549 | 348.433 | 0.077   | 0.029      | 0.026      | –12    | 29.2     | 14.0     | 0.6             | 130.5    | 7.2             | 2.30          | ...                  | LP  | ... | ...   | 0FGL J1714.7–3827    | E   | snr              | CTB 37A         |

Table 1—Continued

| Name 3FGL    | R.A.    | Decl.   | $l$     | $b$     | $\theta_1$ | $\theta_2$ | $\phi$ | $\sigma$ | $F_{35}$ | $\Delta F_{35}$ | $S_{25}$ | $\Delta S_{25}$ | $\Gamma_{25}$ | $\Delta \Gamma_{25}$ | Mod | Var | Flags | $\gamma$ -ray Assoc. | TeV | Class | ID or Assoc.     |
|--------------|---------|---------|---------|---------|------------|------------|--------|----------|----------|-----------------|----------|-----------------|---------------|----------------------|-----|-----|-------|----------------------|-----|-------|------------------|
|              |         |         |         |         |            |            |        |          |          |                 |          |                 |               |                      |     |     |       | 1FGL J1714.5–3830c   |     |       |                  |
|              |         |         |         |         |            |            |        |          |          |                 |          |                 |               |                      |     |     |       | 2FGL J1714.5–3829    |     |       |                  |
|              |         |         |         |         |            |            |        |          |          |                 |          |                 |               |                      |     |     |       | 3EG J1714–3857       |     |       |                  |
| J1714.6–3327 | 258.656 | –33.457 | 352.576 | 3.040   | 0.132      | 0.087      | –30    | 5.4      | 1.2      | 0.2             | 15.5     | 3.2             | 2.36          | 0.12                 | PL  | ... | ...   | 1FGL J1715.2–3319    | ... | ...   | ...              |
| J1715.4–4028 | 258.852 | –40.469 | 346.967 | –1.174  | 0.043      | 0.042      | 42     | 6.5      | 1.4      | 0.3             | 15.3     | 3.3             | 2.10          | 0.16                 | PL  | ... | ...   | 2FGL J1715.4–4024c   | ... | ...   | ...              |
| J1715.7+6837 | 258.939 | 68.631  | 99.306  | 33.788  | 0.060      | 0.054      | –26    | 16.3     | 1.0      | 0.1             | 7.7      | 0.8             | 2.25          | ...                  | LP  | T   | ...   | 2FGL J1714.8+6836    | ... | fsrq  | S4 1716+68       |
| J1716.6–2812 | 259.161 | –28.205 | 357.125 | 5.723   | 0.174      | 0.115      | 6      | 7.9      | 1.2      | 0.2             | 17.6     | 2.3             | 2.49          | 0.09                 | PL  | ... | ...   | 2FGL J1717.3–2809    | ... | glc   | NGC 6316         |
|              |         |         |         |         |            |            |        |          |          |                 |          |                 |               |                      |     |     |       | 3EG J1717–2737       |     |       |                  |
| J1716.7–8112 | 259.190 | –81.215 | 311.694 | –23.333 | 0.075      | 0.072      | 34     | 4.3      | 0.3      | 0.1             | 2.8      | 0.8             | 2.06          | 0.24                 | PL  | ... | ...   | ...                  | ... | bcu   | 1RXS             |
|              |         |         |         |         |            |            |        |          |          |                 |          |                 |               |                      |     |     |       |                      |     |       | J171712.6–811501 |
| J1717.4–5157 | 259.365 | –51.965 | 337.733 | –8.079  | 0.094      | 0.062      | –80    | 12.2     | 1.4      | 0.1             | 20.6     | 2.0             | 2.49          | 0.07                 | PL  | T   | ...   | ...                  | ... | fsrq  | PMN J1717–5155   |
| J1717.6–5802 | 259.408 | –58.044 | 332.635 | –11.503 | 0.125      | 0.076      | –13    | 10.9     | 0.9      | 0.1             | 12.4     | 1.3             | 2.42          | 0.09                 | PL  | ... | 7     | 2FGL J1717.5–5802    | ... | psr   | PSR J1717–5800   |
| J1717.6–4404 | 259.421 | –44.068 | 344.273 | –3.600  | 0.152      | 0.138      | –8     | 7.5      | 1.4      | 0.2             | 24.5     | 3.3             | 2.64          | 0.09                 | PL  | ... | 1     | ...                  | ... | ...   | ...              |
| J1717.8–3342 | 259.451 | –33.700 | 352.762 | 2.359   | 0.039      | 0.034      | –68    | 22.4     | 5.6      | 0.3             | 86.1     | 4.4             | 2.54          | 0.03                 | PL  | T   | ...   | 2FGL J1717.7–3342    | ... | bll   | TXS 1714–336     |
|              |         |         |         |         |            |            |        |          |          |                 |          |                 |               |                      |     |     |       | 1FGL J1717.9–3343    |     |       |                  |
|              |         |         |         |         |            |            |        |          |          |                 |          |                 |               |                      |     |     |       | 3EG J1718–3313       |     |       |                  |
| J1718.0–3726 | 259.506 | –37.448 | 349.724 | 0.162   | 0.030      | 0.026      | –35    | 13.1     | 4.4      | 0.4             | 48.8     | 4.9             | 2.13          | 0.06                 | PL  | ... | 3     | 1FHL J1717.9–3725    | P   | snr   | SNR G349.7+00.2  |
|              |         |         |         |         |            |            |        |          |          |                 |          |                 |               |                      |     |     |       | 2FGL J1718.1–3725    |     |       |                  |
|              |         |         |         |         |            |            |        |          |          |                 |          |                 |               |                      |     |     |       | 1FGL J1717.9–3729c   |     |       |                  |
| J1718.1–3056 | 259.529 | –30.941 | 355.060 | 3.891   | 0.066      | 0.057      | 60     | 7.9      | 1.3      | 0.2             | 17.2     | 2.5             | 2.37          | 0.09                 | PL  | ... | ...   | 2FGL J1718.4–3056    | ... | bcu   | PMN J1718–3056   |
| J1718.1–3825 | 259.545 | –38.428 | 348.941 | –0.428  | 0.034      | 0.030      | 62     | 24.4     | 11.5     | 0.6             | 82.4     | 6.6             | 2.39          | ...                  | EC  | ... | ...   | 2FGL J1718.3–3827    | E   | PSR   | PSR J1718–3825   |
|              |         |         |         |         |            |            |        |          |          |                 |          |                 |               |                      |     |     |       | 1FGL J1718.2–3825    |     |       |                  |
| J1719.2+1744 | 259.811 | 17.742  | 39.518  | 28.087  | 0.033      | 0.032      | –36    | 20.6     | 1.6      | 0.1             | 17.6     | 1.4             | 2.04          | 0.06                 | PL  | T   | ...   | 1FHL J1719.1+1745    | ... | bll   | PKS 1717+177     |
|              |         |         |         |         |            |            |        |          |          |                 |          |                 |               |                      |     |     |       | 2FGL J1719.3+1744    |     |       |                  |
|              |         |         |         |         |            |            |        |          |          |                 |          |                 |               |                      |     |     |       | 1FGL J1719.2+1745    |     |       |                  |
|              |         |         |         |         |            |            |        |          |          |                 |          |                 |               |                      |     |     |       | 0FGL J1719.3+1746    |     |       |                  |
| J1719.2–2433 | 259.819 | –24.551 | 0.487   | 7.318   | 0.200      | 0.160      | –59    | 6.3      | 0.7      | 0.2             | 13.6     | 2.0             | 2.66          | 0.12                 | PL  | ... | 1,4   | ...                  | ... | ...   | ...              |
| J1719.3+1206 | 259.848 | 12.108  | 33.721  | 25.837  | 0.063      | 0.056      | 82     | 6.6      | 0.5      | 0.1             | 5.4      | 1.1             | 2.08          | 0.18                 | PL  | ... | ...   | ...                  | ... | bcu   | 1RXS             |
|              |         |         |         |         |            |            |        |          |          |                 |          |                 |               |                      |     |     |       |                      |     |       | J171921.2+120711 |
| J1720.3–0428 | 260.096 | –4.473  | 17.992  | 17.923  | 0.078      | 0.072      | 47     | 4.3      | 0.5      | 0.2             | 5.8      | 1.7             | 2.09          | 0.18                 | PL  | ... | ...   | 3EG J1719–0430       | ... | ...   | ...              |
| J1720.7+0711 | 260.191 | 7.189   | 28.997  | 23.414  | 0.091      | 0.073      | 74     | 9.5      | 0.9      | 0.1             | 11.2     | 1.4             | 2.35          | 0.09                 | PL  | ... | ...   | 2FGL J1721.0+0711    | ... | ...   | ...              |
|              |         |         |         |         |            |            |        |          |          |                 |          |                 |               |                      |     |     |       | 1FGL J1721.1+0713    |     |       |                  |
| J1721.4–5253 | 260.356 | –52.897 | 337.295 | –9.102  | 0.276      | 0.154      | 10     | 6.3      | 0.6      | 0.1             | 10.6     | 1.8             | 2.58          | 0.12                 | PL  | ... | ...   | ...                  | ... | ...   | ...              |
| J1721.8–3919 | 260.464 | –39.326 | 348.614 | –1.528  | 0.094      | 0.071      | –29    | 5.3      | 1.4      | 0.3             | 18.5     | 3.9             | 2.42          | 0.14                 | PL  | ... | 1     | ...                  | ... | ...   | ...              |
| J1722.7+6104 | 260.690 | 61.082  | 90.168  | 34.161  | 0.377      | 0.229      | 72     | 5.1      | 0.2      | 0.1             | 5.4      | 1.0             | 2.87          | 0.14                 | PL  | ... | ...   | ...                  | ... | fsrq  | GB6 J1722+6105   |
| J1722.7–0415 | 260.691 | –4.264  | 18.495  | 17.517  | 0.111      | 0.087      | 7      | 6.4      | 1.0      | 0.2             | 12.3     | 2.1             | 2.29          | 0.09                 | PL  | ... | ...   | 2FGL J1722.5–0420    | ... | ...   | ...              |
|              |         |         |         |         |            |            |        |          |          |                 |          |                 |               |                      |     |     |       | 1FGL J1722.4–0421    |     |       |                  |

Table 1—Continued

| Name 3FGL     | R.A.    | Decl.   | $l$     | $b$     | $\theta_1$ | $\theta_2$ | $\phi$ | $\sigma$ | $F_{35}$ | $\Delta F_{35}$ | $S_{25}$ | $\Delta S_{25}$ | $\Gamma_{25}$ | $\Delta \Gamma_{25}$ | Mod | Var | Flags | $\gamma$ -ray Assoc.                                                       | TeV | Class | ID or Assoc.   |
|---------------|---------|---------|---------|---------|------------|------------|--------|----------|----------|-----------------|----------|-----------------|---------------|----------------------|-----|-----|-------|----------------------------------------------------------------------------|-----|-------|----------------|
| J1722.7+1014  | 260.691 | 10.243  | 32.238  | 24.302  | 0.032      | 0.030      | 59     | 19.9     | 1.8      | 0.1             | 22.1     | 1.5             | 2.30          | 0.05                 | PL  | T   | ...   | 1FHL J1722.6+1011<br>2FGL J1722.7+1013<br>1FGL J1722.5+1012                | ... | fsrq  | TXS 1720+102   |
| J1722.9–4529  | 260.728 | –45.484 | 343.633 | –5.167  | 0.135      | 0.109      | 37     | 5.9      | 0.9      | 0.2             | 13.1     | 2.6             | 2.51          | 0.13                 | PL  | ... | 1     | ...                                                                        | ... | spp   | ...            |
| J1723.5–5609  | 260.881 | –56.161 | 334.689 | –11.143 | 0.137      | 0.101      | –65    | 4.3      | 0.3      | 0.1             | 5.6      | 1.3             | 2.62          | 0.20                 | PL  | ... | ...   | ...                                                                        | ... | bcu   | PMN J1723–5614 |
| J1723.6–3646  | 260.919 | –36.768 | 350.925 | –0.376  | 0.086      | 0.060      | –2     | 4.2      | 1.6      | 0.4             | 20.6     | 7.4             | 2.35          | 0.23                 | PL  | ... | 3     | ...                                                                        | ... | ...   | ...            |
| J1723.7–7713  | 260.943 | –77.231 | 315.690 | –21.795 | 0.069      | 0.062      | 69     | 14.7     | 1.1      | 0.1             | 15.1     | 1.2             | 2.47          | 0.06                 | PL  | T   | ...   | 2FGL J1725.1–7714                                                          | ... | bcu   | PKS 1716–771   |
| J1723.9+4004  | 260.986 | 40.068  | 64.881  | 33.179  | 0.056      | 0.053      | –31    | 21.7     | 1.2      | 0.1             | 16.4     | 1.0             | 2.45          | 0.05                 | PL  | T   | ...   | 2FGL J1724.0+4003<br>1FGL J1724.0+4002                                     | ... | fsrq  | S4 1722+40     |
| J1725.0–0513  | 261.251 | –5.223  | 17.923  | 16.551  | 0.145      | 0.103      | 84     | 4.7      | 0.6      | 0.2             | 6.9      | 1.7             | 2.02          | 0.18                 | PL  | ... | ...   | 2FGL J1724.9–0508c<br>1FGL J1725.2–0509                                    | ... | ...   | ...            |
| J1725.0+1152  | 261.262 | 11.883  | 34.130  | 24.485  | 0.021      | 0.020      | 83     | 32.7     | 3.5      | 0.2             | 40.8     | 2.4             | 1.89          | 0.05                 | PL  | T   | ...   | 1FHL J1725.1+1151<br>2FGL J1725.0+1151<br>1FGL J1725.0+1151                | P   | bll   | 1H 1720+117    |
| J1725.1–2832  | 261.279 | –28.539 | 357.907 | 3.998   | 0.108      | 0.100      | 19     | 6.1      | 1.1      | 0.2             | 18.5     | 3.0             | 2.60          | 0.11                 | PL  | ... | 1,10  | 1FGL J1725.5–2832                                                          | ... | spp   | ...            |
| J1725.3+5853  | 261.332 | 58.887  | 87.497  | 33.996  | 0.076      | 0.072      | 87     | 8.6      | 0.4      | 0.1             | 5.0      | 0.7             | 2.18          | 0.12                 | PL  | ... | ...   | 2FGL J1725.2+5853<br>1FGL J1725.5+5854                                     | ... | bll   | 7C 1724+5854   |
| J1725.7–3555c | 261.429 | –35.930 | 351.849 | –0.244  | 0.176      | 0.113      | –84    | 4.1      | 2.2      | 0.5             | 31.8     | 10.2            | 2.47          | 0.15                 | PL  | ... | 5,6   | 1FGL J1724.0–3611c                                                         | ... | ...   | ...            |
| J1726.6–3530c | 261.667 | –35.515 | 352.301 | –0.173  | 0.078      | 0.072      | –24    | 7.9      | 4.0      | 0.5             | 54.3     | 8.0             | 2.43          | 0.07                 | PL  | ... | 3,6   | ...                                                                        | ... | ...   | ...            |
| J1727.1+4531  | 261.800 | 45.527  | 71.446  | 33.328  | 0.053      | 0.050      | –43    | 29.9     | 1.4      | 0.1             | 20.0     | 0.9             | 2.53          | ...                  | LP  | T   | ...   | 2FGL J1727.1+4531<br>1FGL J1727.3+4525                                     | ... | fsrq  | S4 1726+45     |
| J1727.4+0634  | 261.872 | 6.576   | 29.211  | 21.646  | 0.287      | 0.240      | –4     | 5.6      | 0.4      | 0.1             | 8.1      | 1.5             | 2.69          | 0.13                 | PL  | ... | ...   | 2FGL J1727.6+0647                                                          | ... | ...   | ...            |
| J1727.6–0654  | 261.914 | –6.913  | 16.756  | 15.127  | 0.309      | 0.223      | –0     | 5.6      | 0.8      | 0.2             | 10.8     | 1.9             | 2.46          | 0.12                 | PL  | ... | 1     | 2FGL J1727.1–0704                                                          | ... | ...   | ...            |
| J1727.7–2637  | 261.946 | –26.625 | 359.833 | 4.568   | 0.261      | 0.177      | –14    | 10.0     | 1.1      | 0.2             | 20.9     | 2.5             | 2.59          | ...                  | LP  | ... | ...   | ...                                                                        | ... | ...   | ...            |
| J1728.0–4606  | 262.001 | –46.109 | 343.605 | –6.253  | 0.094      | 0.084      | –50    | 6.8      | 0.9      | 0.1             | 11.0     | 1.9             | 2.33          | 0.12                 | PL  | ... | ...   | 2FGL J1727.3–4611                                                          | ... | spp   | ...            |
| J1728.0+1217  | 262.002 | 12.289  | 34.864  | 23.995  | 0.067      | 0.064      | –13    | 7.6      | 0.7      | 0.1             | 8.8      | 1.5             | 2.38          | 0.12                 | PL  | T   | ...   | 2FGL J1727.9+1220                                                          | ... | fsrq  | PKS 1725+123   |
| J1728.0–6446  | 262.010 | –64.773 | 327.425 | –16.111 | 0.368      | 0.321      | 79     | 4.4      | 0.2      | 0.1             | 4.9      | 1.0             | 2.91          | 0.19                 | PL  | ... | 4     | ...                                                                        | ... | ...   | ...            |
| J1728.3+5013  | 262.096 | 50.231  | 77.082  | 33.526  | 0.036      | 0.032      | –50    | 18.8     | 1.1      | 0.1             | 12.2     | 1.1             | 1.96          | 0.06                 | PL  | ... | ...   | 1FHL J1728.3+5014<br>2FGL J1728.2+5015<br>1FGL J1727.9+5010                | P   | bll   | I Zw 187       |
| J1728.5+0428  | 262.145 | 4.478   | 27.340  | 20.452  | 0.160      | 0.125      | 70     | 11.7     | 0.9      | 0.1             | 14.9     | 1.4             | 2.59          | 0.08                 | PL  | T   | ...   | 2FGL J1728.2+0429<br>1FGL J1728.2+0431<br>3EG J1727+0429<br>EGR J1727+0416 | ... | fsrq  | PKS 1725+044   |
| J1729.0+6049  | 262.264 | 60.826  | 89.791  | 33.418  | 0.163      | 0.137      | –49    | 4.3      | 0.2      | 0.1             | 3.6      | 1.0             | 2.52          | 0.18                 | PL  | ... | ...   | 3EG J1733+6017                                                             | ... | ...   | ...            |

Table 1—Continued

| Name 3FGL    | R.A.    | Decl.   | $l$     | $b$     | $\theta_1$ | $\theta_2$ | $\phi$ | $\sigma$ | $F_{35}$ | $\Delta F_{35}$ | $S_{25}$ | $\Delta S_{25}$ | $\Gamma_{25}$ | $\Delta \Gamma_{25}$ | Mod | Var | Flags      | $\gamma$ -ray Assoc.                                        | TeV | Class | ID or Assoc.           |
|--------------|---------|---------|---------|---------|------------|------------|--------|----------|----------|-----------------|----------|-----------------|---------------|----------------------|-----|-----|------------|-------------------------------------------------------------|-----|-------|------------------------|
| J1729.5–2824 | 262.375 | –28.411 | 358.550 | 3.267   | 0.597      | 0.503      | –34    | 6.7      | 1.0      | 0.2             | 16.0     | 2.6             | 2.62          | ...                  | LP  | ... | 1,4,5,9,12 | ...                                                         | ... | spp   | ...                    |
| J1729.7–2408 | 262.435 | –24.137 | 2.165   | 5.564   | 0.145      | 0.118      | –89    | 11.7     | 1.6      | 0.3             | 23.4     | 2.4             | 2.57          | ...                  | LP  | ... | 3          | 2FGL J1730.6–2409<br>1FGL J1730.4–2406                      | ... | ...   | ...                    |
| J1729.9–0859 | 262.491 | –8.986  | 15.218  | 13.576  | 0.583      | 0.448      | 56     | 7.2      | 0.4      | 0.1             | 10.7     | 1.5             | 2.61          | ...                  | LP  | ... | 1,9,12     | 2FGL J1729.5–0854                                           | ... | ...   | ...                    |
| J1730.5+0023 | 262.647 | 0.397   | 23.769  | 18.098  | 0.037      | 0.034      | –50    | 22.8     | 2.6      | 0.2             | 29.2     | 1.8             | 2.19          | 0.04                 | PL  | T   | ...        | 1FGL J1730.4+0008<br>1FHL J1730.7+0017<br>2FGL J1730.7+0023 | ... | fsrq  | PKS 1728+004           |
| J1730.6+3711 | 262.662 | 37.190  | 61.821  | 31.360  | 0.082      | 0.080      | –21    | 7.7      | 0.5      | 0.1             | 5.0      | 0.8             | 2.09          | 0.11                 | PL  | ... | ...        | 2FGL J1731.3+3718<br>1FGL J1730.8+3716                      | ... | bll   | GB6 J1730+3714         |
| J1730.6–0357 | 262.665 | –3.952  | 19.804  | 15.966  | 0.079      | 0.070      | 33     | 8.3      | 1.3      | 0.2             | 6.4      | 1.3             | 2.17          | ...                  | LP  | ... | ...        | 2FGL J1730.6–0353<br>1FGL J1730.7–0352                      | ... | ...   | ...                    |
| J1731.8–3001 | 262.964 | –30.021 | 357.483 | 1.954   | 0.038      | 0.032      | 24     | 10.3     | 2.1      | 0.3             | 23.0     | 3.0             | 1.99          | 0.08                 | PL  | ... | ...        | 2FGL J1731.8–3004                                           | ... | bll   | NVSS<br>J173146–300309 |
| J1731.9+5428 | 262.985 | 54.482  | 82.193  | 33.156  | 0.502      | 0.334      | 46     | 7.1      | 0.2      | 0.1             | 6.1      | 0.8             | 2.90          | 0.12                 | PL  | ... | ...        | 1FGL J1732.0–2957<br>2FGL J1730.8+5427                      | ... | ...   | ...                    |
| J1732.4–2709 | 263.123 | –27.150 | 359.969 | 3.403   | 0.073      | 0.064      | –73    | 6.1      | 1.4      | 0.2             | 18.2     | 3.6             | 2.37          | 0.12                 | PL  | ... | ...        | 2FGL J1731.9–2703c                                          | ... | ...   | ...                    |
| J1732.5–3130 | 263.134 | –31.515 | 356.312 | 1.015   | 0.014      | 0.014      | –22    | 58.0     | 30.7     | 0.7             | 149.2    | 4.2             | 2.02          | ...                  | EC  | T   | ...        | 2FGL J1732.5–3131<br>1FGL J1732.5–3131<br>EGR J1732–3126    | ... | PSR   | LAT PSR J1732–3131     |
| J1732.5–5048 | 263.149 | –50.801 | 340.026 | –9.419  | 0.104      | 0.088      | –73    | 6.7      | 0.6      | 0.1             | 8.5      | 1.3             | 2.41          | 0.11                 | PL  | ... | ...        | ...                                                         | ... | PSR   | PSR J1732–5049         |
| J1732.7+5914 | 263.183 | 59.247  | 87.882  | 33.031  | 0.139      | 0.100      | –23    | 4.5      | 0.2      | 0.1             | 2.4      | 0.7             | 2.01          | 0.23                 | PL  | ... | ...        | ...                                                         | ... | ...   | ...                    |
| J1733.0–1305 | 263.256 | –13.086 | 12.025  | 10.813  | 0.029      | 0.027      | –76    | 36.8     | 5.6      | 0.3             | 61.6     | 2.5             | 2.35          | ...                  | LP  | T   | ...        | 2FGL J1733.1–1307<br>1FGL J1733.0–1308<br>3EG J1733–1313    | ... | FSRQ  | PKS 1730–13            |
| J1733.5–2811 | 263.383 | –28.194 | 359.217 | 2.642   | 0.069      | 0.055      | –90    | 5.2      | 1.3      | 0.2             | 17.6     | 4.3             | 2.45          | 0.13                 | PL  | ... | 4,5        | 2FGL J1733.4–2812c                                          | ... | ...   | ...                    |
| J1733.5–3941 | 263.385 | –39.699 | 349.554 | –3.610  | 0.074      | 0.062      | –60    | 6.5      | 1.0      | 0.2             | 11.9     | 2.3             | 2.23          | 0.16                 | PL  | ... | 3          | ...                                                         | ... | ...   | ...                    |
| J1733.8–6056 | 263.464 | –60.933 | 331.221 | –14.772 | 0.075      | 0.067      | 30     | 9.2      | 0.5      | 0.1             | 9.0      | 1.1             | 2.58          | 0.10                 | PL  | ... | 3          | ...                                                         | ... | ...   | ...                    |
| J1734.3+3858 | 263.586 | 38.978  | 64.040  | 31.010  | 0.033      | 0.032      | –0     | 34.7     | 2.3      | 0.1             | 28.6     | 1.2             | 2.31          | 0.03                 | PL  | T   | ...        | 2FGL J1734.3+3858<br>1FGL J1734.4+3859                      | ... | fsrq  | B2 1732+38A            |
| J1734.7–2930 | 263.695 | –29.507 | 358.260 | 1.701   | 0.096      | 0.085      | –2     | 9.0      | 3.4      | 0.4             | 21.0     | 3.2             | 2.25          | ...                  | LP  | ... | 3          | 3EG J1736–2908                                              | ... | ...   | ...                    |
| J1735.4–1118 | 263.862 | –11.309 | 13.887  | 11.225  | 0.045      | 0.040      | 73     | 7.7      | 0.9      | 0.2             | 10.2     | 1.9             | 2.16          | 0.14                 | PL  | ... | ...        | 1FHL J1735.3–1118<br>1FGL J1735.4–1118                      | ... | bcu   | PMN J1735–1117         |
| J1736.0–2701 | 264.019 | –27.020 | 0.511   | 2.802   | 0.085      | 0.081      | –12    | 8.3      | 2.5      | 0.4             | 18.1     | 2.8             | 2.40          | ...                  | LP  | ... | 3,4,5      | ...                                                         | ... | ...   | ...                    |
| J1736.0+2033 | 264.020 | 20.562  | 44.086  | 25.419  | 0.039      | 0.034      | –20    | 12.2     | 0.7      | 0.1             | 8.9      | 1.4             | 1.72          | 0.10                 | PL  | ... | ...        | 1FHL J1735.9+2033<br>2FGL J1735.9+2033<br>1FGL J1735.7+2031 | ... | bcu   | NVSS<br>J173605+203301 |

Table 1—Continued

| Name 3FGL     | R.A.    | Decl.   | $l$     | $b$     | $\theta_1$ | $\theta_2$ | $\phi$ | $\sigma$ | $F_{35}$ | $\Delta F_{35}$ | $S_{25}$ | $\Delta S_{25}$ | $\Gamma_{25}$ | $\Delta \Gamma_{25}$ | Mod | Var | Flags   | $\gamma$ -ray Assoc.                                                                            | TeV | Class | ID or Assoc.                |
|---------------|---------|---------|---------|---------|------------|------------|--------|----------|----------|-----------------|----------|-----------------|---------------|----------------------|-----|-----|---------|-------------------------------------------------------------------------------------------------|-----|-------|-----------------------------|
| J1736.2–4444  | 264.055 | –44.747 | 345.541 | –6.734  | 0.049      | 0.045      | –45    | 17.0     | 2.1      | 0.2             | 26.5     | 1.8             | 2.38          | 0.05                 | PL  | ... | 10      | 2FGL J1736.0–4443<br>1FGL J1735.9–4438                                                          | ... | glc   | NGC 6388                    |
| J1736.4+0634  | 264.124 | 6.568   | 30.273  | 19.642  | 0.211      | 0.193      | –13    | 9.4      | 0.6      | 0.1             | 12.2     | 1.4             | 2.73          | 0.10                 | PL  | T   | 3       | 2FGL J1736.6+0626<br>1FGL J1736.3+0628                                                          | ... | fsrq  | MG1 J173624+0632            |
| J1736.5–2839  | 264.132 | –28.654 | 359.185 | 1.839   | 0.149      | 0.115      | –32    | 8.9      | 3.0      | 0.5             | 20.9     | 2.5             | 2.54          | ...                  | LP  | ... | 12      | 3EG J1736–2908                                                                                  | ... | ...   | ...                         |
| J1737.3–3214c | 264.348 | –32.240 | 356.260 | –0.243  | 0.109      | 0.069      | 10     | 5.8      | 2.2      | 0.4             | 24.8     | 4.6             | 2.14          | 0.09                 | PL  | ... | 3,6     | 2FGL J1737.2–3213<br>1AGL J1736–3235                                                            | ... | spp   | ...                         |
| J1737.9–2511  | 264.476 | –25.186 | 2.283   | 3.437   | 0.163      | 0.130      | 21     | 10.7     | 2.1      | 0.4             | 27.7     | 3.1             | 2.58          | ...                  | LP  | ... | ...     | ...                                                                                             | ... | ...   | ...                         |
| J1739.0+8716  | 264.759 | 87.277  | 120.002 | 27.944  | 0.055      | 0.052      | –30    | 11.4     | 0.6      | 0.1             | 7.2      | 0.8             | 2.28          | 0.08                 | PL  | T   | ...     | 2FGL J1738.9+8716                                                                               | ... | bcu   | NVSS<br>J173722+871744      |
| J1739.4+4955  | 264.873 | 49.927  | 76.889  | 31.725  | 0.043      | 0.039      | 22     | 22.5     | 1.3      | 0.1             | 15.7     | 1.0             | 2.31          | 0.05                 | PL  | T   | ...     | 1FGL J1739.4+8717<br>1FHL J1739.3+4953<br>2FGL J1739.5+4955<br>EGR J1740+4946                   | ... | fsrq  | S4 1738+49                  |
| J1739.9–3124c | 264.990 | –31.403 | 357.259 | –0.258  | 0.087      | 0.058      | 48     | 5.1      | 2.2      | 0.4             | 26.3     | 5.4             | 2.29          | 0.09                 | PL  | ... | 3,4,5,6 | ...                                                                                             | ... | ...   | ...                         |
| J1740.3+5211  | 265.085 | 52.191  | 79.555  | 31.790  | 0.041      | 0.037      | –18    | 29.3     | 1.7      | 0.1             | 23.2     | 1.0             | 2.45          | 0.04                 | PL  | T   | ...     | 1FHL J1740.2+5211<br>2FGL J1740.2+5212<br>1FGL J1740.0+5209<br>3EG J1738+5203<br>EGR J1740+5213 | ... | fsrq  | 4C +51107<br>J174036+534623 |
| J1740.3+4736  | 265.086 | 47.608  | 74.204  | 31.327  | 0.075      | 0.066      | 27     | 6.2      | 0.3      | 0.1             | 3.4      | 0.7             | 1.95          | 0.17                 | PL  | ... | ...     | 2FGL J1740.3+4738                                                                               | ... | fsrq  | S4 1738+47                  |
| J1740.4+5347  | 265.103 | 53.784  | 81.427  | 31.887  | 0.087      | 0.073      | 21     | 6.0      | 0.3      | 0.1             | 3.4      | 0.7             | 2.02          | 0.17                 | PL  | ... | ...     | ...                                                                                             | ... | bcu   | NVSS<br>J174036+534623      |
| J1740.5–2843  | 265.125 | –28.717 | 359.597 | 1.069   | 0.065      | 0.054      | –4     | 15.1     | 6.4      | 0.6             | 67.4     | 6.1             | 2.49          | ...                  | LP  | ... | 3       | EGR J1740–2851                                                                                  | ... | ...   | ...                         |
| J1740.5–2726  | 265.134 | –27.450 | 0.677   | 1.733   | 0.092      | 0.083      | –50    | 12.8     | 3.9      | 0.4             | 38.8     | 4.2             | 2.57          | ...                  | LP  | ... | ...     | 2FGL J1739.6–2726                                                                               | ... | ...   | ...                         |
| J1740.5–2642  | 265.137 | –26.712 | 1.304   | 2.123   | 0.093      | 0.076      | –29    | 8.8      | 2.8      | 0.4             | 16.8     | 2.5             | 2.37          | ...                  | LP  | ... | 3       | ...                                                                                             | ... | ...   | ...                         |
| J1740.8–1933  | 265.213 | –19.565 | 7.432   | 5.827   | 0.108      | 0.086      | –24    | 4.3      | 0.7      | 0.2             | 8.2      | 2.2             | 2.21          | 0.17                 | PL  | ... | ...     | ...                                                                                             | ... | ...   | ...                         |
| J1740.8–6755  | 265.215 | –67.928 | 325.150 | –18.735 | 0.156      | 0.110      | –12    | 5.2      | 0.3      | 0.1             | 4.7      | 0.9             | 2.54          | 0.15                 | PL  | ... | 1       | 2FGL J1741.1–6750                                                                               | ... | ...   | ...                         |
| J1741.1–3053  | 265.290 | –30.894 | 357.827 | –0.206  | 0.117      | 0.105      | 22     | 11.4     | 7.1      | 0.7             | 42.3     | 5.0             | 2.28          | ...                  | LP  | ... | 3       | 2FGL J1740.4–3054c<br>0FGL J1741.4–3046                                                         | ... | snr   | MSH 17–39                   |
| J1741.4+0938  | 265.357 | 9.638   | 33.773  | 19.891  | 0.242      | 0.195      | 28     | 5.2      | 0.4      | 0.1             | 8.7      | 1.5             | 2.75          | 0.13                 | PL  | ... | ...     | ...                                                                                             | ... | ...   | ...                         |
| J1741.5+1351  | 265.385 | 13.855  | 37.881  | 21.633  | 0.125      | 0.112      | –4     | 5.5      | 0.5      | 0.1             | 5.7      | 1.1             | 2.23          | 0.12                 | PL  | ... | 3       | 2FGL J1741.0+1347                                                                               | ... | PSR   | PSR J1741+1351              |
| J1741.9–2539  | 265.476 | –25.662 | 2.357   | 2.418   | 0.048      | 0.039      | –40    | 7.3      | 1.6      | 0.3             | 18.6     | 3.3             | 2.21          | 0.12                 | PL  | ... | ...     | 1FHL J1741.9–2539                                                                               | ... | bcu   | NVSS<br>J174154–253743      |
| J1741.9–2054  | 265.491 | –20.914 | 6.415   | 4.899   | 0.022      | 0.022      | 82     | 67.5     | 16.0     | 0.4             | 118.3    | 2.8             | 2.31          | ...                  | EC  | ... | ...     | 2FGL J1742.0–2540c<br>0FGL J1742.1–2054<br>1FGL J1741.8–2101<br>2FGL J1741.9–2054               | ... | PSR   | LAT PSR J1741–2054          |



Table 1—Continued

| Name 3FGL     | R.A.    | Decl.   | $l$     | $b$     | $\theta_1$ | $\theta_2$ | $\phi$ | $\sigma$ | $F_{35}$ | $\Delta F_{35}$ | $S_{25}$ | $\Delta S_{25}$ | $\Gamma_{25}$ | $\Delta \Gamma_{25}$ | Mod | Var | Flags | $\gamma$ -ray Assoc.                                                            | TeV | Class | ID or Assoc.             |
|---------------|---------|---------|---------|---------|------------|------------|--------|----------|----------|-----------------|----------|-----------------|---------------|----------------------|-----|-----|-------|---------------------------------------------------------------------------------|-----|-------|--------------------------|
| J1742.2+5947  | 265.573 | 59.793  | 88.508  | 31.811  | 0.072      | 0.064      | -29    | 8.9      | 0.4      | 0.1             | 5.3      | 0.7             | 2.30          | 0.12                 | PL  | ... | ...   | 3EG J1741-2050<br>2FGL J1742.1+5948<br>1FGL J1742.1+5947                        | ... | bll   | RGB J1742+597            |
| J1742.4-7237  | 265.622 | -72.618 | 320.713 | -20.878 | 0.424      | 0.370      | 49     | 5.2      | 0.1      | 0.1             | 5.2      | 0.9             | 3.05          | 0.19                 | PL  | ... | 1     | ...                                                                             | ... | ...   | ...                      |
| J1742.6-3321  | 265.665 | -33.356 | 355.902 | -1.775  | 0.067      | 0.062      | -73    | 15.3     | 4.9      | 0.4             | 32.1     | 3.2             | 2.39          | ...                  | LP  | ... | ...   | 2FGL J1742.5-3323                                                               | ... | ...   | ...                      |
| J1743.9+1934  | 265.987 | 19.582  | 43.830  | 23.340  | 0.053      | 0.048      | 24     | 9.9      | 0.6      | 0.1             | 8.0      | 1.3             | 1.78          | 0.11                 | PL  | ... | ...   | 1FHL J1744.2+1938<br>2FGL J1744.1+1934<br>1FGL J1744.2+1934                     | P   | bll   | S3 1741+19               |
| J1743.9-1310  | 265.993 | -13.179 | 13.336  | 8.480   | 0.121      | 0.099      | -38    | 5.0      | 0.7      | 0.1             | 8.2      | 1.8             | 2.24          | 0.13                 | PL  | ... | ...   | ...                                                                             | ... | ...   | ...                      |
| J1744.1-7619  | 266.045 | -76.329 | 317.105 | -22.471 | 0.035      | 0.034      | -50    | 32.8     | 3.9      | 0.2             | 22.5     | 1.3             | 2.11          | ...                  | LP  | ... | ...   | 2FGL J1744.1-7620<br>1FGL J1743.8-7620                                          | ... | ...   | ...                      |
| J1744.3-0353  | 266.076 | -3.898  | 21.575  | 13.026  | 0.125      | 0.109      | 1      | 4.8      | 0.6      | 0.1             | 7.5      | 1.7             | 2.27          | 0.16                 | PL  | ... | ...   | 1FGL J1744.6-0354                                                               | ... | fsrq  | PKS 1741-03              |
| J1744.5-1133  | 266.134 | -11.554 | 14.825  | 9.184   | 0.043      | 0.040      | 37     | 27.6     | 5.3      | 0.3             | 39.2     | 2.2             | 2.32          | ...                  | EC  | ... | ...   | 2FGL J1744.6-1135<br>1FGL J1744.4-1134                                          | ... | PSR   | PSR J1744-1134           |
| J1744.5-2506  | 266.136 | -25.100 | 3.149   | 2.205   | 0.145      | 0.104      | -29    | 7.7      | 1.8      | 0.3             | 32.4     | 4.3             | 2.64          | 0.08                 | PL  | ... | 5     | ...                                                                             | ... | ...   | ...                      |
| J1744.7-3043  | 266.180 | -30.719 | 358.377 | -0.764  | 0.071      | 0.058      | 49     | 6.6      | 3.0      | 0.5             | 38.0     | 6.4             | 2.36          | 0.08                 | PL  | ... | 3,4,5 | 1AGL J1746-3017                                                                 | ... | ...   | ...                      |
| J1744.7-2252  | 266.181 | -22.869 | 5.076   | 3.333   | 0.256      | 0.210      | 75     | 10.1     | 1.0      | 0.2             | 20.0     | 2.2             | 2.54          | ...                  | LP  | ... | 12    | ...                                                                             | ... | ...   | ...                      |
| J1744.8-1557  | 266.215 | -15.959 | 11.034  | 6.876   | 0.195      | 0.133      | 78     | 4.8      | 0.7      | 0.2             | 10.0     | 2.0             | 2.43          | 0.13                 | PL  | ... | 3     | ...                                                                             | ... | ...   | ...                      |
| J1744.9-1725  | 266.248 | -17.433 | 9.777   | 6.093   | 0.037      | 0.037      | 76     | 11.8     | 1.6      | 0.2             | 17.5     | 2.1             | 2.08          | 0.09                 | PL  | ... | ...   | 2FGL J1745.1-1729                                                               | ... | bcu   | 1RXS<br>J174459.5-172640 |
| J1745.1-3011  | 266.297 | -30.199 | 358.874 | -0.579  | 0.068      | 0.049      | 46     | 13.7     | 9.6      | 0.8             | 84.1     | 8.4             | 2.44          | ...                  | LP  | ... | 3,5   | 3EG J1744-3011<br>1AGL J1746-3017                                               | E   | spp   | ...                      |
| J1745.3-2903c | 266.343 | -29.063 | 359.864 | -0.020  | 0.023      | 0.022      | 47     | 20.7     | 38.7     | 2.0             | 230.8    | 19.7            | 2.29          | ...                  | LP  | ... | 5,6,7 | ...                                                                             | ... | ...   | ...                      |
| J1745.4-0754  | 266.352 | -7.900  | 18.147  | 10.825  | 0.045      | 0.038      | -0     | 9.7      | 1.1      | 0.2             | 12.3     | 1.8             | 1.92          | 0.10                 | PL  | ... | ...   | 2FGL J1745.5-0751<br>1FGL J1745.6-0751                                          | ... | bll   | TXS 1742-078             |
| J1745.4+4721  | 266.373 | 47.351  | 74.042  | 30.431  | 0.209      | 0.156      | -71    | 5.8      | 0.3      | 0.1             | 5.0      | 0.8             | 2.56          | 0.14                 | PL  | ... | ...   | ...                                                                             | ... | ...   | ...                      |
| J1745.5+1017  | 266.379 | 10.284  | 34.851  | 19.258  | 0.068      | 0.061      | -48    | 13.6     | 1.6      | 0.2             | 10.6     | 1.5             | 2.26          | ...                  | EC  | ... | ...   | 2FGL J1745.6+1015<br>1FGL J1745.5+1018                                          | ... | PSR   | PSR J1745+1017           |
| J1745.6-2859c | 266.416 | -28.995 | 359.956 | -0.039  | 0.018      | 0.017      | -45    | 12.0     | 21.8     | 1.9             | 268.7    | 25.3            | 2.32          | 0.03                 | PL  | ... | 6,10  | 1FHL J1745.6-2900<br>2FGL J1745.6-2858<br>1FGL J1745.6-2900c                    | P   | spp   | ...                      |
| J1745.7+3952  | 266.439 | 39.867  | 65.572  | 29.038  | 0.084      | 0.059      | 50     | 5.3      | 0.2      | 0.1             | 2.6      | 0.8             | 1.69          | 0.32                 | PL  | ... | ...   | ...                                                                             | ... | bll   | B2 1743+39C              |
| J1746.3-2851c | 266.594 | -28.863 | 0.149   | -0.103  | 0.024      | 0.023      | 37     | 21.0     | 27.5     | 1.8             | 164.5    | 18.5            | 2.32          | ...                  | LP  | ... | 5,6   | 1FHL J1746.3-2851<br>2FGL J1746.6-2851c<br>1FGL J1746.4-2849c<br>3EG J1746-2851 | ... | pwn   | PWN G0.13-0.11           |

Table 1—Continued

| Name 3FGL     | R.A.    | Decl.   | $l$     | $b$     | $\theta_1$ | $\theta_2$ | $\phi$ | $\sigma$ | $F_{35}$ | $\Delta F_{35}$ | $S_{25}$ | $\Delta S_{25}$ | $\Gamma_{25}$ | $\Delta \Gamma_{25}$ | Mod | Var | Flags  | $\gamma$ -ray Assoc.                                                             | TeV | Class | ID or Assoc.       |
|---------------|---------|---------|---------|---------|------------|------------|--------|----------|----------|-----------------|----------|-----------------|---------------|----------------------|-----|-----|--------|----------------------------------------------------------------------------------|-----|-------|--------------------|
| J1746.6+0433  | 266.652 | 4.560   | 29.577  | 16.491  | 0.197      | 0.170      | −73    | 4.4      | 0.5      | 0.1             | 7.5      | 1.7             | 2.54          | 0.16                 | PL  | ... | ...    | ...                                                                              | ... | ...   | ...                |
| J1746.8−3240  | 266.706 | −32.669 | 356.945 | −2.160  | 0.035      | 0.034      | −47    | 26.4     | 8.6      | 0.4             | 70.2     | 4.2             | 2.37          | ...                  | EC  | ... | ...    | 2FGL J1746.5−3238                                                                | ... | PSR   | LAT PSR J1746−3239 |
| J1747.0−3506  | 266.756 | −35.107 | 354.877 | −3.457  | 0.091      | 0.074      | −22    | 11.7     | 1.5      | 0.2             | 27.9     | 2.5             | 2.67          | 0.07                 | PL  | ... | ...    | 2FGL J1747.2−3507                                                                | ... | ...   | ...                |
| J1747.0−2828  | 266.775 | −28.482 | 0.557   | −0.041  | 0.041      | 0.035      | −12    | 20.3     | 19.1     | 1.1             | 145.5    | 8.4             | 2.43          | ...                  | LP  | T   | 5,7    | ...                                                                              | ... | ...   | ...                |
| J1747.1+0139  | 266.785 | 1.655   | 26.959  | 15.039  | 0.255      | 0.241      | −13    | 5.0      | 0.5      | 0.1             | 9.0      | 1.7             | 2.64          | 0.15                 | PL  | ... | 3      | ...                                                                              | ... | bcu   | PMN J1746+0141     |
| J1747.2−2958  | 266.819 | −29.982 | 359.294 | −0.852  | 0.022      | 0.022      | 9      | 34.3     | 21.7     | 0.8             | 178.5    | 9.3             | 2.37          | ...                  | EC  | ... | ...    | 1AGL J1746−3017<br>1FGL J1747.2−2958<br>2FGL J1747.1−3000                        | ... | PSR   | PSR J1747−2958     |
| J1747.3+0324  | 266.846 | 3.413   | 28.606  | 15.797  | 0.139      | 0.089      | 87     | 6.2      | 0.7      | 0.1             | 9.2      | 1.7             | 2.35          | 0.13                 | PL  | ... | ...    | 2FGL J1747.6+0324                                                                | ... | ...   | ...                |
| J1747.6−4037  | 266.922 | −40.630 | 350.183 | −6.399  | 0.067      | 0.059      | −55    | 10.0     | 1.3      | 0.2             | 16.0     | 1.8             | 2.32          | 0.08                 | PL  | ... | ...    | 2FGL J1747.5−4036<br>1FGL J1747.4−4035                                           | ... | PSR   | PSR J1747−4036     |
| J1747.7−2904  | 266.943 | −29.075 | 0.126   | −0.474  | 0.069      | 0.060      | 87     | 7.0      | 5.6      | 0.8             | 84.3     | 14.9            | 2.52          | 0.08                 | PL  | ... | 5,7    | ...                                                                              | ... | ...   | ...                |
| J1748.0−2447  | 267.012 | −24.788 | 3.829   | 1.689   | 0.028      | 0.025      | −48    | 31.6     | 11.1     | 0.5             | 73.1     | 4.4             | 2.26          | ...                  | LP  | T   | ...    | 2FGL J1748.0−2447<br>1FGL J1747.9−2448                                           | E   | glc   | Terzan 5           |
| J1748.0+3405  | 267.014 | 34.090  | 59.346  | 27.182  | 0.068      | 0.058      | −11    | 10.8     | 0.6      | 0.1             | 7.5      | 0.9             | 2.39          | 0.10                 | PL  | ... | ...    | ...                                                                              | ... | fsrq  | MG2 J174803+3403   |
| J1748.0+2701  | 267.015 | 27.022  | 51.834  | 25.064  | 0.097      | 0.079      | −28    | 5.1      | 0.3      | 0.1             | 3.8      | 0.8             | 2.28          | 0.16                 | PL  | ... | 1      | ...                                                                              | ... | ...   | ...                |
| J1748.3−2815c | 267.092 | −28.259 | 0.893   | −0.165  | 0.030      | 0.029      | −42    | 15.1     | 8.2      | 0.9             | 42.3     | 3.4             | 2.19          | ...                  | LP  | ... | 3,6,12 | ...                                                                              | ... | ...   | ...                |
| J1748.5−3912  | 267.131 | −39.206 | 351.498 | −5.814  | 0.096      | 0.076      | 29     | 9.3      | 1.3      | 0.2             | 16.3     | 1.9             | 2.30          | 0.09                 | PL  | ... | 3      | ...                                                                              | ... | ...   | ...                |
| J1748.6+7005  | 267.169 | 70.097  | 100.524 | 30.709  | 0.017      | 0.016      | −37    | 52.7     | 4.1      | 0.1             | 46.0     | 1.6             | 2.06          | 0.02                 | PL  | T   | ...    | 1FHL J1748.5+7006<br>2FGL J1748.8+7006<br>1FGL J1748.5+7004                      | ... | bll   | S4 1749+70         |
| J1748.9−2021  | 267.236 | −20.354 | 7.742   | 3.791   | 0.073      | 0.068      | 85     | 15.1     | 2.3      | 0.2             | 41.3     | 3.0             | 2.64          | 0.06                 | PL  | ... | ...    | 2FGL J1748.7−2020<br>1FGL J1748.7−2020                                           | ... | glc   | NGC 6440           |
| J1749.1+4322  | 267.276 | 43.379  | 69.653  | 29.140  | 0.046      | 0.041      | −53    | 19.3     | 1.1      | 0.1             | 13.2     | 1.0             | 2.25          | 0.06                 | PL  | ... | ...    | 2FGL J1749.1+4323<br>1FGL J1749.0+4323                                           | ... | bll   | B3 1747+433        |
| J1749.2−2911  | 267.315 | −29.193 | 0.193   | −0.814  | 0.080      | 0.057      | 58     | 11.7     | 7.6      | 0.7             | 46.0     | 7.0             | 2.41          | ...                  | LP  | ... | 3,7    | ...                                                                              | ... | ...   | ...                |
| J1749.6−3133  | 267.422 | −31.552 | 358.215 | −2.105  | 0.126      | 0.118      | 15     | 7.3      | 2.3      | 0.4             | 18.8     | 3.2             | 2.48          | ...                  | LP  | ... | 1,4,5  | 2FGL J1749.7−3134c                                                               | ... | ...   | ...                |
| J1749.7−0305  | 267.448 | −3.086  | 22.979  | 12.217  | 0.088      | 0.077      | 40     | 7.4      | 0.9      | 0.2             | 12.8     | 1.9             | 2.43          | 0.12                 | PL  | ... | 3      | 1FGL J1749.5−0301                                                                | ... | ...   | ...                |
| J1750.2−3704  | 267.564 | −37.067 | 353.523 | −5.021  | 0.065      | 0.064      | −29    | 10.4     | 1.5      | 0.2             | 18.7     | 2.0             | 2.34          | 0.07                 | PL  | ... | ...    | ...                                                                              | ... | glc   | NGC 6441           |
| J1750.9−2220  | 267.743 | −22.345 | 6.270   | 2.368   | 0.134      | 0.121      | 9      | 4.3      | 0.9      | 0.2             | 13.0     | 3.3             | 2.46          | 0.16                 | PL  | ... | 4      | ...                                                                              | ... | ...   | ...                |
| J1751.5+0939  | 267.882 | 9.658   | 34.925  | 17.652  | 0.030      | 0.029      | 0      | 35.4     | 4.3      | 0.2             | 38.7     | 1.9             | 2.25          | ...                  | LP  | T   | ...    | 1FHL J1751.5+0938<br>2FGL J1751.5+0938<br>1FGL J1751.5+0937<br>0FGL J1751.5+0935 | ... | bll   | OT 081             |
| J1753.5−5010  | 268.386 | −50.170 | 342.279 | −11.988 | 0.126      | 0.096      | 1      | 8.7      | 0.7      | 0.1             | 10.4     | 1.3             | 2.51          | 0.10                 | PL  | T   | ...    | 2FGL J1753.8−5012                                                                | ... | bcu   | PMN J1753−5015     |

Table 1—Continued

| Name 3FGL     | R.A.    | Decl.   | $l$     | $b$     | $\theta_1$ | $\theta_2$ | $\phi$ | $\sigma$ | $F_{35}$ | $\Delta F_{35}$ | $S_{25}$ | $\Delta S_{25}$ | $\Gamma_{25}$ | $\Delta \Gamma_{25}$ | Mod | Var | Flags | $\gamma$ -ray Assoc. | TeV | Class            | ID or Assoc.    |
|---------------|---------|---------|---------|---------|------------|------------|--------|----------|----------|-----------------|----------|-----------------|---------------|----------------------|-----|-----|-------|----------------------|-----|------------------|-----------------|
|               |         |         |         |         |            |            |        |          |          |                 |          |                 |               |                      |     |     |       | 1FGL J1754.0–5002    |     |                  |                 |
| J1753.6–4447  | 268.404 | –44.793 | 347.085 | –9.416  | 0.080      | 0.063      | 68     | 11.1     | 1.4      | 0.2             | 9.4      | 1.3             | 2.14          | ...                  | LP  | ... | ...   | 2FGL J1753.8–4446    | ... | ...              | ...             |
| J1754.0–2930  | 268.500 | –29.506 | 0.451   | –1.862  | 0.108      | 0.083      | 14     | 15.0     | 4.1      | 0.4             | 41.5     | 4.2             | 2.54          | ...                  | LP  | ... | 3     | 2FGL J1754.1–2930    | ... | ...              | ...             |
| J1754.0–2538  | 268.508 | –25.649 | 3.781   | 0.085   | 0.029      | 0.027      | –87    | 16.8     | 7.7      | 0.6             | 41.7     | 3.7             | 2.08          | ...                  | LP  | ... | 3     | 2FGL J1754.4–2538c   | ... | ...              | ...             |
|               |         |         |         |         |            |            |        |          |          |                 |          |                 |               |                      |     |     |       | 1FGL J1754.5–2537c   |     |                  |                 |
| J1754.0–3321  | 268.518 | –33.363 | 357.124 | –3.822  | 0.133      | 0.115      | –83    | 6.3      | 1.1      | 0.2             | 15.3     | 2.5             | 2.41          | 0.10                 | PL  | ... | 4     | ...                  | ... | ...              | ...             |
| J1754.1+3212  | 268.546 | 32.208  | 57.741  | 25.417  | 0.021      | 0.020      | –79    | 41.6     | 3.4      | 0.2             | 39.5     | 2.1             | 1.90          | 0.03                 | PL  | T   | ...   | 1FHL J1754.2+3213    | ... | bll              | RX J1754.1+3212 |
|               |         |         |         |         |            |            |        |          |          |                 |          |                 |               |                      |     |     |       | 2FGL J1754.3+3212    |     |                  |                 |
|               |         |         |         |         |            |            |        |          |          |                 |          |                 |               |                      |     |     |       | 1FGL J1754.3+3212    |     |                  |                 |
| J1754.3–6424  | 268.579 | –64.405 | 329.121 | –18.445 | 0.116      | 0.096      | 68     | 7.2      | 0.4      | 0.1             | 6.2      | 1.0             | 2.46          | 0.12                 | PL  | ... | ...   | 2FGL J1755.5–6423    | ... | bll              | PMN J1754–6423  |
| J1756.3+5523  | 269.077 | 55.389  | 83.498  | 29.717  | 0.040      | 0.037      | 62     | 10.1     | 0.4      | 0.1             | 4.9      | 0.8             | 1.98          | 0.13                 | PL  | ... | ...   | 1FHL J1756.5+5523    | ... | bll              | 1RXS            |
|               |         |         |         |         |            |            |        |          |          |                 |          |                 |               |                      |     |     |       |                      |     | J175615.5+552217 |                 |
|               |         |         |         |         |            |            |        |          |          |                 |          |                 |               |                      |     |     |       | 2FGL J1756.5+5523    |     |                  |                 |
|               |         |         |         |         |            |            |        |          |          |                 |          |                 |               |                      |     |     |       | 1FGL J1756.6+5524    |     |                  |                 |
| J1756.9+7032  | 269.246 | 70.549  | 100.992 | 29.981  | 0.076      | 0.054      | 31     | 5.5      | 0.2      | 0.1             | 2.4      | 0.7             | 1.71          | 0.24                 | PL  | ... | ...   | ...                  | ... | bll              | MS 1757.7+7034  |
| J1757.1+1533  | 269.290 | 15.560  | 41.175  | 18.873  | 0.232      | 0.136      | 20     | 4.5      | 0.4      | 0.1             | 4.3      | 1.0             | 2.04          | 0.15                 | PL  | ... | ...   | ...                  | ... | bcu              | 87GB 10         |
|               |         |         |         |         |            |            |        |          |          |                 |          |                 |               |                      |     |     |       |                      |     |                  | 175437.6+153548 |
| J1757.4+6536  | 269.361 | 65.602  | 95.278  | 30.071  | 0.061      | 0.054      | –3     | 5.1      | 0.2      | 0.1             | 2.7      | 0.7             | 2.32          | 0.19                 | PL  | ... | ...   | ...                  | ... | bcu              | 7C 1757+6536    |
| J1757.7–6030  | 269.428 | –60.506 | 333.011 | –17.165 | 0.063      | 0.056      | 90     | 9.6      | 0.6      | 0.1             | 3.6      | 0.6             | 1.96          | ...                  | LP  | ... | ...   | 2FGL J1757.5–6028    | ... | ...              | ...             |
| J1757.8–3126  | 269.470 | –31.446 | 359.190 | –3.558  | 0.116      | 0.103      | –9     | 6.0      | 1.2      | 0.2             | 15.8     | 2.7             | 2.42          | 0.10                 | PL  | ... | 4     | ...                  | ... | ...              | ...             |
| J1758.8–2402  | 269.705 | –24.037 | 5.720   | –0.043  | 0.077      | 0.071      | –34    | 5.3      | 2.3      | 0.5             | 25.6     | 5.6             | 1.99          | 0.10                 | PL  | ... | 3,5   | 2FGL J1758.8–2402c   | ... | ...              | ...             |
| J1758.8–2346  | 269.707 | –23.783 | 5.941   | 0.081   | 0.057      | 0.053      | 71     | 7.3      | 3.3      | 0.6             | 36.7     | 6.4             | 2.08          | 0.08                 | PL  | ... | 5     | ...                  | ... | ...              | ...             |
| J1758.8–4108  | 269.713 | –41.136 | 350.793 | –8.483  | 0.068      | 0.064      | 12     | 6.4      | 0.7      | 0.1             | 7.4      | 1.4             | 2.10          | 0.12                 | PL  | ... | ...   | ...                  | ... | ...              | ...             |
| J1759.1–4822  | 269.795 | –48.372 | 344.343 | –11.958 | 0.060      | 0.054      | 15     | 12.8     | 1.2      | 0.1             | 14.0     | 1.4             | 2.30          | 0.08                 | PL  | T   | ...   | 2FGL J1759.2–4819    | ... | bcu              | PMN J1758–4820  |
| J1759.2–3848  | 269.814 | –38.811 | 352.887 | –7.427  | 0.117      | 0.096      | –58    | 5.7      | 0.8      | 0.1             | 8.9      | 1.7             | 2.24          | 0.12                 | PL  | ... | ...   | 2FGL J1759.2–3853    | ... | ...              | ...             |
|               |         |         |         |         |            |            |        |          |          |                 |          |                 |               |                      |     |     |       | EGR J1758–3923       |     |                  |                 |
| J1759.6–2141  | 269.910 | –21.692 | 7.848   | 0.961   | 0.071      | 0.052      | –19    | 5.2      | 1.6      | 0.3             | 19.4     | 4.2             | 2.29          | 0.11                 | PL  | ... | 1     | ...                  | ... | ...              | ...             |
| J1800.0–2955  | 270.023 | –29.926 | 0.748   | –3.217  | 0.116      | 0.103      | 64     | 5.6      | 1.0      | 0.2             | 19.1     | 3.4             | 2.66          | 0.10                 | PL  | ... | ...   | 2FGL J1759.4–2954    | ... | ...              | ...             |
| J1800.5+7827  | 270.131 | 78.462  | 110.033 | 29.078  | 0.017      | 0.017      | 16     | 74.5     | 5.1      | 0.2             | 58.6     | 1.5             | 2.22          | 0.02                 | PL  | T   | ...   | 1FHL J1800.5+7829    | ... | bll              | S5 1803+784     |
|               |         |         |         |         |            |            |        |          |          |                 |          |                 |               |                      |     |     |       | 2FGL J1800.5+7829    |     |                  |                 |
|               |         |         |         |         |            |            |        |          |          |                 |          |                 |               |                      |     |     |       | 1FGL J1800.4+7827    |     |                  |                 |
|               |         |         |         |         |            |            |        |          |          |                 |          |                 |               |                      |     |     |       | 0FGL J1802.2+7827    |     |                  |                 |
| J1800.8–2402  | 270.222 | –24.035 | 5.956   | –0.452  | 0.035      | 0.034      | –3     | 17.5     | 10.3     | 0.8             | 73.3     | 6.8             | 2.12          | ...                  | LP  | ... | ...   | 2FGL J1800.8–2400    | E   | ...              | ...             |
|               |         |         |         |         |            |            |        |          |          |                 |          |                 |               |                      |     |     |       | 1FGL J1800.5–2359c   |     |                  |                 |
| J1801.3–2326e | 270.340 | –23.440 | 6.527   | –0.251  | ...        | ...        | ...    | 62.7     | 53.5     | 1.0             | 415.5    | 9.1             | 2.15          | ...                  | LP  | T   | ...   | 0FGL J1801.6–2327    | E   | SNR              | W28             |
|               |         |         |         |         |            |            |        |          |          |                 |          |                 |               |                      |     |     |       | 1FGL J1801.3–2322c   |     |                  |                 |
|               |         |         |         |         |            |            |        |          |          |                 |          |                 |               |                      |     |     |       | 1FHL J1801.3–2326e   |     |                  |                 |

Table 1—Continued

| Name 3FGL     | R.A.    | Decl.   | $l$     | $b$     | $\theta_1$ | $\theta_2$ | $\phi$ | $\sigma$ | $F_{35}$ | $\Delta F_{35}$ | $S_{25}$ | $\Delta S_{25}$ | $\Gamma_{25}$ | $\Delta \Gamma_{25}$ | Mod | Var | Flags | $\gamma$ -ray Assoc.                                                                                                 | TeV | Class | ID or Assoc.       |
|---------------|---------|---------|---------|---------|------------|------------|--------|----------|----------|-----------------|----------|-----------------|---------------|----------------------|-----|-----|-------|----------------------------------------------------------------------------------------------------------------------|-----|-------|--------------------|
|               |         |         |         |         |            |            |        |          |          |                 |          |                 |               |                      |     |     |       | 2FGL J1801.3–2326e<br>3EG J1800–2338<br>EGR J1800–2328                                                               |     |       |                    |
| J1801.5–7825  | 270.388 | −78.424 | 315.325 | −24.088 | 0.162      | 0.156      | −35    | 8.7      | 0.4      | 0.1             | 8.8      | 1.1             | 2.75          | 0.12                 | PL  | T   | ...   | ...                                                                                                                  | ... | ...   | ...                |
| J1801.5+4403  | 270.397 | 44.053  | 70.924  | 27.070  | 0.119      | 0.100      | −52    | 12.1     | 0.5      | 0.1             | 9.3      | 0.8             | 2.70          | 0.09                 | PL  | T   | ...   | 2FGL J1801.7+4405                                                                                                    | ... | fsrq  | S4 1800+44         |
| J1801.6–2213  | 270.400 | −22.220 | 7.615   | 0.304   | 0.055      | 0.040      | −27    | 5.1      | 1.5      | 0.4             | 16.5     | 4.2             | 1.97          | 0.15                 | PL  | ... | 3     | ...                                                                                                                  | ... | ...   | ...                |
| J1802.4–3043  | 270.614 | −30.724 | 0.304   | −4.054  | 0.082      | 0.060      | 84     | 6.0      | 1.0      | 0.2             | 10.8     | 2.1             | 2.11          | 0.12                 | PL  | ... | ...   | ...                                                                                                                  | ... | ...   | ...                |
| J1802.6–3940  | 270.673 | −39.674 | 352.445 | −8.425  | 0.018      | 0.017      | 73     | 63.6     | 10.1     | 0.3             | 99.8     | 2.8             | 2.27          | ...                  | LP  | T   | ...   | 1FHL J1802.7–3940<br>2FGL J1802.6–3940<br>1FGL J1802.5–3939<br>0FGL J1802.6–3939<br>3EG J1800–3955<br>EGR J1758–3923 | ... | fsrq  | PMN J1802–3940     |
| J1803.1–2147  | 270.783 | −21.787 | 8.166   | 0.210   | 0.027      | 0.025      | −48    | 23.9     | 14.0     | 0.8             | 90.1     | 6.7             | 2.18          | ...                  | EC  | ... | ...   | 2FGL J1803.3–2148<br>1FGL J1803.1–2147c<br>1AGL J1805–2143                                                           | ... | PSR   | LAT PSR J1803–2149 |
| J1803.1–2728  | 270.786 | −27.467 | 3.221   | −2.587  | 0.110      | 0.075      | −4     | 5.9      | 1.2      | 0.2             | 14.5     | 2.7             | 2.34          | 0.11                 | PL  | ... | 1     | ...                                                                                                                  | ... | ...   | ...                |
| J1803.3–6706  | 270.843 | −67.116 | 326.868 | −20.368 | 0.076      | 0.060      | 2      | 10.5     | 0.7      | 0.1             | 8.2      | 1.0             | 2.22          | 0.09                 | PL  | ... | ...   | 2FGL J1802.8–6706                                                                                                    | ... | ...   | ...                |
| J1804.1+0341  | 271.034 | 3.697   | 30.830  | 12.204  | 0.121      | 0.108      | −65    | 4.5      | 0.5      | 0.1             | 5.5      | 1.3             | 2.26          | 0.17                 | PL  | ... | 3     | 1FGL J1804.1+0336                                                                                                    | ... | fsrq  | TXS 1801+036       |
| J1804.1+2532  | 271.039 | 25.543  | 51.664  | 21.168  | 0.162      | 0.154      | −55    | 6.1      | 0.3      | 0.1             | 6.5      | 1.0             | 2.71          | 0.12                 | PL  | ... | ...   | 2FGL J1803.6+2523c                                                                                                   | ... | ...   | ...                |
| J1804.5–0850  | 271.130 | −8.842  | 19.650  | 6.239   | 0.107      | 0.090      | 72     | 8.1      | 1.0      | 0.2             | 19.9     | 2.4             | 2.75          | 0.12                 | PL  | ... | 4     | ...                                                                                                                  | ... | ...   | ...                |
| J1805.6–2136e | 271.408 | −21.612 | 8.604   | −0.211  | ...        | ...        | ...    | 33.2     | 24.2     | 0.9             | 204.4    | 8.6             | 2.07          | ...                  | LP  | T   | ...   | 0FGL J1805.3–2138<br>1AGL J1805–2143<br>1FGL J1805.2–2137c<br>1FHL J1805.6–2136e<br>2FGL J1805.6–2136e               | E   | SNR   | W30                |
| J1805.9+0614  | 271.478 | 6.238   | 33.359  | 12.951  | 0.086      | 0.070      | −50    | 9.3      | 1.1      | 0.2             | 5.5      | 1.0             | 2.08          | ...                  | LP  | ... | ...   | 2FGL J1805.8+0612<br>1FGL J1806.2+0609                                                                               | ... | psr   | PSR J1805+06       |
| J1805.9+3407  | 271.479 | 34.125  | 60.562  | 23.652  | 0.183      | 0.172      | 83     | 4.6      | 0.3      | 0.1             | 4.6      | 1.0             | 2.60          | 0.16                 | PL  | ... | ...   | ...                                                                                                                  | ... | ...   | ...                |
| J1806.2+2744  | 271.555 | 27.749  | 54.056  | 21.512  | 0.292      | 0.248      | −32    | 4.3      | 0.3      | 0.1             | 4.6      | 1.0             | 2.47          | 0.14                 | PL  | ... | ...   | ...                                                                                                                  | ... | ...   | ...                |
| J1806.7–2451  | 271.681 | −24.855 | 5.895   | −2.012  | 0.089      | 0.069      | 39     | 4.2      | 1.0      | 0.3             | 11.0     | 3.2             | 2.21          | 0.14                 | PL  | ... | 4     | ...                                                                                                                  | ... | ...   | ...                |
| J1806.7+6949  | 271.681 | 69.818  | 100.124 | 29.177  | 0.022      | 0.021      | 79     | 46.1     | 3.3      | 0.1             | 39.0     | 1.3             | 2.23          | 0.03                 | PL  | T   | ...   | 1FHL J1806.3+6948<br>2FGL J1806.7+6948<br>1FGL J1807.0+6945                                                          | ... | bll   | 3C 371             |
| J1806.8+5346  | 271.724 | 53.781  | 81.891  | 27.997  | 0.150      | 0.121      | −65    | 5.2      | 0.3      | 0.1             | 4.4      | 0.8             | 2.56          | 0.14                 | PL  | ... | ...   | ...                                                                                                                  | ... | ...   | ...                |

Table 1—Continued

| Name 3FGL     | R.A.    | Decl.   | $l$     | $b$     | $\theta_1$ | $\theta_2$ | $\phi$ | $\sigma$ | $F_{35}$ | $\Delta F_{35}$ | $S_{25}$ | $\Delta S_{25}$ | $\Gamma_{25}$ | $\Delta \Gamma_{25}$ | Mod | Var | Flags | $\gamma$ -ray Assoc.                                                                             | TeV | Class | ID or Assoc.            |
|---------------|---------|---------|---------|---------|------------|------------|--------|----------|----------|-----------------|----------|-----------------|---------------|----------------------|-----|-----|-------|--------------------------------------------------------------------------------------------------|-----|-------|-------------------------|
| J1807.5–4343  | 271.888 | –43.719 | 349.242 | –11.112 | 0.147      | 0.122      | –2     | 4.9      | 0.5      | 0.1             | 5.6      | 1.2             | 2.12          | 0.14                 | PL  | ... | ...   | 1FGL J1807.6–4341                                                                                | ... | glc   | NGC 6541                |
| J1807.8+6427  | 271.951 | 64.455  | 93.993  | 28.949  | 0.068      | 0.065      | –43    | 5.8      | 0.2      | 0.1             | 2.8      | 0.6             | 2.09          | 0.17                 | PL  | ... | ...   | ...                                                                                              | ... | bcu   | 7C 1807+6428            |
| J1807.8–5011  | 271.954 | –50.184 | 343.331 | –14.030 | 0.150      | 0.109      | 74     | 4.5      | 0.4      | 0.1             | 5.0      | 1.2             | 2.42          | 0.18                 | PL  | ... | ...   | 3EG J1806–5005                                                                                   | ... | fsrq  | PMN J1808–5011          |
| J1808.0+4652  | 272.010 | 46.868  | 74.277  | 26.570  | 0.076      | 0.068      | 7      | 4.9      | 0.2      | 0.1             | 2.4      | 0.7             | 1.73          | 0.20                 | PL  | ... | ...   | ...                                                                                              | ... | bll   | RGB J1808+468           |
| J1808.3–3357  | 272.097 | –33.963 | 358.060 | –6.713  | 0.092      | 0.080      | 42     | 8.7      | 1.5      | 0.2             | 8.7      | 1.4             | 2.26          | ...                  | LP  | ... | ...   | 2FGL J1808.3–3356                                                                                | ... | ...   | ...                     |
| J1808.4–3519  | 272.101 | –35.329 | 356.850 | –7.363  | 0.096      | 0.094      | –82    | 4.9      | 0.6      | 0.1             | 7.3      | 1.5             | 2.31          | 0.12                 | PL  | ... | ...   | ...                                                                                              | ... | ...   | ...                     |
| J1808.4–3703  | 272.124 | –37.051 | 355.325 | –8.188  | 0.127      | 0.095      | 32     | 4.5      | 0.5      | 0.1             | 5.8      | 1.3             | 2.19          | 0.14                 | PL  | ... | ...   | ...                                                                                              | ... | ...   | ...                     |
| J1808.5–1952  | 272.141 | –19.872 | 10.457  | 0.038   | 0.070      | 0.058      | 74     | 8.8      | 5.5      | 0.6             | 44.4     | 6.9             | 2.31          | ...                  | LP  | ... | 3,4   | 2FGL J1808.6–1950c<br>1FGL J1808.5–1954c                                                         | ... | glc   | 2MS–GC01                |
| J1809.0+3517  | 272.273 | 35.285  | 61.984  | 23.382  | 0.094      | 0.087      | 32     | 5.4      | 0.3      | 0.1             | 4.4      | 1.0             | 2.44          | 0.17                 | PL  | ... | ...   | ...                                                                                              | ... | ...   | ...                     |
| J1809.2–2725  | 272.315 | –27.428 | 3.916   | –3.755  | 0.133      | 0.099      | –47    | 4.6      | 0.8      | 0.2             | 9.8      | 2.3             | 2.31          | 0.13                 | PL  | ... | 4     | ...                                                                                              | ... | ...   | ...                     |
| J1809.2–2016c | 272.324 | –20.282 | 10.182  | –0.311  | 0.056      | 0.046      | 17     | 5.4      | 2.6      | 0.5             | 32.1     | 7.1             | 2.33          | 0.10                 | PL  | ... | 4,6   | ...                                                                                              | ... | ...   | ...                     |
| J1809.4+2040  | 272.356 | 20.678  | 47.350  | 18.228  | 0.054      | 0.048      | –1     | 6.7      | 0.4      | 0.1             | 4.2      | 1.0             | 1.88          | 0.22                 | PL  | ... | ...   | 1FHL J1809.3+2040<br>2FGL J1809.4+2042                                                           | ... | bll   | RX J1809.3+2041         |
| J1809.7+2909  | 272.432 | 29.158  | 55.761  | 21.274  | 0.038      | 0.033      | 81     | 16.3     | 1.1      | 0.1             | 13.2     | 1.4             | 1.91          | 0.07                 | PL  | ... | ...   | 1FHL J1809.6+2910<br>2FGL J1809.7+2909<br>1FGL J1809.6+2908                                      | ... | bll   | MG2 J180948+2910        |
| J1809.8–2332  | 272.463 | –23.544 | 7.388   | –2.001  | 0.009      | 0.009      | 45     | 129.5    | 63.8     | 0.8             | 448.0    | 6.1             | 2.12          | ...                  | EC  | ... | ...   | 1FHL J1809.8–2329<br>2FGL J1809.8–2332<br>1FGL J1809.8–2332<br>3EG J1809–2328<br>1AGL J1809–2332 | ... | PSR   | PSR J1809–2332          |
| J1810.1–1910  | 272.545 | –19.168 | 11.258  | 0.046   | 0.108      | 0.086      | 42     | 5.1      | 2.1      | 0.6             | 23.7     | 6.4             | 2.10          | 0.15                 | PL  | ... | 3,5   | ...                                                                                              | E   | spp   | ...                     |
| J1810.5+1743  | 272.644 | 17.720  | 44.616  | 16.806  | 0.047      | 0.046      | –40    | 24.0     | 2.5      | 0.2             | 22.4     | 1.4             | 2.34          | ...                  | EC  | ... | ...   | 2FGL J1810.7+1742<br>1FGL J1810.3+1741                                                           | ... | PSR   | PSR J1810+1744          |
| J1810.7+5335  | 272.683 | 53.589  | 81.777  | 27.406  | 0.099      | 0.077      | 6      | 5.6      | 0.2      | 0.1             | 3.1      | 0.8             | 1.78          | 0.18                 | PL  | ... | ...   | 2FGL J1811.0+5340                                                                                | ... | ...   | ...                     |
| J1810.8–2412  | 272.715 | –24.212 | 6.913   | –2.525  | 0.107      | 0.065      | 71     | 6.2      | 1.8      | 0.3             | 21.8     | 4.3             | 2.32          | 0.10                 | PL  | ... | 1,5   | 2FGL J1811.3–2421                                                                                | ... | ...   | ...                     |
| J1810.8+1609  | 272.720 | 16.153  | 43.154  | 16.102  | 0.075      | 0.065      | 53     | 9.4      | 0.9      | 0.1             | 9.8      | 1.3             | 2.11          | 0.09                 | PL  | ... | ...   | 2FGL J1810.8+1606                                                                                | ... | bll   | 87GB<br>180835.5+160714 |
| J1811.2+0340  | 272.818 | 3.679   | 31.636  | 10.610  | 0.036      | 0.034      | –33    | 11.2     | 0.8      | 0.1             | 10.4     | 1.6             | 1.71          | 0.09                 | PL  | ... | 3     | 1FGL J1811.0+1607<br>2FGL J1811.3+0339                                                           | ... | bll   | NVSS<br>J181118+034113  |
| J1811.3–1927c | 272.827 | –19.457 | 11.133  | –0.327  | 0.119      | 0.114      | 0      | 4.4      | 2.1      | 0.5             | 25.0     | 6.6             | 2.24          | 0.12                 | PL  | ... | 6,9   | ...                                                                                              | ... | spp   | ...                     |
| J1813.4–1246  | 273.350 | –12.770 | 17.243  | 2.442   | 0.016      | 0.015      | 44     | 76.2     | 27.3     | 0.6             | 265.4    | 5.8             | 2.40          | ...                  | EC  | ... | ...   | 2FGL J1813.4–1246<br>1FGL J1813.3–1246<br>0FGL J1813.5–1248                                      | ... | PSR   | LAT PSR J1813–1246      |

Table 1—Continued

| Name 3FGL     | R.A.    | Decl.   | $l$     | $b$     | $\theta_1$ | $\theta_2$ | $\phi$ | $\sigma$ | $F_{35}$ | $\Delta F_{35}$ | $S_{25}$ | $\Delta S_{25}$ | $\Gamma_{25}$ | $\Delta \Gamma_{25}$ | Mod | Var | Flags    | $\gamma$ -ray Assoc.                                                             | TeV | Class | ID or Assoc.           |
|---------------|---------|---------|---------|---------|------------|------------|--------|----------|----------|-----------------|----------|-----------------|---------------|----------------------|-----|-----|----------|----------------------------------------------------------------------------------|-----|-------|------------------------|
| J1813.6+0614  | 273.410 | 6.245   | 34.240  | 11.236  | 0.041      | 0.038      | −4     | 11.0     | 0.9      | 0.1             | 10.4     | 1.5             | 1.88          | 0.09                 | PL  | T   | ...      | 2FGL J1813.7+0617                                                                | ... | bll   | TXS 1811+062           |
| J1813.6+3143  | 273.413 | 31.732  | 58.669  | 21.350  | 0.048      | 0.045      | 54     | 17.8     | 1.5      | 0.1             | 11.3     | 1.1             | 2.12          | ...                  | LP  | ... | ...      | 1FHL J1813.4+3145<br>2FGL J1813.5+3143<br>1FGL J1813.4+3141                      | ... | bll   | B2 1811+31             |
| J1813.6−6845  | 273.413 | −68.763 | 325.573 | −21.846 | 0.138      | 0.113      | −89    | 4.7      | 0.3      | 0.1             | 4.2      | 0.9             | 2.38          | 0.14                 | PL  | ... | ...      | ...                                                                              | ... | ...   | ...                    |
| J1813.6+2820  | 273.421 | 28.336  | 55.261  | 20.175  | 0.125      | 0.094      | 75     | 5.1      | 0.4      | 0.1             | 4.2      | 0.9             | 2.21          | 0.16                 | PL  | ... | ...      | ...                                                                              | ... | ...   | ...                    |
| J1813.6−1148  | 273.423 | −11.808 | 18.122  | 2.838   | 0.144      | 0.116      | 21     | 11.8     | 1.2      | 0.2             | 48.1     | 4.8             | 2.68          | ...                  | LP  | ... | 3,5,9,12 | 2FGL J1813.7−1139c                                                               | ... | ...   | ...                    |
| J1814.0−1757c | 273.514 | −17.961 | 12.757  | −0.180  | 0.097      | 0.061      | −86    | 5.4      | 2.8      | 0.6             | 31.3     | 7.5             | 2.18          | 0.12                 | PL  | ... | 6        | 1AGL J1815−1732                                                                  | ... | ...   | ...                    |
| J1814.1−1734c | 273.545 | −17.582 | 13.105  | −0.024  | 0.070      | 0.053      | −64    | 9.0      | 5.3      | 0.6             | 82.0     | 8.8             | 2.55          | 0.05                 | PL  | ... | 6,7      | 2FGL J1814.1−1735c<br>1FGL J1814.0−1736c<br>0FGL J1814.3−1739<br>1AGL J1815−1732 | ... | ...   | ...                    |
| J1815.1+5919  | 273.794 | 59.326  | 88.279  | 27.627  | 0.213      | 0.157      | 42     | 6.2      | 0.3      | 0.1             | 5.1      | 0.8             | 2.69          | 0.12                 | PL  | ... | ...      | ...                                                                              | ... | ...   | ...                    |
| J1816.0−6407  | 274.002 | −64.133 | 330.337 | −20.519 | 0.123      | 0.094      | −16    | 9.9      | 0.6      | 0.1             | 8.9      | 1.0             | 2.54          | 0.09                 | PL  | ... | ...      | 2FGL J1815.6−6407<br>3EG J1813−6419<br>EGR J1814−6423                            | ... | ...   | ...                    |
| J1816.2−2726  | 274.059 | −27.446 | 4.637   | −5.125  | 0.134      | 0.093      | −66    | 7.3      | 1.0      | 0.2             | 13.7     | 2.0             | 2.42          | 0.10                 | PL  | ... | ...      | ...                                                                              | ... | ...   | ...                    |
| J1816.5−1145  | 274.126 | −11.765 | 18.488  | 2.253   | 0.104      | 0.081      | −51    | 5.9      | 1.6      | 0.3             | 23.6     | 5.2             | 2.48          | 0.13                 | PL  | ... | 1,4      | ...                                                                              | ... | ...   | ...                    |
| J1816.5+4512  | 274.132 | 45.201  | 72.854  | 24.754  | 0.045      | 0.043      | −84    | 22.1     | 1.7      | 0.1             | 12.1     | 0.9             | 2.15          | ...                  | EC  | ... | ...      | 2FGL J1816.5+4511<br>1FGL J1816.7+4509                                           | ... | PSR   | PSR J1816+4510         |
| J1816.9−4944  | 274.233 | −49.745 | 344.382 | −15.173 | 0.086      | 0.073      | 78     | 9.7      | 1.0      | 0.1             | 5.2      | 0.8             | 2.21          | ...                  | LP  | T   | 3        | 2FGL J1816.7−4942                                                                | ... | bcu   | PMN J1816−4943         |
| J1817.2−1739  | 274.304 | −17.651 | 13.389  | −0.693  | 0.057      | 0.048      | 56     | 6.4      | 2.5      | 0.4             | 29.4     | 5.5             | 2.27          | 0.10                 | PL  | ... | 1        | 1AGL J1815−1732                                                                  | ... | spp   | ...                    |
| J1817.3−3033  | 274.342 | −30.552 | 1.991   | −6.793  | 0.095      | 0.089      | −84    | 4.3      | 0.5      | 0.1             | 6.2      | 1.6             | 2.18          | 0.16                 | PL  | ... | 4        | ...                                                                              | ... | ...   | ...                    |
| J1817.7+2530  | 274.434 | 25.505  | 52.816  | 18.302  | 0.246      | 0.199      | 15     | 4.7      | 0.3      | 0.1             | 5.5      | 1.1             | 2.59          | 0.14                 | PL  | ... | ...      | 1FGL J1817.0+2519                                                                | ... | ...   | ...                    |
| J1818.5+1320  | 274.633 | 13.337  | 41.310  | 13.244  | 0.205      | 0.112      | 81     | 4.2      | 0.4      | 0.1             | 4.4      | 1.1             | 2.01          | 0.16                 | PL  | ... | ...      | ...                                                                              | ... | ...   | ...                    |
| J1818.6+0903  | 274.655 | 9.061   | 37.373  | 11.375  | 0.060      | 0.052      | 85     | 13.7     | 1.4      | 0.1             | 17.9     | 1.6             | 2.37          | 0.07                 | PL  | T   | ...      | 2FGL J1818.6+0903<br>1FGL J1818.1+0905                                           | ... | fsrq  | MG1 J181841+0903       |
| J1818.7−1528  | 274.696 | −15.470 | 15.487  | 0.010   | 0.092      | 0.069      | 65     | 13.3     | 7.5      | 0.7             | 65.2     | 7.4             | 2.42          | ...                  | LP  | T   | 7        | ...                                                                              | ... | spp   | ...                    |
| J1819.1+2134  | 274.790 | 21.574  | 49.146  | 16.489  | 0.075      | 0.059      | 67     | 6.5      | 0.5      | 0.1             | 5.7      | 1.1             | 2.25          | 0.16                 | PL  | ... | ...      | 2FGL J1818.7+2138                                                                | ... | bcu   | MG2 J181902+2132       |
| J1819.1+4259  | 274.791 | 42.993  | 70.650  | 23.722  | 0.090      | 0.083      | −26    | 5.3      | 0.3      | 0.1             | 4.0      | 0.8             | 2.51          | 0.17                 | PL  | ... | 1        | ...                                                                              | ... | bcu   | NVSS<br>J181927+425800 |
| J1819.5−2045c | 274.876 | −20.766 | 10.898  | −2.642  | 0.131      | 0.087      | −3     | 4.9      | 1.0      | 0.2             | 14.3     | 3.0             | 2.46          | 0.14                 | PL  | ... | 4,6      | ...                                                                              | ... | ...   | ...                    |
| J1819.5−1345  | 274.897 | −13.762 | 17.084  | 0.646   | 0.087      | 0.085      | −74    | 7.7      | 2.9      | 0.4             | 41.2     | 5.9             | 2.48          | 0.09                 | PL  | T   | 1,4      | ...                                                                              | ... | ...   | ...                    |
| J1820.3+3625  | 275.079 | 36.427  | 63.921  | 21.574  | 0.080      | 0.067      | 2      | 6.1      | 0.3      | 0.1             | 3.3      | 0.8             | 1.78          | 0.20                 | PL  | ... | ...      | 2FGL J1820.6+3625                                                                | ... | bcu   | NVSS<br>J182021+362343 |
| J1820.3−1529c | 275.100 | −15.489 | 15.654  | −0.342  | 0.086      | 0.075      | −69    | 4.7      | 2.4      | 0.5             | 29.5     | 8.6             | 2.33          | 0.14                 | PL  | ... | 5,6      | ...                                                                              | ... | ...   | ...                    |
| J1820.4−3217  | 275.103 | −32.286 | 0.737   | −8.165  | 0.157      | 0.110      | 59     | 6.2      | 0.8      | 0.1             | 9.6      | 1.5             | 2.34          | 0.10                 | PL  | ... | 3        | 2FGL J1820.6−3219                                                                | ... | ...   | ...                    |

Table 1—Continued

| Name 3FGL     | R.A.    | Decl.   | $l$     | $b$     | $\theta_1$ | $\theta_2$ | $\phi$ | $\sigma$ | $F_{35}$ | $\Delta F_{35}$ | $S_{25}$ | $\Delta S_{25}$ | $\Gamma_{25}$ | $\Delta \Gamma_{25}$ | Mod | Var | Flags | $\gamma$ -ray Assoc.                                                                             | TeV | Class | ID or Assoc.                      |
|---------------|---------|---------|---------|---------|------------|------------|--------|----------|----------|-----------------|----------|-----------------|---------------|----------------------|-----|-----|-------|--------------------------------------------------------------------------------------------------|-----|-------|-----------------------------------|
| J1821.6–1436c | 275.417 | –14.612 | 16.572  | –0.200  | 0.070      | 0.050      | 55     | 7.7      | 3.7      | 0.5             | 44.5     | 6.9             | 2.29          | 0.09                 | PL  | ... | 6     | 1FGL J1820.5–3216<br>0FGL J1821.4–1444<br>1AGL J1823–1454                                        | ... | ...   | ...                               |
| J1821.9+6636  | 275.477 | 66.601  | 96.536  | 27.639  | 0.091      | 0.067      | –62    | 6.5      | 0.3      | 0.1             | 3.3      | 0.6             | 2.04          | 0.18                 | PL  | ... | ...   | ...                                                                                              | ... | ...   | ...                               |
| J1822.1–7051  | 275.546 | –70.860 | 323.650 | –23.181 | 0.265      | 0.185      | 83     | 5.5      | 0.3      | 0.1             | 5.3      | 1.0             | 2.70          | 0.14                 | PL  | ... | 1     | ...                                                                                              | ... | bcu   | PMN J1823–7056                    |
| J1823.2–4722  | 275.805 | –47.381 | 347.058 | –15.161 | 0.098      | 0.092      | –86    | 5.4      | 0.4      | 0.1             | 4.8      | 1.0             | 2.04          | 0.14                 | PL  | ... | 1     | ...                                                                                              | ... | ...   | ...                               |
| J1823.2–1339  | 275.820 | –13.651 | 17.604  | –0.094  | 0.029      | 0.025      | –25    | 16.6     | 11.5     | 0.7             | 92.9     | 7.9             | 2.29          | ...                  | LP  | ... | ...   | 2FGL J1823.1–1338c<br>1AGL J1823–1454<br>1FGL J1823.2–1336c                                      | ... | ...   | HESS J1825–137 field <sup>a</sup> |
| J1823.4+6857  | 275.865 | 68.951  | 99.194  | 27.677  | 0.065      | 0.049      | –35    | 14.5     | 0.8      | 0.1             | 9.5      | 0.9             | 2.28          | 0.07                 | PL  | ... | ...   | 2FGL J1823.7+6856                                                                                | ... | bll   | 7C 1823+6856                      |
| J1823.6–3453  | 275.909 | –34.895 | 358.680 | –9.934  | 0.025      | 0.023      | –14    | 19.6     | 1.7      | 0.2             | 22.6     | 2.2             | 1.75          | 0.06                 | PL  | ... | ...   | 1FHL J1823.7–3455                                                                                | ... | bcu   | NVSS<br>J182338–345412            |
| J1823.7–3019  | 275.927 | –30.329 | 2.821   | –7.905  | 0.053      | 0.047      | –39    | 11.6     | 1.4      | 0.2             | 16.0     | 1.7             | 2.18          | 0.07                 | PL  | ... | ...   | 2FGL J1823.4–3014                                                                                | ... | PSR   | PSR J1823–3021A                   |
| J1824.0+1017  | 276.022 | 10.291  | 39.101  | 10.702  | 0.089      | 0.079      | –86    | 6.7      | 0.6      | 0.1             | 7.0      | 1.3             | 1.99          | 0.11                 | PL  | ... | ...   | ...                                                                                              | ... | psr   | PSR J1824+10                      |
| J1824.2–5427  | 276.052 | –54.452 | 340.315 | –18.039 | 0.096      | 0.088      | 56     | 5.4      | 0.4      | 0.1             | 4.6      | 0.9             | 2.21          | 0.15                 | PL  | ... | ...   | ...                                                                                              | ... | ...   | ...                               |
| J1824.2+5649  | 276.058 | 56.833  | 85.723  | 26.063  | 0.034      | 0.032      | –16    | 34.5     | 2.0      | 0.1             | 28.3     | 1.1             | 2.46          | 0.03                 | PL  | T   | ...   | 2FGL J1824.0+5650<br>1FGL J1824.0+5651                                                           | ... | bll   | 4C +56.27                         |
| J1824.3–0620  | 276.099 | –6.339  | 24.199  | 3.083   | 0.056      | 0.052      | –69    | 9.8      | 1.9      | 0.2             | 21.9     | 2.8             | 2.24          | 0.09                 | PL  | ... | 3,10  | ...                                                                                              | ... | ...   | ...                               |
| J1824.4+4310  | 276.102 | 43.169  | 71.123  | 22.851  | 0.065      | 0.060      | 21     | 5.0      | 0.2      | 0.1             | 2.3      | 0.7             | 1.72          | 0.21                 | PL  | ... | ...   | 2FGL J1823.8+4312                                                                                | ... | bcu   | 1RXS<br>J182418.7+430954          |
| J1824.5–1351e | 276.130 | –13.852 | 17.567  | –0.453  | ...        | ...        | ...    | 16.8     | 7.8      | 1.2             | 161.2    | 11.8            | 1.59          | ...                  | LP  | ... | ...   | 1FGL J1825.7–1410c<br>1FHL J1824.5–1351e<br>2FGL J1824.5–1351e<br>...                            | E   | PWN   | HESS J1825–137                    |
| J1824.6–2451  | 276.160 | –24.860 | 7.817   | –5.595  | 0.071      | 0.048      | 53     | 19.2     | 3.4      | 0.2             | 28.8     | 2.2             | 2.33          | ...                  | EC  | ... | ...   | 2FGL J1824.8–2449<br>1FGL J1824.5–2449                                                           | ... | PSR   | PSR J1824–2452A                   |
| J1825.2–5230  | 276.321 | –52.509 | 342.270 | –17.465 | 0.044      | 0.040      | –6     | 21.6     | 2.0      | 0.2             | 16.5     | 1.3             | 2.23          | ...                  | LP  | T   | ...   | 2FGL J1825.1–5231                                                                                | ... | bcu   | PKS 1821–525                      |
| J1826.1–1256  | 276.538 | –12.943 | 18.557  | –0.380  | 0.013      | 0.012      | 89     | 76.3     | 53.4     | 0.9             | 414.7    | 8.7             | 2.26          | ...                  | EC  | ... | ...   | 2FGL J1826.1–1256<br>1FGL J1826.1–1256<br>0FGL J1825.9–1256<br>3EG J1826–1302<br>1AGL J1826–1246 | ... | PSR   | LAT PSR J1826–1256                |
| J1826.2–1450  | 276.568 | –14.847 | 16.886  | –1.294  | 0.019      | 0.018      | 2      | 35.1     | 19.1     | 0.7             | 280.7    | 6.5             | 2.57          | ...                  | LP  | ... | ...   | 1FHL J1826.2–1450<br>2FGL J1826.3–1450<br>1FGL J1826.2–1450                                      | P   | HMB   | LS 5039                           |

Table 1—Continued

| Name 3FGL     | R.A.    | Decl.   | $l$     | $b$     | $\theta_1$ | $\theta_2$ | $\phi$ | $\sigma$ | $F_{35}$ | $\Delta F_{35}$ | $S_{25}$ | $\Delta S_{25}$ | $\Gamma_{25}$ | $\Delta \Gamma_{25}$ | Mod | Var | Flags   | $\gamma$ -ray Assoc. | TeV | Class | ID or Assoc.             |
|---------------|---------|---------|---------|---------|------------|------------|--------|----------|----------|-----------------|----------|-----------------|---------------|----------------------|-----|-----|---------|----------------------|-----|-------|--------------------------|
|               |         |         |         |         |            |            |        |          |          |                 |          |                 |               |                      |     |     |         | 0FGL J1826.3–1451    |     |       |                          |
| J1827.3–1446  | 276.834 | –14.767 | 17.076  | –1.484  | 0.062      | 0.044      | 78     | 9.1      | 5.3      | 0.7             | 22.2     | 2.8             | 2.54          | ...                  | LP  | ... | 5,12    | 2FGL J1827.4–1445c   | ... | ...   | ...                      |
| J1827.6–0846  | 276.908 | –8.771  | 22.418  | 1.242   | 0.054      | 0.048      | 53     | 8.7      | 2.4      | 0.3             | 30.6     | 4.1             | 2.36          | 0.08                 | PL  | ... | 3       | 2FGL J1827.4–0846    | ... | ...   | ...                      |
| J1827.7+1141  | 276.925 | 11.697  | 40.782  | 10.518  | 0.104      | 0.085      | 73     | 6.5      | 0.7      | 0.1             | 7.6      | 1.3             | 2.11          | 0.11                 | PL  | ... | ...     | 2FGL J1827.6+1149    | ... | ...   | ...                      |
| J1828.4–1121  | 277.109 | –11.363 | 20.215  | –0.139  | 0.241      | 0.116      | 45     | 9.9      | 4.4      | 0.6             | 44.2     | 6.0             | 2.54          | ...                  | LP  | T   | 1,3,4,9 | 2FGL J1828.3–1124c   | ... | spp   | ...                      |
|               |         |         |         |         |            |            |        |          |          |                 |          |                 |               |                      |     |     |         | 1FGL J1827.9–1128c   |     |       |                          |
| J1828.9–2417  | 277.245 | –24.292 | 8.779   | –6.213  | 0.056      | 0.050      | 34     | 8.8      | 1.0      | 0.2             | 11.4     | 1.8             | 1.99          | 0.12                 | PL  | ... | ...     | 1FHL J1828.9–2417    | ... | bcu   | 1RXS<br>J182853.8–241746 |
|               |         |         |         |         |            |            |        |          |          |                 |          |                 |               |                      |     |     |         | 2FGL J1829.3–2419    |     |       |                          |
| J1829.2+3229  | 277.306 | 32.498  | 60.644  | 18.519  | 0.154      | 0.148      | –82    | 5.7      | 0.4      | 0.1             | 5.1      | 0.9             | 2.29          | 0.12                 | PL  | ... | ...     | 2FGL J1828.7+3231    | ... | ...   | ...                      |
| J1829.2+2731  | 277.313 | 27.525  | 55.798  | 16.679  | 0.131      | 0.115      | 44     | 8.6      | 0.5      | 0.1             | 9.1      | 1.1             | 2.62          | 0.09                 | PL  | ... | 9       | 2FGL J1829.1+2725    | ... | ...   | ...                      |
| J1829.2–1504  | 277.321 | –15.083 | 17.015  | –2.047  | 0.108      | 0.065      | –67    | 5.1      | 0.6      | 0.3             | 8.4      | 2.5             | 1.61          | 0.30                 | PL  | ... | 1       | ...                  | ... | ...   | ...                      |
| J1829.3–0135c | 277.332 | –1.590  | 28.988  | 4.188   | 0.183      | 0.105      | 4      | 4.7      | 1.3      | 0.3             | 17.2     | 4.7             | 2.41          | 0.15                 | PL  | ... | 3,5,6   | ...                  | ... | ...   | ...                      |
| J1829.4+5402  | 277.351 | 54.049  | 82.865  | 24.789  | 0.037      | 0.034      | –27    | 13.2     | 0.6      | 0.1             | 7.2      | 0.9             | 1.93          | 0.09                 | PL  | ... | ...     | 2FGL J1829.2+5402    | ... | bll   | 1RXS<br>J182925.7+540255 |
|               |         |         |         |         |            |            |        |          |          |                 |          |                 |               |                      |     |     |         | 1FGL J1829.8+5404    |     |       |                          |
| J1829.6+4844  | 277.414 | 48.749  | 77.234  | 23.485  | 0.043      | 0.037      | 57     | 24.1     | 1.5      | 0.1             | 19.1     | 1.0             | 2.37          | 0.04                 | PL  | T   | ...     | 2FGL J1829.7+4846    | ... | ssrq  | 3C 380                   |
|               |         |         |         |         |            |            |        |          |          |                 |          |                 |               |                      |     |     |         | 1FGL J1829.8+4845    |     |       |                          |
| J1829.7–1304  | 277.441 | –13.071 | 18.853  | –1.218  | 0.079      | 0.060      | –28    | 6.5      | 2.2      | 0.4             | 25.5     | 4.7             | 2.25          | 0.10                 | PL  | ... | 1       | ...                  | ... | spp   | ...                      |
| J1829.8+1328  | 277.464 | 13.470  | 42.639  | 10.812  | 0.176      | 0.116      | –55    | 4.8      | 0.4      | 0.1             | 5.3      | 1.3             | 1.87          | 0.16                 | PL  | ... | ...     | 2FGL J1830.0+1325    | ... | bll   | MG1 J183001+1323         |
| J1829.9–0203c | 277.488 | –2.054  | 28.647  | 3.836   | 0.181      | 0.128      | 39     | 5.3      | 1.8      | 0.3             | 23.0     | 5.7             | 2.39          | 0.13                 | PL  | ... | 6,9     | 2FGL J1829.8–0204c   | ... | ...   | ...                      |
| J1830.0–4439  | 277.507 | –44.658 | 350.133 | –15.156 | 0.067      | 0.064      | –81    | 19.2     | 1.4      | 0.1             | 17.0     | 1.2             | 2.47          | ...                  | LP  | T   | ...     | 2FGL J1830.2–4441    | ... | bcu   | PMN J1830–4441           |
| J1830.1+0617  | 277.538 | 6.292   | 36.142  | 7.586   | 0.049      | 0.041      | –43    | 13.2     | 1.7      | 0.2             | 18.7     | 1.9             | 2.11          | 0.07                 | PL  | T   | ...     | 2FGL J1830.1+0617    | ... | fsrq  | TXS 1827+062             |
|               |         |         |         |         |            |            |        |          |          |                 |          |                 |               |                      |     |     |         | 1FGL J1830.1+0618    |     |       |                          |
|               |         |         |         |         |            |            |        |          |          |                 |          |                 |               |                      |     |     |         | 0FGL J1830.3+0617    |     |       |                          |
| J1830.7–1630  | 277.698 | –16.514 | 15.911  | –3.030  | 0.075      | 0.055      | –8     | 12.1     | 2.2      | 0.2             | 30.4     | 3.0             | 2.44          | 0.07                 | PL  | ... | ...     | 2FGL J1830.4–1634    | ... | ...   | ...                      |
| J1830.8–3136  | 277.711 | –31.603 | 2.354   | –9.842  | 0.118      | 0.086      | –25    | 5.3      | 0.6      | 0.1             | 6.8      | 1.3             | 2.19          | 0.13                 | PL  | ... | ...     | 2FGL J1830.9–3132    | ... | ...   | ...                      |
| J1831.0–2714  | 277.763 | –27.235 | 6.342   | –7.955  | 0.128      | 0.102      | –13    | 4.9      | 0.6      | 0.1             | 7.2      | 1.5             | 2.21          | 0.15                 | PL  | ... | ...     | ...                  | ... | bcu   | PMN J1831–2714           |
| J1831.6–6503  | 277.919 | –65.066 | 329.953 | –22.406 | 0.102      | 0.072      | –46    | 8.6      | 0.7      | 0.1             | 3.0      | 0.5             | 2.06          | ...                  | LP  | ... | 12      | 2FGL J1832.2–6502    | ... | ...   | ...                      |
|               |         |         |         |         |            |            |        |          |          |                 |          |                 |               |                      |     |     |         | 1FGL J1833.2–6502    |     |       |                          |
| J1831.7–0230  | 277.942 | –2.501  | 28.458  | 3.228   | 0.092      | 0.086      | –34    | 9.3      | 2.8      | 0.4             | 42.6     | 6.4             | 2.63          | ...                  | LP  | ... | ...     | ...                  | ... | ...   | ...                      |
| J1831.7–0157c | 277.948 | –1.961  | 28.941  | 3.471   | 0.106      | 0.099      | –68    | 5.1      | 1.7      | 0.3             | 27.1     | 7.6             | 2.54          | 0.15                 | PL  | ... | 5,6     | 2FGL J1832.0–0200    | ... | ...   | ...                      |
|               |         |         |         |         |            |            |        |          |          |                 |          |                 |               |                      |     |     |         | 1FGL J1831.5–0200c   |     |       |                          |
| J1832.4–5659  | 278.117 | –56.996 | 338.224 | –20.018 | 0.069      | 0.060      | –7     | 12.7     | 0.9      | 0.1             | 10.9     | 1.0             | 2.31          | 0.08                 | PL  | ... | ...     | 2FGL J1832.7–5700    | ... | bll   | PMN J1832–5659           |
|               |         |         |         |         |            |            |        |          |          |                 |          |                 |               |                      |     |     |         | 1FGL J1832.6–5700    |     |       |                          |
| J1833.5–1033  | 278.394 | –10.560 | 21.511  | –0.885  | 0.035      | 0.030      | –40    | 16.9     | 6.0      | 0.4             | 79.2     | 5.3             | 2.39          | 0.04                 | PL  | ... | ...     | 2FGL J1833.6–1032    | ... | PSR   | PSR J1833–1034           |
|               |         |         |         |         |            |            |        |          |          |                 |          |                 |               |                      |     |     |         | 1FGL J1833.5–1034    |     |       |                          |



Table 1—Continued

| Name 3FGL     | R.A.    | Decl.   | $l$     | $b$     | $\theta_1$ | $\theta_2$ | $\phi$ | $\sigma$ | $F_{35}$ | $\Delta F_{35}$ | $S_{25}$ | $\Delta S_{25}$ | $\Gamma_{25}$ | $\Delta \Gamma_{25}$ | Mod | Var | Flags | $\gamma$ -ray Assoc.                                                                                                  | TeV | Class | ID or Assoc.            |
|---------------|---------|---------|---------|---------|------------|------------|--------|----------|----------|-----------------|----------|-----------------|---------------|----------------------|-----|-----|-------|-----------------------------------------------------------------------------------------------------------------------|-----|-------|-------------------------|
| J1833.6–2103  | 278.411 | –21.057 | 12.168  | –5.705  | 0.014      | 0.014      | –27    | 129.7    | 20.5     | 0.4             | 283.2    | 3.5             | 2.49          | ...                  | LP  | T   | ...   | 1FHL J1833.7–2105<br>2FGL J1833.6–2104<br>1FGL J1833.6–2103<br>0FGL J1833.4–2106<br>3EG J1832–2110                    | ... | fsrq  | PKS 1830–211            |
| J1833.9–0711  | 278.480 | –7.193  | 24.538  | 0.592   | 0.098      | 0.065      | –69    | 7.0      | 3.5      | 0.6             | 38.9     | 7.2             | 2.11          | 0.10                 | PL  | T   | 3,5,9 | ...                                                                                                                   | ... | spp   | ...                     |
| J1834.5–0841  | 278.629 | –8.684  | 23.283  | –0.226  | 0.030      | 0.025      | 32     | 13.9     | 6.3      | 0.5             | 71.1     | 6.0             | 2.17          | 0.05                 | PL  | ... | 3     | 0FGL J1834.4–0841<br>1FGL J1834.3–0842c<br>2FGL J1834.3–0848                                                          | E   | snr   | W 41                    |
| J1834.6–0659  | 278.665 | –6.990  | 24.803  | 0.523   | 0.039      | 0.036      | 53     | 9.5      | 4.3      | 0.7             | 47.9     | 8.2             | 2.05          | 0.10                 | PL  | ... | ...   | 1FHL J1834.6–0703                                                                                                     | ... | spp   | ...                     |
| J1834.8–0630c | 278.713 | –6.511  | 25.250  | 0.701   | 0.080      | 0.079      | –16    | 4.7      | 1.9      | 0.5             | 21.7     | 6.0             | 2.21          | 0.13                 | PL  | ... | 6     | ...                                                                                                                   | ... | ...   | ...                     |
| J1835.4+1349  | 278.859 | 13.826  | 43.562  | 9.745   | 0.134      | 0.104      | –63    | 4.2      | 0.4      | 0.1             | 6.2      | 1.5             | 2.46          | 0.16                 | PL  | ... | ...   | 2FGL J1835.4+1349<br>1FGL J1835.3+1345                                                                                | ... | bcu   | TXS 1833+137            |
| J1835.7–3258  | 278.944 | –32.971 | 1.555   | –11.372 | 0.094      | 0.085      | 24     | 8.1      | 1.1      | 0.2             | 5.8      | 1.0             | 2.29          | ...                  | LP  | ... | ...   | 2FGL J1835.6–3258<br>1FGL J1835.3–3255                                                                                | ... | glc   | NGC 6652                |
| J1836.2+5925  | 279.061 | 59.431  | 88.882  | 24.998  | 0.007      | 0.007      | 35     | 438.1    | 99.3     | 0.7             | 598.3    | 3.6             | 1.91          | ...                  | EC  | ... | ...   | 1FHL J1836.4+5925<br>2FGL J1836.2+5926<br>1FGL J1836.2+5925<br>0FGL J1836.2+5924<br>3EG J1835+5918<br>1AGL J1836+5923 | ... | PSR   | LAT PSR J1836+5925      |
| J1836.3+3137  | 279.098 | 31.622  | 60.371  | 16.786  | 0.058      | 0.053      | 67     | 10.1     | 0.8      | 0.1             | 9.6      | 1.2             | 2.35          | 0.09                 | PL  | T   | ...   | 2FGL J1836.2+3137<br>1FGL J1836.3+3135                                                                                | ... | bl    | RX J1836.2+3136         |
| J1836.5–0655e | 279.140 | –6.920  | 25.082  | 0.136   | ...        | ...        | ...    | 14.1     | 9.7      | 1.0             | 108.8    | 10.3            | 1.97          | 0.06                 | PL  | ... | ...   | 1FGL J1837.5–0659c<br>1FHL J1836.5–0655e<br>2FGL J1837.3–0700c                                                        | E   | PWN   | HESS J1837–069          |
| J1837.3–2403  | 279.330 | –24.060 | 9.847   | –7.809  | 0.212      | 0.134      | –47    | 5.1      | 0.7      | 0.1             | 8.7      | 1.7             | 2.40          | 0.14                 | PL  | ... | ...   | ...                                                                                                                   | ... | ...   | ...                     |
| J1837.6–0717  | 279.402 | –7.297  | 24.867  | –0.269  | 0.086      | 0.057      | 34     | 5.6      | 2.4      | 0.6             | 26.6     | 6.7             | 2.04          | 0.13                 | PL  | ... | 1,4,5 | ...                                                                                                                   | ... | ...   | ...                     |
| J1837.9–0607  | 279.488 | –6.126  | 25.946  | 0.194   | 0.055      | 0.049      | –5     | 6.6      | 3.6      | 0.6             | 42.7     | 7.9             | 2.27          | 0.08                 | PL  | ... | 3,4,5 | ...                                                                                                                   | ... | PSR   | PSR J1837–0604          |
| J1838.1+3827  | 279.550 | 38.463  | 67.219  | 18.896  | 0.179      | 0.160      | 22     | 6.9      | 0.3      | 0.1             | 5.9      | 0.9             | 2.72          | 0.14                 | PL  | ... | 1     | 2FGL J1837.9+3821                                                                                                     | ... | ...   | ...                     |
| J1838.5–6006  | 279.636 | –60.111 | 335.319 | –21.740 | 0.106      | 0.091      | 2      | 6.1      | 0.4      | 0.1             | 4.4      | 1.0             | 1.86          | 0.14                 | PL  | ... | ...   | ...                                                                                                                   | ... | bcu   | SUMSS<br>J183806–600033 |
| J1838.8+4802  | 279.702 | 48.037  | 76.943  | 21.829  | 0.030      | 0.028      | –6     | 20.2     | 1.2      | 0.1             | 14.4     | 1.5             | 1.81          | 0.06                 | PL  | ... | ...   | 1FHL J1838.8+4800<br>2FGL J1838.7+4759<br>1FGL J1838.6+4756                                                           | ... | bl    | GB6 J1838+4802          |
| J1838.9–0646  | 279.728 | –6.776  | 25.478  | –0.316  | 0.078      | 0.059      | –66    | 7.1      | 2.6      | 0.5             | 30.0     | 5.2             | 1.92          | 0.10                 | PL  | ... | ...   | ...                                                                                                                   | ... | ...   | ...                     |

Table 1—Continued

| Name 3FGL     | R.A.    | Decl.   | $l$     | $b$     | $\theta_1$ | $\theta_2$ | $\phi$ | $\sigma$ | $F_{35}$ | $\Delta F_{35}$ | $S_{25}$ | $\Delta S_{25}$ | $\Gamma_{25}$ | $\Delta \Gamma_{25}$ | Mod | Var | Flags | $\gamma$ -ray Assoc.                                                             | TeV | Class | ID or Assoc.                      |
|---------------|---------|---------|---------|---------|------------|------------|--------|----------|----------|-----------------|----------|-----------------|---------------|----------------------|-----|-----|-------|----------------------------------------------------------------------------------|-----|-------|-----------------------------------|
| J1838.9–0537  | 279.733 | −5.626  | 26.502  | 0.207   | 0.023      | 0.022      | 53     | 23.3     | 20.1     | 1.1             | 159.6    | 10.9            | 2.27          | ...                  | EC  | ... | ...   | ...                                                                              | ... | PSR   | LAT PSR J1838–0537                |
| J1839.3–0552  | 279.848 | −5.882  | 26.327  | −0.013  | 0.034      | 0.028      | 17     | 14.9     | 14.9     | 1.1             | 101.0    | 10.0            | 2.22          | ...                  | LP  | ... | 5     | 0FGL J1839.0–0549                                                                | ... | ...   | HESS J1841–055 field <sup>a</sup> |
| J1839.9+7646  | 280.000 | 76.783  | 108.082 | 27.004  | 0.434      | 0.280      | −43    | 4.4      | 0.2      | 0.1             | 3.3      | 0.7             | 2.55          | 0.16                 | PL  | ... | ...   | ...                                                                              | ... | ...   | ...                               |
| J1840.1–0412  | 280.039 | −4.214  | 27.896  | 0.582   | 0.073      | 0.065      | 85     | 9.4      | 3.9      | 0.4             | 52.5     | 6.2             | 2.42          | 0.06                 | PL  | ... | ...   | 2FGL J1840.3–0413c<br>EGR J1838–0420                                             | ... | spp   | ...                               |
| J1840.5+6116  | 280.130 | 61.283  | 91.000  | 24.851  | 0.224      | 0.147      | −72    | 5.7      | 0.3      | 0.1             | 5.9      | 1.0             | 2.73          | 0.14                 | PL  | ... | 1,5   | ...                                                                              | ... | ...   | ...                               |
| J1840.9–0532e | 280.230 | −5.550  | 26.796  | −0.199  | ...        | ...        | ...    | 16.8     | 11.8     | 1.0             | 145.8    | 10.6            | 1.81          | 0.04                 | PL  | T   | ...   | ...                                                                              | E   | PWN   | HESS J1841–055                    |
| J1841.2+2910  | 280.301 | 29.183  | 58.442  | 14.893  | 0.048      | 0.043      | −34    | 8.4      | 0.4      | 0.1             | 6.0      | 1.3             | 1.57          | 0.17                 | PL  | ... | ...   | 1FHL J1841.1+2914                                                                | ... | bcu   | MG3 J184126+2910                  |
| J1841.7+3218  | 280.442 | 32.313  | 61.486  | 15.990  | 0.038      | 0.036      | −83    | 12.8     | 0.9      | 0.1             | 10.4     | 1.2             | 2.06          | 0.10                 | PL  | ... | ...   | 1FHL J1841.8+3219<br>2FGL J1841.7+3221<br>1FGL J1841.9+3220                      | ... | bll   | RX J1841.7+3218                   |
| J1842.2+2742  | 280.563 | 27.703  | 57.131  | 14.096  | 0.079      | 0.064      | −18    | 8.3      | 0.7      | 0.1             | 7.8      | 1.2             | 2.13          | 0.10                 | PL  | ... | ...   | 2FGL J1842.3+2740                                                                | ... | ...   | ...                               |
| J1842.3–5841  | 280.594 | −58.688 | 336.938 | −21.795 | 0.040      | 0.035      | −88    | 10.2     | 0.5      | 0.1             | 6.4      | 1.1             | 1.70          | 0.12                 | PL  | ... | ...   | 2FGL J1842.3–5839                                                                | ... | bcu   | 1RXS<br>J184230.6–584202          |
| J1842.8+6810  | 280.703 | 68.180  | 98.560  | 25.834  | 0.289      | 0.179      | −89    | 4.6      | 0.3      | 0.1             | 4.3      | 1.0             | 2.55          | 0.17                 | PL  | T   | 5     | 1FGL J1842.3–5845<br>...                                                         | ... | fsrq  | S4 1842.8+68                      |
| J1843.0–0359c | 280.762 | −3.989  | 28.426  | 0.044   | 0.120      | 0.079      | 7      | 6.9      | 5.0      | 0.7             | 30.6     | 6.3             | 2.28          | ...                  | LP  | ... | 1,5,6 | 2FGL J1842.8–0359c<br>1FGL J1842.9–0359c                                         | ... | ...   | ...                               |
| J1843.6–1114  | 280.915 | −11.238 | 22.041  | −3.397  | 0.202      | 0.144      | 87     | 7.0      | 1.0      | 0.2             | 19.8     | 2.8             | 2.73          | 0.10                 | PL  | ... | ...   | ...                                                                              | ... | PSR   | PSR J1843–1113                    |
| J1843.7–0322  | 280.928 | −3.377  | 29.047  | 0.176   | 0.085      | 0.077      | −25    | 13.1     | 8.1      | 0.8             | 94.0     | 6.5             | 2.48          | ...                  | LP  | ... | ...   | ...                                                                              | ... | ...   | ...                               |
| J1844.1+5709  | 281.043 | 57.161  | 86.709  | 23.479  | 0.153      | 0.087      | −74    | 9.0      | 0.5      | 0.1             | 6.7      | 0.9             | 2.39          | 0.10                 | PL  | ... | ...   | 2FGL J1844.7+5716                                                                | ... | bll   | TXS 1843+571                      |
| J1844.3+1547  | 281.083 | 15.786  | 46.297  | 8.661   | 0.040      | 0.038      | −10    | 14.9     | 1.6      | 0.2             | 17.7     | 1.7             | 2.03          | 0.07                 | PL  | ... | ...   | 2FGL J1844.3+1548                                                                | ... | bcu   | NVSS<br>J184425+154646            |
| J1844.3–0344  | 281.100 | −3.747  | 28.796  | −0.145  | 0.056      | 0.047      | −5     | 10.1     | 6.0      | 0.9             | 28.3     | 4.7             | 2.22          | ...                  | LP  | ... | ...   | 1FGL J1844.1+1547<br>2FGL J1844.3–0343c<br>1FGL J1844.2–0342c                    | ... | ...   | ...                               |
| J1844.7–1224  | 281.182 | −12.413 | 21.109  | −4.162  | 0.105      | 0.080      | 73     | 5.4      | 0.9      | 0.2             | 10.3     | 2.8             | 2.28          | 0.21                 | PL  | ... | 1     | ...                                                                              | ... | ...   | ...                               |
| J1845.5–2524  | 281.387 | −25.410 | 9.441   | −10.079 | 0.108      | 0.081      | 20     | 9.2      | 1.1      | 0.1             | 12.9     | 1.6             | 2.28          | 0.09                 | PL  | ... | ...   | ...                                                                              | ... | ...   | ...                               |
| J1846.3+0919  | 281.596 | 9.332   | 40.690  | 5.354   | 0.030      | 0.029      | 22     | 26.3     | 4.8      | 0.3             | 24.8     | 1.6             | 2.03          | ...                  | EC  | ... | ...   | 2FGL J1846.4+0920<br>1FGL J1846.4+0919                                           | ... | PSR   | LAT PSR J1846+0919                |
| J1848.1–4230  | 282.046 | −42.513 | 353.497 | −17.387 | 0.121      | 0.085      | 64     | 5.5      | 0.4      | 0.1             | 4.8      | 1.1             | 1.95          | 0.14                 | PL  | ... | ...   | ...                                                                              | ... | bcu   | PMN J1848–4230                    |
| J1848.4+3216  | 282.107 | 32.282  | 62.020  | 14.679  | 0.036      | 0.032      | 6      | 14.0     | 2.4      | 0.2             | 32.5     | 3.5             | 2.41          | 0.07                 | PL  | T   | ...   | 0FGL J1847.8+3223<br>1FGL J1848.5+3224<br>1FHL J1848.5+3219<br>2FGL J1848.5+3216 | ... | FSRQ  | B2 1846+32A                       |
| J1848.4–0141  | 282.118 | −1.693  | 31.088  | −0.113  | 0.081      | 0.057      | 20     | 18.7     | 12.9     | 0.8             | 114.6    | 8.1             | 2.36          | ...                  | LP  | ... | 3     | 2FGL J1848.2–0139c<br>1FGL J1848.1–0145c                                         | E   | ...   | ...                               |

Table 1—Continued

| Name 3FGL     | R.A.    | Decl.   | $l$     | $b$     | $\theta_1$ | $\theta_2$ | $\phi$ | $\sigma$ | $F_{35}$ | $\Delta F_{35}$ | $S_{25}$ | $\Delta S_{25}$ | $\Gamma_{25}$ | $\Delta \Gamma_{25}$ | Mod | Var | Flags     | $\gamma$ -ray Assoc. | TeV | Class | ID or Assoc.             |
|---------------|---------|---------|---------|---------|------------|------------|--------|----------|----------|-----------------|----------|-----------------|---------------|----------------------|-----|-----|-----------|----------------------|-----|-------|--------------------------|
|               |         |         |         |         |            |            |        |          |          |                 |          |                 |               |                      |     |     |           | 0FGL J1848.6–0138    |     |       |                          |
| J1848.6+3232  | 282.157 | 32.544  | 62.286  | 14.743  | 0.065      | 0.048      | 7      | 11.6     | 2.4      | 0.2             | 20.4     | 3.5             | 2.40          | ...                  | LP  | T   | 5,7       | ...                  | ... | ...   | ...                      |
| J1848.9+4247  | 282.225 | 42.791  | 72.246  | 18.481  | 0.066      | 0.047      | 45     | 6.3      | 0.2      | 0.1             | 3.4      | 0.9             | 1.66          | 0.26                 | PL  | ... | ...       | ...                  | ... | bll   | RGB J1848+427            |
| J1849.2+6705  | 282.324 | 67.093  | 97.490  | 25.041  | 0.020      | 0.020      | 59     | 63.3     | 5.0      | 0.2             | 49.2     | 1.6             | 2.24          | ...                  | LP  | T   | ...       | 1FHL J1849.3+6705    | ... | FSRQ  | S4 1849+67               |
|               |         |         |         |         |            |            |        |          |          |                 |          |                 |               |                      |     |     |           | 2FGL J1849.4+6706    |     |       |                          |
|               |         |         |         |         |            |            |        |          |          |                 |          |                 |               |                      |     |     |           | 1FGL J1849.3+6705    |     |       |                          |
|               |         |         |         |         |            |            |        |          |          |                 |          |                 |               |                      |     |     |           | 0FGL J1849.4+6706    |     |       |                          |
|               |         |         |         |         |            |            |        |          |          |                 |          |                 |               |                      |     |     |           | 1AGL J1846+6714      |     |       |                          |
| J1849.3–1645  | 282.335 | –16.764 | 17.701  | –7.107  | 0.058      | 0.048      | –80    | 6.2      | 0.4      | 0.1             | 6.0      | 1.5             | 1.61          | 0.15                 | PL  | ... | ...       | ...                  | ... | bcu   | 1RXS<br>J184919.7–164726 |
| J1849.4–0057  | 282.355 | –0.952  | 31.855  | 0.014   | 0.039      | 0.036      | 85     | 13.2     | 6.8      | 0.7             | 48.9     | 6.6             | 2.21          | ...                  | LP  | ... | ...       | 2FGL J1849.3–0055    | ... | snr   | 3C 391                   |
| J1849.4–4312  | 282.363 | –43.207 | 352.904 | –17.852 | 0.043      | 0.040      | –2     | 13.2     | 1.2      | 0.1             | 12.9     | 1.3             | 2.07          | 0.07                 | PL  | ... | ...       | 2FGL J1849.7–4310    | ... | bll   | PMN J1849–4314           |
|               |         |         |         |         |            |            |        |          |          |                 |          |                 |               |                      |     |     |           | 1FGL J1849.6–4314    |     |       |                          |
| J1849.5+2751  | 282.378 | 27.857  | 57.944  | 12.690  | 0.137      | 0.095      | –90    | 7.6      | 0.6      | 0.1             | 8.0      | 1.1             | 2.33          | 0.10                 | PL  | ... | ...       | 2FGL J1849.5+2744    | ... | bll   | MG2 J184929+2748         |
| J1849.5–0124c | 282.397 | –1.413  | 31.464  | –0.233  | 0.076      | 0.066      | 68     | 4.9      | 2.9      | 0.6             | 34.3     | 8.5             | 2.28          | 0.11                 | PL  | ... | 3,4,5,6,9 | 2FGL J1849.9–0125c   | ... | ...   | ...                      |
|               |         |         |         |         |            |            |        |          |          |                 |          |                 |               |                      |     |     |           | 1FGL J1849.7–0121c   |     |       | 115                      |
| J1850.5–0024  | 282.632 | –0.405  | 32.468  | 0.017   | 0.055      | 0.044      | 6      | 9.4      | 4.3      | 0.5             | 57.6     | 7.3             | 2.42          | 0.06                 | PL  | ... | 4,5       | 2FGL J1850.7–0014c   | ... | ...   | ...                      |
|               |         |         |         |         |            |            |        |          |          |                 |          |                 |               |                      |     |     |           | 1FGL J1850.2–0019c   |     |       | –                        |
| J1851.2+0423  | 282.805 | 4.391   | 36.817  | 2.049   | 0.145      | 0.133      | –18    | 9.6      | 0.8      | 0.2             | 32.3     | 3.7             | 2.71          | ...                  | LP  | ... | 1,5,12    | ...                  | ... | ...   | ...                      |
| J1852.4+4856  | 283.108 | 48.947  | 78.609  | 19.957  | 0.034      | 0.032      | 69     | 29.3     | 1.8      | 0.1             | 22.3     | 1.1             | 2.31          | 0.04                 | PL  | T   | ...       | 1FHL J1852.3+4853    | ... | fsrq  | S4 1851+48               |
|               |         |         |         |         |            |            |        |          |          |                 |          |                 |               |                      |     |     |           | 2FGL J1852.5+4856    |     |       |                          |
|               |         |         |         |         |            |            |        |          |          |                 |          |                 |               |                      |     |     |           | 1FGL J1852.5+4853    |     |       |                          |
| J1852.8+0158  | 283.209 | 1.972   | 34.847  | 0.588   | 0.063      | 0.056      | –20    | 13.7     | 5.3      | 0.5             | 82.5     | 6.5             | 2.55          | 0.05                 | PL  | ... | 3         | 2FGL J1852.8+0156c   | ... | ...   | ...                      |
| J1853.2+0006  | 283.301 | 0.109   | 33.230  | –0.344  | 0.147      | 0.079      | –30    | 12.2     | 5.4      | 0.6             | 53.2     | 5.5             | 2.45          | ...                  | LP  | ... | 3,4       | 1FGL J1853.1+0032c   | ... | psr   | PSR J1853–0004           |
| J1855.1–6008  | 283.780 | –60.142 | 335.875 | –23.739 | 0.079      | 0.068      | 85     | 4.2      | 0.2      | 0.1             | 2.3      | 0.7             | 1.81          | 0.19                 | PL  | ... | ...       | ...                  | ... | bcu   | PMN J1854–6009           |
| J1855.1–2243  | 283.796 | –22.717 | 12.870  | –10.924 | 0.074      | 0.069      | –20    | 4.3      | 0.3      | 0.1             | 3.8      | 1.1             | 1.82          | 0.19                 | PL  | ... | ...       | ...                  | ... | glc   | NGC 6717                 |
| J1855.4+0454  | 283.856 | 4.912   | 37.758  | 1.353   | 0.089      | 0.067      | 72     | 9.5      | 2.9      | 0.3             | 45.4     | 5.2             | 2.54          | 0.07                 | PL  | ... | 4         | ...                  | ... | ...   | ...                      |
| J1855.6+0753  | 283.911 | 7.883   | 40.431  | 2.657   | 0.168      | 0.143      | –5     | 9.7      | 2.0      | 0.3             | 33.7     | 3.5             | 2.60          | 0.07                 | PL  | ... | 1,4       | ...                  | ... | ...   | ...                      |
| J1855.9+0121e | 283.990 | 1.355   | 34.654  | –0.388  | ...        | ...        | ...    | 68.3     | 70.7     | 1.3             | 535.7    | 12.9            | 2.20          | ...                  | LP  | T   | ...       | 0FGL J1855.9+0126    | ... | SNR   | W44                      |
|               |         |         |         |         |            |            |        |          |          |                 |          |                 |               |                      |     |     |           | 1AGL J1857+0137      |     |       |                          |
|               |         |         |         |         |            |            |        |          |          |                 |          |                 |               |                      |     |     |           | 1FGL J1856.1+0122    |     |       |                          |
|               |         |         |         |         |            |            |        |          |          |                 |          |                 |               |                      |     |     |           | 1FHL J1855.9+0121e   |     |       |                          |
|               |         |         |         |         |            |            |        |          |          |                 |          |                 |               |                      |     |     |           | 2FGL J1855.9+0121e   |     |       |                          |
|               |         |         |         |         |            |            |        |          |          |                 |          |                 |               |                      |     |     |           | 3EG J1856+0114       |     |       |                          |
| J1856.1–1217  | 284.032 | –12.300 | 22.465  | –6.600  | 0.068      | 0.057      | 12     | 8.4      | 0.9      | 0.1             | 14.9     | 2.0             | 2.59          | 0.11                 | PL  | ... | 3         | ...                  | ... | ...   | ...                      |
| J1857.0–7341  | 284.253 | –73.687 | 321.193 | –26.341 | 0.230      | 0.184      | –90    | 7.8      | 0.3      | 0.1             | 7.3      | 1.0             | 2.90          | 0.13                 | PL  | ... | 3         | ...                  | ... | ...   | ...                      |

Table 1—Continued

| Name 3FGL     | R.A.    | Decl.   | $l$     | $b$     | $\theta_1$ | $\theta_2$ | $\phi$ | $\sigma$ | $F_{35}$ | $\Delta F_{35}$ | $S_{25}$ | $\Delta S_{25}$ | $\Gamma_{25}$ | $\Delta \Gamma_{25}$ | Mod | Var | Flags   | $\gamma$ -ray Assoc. | TeV | Class | ID or Assoc.     |
|---------------|---------|---------|---------|---------|------------|------------|--------|----------|----------|-----------------|----------|-----------------|---------------|----------------------|-----|-----|---------|----------------------|-----|-------|------------------|
| J1857.2+0059  | 284.310 | 0.986   | 34.471  | -0.841  | 0.042      | 0.036      | -59    | 12.4     | 7.5      | 0.9             | 48.5     | 8.7             | 2.22          | ...                  | LP  | ... | 3,5     | 2FGL J1857.2+0055c   | ... | ...   | ...              |
| J1857.8+0129c | 284.471 | 1.498   | 35.000  | -0.751  | 0.107      | 0.073      | -19    | 4.5      | 2.5      | 0.6             | 31.9     | 8.8             | 2.34          | 0.11                 | PL  | ... | 4,5,6   | 2FGL J1858.5+0129c   | ... | ...   | ...              |
|               |         |         |         |         |            |            |        |          |          |                 |          |                 |               |                      |     |     |         | 1AGL J1857+0137      |     |       |                  |
| J1857.9+0355  | 284.489 | 3.928   | 37.170  | 0.343   | 0.072      | 0.064      | 41     | 9.3      | 5.1      | 0.6             | 37.3     | 5.9             | 2.40          | ...                  | LP  | ... | 3,4     | 2FGL J1857.8+0355c   | ... | ...   | ...              |
|               |         |         |         |         |            |            |        |          |          |                 |          |                 |               |                      |     |     |         | 1FGL J1857.9+0352c   |     |       |                  |
| J1857.9+0210  | 284.490 | 2.170   | 35.608  | -0.461  | 0.060      | 0.058      | 13     | 15.2     | 8.2      | 0.6             | 68.0     | 6.9             | 2.36          | ...                  | LP  | ... | ...     | 2FGL J1857.6+0211    | E   | ...   | ...              |
|               |         |         |         |         |            |            |        |          |          |                 |          |                 |               |                      |     |     |         | EGR J1856+0235       |     |       |                  |
| J1857.9+7319  | 284.490 | 73.327  | 104.415 | 25.439  | 0.122      | 0.100      | -77    | 7.0      | 0.3      | 0.1             | 4.8      | 0.7             | 2.64          | 0.12                 | PL  | ... | 1       | ...                  | ... | ...   | ...              |
| J1857.9+5549  | 284.500 | 55.825  | 85.878  | 21.281  | 0.183      | 0.138      | -89    | 4.5      | 0.2      | 0.1             | 6.2      | 1.1             | 2.96          | 0.18                 | PL  | ... | 5       | ...                  | ... | ...   | ...              |
| J1858.0-5423  | 284.501 | -54.391 | 342.040 | -22.679 | 0.185      | 0.128      | 47     | 5.1      | 0.4      | 0.1             | 4.4      | 0.9             | 2.12          | 0.13                 | PL  | ... | ...     | ...                  | ... | ...   | ...              |
| J1858.2-2215  | 284.559 | -22.250 | 13.604  | -11.367 | 0.065      | 0.060      | 43     | 12.0     | 1.7      | 0.2             | 8.3      | 1.1             | 2.11          | ...                  | EC  | ... | ...     | 2FGL J1858.3-2218    | ... | PSR   | PSR J1858-2216   |
|               |         |         |         |         |            |            |        |          |          |                 |          |                 |               |                      |     |     |         | 1FGL J1858.1-2218    |     |       |                  |
| J1858.4-2509  | 284.601 | -25.154 | 10.921  | -12.610 | 0.082      | 0.073      | 65     | 12.3     | 1.3      | 0.1             | 15.9     | 1.5             | 2.29          | 0.07                 | PL  | T   | ...     | 2FGL J1858.1-2510    | ... | bcu   | PMN J1858-2511   |
| J1859.6+0102  | 284.915 | 1.035   | 34.792  | -1.357  | 0.154      | 0.128      | 44     | 8.0      | 4.0      | 0.5             | 35.8     | 6.1             | 2.39          | ...                  | LP  | ... | 1,3,5   | ...                  | ... | ...   | ...              |
| J1900.3+0411c | 285.098 | 4.193   | 37.683  | -0.076  | 0.203      | 0.068      | -63    | 5.1      | 2.3      | 0.5             | 26.7     | 6.4             | 2.22          | 0.12                 | PL  | ... | 1,3,6,9 | 1FGL J1900.3+0420c   | ... | ...   | ...              |
|               |         |         |         |         |            |            |        |          |          |                 |          |                 |               |                      |     |     |         | 0FGL J1900.0+0356    |     |       |                  |
|               |         |         |         |         |            |            |        |          |          |                 |          |                 |               |                      |     |     |         | 1AGL J1901+0429      |     |       |                  |
| J1900.8+0337  | 285.205 | 3.623   | 37.226  | -0.432  | 0.127      | 0.103      | -77    | 10.1     | 2.7      | 0.5             | 51.5     | 5.4             | 2.47          | ...                  | LP  | ... | 1,4,12  | ...                  | ... | ...   | ...              |
| J1901.1+0728  | 285.296 | 7.476   | 40.693  | 1.250   | 0.106      | 0.100      | 13     | 8.7      | 3.2      | 0.4             | 31.4     | 4.8             | 2.44          | ...                  | LP  | ... | 1,3,4   | ...                  | ... | ...   | ...              |
| J1901.5-0126  | 285.399 | -1.448  | 32.801  | -2.921  | 0.056      | 0.053      | 21     | 14.0     | 2.1      | 0.2             | 36.3     | 2.9             | 2.62          | 0.06                 | PL  | ... | ...     | ...                  | ... | ...   | ...              |
| J1902.0-5107  | 285.513 | -51.125 | 345.624 | -22.387 | 0.039      | 0.037      | 4      | 28.9     | 2.7      | 0.2             | 21.5     | 1.2             | 2.24          | ...                  | EC  | ... | ...     | 2FGL J1902.0-5109    | ... | PSR   | PSR J1902-5105   |
|               |         |         |         |         |            |            |        |          |          |                 |          |                 |               |                      |     |     |         | 1FGL J1902.0-5110    |     |       |                  |
| J1902.3-3702c | 285.579 | -37.043 | 359.877 | -17.963 | 0.155      | 0.127      | -54    | 4.7      | 0.5      | 0.1             | 6.6      | 1.3             | 2.32          | 0.12                 | PL  | ... | 6       | ...                  | ... | ...   | ...              |
| J1902.6+0655  | 285.657 | 6.932   | 40.374  | 0.682   | 0.081      | 0.055      | 74     | 6.0      | 1.9      | 0.4             | 22.1     | 4.9             | 2.23          | 0.12                 | PL  | ... | 3       | ...                  | ... | ...   | ...              |
| J1902.9-6745  | 285.743 | -67.753 | 327.820 | -26.040 | 0.125      | 0.093      | 12     | 10.3     | 0.5      | 0.1             | 8.5      | 0.9             | 2.60          | 0.09                 | PL  | T   | ...     | 2FGL J1902.5-6746    | ... | fsrq  | PMN J1903-6749   |
|               |         |         |         |         |            |            |        |          |          |                 |          |                 |               |                      |     |     |         | 1FGL J1902.3-6802    |     |       |                  |
| J1903.2+5541  | 285.821 | 55.685  | 85.979  | 20.530  | 0.020      | 0.018      | -87    | 46.9     | 4.4      | 0.2             | 37.8     | 2.3             | 1.93          | ...                  | LP  | T   | ...     | 1FHL J1903.4+5541    | ... | bl    | TXS 1902+556     |
|               |         |         |         |         |            |            |        |          |          |                 |          |                 |               |                      |     |     |         | 2FGL J1903.3+5539    |     |       |                  |
|               |         |         |         |         |            |            |        |          |          |                 |          |                 |               |                      |     |     |         | 1FGL J1903.0+5539    |     |       |                  |
| J1903.6-7052  | 285.916 | -70.879 | 324.372 | -26.511 | 0.054      | 0.051      | 16     | 16.3     | 1.0      | 0.1             | 12.3     | 1.0             | 2.32          | 0.07                 | PL  | ... | 10      | 2FGL J1902.7-7053    | ... | PSR   | PSR J1903-7051   |
|               |         |         |         |         |            |            |        |          |          |                 |          |                 |               |                      |     |     |         | 1FGL J1901.6-7051    |     |       |                  |
| J1903.9+0052  | 285.998 | 0.870   | 35.139  | -2.396  | 0.079      | 0.071      | 79     | 4.4      | 0.9      | 0.2             | 10.2     | 3.0             | 2.14          | 0.20                 | PL  | ... | ...     | ...                  | ... | ...   | ...              |
| J1904.5+3627  | 286.138 | 36.459  | 67.335  | 13.299  | 0.112      | 0.076      | 58     | 6.2      | 0.4      | 0.1             | 4.8      | 0.9             | 2.10          | 0.17                 | PL  | ... | ...     | ...                  | ... | bcu   | MG2 J190411+3627 |
| J1904.7-0708  | 286.198 | -7.138  | 28.071  | -6.205  | 0.067      | 0.062      | 48     | 11.7     | 1.3      | 0.2             | 21.4     | 2.1             | 2.59          | 0.08                 | PL  | ... | 3       | 2FGL J1904.8-0705    | ... | ...   | ...              |
|               |         |         |         |         |            |            |        |          |          |                 |          |                 |               |                      |     |     |         | 1FGL J1904.4-0703    |     |       |                  |

Table 1—Continued

| Name 3FGL    | R.A.    | Decl.   | $l$     | $b$     | $\theta_1$ | $\theta_2$ | $\phi$ | $\sigma$ | $F_{35}$ | $\Delta F_{35}$ | $S_{25}$ | $\Delta S_{25}$ | $\Gamma_{25}$ | $\Delta \Gamma_{25}$ | Mod | Var | Flags    | $\gamma$ -ray Assoc.                                                                            | TeV | Class | ID or Assoc.             |
|--------------|---------|---------|---------|---------|------------|------------|--------|----------|----------|-----------------|----------|-----------------|---------------|----------------------|-----|-----|----------|-------------------------------------------------------------------------------------------------|-----|-------|--------------------------|
| J1904.9+0818 | 286.243 | 8.306   | 41.862  | 0.796   | 0.107      | 0.079      | 23     | 4.7      | 1.4      | 0.3             | 17.0     | 4.4             | 2.30          | 0.13                 | PL  | ... | 4,5      | ...                                                                                             | ... | ...   | ...                      |
| J1906.6+0720 | 286.671 | 7.334   | 41.193  | -0.028  | 0.037      | 0.027      | -39    | 26.3     | 12.9     | 0.6             | 99.5     | 5.8             | 2.24          | ...                  | LP  | ... | ...      | 2FGL J1906.5+0720<br>1FGL J1906.6+0716c                                                         | ... | ...   | ...                      |
| J1907.9+0602 | 286.986 | 6.039   | 40.187  | -0.901  | 0.013      | 0.013      | -46    | 84.0     | 38.4     | 0.7             | 319.1    | 5.6             | 2.24          | ...                  | EC  | ... | ...      | 1FHL J1907.7+0600<br>2FGL J1907.9+0602<br>1FGL J1907.9+0602<br>1AGL J1908+0614                  | E   | PSR   | LAT PSR J1907+0602       |
| J1908.8-0130 | 287.202 | -1.517  | 33.562  | -4.556  | 0.084      | 0.065      | -7     | 9.0      | 1.7      | 0.2             | 7.1      | 0.9             | 2.27          | ...                  | LP  | ... | 12       | 2FGL J1908.8-0132<br><br>1FGL J1908.5-0138                                                      | ... | bcu   | NVSS<br>J190836-012642   |
| J1908.9+1022 | 287.228 | 10.375  | 44.146  | 0.884   | 0.126      | 0.096      | -82    | 6.4      | 1.7      | 0.3             | 27.2     | 4.2             | 2.59          | 0.09                 | PL  | ... | 3,4      | ...                                                                                             | ... | ...   | ...                      |
| J1910.7-6000 | 287.695 | -60.000 | 336.474 | -25.621 | 0.092      | 0.084      | 6      | 8.0      | 0.5      | 0.1             | 5.9      | 0.9             | 2.20          | 0.10                 | PL  | ... | 3        | ...                                                                                             | ... | glc   | NGC 6752                 |
| J1910.8+2855 | 287.725 | 28.929  | 60.967  | 8.888   | 0.051      | 0.045      | -63    | 6.5      | 0.2      | 0.1             | 4.1      | 1.1             | 1.46          | 0.17                 | PL  | ... | ...      | ...                                                                                             | ... | bcu   | 1RXS<br>J191053.2+285622 |
| J1910.9+0906 | 287.744 | 9.101   | 43.250  | -0.155  | 0.017      | 0.016      | -80    | 41.8     | 20.3     | 0.7             | 183.5    | 7.7             | 2.18          | ...                  | LP  | ... | ...      | 1FHL J1911.0+0905<br>2FGL J1911.0+0905<br>1FGL J1910.9+0906c<br>0FGL J1911.0+0905               | ... | snr   | W 49B<br>-117-           |
| J1911.1-5318 | 287.795 | -53.303 | 343.716 | -24.291 | 0.191      | 0.156      | 40     | 4.6      | 0.3      | 0.1             | 4.4      | 0.9             | 2.45          | 0.14                 | PL  | ... | ...      | 1FGL J1911.1-5306                                                                               | ... | ...   | ...                      |
| J1911.2-2006 | 287.802 | -20.112 | 16.883  | -13.226 | 0.037      | 0.035      | -1     | 32.1     | 3.7      | 0.2             | 49.6     | 1.9             | 2.41          | 0.03                 | PL  | T   | ...      | 2FGL J1911.1-2005<br>1FGL J1911.2-2007<br>0FGL J1911.2-2011<br>3EG J1911-2000<br>EGR J1912-2000 | ... | fsrq  | PKS B1908-201            |
| J1911.4-1908 | 287.859 | -19.137 | 17.817  | -12.871 | 0.050      | 0.045      | -36    | 9.8      | 0.7      | 0.1             | 9.2      | 1.5             | 1.77          | 0.11                 | PL  | ... | ...      | 1FHL J1910.9-1906<br>2FGL J1911.5-1908<br>1FGL J1911.7+0307                                     | ... | bcu   | PMN J1911-1908           |
| J1911.7+0307 | 287.931 | 3.130   | 38.037  | -3.076  | 0.087      | 0.065      | -23    | 7.1      | 1.2      | 0.2             | 14.4     | 2.5             | 2.32          | 0.12                 | PL  | ... | ...      | ...                                                                                             | ... | ...   | ...                      |
| J1912.0-0804 | 288.023 | -8.080  | 28.036  | -8.244  | 0.085      | 0.069      | -76    | 5.7      | 0.7      | 0.1             | 8.5      | 1.7             | 2.30          | 0.15                 | PL  | T   | 3        | ...                                                                                             | ... | bcu   | PMN J1912-0804           |
| J1912.6-1223 | 288.164 | -12.398 | 24.170  | -10.269 | 0.100      | 0.085      | 0      | 10.8     | 1.1      | 0.1             | 16.1     | 1.7             | 2.49          | 0.09                 | PL  | T   | ...      | ...                                                                                             | ... | bcu   | TXS 1909-124             |
| J1912.7+4610 | 288.178 | 46.172  | 77.167  | 15.773  | 0.169      | 0.156      | 22     | 4.8      | 0.3      | 0.1             | 4.0      | 0.8             | 2.39          | 0.15                 | PL  | ... | ...      | ...                                                                                             | ... | ...   | ...                      |
| J1912.9-8008 | 288.234 | -80.149 | 314.015 | -27.615 | 0.053      | 0.045      | 83     | 21.3     | 2.0      | 0.1             | 18.8     | 1.4             | 2.32          | ...                  | LP  | T   | ...      | ...                                                                                             | ... | fsrq  | PKS 1903-80              |
| J1913.0+0910 | 288.261 | 9.182   | 43.558  | -0.570  | 0.097      | 0.079      | -59    | 10.1     | 5.3      | 0.6             | 41.2     | 6.3             | 2.39          | ...                  | EC  | ... | 5,7      | ...                                                                                             | ... | PSR   | PSR J1913+0904           |
| J1913.5-3631 | 288.385 | -36.533 | 1.204   | -19.895 | 0.101      | 0.080      | -35    | 6.3      | 0.6      | 0.1             | 6.8      | 1.2             | 2.16          | 0.12                 | PL  | T   | 1        | ...                                                                                             | ... | bcu   | PMN J1913-3630           |
| J1913.9+4441 | 288.496 | 44.691  | 75.846  | 14.984  | 0.090      | 0.056      | -24    | 8.1      | 0.4      | 0.1             | 5.2      | 1.0             | 1.85          | 0.13                 | PL  | ... | ...      | 2FGL J1913.4+4440                                                                               | ... | bcu   | 1RXS<br>J191401.9+443849 |
| J1915.2+0954 | 288.802 | 9.908   | 44.450  | -0.705  | 0.099      | 0.073      | 66     | 7.7      | 1.6      | 0.4             | 31.0     | 4.2             | 2.36          | ...                  | LP  | ... | 3,4,9,12 | ...                                                                                             | ... | ...   | ...                      |
| J1915.9+1112 | 289.000 | 11.216  | 45.698  | -0.268  | 0.147      | 0.120      | 2      | 10.7     | 3.8      | 0.5             | 38.2     | 4.1             | 2.41          | ...                  | LP  | ... | 3,4      | 2FGL J1916.1+1106<br>1FGL J1916.0+1110c                                                         | ... | spp   | ...                      |

Table 1—Continued

| Name 3FGL     | R.A.    | Decl.   | $l$     | $b$     | $\theta_1$ | $\theta_2$ | $\phi$ | $\sigma$ | $F_{35}$ | $\Delta F_{35}$ | $S_{25}$ | $\Delta S_{25}$ | $\Gamma_{25}$ | $\Delta \Gamma_{25}$ | Mod | Var | Flags | $\gamma$ -ray Assoc.                                                                                  | TeV | Class | ID or Assoc.             |
|---------------|---------|---------|---------|---------|------------|------------|--------|----------|----------|-----------------|----------|-----------------|---------------|----------------------|-----|-----|-------|-------------------------------------------------------------------------------------------------------|-----|-------|--------------------------|
| J1917.1–3024  | 289.289 | −30.417 | 7.551   | −18.469 | 0.091      | 0.076      | 19     | 9.5      | 0.9      | 0.1             | 10.3     | 1.3             | 2.24          | 0.10                 | PL  | ... | ...   | 2FGL J1917.0–3027<br>1FGL J1916.9–3028                                                                | ... | ...   | ...                      |
| J1917.7–1921  | 289.443 | −19.366 | 18.236  | −14.328 | 0.023      | 0.022      | 56     | 28.8     | 2.9      | 0.2             | 34.0     | 2.3             | 1.87          | 0.04                 | PL  | T   | ...   | 1FHL J1917.7–1921<br>2FGL J1917.6–1921<br>1FGL J1917.7–1922                                           | ... | bll   | 1H 1914–194              |
| J1918.0+3750  | 289.500 | 37.843  | 69.772  | 11.447  | 0.090      | 0.070      | −34    | 4.4      | 0.3      | 0.1             | 3.4      | 0.9             | 2.19          | 0.19                 | PL  | ... | ...   | ...                                                                                                   | ... | bcu   | 1RXS<br>J191810.2+375315 |
| J1918.2–4110  | 289.569 | −41.176 | 356.796 | −22.240 | 0.026      | 0.024      | −37    | 27.8     | 2.9      | 0.2             | 21.6     | 1.9             | 1.87          | ...                  | LP  | ... | ...   | 1FHL J1918.1–4109<br>2FGL J1918.2–4110<br>1FGL J1918.4–4108                                           | ... | bll   | PMN J1918–4111           |
| J1919.0+0452  | 289.761 | 4.874   | 40.431  | −3.888  | 0.187      | 0.142      | 79     | 4.9      | 0.7      | 0.2             | 12.2     | 2.4             | 2.60          | 0.13                 | PL  | ... | 4     | ...                                                                                                   | ... | ...   | ...                      |
| J1919.9+1407  | 289.981 | 14.118  | 48.710  | 0.242   | 0.078      | 0.062      | −44    | 10.9     | 4.4      | 0.5             | 46.9     | 5.3             | 2.44          | ...                  | LP  | ... | 3,5   | 1AGL J1922+1351                                                                                       | ... | ...   | ...                      |
| J1921.2+0136  | 290.307 | 1.607   | 37.779  | −5.884  | 0.105      | 0.074      | −37    | 9.3      | 1.3      | 0.2             | 15.9     | 1.9             | 2.34          | 0.09                 | PL  | ... | ...   | 2FGL J1921.3+0131<br>1FGL J1921.2+0132                                                                | ... | psr   | PSR J1921+01             |
| J1921.2+1506  | 290.308 | 15.109  | 49.734  | 0.428   | 0.282      | 0.241      | −62    | 8.7      | 1.8      | 0.3             | 30.5     | 3.6             | 2.53          | ...                  | LP  | ... | 5,12  | 1AGL J1922+1351                                                                                       | ... | ...   | ...                      |
| J1921.2–1232  | 290.316 | −12.550 | 24.956  | −12.229 | 0.050      | 0.042      | 58     | 10.6     | 1.0      | 0.1             | 11.1     | 1.5             | 2.04          | 0.09                 | PL  | ... | 3     | 2FGL J1921.3–1231<br>1FGL J1921.1–1234                                                                | ... | bll   | TXS 1918–126<br>$\infty$ |
| J1921.6+1934  | 290.407 | 19.581  | 53.727  | 2.446   | 0.133      | 0.107      | −71    | 4.2      | 0.8      | 0.2             | 11.7     | 2.6             | 2.49          | 0.13                 | PL  | ... | 4     | ...                                                                                                   | ... | ...   | ...                      |
| J1921.9–1607  | 290.486 | −16.124 | 21.704  | −13.892 | 0.032      | 0.030      | −60    | 14.1     | 0.9      | 0.1             | 14.0     | 2.0             | 1.62          | 0.08                 | PL  | ... | ...   | 1FHL J1922.0–1607<br>2FGL J1921.9–1608<br>1FGL J1922.0–1608                                           | ... | bll   | PMN J1921–1607           |
| J1922.2+2313  | 290.565 | 23.226  | 57.022  | 4.023   | 0.078      | 0.051      | 64     | 4.7      | 0.3      | 0.1             | 3.9      | 1.2             | 1.62          | 0.23                 | PL  | ... | 3     | ...                                                                                                   | ... | ...   | ...                      |
| J1923.2+1408e | 290.818 | 14.145  | 49.116  | −0.462  | ...        | ...        | ...    | 75.0     | 39.6     | 0.8             | 345.8    | 7.9             | 2.15          | ...                  | LP  | ... | ...   | 0FGL J1923.0+1411<br>1AGL J1922+1351<br>1FGL J1922.9+1411<br>1FHL J1923.2+1408e<br>2FGL J1923.2+1408e | E   | SNR   | W51C                     |
| J1923.2–7452  | 290.820 | −74.882 | 319.973 | −28.187 | 0.051      | 0.045      | 44     | 11.2     | 0.7      | 0.1             | 8.0      | 1.0             | 2.22          | 0.10                 | PL  | ... | ...   | 2FGL J1922.6–7454                                                                                     | ... | ...   | ...                      |
| J1923.5–2104  | 290.885 | −21.073 | 17.183  | −16.255 | 0.026      | 0.026      | −22    | 41.0     | 4.7      | 0.2             | 38.5     | 1.8             | 2.19          | ...                  | LP  | T   | ...   | 2FGL J1923.5–2105<br>1FGL J1923.5–2104<br>0FGL J1923.3–2101                                           | ... | fsrq  | TXS 1920–211             |
| J1924.8–1034  | 291.209 | −10.582 | 27.158  | −12.168 | 0.112      | 0.081      | 77     | 10.5     | 1.1      | 0.1             | 13.7     | 1.5             | 2.34          | 0.08                 | PL  | ... | 3     | 2FGL J1924.9–1036                                                                                     | ... | ...   | ...                      |
| J1924.8–2914  | 291.219 | −29.235 | 9.353   | −19.610 | 0.043      | 0.041      | 71     | 27.4     | 2.2      | 0.2             | 31.9     | 1.5             | 2.50          | 0.04                 | PL  | T   | ...   | 2FGL J1924.8–2912<br>1FGL J1925.2–2919                                                                | ... | fsrq  | PKS B1921–293            |
| J1924.9+2817  | 291.237 | 28.300  | 61.810  | 5.855   | 0.058      | 0.054      | 49     | 5.8      | 0.4      | 0.1             | 4.9      | 1.1             | 1.88          | 0.18                 | PL  | ... | 3     | ...                                                                                                   | ... | bcu   | NVSS<br>J192502+281542   |
| J1925.4+1605  | 291.353 | 16.096  | 51.080  | 0.007   | 0.149      | 0.093      | 54     | 8.9      | 2.8      | 0.3             | 36.3     | 4.3             | 2.38          | 0.07                 | PL  | ... | 3,4   | 1FGL J1926.1+1601c                                                                                    | ... | ...   | ...                      |

Table 1—Continued

| Name 3FGL     | R.A.    | Decl.   | $l$     | $b$     | $\theta_1$ | $\theta_2$ | $\phi$ | $\sigma$ | $F_{35}$ | $\Delta F_{35}$ | $S_{25}$ | $\Delta S_{25}$ | $\Gamma_{25}$ | $\Delta \Gamma_{25}$ | Mod | Var | Flags | $\gamma$ -ray Assoc.                                        | TeV | Class | ID or Assoc.             |
|---------------|---------|---------|---------|---------|------------|------------|--------|----------|----------|-----------------|----------|-----------------|---------------|----------------------|-----|-----|-------|-------------------------------------------------------------|-----|-------|--------------------------|
| J1925.4+1727  | 291.373 | 17.463  | 52.292  | 0.639   | 0.103      | 0.086      | −16    | 9.6      | 3.8      | 0.4             | 21.1     | 3.5             | 2.36          | ...                  | LP  | ... | ...   | 2FGL J1924.8+1724c<br>1FGL J1925.0+1720c<br>3EG J1928+1733  | ... | ...   | ...                      |
| J1925.7+1228  | 291.428 | 12.467  | 47.919  | −1.779  | 0.121      | 0.110      | 23     | 6.4      | 1.3      | 0.2             | 21.3     | 3.3             | 2.61          | 0.10                 | PL  | T   | 1,4   | ...                                                         | ... | bcu   | TXS 1923+123             |
| J1925.8−7826  | 291.451 | −78.438 | 315.935 | −28.254 | 0.221      | 0.164      | −76    | 6.2      | 0.5      | 0.1             | 7.3      | 1.2             | 2.51          | 0.12                 | PL  | ... | 1     | 2FGL J1925.7−7836c                                          | ... | ...   | ...                      |
| J1926.8+6154  | 291.707 | 61.902  | 93.299  | 19.741  | 0.023      | 0.023      | −25    | 26.1     | 1.7      | 0.1             | 20.4     | 1.5             | 1.86          | 0.05                 | PL  | T   | ...   | 1FHL J1926.9+6153                                           | ... | bl    | 1RXS<br>J192649.5+615445 |
|               |         |         |         |         |            |            |        |          |          |                 |          |                 |               |                      |     |     |       | 2FGL J1927.0+6153<br>1FGL J1926.8+6153                      |     |       |                          |
| J1927.7+6118  | 291.928 | 61.308  | 92.751  | 19.430  | 0.033      | 0.030      | −5     | 15.6     | 1.1      | 0.1             | 12.8     | 1.1             | 2.27          | 0.07                 | PL  | ... | ...   | 2FGL J1927.5+6117                                           | ... | bl    | S4 1926+61               |
| J1928.4+1838  | 292.113 | 18.634  | 53.656  | 0.577   | 0.175      | 0.131      | −23    | 5.8      | 1.6      | 0.3             | 21.9     | 4.1             | 2.42          | 0.11                 | PL  | ... | 1,4,5 | ...                                                         | ... | ...   | ...                      |
| J1928.9+1739  | 292.237 | 17.657  | 52.854  | 0.007   | 0.080      | 0.058      | −5     | 8.5      | 3.5      | 0.4             | 25.0     | 4.2             | 2.32          | ...                  | LP  | ... | 3,4   | 2FGL J1928.8+1740c<br>1FGL J1929.0+1741c<br>3EG J1928+1733  | ... | ...   | ...                      |
| J1931.1+1659  | 292.779 | 16.991  | 52.519  | −0.766  | 0.189      | 0.115      | −17    | 5.1      | 1.6      | 0.3             | 20.5     | 3.9             | 2.37          | 0.10                 | PL  | ... | 1,4   | 1FGL J1930.8+1653c                                          | ... | ...   | ...                      |
| J1931.1+0937  | 292.783 | 9.630   | 46.053  | −4.298  | 0.021      | 0.019      | −38    | 26.3     | 3.2      | 0.2             | 37.9     | 2.6             | 1.87          | 0.05                 | PL  | T   | ...   | 1FHL J1931.0+0938<br>2FGL J1931.1+0938<br>1FGL J1931.2+0939 | ... | bl    | RX J1931.1+0937          |
| J1932.2+1916  | 293.058 | 19.268  | 54.641  | 0.098   | 0.047      | 0.043      | 84     | 24.8     | 7.8      | 0.4             | 65.7     | 3.7             | 2.41          | ...                  | EC  | ... | 3     | 2FGL J1932.1+1913<br>1FGL J1932.1+1914c                     | ... | PSR   | LAT PSR J1932+1916       |
| J1932.6−4537  | 293.170 | −45.628 | 352.845 | −25.934 | 0.096      | 0.087      | 44     | 8.5      | 0.5      | 0.1             | 7.7      | 1.0             | 2.52          | 0.11                 | PL  | T   | ...   | ...                                                         | ... | fsrq  | PKS 1929−457             |
| J1933.4+0727  | 293.351 | 7.464   | 44.409  | −5.823  | 0.085      | 0.064      | 7      | 6.3      | 0.5      | 0.1             | 6.2      | 1.4             | 1.74          | 0.16                 | PL  | ... | ...   | 2FGL J1933.3+0722                                           | ... | bcu   | 1RXS<br>J193320.3+072616 |
|               |         |         |         |         |            |            |        |          |          |                 |          |                 |               |                      |     |     |       | 1FGL J1933.3+0723                                           |     |       |                          |
| J1934.2+6002  | 293.550 | 60.040  | 91.827  | 18.216  | 0.072      | 0.056      | 33     | 6.6      | 0.3      | 0.1             | 3.7      | 0.7             | 2.14          | 0.17                 | PL  | ... | ...   | ...                                                         | ... | ...   | ...                      |
| J1935.2−7924c | 293.803 | −79.408 | 314.799 | −28.638 | 0.119      | 0.111      | −31    | 6.6      | 0.5      | 0.1             | 8.6      | 1.4             | 2.56          | 0.10                 | PL  | ... | 1,5,6 | 1FGL J1927.3−7932c                                          | ... | ...   | ...                      |
| J1935.5+8355  | 293.897 | 83.927  | 116.309 | 25.811  | 0.121      | 0.089      | −76    | 6.5      | 0.3      | 0.1             | 4.1      | 0.7             | 2.35          | 0.13                 | PL  | ... | ...   | 2FGL J1936.9+8402                                           | ... | bcu   | 6C B194425+834912        |
| J1936.6−4215  | 294.164 | −42.266 | 356.664 | −25.836 | 0.200      | 0.154      | 15     | 4.1      | 0.3      | 0.1             | 4.1      | 0.9             | 2.31          | 0.15                 | PL  | ... | ...   | ...                                                         | ... | ...   | ...                      |
| J1936.9−4719  | 294.245 | −47.329 | 351.168 | −27.023 | 0.033      | 0.032      | −5     | 12.4     | 0.6      | 0.1             | 9.2      | 1.5             | 1.64          | 0.10                 | PL  | ... | ...   | 1FHL J1936.8−4721<br>2FGL J1936.8−4721<br>1FGL J1936.9−4720 | ... | bl    | PMN J1936−4719           |
| J1937.0−3956  | 294.274 | −39.940 | 359.183 | −25.327 | 0.120      | 0.086      | −83    | 15.6     | 0.9      | 0.1             | 16.3     | 1.2             | 2.68          | 0.07                 | PL  | T   | ...   | 2FGL J1937.2−3955<br>1FGL J1938.2−3957                      | ... | fsrq  | PKS 1933−400             |
| J1939.6−4925  | 294.921 | −49.430 | 348.938 | −27.861 | 0.086      | 0.061      | 49     | 6.0      | 0.3      | 0.1             | 4.1      | 1.1             | 1.62          | 0.15                 | PL  | ... | ...   | ...                                                         | ... | bcu   | SUMSS<br>J193946−492539  |
| J1941.2−6210  | 295.302 | −62.175 | 334.521 | −29.523 | 0.060      | 0.054      | 34     | 19.5     | 1.4      | 0.1             | 18.7     | 1.2             | 2.43          | 0.05                 | PL  | T   | ...   | 2FGL J1940.8−6213                                           | ... | bcu   | PKS 1936−623             |
| J1941.8+7218  | 295.452 | 72.316  | 104.277 | 22.055  | 0.113      | 0.104      | 65     | 10.6     | 0.6      | 0.1             | 9.6      | 1.0             | 2.54          | 0.08                 | PL  | T   | ...   | 2FGL J1941.6+7218                                           | ... | bcu   | 87GB<br>194202.1+721428  |
|               |         |         |         |         |            |            |        |          |          |                 |          |                 |               |                      |     |     |       | 1FGL J1941.6+7214                                           |     |       |                          |

Table 1—Continued

| Name 3FGL    | R.A.    | Decl.   | $l$     | $b$     | $\theta_1$ | $\theta_2$ | $\phi$ | $\sigma$ | $F_{35}$ | $\Delta F_{35}$ | $S_{25}$ | $\Delta S_{25}$ | $\Gamma_{25}$ | $\Delta \Gamma_{25}$ | Mod | Var | Flags | $\gamma$ -ray Assoc.                                                             | TeV | Class | ID or Assoc.             |
|--------------|---------|---------|---------|---------|------------|------------|--------|----------|----------|-----------------|----------|-----------------|---------------|----------------------|-----|-----|-------|----------------------------------------------------------------------------------|-----|-------|--------------------------|
| J1942.7+1033 | 295.693 | 10.550  | 48.249  | -6.365  | 0.023      | 0.023      | -35    | 23.1     | 2.5      | 0.2             | 30.1     | 2.4             | 1.82          | 0.05                 | PL  | ... | ...   | 1FHL J1942.8+1034                                                                | ... | bcu   | 1RXS<br>J194246.3+103339 |
|              |         |         |         |         |            |            |        |          |          |                 |          |                 |               |                      |     |     |       | 2FGL J1942.8+1033<br>1FGL J1942.7+1033                                           |     |       |                          |
| J1943.2-3510 | 295.817 | -35.168 | 4.628   | -25.200 | 0.152      | 0.138      | -35    | 6.9      | 0.5      | 0.1             | 7.8      | 1.1             | 2.59          | 0.12                 | PL  | ... | ...   | ...                                                                              | ... | bll   | 1RXS<br>J194306.8-351001 |
| J1943.8+2518 | 295.971 | 25.303  | 61.222  | 0.709   | 0.123      | 0.089      | 20     | 6.4      | 1.3      | 0.2             | 16.7     | 2.8             | 2.35          | 0.10                 | PL  | ... | 1,4   | ...                                                                              | ... | ...   | ...                      |
| J1944.0-0535 | 296.000 | -5.591  | 33.906  | -14.229 | 0.107      | 0.087      | -85    | 4.4      | 0.4      | 0.1             | 5.4      | 1.4             | 2.35          | 0.20                 | PL  | ... | ...   | ...                                                                              | ... | ...   | ...                      |
| J1944.1+3919 | 296.039 | 39.325  | 73.482  | 7.584   | 0.078      | 0.066      | -56    | 6.2      | 0.5      | 0.1             | 5.9      | 1.1             | 2.18          | 0.13                 | PL  | ... | ...   | ...                                                                              | ... | ...   | ...                      |
| J1944.1-4523 | 296.045 | -45.398 | 353.579 | -27.854 | 0.052      | 0.047      | -70    | 5.4      | 0.2      | 0.1             | 2.5      | 0.9             | 1.56          | 0.26                 | PL  | ... | ...   | ...                                                                              | ... | bcu   | 1RXS<br>J194422.6-452326 |
| J1944.8+4300 | 296.222 | 43.005  | 76.807  | 9.241   | 0.095      | 0.090      | 9      | 4.3      | 0.3      | 0.1             | 3.6      | 0.9             | 2.02          | 0.19                 | PL  | ... | ...   | ...                                                                              | ... | ...   | ...                      |
| J1945.3+7329 | 296.344 | 73.490  | 105.563 | 22.223  | 0.266      | 0.211      | -7     | 4.2      | 0.3      | 0.1             | 4.2      | 0.9             | 2.54          | 0.14                 | PL  | ... | 5     | 2FGL J1944.3+7325                                                                | ... | ...   | ...                      |
| J1945.9-3115 | 296.486 | -31.263 | 8.922   | -24.574 | 0.072      | 0.058      | 49     | 11.0     | 0.9      | 0.1             | 11.6     | 1.2             | 2.35          | 0.08                 | PL  | ... | ...   | 2FGL J1946.1-3115<br>1FGL J1946.1-3118                                           | ... | bll   | PKS 1942-313             |
| J1946.4-5403 | 296.614 | -54.057 | 343.888 | -29.563 | 0.063      | 0.052      | -63    | 20.3     | 1.7      | 0.1             | 11.3     | 0.9             | 2.19          | ...                  | LP  | ... | ...   | 2FGL J1946.4-5402<br>1FGL J1946.7-5404                                           | ... | ...   | ...                      |
| J1947.4-1121 | 296.857 | -11.354 | 28.899  | -17.508 | 0.213      | 0.157      | -11    | 5.4      | 0.5      | 0.1             | 6.6      | 1.3             | 2.28          | 0.12                 | PL  | ... | 1     | 2FGL J1946.7-1118                                                                | ... | ...   | ...                      |
| J1947.9-0743 | 296.979 | -7.720  | 32.376  | -16.045 | 0.147      | 0.128      | -47    | 6.1      | 0.6      | 0.1             | 7.6      | 1.3             | 2.39          | 0.12                 | PL  | ... | 1     | 2FGL J1947.8-0739                                                                | ... | ...   | ...                      |
| J1948.1-7059 | 297.037 | -70.989 | 324.353 | -30.140 | 0.169      | 0.123      | 62     | 4.1      | 0.3      | 0.1             | 4.1      | 1.0             | 2.58          | 0.18                 | PL  | ... | ...   | ...                                                                              | ... | ...   | ...                      |
| J1949.0+1312 | 297.257 | 13.210  | 51.336  | -6.387  | 0.054      | 0.049      | 18     | 6.1      | 0.6      | 0.1             | 6.9      | 1.5             | 2.16          | 0.13                 | PL  | ... | ...   | ...                                                                              | ... | bcu   | 87GB<br>194635.4+130713  |
| J1949.3+2433 | 297.329 | 24.565  | 61.204  | -0.727  | 0.080      | 0.065      | 29     | 8.2      | 2.4      | 0.3             | 16.9     | 2.6             | 2.38          | ...                  | LP  | ... | 1,3,4 | ...                                                                              | ... | ...   | ...                      |
| J1949.4-6140 | 297.364 | -61.680 | 335.134 | -30.474 | 0.125      | 0.114      | 28     | 4.7      | 0.3      | 0.1             | 3.6      | 0.9             | 2.31          | 0.20                 | PL  | ... | ...   | ...                                                                              | ... | bcu   | PMN J1949-6137           |
| J1949.5-1454 | 297.394 | -14.914 | 25.714  | -19.463 | 0.165      | 0.119      | -65    | 5.8      | 0.6      | 0.1             | 6.9      | 1.2             | 2.32          | 0.11                 | PL  | ... | 1     | 2FGL J1949.4-1457                                                                | ... | ...   | ...                      |
| J1949.6+2355 | 297.410 | 23.925  | 60.690  | -1.115  | 0.103      | 0.098      | -7     | 4.7      | 1.0      | 0.2             | 12.1     | 2.9             | 2.29          | 0.13                 | PL  | ... | ...   | 2FGL J1949.7+2405                                                                | ... | ...   | ...                      |
| J1949.7-8109 | 297.438 | -81.164 | 312.719 | -29.011 | 0.165      | 0.146      | 5      | 5.5      | 0.5      | 0.1             | 6.5      | 1.2             | 2.33          | 0.12                 | PL  | ... | 1     | ...                                                                              | ... | ...   | ...                      |
| J1950.2+1215 | 297.559 | 12.255  | 50.650  | -7.117  | 0.165      | 0.128      | 81     | 9.4      | 0.9      | 0.1             | 16.1     | 1.8             | 2.63          | 0.08                 | PL  | ... | ...   | 2FGL J1950.3+1223<br>1FGL J1950.4+1226                                           | ... | ...   | ...                      |
| J1951.3+6909 | 297.833 | 69.156  | 101.455 | 20.140  | 0.118      | 0.116      | 9      | 5.7      | 0.3      | 0.1             | 5.3      | 0.9             | 2.70          | 0.13                 | PL  | ... | 1     | ...                                                                              | ... | ...   | ...                      |
| J1951.6+2926 | 297.906 | 29.450  | 65.670  | 1.317   | 0.166      | 0.112      | -70    | 6.2      | 1.7      | 0.3             | 10.1     | 2.1             | 2.32          | ...                  | LP  | ... | 1     | ...                                                                              | ... | spp   | ...                      |
| J1951.8-1102 | 297.969 | -11.034 | 29.691  | -18.359 | 0.139      | 0.106      | -89    | 4.1      | 0.4      | 0.1             | 4.7      | 1.3             | 2.10          | 0.16                 | PL  | ... | 5     | ...                                                                              | ... | ...   | ...                      |
| J1952.9+3253 | 298.250 | 32.893  | 68.782  | 2.826   | 0.015      | 0.014      | 63     | 85.6     | 20.3     | 0.4             | 151.2    | 2.8             | 2.17          | ...                  | EC  | ... | ...   | 0FGL J1953.2+3249<br>1FGL J1952.9+3252<br>1FHL J1953.3+3251<br>2FGL J1953.0+3253 | ... | PSR   | PSR J1952+3252           |
| J1953.3+3847 | 298.329 | 38.798  | 73.910  | 5.779   | 0.179      | 0.140      | 1      | 5.8      | 0.6      | 0.1             | 10.0     | 1.8             | 2.56          | 0.12                 | PL  | ... | ...   | ...                                                                              | ... | ...   | ...                      |
| J1953.4+7653 | 298.362 | 76.890  | 109.200 | 22.963  | 0.145      | 0.124      | 3      | 5.2      | 0.3      | 0.1             | 4.1      | 0.9             | 2.36          | 0.14                 | PL  | ... | 5     | ...                                                                              | ... | ...   | ...                      |
| J1954.2+2836 | 298.574 | 28.605  | 65.245  | 0.383   | 0.019      | 0.019      | 69     | 47.8     | 15.0     | 0.5             | 107.7    | 3.7             | 2.18          | ...                  | EC  | ... | ...   | 2FGL J1954.3+2836                                                                | ... | PSR   | LAT PSR J1954+2836       |



Table 1—Continued

| Name 3FGL    | R.A.    | Decl.   | $l$     | $b$     | $\theta_1$ | $\theta_2$ | $\phi$ | $\sigma$ | $F_{35}$ | $\Delta F_{35}$ | $S_{25}$ | $\Delta S_{25}$ | $\Gamma_{25}$ | $\Delta \Gamma_{25}$ | Mod | Var | Flags | $\gamma$ -ray Assoc.                                        | TeV | Class | ID or Assoc.             |
|--------------|---------|---------|---------|---------|------------|------------|--------|----------|----------|-----------------|----------|-----------------|---------------|----------------------|-----|-----|-------|-------------------------------------------------------------|-----|-------|--------------------------|
| J1954.8–1122 | 298.702 | –11.377 | 29.684  | –19.156 | 0.053      | 0.049      | –62    | 19.2     | 2.1      | 0.2             | 25.5     | 1.7             | 2.27          | 0.05                 | PL  | T   | ...   | 1FGL J1954.3+2836<br>0FGL J1954.4+2838<br>2FGL J1954.6–1122 | ... | fsrq  | TXS 1951–115             |
| J1954.9–5640 | 298.743 | –56.676 | 340.983 | –30.986 | 0.033      | 0.032      | –75    | 9.0      | 0.4      | 0.1             | 5.3      | 1.0             | 1.88          | 0.16                 | PL  | ... | ...   | 1FGL J1954.8–1124<br>2FGL J1955.0–5639                      | ... | bcu   | 1RXS<br>J195503.1–564031 |
| J1955.0–1605 | 298.751 | –16.091 | 25.125  | –21.133 | 0.044      | 0.042      | 45     | 10.0     | 0.8      | 0.1             | 8.9      | 1.3             | 2.05          | 0.10                 | PL  | ... | ...   | 2FGL J1954.4–1607                                           | ... | bcu   | 1RXS<br>J195500.6–160328 |
| J1955.1+1357 | 298.797 | 13.954  | 52.741  | –7.308  | 0.053      | 0.052      | –89    | 12.9     | 1.3      | 0.1             | 15.6     | 1.5             | 2.24          | 0.07                 | PL  | T   | ...   | 2FGL J1955.2+1356                                           | ... | fsrq  | 87GB<br>195252.4+135009  |
| J1955.7–7019 | 298.948 | –70.322 | 325.066 | –30.824 | 0.113      | 0.092      | –86    | 4.6      | 0.3      | 0.1             | 3.3      | 0.8             | 2.20          | 0.19                 | PL  | ... | ...   | 1FGL J1954.8+1402<br>...                                    | ... | ...   | ...                      |
| J1955.9+0212 | 298.977 | 2.206   | 42.439  | –13.258 | 0.078      | 0.059      | –10    | 6.1      | 0.5      | 0.1             | 5.3      | 1.2             | 1.93          | 0.15                 | PL  | ... | ...   | ...                                                         | ... | bcu   | NVSS<br>J195547+021514   |
| J1957.0–3234 | 299.251 | –32.583 | 8.288   | –27.206 | 0.242      | 0.180      | –54    | 5.4      | 0.3      | 0.1             | 6.4      | 1.1             | 2.71          | 0.14                 | PL  | ... | 1     | ...                                                         | ... | fsrq  | PKS 1953–325             |
| J1957.7+5034 | 299.434 | 50.570  | 84.605  | 11.008  | 0.040      | 0.039      | –1     | 39.6     | 3.1      | 0.2             | 32.2     | 1.2             | 2.42          | ...                  | EC  | ... | ...   | 2FGL J1957.9+5033<br>1FGL J1957.6+5033                      | ... | PSR   | LAT PSR J1957+5033       |
| J1957.9–0712 | 299.484 | –7.211  | 34.000  | –18.050 | 0.124      | 0.115      | 1      | 5.9      | 0.5      | 0.1             | 6.3      | 1.2             | 2.38          | 0.13                 | PL  | ... | 9     | ...                                                         | ... | ...   | ...                      |
| J1958.0–3847 | 299.518 | –38.784 | 1.547   | –28.980 | 0.034      | 0.032      | –6     | 37.7     | 3.0      | 0.2             | 34.8     | 1.4             | 2.39          | ...                  | LP  | T   | ...   | 2FGL J1958.2–3848<br>1FGL J1958.4–3847                      | ... | fsrq  | PKS 1954–388             |
| J1958.1+2436 | 299.526 | 24.614  | 62.274  | –2.415  | 0.064      | 0.047      | –37    | 5.3      | 0.4      | 0.2             | 6.0      | 1.7             | 1.68          | 0.22                 | PL  | ... | ...   | ...                                                         | ... | ...   | ...                      |
| J1958.1–0243 | 299.527 | –2.721  | 38.209  | –16.060 | 0.246      | 0.205      | –74    | 5.6      | 0.4      | 0.1             | 8.1      | 1.3             | 2.74          | 0.14                 | PL  | ... | 1     | ...                                                         | ... | ...   | ...                      |
| J1958.2–1413 | 299.568 | –14.222 | 27.299  | –21.104 | 0.178      | 0.146      | –26    | 5.1      | 0.4      | 0.1             | 6.0      | 1.2             | 2.41          | 0.12                 | PL  | ... | 1     | 3EG J1955–1414                                              | ... | ...   | ...                      |
| J1958.2–3011 | 299.575 | –30.190 | 10.949  | –26.780 | 0.052      | 0.046      | –18    | 7.1      | 0.5      | 0.1             | 6.0      | 1.2             | 1.82          | 0.17                 | PL  | ... | ...   | 1FHL J1958.4–3015                                           | ... | bll   | 1RXS<br>J195815.6–301119 |
| J1958.6+2845 | 299.663 | 28.762  | 65.876  | –0.352  | 0.019      | 0.019      | –19    | 48.9     | 14.9     | 0.5             | 99.0     | 3.3             | 2.18          | ...                  | EC  | ... | 10    | 2FGL J1958.4–3012<br>1FGL J1958.4–3013<br>1FHL J1958.6+2845 | ... | PSR   | LAT PSR J1958+2846       |
| J1958.6+3844 | 299.674 | 38.745  | 74.405  | 4.852   | 0.203      | 0.162      | –64    | 4.8      | 0.6      | 0.1             | 9.8      | 2.0             | 2.64          | 0.13                 | PL  | ... | 4,5   | 2FGL J1958.6+2845<br>1FGL J1958.6+2845<br>3EG J1958+2909    | ... | ...   | ...                      |
| J1959.1–4245 | 299.781 | –42.760 | 357.121 | –29.985 | 0.062      | 0.054      | –50    | 22.5     | 1.4      | 0.1             | 20.7     | 1.1             | 2.47          | 0.05                 | PL  | T   | ...   | 2FGL J1959.1–4245<br>1FGL J1959.3–4241                      | ... | fsrq  | PMN J1959–4246           |
| J1959.5+2047 | 299.893 | 20.798  | 59.187  | –4.693  | 0.058      | 0.053      | –2     | 17.2     | 2.5      | 0.2             | 17.9     | 1.5             | 2.36          | ...                  | EC  | ... | ...   | 2FGL J1959.5+2047<br>1FGL J1959.6+2047                      | ... | PSR   | PSR J1959+2048           |
| J1959.8–4725 | 299.964 | –47.428 | 351.801 | –30.856 | 0.030      | 0.028      | 58     | 19.2     | 1.4      | 0.1             | 11.1     | 1.4             | 1.81          | ...                  | LP  | ... | ...   | 2FGL J1959.9–4727                                           | ... | bcu   | SUMSS<br>J195945–472519  |
| J2000.0+6509 | 300.016 | 65.154  | 98.012  | 17.666  | 0.013      | 0.013      | 83     | 61.9     | 5.8      | 0.2             | 68.2     | 2.5             | 1.88          | 0.02                 | PL  | T   | ...   | 1FGL J1959.7–4730<br>1FHL J2000.0+6509<br>2FGL J2000.0+6509 | P   | bll   | 1ES 1959+650             |

Table 1—Continued

| Name 3FGL    | R.A.    | Decl.   | $l$     | $b$     | $\theta_1$ | $\theta_2$ | $\phi$ | $\sigma$ | $F_{35}$ | $\Delta F_{35}$ | $S_{25}$ | $\Delta S_{25}$ | $\Gamma_{25}$ | $\Delta \Gamma_{25}$ | Mod | Var | Flags | $\gamma$ -ray Assoc. | TeV | Class | ID or Assoc.     |
|--------------|---------|---------|---------|---------|------------|------------|--------|----------|----------|-----------------|----------|-----------------|---------------|----------------------|-----|-----|-------|----------------------|-----|-------|------------------|
|              |         |         |         |         |            |            |        |          |          |                 |          |                 |               |                      |     |     |       | 1FGL J2000.0+6508    |     |       |                  |
|              |         |         |         |         |            |            |        |          |          |                 |          |                 |               |                      |     |     |       | 0FGL J2000.2+6506    |     |       |                  |
| J2000.1+4212 | 300.029 | 42.209  | 77.523  | 6.416   | 0.069      | 0.057      | −43    | 7.4      | 0.8      | 0.1             | 10.7     | 1.6             | 2.47          | 0.10                 | PL  | ... | ...   | 2FGL J1959.9+4212    | ... | bcu   | MG4 J195957+4213 |
| J2000.4−2926 | 300.108 | −29.444 | 11.902  | −26.998 | 0.138      | 0.094      | 80     | 7.4      | 0.6      | 0.1             | 9.9      | 1.2             | 2.60          | 0.11                 | PL  | ... | ...   | 2FGL J1959.6−2931    | ... | fsrq  | PMN J2000−2931   |
| J2001.0−1750 | 300.259 | −17.845 | 23.989  | −23.146 | 0.040      | 0.036      | −8     | 21.1     | 1.8      | 0.1             | 22.4     | 1.4             | 2.31          | 0.05                 | PL  | T   | ...   | 1FHL J2001.1−1752    | ... | fsrq  | PKS 1958−179     |
|              |         |         |         |         |            |            |        |          |          |                 |          |                 |               |                      |     |     |       | 2FGL J2000.8−1751    |     |       |                  |
|              |         |         |         |         |            |            |        |          |          |                 |          |                 |               |                      |     |     |       | 1FGL J2000.9−1749    |     |       |                  |
| J2001.1+4352 | 300.297 | 43.880  | 79.064  | 7.113   | 0.012      | 0.012      | −15    | 55.8     | 8.1      | 0.3             | 91.7     | 3.1             | 1.97          | 0.02                 | PL  | T   | ...   | 1FHL J2001.1+4353    | P   | bl    | MG4 J200112+4352 |
|              |         |         |         |         |            |            |        |          |          |                 |          |                 |               |                      |     |     |       | 2FGL J2001.1+4352    |     |       |                  |
|              |         |         |         |         |            |            |        |          |          |                 |          |                 |               |                      |     |     |       | 1FGL J2001.1+4351    |     |       |                  |
|              |         |         |         |         |            |            |        |          |          |                 |          |                 |               |                      |     |     |       | 0FGL J2001.0+4352    |     |       |                  |
| J2001.8+7041 | 300.458 | 70.692  | 103.341 | 19.960  | 0.049      | 0.044      | 77     | 10.8     | 0.7      | 0.1             | 8.1      | 1.1             | 2.08          | 0.09                 | PL  | ... | ...   | 2FGL J2001.7+7042    | ... | bl    | TXS 2001+705     |
|              |         |         |         |         |            |            |        |          |          |                 |          |                 |               |                      |     |     |       | 1FGL J2001.9+7040    |     |       |                  |
| J2002.7+6303 | 300.697 | 63.057  | 96.207  | 16.437  | 0.080      | 0.067      | 26     | 5.4      | 0.3      | 0.1             | 3.4      | 0.8             | 2.13          | 0.22                 | PL  | ... | ...   | 1FHL J2002.6+6303    | ... | bcu   | 1RXS             |
|              |         |         |         |         |            |            |        |          |          |                 |          |                 |               |                      |     |     |       |                      |     |       | J200245.4+630226 |
| J2004.4+3338 | 301.103 | 33.645  | 70.671  | 1.185   | 0.035      | 0.033      | 43     | 18.5     | 3.6      | 0.3             | 43.1     | 2.8             | 2.30          | 0.04                 | PL  | ... | ...   | 1FHL J2004.4+3339    | ... | ...   | ...              |
|              |         |         |         |         |            |            |        |          |          |                 |          |                 |               |                      |     |     |       | 2FGL J2004.4+3339c   |     |       |                  |
|              |         |         |         |         |            |            |        |          |          |                 |          |                 |               |                      |     |     |       | 1FGL J2004.7+3343    |     |       |                  |
| J2004.8+7003 | 301.220 | 70.060  | 102.856 | 19.453  | 0.043      | 0.037      | 79     | 11.1     | 0.7      | 0.1             | 7.9      | 1.1             | 1.91          | 0.10                 | PL  | ... | ...   | 1FHL J2004.7+7003    | ... | bl    | 1RXS             |
|              |         |         |         |         |            |            |        |          |          |                 |          |                 |               |                      |     |     |       |                      |     |       | J200504.0+700445 |
|              |         |         |         |         |            |            |        |          |          |                 |          |                 |               |                      |     |     |       | 2FGL J2004.6+7004    |     |       |                  |
|              |         |         |         |         |            |            |        |          |          |                 |          |                 |               |                      |     |     |       | 1FGL J2004.8+7004    |     |       |                  |
| J2005.2+7752 | 301.310 | 77.881  | 110.461 | 22.749  | 0.036      | 0.034      | 76     | 25.4     | 1.8      | 0.1             | 20.7     | 1.1             | 2.22          | 0.04                 | PL  | T   | ...   | 2FGL J2004.5+7754    | ... | bl    | S5 2007+77       |
|              |         |         |         |         |            |            |        |          |          |                 |          |                 |               |                      |     |     |       | 1FGL J2006.0+7751    |     |       |                  |
| J2005.7−8241 | 301.438 | −82.699 | 310.866 | −29.230 | 0.130      | 0.115      | 0      | 4.6      | 0.3      | 0.1             | 5.5      | 1.1             | 2.68          | 0.15                 | PL  | ... | ...   | ...                  | ... | ...   | ...              |
| J2006.0−2311 | 301.506 | −23.193 | 18.973  | −26.177 | 0.132      | 0.099      | −12    | 11.0     | 0.8      | 0.1             | 11.5     | 1.2             | 2.50          | 0.08                 | PL  | T   | ...   | 1FGL J2006.6−2302    | ... | fsrq  | TXS 2002−233     |
|              |         |         |         |         |            |            |        |          |          |                 |          |                 |               |                      |     |     |       | 3EG J2006−2321       |     |       |                  |
| J2006.5−0939 | 301.628 | −9.666  | 32.637  | −21.029 | 0.201      | 0.170      | 5      | 4.3      | 0.4      | 0.1             | 4.8      | 1.1             | 2.44          | 0.14                 | PL  | ... | ...   | 2FGL J2006.2−0929    | ... | ...   | ...              |
| J2006.6+0150 | 301.659 | 1.846   | 43.443  | −15.782 | 0.067      | 0.064      | −24    | 5.5      | 0.4      | 0.1             | 4.2      | 1.0             | 1.87          | 0.13                 | PL  | ... | ...   | 1FGL J2007.0+0145    | ... | ...   | ...              |
| J2007.3+6605 | 301.835 | 66.092  | 99.249  | 17.432  | 0.121      | 0.102      | 85     | 8.2      | 0.5      | 0.1             | 8.4      | 1.1             | 2.59          | 0.09                 | PL  | T   | 5     | ...                  | ... | fsrq  | TXS 2007+659     |
| J2007.7−7728 | 301.949 | −77.475 | 316.699 | −30.548 | 0.151      | 0.117      | 33     | 9.3      | 0.5      | 0.1             | 8.8      | 1.0             | 2.68          | 0.10                 | PL  | T   | ...   | ...                  | ... | bcu   | PKS 2000−776     |
| J2007.8−4429 | 301.971 | −44.498 | 355.424 | −31.832 | 0.076      | 0.066      | 26     | 9.7      | 0.6      | 0.1             | 8.0      | 1.0             | 2.47          | 0.09                 | PL  | ... | ...   | 2FGL J2007.9−4430    | ... | nlsy1 | PKS 2004−447     |
|              |         |         |         |         |            |            |        |          |          |                 |          |                 |               |                      |     |     |       | 1FGL J2007.9−4430    |     |       |                  |
| J2009.2−1458 | 302.304 | −14.978 | 27.703  | −23.832 | 0.531      | 0.156      | 6      | 5.6      | 0.4      | 0.1             | 7.4      | 1.3             | 2.64          | 0.12                 | PL  | ... | 9     | 2FGL J2009.2−1505    | ... | ...   | ...              |
| J2009.3−4849 | 302.349 | −48.828 | 350.378 | −32.596 | 0.018      | 0.018      | −33    | 40.3     | 3.6      | 0.2             | 44.9     | 2.6             | 1.77          | 0.03                 | PL  | T   | ...   | 1FHL J2009.4−4849    | P   | BLL   | PKS 2005−489     |
|              |         |         |         |         |            |            |        |          |          |                 |          |                 |               |                      |     |     |       | 2FGL J2009.5−4850    |     |       |                  |
|              |         |         |         |         |            |            |        |          |          |                 |          |                 |               |                      |     |     |       | 1FGL J2009.5−4849    |     |       |                  |

Table 1—Continued

| Name 3FGL    | R.A.    | Decl.   | $l$     | $b$     | $\theta_1$ | $\theta_2$ | $\phi$ | $\sigma$ | $F_{35}$ | $\Delta F_{35}$ | $S_{25}$ | $\Delta S_{25}$ | $\Gamma_{25}$ | $\Delta \Gamma_{25}$ | Mod | Var | Flags | $\gamma$ -ray Assoc. | TeV | Class | ID or Assoc.     |
|--------------|---------|---------|---------|---------|------------|------------|--------|----------|----------|-----------------|----------|-----------------|---------------|----------------------|-----|-----|-------|----------------------|-----|-------|------------------|
| J2010.0–2120 | 302.506 | –21.334 | 21.275  | –26.399 | 0.167      | 0.119      | 29     | 4.5      | 0.4      | 0.1             | 4.3      | 1.0             | 2.05          | 0.14                 | PL  | ... | ...   | 0FGL J2009.4–4850    | ... | ...   | ...              |
| J2010.3+7228 | 302.576 | 72.467  | 105.350 | 20.142  | 0.052      | 0.045      | 52     | 18.4     | 1.4      | 0.1             | 13.5     | 1.1             | 2.32          | ...                  | LP  | T   | 3     | 2FGL J2009.7+7225    | ... | bll   | 4C +72.28        |
| J2011.1+4203 | 302.798 | 42.056  | 78.486  | 4.594   | 0.126      | 0.120      | –68    | 4.3      | 0.7      | 0.2             | 10.8     | 2.3             | 2.54          | 0.12                 | PL  | ... | 4     | 1FGL J2009.1+7228    | ... | ...   | ...              |
| J2012.0+4629 | 303.002 | 46.496  | 82.317  | 6.878   | 0.026      | 0.025      | –89    | 21.1     | 2.5      | 0.2             | 27.5     | 1.9             | 2.11          | 0.05                 | PL  | T   | ...   | 1FHL J2012.1+4629    | ... | bll   | 7C 2010+4619     |
| J2012.1–1643 | 303.033 | –16.721 | 26.242  | –25.160 | 0.298      | 0.270      | –87    | 8.1      | 0.3      | 0.1             | 6.9      | 0.9             | 2.66          | ...                  | LP  | T   | 12    | 2FGL J2012.1+4630    | ... | bll   | PMN J2012–1646   |
| J2014.3–0047 | 303.575 | –0.794  | 41.981  | –18.730 | 0.049      | 0.040      | –84    | 9.5      | 0.7      | 0.1             | 8.7      | 1.4             | 1.83          | 0.11                 | PL  | T   | ...   | 1FGL J2012.2+4629    | ... | bll   | PMN J2014–0047   |
| J2014.4+3606 | 303.615 | 36.109  | 73.860  | 0.797   | 0.119      | 0.106      | 51     | 4.5      | 1.1      | 0.2             | 15.0     | 3.4             | 2.40          | 0.11                 | PL  | ... | 5     | 2FGL J2014.0–0046    | ... | spp   | ...              |
| J2014.5+0648 | 303.641 | 6.810   | 48.931  | –15.039 | 0.062      | 0.045      | 38     | 9.0      | 0.7      | 0.1             | 7.9      | 1.4             | 1.92          | 0.13                 | PL  | ... | ...   | 1FGL J2014.5–0047    | ... | bcu   | NVSS             |
| J2014.5+5246 | 303.649 | 52.769  | 87.889  | 9.900   | 0.082      | 0.071      | –86    | 4.4      | 0.3      | 0.1             | 4.2      | 1.2             | 2.42          | 0.24                 | PL  | ... | ...   | 2FGL J2014.7+0646    | ... | bcu   | J201431+064849   |
| J2014.9+1623 | 303.743 | 16.398  | 57.364  | –10.115 | 0.075      | 0.060      | –90    | 5.7      | 0.5      | 0.1             | 6.0      | 1.2             | 2.41          | 0.15                 | PL  | ... | ...   | 1FGL J2014.4+0647    | ... | bcu   | 4C +16.67        |
| J2015.2–0138 | 303.812 | –1.647  | 41.306  | –19.344 | 0.053      | 0.045      | 25     | 12.7     | 1.1      | 0.1             | 12.0     | 1.3             | 2.15          | 0.07                 | PL  | ... | ...   | 2FGL J2014.9+1623    | ... | bll   | PKS 2012–017     |
| J2015.3–1431 | 303.849 | –14.531 | 28.806  | –25.025 | 0.068      | 0.060      | –45    | 4.8      | 0.2      | 0.1             | 2.9      | 0.9             | 1.77          | 0.22                 | PL  | ... | ...   | 1FGL J2015.3–0129    | ... | ...   | ...              |
| J2015.6+3709 | 303.908 | 37.161  | 74.865  | 1.186   | 0.030      | 0.024      | 77     | 32.1     | 9.3      | 0.4             | 93.5     | 4.3             | 2.39          | ...                  | LP  | T   | ...   | 1FHL J2015.3–1432    | ... | ...   | ...              |
| J2016.4–0905 | 304.102 | –9.084  | 34.341  | –22.980 | 0.035      | 0.030      | 70     | 18.4     | 1.4      | 0.1             | 15.7     | 1.5             | 1.98          | 0.07                 | PL  | T   | ...   | 1FHL J2015.8+3710    | P   | FSRQ  | MG2 J201534+3710 |
| J2017.3+0602 | 304.349 | 6.048   | 48.621  | –16.032 | 0.022      | 0.022      | 58     | 43.4     | 5.9      | 0.2             | 35.0     | 1.7             | 1.92          | ...                  | EC  | ... | ...   | 2FGL J2015.6+3709    | ... | PSR   | PSR J2017+0603   |
| J2017.6–4110 | 304.405 | –41.170 | 359.638 | –33.107 | 0.091      | 0.072      | 23     | 4.7      | 0.3      | 0.1             | 3.4      | 0.9             | 2.16          | 0.19                 | PL  | ... | ...   | 1FGL J2015.7+3708    | ... | bcu   | 1RXS             |
| J2017.6–1616 | 304.425 | –16.269 | 27.275  | –26.217 | 0.075      | 0.068      | 49     | 11.5     | 0.9      | 0.1             | 10.4     | 1.2             | 2.10          | 0.08                 | PL  | ... | ...   | 3EG J2016+3657       | ... | psr   | J201731.2–411452 |
| J2017.9+3627 | 304.485 | 36.459  | 74.542  | 0.411   | 0.034      | 0.032      | –55    | 25.0     | 10.2     | 0.5             | 65.2     | 4.2             | 2.34          | ...                  | LP  | ... | ...   | 2FGL J2016.3–0904    | E   | ...   | ...              |
| J2018.5+3851 | 304.632 | 38.860  | 76.593  | 1.664   | 0.053      | 0.044      | –15    | 7.9      | 1.7      | 0.2             | 19.2     | 2.9             | 2.23          | 0.10                 | PL  | ... | ...   | 1FGL J2016.2–0903    | ... | bcu   | TXS 2016+386     |

Table 1—Continued

| Name 3FGL     | R.A.    | Decl.   | $l$     | $b$     | $\theta_1$ | $\theta_2$ | $\phi$ | $\sigma$ | $F_{35}$ | $\Delta F_{35}$ | $S_{25}$ | $\Delta S_{25}$ | $\Gamma_{25}$ | $\Delta \Gamma_{25}$ | Mod | Var | Flags     | $\gamma$ -ray Assoc. | TeV | Class | ID or Assoc.                     |
|---------------|---------|---------|---------|---------|------------|------------|--------|----------|----------|-----------------|----------|-----------------|---------------|----------------------|-----|-----|-----------|----------------------|-----|-------|----------------------------------|
| J2018.6+4213  | 304.675 | 42.230  | 79.403  | 3.531   | 0.212      | 0.112      | 57     | 8.5      | 2.0      | 0.2             | 23.6     | 3.1             | 2.27          | 0.08                 | PL  | ... | 1,3       | 2FGL J2018.2+3850c   | ... | ...   | Cygnus Cocoon field <sup>a</sup> |
| J2021.0+4031e | 305.270 | 40.520  | 78.241  | 2.197   | ...        | ...        | ...    | ...      | 0.7      | ...             | 11.4     | ...             | 1.53          | ...                  | PL  | ... | 4,5       | 1AGL J2022+4032      | E   | SNR   | Gamma Cygni                      |
|               |         |         |         |         |            |            |        |          |          |                 |          |                 |               |                      |     |     |           | 1FGL J2020.0+4049    |     |       |                                  |
|               |         |         |         |         |            |            |        |          |          |                 |          |                 |               |                      |     |     |           | 1FHL J2021.0+4031e   |     |       |                                  |
| J2021.1+3651  | 305.278 | 36.861  | 75.233  | 0.113   | 0.009      | 0.009      | 36     | 145.1    | 68.8     | 0.8             | 503.7    | 5.8             | 2.17          | ...                  | EC  | ... | ...       | 2FGL J2019.1+4040    | E   | PSR   | PSR J2021+3651                   |
|               |         |         |         |         |            |            |        |          |          |                 |          |                 |               |                      |     |     |           | 1FHL J2021.0+3651    |     |       |                                  |
|               |         |         |         |         |            |            |        |          |          |                 |          |                 |               |                      |     |     |           | 2FGL J2021.0+3651    |     |       |                                  |
|               |         |         |         |         |            |            |        |          |          |                 |          |                 |               |                      |     |     |           | 1FGL J2021.0+3651    |     |       |                                  |
|               |         |         |         |         |            |            |        |          |          |                 |          |                 |               |                      |     |     |           | 0FGL J2020.8+3649    |     |       |                                  |
| J2021.5+4026  | 305.386 | 40.448  | 78.232  | 2.083   | 0.008      | 0.008      | -17    | 237.0    | 121.0    | 1.0             | 883.4    | 6.1             | 2.13          | ...                  | EC  | T   | 10        | 1AGL J2021+3652      | ... | PSR   | LAT PSR J2021+4026               |
|               |         |         |         |         |            |            |        |          |          |                 |          |                 |               |                      |     |     |           | 2FGL J2021.5+4026    |     |       |                                  |
|               |         |         |         |         |            |            |        |          |          |                 |          |                 |               |                      |     |     |           | 1FGL J2021.5+4026    |     |       |                                  |
|               |         |         |         |         |            |            |        |          |          |                 |          |                 |               |                      |     |     |           | 0FGL J2021.5+4026    |     |       |                                  |
| J2021.9+0630  | 305.485 | 6.503   | 49.629  | -16.771 | 0.086      | 0.078      | -16    | 7.5      | 0.6      | 0.1             | 7.1      | 1.2             | 2.06          | 0.13                 | PL  | ... | ...       | 1AGL J2022+4032      | ... | bll   | 87GB                             |
|               |         |         |         |         |            |            |        |          |          |                 |          |                 |               |                      |     |     |           | 2FGL J2021.5+0632    | ... |       | 201926.8+061922                  |
| J2022.2+3840  | 305.563 | 38.678  | 76.855  | 0.963   | 0.104      | 0.092      | 67     | 12.8     | 2.7      | 0.5             | 38.4     | 3.9             | 2.48          | ...                  | LP  | ... | 3,10,12   | 2FGL J2022.8+3843c   | ... | spp   | Cygnus Cocoon field <sup>a</sup> |
| J2022.2-7220  | 305.565 | -72.340 | 322.334 | -32.596 | 0.095      | 0.092      | 36     | 4.7      | 0.2      | 0.1             | 2.6      | 0.7             | 1.95          | 0.20                 | PL  | ... | ...       | ...                  | ... | ...   | ...                              |
| J2022.2-4515  | 305.572 | -45.250 | 354.892 | -34.455 | 0.096      | 0.084      | 87     | 8.7      | 0.6      | 0.1             | 7.0      | 0.9             | 2.35          | 0.10                 | PL  | ... | ...       | 2FGL J2022.3-4518    | ... | bll   | PMN J2022-4513                   |
|               |         |         |         |         |            |            |        |          |          |                 |          |                 |               |                      |     |     |           | 1FGL J2022.5-4532    |     |       |                                  |
| J2022.5+7612  | 305.649 | 76.208  | 109.303 | 21.140  | 0.051      | 0.042      | -46    | 16.2     | 1.2      | 0.1             | 15.8     | 1.1             | 2.35          | 0.05                 | PL  | ... | ...       | 2FGL J2022.5+7614    | ... | bll   | S5 2023+760                      |
| J2023.2+3154  | 305.804 | 31.902  | 71.404  | -3.071  | 0.106      | 0.075      | 41     | 5.9      | 0.8      | 0.2             | 9.0      | 1.8             | 2.07          | 0.12                 | PL  | ... | ...       | ...                  | ... | bcu   | 4C +31.56                        |
| J2023.5+4126  | 305.876 | 41.434  | 79.254  | 2.342   | 0.098      | 0.090      | 85     | 11.6     | 2.5      | 0.4             | 34.8     | 3.3             | 2.31          | ...                  | LP  | ... | 1,3,10,12 | ...                  | ... | ...   | Cygnus Cocoon field <sup>a</sup> |
| J2023.6-1139  | 305.911 | -11.652 | 32.622  | -25.683 | 0.054      | 0.046      | 24     | 13.9     | 1.1      | 0.1             | 11.9     | 1.4             | 1.96          | 0.07                 | PL  | ... | ...       | 2FGL J2023.4-1137    | ... | fsrq  | PMN J2023-1140                   |
|               |         |         |         |         |            |            |        |          |          |                 |          |                 |               |                      |     |     |           | 1FGL J2023.7-1141    |     |       |                                  |
| J2024.4-0848  | 306.102 | -8.809  | 35.551  | -24.639 | 0.058      | 0.051      | -78    | 9.0      | 0.5      | 0.1             | 6.7      | 1.3             | 1.70          | 0.14                 | PL  | ... | ...       | ...                  | ... | bcu   | 1RXS                             |
|               |         |         |         |         |            |            |        |          |          |                 |          |                 |               |                      |     |     |           |                      |     |       | J202428.9-084810                 |
| J2024.4-3254  | 306.108 | -32.905 | 9.623   | -32.864 | 0.187      | 0.139      | 28     | 11.1     | 0.5      | 0.1             | 11.0     | 1.0             | 2.79          | 0.10                 | PL  | T   | ...       | ...                  | ... | fsrq  | PKS 2021-330                     |
| J2024.6+0309  | 306.154 | 3.159   | 46.958  | -19.044 | 0.130      | 0.099      | 29     | 5.5      | 0.5      | 0.1             | 5.2      | 1.1             | 1.91          | 0.14                 | PL  | ... | ...       | ...                  | ... | ...   | ...                              |
| J2024.6+3747  | 306.172 | 37.797  | 76.407  | 0.065   | 0.229      | 0.140      | 0      | 7.0      | 2.3      | 1.0             | 20.0     | 3.2             | 2.40          | ...                  | LP  | ... | 1,5       | ...                  | ... | ...   | ...                              |
| J2024.8-2331  | 306.210 | -23.528 | 20.240  | -30.361 | 0.081      | 0.073      | -51    | 4.2      | 0.3      | 0.1             | 2.9      | 0.8             | 1.95          | 0.17                 | PL  | ... | ...       | ...                  | ... | ...   | ...                              |
| J2025.1-2858  | 306.277 | -28.976 | 14.175  | -32.028 | 0.094      | 0.076      | 39     | 4.5      | 0.3      | 0.1             | 3.7      | 0.9             | 2.19          | 0.22                 | PL  | ... | ...       | ...                  | ... | ...   | ...                              |
| J2025.2+3340  | 306.322 | 33.669  | 73.103  | -2.414  | 0.055      | 0.049      | -64    | 14.7     | 3.2      | 0.3             | 41.2     | 3.5             | 2.54          | ...                  | LP  | T   | 3         | 2FGL J2025.1+3341    | ... | bcu   | B2 2023+33                       |
| J2025.6-0736  | 306.422 | -7.601  | 36.896  | -24.392 | 0.022      | 0.021      | -13    | 63.1     | 7.0      | 0.2             | 72.9     | 2.1             | 2.33          | ...                  | LP  | T   | ...       | 1FHL J2025.8-0734    | ... | fsrq  | PKS 2023-07                      |
|               |         |         |         |         |            |            |        |          |          |                 |          |                 |               |                      |     |     |           | 2FGL J2025.6-0736    |     |       |                                  |
|               |         |         |         |         |            |            |        |          |          |                 |          |                 |               |                      |     |     |           | 1FGL J2025.6-0735    |     |       |                                  |

Table 1—Continued

| Name 3FGL     | R.A.    | Decl.   | $l$     | $b$     | $\theta_1$ | $\theta_2$ | $\phi$ | $\sigma$ | $F_{35}$ | $\Delta F_{35}$ | $S_{25}$ | $\Delta S_{25}$ | $\Gamma_{25}$ | $\Delta \Gamma_{25}$ | Mod | Var | Flags    | $\gamma$ -ray Assoc.                                                                                | TeV | Class | ID or Assoc.                          |     |
|---------------|---------|---------|---------|---------|------------|------------|--------|----------|----------|-----------------|----------|-----------------|---------------|----------------------|-----|-----|----------|-----------------------------------------------------------------------------------------------------|-----|-------|---------------------------------------|-----|
|               |         |         |         |         |            |            |        |          |          |                 |          |                 |               |                      |     |     |          | 0FGL J2025.6−0736<br>3EG J2025−0744<br>1AGL J2026−0732                                              |     |       |                                       |     |
| J2026.3+7644  | 306.581 | 76.742  | 109.917 | 21.206  | 0.087      | 0.071      | −70    | 5.0      | 0.2      | 0.1             | 2.9      | 0.8             | 1.84          | 0.19                 | PL  | ... | ...      | ...                                                                                                 | ... | bcu   | 1RXS<br>J202633.4+764432              |     |
| J2026.3+1430  | 306.587 | 14.515  | 57.260  | −13.439 | 0.093      | 0.074      | 49     | 7.1      | 0.5      | 0.1             | 6.2      | 1.0             | 2.16          | 0.12                 | PL  | ... | ...      | ...                                                                                                 | ... | ...   | ...                                   |     |
| J2026.4+4709  | 306.600 | 47.162  | 84.253  | 5.206   | 0.140      | 0.101      | 23     | 4.4      | 0.6      | 0.1             | 8.9      | 1.9             | 2.56          | 0.14                 | PL  | ... | 3,4      | ...                                                                                                 | ... | ...   | ...                                   |     |
| J2026.8+4003  | 306.716 | 40.053  | 78.492  | 1.025   | 0.228      | 0.112      | 82     | 9.0      | 2.4      | 0.4             | 30.7     | 3.7             | 2.28          | ...                  | LP  | ... | 1,3,5,12 | ...                                                                                                 | ... | ...   | Cygnus Cocoon field <sup>a</sup>      |     |
| J2026.8+2813  | 306.718 | 28.231  | 68.842  | −5.823  | 0.159      | 0.142      | 10     | 7.6      | 1.1      | 0.2             | 7.7      | 1.5             | 2.45          | ...                  | LP  | ... | 3        | ...                                                                                                 | ... | ...   | ...                                   |     |
| J2028.3+3332  | 307.084 | 33.542  | 73.368  | −3.005  | 0.023      | 0.022      | −86    | 38.6     | 10.1     | 0.4             | 64.1     | 3.3             | 2.25          | ...                  | EC  | ... | ...      | 2FGL J2028.3+3332                                                                                   | ... | PSR   | LAT PSR J2028+3332                    |     |
| J2028.5+4040c | 307.135 | 40.677  | 79.186  | 1.129   | 0.143      | 0.093      | −29    | 5.0      | 1.5      | 0.3             | 16.7     | 3.7             | 2.19          | 0.10                 | PL  | ... | 3,5,6    | ...                                                                                                 | ... | ...   | Cygnus Cocoon field <sup>a</sup>      |     |
| J2028.6+4110e | 307.170 | 41.170  | 79.601  | 1.396   | ...        | ...        | ...    | ...      | 58.0     | ...             | 657.5    | ...             | 2.17          | ...                  | PL  | ... | ...      | 1FHL J2028.6+4110e                                                                                  | E   | SFR   | Cygnus Cocoon                         |     |
| J2028.7+1012  | 307.191 | 10.207  | 53.842  | −16.266 | 0.125      | 0.092      | −78    | 4.3      | 0.3      | 0.1             | 4.6      | 1.2             | 2.45          | 0.17                 | PL  | ... | ...      | ...                                                                                                 | ... | ...   | ...                                   |     |
| J2029.4+4923  | 307.357 | 49.400  | 86.380  | 6.088   | 0.061      | 0.055      | −11    | 13.7     | 1.8      | 0.2             | 24.1     | 1.9             | 2.41          | 0.06                 | PL  | T   | 10       | 2FGL J2029.4+4924<br>1FGL J2029.2+4924                                                              | ... | bll   | MG4 J202932+4925<br> <br>J2029.2+4924 |     |
| J2029.5−4232  | 307.389 | −42.537 | 358.345 | −35.488 | 0.216      | 0.174      | 48     | 6.4      | 0.4      | 0.1             | 6.0      | 0.9             | 2.50          | 0.11                 | PL  | ... | ...      | EGR J2027−4206                                                                                      | ... | ...   | ...                                   | ... |
| J2030.0+3642  | 307.501 | 36.703  | 76.133  | −1.432  | 0.030      | 0.027      | 18     | 27.7     | 7.8      | 0.4             | 45.8     | 2.8             | 2.17          | ...                  | EC  | ... | ...      | 2FGL J2030.0+3640<br>1FGL J2030.0+3641                                                              | ... | PSR   | PSR J2030+3641<br> <br>J2030.0+3641   |     |
| J2030.2−0622  | 307.570 | −6.371  | 38.668  | −24.857 | 0.070      | 0.064      | −62    | 9.8      | 0.6      | 0.1             | 10.7     | 1.3             | 2.64          | 0.11                 | PL  | T   | ...      | 2FGL J2030.3−0622<br>1FGL J2030.3−0617                                                              | ... | fsrq  | TXS 2027−065                          |     |
| J2030.5−1439  | 307.629 | −14.654 | 30.304  | −28.432 | 0.075      | 0.065      | 42     | 4.4      | 0.2      | 0.1             | 2.6      | 0.8             | 1.87          | 0.22                 | PL  | ... | ...      | ...                                                                                                 | ... | ...   | ...                                   |     |
| J2030.8+4416  | 307.716 | 44.270  | 82.349  | 2.890   | 0.039      | 0.038      | 22     | 24.9     | 7.2      | 0.4             | 52.4     | 3.1             | 2.31          | ...                  | EC  | ... | ...      | 2FGL J2030.7+4417<br>1FGL J2030.9+4411                                                              | ... | PSR   | LAT PSR J2030+4415                    |     |
| J2031.0+1937  | 307.761 | 19.619  | 62.243  | −11.530 | 0.055      | 0.051      | −14    | 8.9      | 0.6      | 0.1             | 7.0      | 1.2             | 1.83          | 0.12                 | PL  | ... | ...      | 1FHL J2031.4+1941<br>2FGL J2031.0+1938                                                              | ... | bcu   | RX J2030.8+1935                       |     |
| J2031.8+1223  | 307.953 | 12.387  | 56.170  | −15.714 | 0.086      | 0.072      | −23    | 8.4      | 0.7      | 0.1             | 10.3     | 1.5             | 2.45          | 0.10                 | PL  | ... | ...      | 2FGL J2031.7+1223<br>1FGL J2031.5+1219<br>EGR J2032+1226                                            | ... | bll   | PKS 2029+121                          |     |
| J2032.2+4126  | 308.060 | 41.447  | 80.219  | 1.019   | 0.014      | 0.014      | 17     | 63.2     | 24.6     | 0.6             | 160.5    | 4.8             | 2.08          | ...                  | EC  | ... | ...      | 1FHL J2032.1+4125<br>2FGL J2032.2+4126<br>1FGL J2032.2+4127<br>0FGL J2032.2+4122<br>1AGL J2032+4102 | E   | PSR   | LAT PSR J2032+4127                    |     |
| J2032.5+4032  | 308.125 | 40.535  | 79.514  | 0.438   | 0.165      | 0.115      | 7      | 16.1     | 4.5      | 0.5             | 54.8     | 4.3             | 2.43          | ...                  | LP  | T   | ...      | 1AGL J2032+4102                                                                                     | ... | ...   | Cygnus Cocoon field <sup>a</sup>      |     |
| J2032.5+3921  | 308.139 | 39.359  | 78.574  | −0.269  | 0.095      | 0.069      | 52     | 11.3     | 4.1      | 0.4             | 31.7     | 3.7             | 2.32          | ...                  | LP  | ... | 3        | 1FGL J2032.8+3928                                                                                   | ... | ...   | Cygnus Cocoon field <sup>a</sup>      |     |
| J2033.3+4348c | 308.338 | 43.812  | 82.244  | 2.258   | 0.074      | 0.063      | −74    | 4.4      | 1.1      | 0.3             | 12.6     | 3.5             | 2.24          | 0.14                 | PL  | ... | 4,5,6    | ...                                                                                                 | ... | ...   | Cygnus Cocoon field <sup>a</sup>      |     |

Table 1—Continued

| Name 3FGL     | R.A.    | Decl.   | $l$     | $b$     | $\theta_1$ | $\theta_2$ | $\phi$ | $\sigma$ | $F_{35}$ | $\Delta F_{35}$ | $S_{25}$ | $\Delta S_{25}$ | $\Gamma_{25}$ | $\Delta \Gamma_{25}$ | Mod | Var | Flags    | $\gamma$ -ray Assoc.                                        | TeV | Class | ID or Assoc.                     |
|---------------|---------|---------|---------|---------|------------|------------|--------|----------|----------|-----------------|----------|-----------------|---------------|----------------------|-----|-----|----------|-------------------------------------------------------------|-----|-------|----------------------------------|
| J2033.6+6309  | 308.421 | 63.151  | 98.160  | 13.497  | 0.062      | 0.061      | −5     | 5.1      | 0.3      | 0.1             | 3.4      | 0.9             | 1.90          | 0.20                 | PL  | ... | 3        | ...                                                         | ... | bcu   | 87GB<br>203249.5+625814          |
| J2034.3+1155  | 308.585 | 11.922  | 56.117  | −16.486 | 0.133      | 0.116      | −2     | 4.9      | 0.5      | 0.1             | 6.9      | 1.7             | 2.47          | 0.15                 | PL  | ... | 5        | ...                                                         | ... | fsrq  | TXS 2032+117                     |
| J2034.4+3833c | 308.621 | 38.564  | 78.158  | −1.043  | 0.053      | 0.052      | −85    | 8.9      | 1.3      | 0.2             | 26.1     | 3.0             | 2.39          | ...                  | LP  | ... | 3,5,6,12 | ...                                                         | ... | ...   | Cygnus Cocoon field <sup>a</sup> |
| J2034.6+4302  | 308.670 | 43.039  | 81.767  | 1.604   | 0.138      | 0.119      | −50    | 10.3     | 2.7      | 0.4             | 30.3     | 3.5             | 2.39          | ...                  | LP  | ... | 3        | ...                                                         | ... | ...   | Cygnus Cocoon field <sup>a</sup> |
| J2034.6−4202  | 308.673 | −42.040 | 359.076 | −36.383 | 0.063      | 0.057      | 12     | 7.4      | 0.4      | 0.1             | 5.1      | 1.0             | 1.95          | 0.13                 | PL  | ... | ...      | 2FGL J2034.7−4201<br>1FGL J2034.6−4202                      | ... | ...   | ...                              |
| J2035.0+3634  | 308.758 | 36.581  | 76.633  | −2.315  | 0.052      | 0.045      | 22     | 11.9     | 2.5      | 0.3             | 12.3     | 1.8             | 2.13          | ...                  | LP  | ... | 3        | 2FGL J2034.9+3632<br>1FGL J2034.7+3639                      | ... | ...   | ...                              |
| J2035.3+1055  | 308.827 | 10.924  | 55.379  | −17.231 | 0.052      | 0.048      | 20     | 19.8     | 1.8      | 0.1             | 25.0     | 1.6             | 2.47          | 0.05                 | PL  | T   | ...      | 2FGL J2035.4+1058<br>1FGL J2035.4+1100                      | ... | fsrq  | PKS 2032+107                     |
| J2035.6+3146  | 308.908 | 31.770  | 72.841  | −5.289  | 0.103      | 0.084      | 14     | 4.6      | 0.4      | 0.1             | 8.2      | 1.8             | 2.68          | 0.17                 | PL  | ... | 4        | ...                                                         | ... | ...   | ...                              |
| J2035.8+4902  | 308.958 | 49.047  | 86.712  | 5.034   | 0.056      | 0.048      | 74     | 4.8      | 0.6      | 0.2             | 6.2      | 1.7             | 2.10          | 0.16                 | PL  | ... | ...      | ...                                                         | ... | ...   | ...                              |
| J2036.4+6551  | 309.105 | 65.857  | 100.636 | 14.781  | 0.046      | 0.045      | −52    | 9.6      | 0.6      | 0.1             | 6.8      | 1.0             | 2.01          | 0.10                 | PL  | ... | ...      | 2FGL J2036.6+6551                                           | ... | bll   | 87GB<br>203539.4+654245          |
| J2036.6−3325  | 309.174 | −33.427 | 9.672   | −35.483 | 0.111      | 0.077      | −40    | 4.2      | 0.1      | 0.1             | 2.8      | 1.0             | 1.30          | 0.25                 | PL  | ... | ...      | 1FGL J2038.1+6552<br>1FHL J2036.9−3325                      | ... | bcu   | 1RXS J203650.9−332817            |
| J2036.8+4234c | 309.222 | 42.568  | 81.634  | 0.997   | 0.077      | 0.073      | 84     | 5.4      | 1.7      | 0.3             | 19.6     | 4.2             | 2.25          | 0.10                 | PL  | ... | 1,4,5,6  | ...                                                         | ... | ...   | Cygnus Cocoon field <sup>a</sup> |
| J2036.8−2830  | 309.222 | −28.505 | 15.529  | −34.396 | 0.148      | 0.115      | 1      | 7.6      | 0.4      | 0.1             | 6.8      | 1.0             | 2.58          | 0.12                 | PL  | ... | ...      | ...                                                         | ... | fsrq  | PMN J2036−2830                   |
| J2037.4+4132c | 309.354 | 41.534  | 80.869  | 0.295   | 0.090      | 0.070      | 25     | 6.4      | 1.8      | 0.3             | 20.8     | 4.2             | 2.18          | 0.11                 | PL  | ... | 6        | ...                                                         | ... | ...   | Cygnus Cocoon field <sup>a</sup> |
| J2038.4+4212  | 309.625 | 42.208  | 81.528  | 0.543   | 0.059      | 0.054      | −14    | 11.8     | 4.8      | 0.4             | 39.2     | 4.8             | 2.32          | ...                  | LP  | ... | 3        | ...                                                         | ... | ...   | Cygnus Cocoon field <sup>a</sup> |
| J2038.8+5113  | 309.703 | 51.221  | 88.747  | 5.956   | 0.127      | 0.096      | −24    | 7.9      | 0.8      | 0.1             | 20.8     | 2.4             | 2.89          | 0.10                 | PL  | T   | 5        | ...                                                         | ... | fsrq  | 3C 418                           |
| J2038.8−3613  | 309.706 | −36.218 | 6.379   | −36.419 | 0.120      | 0.115      | 73     | 7.8      | 0.5      | 0.1             | 7.2      | 1.0             | 2.45          | 0.10                 | PL  | ... | ...      | ...                                                         | ... | ...   | ...                              |
| J2039.0−1047  | 309.752 | −10.798 | 35.276  | −28.742 | 0.032      | 0.031      | 46     | 25.9     | 2.4      | 0.2             | 18.1     | 1.5             | 2.01          | ...                  | LP  | T   | ...      | 1FHL J2039.2−1045<br>2FGL J2039.1−1046<br>1FGL J2039.0−1047 | ... | bll   | TXS 2036−109                     |
| J2039.4+4111  | 309.854 | 41.198  | 80.830  | −0.208  | 0.200      | 0.100      | −59    | 10.7     | 2.9      | 0.5             | 35.3     | 4.0             | 2.41          | ...                  | LP  | ... | 3,9      | 2FGL J2040.1+4105c                                          | ... | ...   | Cygnus Cocoon field <sup>a</sup> |
| J2039.5+5217  | 309.894 | 52.298  | 89.684  | 6.511   | 0.068      | 0.057      | 26     | 5.2      | 0.4      | 0.1             | 4.6      | 1.3             | 1.89          | 0.22                 | PL  | ... | ...      | 2FGL J2039.6+5218                                           | ... | bll   | 1ES 2037+521                     |
| J2039.6−5618  | 309.918 | −56.312 | 341.231 | −37.155 | 0.043      | 0.040      | 75     | 25.4     | 2.3      | 0.2             | 17.1     | 1.4             | 2.16          | ...                  | LP  | ... | ...      | 2FGL J2039.8−5620<br>1FGL J2039.4−5621                      | ... | ...   | ...                              |
| J2039.7+1237  | 309.937 | 12.626  | 57.494  | −17.197 | 0.151      | 0.127      | −36    | 4.1      | 0.3      | 0.1             | 3.5      | 1.0             | 2.10          | 0.21                 | PL  | ... | ...      | ...                                                         | ... | ...   | ...                              |
| J2040.0−5734  | 310.007 | −57.575 | 339.651 | −37.059 | 0.112      | 0.102      | −75    | 4.6      | 0.3      | 0.1             | 3.7      | 0.9             | 2.27          | 0.19                 | PL  | ... | ...      | ...                                                         | ... | bcu   | PKS 2036−577                     |
| J2040.2−7115  | 310.072 | −71.260 | 323.150 | −34.233 | 0.050      | 0.045      | −23    | 11.1     | 0.6      | 0.1             | 7.2      | 1.1             | 1.80          | 0.11                 | PL  | ... | ...      | 1FHL J2040.0−7119<br>2FGL J2040.2−7109                      | ... | bcu   | PKS 2035−714                     |
| J2041.1+4736  | 310.281 | 47.603  | 86.091  | 3.462   | 0.050      | 0.049      | −41    | 18.4     | 3.5      | 0.3             | 31.9     | 2.3             | 2.38          | ...                  | LP  | ... | ...      | 2FGL J2041.2+4735                                           | ... | ...   | ...                              |
| J2041.7−3732  | 310.447 | −37.546 | 4.851   | −37.204 | 0.045      | 0.043      | −56    | 7.0      | 0.4      | 0.1             | 4.6      | 1.0             | 1.78          | 0.17                 | PL  | ... | ...      | ...                                                         | ... | bll   | NVSS<br>J204150−373341           |

Table 1—Continued

| Name 3FGL     | R.A.    | Decl.   | $l$     | $b$     | $\theta_1$ | $\theta_2$ | $\phi$ | $\sigma$ | $F_{35}$ | $\Delta F_{35}$ | $S_{25}$ | $\Delta S_{25}$ | $\Gamma_{25}$ | $\Delta \Gamma_{25}$ | Mod | Var | Flags    | $\gamma$ -ray Assoc.                                                             | TeV | Class | ID or Assoc.                     |
|---------------|---------|---------|---------|---------|------------|------------|--------|----------|----------|-----------------|----------|-----------------|---------------|----------------------|-----|-----|----------|----------------------------------------------------------------------------------|-----|-------|----------------------------------|
| J2041.9–7318  | 310.477 | –73.306 | 320.753 | –33.730 | 0.052      | 0.045      | 4      | 8.7      | 0.4      | 0.1             | 5.1      | 0.9             | 2.21          | 0.17                 | PL  | ... | ...      | 2FGL J2042.8–7317                                                                | ... | bcu   | SUMSS<br>J204201–731911          |
| J2042.1+2428  | 310.529 | 24.471  | 67.787  | –10.794 | 0.047      | 0.045      | –24    | 8.4      | 0.5      | 0.1             | 6.1      | 1.1             | 1.87          | 0.14                 | PL  | ... | ...      | 1FGL J2043.0–7317<br>1FHL J2042.4+2426<br>2FGL J2042.1+2428<br>1FGL J2042.2+2427 | ... | bll   | MG2 J204208+2426                 |
| J2042.1+0247  | 310.536 | 2.793   | 49.009  | –22.996 | 0.139      | 0.113      | 47     | 7.5      | 0.7      | 0.1             | 3.6      | 0.6             | 2.29          | ...                  | LP  | ... | 12       | ...                                                                              | ... | PSR   | PSR J2042+0246                   |
| J2042.3–5416  | 310.596 | –54.269 | 343.745 | –37.738 | 0.210      | 0.199      | –10    | 5.0      | 0.3      | 0.1             | 4.5      | 0.9             | 2.55          | 0.17                 | PL  | ... | ...      | ...                                                                              | ... | ...   | ...                              |
| J2042.4+4209  | 310.614 | 42.153  | 81.932  | –0.071  | 0.163      | 0.088      | 0      | 10.7     | 3.5      | 0.4             | 30.5     | 3.7             | 2.35          | ...                  | LP  | ... | 3,9      | ...                                                                              | ... | ...   | Cygnus Cocoon field <sup>a</sup> |
| J2043.1+4350  | 310.777 | 43.835  | 83.329  | 0.873   | 0.124      | 0.097      | 70     | 8.4      | 0.8      | 0.2             | 21.2     | 2.5             | 2.46          | ...                  | LP  | ... | 1,4,5,12 | ...                                                                              | ... | ...   | ...                              |
| J2043.2+1711  | 310.816 | 17.184  | 61.901  | –15.301 | 0.031      | 0.029      | –52    | 39.0     | 4.4      | 0.2             | 30.2     | 1.4             | 2.07          | ...                  | EC  | ... | ...      | 2FGL J2043.2+1711<br>1FGL J2043.2+1709                                           | ... | PSR   | PSR J2043+1711                   |
| J2043.6+0001  | 310.901 | 0.029   | 46.611  | –24.719 | 0.103      | 0.083      | 89     | 4.3      | 0.2      | 0.1             | 2.9      | 0.9             | 1.69          | 0.20                 | PL  | ... | ...      | ...                                                                              | ... | ...   | ...                              |
| J2043.8+2741  | 310.950 | 27.699  | 70.636  | –9.154  | 0.073      | 0.066      | 6      | 13.8     | 1.5      | 0.2             | 11.8     | 1.2             | 2.40          | ...                  | EC  | ... | ...      | 2FGL J2043.7+2743<br>1FGL J2043.7+2740                                           | ... | PSR   | PSR J2043+2740                   |
| J2043.8–4801  | 310.950 | –48.021 | 351.654 | –38.263 | 0.078      | 0.075      | –23    | 9.6      | 0.6      | 0.1             | 7.3      | 0.9             | 2.24          | 0.10                 | PL  | ... | 3,10     | 2FGL J2044.4–4757                                                                | ... | ...   | ...                              |
| J2044.0+1035  | 311.000 | 10.590  | 56.325  | –19.196 | 0.121      | 0.119      | 36     | 5.1      | 0.4      | 0.1             | 5.0      | 1.0             | 2.29          | 0.14                 | PL  | ... | ...      | ...                                                                              | ... | ...   | ...                              |
| J2045.2+5026e | 311.320 | 50.440  | 88.753  | 4.670   | ...        | ...        | ...    | 31.5     | 10.7     | 0.5             | 89.8     | 3.9             | 2.29          | ...                  | LP  | ... | ...      | 1FGL J2046.0+4954<br>2FGL J2046.0+4954<br>...                                    | ... | SNR   | HB21                             |
| J2045.6–6838  | 311.407 | –68.635 | 326.055 | –35.422 | 0.132      | 0.100      | 19     | 5.6      | 0.4      | 0.1             | 4.8      | 0.9             | 2.39          | 0.13                 | PL  | ... | 1        | ...                                                                              | ... | ...   | ...                              |
| J2046.7–1011  | 311.684 | –10.187 | 36.844  | –30.197 | 0.093      | 0.082      | 90     | 4.8      | 0.2      | 0.1             | 3.4      | 1.1             | 1.61          | 0.19                 | PL  | ... | ...      | ...                                                                              | ... | bcu   | PMN J2046–1010                   |
| J2046.7–4259  | 311.698 | –42.984 | 358.101 | –38.677 | 0.164      | 0.129      | 21     | 4.4      | 0.3      | 0.1             | 3.3      | 0.8             | 2.01          | 0.16                 | PL  | ... | ...      | 2FGL J2046.2–4259                                                                | ... | ...   | ...                              |
| J2047.1+1054  | 311.778 | 10.914  | 57.064  | –19.649 | 0.122      | 0.099      | 4      | 7.8      | 0.7      | 0.1             | 3.6      | 0.6             | 2.14          | ...                  | EC  | ... | 12       | 2FGL J2046.7+1055<br>1FGL J2047.6+1055                                           | ... | PSR   | PSR J2047+1053                   |
| J2047.9–3119  | 311.984 | –31.324 | 12.831  | –37.379 | 0.116      | 0.079      | 3      | 7.1      | 0.4      | 0.1             | 6.4      | 1.0             | 2.52          | 0.15                 | PL  | ... | ...      | ...                                                                              | ... | ...   | ...                              |
| J2048.8+4436  | 312.224 | 44.608  | 84.581  | 0.545   | 0.179      | 0.124      | 55     | 11.9     | 2.1      | 0.3             | 23.2     | 2.1             | 2.52          | ...                  | LP  | ... | 12       | ...                                                                              | ... | ...   | ...                              |
| J2049.0–6801  | 312.256 | –68.029 | 326.659 | –35.896 | 0.093      | 0.077      | –46    | 6.5      | 0.4      | 0.1             | 4.4      | 0.9             | 2.06          | 0.14                 | PL  | ... | ...      | ...                                                                              | ... | bcu   | PKS 2043–682                     |
| J2049.7+1002  | 312.440 | 10.045  | 56.687  | –20.676 | 0.090      | 0.070      | –42    | 11.1     | 0.8      | 0.1             | 10.9     | 1.2             | 2.40          | 0.08                 | PL  | T   | ...      | 2FGL J2049.8+1001<br>1FGL J2049.7+1003                                           | ... | bcu   | PKS 2047+098                     |
| J2050.2+0409  | 312.568 | 4.153   | 51.432  | –24.010 | 0.115      | 0.078      | –23    | 7.7      | 0.6      | 0.1             | 6.5      | 1.1             | 2.07          | 0.11                 | PL  | ... | ...      | 2FGL J2050.0+0408<br>1FGL J2050.1+0407                                           | ... | bll   | PKS 2047+039                     |
| J2051.0+3040e | 312.750 | 30.670  | 73.985  | –8.563  | ...        | ...        | ...    | 37.9     | 10.2     | 0.4             | 82.5     | 3.0             | 2.17          | ...                  | LP  | ... | ...      | 1FGL J2046.4+3041<br>2FGL J2051.0+3040e                                          | ... | SNR   | Cygnus Loop                      |
| J2051.3–0828  | 312.828 | –8.480  | 39.197  | –30.461 | 0.110      | 0.086      | –66    | 7.4      | 0.7      | 0.1             | 3.2      | 0.5             | 2.02          | ...                  | EC  | ... | 12       | ...                                                                              | ... | PSR   | PSR J2051–0827                   |
| J2051.8–5535  | 312.969 | –55.595 | 341.865 | –38.939 | 0.093      | 0.079      | –35    | 7.1      | 0.4      | 0.1             | 6.0      | 1.0             | 2.58          | 0.15                 | PL  | T   | ...      | ...                                                                              | ... | bcu   | PMN J2052–5533                   |

Table 1—Continued

| Name 3FGL    | R.A.    | Decl.   | $l$     | $b$     | $\theta_1$ | $\theta_2$ | $\phi$ | $\sigma$ | $F_{35}$ | $\Delta F_{35}$ | $S_{25}$ | $\Delta S_{25}$ | $\Gamma_{25}$ | $\Delta \Gamma_{25}$ | Mod | Var | Flags | $\gamma$ -ray Assoc.                                                                               | TeV | Class | ID or Assoc.                   |
|--------------|---------|---------|---------|---------|------------|------------|--------|----------|----------|-----------------|----------|-----------------|---------------|----------------------|-----|-----|-------|----------------------------------------------------------------------------------------------------|-----|-------|--------------------------------|
| J2052.7+1217 | 313.196 | 12.298  | 59.113  | -20.004 | 0.108      | 0.094      | -76    | 7.2      | 0.6      | 0.1             | 6.5      | 1.0             | 2.25          | 0.11                 | PL  | ... | ...   | 2FGL J2053.2+1212c                                                                                 | ... | psr   | PSR J2052+12                   |
| J2053.1+6027 | 313.288 | 60.458  | 97.353  | 10.047  | 0.164      | 0.123      | -88    | 7.8      | 0.6      | 0.1             | 10.3     | 1.4             | 2.67          | 0.10                 | PL  | ... | 1,4   | ...                                                                                                | ... | ...   | ...                            |
| J2053.4-4052 | 313.357 | -40.871 | 0.917   | -39.786 | 0.194      | 0.142      | -15    | 4.3      | 0.3      | 0.1             | 3.6      | 0.8             | 2.29          | 0.17                 | PL  | ... | ...   | ...                                                                                                | ... | ...   | ...                            |
| J2053.9+2922 | 313.476 | 29.374  | 73.361  | -9.865  | 0.045      | 0.041      | 49     | 7.7      | 0.4      | 0.1             | 6.0      | 1.3             | 1.54          | 0.13                 | PL  | ... | 1     | ...                                                                                                | ... | ...   | Cygnus Loop field <sup>a</sup> |
| J2054.3+6907 | 313.587 | 69.131  | 104.421 | 15.312  | 0.133      | 0.101      | 75     | 5.4      | 0.4      | 0.1             | 5.5      | 1.0             | 2.46          | 0.12                 | PL  | ... | 3     | ...                                                                                                | ... | ...   | ...                            |
| J2054.8-4908 | 313.725 | -49.136 | 350.135 | -40.059 | 0.216      | 0.123      | 80     | 4.7      | 0.3      | 0.1             | 4.0      | 0.9             | 2.35          | 0.19                 | PL  | ... | ...   | ...                                                                                                | ... | ...   | ...                            |
| J2055.0+0016 | 313.751 | 0.268   | 48.450  | -27.053 | 0.056      | 0.055      | -38    | 4.9      | 0.2      | 0.1             | 3.2      | 1.0             | 1.73          | 0.20                 | PL  | ... | ...   | ...                                                                                                | ... | bll   | RGB J2054+002                  |
| J2055.2-0019 | 313.807 | -0.332  | 47.903  | -27.408 | 0.077      | 0.058      | -51    | 6.9      | 0.4      | 0.1             | 5.5      | 1.3             | 1.62          | 0.14                 | PL  | ... | ...   | 2FGL J2055.4-0023                                                                                  | ... | bll   | 1RXS<br>J205528.2-002123       |
| J2055.6+1609 | 313.901 | 16.156  | 62.846  | -18.296 | 0.131      | 0.111      | -77    | 4.5      | 0.3      | 0.1             | 4.3      | 1.0             | 2.50          | 0.16                 | PL  | ... | ...   | ...                                                                                                | ... | ...   | ...                            |
| J2055.8+2539 | 313.963 | 25.667  | 70.694  | -12.527 | 0.023      | 0.023      | 74     | 63.7     | 9.0      | 0.3             | 54.8     | 1.5             | 2.12          | ...                  | EC  | ... | ...   | 2FGL J2055.8+2539<br>1FGL J2055.8+2539<br>0FGL J2055.5+2540                                        | ... | PSR   | LAT PSR J2055+2539             |
| J2056.2-4714 | 314.067 | -47.248 | 352.589 | -40.381 | 0.021      | 0.021      | -89    | 78.9     | 6.3      | 0.2             | 77.4     | 1.8             | 2.40          | ...                  | LP  | T   | ...   | 1FHL J2056.3-4712<br>2FGL J2056.2-4715<br>1FGL J2056.3-4714<br>0FGL J2056.1-4715<br>3EG J2055-4716 | ... | fsrq  | PKS 2052-47<br>-128-           |
| J2056.3-5925 | 314.097 | -59.422 | 336.888 | -38.856 | 0.135      | 0.117      | 44     | 5.8      | 0.4      | 0.1             | 4.3      | 0.8             | 2.30          | 0.12                 | PL  | ... | ...   | ...                                                                                                | ... | ...   | ...                            |
| J2056.7+4938 | 314.179 | 49.641  | 89.301  | 2.744   | 0.029      | 0.025      | 31     | 12.5     | 1.3      | 0.2             | 16.3     | 2.1             | 1.78          | 0.08                 | PL  | ... | ...   | 2FGL J2056.7+4939<br>1FGL J2056.7+4938                                                             | ... | bcu   | RGB J2056+496                  |
| J2058.0+4347 | 314.503 | 43.795  | 85.006  | -1.230  | 0.199      | 0.161      | -76    | 14.1     | 1.2      | 0.2             | 32.8     | 2.3             | 2.92          | 0.07                 | PL  | ... | 1     | ...                                                                                                | ... | ...   | ...                            |
| J2058.3+3729 | 314.581 | 37.489  | 80.251  | -5.381  | 0.130      | 0.095      | 72     | 7.3      | 0.4      | 0.1             | 11.5     | 1.5             | 2.95          | 0.16                 | PL  | ... | 1,4   | ...                                                                                                | ... | ...   | ...                            |
| J2059.9+2029 | 314.995 | 20.488  | 67.114  | -16.491 | 0.165      | 0.164      | -89    | 4.7      | 0.3      | 0.1             | 5.3      | 1.1             | 2.58          | 0.15                 | PL  | ... | ...   | ...                                                                                                | ... | ...   | ...                            |
| J2100.6-7844 | 315.158 | -78.746 | 314.235 | -32.685 | 0.193      | 0.153      | -68    | 4.6      | 0.2      | 0.1             | 4.8      | 1.0             | 2.73          | 0.18                 | PL  | ... | ...   | ...                                                                                                | ... | ...   | ...                            |
| J2102.3+4547 | 315.589 | 45.785  | 87.012  | -0.501  | 0.135      | 0.116      | 18     | 7.7      | 1.3      | 0.2             | 10.2     | 1.7             | 2.51          | ...                  | LP  | T   | 3     | 2FGL J2102.2+4546                                                                                  | ... | NOV   | V407 Cyg                       |
| J2102.8+4704 | 315.724 | 47.069  | 88.035  | 0.282   | 0.095      | 0.072      | -83    | 5.7      | 0.9      | 0.2             | 9.6      | 1.9             | 2.07          | 0.12                 | PL  | ... | ...   | 2FGL J2103.4+4706                                                                                  | ... | ...   | ...                            |
| J2103.7-1113 | 315.942 | -11.229 | 37.858  | -34.423 | 0.066      | 0.056      | -10    | 12.3     | 1.1      | 0.1             | 6.2      | 0.9             | 2.06          | ...                  | LP  | ... | ...   | 2FGL J2103.5-1112                                                                                  | ... | ...   | ...                            |
| J2103.9-6233 | 315.986 | -62.561 | 332.688 | -38.962 | 0.038      | 0.036      | -2     | 21.1     | 1.4      | 0.1             | 15.2     | 1.3             | 1.98          | 0.05                 | PL  | T   | ...   | 2FGL J2103.6-6236<br>1FGL J2103.9-6237                                                             | ... | bcu   | PMN J2103-6232                 |
| J2103.9-3546 | 315.999 | -35.775 | 7.845   | -41.400 | 0.080      | 0.073      | 84     | 10.4     | 0.7      | 0.1             | 8.8      | 1.0             | 2.36          | 0.09                 | PL  | T   | ...   | ...                                                                                                | ... | bcu   | NVSS<br>J210353-354620         |
| J2104.2-0211 | 316.052 | -2.191  | 47.378  | -30.285 | 0.124      | 0.074      | 64     | 4.1      | 0.2      | 0.1             | 2.6      | 0.9             | 1.52          | 0.21                 | PL  | ... | ...   | ...                                                                                                | ... | bcu   | NVSS<br>J210421-021239         |
| J2104.7+2113 | 316.193 | 21.228  | 68.447  | -16.904 | 0.078      | 0.068      | -30    | 5.0      | 0.3      | 0.1             | 3.6      | 1.0             | 2.05          | 0.19                 | PL  | ... | ...   | 1FGL J2104.6+2119                                                                                  | ... | ...   | ...                            |
| J2106.1+2505 | 316.530 | 25.098  | 71.755  | -14.681 | 0.171      | 0.133      | -74    | 4.3      | 0.3      | 0.1             | 4.8      | 1.1             | 2.53          | 0.15                 | PL  | ... | ...   | ...                                                                                                | ... | bcu   | MG3 J210642+2501               |
| J2107.1+2248 | 316.795 | 22.804  | 70.088  | -16.337 | 0.228      | 0.159      | 63     | 4.6      | 0.4      | 0.1             | 5.2      | 1.1             | 2.48          | 0.15                 | PL  | ... | ...   | ...                                                                                                | ... | ...   | ...                            |
| J2107.7-4822 | 316.931 | -48.370 | 350.930 | -42.226 | 0.212      | 0.176      | 35     | 4.9      | 0.2      | 0.1             | 4.9      | 1.0             | 2.71          | 0.19                 | PL  | ... | ...   | ...                                                                                                | ... | bcu   | PMN J2107-4827                 |



Table 1—Continued

| Name 3FGL    | R.A.    | Decl.   | $l$     | $b$     | $\theta_1$ | $\theta_2$ | $\phi$ | $\sigma$ | $F_{35}$ | $\Delta F_{35}$ | $S_{25}$ | $\Delta S_{25}$ | $\Gamma_{25}$ | $\Delta \Gamma_{25}$ | Mod | Var | Flags  | $\gamma$ -ray Assoc.                                        | TeV | Class | ID or Assoc.             |
|--------------|---------|---------|---------|---------|------------|------------|--------|----------|----------|-----------------|----------|-----------------|---------------|----------------------|-----|-----|--------|-------------------------------------------------------------|-----|-------|--------------------------|
| J2108.0+3654 | 317.005 | 36.914  | 81.097  | -7.211  | 0.060      | 0.058      | 2      | 6.4      | 0.5      | 0.1             | 5.2      | 1.1             | 1.93          | 0.16                 | PL  | ... | ...    | 2FGL J2107.8+3652                                           | ... | bcu   | TXS 2106+367             |
| J2108.1+5202 | 317.045 | 52.042  | 92.302  | 2.978   | 0.084      | 0.061      | 40     | 9.7      | 1.7      | 0.2             | 24.5     | 2.5             | 2.50          | 0.07                 | PL  | ... | 3      | 2FGL J2107.9+5207c<br>1FGL J2107.5+5202c                    | ... | ...   | ...                      |
| J2108.6-8619 | 317.163 | -86.318 | 306.415 | -29.160 | 0.087      | 0.065      | -31    | 4.7      | 0.2      | 0.1             | 2.6      | 0.8             | 1.74          | 0.27                 | PL  | ... | 3      | ...                                                         | ... | bcu   | 1RXS<br>J210959.5-861853 |
| J2108.6-0250 | 317.173 | -2.842  | 47.384  | -31.580 | 0.065      | 0.063      | -5     | 5.1      | 0.2      | 0.1             | 2.8      | 0.8             | 1.94          | 0.18                 | PL  | ... | ...    | 2FGL J2108.7-0246<br>1FGL J2108.5-0249                      | ... | bll   | TXS 2106-030             |
| J2109.1-6638 | 317.277 | -66.638 | 327.522 | -38.176 | 0.061      | 0.049      | 14     | 13.1     | 0.7      | 0.1             | 8.1      | 1.0             | 2.01          | 0.08                 | PL  | ... | ...    | 1FHL J2109.2-6635<br>2FGL J2108.9-6636<br>1FGL J2108.6-6646 | ... | bcu   | PKS 2104-668             |
| J2109.4+1437 | 317.359 | 14.620  | 63.689  | -21.881 | 0.112      | 0.095      | 81     | 10.2     | 0.5      | 0.1             | 10.2     | 1.1             | 2.73          | 0.10                 | PL  | T   | ...    | ...                                                         | ... | ...   | ...                      |
| J2110.0+0442 | 317.513 | 4.705   | 54.942  | -27.837 | 0.135      | 0.094      | 69     | 5.1      | 0.4      | 0.1             | 4.0      | 0.9             | 2.06          | 0.16                 | PL  | ... | ...    | ...                                                         | ... | ...   | ...                      |
| J2110.0+0812 | 317.518 | 8.202   | 58.162  | -25.842 | 0.086      | 0.079      | -86    | 10.7     | 1.0      | 0.1             | 11.8     | 1.3             | 2.33          | 0.07                 | PL  | T   | ...    | 2FGL J2109.9+0807<br>1FGL J2110.0+0811                      | ... | fsrq  | PMN J2110+0810           |
| J2110.3-1013 | 317.576 | -10.223 | 39.813  | -35.433 | 0.374      | 0.263      | -75    | 7.1      | 0.4      | 0.1             | 7.6      | 1.0             | 2.71          | 0.12                 | PL  | ... | ...    | ...                                                         | ... | fsrq  | PKS 2107-105             |
| J2110.3+3540 | 317.585 | 35.668  | 80.483  | -8.394  | 0.289      | 0.209      | 84     | 5.5      | 0.4      | 0.1             | 7.0      | 1.2             | 2.64          | 0.14                 | PL  | ... | 1      | ...                                                         | ... | bcu   | B2 2107+35A              |
| J2110.4+5946 | 317.619 | 59.779  | 98.253  | 7.968   | 0.079      | 0.071      | 9      | 7.4      | 0.6      | 0.1             | 9.9      | 1.5             | 2.53          | 0.11                 | PL  | ... | 3      | ...                                                         | ... | ...   | ...                      |
| J2111.4+4605 | 317.866 | 46.090  | 88.304  | -1.466  | 0.024      | 0.023      | -12    | 35.1     | 6.2      | 0.3             | 43.8     | 2.2             | 2.15          | ...                  | EC  | ... | ...    | 2FGL J2111.3+4605<br>1FGL J2111.3+4607<br>0FGL J2110.8+4608 | ... | PSR   | PSR J2111+4606           |
| J2112.5-3044 | 318.145 | -30.734 | 14.898  | -42.449 | 0.036      | 0.033      | 45     | 30.1     | 3.3      | 0.2             | 19.0     | 1.4             | 2.02          | ...                  | LP  | ... | ...    | 2FGL J2112.5-3042<br>1FGL J2112.5-3044                      | ... | ...   | ...                      |
| J2112.7+0819 | 318.190 | 8.325   | 58.707  | -26.310 | 0.040      | 0.038      | 65     | 11.3     | 0.7      | 0.1             | 8.1      | 1.3             | 1.81          | 0.12                 | PL  | ... | ...    | 2FGL J2112.5+0818                                           | ... | bcu   | 1RXS<br>J211242.5+081831 |
| J2114.0+5239 | 318.524 | 52.652  | 93.366  | 2.734   | 0.069      | 0.060      | -26    | 7.0      | 1.6      | 0.3             | 11.7     | 1.7             | 2.37          | ...                  | LP  | ... | 4,5,12 | ...                                                         | ... | ...   | ...                      |
| J2114.7+3130 | 318.693 | 31.507  | 77.994  | -11.884 | 0.111      | 0.094      | 50     | 5.1      | 0.4      | 0.1             | 5.1      | 1.1             | 2.35          | 0.16                 | PL  | ... | ...    | ...                                                         | ... | bcu   | B2 2112+31               |
| J2114.9+5448 | 318.725 | 54.816  | 95.016  | 4.142   | 0.076      | 0.055      | 40     | 9.2      | 1.4      | 0.2             | 6.5      | 0.9             | 2.20          | ...                  | LP  | ... | 12     | 2FGL J2114.1+5440                                           | ... | psr   | PSR J2114+54             |
| J2115.2+1215 | 318.822 | 12.260  | 62.606  | -24.451 | 0.163      | 0.082      | -12    | 6.2      | 0.4      | 0.1             | 4.8      | 1.0             | 2.16          | 0.17                 | PL  | ... | ...    | 2FGL J2115.4+1213                                           | ... | ...   | ...                      |
| J2115.4+2933 | 318.851 | 29.555  | 76.611  | -13.300 | 0.046      | 0.040      | -83    | 16.4     | 1.2      | 0.1             | 16.0     | 1.2             | 2.37          | 0.06                 | PL  | ... | ...    | 1FHL J2115.6+2935<br>2FGL J2115.3+2932<br>1FGL J2115.5+2937 | ... | fsrq  | B2 2113+29               |
| J2116.1+3339 | 319.047 | 33.650  | 79.805  | -10.647 | 0.021      | 0.019      | -90    | 36.0     | 3.4      | 0.2             | 39.5     | 2.2             | 1.91          | 0.03                 | PL  | T   | ...    | 1FHL J2116.2+3339<br>2FGL J2116.2+3339<br>1FGL J2116.1+3338 | ... | bll   | B2 2114+33               |
| J2116.2+4422 | 319.064 | 44.381  | 87.647  | -3.255  | 0.206      | 0.169      | 16     | 4.2      | 0.3      | 0.1             | 8.1      | 1.8             | 2.89          | 0.27                 | PL  | ... | 4,5    | ...                                                         | ... | ...   | ...                      |
| J2116.9+1343 | 319.234 | 13.728  | 64.144  | -23.862 | 0.122      | 0.109      | 6      | 5.0      | 0.3      | 0.1             | 4.2      | 1.0             | 2.36          | 0.18                 | PL  | ... | ...    | ...                                                         | ... | ...   | ...                      |
| J2117.6+3725 | 319.421 | 37.426  | 82.798  | -8.274  | 0.113      | 0.086      | 70     | 14.5     | 1.4      | 0.1             | 12.8     | 1.3             | 2.39          | ...                  | LP  | ... | ...    | 2FGL J2117.5+3730                                           | ... | ...   | ...                      |

Table 1—Continued

| Name 3FGL    | R.A.    | Decl.   | $l$     | $b$     | $\theta_1$ | $\theta_2$ | $\phi$ | $\sigma$ | $F_{35}$ | $\Delta F_{35}$ | $S_{25}$ | $\Delta S_{25}$ | $\Gamma_{25}$ | $\Delta \Gamma_{25}$ | Mod | Var | Flags  | $\gamma$ -ray Assoc.                                        | TeV | Class | ID or Assoc.           |
|--------------|---------|---------|---------|---------|------------|------------|--------|----------|----------|-----------------|----------|-----------------|---------------|----------------------|-----|-----|--------|-------------------------------------------------------------|-----|-------|------------------------|
| J2118.0–3241 | 319.511 | –32.692 | 12.493  | –43.900 | 0.078      | 0.071      | –59    | 4.1      | 0.3      | 0.1             | 3.9      | 2.1             | 2.31          | 0.41                 | PL  | ... | ...    | 1FGL J2116.8+3729<br>1FGL J2118.3–3237                      | ... | bcu   | NVSS<br>J211754–324326 |
| J2118.3+5751 | 319.588 | 57.863  | 97.552  | 5.911   | 0.128      | 0.091      | –69    | 5.8      | 0.6      | 0.1             | 9.0      | 1.7             | 2.48          | 0.12                 | PL  | ... | ...    | ...                                                         | ... | ...   | ...                    |
| J2118.4+0013 | 319.602 | 0.232   | 51.961  | –32.043 | 0.119      | 0.114      | –89    | 4.4      | 0.3      | 0.1             | 3.0      | 0.8             | 1.94          | 0.19                 | PL  | ... | ...    | 1FGL J2117.8+0016                                           | ... | fsrq  | PMN J2118+0013         |
| J2119.2–3313 | 319.820 | –33.225 | 11.804  | –44.226 | 0.137      | 0.132      | 13     | 4.4      | 0.4      | 0.1             | 5.5      | 2.0             | 2.35          | 0.29                 | PL  | ... | ...    | ...                                                         | ... | bcu   | PMN J2118–3316         |
| J2120.4–1256 | 320.123 | –12.946 | 38.066  | –38.854 | 0.199      | 0.146      | 87     | 6.7      | 0.4      | 0.1             | 6.1      | 0.9             | 2.57          | 0.12                 | PL  | ... | ...    | 2FGL J2120.6–1301<br>1FGL J2120.2–1259                      | ... | ...   | ...                    |
| J2121.0+1901 | 320.269 | 19.024  | 69.250  | –21.255 | 0.032      | 0.031      | –76    | 27.4     | 2.2      | 0.1             | 25.0     | 1.4             | 2.16          | 0.04                 | PL  | ... | ...    | 1FHL J2121.0+1901<br>2FGL J2121.0+1901<br>1FGL J2120.9+1901 | ... | fsrq  | OX 131                 |
| J2121.5–8253 | 320.381 | –82.893 | 309.527 | –31.302 | 0.181      | 0.160      | –87    | 4.6      | 0.3      | 0.1             | 5.4      | 1.2             | 2.58          | 0.17                 | PL  | ... | ...    | ...                                                         | ... | ...   | ...                    |
| J2123.6+0533 | 320.921 | 5.563   | 57.972  | –30.126 | 0.120      | 0.096      | –56    | 6.8      | 0.5      | 0.1             | 5.5      | 0.9             | 2.17          | 0.12                 | PL  | ... | ...    | ...                                                         | ... | fsrq  | OX 036                 |
| J2124.7–3358 | 321.194 | –33.973 | 10.936  | –45.446 | 0.023      | 0.022      | –20    | 56.6     | 7.5      | 0.3             | 39.4     | 1.4             | 1.97          | ...                  | EC  | ... | ...    | 2FGL J2124.6–3357<br>1FGL J2124.7–3358<br>0FGL J2124.7–3358 | ... | PSR   | PSR J2124–3358<br>130  |
| J2125.8+5832 | 321.461 | 58.549  | 98.741  | 5.697   | 0.145      | 0.083      | –55    | 7.5      | 0.9      | 0.2             | 7.9      | 1.1             | 2.46          | ...                  | LP  | ... | 1,4,12 | ...                                                         | ... | ...   | ...                    |
| J2126.5–4605 | 321.628 | –46.087 | 353.600 | –45.644 | 0.043      | 0.042      | –13    | 34.0     | 1.9      | 0.1             | 28.7     | 1.1             | 2.50          | 0.04                 | PL  | T   | ...    | 1FGL J2126.1–4603                                           | ... | FSRQ  | PKS 2123–463           |
| J2126.5–3926 | 321.629 | –39.446 | 3.122   | –46.061 | 0.202      | 0.140      | –58    | 4.1      | 0.3      | 0.1             | 3.1      | 0.8             | 2.20          | 0.19                 | PL  | ... | ...    | ...                                                         | ... | bcu   | PMN J2126–3921         |
| J2127.1–5615 | 321.784 | –56.255 | 339.580 | –43.613 | 0.260      | 0.212      | 46     | 4.4      | 0.3      | 0.1             | 3.7      | 0.9             | 2.50          | 0.19                 | PL  | ... | ...    | ...                                                         | ... | ...   | ...                    |
| J2127.5–6001 | 321.893 | –60.031 | 334.661 | –42.454 | 0.094      | 0.074      | –25    | 4.6      | 0.2      | 0.1             | 2.3      | 0.7             | 1.95          | 0.20                 | PL  | ... | ...    | ...                                                         | ... | ...   | ...                    |
| J2127.7+3612 | 321.948 | 36.202  | 83.353  | –10.574 | 0.040      | 0.036      | 75     | 14.3     | 1.1      | 0.1             | 12.8     | 1.4             | 1.90          | 0.07                 | PL  | ... | ...    | 1FHL J2127.8+3614<br>2FGL J2127.8+3614                      | ... | bll   | B2 2125+35             |
| J2129.6–0427 | 322.410 | –4.465  | 48.916  | –36.905 | 0.082      | 0.076      | –83    | 13.0     | 0.9      | 0.1             | 10.5     | 1.1             | 2.22          | 0.07                 | PL  | ... | ...    | 2FGL J2129.8–0428<br>1FGL J2129.8–0427                      | ... | PSR   | PSR J2129–0429         |
| J2130.4–4237 | 322.615 | –42.632 | 358.467 | –46.683 | 0.241      | 0.121      | 45     | 8.8      | 0.5      | 0.1             | 8.0      | 1.0             | 2.56          | 0.10                 | PL  | T   | 9      | ...                                                         | ... | ...   | ...                    |
| J2130.8–2745 | 322.723 | –27.766 | 19.997  | –45.823 | 0.069      | 0.054      | –14    | 8.8      | 0.4      | 0.1             | 5.8      | 1.1             | 1.70          | 0.11                 | PL  | ... | ...    | ...                                                         | ... | bll   | RBS 1751               |
| J2131.1–6625 | 322.791 | –66.417 | 326.642 | –40.274 | 0.107      | 0.093      | –13    | 10.1     | 0.5      | 0.1             | 7.3      | 0.8             | 2.45          | 0.09                 | PL  | ... | ...    | ...                                                         | ... | ...   | ...                    |
| J2131.5–0915 | 322.891 | –9.253  | 43.894  | –39.667 | 0.035      | 0.033      | –19    | 13.7     | 0.9      | 0.1             | 9.6      | 1.1             | 2.02          | 0.09                 | PL  | ... | ...    | 1FHL J2131.6–0913<br>2FGL J2131.6–0914<br>1FGL J2131.7–0914 | ... | bll   | RBS 1752               |
| J2131.5+2605 | 322.896 | 26.097  | 76.539  | –18.273 | 0.481      | 0.131      | –47    | 4.1      | 0.4      | 0.1             | 4.3      | 1.1             | 2.27          | 0.17                 | PL  | ... | 9      | 2FGL J2132.5+2605                                           | ... | ...   | ...                    |
| J2131.8–2516 | 322.954 | –25.271 | 23.545  | –45.480 | 0.050      | 0.049      | 71     | 7.0      | 0.4      | 0.1             | 3.9      | 0.8             | 2.01          | 0.15                 | PL  | ... | ...    | ...                                                         | ... | bll   | RBS 1755               |
| J2132.4–5420 | 323.108 | –54.347 | 341.826 | –44.885 | 0.113      | 0.092      | –84    | 13.6     | 0.6      | 0.1             | 10.5     | 0.9             | 2.63          | 0.08                 | PL  | T   | ...    | 2FGL J2131.0–5417                                           | ... | bcu   | PMN J2132–5420         |
| J2133.0–6433 | 323.259 | –64.553 | 328.739 | –41.268 | 0.095      | 0.082      | –50    | 10.1     | 0.8      | 0.1             | 4.0      | 0.7             | 2.20          | ...                  | LP  | ... | ...    | 2FGL J2133.5–6431<br>1FGL J2134.3–6429                      | ... | ...   | ...                    |

Table 1—Continued

| Name 3FGL    | R.A.    | Decl.   | $l$     | $b$     | $\theta_1$ | $\theta_2$ | $\phi$ | $\sigma$ | $F_{35}$ | $\Delta F_{35}$ | $S_{25}$ | $\Delta S_{25}$ | $\Gamma_{25}$ | $\Delta \Gamma_{25}$ | Mod | Var | Flags | $\gamma$ -ray Assoc. | TeV | Class | ID or Assoc.            |
|--------------|---------|---------|---------|---------|------------|------------|--------|----------|----------|-----------------|----------|-----------------|---------------|----------------------|-----|-----|-------|----------------------|-----|-------|-------------------------|
| J2133.3+2533 | 323.348 | 25.556  | 76.429  | -18.942 | 0.103      | 0.080      | -4     | 5.0      | 0.3      | 0.1             | 3.8      | 1.0             | 2.01          | 0.19                 | PL  | ... | ...   | 1FGL J2133.4+2532    | ... | bcu   | 87GB<br>213100.1+251534 |
| J2133.6+2821 | 323.404 | 28.358  | 78.561  | -17.009 | 0.212      | 0.194      | -45    | 4.1      | 0.3      | 0.1             | 4.3      | 1.0             | 2.62          | 0.17                 | PL  | ... | ...   | ...                  | ... | ...   | ...                     |
| J2133.8+6648 | 323.467 | 66.800  | 105.194 | 11.006  | 0.036      | 0.031      | 68     | 14.4     | 1.3      | 0.1             | 14.4     | 1.4             | 2.08          | 0.07                 | PL  | T   | 3     | 2FGL J2133.9+6645    | ... | bcu   | NVSS<br>J213349+664706  |
| J2134.1-0152 | 323.532 | -1.870  | 52.402  | -36.485 | 0.043      | 0.042      | -19    | 16.5     | 1.1      | 0.1             | 12.8     | 1.1             | 2.21          | 0.06                 | PL  | T   | ...   | 2FGL J2133.8-0154    | ... | bll   | PKS 2131-021            |
|              |         |         |         |         |            |            |        |          |          |                 |          |                 |               |                      |     |     |       | 1FGL J2134.0-0203    |     |       |                         |
| J2134.5-2131 | 323.646 | -21.522 | 28.921  | -45.083 | 0.055      | 0.046      | 16     | 11.4     | 0.7      | 0.1             | 7.9      | 1.0             | 2.13          | 0.09                 | PL  | ... | ...   | 1FHL J2134.6-2130    | ... | ...   | ...                     |
|              |         |         |         |         |            |            |        |          |          |                 |          |                 |               |                      |     |     |       | 2FGL J2134.6-2130    |     |       |                         |
|              |         |         |         |         |            |            |        |          |          |                 |          |                 |               |                      |     |     |       | 1FGL J2134.5-2130    |     |       |                         |
| J2135.3-5008 | 323.828 | -50.144 | 347.479 | -46.385 | 0.080      | 0.069      | 75     | 12.0     | 0.8      | 0.1             | 12.0     | 1.2             | 2.47          | 0.07                 | PL  | T   | ...   | 2FGL J2135.6-4959    | ... | fsrq  | PMN J2135-5006          |
|              |         |         |         |         |            |            |        |          |          |                 |          |                 |               |                      |     |     |       | 1FGL J2135.8-4957    |     |       |                         |
| J2135.6+5742 | 323.901 | 57.713  | 99.106  | 4.206   | 0.147      | 0.112      | 59     | 5.4      | 0.6      | 0.1             | 9.7      | 1.8             | 2.59          | 0.13                 | PL  | ... | 3,4   | ...                  | ... | ...   | ...                     |
| J2138.2-4939 | 324.554 | -49.656 | 348.017 | -46.952 | 0.205      | 0.173      | 27     | 4.2      | 0.3      | 0.1             | 4.3      | 1.1             | 2.42          | 0.16                 | PL  | ... | 5     | ...                  | ... | ...   | ...                     |
| J2139.4-4235 | 324.852 | -42.598 | 358.303 | -48.327 | 0.024      | 0.023      | -87    | 45.8     | 4.3      | 0.2             | 37.5     | 1.9             | 2.09          | ...                  | LP  | T   | ...   | 1FHL J2139.4-4238    | ... | bll   | MH 2136-428             |
|              |         |         |         |         |            |            |        |          |          |                 |          |                 |               |                      |     |     |       | 2FGL J2139.3-4236    |     |       |                         |
|              |         |         |         |         |            |            |        |          |          |                 |          |                 |               |                      |     |     |       | 1FGL J2139.3-4235    |     |       |                         |
|              |         |         |         |         |            |            |        |          |          |                 |          |                 |               |                      |     |     |       | 0FGL J2139.4-4238    |     |       |                         |
| J2139.5+3919 | 324.897 | 39.324  | 87.254  | -9.908  | 0.165      | 0.130      | 63     | 6.3      | 0.4      | 0.1             | 7.6      | 1.2             | 2.69          | 0.17                 | PL  | ... | 1,4   | ...                  | ... | ...   | ...                     |
| J2140.0+4715 | 325.015 | 47.257  | 92.640  | -4.044  | 0.043      | 0.040      | 57     | 25.2     | 3.9      | 0.2             | 23.1     | 1.5             | 2.27          | ...                  | EC  | ... | ...   | 2FGL J2139.8+4714    | ... | PSR   | LAT PSR J2139+4716      |
|              |         |         |         |         |            |            |        |          |          |                 |          |                 |               |                      |     |     |       | 1FGL J2139.9+4715    |     |       |                         |
| J2141.6-6412 | 325.412 | -64.201 | 328.602 | -42.259 | 0.062      | 0.059      | 77     | 16.6     | 1.0      | 0.1             | 14.2     | 1.0             | 2.50          | 0.06                 | PL  | T   | ...   | ...                  | ... | bcu   | PMN J2141-6411          |
| J2141.7-3734 | 325.428 | -37.572 | 5.871   | -49.045 | 0.198      | 0.122      | 21     | 7.9      | 0.4      | 0.1             | 6.7      | 0.9             | 2.59          | 0.11                 | PL  | T   | ...   | 2FGL J2141.7-3739    | ... | fsrq  | PKS 2138-377            |
| J2142.2-2546 | 325.570 | -25.781 | 23.613  | -47.895 | 0.158      | 0.116      | 16     | 6.7      | 0.4      | 0.1             | 5.0      | 0.8             | 2.23          | 0.13                 | PL  | ... | ...   | ...                  | ... | bcu   | PMN J2142-2551          |
| J2142.6-2029 | 325.656 | -20.499 | 31.142  | -46.557 | 0.071      | 0.065      | 57     | 4.1      | 0.1      | 0.1             | 2.1      | 0.8             | 1.52          | 0.33                 | PL  | ... | ...   | 1FHL J2142.6-2027    | ... | ...   | ...                     |
| J2142.7+1957 | 325.682 | 19.958  | 73.733  | -24.392 | 0.068      | 0.060      | 13     | 4.4      | 0.2      | 0.1             | 2.6      | 0.8             | 2.01          | 0.25                 | PL  | ... | ...   | ...                  | ... | ...   | ...                     |
| J2143.1-3928 | 325.781 | -39.467 | 2.963   | -49.265 | 0.080      | 0.056      | 1      | 8.4      | 0.5      | 0.1             | 5.7      | 0.9             | 2.07          | 0.13                 | PL  | ... | ...   | 2FGL J2143.2-3929    | ... | bll   | PMN J2143-3929          |
|              |         |         |         |         |            |            |        |          |          |                 |          |                 |               |                      |     |     |       | 1FGL J2143.1-3927    |     |       |                         |
| J2143.5+1744 | 325.896 | 17.734  | 72.117  | -26.080 | 0.030      | 0.029      | 78     | 60.6     | 4.4      | 0.2             | 64.0     | 1.7             | 2.52          | ...                  | LP  | T   | ...   | 2FGL J2143.5+1743    | ... | fsrq  | OX 169                  |
|              |         |         |         |         |            |            |        |          |          |                 |          |                 |               |                      |     |     |       | 1FGL J2143.4+1742    |     |       |                         |
|              |         |         |         |         |            |            |        |          |          |                 |          |                 |               |                      |     |     |       | 0FGL J2143.2+1741    |     |       |                         |
| J2144.2+3132 | 326.051 | 31.542  | 82.589  | -16.296 | 0.076      | 0.071      | -19    | 8.3      | 0.6      | 0.1             | 7.2      | 1.0             | 2.36          | 0.11                 | PL  | ... | ...   | ...                  | ... | bcu   | MG3 J214415+3132        |
| J2144.6-5640 | 326.155 | -56.680 | 337.889 | -45.749 | 0.084      | 0.076      | -40    | 4.2      | 0.2      | 0.1             | 2.8      | 0.9             | 2.46          | 0.31                 | PL  | ... | ...   | ...                  | ... | ...   | ...                     |
| J2144.6+6606 | 326.163 | 66.104  | 105.527 | 9.766   | 0.097      | 0.085      | -20    | 4.1      | 0.4      | 0.1             | 6.1      | 1.7             | 2.46          | 0.15                 | PL  | ... | ...   | ...                  | ... | ...   | ...                     |
| J2144.9-3356 | 326.229 | -33.936 | 11.475  | -49.607 | 0.051      | 0.050      | 31     | 19.2     | 1.2      | 0.1             | 14.3     | 1.0             | 2.30          | 0.06                 | PL  | T   | ...   | 2FGL J2144.8-3356    | ... | fsrq  | PMN J2145-3357          |
|              |         |         |         |         |            |            |        |          |          |                 |          |                 |               |                      |     |     |       | 1FGL J2145.4-3358    |     |       |                         |
| J2145.5+1007 | 326.376 | 10.130  | 66.047  | -31.538 | 0.066      | 0.061      | -33    | 5.2      | 0.2      | 0.1             | 2.7      | 0.9             | 1.55          | 0.25                 | PL  | ... | ...   | ...                  | ... | ...   | ...                     |

Table 1—Continued

| Name 3FGL     | R.A.    | Decl.   | $l$     | $b$     | $\theta_1$ | $\theta_2$ | $\phi$ | $\sigma$ | $F_{35}$ | $\Delta F_{35}$ | $S_{25}$ | $\Delta S_{25}$ | $\Gamma_{25}$ | $\Delta \Gamma_{25}$ | Mod | Var | Flags | $\gamma$ -ray Assoc. | TeV | Class | ID or Assoc.              |
|---------------|---------|---------|---------|---------|------------|------------|--------|----------|----------|-----------------|----------|-----------------|---------------|----------------------|-----|-----|-------|----------------------|-----|-------|---------------------------|
| J2145.7+0717  | 326.448 | 7.297   | 63.532  | -33.418 | 0.085      | 0.081      | 73     | 8.1      | 0.4      | 0.1             | 7.4      | 1.1             | 2.66          | 0.13                 | PL  | ... | 3     | ...                  | ... | bll   | MS 2143.4+0704            |
| J2146.6-1344  | 326.662 | -13.744 | 40.661  | -44.969 | 0.042      | 0.035      | -86    | 16.3     | 1.0      | 0.1             | 13.7     | 1.8             | 1.66          | 0.07                 | PL  | ... | ...   | 1FHL J2146.5-1344    | ... | bll   | NVSS<br>J214637-134359    |
|               |         |         |         |         |            |            |        |          |          |                 |          |                 |               |                      |     |     |       | 2FGL J2146.6-1345    |     |       |                           |
|               |         |         |         |         |            |            |        |          |          |                 |          |                 |               |                      |     |     |       | 1FGL J2146.6-1345    |     |       |                           |
| J2146.7-1527  | 326.695 | -15.455 | 38.456  | -45.694 | 0.122      | 0.110      | 65     | 6.8      | 0.4      | 0.1             | 5.7      | 0.9             | 2.46          | 0.12                 | PL  | ... | ...   | 2FGL J2146.5-1530    | ... | fsrq  | PKS 2143-156              |
| J2147.2+0929  | 326.810 | 9.498   | 65.811  | -32.275 | 0.046      | 0.042      | -37    | 29.4     | 2.5      | 0.1             | 35.6     | 1.5             | 2.54          | ...                  | LP  | T   | ...   | 2FGL J2147.3+0930    | ... | FSRQ  | PKS 2144+092              |
|               |         |         |         |         |            |            |        |          |          |                 |          |                 |               |                      |     |     |       | 1FGL J2147.2+0929    |     |       |                           |
|               |         |         |         |         |            |            |        |          |          |                 |          |                 |               |                      |     |     |       | 0FGL J2147.1+0931    |     |       |                           |
| J2147.2+4730c | 326.810 | 47.515  | 93.734  | -4.641  | 0.283      | 0.207      | -39    | 4.9      | 0.5      | 0.1             | 8.3      | 1.5             | 2.56          | 0.13                 | PL  | ... | 4,5,6 | ...                  | ... | ...   | ...                       |
| J2147.3-7536  | 326.840 | -75.609 | 315.793 | -36.533 | 0.023      | 0.022      | 58     | 75.8     | 5.3      | 0.2             | 71.7     | 1.6             | 2.47          | ...                  | LP  | T   | ...   | 1FHL J2147.5-7536    | ... | FSRQ  | PKS 2142-75               |
|               |         |         |         |         |            |            |        |          |          |                 |          |                 |               |                      |     |     |       | 2FGL J2147.4-7534    |     |       |                           |
| J2149.6+1915  | 327.408 | 19.256  | 74.445  | -26.042 | 0.119      | 0.113      | -60    | 9.5      | 0.6      | 0.1             | 9.9      | 1.2             | 2.57          | 0.10                 | PL  | T   | ...   | ...                  | ... | bcu   | TXS 2147+191              |
| J2149.7+0323  | 327.441 | 3.384   | 60.554  | -36.634 | 0.079      | 0.060      | -37    | 10.4     | 0.7      | 0.1             | 7.6      | 1.0             | 2.15          | 0.10                 | PL  | ... | ...   | 2FGL J2149.6+0326    | ... | bll   | PKS B2147+031             |
|               |         |         |         |         |            |            |        |          |          |                 |          |                 |               |                      |     |     |       | 1FGL J2149.7+0327    |     |       |                           |
| J2150.2-1411  | 327.568 | -14.187 | 40.609  | -45.953 | 0.047      | 0.041      | -16    | 9.9      | 0.5      | 0.1             | 6.3      | 1.1             | 1.83          | 0.12                 | PL  | ... | ...   | 1FHL J2150.2-1413    | ... | bll   | TXS 2146-144              |
|               |         |         |         |         |            |            |        |          |          |                 |          |                 |               |                      |     |     |       | 2FGL J2150.2-1412    |     |       |                           |
|               |         |         |         |         |            |            |        |          |          |                 |          |                 |               |                      |     |     |       | 1FGL J2150.3-1410    |     |       |                           |
| J2150.5-1754  | 327.640 | -17.911 | 35.639  | -47.455 | 0.116      | 0.113      | 61     | 8.4      | 0.4      | 0.1             | 7.0      | 0.9             | 2.66          | 0.11                 | PL  | ... | ...   | ...                  | ... | ...   | ...                       |
| J2151.6+4154  | 327.903 | 41.906  | 90.718  | -9.449  | 0.058      | 0.046      | -62    | 8.4      | 0.6      | 0.1             | 7.0      | 1.2             | 1.85          | 0.12                 | PL  | ... | ...   | ...                  | ... | ...   | ...                       |
| J2151.6-2744  | 327.918 | -27.736 | 21.316  | -50.335 | 0.242      | 0.181      | -41    | 5.2      | 0.3      | 0.1             | 4.4      | 0.8             | 2.51          | 0.15                 | PL  | ... | ...   | 2FGL J2150.8-2738    | ... | fsrq  | PMN J2151-2742            |
| J2151.8-3025  | 327.953 | -30.429 | 17.130  | -50.756 | 0.078      | 0.077      | -77    | 27.7     | 0.6      | 0.1             | 29.6     | 1.3             | 2.97          | ...                  | LP  | T   | ...   | 2FGL J2151.5-3021    | ... | fsrq  | PKS 2149-306              |
| J2152.4+1735  | 328.107 | 17.585  | 73.647  | -27.693 | 0.091      | 0.080      | 14     | 4.4      | 0.3      | 0.1             | 3.0      | 0.8             | 2.05          | 0.20                 | PL  | ... | ...   | 2FGL J2152.4+1735    | ... | bll   | S3 2150+17                |
|               |         |         |         |         |            |            |        |          |          |                 |          |                 |               |                      |     |     |       | 1FGL J2152.5+1734    |     |       |                           |
| J2152.9-0045  | 328.230 | -0.753  | 56.935  | -39.740 | 0.079      | 0.071      | 30     | 5.4      | 0.3      | 0.1             | 3.8      | 1.0             | 1.95          | 0.19                 | PL  | ... | ...   | ...                  | ... | bll   | RBS 1792                  |
| J2153.9+6626  | 328.486 | 66.448  | 106.477 | 9.427   | 0.139      | 0.117      | -29    | 4.4      | 0.5      | 0.1             | 6.9      | 1.6             | 2.53          | 0.14                 | PL  | ... | ...   | ...                  | ... | ...   | ...                       |
| J2154.0-1137  | 328.507 | -11.628 | 44.487  | -45.663 | 0.097      | 0.086      | -37    | 13.5     | 0.8      | 0.1             | 11.0     | 1.0             | 2.49          | 0.07                 | PL  | T   | ...   | 2FGL J2154.0-1138    | ... | fsrq  | PMN J2153-1136            |
| J2156.0+1818  | 329.014 | 18.301  | 74.910  | -27.789 | 0.054      | 0.051      | 45     | 7.8      | 0.5      | 0.1             | 5.4      | 1.0             | 1.91          | 0.14                 | PL  | ... | ...   | ...                  | ... | bcu   | RX J2156.0+1818           |
| J2156.9-0855  | 329.241 | -8.919  | 48.365  | -45.008 | 0.058      | 0.057      | 2      | 5.7      | 0.3      | 0.1             | 3.2      | 0.9             | 1.90          | 0.17                 | PL  | ... | ...   | ...                  | ... | bll   | FIRST<br>J215650.3-085535 |
| J2157.5+3126  | 329.380 | 31.450  | 84.757  | -18.241 | 0.025      | 0.024      | 10     | 56.7     | 5.8      | 0.2             | 55.3     | 2.0             | 2.28          | ...                  | LP  | T   | ...   | 2FGL J2157.4+3129    | ... | fsrq  | B2 2155+31                |
|               |         |         |         |         |            |            |        |          |          |                 |          |                 |               |                      |     |     |       | 1FGL J2157.4+3129    |     |       |                           |
|               |         |         |         |         |            |            |        |          |          |                 |          |                 |               |                      |     |     |       | 0FGL J2157.5+3125    |     |       |                           |
| J2158.0-1501  | 329.522 | -15.032 | 40.621  | -48.024 | 0.053      | 0.048      | -64    | 16.4     | 1.1      | 0.1             | 12.6     | 1.1             | 2.27          | 0.07                 | PL  | T   | ...   | 2FGL J2157.9-1501    | ... | fsrq  | PKS 2155-152              |
|               |         |         |         |         |            |            |        |          |          |                 |          |                 |               |                      |     |     |       | 1FGL J2157.9-1503    |     |       |                           |
| J2158.8-3013  | 329.720 | -30.227 | 17.729  | -52.249 | 0.009      | 0.009      | -87    | 142.1    | 21.7     | 0.4             | 230.5    | 6.2             | 1.83          | ...                  | LP  | T   | ...   | 1FHL J2158.8-3013    | P   | bll   | PKS 2155-304              |
|               |         |         |         |         |            |            |        |          |          |                 |          |                 |               |                      |     |     |       | 2FGL J2158.8-3013    |     |       |                           |

Table 1—Continued

| Name         | 3FGL    | R.A.    | Decl.   | $l$     | $b$   | $\theta_1$ | $\theta_2$ | $\phi$ | $\sigma$ | $F_{35}$ | $\Delta F_{35}$ | $S_{25}$ | $\Delta S_{25}$ | $\Gamma_{25}$ | $\Delta \Gamma_{25}$ | Mod | Var | Flags                                                                                                                                     | $\gamma$ -ray Assoc.                                                       | TeV  | Class              | ID or Assoc.           |
|--------------|---------|---------|---------|---------|-------|------------|------------|--------|----------|----------|-----------------|----------|-----------------|---------------|----------------------|-----|-----|-------------------------------------------------------------------------------------------------------------------------------------------|----------------------------------------------------------------------------|------|--------------------|------------------------|
|              |         |         |         |         |       |            |            |        |          |          |                 |          |                 |               |                      |     |     |                                                                                                                                           | 1FGL J2158.8–3013<br>0FGL J2158.8–3014<br>3EG J2158–3023<br>EGR J2200–3015 |      |                    |                        |
| J2159.2–2841 | 329.817 | –28.687 | 20.238  | –52.139 | 0.060 | 0.053      | –18        | 7.8    | 0.4      | 0.1      | 4.8             | 0.9      | 1.94            | 0.16          | PL                   | ... | ... | ...                                                                                                                                       |                                                                            | ...  | bcu                | NVSS<br>J215910–284115 |
| J2159.8+1025 | 329.951 | 10.432  | 69.107  | –33.955 | 0.213 | 0.195      | 66         | 5.0    | 0.3      | 0.1      | 4.6             | 0.9      | 2.63            | 0.19          | PL                   | ... | ... | 2FGL J2159.9+1023                                                                                                                         | ...                                                                        | ...  | bll                | TXS 2157+102           |
| J2200.0–6930 | 330.024 | –69.504 | 321.310 | –40.968 | 0.127 | 0.081      | 42         | 9.5    | 0.5      | 0.1      | 7.0             | 0.9      | 2.48            | 0.11          | PL                   | ... | ... | 2FGL J2200.1–6931                                                                                                                         | ...                                                                        | ...  | ...                | ...                    |
| J2200.2+2139 | 330.061 | 21.654  | 78.288  | –26.020 | 0.066 | 0.062      | –23        | 5.2    | 0.3      | 0.1      | 2.9             | 0.8      | 1.98            | 0.21          | PL                   | ... | ... | ...                                                                                                                                       | ...                                                                        | ...  | bll                | TXS 2157+213           |
| J2200.9–2412 | 330.240 | –24.204 | 27.490  | –51.655 | 0.123 | 0.101      | –2         | 5.5    | 0.3      | 0.1      | 3.9             | 0.8      | 2.45            | 0.17          | PL                   | ... | 1   | ...                                                                                                                                       | ...                                                                        | ...  | bcu                | NVSS<br>J220036–241428 |
| J2201.7+5047 | 330.434 | 50.800  | 97.642  | –3.546  | 0.042 | 0.041      | –82        | 27.4   | 2.2      | 0.2      | 36.2            | 1.5      | 2.59            | 0.04          | PL                   | T   | 10  | ...                                                                                                                                       | ...                                                                        | fsrq | NRAO 676           |                        |
| J2202.4–8339 | 330.610 | –83.656 | 307.944 | –31.735 | 0.052 | 0.048      | –58        | 23.1   | 2.0      | 0.1      | 23.1            | 1.8      | 2.47            | ...           | LP                   | T   | ... | 2FGL J2201.9–8335                                                                                                                         | ...                                                                        | fsrq | PKS 2155–83        |                        |
| J2202.7+4217 | 330.687 | 42.284  | 92.598  | –10.440 | 0.012 | 0.012      | 87         | 128.8  | 16.5     | 0.3      | 177.3           | 3.0      | 2.25            | ...           | LP                   | T   | ... | 1FGL J2201.6–8327<br>1FHL J2202.7+4216<br>2FGL J2202.8+4216<br>1FGL J2202.8+4216<br>0FGL J2202.4+4217<br>3EG J2202+4217<br>EGR J2204+4225 | P                                                                          | BLL  | BL Lacertae<br>133 |                        |
| J2203.4+1725 | 330.864 | 17.427  | 75.672  | –29.638 | 0.023 | 0.022      | –35        | 54.1   | 4.8      | 0.2      | 49.3            | 1.8      | 2.26            | ...           | LP                   | T   | ... | 1FHL J2203.4+1724<br>2FGL J2203.4+1726<br>1FGL J2203.5+1726<br>0FGL J2203.2+1731                                                          | ...                                                                        | fsrq | PKS 2201+171       |                        |
| J2203.7+3143 | 330.939 | 31.732  | 86.027  | –18.869 | 0.339 | 0.289      | 30         | 5.0    | 0.2      | 0.1      | 7.4             | 1.4      | 3.07            | 0.19          | PL                   | ... | ... | ...                                                                                                                                       | ...                                                                        | fsrq | 4C +31.63          |                        |
| J2204.4+0439 | 331.104 | 4.666   | 64.725  | –38.656 | 0.063 | 0.055      | 21         | 8.4    | 0.5      | 0.1      | 5.5             | 0.9      | 2.12            | 0.11          | PL                   | ... | ... | 2FGL J2204.6+0442<br>1FGL J2204.6+0442                                                                                                    | ...                                                                        | ...  | bll                | 4C +04.77              |
| J2205.9–4704 | 331.476 | –47.081 | 350.001 | –52.059 | 0.168 | 0.130      | 77         | 4.4    | 0.1      | 0.1      | 3.7             | 0.8      | 2.91            | 0.25          | PL                   | ... | ... | ...                                                                                                                                       | ...                                                                        | ...  | ...                | ...                    |
| J2206.5+6451 | 331.629 | 64.856  | 106.530 | 7.377   | 0.175 | 0.151      | –45        | 8.6    | 0.9      | 0.2      | 12.4            | 1.9      | 2.52            | ...           | LP                   | ... | ... | 2FGL J2206.6+6500<br>1FGL J2207.5+6440                                                                                                    | ...                                                                        | ...  | ...                | ...                    |
| J2206.9–0031 | 331.747 | –0.524  | 59.959  | –42.429 | 0.075 | 0.069      | –58        | 9.4    | 0.6      | 0.1      | 7.4             | 1.0      | 2.25            | 0.10          | PL                   | ... | ... | 2FGL J2206.6–0029<br>1FGL J2207.1–0021                                                                                                    | ...                                                                        | ...  | bll                | PMN J2206–0031         |
| J2207.8–5345 | 331.950 | –53.764 | 339.908 | –49.941 | 0.073 | 0.064      | 51         | 18.4   | 0.8      | 0.1      | 12.9            | 0.8      | 2.58            | 0.06          | PL                   | T   | ... | 2FGL J2208.1–5345<br>1FGL J2207.8–5344<br>0FGL J2207.0–5347                                                                               | ...                                                                        | fsrq | PKS 2204–54        |                        |
| J2209.0+3652 | 332.267 | 36.869  | 90.238  | –15.491 | 0.150 | 0.133      | –7         | 5.6    | 0.2      | 0.1      | 5.8             | 1.0      | 2.84            | 0.16          | PL                   | ... | 1   | ...                                                                                                                                       | ...                                                                        | ...  | ...                | ...                    |
| J2209.8–0450 | 332.467 | –4.850  | 55.685  | –45.558 | 0.087 | 0.073      | 37         | 6.5    | 0.2      | 0.1      | 4.3             | 1.3      | 1.27            | 0.32          | PL                   | ... | ... | ...                                                                                                                                       | ...                                                                        | ...  | ...                | ...                    |

Table 1—Continued

| Name 3FGL    | R.A.    | Decl.   | $l$     | $b$     | $\theta_1$ | $\theta_2$ | $\phi$ | $\sigma$ | $F_{35}$ | $\Delta F_{35}$ | $S_{25}$ | $\Delta S_{25}$ | $\Gamma_{25}$ | $\Delta \Gamma_{25}$ | Mod | Var | Flags | $\gamma$ -ray Assoc.                                        | TeV | Class | ID or Assoc.                   |
|--------------|---------|---------|---------|---------|------------|------------|--------|----------|----------|-----------------|----------|-----------------|---------------|----------------------|-----|-----|-------|-------------------------------------------------------------|-----|-------|--------------------------------|
| J2210.1+5925 | 332.526 | 59.421  | 103.686 | 2.719   | 0.207      | 0.166      | 27     | 9.7      | 1.2      | 0.2             | 20.5     | 2.1             | 2.62          | 0.07                 | PL  | ... | 3     | 2FGL J2210.1+5913                                           | ... | ...   | ...                            |
| J2210.1+6043 | 332.531 | 60.725  | 104.441 | 3.782   | 0.060      | 0.053      | 34     | 5.2      | 0.5      | 0.2             | 6.3      | 2.2             | 2.21          | 0.22                 | PL  | ... | ...   | ...                                                         | ... | ...   | ...                            |
| J2210.2+6509 | 332.553 | 65.164  | 107.031 | 7.397   | 0.093      | 0.082      | -56    | 4.4      | 0.6      | 0.1             | 8.3      | 2.3             | 2.48          | 0.16                 | PL  | ... | ...   | ...                                                         | ... | ...   | ...                            |
| J2212.0+2355 | 333.001 | 23.924  | 82.223  | -26.077 | 0.043      | 0.041      | 76     | 15.9     | 1.1      | 0.1             | 12.7     | 1.1             | 2.21          | 0.07                 | PL  | ... | ...   | 2FGL J2211.9+2355<br>1FGL J2212.1+2358<br>3EG J2209+2401    | ... | fsrq  | PKS 2209+236                   |
| J2212.3-7039 | 333.090 | -70.656 | 319.253 | -41.059 | 0.151      | 0.139      | -46    | 5.2      | 0.2      | 0.1             | 4.4      | 0.9             | 2.76          | 0.22                 | PL  | ... | ...   | ...                                                         | ... | bcu   | PMN J2211-7039                 |
| J2212.5+0703 | 333.147 | 7.060   | 68.743  | -38.565 | 0.096      | 0.083      | 11     | 14.3     | 1.2      | 0.1             | 9.0      | 1.0             | 2.22          | ...                  | LP  | ... | ...   | 2FGL J2212.6+0702<br>1FGL J2212.9+0654                      | ... | ...   | ...                            |
| J2212.6+2801 | 333.174 | 28.019  | 85.175  | -22.981 | 0.070      | 0.054      | 78     | 7.9      | 0.4      | 0.1             | 5.4      | 1.1             | 1.79          | 0.12                 | PL  | ... | ...   | 1FHL J2212.5+2803                                           | ... | bcu   | MG3 J221240+2759               |
| J2213.1-2532 | 333.283 | -25.535 | 26.333  | -54.640 | 0.202      | 0.116      | -20    | 10.3     | 0.5      | 0.1             | 7.6      | 0.8             | 2.55          | 0.10                 | PL  | ... | ...   | 2FGL J2213.1-2527<br>1FGL J2213.1-2529                      | ... | fsrq  | PKS 2210-25                    |
| J2213.6-4755 | 333.405 | -47.921 | 348.016 | -53.032 | 0.068      | 0.067      | -84    | 5.7      | 0.3      | 0.1             | 2.9      | 0.7             | 1.89          | 0.17                 | PL  | ... | ...   | 2FGL J2213.7-4754                                           | ... | bcu   | SUMSS<br>J221330-475426        |
| J2214.6+3000 | 333.661 | 30.008  | 86.854  | -21.667 | 0.024      | 0.024      | 43     | 50.7     | 5.6      | 0.2             | 33.0     | 1.2             | 2.02          | ...                  | EC  | ... | ...   | 2FGL J2214.7+3000<br>1FGL J2214.8+3002<br>0FGL J2214.8+3002 | ... | PSR   | PSR J2214+3000<br>J2214.8+3002 |
| J2215.5+6122 | 333.877 | 61.380  | 105.352 | 3.950   | 0.143      | 0.116      | -58    | 5.7      | 0.8      | 0.2             | 13.0     | 2.3             | 2.53          | 0.10                 | PL  | ... | ...   | ...                                                         | ... | ...   | ...                            |
| J2215.6+5134 | 333.911 | 51.577  | 99.872  | -4.181  | 0.040      | 0.036      | 1      | 19.3     | 2.2      | 0.2             | 13.7     | 1.1             | 2.13          | ...                  | EC  | ... | ...   | 2FGL J2215.7+5135<br>1FGL J2216.1+5139                      | ... | PSR   | PSR J2215+5135                 |
| J2217.0+2421 | 334.268 | 24.364  | 83.535  | -26.460 | 0.064      | 0.051      | 47     | 13.5     | 1.0      | 0.1             | 11.0     | 1.1             | 2.22          | 0.08                 | PL  | ... | ...   | 2FGL J2217.1+2422<br>1FGL J2217.1+2423                      | ... | bll   | B2 2214+24B                    |
| J2217.2+6346 | 334.307 | 63.774  | 106.860 | 5.824   | 0.069      | 0.056      | -32    | 7.1      | 0.9      | 0.1             | 11.4     | 2.0             | 2.31          | 0.10                 | PL  | ... | 4,5   | ...                                                         | ... | ...   | ...                            |
| J2217.8+3207 | 334.462 | 32.132  | 88.802  | -20.374 | 0.265      | 0.180      | -15    | 4.3      | 0.3      | 0.1             | 3.8      | 0.9             | 2.39          | 0.18                 | PL  | ... | ...   | ...                                                         | ... | ...   | ...                            |
| J2219.2+1806 | 334.804 | 18.103  | 79.451  | -31.629 | 0.142      | 0.111      | 3      | 6.7      | 0.4      | 0.1             | 5.3      | 0.9             | 2.50          | 0.13                 | PL  | ... | ...   | 2FGL J2219.1+1805<br>1FGL J2219.3+1804                      | ... | fsrq  | MG1 J221916+1806               |
| J2220.3+2812 | 335.086 | 28.203  | 86.757  | -23.858 | 0.141      | 0.080      | -49    | 4.9      | 0.3      | 0.1             | 3.0      | 0.8             | 1.83          | 0.19                 | PL  | ... | ...   | ...                                                         | ... | bcu   | RX J2220.4+2814                |
| J2220.6-6833 | 335.151 | -68.554 | 320.733 | -42.988 | 0.113      | 0.094      | -77    | 5.8      | 0.3      | 0.1             | 3.3      | 0.7             | 2.01          | 0.15                 | PL  | ... | ...   | ...                                                         | ... | ...   | ...                            |
| J2221.6-5225 | 335.411 | -52.422 | 340.358 | -52.398 | 0.039      | 0.037      | 32     | 15.9     | 0.8      | 0.1             | 9.5      | 1.1             | 1.93          | 0.08                 | PL  | ... | ...   | 1FHL J2221.3-5225<br>2FGL J2221.6-5223<br>1FGL J2222.5-5218 | ... | bll   | PMN J2221-5224                 |
| J2221.6+6507 | 335.414 | 65.127  | 108.012 | 6.690   | 0.268      | 0.119      | -46    | 7.4      | 0.7      | 0.2             | 9.3      | 1.7             | 2.65          | ...                  | LP  | ... | ...   | ...                                                         | ... | ...   | ...                            |
| J2221.7+6318 | 335.435 | 63.303  | 107.022 | 5.154   | 0.222      | 0.172      | -44    | 8.4      | 1.1      | 0.2             | 11.9     | 1.7             | 2.39          | ...                  | LP  | ... | 1     | 2FGL J2221.0+6307                                           | ... | ...   | ...                            |
| J2222.3-3500 | 335.590 | -35.012 | 9.649   | -57.320 | 0.155      | 0.145      | 43     | 4.6      | 0.2      | 0.1             | 3.1      | 0.6             | 2.37          | 0.18                 | PL  | T   | ...   | 2FGL J2222.0-3503                                           | ... | fsrq  | PKS 2220-351                   |
| J2223.3+0103 | 335.838 | 1.052   | 65.216  | -44.595 | 0.085      | 0.066      | 56     | 6.3      | 0.3      | 0.1             | 4.0      | 1.0             | 1.81          | 0.16                 | PL  | ... | ...   | 1FHL J2223.4+0104<br>2FGL J2223.4+0104                      | ... | ...   | ...                            |

Table 1—Continued

| Name 3FGL    | R.A.    | Decl.   | $l$     | $b$     | $\theta_1$ | $\theta_2$ | $\phi$ | $\sigma$ | $F_{35}$ | $\Delta F_{35}$ | $S_{25}$ | $\Delta S_{25}$ | $\Gamma_{25}$ | $\Delta \Gamma_{25}$ | Mod | Var | Flags | $\gamma$ -ray Assoc. | TeV | Class | ID or Assoc.     |
|--------------|---------|---------|---------|---------|------------|------------|--------|----------|----------|-----------------|----------|-----------------|---------------|----------------------|-----|-----|-------|----------------------|-----|-------|------------------|
|              |         |         |         |         |            |            |        |          |          |                 |          |                 |               |                      |     |     |       | 1FGL J2223.3+0103    |     |       |                  |
| J2224.4+0351 | 336.102 | 3.859   | 68.338  | -42.901 | 0.075      | 0.051      | 57     | 5.8      | 0.2      | 0.1             | 3.3      | 1.0             | 1.60          | 0.21                 | PL  | ... | ...   | ...                  | ... | ...   | ...              |
| J2224.6-1122 | 336.174 | -11.370 | 50.287  | -52.148 | 0.274      | 0.125      | 47     | 6.5      | 0.4      | 0.1             | 5.3      | 0.9             | 2.45          | 0.14                 | PL  | ... | ...   | ...                  | ... | bll   | PKS 2221-116     |
| J2225.8+6045 | 336.465 | 60.765  | 106.067 | 2.753   | 0.536      | 0.191      | 40     | 4.1      | 0.5      | 0.2             | 5.9      | 2.0             | 1.95          | 0.20                 | PL  | ... | 9     | 3EG J2227+6122       | E   | spp   | ...              |
|              |         |         |         |         |            |            |        |          |          |                 |          |                 |               |                      |     |     |       | EGR J2227+6114       |     |       |                  |
| J2225.8-0454 | 336.468 | -4.901  | 59.040  | -48.830 | 0.052      | 0.047      | 82     | 27.0     | 1.9      | 0.1             | 24.7     | 1.3             | 2.36          | 0.04                 | PL  | T   | ...   | 2FGL J2225.6-0454    | ... | fsrq  | 3C 446           |
|              |         |         |         |         |            |            |        |          |          |                 |          |                 |               |                      |     |     |       | 1FGL J2225.8-0457    |     |       |                  |
| J2227.8+0040 | 336.958 | 0.674   | 65.865  | -45.685 | 0.139      | 0.101      | -71    | 9.2      | 0.7      | 0.1             | 7.9      | 1.1             | 2.14          | 0.09                 | PL  | ... | ...   | 2FGL J2227.8+0051    | ... | bll   | PMN J2227+0037   |
| J2228.5-1636 | 337.149 | -16.602 | 43.121  | -55.367 | 0.100      | 0.096      | -25    | 5.7      | 0.3      | 0.1             | 4.4      | 0.9             | 2.51          | 0.19                 | PL  | ... | ...   | 2FGL J2228.6-1633    | ... | ...   | ...              |
|              |         |         |         |         |            |            |        |          |          |                 |          |                 |               |                      |     |     |       | 1FGL J2228.5-1633    |     |       |                  |
| J2229.0+6114 | 337.271 | 61.242  | 106.650 | 2.954   | 0.011      | 0.010      | 47     | 106.6    | 29.5     | 0.5             | 234.7    | 3.2             | 2.17          | ...                  | EC  | ... | ...   | 1FHL J2229.0+6114    | E   | PSR   | PSR J2229+6114   |
|              |         |         |         |         |            |            |        |          |          |                 |          |                 |               |                      |     |     |       | 2FGL J2229.0+6114    |     |       |                  |
|              |         |         |         |         |            |            |        |          |          |                 |          |                 |               |                      |     |     |       | 1FGL J2229.0+6114    |     |       |                  |
|              |         |         |         |         |            |            |        |          |          |                 |          |                 |               |                      |     |     |       | 0FGL J2229.0+6114    |     |       |                  |
|              |         |         |         |         |            |            |        |          |          |                 |          |                 |               |                      |     |     |       | 3EG J2227+6122       |     |       |                  |
|              |         |         |         |         |            |            |        |          |          |                 |          |                 |               |                      |     |     |       | EGR J2227+6114       |     |       |                  |
|              |         |         |         |         |            |            |        |          |          |                 |          |                 |               |                      |     |     |       | 1AGL J2231+6109      |     |       |                  |
| J2229.1+2255 | 337.283 | 22.929  | 85.033  | -29.277 | 0.051      | 0.050      | -20    | 6.5      | 0.3      | 0.1             | 4.1      | 0.9             | 2.24          | 0.17                 | PL  | ... | ...   | ...                  | ... | ...   | ...              |
| J2229.7-0833 | 337.434 | -8.551  | 55.234  | -51.717 | 0.032      | 0.030      | -48    | 58.6     | 3.5      | 0.2             | 54.1     | 1.4             | 2.55          | ...                  | LP  | T   | ...   | 2FGL J2229.7-0832    | ... | FSRQ  | PKS 2227-08      |
|              |         |         |         |         |            |            |        |          |          |                 |          |                 |               |                      |     |     |       | 1FGL J2229.7-0832    |     |       |                  |
|              |         |         |         |         |            |            |        |          |          |                 |          |                 |               |                      |     |     |       | 0FGL J2229.8-0829    |     |       |                  |
| J2230.5-7817 | 337.641 | -78.298 | 311.292 | -36.440 | 0.068      | 0.065      | -74    | 12.4     | 0.7      | 0.1             | 10.6     | 1.0             | 2.51          | 0.08                 | PL  | T   | ...   | ...                  | ... | bcu   | PKS 2225-785     |
| J2230.6-4419 | 337.669 | -44.331 | 352.169 | -57.026 | 0.170      | 0.140      | 73     | 5.6      | 0.2      | 0.1             | 3.7      | 0.7             | 2.57          | 0.17                 | PL  | ... | ...   | ...                  | ... | fsrq  | PKS 2227-445     |
| J2232.5+1143 | 338.139 | 11.720  | 77.418  | -38.583 | 0.026      | 0.025      | -61    | 72.2     | 5.0      | 0.2             | 72.6     | 1.6             | 2.52          | ...                  | LP  | T   | ...   | 2FGL J2232.4+1143    | ... | FSRQ  | CTA 102          |
|              |         |         |         |         |            |            |        |          |          |                 |          |                 |               |                      |     |     |       | 1FGL J2232.5+1144    |     |       |                  |
|              |         |         |         |         |            |            |        |          |          |                 |          |                 |               |                      |     |     |       | 0FGL J2232.4+1141    |     |       |                  |
|              |         |         |         |         |            |            |        |          |          |                 |          |                 |               |                      |     |     |       | 3EG J2232+1147       |     |       |                  |
| J2232.9-2021 | 338.238 | -20.358 | 37.461  | -57.702 | 0.058      | 0.057      | 42     | 5.9      | 0.4      | 0.1             | 4.0      | 0.8             | 2.08          | 0.15                 | PL  | ... | ...   | ...                  | ... | bcu   | 1RXS             |
|              |         |         |         |         |            |            |        |          |          |                 |          |                 |               |                      |     |     |       |                      |     |       | J223249.5-202232 |
| J2233.1+6542 | 338.279 | 65.715  | 109.343 | 6.561   | 0.096      | 0.086      | -47    | 12.7     | 1.5      | 0.2             | 17.2     | 1.7             | 2.52          | ...                  | LP  | ... | ...   | ...                  | ... | ...   | ...              |
| J2233.5-1235 | 338.397 | -12.600 | 50.305  | -54.646 | 0.183      | 0.142      | 10     | 4.5      | 0.3      | 0.1             | 3.8      | 0.9             | 2.37          | 0.20                 | PL  | ... | ...   | ...                  | ... | bcu   | PKS 2231-127     |
| J2234.1-2655 | 338.530 | -26.928 | 25.307  | -59.517 | 0.061      | 0.055      | -41    | 8.2      | 0.4      | 0.1             | 4.7      | 0.8             | 2.19          | 0.14                 | PL  | ... | ...   | ...                  | ... | bcu   | PMN J2234-2656   |
| J2234.8+0945 | 338.710 | 9.753   | 76.305  | -40.440 | 0.065      | 0.060      | 7      | 14.8     | 1.4      | 0.1             | 8.3      | 1.0             | 2.19          | ...                  | EC  | ... | ...   | 2FGL J2234.7+0945    | ... | PSR   | PSR J2234+0944   |
|              |         |         |         |         |            |            |        |          |          |                 |          |                 |               |                      |     |     |       | 1FGL J2234.8+0944    |     |       |                  |
| J2235.3-4835 | 338.836 | -48.590 | 344.487 | -56.087 | 0.089      | 0.082      | 2      | 15.8     | 0.7      | 0.1             | 10.8     | 0.8             | 2.49          | 0.07                 | PL  | T   | ...   | 2FGL J2234.9-4831    | ... | fsrq  | PKS 2232-488     |
|              |         |         |         |         |            |            |        |          |          |                 |          |                 |               |                      |     |     |       | 1FGL J2235.7-4817    |     |       |                  |

Table 1—Continued

| Name 3FGL    | R.A.    | Decl.   | $l$     | $b$     | $\theta_1$ | $\theta_2$ | $\phi$ | $\sigma$ | $F_{35}$ | $\Delta F_{35}$ | $S_{25}$ | $\Delta S_{25}$ | $\Gamma_{25}$ | $\Delta \Gamma_{25}$ | Mod | Var | Flags  | $\gamma$ -ray Assoc. | TeV | Class | ID or Assoc.       |
|--------------|---------|---------|---------|---------|------------|------------|--------|----------|----------|-----------------|----------|-----------------|---------------|----------------------|-----|-----|--------|----------------------|-----|-------|--------------------|
| J2235.6–2319 | 338.911 | –23.329 | 32.362  | –59.149 | 0.400      | 0.251      | 43     | 9.3      | 0.3      | 0.1             | 7.3      | 0.8             | 2.82          | 0.11                 | PL  | T   | ...    | EGR J2233–4812       | ... | bcu   | PMN J2236–2309     |
| J2236.0–3629 | 339.006 | –36.499 | 6.259   | –59.925 | 0.077      | 0.058      | 1      | 14.3     | 0.8      | 0.1             | 9.1      | 0.9             | 2.20          | 0.07                 | PL  | T   | ...    | 2FGL J2236.1–3628    | ... | bll   | NVSS               |
| J2236.0–1706 | 339.019 | –17.105 | 43.595  | –57.207 | 0.108      | 0.099      | –30    | 5.4      | 0.3      | 0.1             | 3.8      | 0.8             | 2.13          | 0.16                 | PL  | ... | ...    | ...                  | ... | fsrq  | J223554–362901     |
| J2236.2–5049 | 339.057 | –50.828 | 340.880 | –55.149 | 0.227      | 0.188      | –59    | 5.8      | 0.3      | 0.1             | 4.3      | 0.8             | 2.61          | 0.15                 | PL  | ... | ...    | ...                  | ... | bcu   | PKS 2233–173       |
| J2236.3+2829 | 339.077 | 28.489  | 90.107  | –25.635 | 0.027      | 0.027      | 13     | 52.1     | 4.3      | 0.2             | 43.6     | 1.6             | 2.28          | ...                  | LP  | T   | ...    | 1FHL J2236.2+2827    | ... | bll   | SUMSS              |
| J2236.5–1432 | 339.135 | –14.545 | 47.890  | –56.203 | 0.019      | 0.018      | –10    | 69.5     | 6.9      | 0.2             | 63.9     | 2.2             | 2.15          | ...                  | LP  | T   | ...    | 2FGL J2236.4+2828    | ... | BLL   | J223605–505521     |
| J2237.1–3921 | 339.289 | –39.361 | 0.592   | –59.602 | 0.047      | 0.045      | –72    | 11.6     | 0.6      | 0.1             | 7.2      | 0.8             | 2.23          | 0.09                 | PL  | T   | ...    | 1FHL J2236.3–1432    | ... | bll   | B2 2234+28A        |
| J2237.5–8326 | 339.391 | –83.437 | 307.220 | –32.537 | 0.111      | 0.104      | 24     | 6.1      | 0.5      | 0.1             | 7.3      | 1.5             | 2.43          | 0.14                 | PL  | ... | ...    | 2FGL J2236.5–1431    | ... | fsrq  | PKS 2233–148       |
| J2237.9+6320 | 339.482 | 63.334  | 108.598 | 4.241   | 0.101      | 0.092      | 21     | 7.2      | 0.6      | 0.1             | 9.7      | 1.4             | 2.40          | ...                  | LP  | ... | 1,3,12 | 1FGL J2236.4–1432    | ... | BLL   | 2FGL J2237.2–3920  |
| J2238.4+5903 | 339.606 | 59.053  | 106.553 | 0.478   | 0.024      | 0.023      | 77     | 34.9     | 7.9      | 0.3             | 59.0     | 4.5             | 2.24          | ...                  | EC  | ... | ...    | 2FGL J2237.2–3919    | ... | fsrq  | NVSS               |
| J2240.9+5831 | 340.241 | 58.526  | 106.586 | –0.142  | 0.096      | 0.083      | –9     | 7.7      | 1.6      | 1.3             | 7.7      | 7.6             | 2.26          | ...                  | EC  | ... | 5      | 1FGL J2237.2–3919    | ... | ...   | J223708–392137     |
| J2240.9+4121 | 340.242 | 41.353  | 98.148  | –15.156 | 0.083      | 0.076      | –9     | 5.1      | 0.4      | 0.1             | 4.7      | 1.2             | 2.20          | 0.16                 | PL  | ... | ...    | 2FGL J2237.2+6316    | ... | ...   | ...                |
| J2241.6–5237 | 340.418 | –52.623 | 337.443 | –54.916 | 0.025      | 0.024      | 82     | 51.8     | 5.2      | 0.2             | 31.0     | 1.2             | 1.99          | ...                  | EC  | ... | ...    | 2FGL J2238.4+5902    | ... | PSR   | LAT PSR J2238+5903 |
| J2243.2–3933 | 340.806 | –39.565 | 359.613 | –60.685 | 0.127      | 0.093      | –42    | 5.6      | 0.3      | 0.1             | 3.4      | 0.7             | 2.12          | 0.15                 | PL  | ... | ...    | 1FGL J2238.4+5903    | ... | PSR   | PSR J2238+5903     |
| J2243.4–2541 | 340.864 | –25.694 | 28.454  | –61.385 | 0.046      | 0.044      | 2      | 25.9     | 1.6      | 0.1             | 19.6     | 1.1             | 2.27          | 0.05                 | PL  | ... | ...    | 2FGL J2239.8+5825    | ... | PSR   | PSR J2240+5832     |
| J2243.6–1230 | 340.925 | –12.510 | 52.644  | –56.733 | 0.067      | 0.064      | –71    | 6.8      | 0.4      | 0.1             | 4.4      | 0.9             | 2.14          | 0.17                 | PL  | ... | ...    | 1FGL J2240.9+5825    | ... | bll   | B3 2238+410        |
| J2243.9+2021 | 340.991 | 20.365  | 86.590  | –33.361 | 0.019      | 0.017      | 61     | 45.9     | 4.1      | 0.2             | 50.9     | 2.8             | 1.79          | 0.03                 | PL  | ... | ...    | 2FGL J2241.7–5236    | ... | PSR   | PSR J2241–5236     |
| J2244.1+4057 | 341.043 | 40.965  | 98.494  | –15.790 | 0.038      | 0.037      | 33     | 18.6     | 1.6      | 0.1             | 19.9     | 1.5             | 2.29          | 0.05                 | PL  | T   | ...    | 1FGL J2241.9–5236    | ... | PSR   | PSR J2241–5236     |
| J2244.6+2503 | 341.160 | 25.051  | 89.763  | –29.533 | 0.091      | 0.077      | 58     | 4.3      | 0.2      | 0.1             | 2.7      | 0.8             | 1.92          | 0.18                 | PL  | ... | ...    | 0FGL J2241.7–5239    | ... | bcu   | NVSS               |
| J2246.2+1547 | 341.558 | 15.791  | 83.920  | –37.421 | 0.048      | 0.046      | –61    | 9.5      | 0.7      | 0.1             | 7.8      | 1.5             | 2.18          | 0.16                 | PL  | ... | ...    | 2FGL J2243.2–2540    | ... | bll   | J224326–393353     |
| J2246.3+1549 | 341.558 | 15.791  | 83.920  | –37.421 | 0.048      | 0.046      | –61    | 9.5      | 0.7      | 0.1             | 7.8      | 1.5             | 2.18          | 0.16                 | PL  | ... | ...    | 1FGL J2243.1–2541    | ... | bll   | PKS 2240–260       |
| J2246.3+1549 | 341.558 | 15.791  | 83.920  | –37.421 | 0.048      | 0.046      | –61    | 9.5      | 0.7      | 0.1             | 7.8      | 1.5             | 2.18          | 0.16                 | PL  | ... | ...    | ...                  | ... | bll   | RBS 1888           |
| J2246.3+1549 | 341.558 | 15.791  | 83.920  | –37.421 | 0.048      | 0.046      | –61    | 9.5      | 0.7      | 0.1             | 7.8      | 1.5             | 2.18          | 0.16                 | PL  | ... | ...    | 1FHL J2244.0+2020    | ... | bll   | RGB J2243+203      |
| J2246.3+1549 | 341.558 | 15.791  | 83.920  | –37.421 | 0.048      | 0.046      | –61    | 9.5      | 0.7      | 0.1             | 7.8      | 1.5             | 2.18          | 0.16                 | PL  | ... | ...    | 2FGL J2243.9+2021    | ... | bll   | TXS 2241+406       |
| J2246.3+1549 | 341.558 | 15.791  | 83.920  | –37.421 | 0.048      | 0.046      | –61    | 9.5      | 0.7      | 0.1             | 7.8      | 1.5             | 2.18          | 0.16                 | PL  | ... | ...    | 1FGL J2244.0+2021    | ... | bll   | TXS 2241+406       |
| J2246.3+1549 | 341.558 | 15.791  | 83.920  | –37.421 | 0.048      | 0.046      | –61    | 9.5      | 0.7      | 0.1             | 7.8      | 1.5             | 2.18          | 0.16                 | PL  | ... | ...    | 2FGL J2244.1+4059    | ... | bll   | TXS 2241+406       |
| J2246.3+1549 | 341.558 | 15.791  | 83.920  | –37.421 | 0.048      | 0.046      | –61    | 9.5      | 0.7      | 0.1             | 7.8      | 1.5             | 2.18          | 0.16                 | PL  | ... | ...    | 1FGL J2243.4+4104    | ... | bll   | TXS 2241+406       |
| J2246.3+1549 | 341.558 | 15.791  | 83.920  | –37.421 | 0.048      | 0.046      | –61    | 9.5      | 0.7      | 0.1             | 7.8      | 1.5             | 2.18          | 0.16                 | PL  | ... | ...    | ...                  | ... | ...   | ...                |
| J2246.3+1549 | 341.558 | 15.791  | 83.920  | –37.421 | 0.048      | 0.046      | –61    | 9.5      | 0.7      | 0.1             | 7.8      | 1.5             | 2.18          | 0.16                 | PL  | ... | ...    | 2FGL J2246.3+1549    | ... | bcu   | NVSS               |
| J2246.3+1549 | 341.558 | 15.791  | 83.920  | –37.421 | 0.048      | 0.046      | –61    | 9.5      | 0.7      | 0.1             | 7.8      | 1.5             | 2.18          | 0.16                 | PL  | ... | ...    | 1FGL J2246.3+1549    | ... | bcu   | J224604+154437     |
| J2246.3+1549 | 341.558 | 15.791  | 83.920  | –37.421 | 0.048      | 0.046      | –61    | 9.5      | 0.7      | 0.1             | 7.8      | 1.5             | 2.18          | 0.16                 | PL  | ... | ...    | 3EG J2243+1509       | ... | bcu   | J224604+154437     |



Table 1—Continued

| Name 3FGL    | R.A.    | Decl.   | $l$     | $b$     | $\theta_1$ | $\theta_2$ | $\phi$ | $\sigma$ | $F_{35}$ | $\Delta F_{35}$ | $S_{25}$ | $\Delta S_{25}$ | $\Gamma_{25}$ | $\Delta \Gamma_{25}$ | Mod | Var | Flags | $\gamma$ -ray Assoc.                                                                                                                    | TeV | Class | ID or Assoc.            |
|--------------|---------|---------|---------|---------|------------|------------|--------|----------|----------|-----------------|----------|-----------------|---------------|----------------------|-----|-----|-------|-----------------------------------------------------------------------------------------------------------------------------------------|-----|-------|-------------------------|
| J2246.7–5205 | 341.679 | –52.089 | 337.455 | –55.853 | 0.061      | 0.045      | 76     | 7.4      | 0.2      | 0.1             | 4.3      | 1.1             | 1.44          | 0.18                 | PL  | ... | 9     | 1FHL J2246.9–5205<br>2FGL J2246.8–5203                                                                                                  | ... | bcu   | RBS 1895                |
| J2247.2–0004 | 341.812 | –0.072  | 69.996  | –49.735 | 0.067      | 0.055      | 55     | 10.1     | 0.7      | 0.1             | 7.5      | 1.0             | 2.11          | 0.09                 | PL  | ... | ...   | 2FGL J2247.2–0002<br>1FGL J2247.3+0000                                                                                                  | ... | ...   | ...                     |
| J2247.8+4413 | 341.960 | 44.224  | 100.718 | –13.252 | 0.037      | 0.033      | 65     | 9.9      | 0.5      | 0.1             | 6.6      | 1.2             | 1.80          | 0.14                 | PL  | ... | ...   | 1FHL J2247.7+4412<br>2FGL J2247.8+4412                                                                                                  | ... | bll   | NVSS<br>J224753+441317  |
| J2248.6–3235 | 342.161 | –32.597 | 13.808  | –62.921 | 0.212      | 0.184      | 8      | 6.8      | 0.2      | 0.1             | 5.0      | 0.7             | 2.82          | 0.14                 | PL  | ... | ...   | ...                                                                                                                                     | ... | fsrq  | PKS 2245–328            |
| J2249.3–5943 | 342.348 | –59.723 | 327.097 | –51.295 | 0.111      | 0.092      | 5      | 4.1      | 0.2      | 0.1             | 2.1      | 0.6             | 2.17          | 0.22                 | PL  | ... | ...   | ...                                                                                                                                     | ... | ...   | ...                     |
| J2250.1+3825 | 342.527 | 38.419  | 98.261  | –18.572 | 0.030      | 0.027      | 85     | 16.5     | 1.1      | 0.1             | 12.7     | 1.3             | 1.91          | 0.07                 | PL  | ... | ...   | 1FHL J2250.1+3823<br>2FGL J2250.0+3825<br>1FGL J2250.1+3825                                                                             | P   | bll   | B3 2247+381             |
| J2250.3+1747 | 342.581 | 17.796  | 86.354  | –36.331 | 0.091      | 0.076      | –89    | 7.2      | 0.5      | 0.1             | 11.3     | 2.0             | 2.79          | 0.13                 | PL  | T   | ...   | 3EG J2248+1745<br>EGRc J2249+1724                                                                                                       | ... | ...   | ...                     |
| J2250.3–4206 | 342.584 | –42.103 | 353.782 | –61.161 | 0.050      | 0.044      | –48    | 11.6     | 0.6      | 0.1             | 6.6      | 0.9             | 2.03          | 0.09                 | PL  | ... | ...   | 2FGL J2250.2–4205                                                                                                                       | ... | bcu   | PMN J2250–4206          |
| J2250.6+3308 | 342.673 | 33.142  | 95.658  | –23.257 | 0.134      | 0.122      | –22    | 6.2      | 0.4      | 0.1             | 5.3      | 0.9             | 2.35          | 0.11                 | PL  | ... | ...   | ...                                                                                                                                     | ... | ...   | ...                     |
| J2250.7–2806 | 342.680 | –28.116 | 23.740  | –63.310 | 0.025      | 0.023      | 88     | 48.4     | 4.1      | 0.2             | 47.1     | 1.7             | 2.18          | 0.03                 | PL  | T   | ...   | 1FHL J2250.7–2811<br>2FGL J2250.8–2808<br>1FGL J2250.8–2809                                                                             | ... | bcu   | PMN J2250–2806          |
| J2251.5–4928 | 342.896 | –49.468 | 340.648 | –57.956 | 0.058      | 0.048      | 40     | 12.2     | 0.6      | 0.1             | 6.9      | 0.9             | 1.97          | 0.09                 | PL  | ... | ...   | 2FGL J2251.1–4927                                                                                                                       | ... | bcu   | SUMSS<br>J225128–492912 |
| J2251.9+4031 | 342.988 | 40.524  | 99.627  | –16.879 | 0.055      | 0.048      | 60     | 13.0     | 0.9      | 0.1             | 11.1     | 1.1             | 2.25          | 0.08                 | PL  | ... | ...   | 1FGL J2251.2–4928<br>2FGL J2251.9+4032<br>1FGL J2251.7+4030                                                                             | ... | bll   | MG4 J225201+4030        |
| J2253.1–1237 | 343.297 | –12.628 | 54.722  | –58.770 | 0.172      | 0.141      | –7     | 5.7      | 0.3      | 0.1             | 4.4      | 0.8             | 2.44          | 0.13                 | PL  | ... | ...   | ...                                                                                                                                     | ... | ...   | ...                     |
| J2254.0+1608 | 343.502 | 16.146  | 86.121  | –38.192 | 0.007      | 0.007      | –47    | 480.7    | 106.1    | 0.7             | 1234.3   | 5.4             | 2.35          | ...                  | EC  | T   | ...   | 1FHL J2253.9+1608<br>2FGL J2253.9+1609<br>1FGL J2253.9+1608<br>0FGL J2254.0+1609<br>3EG J2254+1601<br>EGR J2253+1606<br>1AGL J2254+1602 | ... | FSRQ  | 3C 454.3                |
| J2254.0+1403 | 343.506 | 14.062  | 84.618  | –39.918 | 0.106      | 0.092      | 54     | 5.4      | 0.4      | 0.1             | 4.8      | 1.3             | 2.24          | 0.21                 | PL  | ... | ...   | 2FGL J2254.1+1401                                                                                                                       | ... | bll   | NVSS<br>J225354+140439  |
| J2254.1+6229 | 343.547 | 62.497  | 109.852 | 2.641   | 0.186      | 0.095      | 81     | 9.0      | 1.0      | 0.2             | 17.3     | 1.9             | 2.63          | 0.08                 | PL  | ... | 3     | ...                                                                                                                                     | ... | ...   | ...                     |
| J2254.6+4253 | 343.657 | 42.888  | 101.211 | –15.003 | 0.412      | 0.246      | 6      | 6.3      | 0.4      | 0.1             | 6.8      | 1.1             | 2.66          | 0.12                 | PL  | ... | ...   | ...                                                                                                                                     | ... | ...   | ...                     |
| J2255.1+2411 | 343.779 | 24.187  | 91.595  | –31.513 | 0.054      | 0.049      | 86     | 12.6     | 0.9      | 0.1             | 9.6      | 1.1             | 2.02          | 0.09                 | PL  | T   | ...   | 2FGL J2255.2+2408                                                                                                                       | ... | bll   | MG3 J225517+2409        |
| J2256.7–1022 | 344.184 | –10.382 | 59.217  | –58.236 | 0.061      | 0.056      | –54    | 16.1     | 1.3      | 0.1             | 7.7      | 0.8             | 2.06          | ...                  | EC  | ... | ...   | 2FGL J2256.9–1023                                                                                                                       | ... | PSR   | PSR J2256–1024          |

Table 1—Continued

| Name 3FGL    | R.A.    | Decl.   | $l$     | $b$     | $\theta_1$ | $\theta_2$ | $\phi$ | $\sigma$ | $F_{35}$ | $\Delta F_{35}$ | $S_{25}$ | $\Delta S_{25}$ | $\Gamma_{25}$ | $\Delta \Gamma_{25}$ | Mod | Var | Flags | $\gamma$ -ray Assoc.                                        | TeV | Class | ID or Assoc.             |
|--------------|---------|---------|---------|---------|------------|------------|--------|----------|----------|-----------------|----------|-----------------|---------------|----------------------|-----|-----|-------|-------------------------------------------------------------|-----|-------|--------------------------|
| J2256.7–2011 | 344.189 | –20.188 | 41.565  | –62.906 | 0.046      | 0.043      | –76    | 15.5     | 0.9      | 0.1             | 10.5     | 1.0             | 2.09          | 0.07                 | PL  | ... | ...   | 1FGL J2256.9–1024<br>2FGL J2256.4–2009<br>1FGL J2256.3–2009 | ... | bll   | PKS 2254–204             |
| J2258.0–2759 | 344.512 | –27.985 | 24.355  | –64.910 | 0.029      | 0.028      | 64     | 56.8     | 4.3      | 0.2             | 48.7     | 1.5             | 2.37          | ...                  | LP  | T   | ...   | 2FGL J2258.0–2759<br>1FGL J2258.0–2757<br>EGR J2258–2745    | ... | fsrq  | PKS 2255–282             |
| J2258.1–8248 | 344.541 | –82.806 | 307.013 | –33.402 | 0.072      | 0.067      | –64    | 8.8      | 0.7      | 0.1             | 8.1      | 1.2             | 2.19          | 0.11                 | PL  | ... | ...   | 2FGL J2259.0–8254<br>1FGL J2259.9–8255                      | ... | bcu   | PMN J2258–8246           |
| J2258.2–3645 | 344.562 | –36.750 | 3.903   | –64.252 | 0.087      | 0.079      | –17    | 5.6      | 0.3      | 0.1             | 3.1      | 0.7             | 1.96          | 0.16                 | PL  | ... | ...   | 1FHL J2257.9–3644<br>2FGL J2257.9–3646<br>1FGL J2257.9–3643 | ... | ...   | ...                      |
| J2258.3–5526 | 344.599 | –55.439 | 330.935 | –55.106 | 0.105      | 0.099      | 23     | 5.5      | 0.3      | 0.1             | 3.2      | 0.7             | 2.31          | 0.17                 | PL  | ... | ...   | 2FGL J2258.8–5524<br>1FGL J2258.9–5525                      | ... | bll   | PMN J2258–5526           |
| J2258.8+2437 | 344.724 | 24.624  | 92.727  | –31.565 | 0.252      | 0.125      | 71     | 4.6      | 0.3      | 0.1             | 4.6      | 1.0             | 2.43          | 0.17                 | PL  | ... | 9     | ...                                                         | ... | ...   | ...                      |
| J2259.9–1553 | 344.996 | –15.897 | 50.688  | –61.838 | 0.145      | 0.130      | 2      | 5.8      | 0.3      | 0.1             | 3.8      | 0.8             | 2.11          | 0.14                 | PL  | ... | ...   | ...                                                         | ... | ...   | ...                      |
| J2300.0+4053 | 345.024 | 40.893  | 101.243 | –17.243 | 0.060      | 0.052      | 73     | 5.2      | 0.2      | 0.1             | 2.9      | 0.9             | 1.51          | 0.26                 | PL  | ... | ...   | ...                                                         | ... | ...   | ...                      |
| J2300.1–3547 | 345.043 | –35.788 | 5.881   | –64.847 | 0.150      | 0.117      | 56     | 6.0      | 0.3      | 0.1             | 3.8      | 0.7             | 2.18          | 0.14                 | PL  | ... | ...   | 2FGL J2300.0–3553                                           | ... | ...   | ...                      |
| J2300.3+3136 | 345.078 | 31.616  | 96.829  | –25.563 | 0.034      | 0.032      | 55     | 15.6     | 0.9      | 0.1             | 10.6     | 1.3             | 1.85          | 0.07                 | PL  | ... | ...   | 2FGL J2300.6+3139                                           | ... | bll   | NVSS<br>J230022+313703   |
| J2301.2+5853 | 345.313 | 58.898  | 109.109 | –0.985  | 0.055      | 0.049      | 14     | 6.1      | 0.4      | 0.1             | 6.5      | 1.5             | 1.51          | 0.12                 | PL  | ... | ...   | 1FGL J2300.4+3138<br>...                                    | ... | snr   | CTB 109                  |
| J2302.7+4443 | 345.685 | 44.722  | 103.395 | –13.987 | 0.022      | 0.021      | –13    | 51.7     | 6.5      | 0.2             | 38.1     | 1.4             | 1.96          | ...                  | EC  | ... | ...   | 2FGL J2302.7+4443<br>1FGL J2302.8+4443<br>0FGL J2302.9+4443 | ... | PSR   | PSR J2302+4442           |
| J2303.7+5555 | 345.944 | 55.917  | 108.203 | –3.845  | 0.057      | 0.051      | –8     | 5.6      | 0.3      | 0.1             | 4.0      | 1.0             | 1.75          | 0.15                 | PL  | ... | ...   | ...                                                         | ... | ...   | ...                      |
| J2304.6+3704 | 346.161 | 37.083  | 100.345 | –21.061 | 0.031      | 0.029      | 57     | 13.0     | 0.7      | 0.1             | 8.9      | 1.2             | 1.82          | 0.11                 | PL  | ... | ...   | 1FHL J2304.6+3704                                           | ... | bll   | 1RXS<br>J230437.1+370506 |
| J2305.3–4219 | 346.341 | –42.327 | 350.892 | –63.611 | 0.083      | 0.073      | –83    | 4.3      | 0.2      | 0.1             | 2.1      | 0.6             | 2.05          | 0.24                 | PL  | ... | ...   | 2FGL J2304.7+3703<br>1FGL J2304.3+3709<br>EGR J2308+3645    | ... | bcu   | SUMSS<br>J230512–421859  |
| J2305.8+1658 | 346.473 | 16.978  | 89.772  | –39.004 | 0.122      | 0.113      | 49     | 4.6      | 0.3      | 0.1             | 6.0      | 1.5             | 2.76          | 0.18                 | PL  | ... | ...   | ...                                                         | ... | ...   | ...                      |
| J2307.4–1208 | 346.854 | –12.136 | 59.414  | –61.386 | 0.095      | 0.081      | 73     | 5.0      | 0.2      | 0.1             | 3.0      | 0.9             | 1.77          | 0.19                 | PL  | ... | ...   | ...                                                         | ... | bll   | 1RXS<br>J230722.5–120520 |
| J2307.7+1449 | 346.940 | 14.822  | 88.834  | –41.085 | 0.057      | 0.051      | –55    | 13.4     | 1.1      | 0.1             | 12.8     | 1.3             | 2.24          | 0.08                 | PL  | ... | ...   | 1FGL J2307.3+1452<br>1FHL J2308.1+1459<br>2FGL J2308.0+1457 | ... | bll   | MG1 J230734+1449         |
| J2309.0+5428 | 347.252 | 54.476  | 108.320 | –5.464  | 0.083      | 0.070      | –16    | 4.6      | 0.2      | 0.1             | 2.9      | 0.9             | 1.70          | 0.25                 | PL  | ... | ...   | ...                                                         | ... | ...   | ...                      |

Table 1—Continued

| Name 3FGL    | R.A.    | Decl.   | $l$     | $b$     | $\theta_1$ | $\theta_2$ | $\phi$ | $\sigma$ | $F_{35}$ | $\Delta F_{35}$ | $S_{25}$ | $\Delta S_{25}$ | $\Gamma_{25}$ | $\Delta \Gamma_{25}$ | Mod | Var | Flags | $\gamma$ -ray Assoc. | TeV | Class | ID or Assoc.             |
|--------------|---------|---------|---------|---------|------------|------------|--------|----------|----------|-----------------|----------|-----------------|---------------|----------------------|-----|-----|-------|----------------------|-----|-------|--------------------------|
| J2309.6–3633 | 347.415 | –36.562 | 2.908   | –66.512 | 0.049      | 0.046      | –77    | 9.3      | 0.4      | 0.1             | 5.3      | 1.0             | 1.85          | 0.12                 | PL  | ... | ...   | 2FGL J2309.8–3627    | ... | bcu   | 1RXS<br>J230940.6–363241 |
|              |         |         |         |         |            |            |        |          |          |                 |          |                 |               |                      |     |     |       | 1FGL J2310.0–3627    |     |       |                          |
| J2310.1–0557 | 347.546 | –5.952  | 69.695  | –57.939 | 0.128      | 0.114      | –53    | 9.0      | 0.8      | 0.1             | 3.5      | 0.6             | 2.06          | ...                  | LP  | ... | ...   | ...                  | ... | ...   | ...                      |
| J2311.0+3425 | 347.764 | 34.423  | 100.411 | –24.021 | 0.023      | 0.022      | –15    | 66.9     | 5.3      | 0.2             | 59.6     | 1.6             | 2.34          | ...                  | LP  | T   | ...   | 1FHL J2311.0+3425    | ... | FSRQ  | B2 2308+34               |
|              |         |         |         |         |            |            |        |          |          |                 |          |                 |               |                      |     |     |       | 2FGL J2311.0+3425    |     |       |                          |
|              |         |         |         |         |            |            |        |          |          |                 |          |                 |               |                      |     |     |       | 1FGL J2311.0+3425    |     |       |                          |
| J2311.0+0204 | 347.765 | 2.081   | 79.328  | –52.083 | 0.049      | 0.049      | –4     | 8.8      | 0.5      | 0.1             | 5.9      | 0.9             | 2.27          | 0.11                 | PL  | T   | ...   | 2FGL J2310.9+0204    | ... | bll   | NVSS<br>J231101+020504   |
|              |         |         |         |         |            |            |        |          |          |                 |          |                 |               |                      |     |     |       | 1FGL J2310.9+0204    |     |       |                          |
| J2312.9–6923 | 348.240 | –69.393 | 314.977 | –45.363 | 0.078      | 0.070      | –34    | 4.9      | 0.2      | 0.1             | 2.3      | 0.7             | 1.80          | 0.21                 | PL  | ... | ...   | ...                  | ... | bcu   | SUMSS<br>J231347–692332  |
| J2313.1+3935 | 348.277 | 39.586  | 103.054 | –19.460 | 0.193      | 0.157      | 73     | 5.5      | 0.2      | 0.1             | 5.2      | 0.9             | 2.79          | 0.16                 | PL  | ... | 4     | ...                  | ... | ...   | ...                      |
| J2314.0+1443 | 348.518 | 14.731  | 90.531  | –41.934 | 0.049      | 0.044      | 62     | 11.7     | 0.6      | 0.1             | 8.0      | 1.3             | 1.76          | 0.11                 | PL  | ... | ...   | 1FHL J2314.0+1446    | ... | bll   | RGB J2313+147            |
|              |         |         |         |         |            |            |        |          |          |                 |          |                 |               |                      |     |     |       | 2FGL J2314.0+1446    |     |       |                          |
|              |         |         |         |         |            |            |        |          |          |                 |          |                 |               |                      |     |     |       | 1FGL J2314.1+1444    |     |       |                          |
| J2315.7–5018 | 348.942 | –50.312 | 334.664 | –60.511 | 0.092      | 0.070      | 2      | 10.1     | 0.6      | 0.1             | 6.7      | 0.9             | 2.19          | 0.10                 | PL  | ... | ...   | 2FGL J2315.7–5014    | ... | bll   | PKS 2312–505             |
|              |         |         |         |         |            |            |        |          |          |                 |          |                 |               |                      |     |     |       | 1FGL J2315.9–5014    |     |       |                          |
| J2316.8–5209 | 349.216 | –52.166 | 331.773 | –59.339 | 0.064      | 0.059      | –23    | 5.6      | 0.2      | 0.1             | 2.7      | 0.8             | 1.73          | 0.22                 | PL  | ... | ...   | ...                  | ... | bcu   | SUMSS<br>J231701–521003  |
| J2317.3–4534 | 349.345 | –45.570 | 342.100 | –63.755 | 0.061      | 0.049      | 79     | 14.8     | 0.8      | 0.1             | 9.1      | 0.9             | 2.19          | 0.08                 | PL  | ... | ...   | 2FGL J2317.3–4534    | ... | bcu   | 1RXS<br>J231733.0–453348 |
| J2318.6+1912 | 349.655 | 19.210  | 94.548  | –38.493 | 0.235      | 0.224      | 84     | 6.7      | 0.3      | 0.1             | 6.2      | 0.9             | 2.74          | 0.13                 | PL  | ... | ...   | ...                  | ... | bcu   | TXS 2315+189             |
| J2318.6–3829 | 349.666 | –38.497 | 356.688 | –67.531 | 0.153      | 0.125      | –59    | 6.0      | 0.3      | 0.1             | 3.9      | 0.7             | 2.38          | 0.15                 | PL  | ... | ...   | 2FGL J2319.3–3830    | ... | ...   | ...                      |
| J2319.2–4207 | 349.804 | –42.132 | 348.384 | –65.951 | 0.073      | 0.056      | –4     | 8.6      | 0.4      | 0.1             | 4.8      | 0.8             | 2.10          | 0.13                 | PL  | ... | ...   | 2FGL J2319.1–4208    | ... | bll   | PKS 2316–423             |
| J2321.2–6439 | 350.318 | –64.666 | 317.657 | –49.806 | 0.110      | 0.096      | 62     | 4.3      | 0.2      | 0.1             | 2.6      | 0.7             | 2.40          | 0.22                 | PL  | ... | ...   | ...                  | ... | bcu   | PMN J2321–6438           |
| J2321.3+5113 | 350.345 | 51.221  | 108.873 | –9.176  | 0.085      | 0.084      | –24    | 4.3      | 0.3      | 0.1             | 3.1      | 0.9             | 2.02          | 0.22                 | PL  | ... | ...   | ...                  | ... | ...   | ...                      |
| J2321.6–1619 | 350.405 | –16.331 | 55.743  | –66.570 | 0.059      | 0.051      | 85     | 4.9      | 0.1      | 0.1             | 2.2      | 0.8             | 1.53          | 0.21                 | PL  | ... | ...   | ...                  | ... | ...   | ...                      |
| J2321.6+4438 | 350.416 | 44.634  | 106.568 | –15.366 | 0.309      | 0.256      | –74    | 4.6      | 0.3      | 0.1             | 4.6      | 0.9             | 2.64          | 0.16                 | PL  | ... | 4     | ...                  | ... | fsrq  | B3 2319+444              |
| J2321.9+2732 | 350.479 | 27.540  | 99.670  | –31.256 | 0.097      | 0.081      | –13    | 11.8     | 0.8      | 0.1             | 9.5      | 1.0             | 2.28          | 0.08                 | PL  | ... | ...   | 2FGL J2321.0+2737    | ... | fsrq  | 4C +27.50                |
|              |         |         |         |         |            |            |        |          |          |                 |          |                 |               |                      |     |     |       | 1FGL J2321.6+2726    |     |       |                          |
| J2321.9+3204 | 350.479 | 32.070  | 101.686 | –27.082 | 0.045      | 0.041      | 21     | 26.4     | 2.1      | 0.1             | 19.3     | 1.2             | 2.25          | ...                  | LP  | T   | ...   | 2FGL J2322.2+3206    | ... | fsrq  | B2 2319+31               |
|              |         |         |         |         |            |            |        |          |          |                 |          |                 |               |                      |     |     |       | 1FGL J2322.0+3208    |     |       |                          |
| J2322.5+3436 | 350.627 | 34.603  | 102.871 | –24.781 | 0.041      | 0.037      | –54    | 8.9      | 0.3      | 0.1             | 5.1      | 1.2             | 1.44          | 0.20                 | PL  | ... | ...   | 1FHL J2322.5+3436    | ... | bll   | TXS 2320+343             |
|              |         |         |         |         |            |            |        |          |          |                 |          |                 |               |                      |     |     |       | 2FGL J2322.6+3435    |     |       |                          |
|              |         |         |         |         |            |            |        |          |          |                 |          |                 |               |                      |     |     |       | 1FGL J2322.6+3435    |     |       |                          |
| J2322.9–4917 | 350.734 | –49.289 | 334.544 | –62.053 | 0.064      | 0.053      | –50    | 10.0     | 0.5      | 0.1             | 6.2      | 1.0             | 1.96          | 0.12                 | PL  | ... | ...   | 2FGL J2323.0–4918    | ... | bcu   | SUMSS<br>J232254–491629  |
|              |         |         |         |         |            |            |        |          |          |                 |          |                 |               |                      |     |     |       | 1FGL J2323.0–4919    |     |       |                          |
| J2323.4+5849 | 350.870 | 58.819  | 111.747 | –2.129  | 0.017      | 0.016      | –42    | 36.7     | 5.5      | 0.3             | 48.3     | 2.8             | 1.79          | ...                  | LP  | ... | ...   | 1FHL J2323.3+5849    | P   | snr   | Cas A                    |
|              |         |         |         |         |            |            |        |          |          |                 |          |                 |               |                      |     |     |       | 2FGL J2323.4+5849    |     |       |                          |

Table 1—Continued

| Name 3FGL    | R.A.    | Decl.   | $l$     | $b$     | $\theta_1$ | $\theta_2$ | $\phi$ | $\sigma$ | $F_{35}$ | $\Delta F_{35}$ | $S_{25}$ | $\Delta S_{25}$ | $\Gamma_{25}$ | $\Delta \Gamma_{25}$ | Mod | Var | Flags | $\gamma$ -ray Assoc.                                                             | TeV | Class | ID or Assoc.           |
|--------------|---------|---------|---------|---------|------------|------------|--------|----------|----------|-----------------|----------|-----------------|---------------|----------------------|-----|-----|-------|----------------------------------------------------------------------------------|-----|-------|------------------------|
| J2323.5−0315 | 350.898 | −3.265  | 77.790  | −58.215 | 0.036      | 0.034      | 84     | 39.3     | 3.0      | 0.2             | 31.7     | 1.4             | 2.31          | ...                  | LP  | T   | ...   | 1FGL J2323.4+5849<br>2FGL J2323.6−0316<br>1FGL J2323.5−0315<br>3EG J2321−0328    | ... | fsrq  | PKS 2320−035           |
| J2323.7+2523 | 350.947 | 25.388  | 99.114  | −33.398 | 0.132      | 0.121      | −50    | 4.5      | 0.3      | 0.1             | 3.2      | 0.8             | 2.14          | 0.19                 | PL  | ... | ...   | ...                                                                              | ... | ...   | ...                    |
| J2323.9+4211 | 350.981 | 42.184  | 106.074 | −17.805 | 0.023      | 0.022      | −47    | 25.1     | 1.8      | 0.1             | 20.9     | 1.6             | 1.89          | 0.05                 | PL  | T   | ...   | 1FHL J2323.8+4210<br>2FGL J2323.8+4212<br>1FGL J2323.5+4211                      | ... | bll   | 1ES 2321+419           |
| J2324.7−4040 | 351.184 | −40.675 | 350.209 | −67.586 | 0.029      | 0.027      | −55    | 22.2     | 1.5      | 0.1             | 18.7     | 1.8             | 1.76          | 0.06                 | PL  | ... | ...   | 1FHL J2324.6−4041<br>2FGL J2324.7−4042                                           | ... | bll   | 1ES 2322−409           |
| J2324.7+0801 | 351.192 | 8.031   | 89.026  | −49.051 | 0.054      | 0.042      | 76     | 13.0     | 0.9      | 0.1             | 9.7      | 1.1             | 2.15          | 0.09                 | PL  | T   | ...   | 2FGL J2324.6+0801                                                                | ... | bll   | PMN J2324+0801         |
| J2325.2+3957 | 351.320 | 39.954  | 105.507 | −19.984 | 0.031      | 0.031      | 15     | 23.4     | 2.0      | 0.1             | 14.7     | 1.3             | 2.01          | ...                  | LP  | T   | ...   | 1FHL J2325.4+3959<br>2FGL J2325.3+3957<br>1FGL J2325.2+3957<br>0FGL J2325.3+3959 | ... | bll   | B3 2322+396            |
| J2325.3−3557 | 351.345 | −35.955 | 1.821   | −69.713 | 0.042      | 0.040      | −37    | 32.1     | 2.2      | 0.1             | 17.9     | 1.1             | 2.22          | ...                  | LP  | T   | ...   | 2FGL J2325.3−3557<br>1FGL J2325.5−3559                                           | ... | fsrq  | CTS 0496               |
| J2325.4−4758 | 351.358 | −47.975 | 335.983 | −63.262 | 0.049      | 0.040      | −26    | 17.9     | 1.2      | 0.1             | 14.4     | 1.2             | 2.31          | 0.07                 | PL  | T   | ...   | 1FHL J2325.5−4759<br>2FGL J2325.4−4758<br>1FGL J2325.6−4758                      | ... | bll   | PKS 2322−482           |
| J2325.6+1650 | 351.423 | 16.833  | 95.151  | −41.367 | 0.093      | 0.069      | −32    | 6.8      | 0.4      | 0.1             | 4.2      | 0.8             | 2.10          | 0.13                 | PL  | ... | ...   | 2FGL J2325.4+1650                                                                | ... | bll   | NVSS<br>J232538+164641 |
| J2327.2−4130 | 351.825 | −41.508 | 347.687 | −67.557 | 0.339      | 0.220      | 69     | 4.3      | 0.3      | 0.1             | 3.8      | 1.0             | 2.40          | 0.17                 | PL  | ... | ...   | ...                                                                              | ... | ...   | ...                    |
| J2327.7+0941 | 351.944 | 9.686   | 91.224  | −47.968 | 0.071      | 0.064      | 37     | 21.5     | 1.3      | 0.1             | 24.0     | 1.4             | 2.68          | 0.05                 | PL  | T   | ...   | 2FGL J2327.5+0940<br>1FGL J2327.7+0943<br>0FGL J2327.3+0947                      | ... | fsrq  | PKS 2325+093           |
| J2328.4−4034 | 352.113 | −40.580 | 349.458 | −68.239 | 0.037      | 0.035      | −56    | 23.9     | 2.0      | 0.1             | 24.2     | 1.4             | 2.31          | 0.04                 | PL  | T   | ...   | 2FGL J2327.9−4037<br>...                                                         | ... | bcu   | PKS 2325−408           |
| J2329.2+3754 | 352.318 | 37.914  | 105.540 | −22.167 | 0.034      | 0.032      | 49     | 13.2     | 0.8      | 0.1             | 9.6      | 1.2             | 1.93          | 0.09                 | PL  | ... | ...   | 1FHL J2329.1+3754<br>2FGL J2329.2+3755<br>1FGL J2329.2+3755                      | ... | bll   | NVSS<br>J232914+375414 |
| J2329.3−4955 | 352.331 | −49.923 | 332.005 | −62.314 | 0.014      | 0.014      | −32    | 130.0    | 14.1     | 0.3             | 147.7    | 2.3             | 2.27          | ...                  | LP  | T   | ...   | 1FHL J2329.2−4957<br>2FGL J2329.2−4956<br>1FGL J2329.2−4954                      | ... | fsrq  | PKS 2326−502           |
| J2329.8+6102 | 352.457 | 61.040  | 113.214 | −0.282  | 0.065      | 0.057      | −60    | 5.6      | 0.6      | 0.1             | 6.5      | 1.4             | 2.06          | 0.17                 | PL  | ... | ...   | ...                                                                              | ... | ...   | ...                    |
| J2329.9−4734 | 352.479 | −47.571 | 335.452 | −64.084 | 0.096      | 0.079      | −73    | 6.5      | 0.4      | 0.1             | 4.3      | 0.9             | 2.23          | 0.16                 | PL  | ... | ...   | 2FGL J2329.7−4744                                                                | ... | fsrq  | PKS 2326−477           |

Table 1—Continued

| Name 3FGL    | R.A.    | Decl.   | $l$     | $b$     | $\theta_1$ | $\theta_2$ | $\phi$ | $\sigma$ | $F_{35}$ | $\Delta F_{35}$ | $S_{25}$ | $\Delta S_{25}$ | $\Gamma_{25}$ | $\Delta \Gamma_{25}$ | Mod | Var | Flags | $\gamma$ -ray Assoc. | TeV | Class | ID or Assoc.     |
|--------------|---------|---------|---------|---------|------------|------------|--------|----------|----------|-----------------|----------|-----------------|---------------|----------------------|-----|-----|-------|----------------------|-----|-------|------------------|
| J2330.4–3726 | 352.608 | –37.449 | 356.677 | –70.075 | 0.112      | 0.089      | 10     | 5.9      | 0.3      | 0.1             | 3.7      | 0.7             | 2.32          | 0.15                 | PL  | ... | ...   | 2FGL J2330.6–3723    | ... | bll   | PKS 2327–376     |
| J2330.5+1104 | 352.637 | 11.077  | 93.074  | –47.051 | 0.128      | 0.116      | –90    | 7.5      | 0.5      | 0.1             | 7.3      | 1.1             | 2.56          | 0.11                 | PL  | ... | ...   | 2FGL J2330.2+1107    | ... | fsrq  | 4C +10.73        |
| J2330.8–2144 | 352.709 | –21.746 | 44.910  | –70.908 | 0.056      | 0.047      | –28    | 26.4     | 1.5      | 0.1             | 17.6     | 1.1             | 2.41          | ...                  | LP  | T   | ...   | 2FGL J2330.9–2144    | ... | fsrq  | PMN J2331–2148   |
|              |         |         |         |         |            |            |        |          |          |                 |          |                 |               |                      |     |     |       | 1FGL J2331.0–2145    |     |       |                  |
| J2331.9–1609 | 352.992 | –16.157 | 59.643  | –68.567 | 0.149      | 0.116      | –17    | 6.3      | 0.4      | 0.1             | 4.1      | 0.8             | 2.17          | 0.13                 | PL  | ... | ...   | 2FGL J2331.8–1607    | ... | ...   | ...              |
| J2333.0–5525 | 353.264 | –55.426 | 324.196 | –58.347 | 0.083      | 0.075      | –23    | 10.7     | 0.5      | 0.1             | 6.1      | 0.7             | 2.22          | 0.09                 | PL  | ... | ...   | 1FGL J2333.0–5535    | ... | ...   | ...              |
| J2334.1+0732 | 353.543 | 7.541   | 91.823  | –50.604 | 0.101      | 0.078      | 7      | 11.3     | 0.7      | 0.1             | 10.2     | 1.0             | 2.50          | 0.08                 | PL  | T   | ...   | 2FGL J2334.3+0734    | ... | fsrq  | TXS 2331+073     |
|              |         |         |         |         |            |            |        |          |          |                 |          |                 |               |                      |     |     |       | 1FGL J2334.3+0735    |     |       |                  |
| J2334.4–7948 | 353.608 | –79.804 | 307.106 | –36.692 | 0.183      | 0.154      | 84     | 4.1      | 0.2      | 0.1             | 3.7      | 0.9             | 2.62          | 0.19                 | PL  | ... | 4     | ...                  | ... | ...   | ...              |
| J2334.8+1432 | 353.724 | 14.540  | 96.576  | –44.380 | 0.034      | 0.031      | 52     | 19.6     | 1.3      | 0.1             | 15.2     | 1.5             | 1.88          | 0.06                 | PL  | T   | ...   | 1FHL J2334.7+1433    | ... | bll   | NVSS             |
|              |         |         |         |         |            |            |        |          |          |                 |          |                 |               |                      |     |     |       |                      |     |       | J233453+143214   |
|              |         |         |         |         |            |            |        |          |          |                 |          |                 |               |                      |     |     |       | 2FGL J2334.8+1431    |     |       |                  |
|              |         |         |         |         |            |            |        |          |          |                 |          |                 |               |                      |     |     |       | 1FGL J2334.7+1429    |     |       |                  |
| J2335.1–0133 | 353.786 | –1.552  | 84.160  | –58.558 | 0.293      | 0.155      | 19     | 5.9      | 0.4      | 0.1             | 5.6      | 1.0             | 2.46          | 0.14                 | PL  | ... | ...   | ...                  | ... | fsrq  | PKS 2332–017     |
| J2335.6–2342 | 353.901 | –23.713 | 40.008  | –72.558 | 0.176      | 0.134      | 49     | 6.7      | 0.3      | 0.1             | 5.0      | 0.8             | 2.65          | 0.14                 | PL  | ... | ...   | ...                  | ... | ...   | ...              |
| J2336.5+2356 | 354.132 | 23.937  | 101.713 | –35.830 | 0.096      | 0.078      | 37     | 5.9      | 0.3      | 0.1             | 3.7      | 0.8             | 2.13          | 0.18                 | PL  | ... | ...   | ...                  | ... | bcu   | B2 2334+23       |
| J2336.5–7620 | 354.133 | –76.334 | 308.611 | –39.957 | 0.098      | 0.082      | 26     | 8.1      | 0.5      | 0.1             | 5.9      | 0.8             | 2.33          | 0.11                 | PL  | ... | ...   | ...                  | ... | bcu   | PMN J2336–7620   |
| J2336.5–4116 | 354.134 | –41.271 | 345.523 | –69.113 | 0.065      | 0.057      | –89    | 16.5     | 1.0      | 0.1             | 11.3     | 1.0             | 2.24          | 0.07                 | PL  | T   | ...   | 2FGL J2336.3–4111    | ... | fsrq  | PKS 2333–415     |
| J2337.2–8425 | 354.314 | –84.422 | 305.031 | –32.401 | 0.086      | 0.071      | –9     | 4.7      | 0.3      | 0.1             | 3.2      | 1.0             | 2.14          | 0.23                 | PL  | ... | ...   | ...                  | ... | ...   | ...              |
| J2337.5+4108 | 354.394 | 41.139  | 108.263 | –19.620 | 0.141      | 0.110      | 85     | 4.4      | 0.3      | 0.1             | 3.4      | 0.8             | 2.23          | 0.16                 | PL  | ... | ...   | ...                  | ... | ...   | ...              |
| J2338.1–0229 | 354.544 | –2.499  | 84.360  | –59.767 | 0.067      | 0.055      | 3      | 19.0     | 1.3      | 0.1             | 18.6     | 1.2             | 2.50          | 0.06                 | PL  | T   | ...   | 2FGL J2338.1–0229    | ... | fsrq  | PKS 2335–027     |
|              |         |         |         |         |            |            |        |          |          |                 |          |                 |               |                      |     |     |       | 1FGL J2338.3–0231    |     |       |                  |
| J2338.7–7401 | 354.690 | –74.020 | 309.582 | –42.157 | 0.063      | 0.056      | –4     | 10.3     | 0.5      | 0.1             | 6.3      | 1.0             | 1.89          | 0.11                 | PL  | T   | ...   | ...                  | ... | bcu   | 1RXS             |
|              |         |         |         |         |            |            |        |          |          |                 |          |                 |               |                      |     |     |       |                      |     |       | J233919.8–740439 |
| J2338.7+0251 | 354.694 | 2.857   | 89.801  | –55.271 | 0.197      | 0.160      | –37    | 4.8      | 0.3      | 0.1             | 4.3      | 0.9             | 2.58          | 0.15                 | PL  | ... | ...   | ...                  | ... | ...   | ...              |
| J2339.0+2122 | 354.754 | 21.383  | 101.257 | –38.421 | 0.067      | 0.054      | 49     | 8.4      | 0.5      | 0.1             | 5.7      | 0.9             | 2.18          | 0.12                 | PL  | ... | ...   | 2FGL J2339.0+2125    | ... | bll   | RX J2338.8+2124  |
|              |         |         |         |         |            |            |        |          |          |                 |          |                 |               |                      |     |     |       | 1FGL J2339.0+2123    |     |       |                  |
| J2339.6–0533 | 354.902 | –5.552  | 81.333  | –62.471 | 0.026      | 0.025      | 44     | 45.7     | 4.5      | 0.2             | 30.1     | 1.4             | 1.99          | ...                  | EC  | ... | ...   | 1FHL J2339.8–0530    | ... | PSR   | PSR J2339–0533   |
|              |         |         |         |         |            |            |        |          |          |                 |          |                 |               |                      |     |     |       | 2FGL J2339.6–0532    |     |       |                  |
|              |         |         |         |         |            |            |        |          |          |                 |          |                 |               |                      |     |     |       | 1FGL J2339.7–0531    |     |       |                  |
|              |         |         |         |         |            |            |        |          |          |                 |          |                 |               |                      |     |     |       | 0FGL J2339.8–0530    |     |       |                  |
| J2340.7+3847 | 355.188 | 38.797  | 108.145 | –22.037 | 0.168      | 0.106      | –32    | 4.2      | 0.3      | 0.1             | 2.9      | 0.8             | 1.92          | 0.27                 | PL  | ... | ...   | ...                  | ... | ...   | ...              |
| J2340.7+8016 | 355.199 | 80.271  | 119.845 | 17.825  | 0.023      | 0.022      | –69    | 32.1     | 2.4      | 0.1             | 28.1     | 1.6             | 1.92          | 0.04                 | PL  | ... | ...   | 1FHL J2341.3+8016    | ... | bll   | 1RXS             |
|              |         |         |         |         |            |            |        |          |          |                 |          |                 |               |                      |     |     |       |                      |     |       | J234051.4+801513 |
|              |         |         |         |         |            |            |        |          |          |                 |          |                 |               |                      |     |     |       | 2FGL J2341.7+8016    |     |       |                  |
|              |         |         |         |         |            |            |        |          |          |                 |          |                 |               |                      |     |     |       | 1FGL J2341.6+8015    |     |       |                  |
| J2343.0–4748 | 355.763 | –47.802 | 331.241 | –65.394 | 0.131      | 0.111      | –16    | 9.3      | 0.5      | 0.1             | 5.8      | 0.8             | 2.16          | 0.10                 | PL  | ... | 7     | 2FGL J2343.3–4752    | ... | ...   | ...              |
| J2343.6+1551 | 355.912 | 15.861  | 100.002 | –43.972 | 0.494      | 0.299      | –89    | 4.5      | 0.2      | 0.1             | 4.0      | 0.8             | 2.66          | 0.15                 | PL  | ... | ...   | ...                  | ... | fsrq  | MG1 J234342+1542 |

Table 1—Continued

| Name 3FGL    | R.A.    | Decl.   | $l$     | $b$     | $\theta_1$ | $\theta_2$ | $\phi$ | $\sigma$ | $F_{35}$ | $\Delta F_{35}$ | $S_{25}$ | $\Delta S_{25}$ | $\Gamma_{25}$ | $\Delta \Gamma_{25}$ | Mod | Var | Flags | $\gamma$ -ray Assoc. | TeV | Class | ID or Assoc.             |
|--------------|---------|---------|---------|---------|------------|------------|--------|----------|----------|-----------------|----------|-----------------|---------------|----------------------|-----|-----|-------|----------------------|-----|-------|--------------------------|
| J2343.7+3437 | 355.940 | 34.631  | 107.454 | -26.199 | 0.071      | 0.053      | -72    | 6.8      | 0.3      | 0.1             | 3.8      | 0.9             | 1.75          | 0.16                 | PL  | ... | ...   | 2FGL J2343.6+3437    | ... | bll   | 1RXS<br>J234332.5+343957 |
|              |         |         |         |         |            |            |        |          |          |                 |          |                 |               |                      |     |     |       | 1FGL J2343.6+3437    |     |       |                          |
| J2344.4+0549 | 356.103 | 5.831   | 94.274  | -53.270 | 0.194      | 0.119      | -88    | 4.7      | 0.4      | 0.1             | 4.2      | 0.9             | 2.19          | 0.15                 | PL  | ... | ...   | ...                  | ... | bcu   | 1RXS<br>J234354.4+054713 |
| J2344.9-5647 | 356.225 | -56.790 | 320.170 | -58.056 | 0.154      | 0.115      | 27     | 6.8      | 0.2      | 0.1             | 4.6      | 0.7             | 2.70          | 0.13                 | PL  | ... | 9     | ...                  | ... | ...   | ...                      |
| J2345.2-1554 | 356.307 | -15.913 | 65.697  | -70.986 | 0.015      | 0.015      | -64    | 82.3     | 11.4     | 0.3             | 100.5    | 2.9             | 2.09          | ...                  | LP  | T   | ...   | 1FHL J2345.0-1556    | ... | FSRQ  | PMN J2345-1555           |
|              |         |         |         |         |            |            |        |          |          |                 |          |                 |               |                      |     |     |       | 2FGL J2345.0-1553    |     |       |                          |
|              |         |         |         |         |            |            |        |          |          |                 |          |                 |               |                      |     |     |       | 0FGL J2345.5-1559    |     |       |                          |
| J2346.7+0705 | 356.678 | 7.086   | 96.001  | -52.368 | 0.045      | 0.043      | 63     | 13.8     | 0.9      | 0.1             | 11.8     | 1.5             | 1.78          | 0.09                 | PL  | ... | ...   | 1FHL J2347.2+0707    | ... | bcu   | TXS 2344+068             |
| J2347.0+5142 | 356.764 | 51.708  | 112.889 | -9.904  | 0.018      | 0.017      | 7      | 32.0     | 2.4      | 0.1             | 30.4     | 2.0             | 1.78          | 0.04                 | PL  | T   | ...   | 1FHL J2347.0+5142    | P   | bll   | 1ES 2344+514             |
|              |         |         |         |         |            |            |        |          |          |                 |          |                 |               |                      |     |     |       | 2FGL J2347.0+5142    |     |       |                          |
|              |         |         |         |         |            |            |        |          |          |                 |          |                 |               |                      |     |     |       | 1FGL J2347.1+5142    |     |       |                          |
| J2347.9+5436 | 356.983 | 54.605  | 113.744 | -7.129  | 0.069      | 0.063      | 18     | 4.7      | 0.2      | 0.1             | 3.0      | 0.9             | 1.73          | 0.22                 | PL  | ... | ...   | ...                  | ... | bcu   | NVSS<br>J234753+543627   |
| J2348.0-1630 | 357.009 | -16.502 | 65.580  | -71.880 | 0.032      | 0.031      | -0     | 26.0     | 2.6      | 0.2             | 29.4     | 1.7             | 2.20          | 0.05                 | PL  | T   | ...   | 2FGL J2347.9-1629    | ... | fsrq  | PKS 2347-16              |
|              |         |         |         |         |            |            |        |          |          |                 |          |                 |               |                      |     |     |       | 1FGL J2348.0-1629    |     |       |                          |
| J2348.4-5100 | 357.100 | -51.008 | 325.284 | -63.297 | 0.230      | 0.183      | 85     | 5.9      | 0.3      | 0.1             | 4.0      | 0.7             | 2.31          | 0.14                 | PL  | ... | ...   | ...                  | ... | bcu   | SUMSS<br>J234852-510311  |
| J2350.4-3004 | 357.606 | -30.072 | 16.940  | -76.300 | 0.064      | 0.056      | -60    | 9.1      | 0.5      | 0.1             | 5.7      | 0.9             | 2.08          | 0.13                 | PL  | ... | ...   | 2FGL J2350.2-3002    | ... | bll   | NVSS<br>J235034-300603   |
|              |         |         |         |         |            |            |        |          |          |                 |          |                 |               |                      |     |     |       | 1FGL J2350.1-3005    |     |       |                          |
| J2351.9-7601 | 357.982 | -76.030 | 307.612 | -40.553 | 0.098      | 0.077      | -70    | 6.1      | 0.3      | 0.1             | 3.8      | 1.0             | 1.69          | 0.16                 | PL  | ... | ...   | 2FGL J2351.6-7558    | ... | ...   | ...                      |
| J2352.0+1752 | 358.015 | 17.881  | 103.542 | -42.744 | 0.068      | 0.058      | -1     | 8.9      | 0.5      | 0.1             | 5.6      | 0.9             | 2.01          | 0.12                 | PL  | ... | ...   | 2FGL J2352.0+1753    | ... | bll   | CLASS J2352+1749         |
|              |         |         |         |         |            |            |        |          |          |                 |          |                 |               |                      |     |     |       | 1FGL J2352.1+1752    |     |       |                          |
| J2353.3-4805 | 358.332 | -48.084 | 327.451 | -66.184 | 0.155      | 0.138      | 8      | 4.5      | 0.2      | 0.1             | 2.6      | 0.7             | 2.01          | 0.17                 | PL  | ... | ...   | ...                  | ... | bcu   | SUMSS<br>J235310-480558  |
| J2353.3+6639 | 358.337 | 66.659  | 117.213 | 4.435   | 0.340      | 0.104      | 5      | 9.1      | 1.0      | 0.2             | 11.8     | 1.4             | 2.45          | ...                  | LP  | ... | 9,12  | 2FGL J2353.3+6643c   | ... | ...   | ...                      |
| J2353.6-3037 | 358.405 | -30.620 | 14.083  | -76.881 | 0.078      | 0.067      | -79    | 8.0      | 0.4      | 0.1             | 5.3      | 0.9             | 2.28          | 0.13                 | PL  | ... | ...   | 2FGL J2353.5-3034    | ... | bll   | PKS 2351-309             |
| J2353.7-3911 | 358.440 | -39.191 | 344.176 | -72.978 | 0.243      | 0.156      | 19     | 4.6      | 0.2      | 0.1             | 2.8      | 0.6             | 2.28          | 0.19                 | PL  | ... | ...   | ...                  | ... | bcu   | NVSS<br>J235342-391442   |
| J2354.0+2722 | 358.502 | 27.373  | 107.569 | -33.780 | 0.106      | 0.104      | -36    | 4.2      | 0.2      | 0.1             | 2.6      | 0.7             | 2.15          | 0.21                 | PL  | ... | ...   | ...                  | ... | ...   | ...                      |
| J2354.1+4605 | 358.539 | 46.091  | 112.672 | -15.636 | 0.185      | 0.162      | -24    | 6.3      | 0.4      | 0.1             | 5.3      | 0.8             | 2.48          | 0.12                 | PL  | ... | ...   | ...                  | ... | fsrq  | 4C +45.51                |
| J2354.4-6612 | 358.602 | -66.203 | 311.813 | -49.931 | 0.133      | 0.110      | 47     | 6.4      | 0.3      | 0.1             | 4.0      | 0.7             | 2.31          | 0.13                 | PL  | ... | ...   | 2FGL J2354.2-6615    | ... | ...   | ...                      |
|              |         |         |         |         |            |            |        |          |          |                 |          |                 |               |                      |     |     |       | 1FGL J2355.9-6613    |     |       |                          |
| J2354.8-5245 | 358.702 | -52.763 | 321.483 | -62.278 | 0.155      | 0.113      | -15    | 5.5      | 0.4      | 0.1             | 4.8      | 1.0             | 2.41          | 0.13                 | PL  | ... | 5     | 1FGL J2356.0-5253    | ... | ...   | ...                      |
| J2355.4+6939 | 358.864 | 69.650  | 118.068 | 7.309   | 0.297      | 0.193      | -27    | 4.3      | 0.4      | 0.1             | 6.9      | 1.6             | 2.54          | 0.14                 | PL  | ... | 4     | ...                  | ... | ...   | ...                      |
| J2355.5+8154 | 358.890 | 81.900  | 120.868 | 19.253  | 0.275      | 0.189      | 7      | 5.8      | 0.2      | 0.1             | 5.4      | 0.9             | 2.87          | 0.19                 | PL  | ... | 1     | ...                  | ... | fsrq  | S5 2353+81               |
| J2356.0+4037 | 359.021 | 40.632  | 111.719 | -21.031 | 0.058      | 0.052      | -21    | 9.1      | 0.4      | 0.1             | 5.8      | 1.1             | 1.72          | 0.14                 | PL  | ... | ...   | 2FGL J2356.1+4034    | ... | bll   | NVSS<br>J235612+403648   |
|              |         |         |         |         |            |            |        |          |          |                 |          |                 |               |                      |     |     |       | 1FGL J2356.1+4037    |     |       |                          |
| J2356.9+6812 | 359.239 | 68.215  | 117.892 | 5.878   | 0.164      | 0.116      | -26    | 5.9      | 0.8      | 0.1             | 13.1     | 2.3             | 2.63          | 0.10                 | PL  | ... | ...   | ...                  | ... | ...   | ...                      |
| J2357.3-0150 | 359.350 | -1.844  | 93.540  | -61.593 | 0.086      | 0.079      | 87     | 5.5      | 0.3      | 0.1             | 3.4      | 0.8             | 2.12          | 0.16                 | PL  | ... | ...   | ...                  | ... | bll   | PKS 2354-021             |

Table 1—Continued

| Name 3FGL    | R.A.    | Decl.   | $l$     | $b$     | $\theta_1$ | $\theta_2$ | $\phi$ | $\sigma$ | $F_{35}$ | $\Delta F_{35}$ | $S_{25}$ | $\Delta S_{25}$ | $\Gamma_{25}$ | $\Delta \Gamma_{25}$ | Mod | Var | Flags | $\gamma$ -ray Assoc.                                        | TeV | Class | ID or Assoc.   |
|--------------|---------|---------|---------|---------|------------|------------|--------|----------|----------|-----------------|----------|-----------------|---------------|----------------------|-----|-----|-------|-------------------------------------------------------------|-----|-------|----------------|
| J2357.4–1716 | 359.360 | –17.270 | 68.464  | –74.103 | 0.068      | 0.052      | –20    | 8.6      | 0.4      | 0.1             | 5.0      | 1.0             | 1.80          | 0.13                 | PL  | ... | ...   | ...                                                         | ... | bll   | RBS 2066       |
| J2357.8–5310 | 359.451 | –53.178 | 320.217 | –62.113 | 0.078      | 0.069      | –54    | 12.3     | 0.8      | 0.1             | 11.8     | 1.2             | 2.46          | 0.07                 | PL  | T   | ...   | ...                                                         | ... | fsrq  | PKS 2355–534   |
| J2358.0–4552 | 359.506 | –45.873 | 328.916 | –68.467 | 0.174      | 0.125      | –27    | 7.6      | 0.3      | 0.1             | 4.9      | 0.7             | 2.62          | 0.13                 | PL  | ... | ...   | ...                                                         | ... | fsrq  | PKS 2355–461   |
| J2358.2–1022 | 359.550 | –10.370 | 83.595  | –69.070 | 0.253      | 0.213      | 59     | 6.4      | 0.2      | 0.1             | 5.1      | 0.8             | 2.80          | 0.13                 | PL  | ... | ...   | ...                                                         | ... | fsrq  | PKS 2355–106   |
| J2358.3–2853 | 359.598 | –28.891 | 21.283  | –78.167 | 0.124      | 0.109      | –39    | 6.2      | 0.3      | 0.1             | 3.9      | 0.7             | 2.41          | 0.16                 | PL  | ... | ...   | ...                                                         | ... | bcl   | PMN J2358–2853 |
| J2358.5+3827 | 359.634 | 38.454  | 111.687 | –23.260 | 0.101      | 0.075      | 80     | 5.9      | 0.4      | 0.1             | 4.2      | 0.9             | 2.08          | 0.16                 | PL  | ... | ...   | ...                                                         | ... | ...   | ...            |
| J2358.6–1809 | 359.666 | –18.159 | 66.604  | –74.895 | 0.072      | 0.064      | 20     | 6.5      | 0.3      | 0.1             | 3.7      | 0.9             | 1.82          | 0.16                 | PL  | ... | ...   | 2FGL J2358.4–1811<br>1FGL J2358.5–1809                      | ... | ...   | ...            |
| J2358.9+3926 | 359.736 | 39.448  | 112.008 | –22.308 | 0.175      | 0.142      | 10     | 4.7      | 0.3      | 0.1             | 3.9      | 0.9             | 2.21          | 0.18                 | PL  | ... | ...   | ...                                                         | ... | fsrq  | B2 2356+39     |
| J2359.3–3038 | 359.829 | –30.646 | 12.707  | –78.070 | 0.054      | 0.051      | –7     | 11.1     | 0.6      | 0.1             | 6.6      | 0.9             | 2.02          | 0.12                 | PL  | ... | ...   | 1FHL J2359.2–3037<br>2FGL J2359.0–3037<br>1FGL J2359.0–3035 | P   | bll   | H 2356–309     |
| J2359.5–2052 | 359.881 | –20.883 | 57.947  | –76.612 | 0.086      | 0.073      | –22    | 6.9      | 0.3      | 0.1             | 3.8      | 0.7             | 2.02          | 0.16                 | PL  | ... | ...   | ...                                                         | ... | bll   | TXS 2356–210   |

References. —

Note. — The definitions of the columns are provided in Table 4.

<sup>a</sup>Within the indicated extended source on the sky
